# Supplementary material for: Fermi Large Area Telescope Second Source Catalog
Source: arXiv:1108.1435 ancillary file (2012-02-23)
Supplement: Supplementary file 1 [file table4_full.pdf]

Table 1. LAT 2-year Catalog

| Name 2FGL     | R.A.  | Decl.   | $l$     | $b$     | $\theta_1$ | $\theta_2$ | $\phi$ | $\sigma$ | $F_{35}$ | $\Delta F_{35}$ | $S_{25}$ | $\Delta S_{25}$ | $\Gamma_{25}$ | $\Delta \Gamma_{25}$ | Mod | Var | Flags  | $\gamma$ -ray Assoc. | TeV | Class | ID or Assoc.                                                                                |
|---------------|-------|---------|---------|---------|------------|------------|--------|----------|----------|-----------------|----------|-----------------|---------------|----------------------|-----|-----|--------|----------------------|-----|-------|---------------------------------------------------------------------------------------------|
| J0000.9–0748  | 0.234 | −7.815  | 88.829  | −67.281 | 0.195      | 0.167      | 48     | 5.9      | 0.5      | 0.1             | 6.8      | 1.2             | 2.39          | 0.14                 | PL  | ... | ...    | 1FGL J0000.9–0745    | ... | bzb   | PMN J0001–0746                                                                              |
| J0001.7–4159  | 0.439 | −41.996 | 334.076 | −71.997 | 0.122      | 0.115      | 62     | 5.9      | 0.5      | 0.1             | 5.3      | 1.1             | 2.14          | 0.19                 | PL  | T   | ...    | 1FGL J0001.9–4158    | ... | agu   | 1RXS J000135.5–41551                                                                        |
| J0002.7+6220  | 0.680 | 62.340  | 117.312 | 0.001   | 0.093      | 0.089      | 9      | 13.7     | 2.9      | 0.3             | 25.2     | 2.5             | 2.34          | ...                  | LP  | ... | ...    | 1FGL J0003.1+6227    | ... | ...   | ...                                                                                         |
| J0004.2+2208  | 1.056 | 22.137  | 108.732 | −39.430 | 0.194      | 0.137      | 63     | 5.4      | 0.4      | 0.1             | 6.3      | 1.2             | 2.49          | 0.15                 | PL  | ... | ...    | 1FGL J0004.3+2207    | ... | ...   | ...                                                                                         |
| J0004.7–4736  | 1.180 | −47.612 | 323.890 | −67.571 | 0.112      | 0.096      | 14     | 12.6     | 0.9      | 0.1             | 13.1     | 1.3             | 2.45          | 0.09                 | PL  | T   | ...    | 1FGL J0004.7–4737    | ... | bzq   | PKS 0002–478                                                                                |
| J0006.1+3821  | 1.525 | 38.350  | 113.245 | −23.667 | 0.144      | 0.123      | 71     | 12.2     | 1.0      | 0.1             | 16.1     | 1.5             | 2.60          | 0.08                 | PL  | ... | ...    | 1FGL J0005.7+3815    | ... | bzq   | S4 0003+38                                                                                  |
| J0007.0+7303  | 1.774 | 73.055  | 119.665 | 10.465  | 0.010      | 0.010      | −33    | 189.5    | 65.7     | 0.9             | 429.6    | 5.5             | 1.89          | ...                  | EC  | ... | ...    | 1FGL J0007.0+7303    | ... | PSR   | LAT PSR J0007+7303                                                                          |
|               |       |         |         |         |            |            |        |          |          |                 |          |                 |               |                      |     |     |        | 0FGL J0007.4+7303    |     |       |                                                                                             |
|               |       |         |         |         |            |            |        |          |          |                 |          |                 |               |                      |     |     |        | EGR J0008+7308       |     |       |                                                                                             |
|               |       |         |         |         |            |            |        |          |          |                 |          |                 |               |                      |     |     |        | 1AGL J0006+7311      |     |       |                                                                                             |
| J0007.7+6825c | 1.925 | 68.423  | 118.911 | 5.894   | 0.173      | 0.170      | 64     | 6.2      | 1.0      | 0.2             | 17.5     | 2.7             | 2.61          | 0.10                 | PL  | ... | 6,10   | 1FGL J0005.1+6829    | ... | ...   | ...                                                                                         |
| J0007.8+4713  | 1.974 | 47.230  | 115.304 | −14.996 | 0.062      | 0.053      | 29     | 17.6     | 2.1      | 0.2             | 23.7     | 2.1             | 2.10          | 0.06                 | PL  | ... | ...    | ...                  | ... | bzb   | MG4 J000800+4712                                                                            |
| J0008.7–2344  | 2.196 | −23.736 | 49.986  | −79.795 | 0.189      | 0.161      | −9     | 4.1      | 0.3      | 0.1             | 4.7      | 1.8             | 1.62          | 0.25                 | PL  | ... | ...    | ...                  | ... | bzb   | RBS 0016                                                                                    |
| J0009.0+0632  | 2.262 | 6.542   | 104.453 | −54.801 | 0.129      | 0.123      | −10    | 5.7      | 0.5      | 0.1             | 6.7      | 1.3             | 2.40          | 0.16                 | PL  | ... | ...    | 1FGL J0008.9+0635    | ... | bzb   | CRATES J000903.95+062821.5                                                                  |
| J0009.1+5030  | 2.291 | 50.506  | 116.089 | −11.803 | 0.054      | 0.046      | 53     | 17.1     | 2.1      | 0.2             | 25.5     | 2.8             | 1.85          | 0.06                 | PL  | T   | ...    | 1FGL J0009.1+5031    | ... | agu   | NVSS J000922+503028                                                                         |
| J0009.9–3206  | 2.484 | −32.112 | 1.511   | −79.703 | 0.159      | 0.136      | −75    | 5.1      | 0.4      | 0.1             | 5.1      | 1.1             | 2.17          | 0.16                 | PL  | ... | 1      | ...                  | ... | agu   | IC 1531 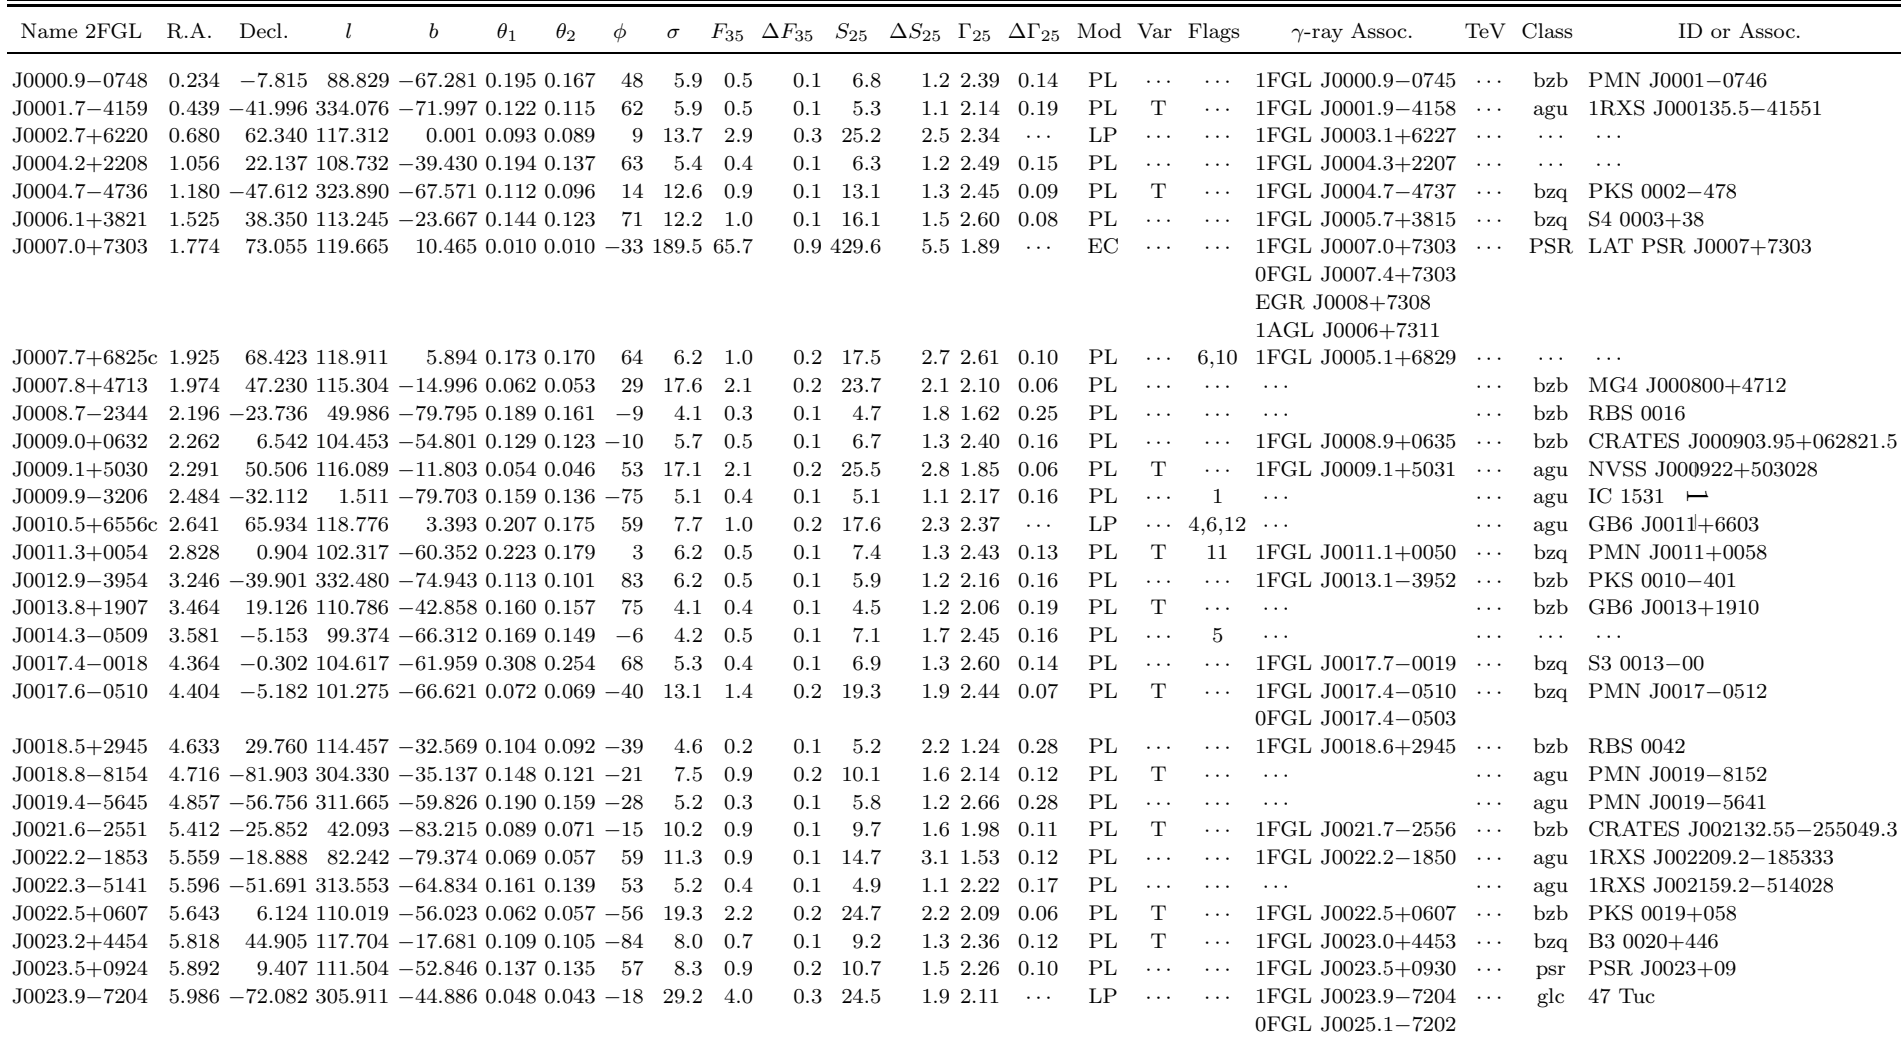 |
| J0010.5+6556c | 2.641 | 65.934  | 118.776 | 3.393   | 0.207      | 0.175      | 59     | 7.7      | 1.0      | 0.2             | 17.6     | 2.3             | 2.37          | ...                  | LP  | ... | 4,6,12 | ...                  | ... | agu   | GB6 J0011+6603                                                                              |
| J0011.3+0054  | 2.828 | 0.904   | 102.317 | −60.352 | 0.223      | 0.179      | 3      | 6.2      | 0.5      | 0.1             | 7.4      | 1.3             | 2.43          | 0.13                 | PL  | T   | 11     | 1FGL J0011.1+0050    | ... | bzq   | PMN J0011+0058                                                                              |
| J0012.9–3954  | 3.246 | −39.901 | 332.480 | −74.943 | 0.113      | 0.101      | 83     | 6.2      | 0.5      | 0.1             | 5.9      | 1.2             | 2.16          | 0.16                 | PL  | ... | ...    | 1FGL J0013.1–3952    | ... | bzb   | PKS 0010–401                                                                                |
| J0013.8+1907  | 3.464 | 19.126  | 110.786 | −42.858 | 0.160      | 0.157      | 75     | 4.1      | 0.4      | 0.1             | 4.5      | 1.2             | 2.06          | 0.19                 | PL  | T   | ...    | ...                  | ... | bzb   | GB6 J0013+1910                                                                              |
| J0014.3–0509  | 3.581 | −5.153  | 99.374  | −66.312 | 0.169      | 0.149      | −6     | 4.2      | 0.5      | 0.1             | 7.1      | 1.7             | 2.45          | 0.16                 | PL  | ... | 5      | ...                  | ... | ...   | ...                                                                                         |
| J0017.4–0018  | 4.364 | −0.302  | 104.617 | −61.959 | 0.308      | 0.254      | 68     | 5.3      | 0.4      | 0.1             | 6.9      | 1.3             | 2.60          | 0.14                 | PL  | ... | ...    | 1FGL J0017.7–0019    | ... | bzq   | S3 0013–00                                                                                  |
| J0017.6–0510  | 4.404 | −5.182  | 101.275 | −66.621 | 0.072      | 0.069      | −40    | 13.1     | 1.4      | 0.2             | 19.3     | 1.9             | 2.44          | 0.07                 | PL  | T   | ...    | 1FGL J0017.4–0510    | ... | bzq   | PMN J0017–0512                                                                              |
|               |       |         |         |         |            |            |        |          |          |                 |          |                 |               |                      |     |     |        | 0FGL J0017.4–0503    |     |       |                                                                                             |
| J0018.5+2945  | 4.633 | 29.760  | 114.457 | −32.569 | 0.104      | 0.092      | −39    | 4.6      | 0.2      | 0.1             | 5.2      | 2.2             | 1.24          | 0.28                 | PL  | ... | ...    | 1FGL J0018.6+2945    | ... | bzb   | RBS 0042                                                                                    |
| J0018.8–8154  | 4.716 | −81.903 | 304.330 | −35.137 | 0.148      | 0.121      | −21    | 7.5      | 0.9      | 0.2             | 10.1     | 1.6             | 2.14          | 0.12                 | PL  | T   | ...    | ...                  | ... | agu   | PMN J0019–8152                                                                              |
| J0019.4–5645  | 4.857 | −56.756 | 311.665 | −59.826 | 0.190      | 0.159      | −28    | 5.2      | 0.3      | 0.1             | 5.8      | 1.2             | 2.66          | 0.28                 | PL  | ... | ...    | ...                  | ... | agu   | PMN J0019–5641                                                                              |
| J0021.6–2551  | 5.412 | −25.852 | 42.093  | −83.215 | 0.089      | 0.071      | −15    | 10.2     | 0.9      | 0.1             | 9.7      | 1.6             | 1.98          | 0.11                 | PL  | T   | ...    | 1FGL J0021.7–2556    | ... | bzb   | CRATES J002132.55–255049.3                                                                  |
| J0022.2–1853  | 5.559 | −18.888 | 82.242  | −79.374 | 0.069      | 0.057      | 59     | 11.3     | 0.9      | 0.1             | 14.7     | 3.1             | 1.53          | 0.12                 | PL  | ... | ...    | 1FGL J0022.2–1850    | ... | agu   | 1RXS J002209.2–185333                                                                       |
| J0022.3–5141  | 5.596 | −51.691 | 313.553 | −64.834 | 0.161      | 0.139      | 53     | 5.2      | 0.4      | 0.1             | 4.9      | 1.1             | 2.22          | 0.17                 | PL  | ... | ...    | ...                  | ... | agu   | 1RXS J002159.2–514028                                                                       |
| J0022.5+0607  | 5.643 | 6.124   | 110.019 | −56.023 | 0.062      | 0.057      | −56    | 19.3     | 2.2      | 0.2             | 24.7     | 2.2             | 2.09          | 0.06                 | PL  | T   | ...    | 1FGL J0022.5+0607    | ... | bzb   | PKS 0019+058                                                                                |
| J0023.2+4454  | 5.818 | 44.905  | 117.704 | −17.681 | 0.109      | 0.105      | −84    | 8.0      | 0.7      | 0.1             | 9.2      | 1.3             | 2.36          | 0.12                 | PL  | T   | ...    | 1FGL J0023.0+4453    | ... | bzq   | B3 0020+446                                                                                 |
| J0023.5+0924  | 5.892 | 9.407   | 111.504 | −52.846 | 0.137      | 0.135      | 57     | 8.3      | 0.9      | 0.2             | 10.7     | 1.5             | 2.26          | 0.10                 | PL  | ... | ...    | 1FGL J0023.5+0930    | ... | psr   | PSR J0023+09                                                                                |
| J0023.9–7204  | 5.986 | −72.082 | 305.911 | −44.886 | 0.048      | 0.043      | −18    | 29.2     | 4.0      | 0.3             | 24.5     | 1.9             | 2.11          | ...                  | LP  | ... | ...    | 1FGL J0023.9–7204    | ... | glc   | 47 Tuc                                                                                      |
|               |       |         |         |         |            |            |        |          |          |                 |          |                 |               |                      |     |     |        | 0FGL J0025.1–7202    |     |       |                                                                                             |

Table 1—Continued

| Name 2FGL    | R.A.   | Decl.   | $l$     | $b$     | $\theta_1$ | $\theta_2$ | $\phi$ | $\sigma$ | $F_{35}$ | $\Delta F_{35}$ | $S_{25}$ | $\Delta S_{25}$ | $\Gamma_{25}$ | $\Delta \Gamma_{25}$ | Mod | Var | Flags | $\gamma$ -ray Assoc. | TeV | Class | ID or Assoc.        | Ref. |
|--------------|--------|---------|---------|---------|------------|------------|--------|----------|----------|-----------------|----------|-----------------|---------------|----------------------|-----|-----|-------|----------------------|-----|-------|---------------------|------|
| J0024.5+0346 | 6.146  | 3.783   | 110.064 | -58.416 | 0.199      | 0.139      | -38    | 4.7      | 0.5      | 0.1             | 5.9      | 1.3             | 2.24          | 0.16                 | PL  | T   | ...   | 1FGL J0024.6+0346    | ... | bzq   | GB6 J0024+0349      | ...  |
| J0029.2-7043 | 7.301  | -70.725 | 305.584 | -46.288 | 0.167      | 0.155      | -38    | 7.4      | 0.7      | 0.1             | 9.4      | 1.4             | 2.47          | 0.15                 | PL  | ... | ...   | ...                  | ... | bzb   | PKS 0026-710        | ...  |
| J0030.2-4223 | 7.573  | -42.386 | 317.356 | -74.145 | 0.085      | 0.077      | -67    | 15.8     | 1.0      | 0.1             | 16.5     | 1.3             | 2.61          | 0.08                 | PL  | T   | ...   | 1FGL J0029.9-4221    | ... | bzq   | PKS 0027-426        | ...  |
| J0030.4+0450 | 7.601  | 4.839   | 113.111 | -57.631 | 0.033      | 0.031      | 52     | 56.8     | 10.0     | 0.4             | 62.5     | 2.2             | 2.04          | ...                  | EC  | ... | ...   | 1FGL J0030.4+0451    | ... | PSR   | PSR J0030+0451      | ...  |
|              |        |         |         |         |            |            |        |          |          |                 |          |                 |               |                      |     |     |       | 0FGL J0030.3+0450    |     |       |                     |      |
| J0031.0+0724 | 7.775  | 7.414   | 114.095 | -55.108 | 0.119      | 0.103      | 87     | 4.4      | 0.3      | 0.1             | 4.0      | 1.3             | 1.89          | 0.27                 | PL  | ... | ...   | 1FGL J0030.7+0724    | ... | ...   | ...                 | ...  |
| J0032.7-5521 | 8.179  | -55.356 | 308.523 | -61.568 | 0.065      | 0.061      | 48     | 17.6     | 1.5      | 0.2             | 18.2     | 1.5             | 2.27          | 0.07                 | PL  | T   | ...   | 1FGL J0032.7-5519    | ... | ...   | ...                 | ...  |
| J0033.5-1921 | 8.391  | -19.357 | 94.171  | -81.213 | 0.036      | 0.035      | -4     | 27.1     | 3.1      | 0.2             | 40.0     | 3.9             | 1.76          | 0.05                 | PL  | ... | ...   | 1FGL J0033.5-1921    | ... | bzb   | KUV 00311-1938      | ...  |
|              |        |         |         |         |            |            |        |          |          |                 |          |                 |               |                      |     |     |       | 0FGL J0033.6-1921    |     |       |                     |      |
| J0034.4-0534 | 8.613  | -5.582  | 111.549 | -68.078 | 0.069      | 0.064      | 16     | 20.2     | 2.4      | 0.2             | 16.3     | 1.4             | 2.20          | ...                  | EC  | ... | ...   | 1FGL J0034.3-0534    | ... | PSR   | PSR J0034-0534      | ...  |
| J0035.2+1515 | 8.809  | 15.258  | 117.151 | -47.431 | 0.065      | 0.058      | -82    | 12.1     | 1.1      | 0.2             | 16.0     | 3.0             | 1.62          | 0.11                 | PL  | ... | ...   | 1FGL J0035.1+1516    | ... | bzb   | RX J0035.2+1515     | ...  |
| J0035.8+5951 | 8.964  | 59.854  | 120.975 | -2.959  | 0.041      | 0.040      | 50     | 15.1     | 2.4      | 0.2             | 28.6     | 3.1             | 1.87          | 0.07                 | PL  | T   | ...   | 1FGL J0035.9+5951    | ... | bzb   | 1ES 0033+595        | ...  |
|              |        |         |         |         |            |            |        |          |          |                 |          |                 |               |                      |     |     |       | 0FGL J0036.7+5951    |     |       |                     |      |
| J0037.8+1238 | 9.473  | 12.645  | 117.778 | -50.091 | 0.074      | 0.072      | -10    | 10.9     | 1.1      | 0.2             | 12.8     | 1.6             | 2.22          | 0.10                 | PL  | ... | ...   | 1FGL J0038.0+1236    | ... | bzb   | NVSS J003750+123818 | ...  |
| J0038.1+0015 | 9.542  | 0.265   | 115.751 | -62.422 | 0.147      | 0.132      | 36     | 4.4      | 0.4      | 0.1             | 4.3      | 1.3             | 1.93          | 0.22                 | PL  | ... | ...   | ...                  | ... | bzb   | BZB J0038+0013      | ...  |
| J0038.3-2457 | 9.583  | -24.963 | 68.538  | -86.346 | 0.173      | 0.119      | -9     | 9.8      | 0.8      | 0.1             | 10.6     | 1.3             | 2.39          | 0.11                 | PL  | T   | ...   | 1FGL J0038.4-2504    | ... | bzq   | PKS 0035-252        | ...  |
| J0038.7-2215 | 9.692  | -22.252 | 91.707  | -84.339 | 0.160      | 0.118      | 23     | 4.8      | 0.3      | 0.1             | 4.8      | 1.7             | 1.69          | 0.20                 | PL  | ... | ...   | ...                  | ... | agu   | PMN J0039+2220      | ...  |
| J0038.8+6259 | 9.720  | 62.997  | 121.508 | 0.160   | 0.094      | 0.084      | 42     | 5.6      | 1.3      | 0.2             | 14.4     | 2.6             | 2.19          | 0.10                 | PL  | ... | 10    | 1FGL J0038.6+6306    | ... | ...   | ...                 | ...  |
| J0039.1+4331 | 9.780  | 43.527  | 120.568 | -19.288 | 0.118      | 0.088      | 7      | 4.8      | 0.4      | 0.1             | 4.7      | 1.4             | 1.79          | 0.18                 | PL  | ... | ...   | 1FGL J0039.2+4331    | ... | ...   | ...                 | ...  |
| J0042.5+4114 | 10.633 | 41.245  | 121.132 | -21.596 | 0.215      | 0.176      | 8      | 5.2      | 0.5      | 0.1             | 6.5      | 1.3             | 2.26          | 0.15                 | PL  | ... | ...   | ...                  | ... | gal   | M 31                | ...  |
| J0043.7+3426 | 10.941 | 34.439  | 121.134 | -28.406 | 0.064      | 0.059      | 87     | 16.5     | 1.9      | 0.2             | 21.2     | 2.0             | 2.12          | 0.06                 | PL  | ... | ...   | 1FGL J0043.6+3424    | ... | bzq   | GB6 J0043+3426      | ...  |
| J0044.7-3702 | 11.195 | -37.040 | 310.595 | -79.989 | 0.166      | 0.141      | -68    | 8.1      | 0.5      | 0.1             | 8.4      | 1.1             | 2.57          | 0.12                 | PL  | T   | 2     | ...                  | ... | agu   | PKS 0042-373        | ...  |
| J0045.3+2127 | 11.335 | 21.452  | 121.041 | -41.397 | 0.047      | 0.047      | 55     | 15.2     | 1.5      | 0.2             | 17.1     | 2.1             | 1.95          | 0.09                 | PL  | T   | ...   | 1FGL J0045.3+2127    | ... | bzb   | GB6 J0045+2127      | ...  |
| J0045.5+1218 | 11.396 | 12.312  | 120.683 | -50.534 | 0.079      | 0.075      | -82    | 9.7      | 1.0      | 0.2             | 11.2     | 1.7             | 2.07          | 0.11                 | PL  | ... | ...   | ...                  | ... | agu   | GB6 J0045+1217      | ...  |
| J0046.7-8416 | 11.693 | -84.270 | 303.071 | -32.857 | 0.161      | 0.130      | 40     | 7.6      | 0.7      | 0.1             | 11.0     | 1.5             | 2.53          | 0.11                 | PL  | ... | ...   | 1FGL J0048.0-8412    | ... | bzq   | PKS 0044-84         | ...  |
| J0047.0-2516 | 11.755 | -25.275 | 94.545  | -87.899 | 0.190      | 0.138      | 78     | 6.9      | 0.6      | 0.1             | 7.6      | 1.3             | 2.31          | 0.13                 | PL  | ... | ...   | 1FGL J0047.3-2512    | P   | sbq   | NGC 0253            | ...  |
| J0047.2+5657 | 11.809 | 56.961  | 122.356 | -5.906  | 0.073      | 0.057      | 35     | 13.6     | 2.0      | 0.2             | 22.2     | 2.3             | 2.06          | 0.07                 | PL  | ... | ...   | 1FGL J0046.8+5658    | ... | bzb   | GB6 J0047+5657      | ...  |
| J0047.9+2232 | 11.995 | 22.538  | 121.885 | -40.326 | 0.075      | 0.073      | -55    | 15.4     | 1.5      | 0.2             | 19.6     | 1.6             | 2.42          | 0.07                 | PL  | T   | ...   | 1FGL J0048.0+2232    | ... | bzq   | NVSS J004802+223525 | ...  |
| J0048.8-6347 | 12.218 | -63.796 | 303.406 | -53.330 | 0.135      | 0.128      | 64     | 4.1      | 0.4      | 0.1             | 3.9      | 1.1             | 2.05          | 0.19                 | PL  | ... | ...   | ...                  | ... | ...   | ...                 | ...  |
| J0049.7-5738 | 12.444 | -57.646 | 303.369 | -59.481 | 0.096      | 0.092      | 38     | 6.3      | 0.5      | 0.1             | 5.9      | 1.2             | 2.23          | 0.16                 | PL  | ... | ...   | 1FGL J0049.8-5738    | ... | bzq   | PKS 0047-579        | ...  |
| J0050.1-0452 | 12.531 | -4.879  | 122.069 | -67.749 | 0.148      | 0.120      | 8      | 5.8      | 0.5      | 0.1             | 7.0      | 1.3             | 2.42          | 0.16                 | PL  | T   | ...   | 1FGL J0050.0-0446    | ... | bzq   | PKS 0047-051        | ...  |
| J0050.2+0234 | 12.557 | 2.576   | 122.322 | -60.294 | 0.157      | 0.134      | -89    | 7.1      | 0.7      | 0.1             | 7.9      | 1.3             | 2.27          | 0.13                 | PL  | ... | ...   | 1FGL J0050.2+0235    | ... | bzb   | PKS 0047+023        | ...  |
| J0050.6-0929 | 12.668 | -9.496  | 122.310 | -72.367 | 0.050      | 0.046      | 64     | 30.6     | 3.9      | 0.3             | 43.2     | 2.6             | 2.14          | 0.04                 | PL  | T   | ...   | 1FGL J0050.6-0928    | ... | bzb   | PKS 0048-09         | ...  |
|              |        |         |         |         |            |            |        |          |          |                 |          |                 |               |                      |     |     |       | 0FGL J0050.5-0928    |     |       |                     |      |
| J0051.0-0648 | 12.753 | -6.808  | 122.627 | -69.680 | 0.106      | 0.098      | 63     | 11.2     | 1.2      | 0.2             | 14.4     | 1.7             | 2.22          | 0.09                 | PL  | T   | ...   | 1FGL J0051.1-0649    | ... | bzq   | PKS 0048-071        | ...  |

Table 1—Continued

| Name 2FGL     | R.A.   | Decl.   | $l$     | $b$     | $\theta_1$ | $\theta_2$ | $\phi$ | $\sigma$ | $F_{35}$ | $\Delta F_{35}$ | $S_{25}$ | $\Delta S_{25}$ | $\Gamma_{25}$ | $\Delta \Gamma_{25}$ | Mod | Var | Flags | $\gamma$ -ray Assoc. | TeV | Class | ID or Assoc.          | Ref. |
|---------------|--------|---------|---------|---------|------------|------------|--------|----------|----------|-----------------|----------|-----------------|---------------|----------------------|-----|-----|-------|----------------------|-----|-------|-----------------------|------|
|               |        |         |         |         |            |            |        |          |          |                 |          |                 |               |                      |     |     |       | 0FGL J0051.1–0647    |     |       |                       |      |
| J0051.4–6241  | 12.860 | –62.686 | 302.931 | –54.442 | 0.052      | 0.049      | –44    | 16.2     | 1.4      | 0.2             | 19.5     | 2.9             | 1.69          | 0.08                 | PL  | ... | ...   | 1FGL J0051.4–6242    | ... | agu   | 1RXS J005117.7–624154 | ...  |
| J0055.0–2454  | 13.757 | –24.904 | 143.068 | –87.634 | 0.122      | 0.099      | 14     | 5.1      | 0.4      | 0.1             | 5.7      | 1.7             | 1.76          | 0.17                 | PL  | ... | ...   | 1FGL J0054.9–2455    | ... | agu   | 1RXS J005447.2–245532 | ...  |
| J0056.8–2111  | 14.222 | –21.197 | 135.057 | –83.940 | 0.131      | 0.118      | 66     | 5.7      | 0.5      | 0.1             | 5.9      | 1.6             | 1.82          | 0.20                 | PL  | ... | 2     | ...                  | ... | agu   | PMN J0056–2117        | ...  |
| J0057.9+3311  | 14.480 | 33.185  | 124.493 | –29.668 | 0.140      | 0.117      | 40     | 8.0      | 0.8      | 0.1             | 9.4      | 1.4             | 2.23          | 0.11                 | PL  | T   | ...   | 1FGL J0058.0+3314    | ... | bzq   | MG3 J005830+3311      | ...  |
| J0057.9–3236  | 14.493 | –32.607 | 288.837 | –84.341 | 0.084      | 0.081      | 2      | 10.8     | 0.9      | 0.1             | 10.3     | 1.5             | 2.10          | 0.10                 | PL  | ... | ...   | 1FGL J0058.4–3235    | ... | bzb   | PKS 0055–328          | ...  |
| J0059.0–7242e | 14.750 | –72.700 | 302.145 | –44.417 | ...        | ...        | ...    | 14.4     | 3.0      | 0.3             | 34.1     | 3.0             | 2.19          | 0.06                 | PL  | ... | ...   | 1FGL J0101.3–7257    | ... | GAL   | SMC                   | 1    |
| J0059.2–0151  | 14.819 | –1.852  | 127.512 | –64.654 | 0.093      | 0.090      | –60    | 4.6      | 0.2      | 0.1             | 6.3      | 2.8             | 1.15          | 0.36                 | PL  | ... | ...   | ...                  | ... | agu   | 1RXS J005916.3–015030 | ...  |
| J0059.7–5700  | 14.936 | –57.004 | 300.664 | –60.087 | 0.208      | 0.169      | 45     | 8.4      | 0.5      | 0.1             | 10.6     | 1.3             | 2.70          | 0.13                 | PL  | T   | ...   | ...                  | ... | agu   | PKS 0056–572          | ...  |
| J0100.2+0746  | 15.063 | 7.776   | 126.744 | –55.030 | 0.047      | 0.042      | –74    | 18.4     | 2.0      | 0.2             | 26.7     | 3.5             | 1.71          | 0.07                 | PL  | T   | ...   | 1FGL J0100.2+0747    | ... | bzb   | GB6 J0100+0745        | ...  |
|               |        |         |         |         |            |            |        |          |          |                 |          |                 |               |                      |     |     |       | 0FGL J0100.2+0750    |     |       |                       |      |
| J0101.2–6425  | 15.312 | –64.420 | 301.186 | –52.675 | 0.072      | 0.067      | –6     | 18.2     | 2.2      | 0.2             | 10.8     | 1.2             | 2.02          | ...                  | EC  | ... | ...   | 1FGL J0101.0–6423    | ... | PSR   | PSR J0101–6422        | ...  |
| J0102.2+0943  | 15.553 | 9.726   | 127.352 | –53.053 | 0.134      | 0.120      | –35    | 5.5      | 0.5      | 0.1             | 6.0      | 1.4             | 2.07          | 0.18                 | PL  | ... | ...   | 1FGL J0102.3+0942    | ... | ...   | ...                   | ...  |
| J0102.3+4216  | 15.586 | 42.275  | 125.087 | –20.551 | 0.142      | 0.122      | 46     | 10.6     | 0.8      | 0.1             | 13.1     | 1.4             | 2.61          | 0.09                 | PL  | T   | ...   | 1FGL J0102.2+4223    | ... | bzq   | GB6 J0102+4214        | ...  |
| J0102.7+5827  | 15.688 | 58.462  | 124.416 | –4.377  | 0.061      | 0.058      | 26     | 16.8     | 2.8      | 0.2             | 33.1     | 2.4             | 2.28          | 0.05                 | PL  | T   | ...   | 1FGL J0102.8+5827    | ... | bzq   | TXS 0059+581          | ...  |
| J0102.9+4838  | 15.742 | 48.647  | 124.896 | –14.181 | 0.068      | 0.059      | 83     | 13.3     | 2.4      | 0.3             | 13.2     | 2.2             | 2.14          | ...                  | LP  | ... | 5     | 1FGL J0103.1+4840    | ... | psr   | PSR J0103+48          | ...  |
| J0103.5+5336  | 15.894 | 53.604  | 124.756 | –9.224  | 0.070      | 0.065      | –21    | 5.8      | 0.6      | 0.1             | 7.4      | 1.9             | 1.75          | 0.16                 | PL  | ... | ...   | ...                  | ... | agu   | 1RXS J010325.9+533721 | ...  |
| J0103.8+1324  | 15.953 | 13.401  | 127.556 | –49.360 | 0.155      | 0.112      | –82    | 4.9      | 0.4      | 0.1             | 4.9      | 1.3             | 1.97          | 0.21                 | PL  | ... | ...   | ...                  | ... | ...   | ...                   | ...  |
| J0105.0–2411  | 16.251 | –24.197 | 169.888 | –85.765 | 0.184      | 0.147      | 4      | 9.4      | 0.8      | 0.1             | 10.2     | 1.3             | 2.41          | 0.11                 | PL  | T   | ...   | 1FGL J0104.4–2406    | ... | bzq   | PKS 0102–245          | ...  |
| J0105.3+3930  | 16.343 | 39.516  | 125.857 | –23.276 | 0.108      | 0.107      | 76     | 7.0      | 0.6      | 0.1             | 7.4      | 1.3             | 2.21          | 0.13                 | PL  | T   | ...   | 1FGL J0105.7+3930    | ... | bzb   | GB6 J0105+3928        | ...  |
| J0106.5+4854  | 16.646 | 48.913  | 125.495 | –13.884 | 0.057      | 0.054      | 35     | 17.3     | 3.3      | 0.3             | 20.6     | 2.7             | 2.10          | ...                  | LP  | ... | ...   | 1FGL J0106.7+4853    | ... | ...   | ...                   | ...  |
| J0108.6+0135  | 17.174 | 1.591   | 131.850 | –60.982 | 0.035      | 0.034      | –43    | 60.5     | 6.4      | 0.3             | 79.7     | 2.5             | 2.41          | ...                  | LP  | T   | ...   | 1FGL J0108.6+0135    | ... | bzq   | 4C +01.02             | ...  |
| J0109.0+1817  | 17.264 | 18.292  | 128.789 | –44.380 | 0.093      | 0.086      | –47    | 5.8      | 0.5      | 0.1             | 5.6      | 1.3             | 1.99          | 0.17                 | PL  | ... | ...   | 1FGL J0109.0+1816    | ... | bzb   | MG1 J010908+1816      | ...  |
| J0109.9+6132  | 17.486 | 61.541  | 125.136 | –1.251  | 0.044      | 0.044      | –79    | 32.9     | 5.3      | 0.3             | 69.8     | 2.8             | 2.48          | ...                  | LP  | T   | ...   | ...                  | ... | bzq   | TXS 0106+612          | ...  |
| J0110.3+6805  | 17.579 | 68.098  | 124.699 | 5.291   | 0.055      | 0.050      | –32    | 11.5     | 1.9      | 0.2             | 21.2     | 2.4             | 2.13          | 0.08                 | PL  | ... | ...   | 1FGL J0110.0+6806    | ... | agu   | 4C +67.04             | ...  |
| J0112.1+2245  | 18.033 | 22.764  | 129.151 | –39.858 | 0.029      | 0.027      | –70    | 49.4     | 7.1      | 0.3             | 79.2     | 3.5             | 2.07          | 0.03                 | PL  | T   | ...   | 1FGL J0112.0+2247    | ... | bzb   | S2 0109+22            | ...  |
|               |        |         |         |         |            |            |        |          |          |                 |          |                 |               |                      |     |     |       | 0FGL J0112.1+2247    |     |       |                       |      |
| J0112.8+3208  | 18.207 | 32.139  | 128.188 | –30.515 | 0.042      | 0.040      | 63     | 39.5     | 4.6      | 0.3             | 55.8     | 2.3             | 2.31          | 0.03                 | PL  | T   | ...   | 1FGL J0112.9+3207    | ... | bzq   | 4C 31.03              | ...  |
| J0113.2–3557  | 18.315 | –35.951 | 276.530 | –80.032 | 0.175      | 0.167      | 21     | 4.5      | 0.4      | 0.1             | 4.4      | 1.1             | 2.16          | 0.19                 | PL  | ... | ...   | ...                  | ... | bzq   | PMN J0113–3551        | ...  |
| J0113.7+4948  | 18.441 | 49.801  | 126.625 | –12.911 | 0.090      | 0.083      | 2      | 7.4      | 0.9      | 0.2             | 10.2     | 1.7             | 2.26          | 0.12                 | PL  | ... | ...   | 1FGL J0113.8+4945    | ... | bzq   | S4 0110+49            | ...  |
| J0114.7+1326  | 18.675 | 13.441  | 131.580 | –49.040 | 0.087      | 0.072      | 74     | 12.2     | 1.2      | 0.2             | 13.8     | 1.6             | 2.19          | 0.09                 | PL  | T   | ...   | 1FGL J0114.4+1327    | ... | bzb   | GB6 J0114+1325        | ...  |
| J0115.4+0358  | 18.875 | 3.967   | 134.430 | –58.366 | 0.080      | 0.077      | 79     | 14.7     | 1.6      | 0.2             | 17.6     | 1.9             | 2.07          | 0.08                 | PL  | ... | ...   | 1FGL J0115.7+0357    | ... | bzb   | PMN J0115+0356        | ...  |
| J0115.7+2518  | 18.934 | 25.301  | 129.835 | –37.245 | 0.059      | 0.055      | 20     | 12.1     | 1.3      | 0.2             | 14.4     | 1.9             | 2.00          | 0.09                 | PL  | ... | ...   | 1FGL J0115.5+2519    | ... | bzb   | RX J0115.7+2519       | ...  |
| J0116.0–1134  | 19.003 | –11.571 | 144.472 | –73.407 | 0.098      | 0.090      | 46     | 17.9     | 1.5      | 0.2             | 20.7     | 1.5             | 2.44          | 0.07                 | PL  | T   | ...   | 1FGL J0115.5–1132    | ... | bzq   | PKS 0113–118          | ...  |
| J0116.6–6153  | 19.175 | –61.887 | 297.749 | –54.986 | 0.101      | 0.086      | –74    | 5.5      | 0.3      | 0.1             | 4.5      | 1.6             | 1.63          | 0.24                 | PL  | ... | ...   | ...                  | ... | ...   | ...                   | ...  |

Table 1—Continued

| Name 2FGL    | R.A.   | Decl.   | $l$     | $b$     | $\theta_1$ | $\theta_2$ | $\phi$ | $\sigma$ | $F_{35}$ | $\Delta F_{35}$ | $S_{25}$ | $\Delta S_{25}$ | $\Gamma_{25}$ | $\Delta \Gamma_{25}$ | Mod | Var | Flags | $\gamma$ -ray Assoc.                   | TeV | Class | ID or Assoc.          | Ref. |
|--------------|--------|---------|---------|---------|------------|------------|--------|----------|----------|-----------------|----------|-----------------|---------------|----------------------|-----|-----|-------|----------------------------------------|-----|-------|-----------------------|------|
| J0118.6–4631 | 19.665 | –46.525 | 289.226 | –69.872 | 0.134      | 0.109      | –66    | 4.5      | 0.3      | 0.1             | 4.0      | 1.4             | 1.78          | 0.28                 | PL  | ... | ...   | ...                                    | ... | agu   | SUMSS J011902–462637  | ...  |
| J0118.8–2142 | 19.724 | –21.706 | 173.461 | –81.728 | 0.049      | 0.048      | –38    | 40.3     | 4.3      | 0.3             | 44.1     | 2.2             | 2.27          | ...                  | LP  | T   | ...   | 1FGL J0118.7–2137<br>0FGL J0118.7–2139 | ... | bzq   | PKS 0116–219          | ...  |
| J0120.4–2700 | 20.124 | –27.015 | 213.584 | –83.531 | 0.031      | 0.030      | –59    | 35.2     | 4.3      | 0.3             | 49.7     | 3.5             | 1.93          | 0.04                 | PL  | T   | ...   | 1FGL J0120.5–2700<br>0FGL J0120.5–2703 | ... | bzb   | PKS 0118–272          | ...  |
| J0122.6+3425 | 20.665 | 34.420  | 130.223 | –28.009 | 0.096      | 0.077      | –24    | 5.7      | 0.4      | 0.1             | 5.8      | 2.0             | 1.53          | 0.21                 | PL  | ... | 2     | ...                                    | ... | bzb   | 1ES 0120+340          | ...  |
| J0124.5–0621 | 21.149 | –6.364  | 145.208 | –67.790 | 0.201      | 0.172      | 14     | 6.1      | 0.6      | 0.1             | 7.2      | 1.3             | 2.24          | 0.13                 | PL  | ... | ...   | 1FGL J0124.6–0616                      | ... | bzb   | PMN J0124–0624        | ...  |
| J0124.6–2322 | 21.155 | –23.369 | 188.135 | –81.611 | 0.113      | 0.109      | –55    | 7.5      | 0.7      | 0.1             | 8.1      | 1.3             | 2.31          | 0.15                 | PL  | ... | 2     | ...                                    | ... | ...   | ...                   | ...  |
| J0127.2+0324 | 21.819 | 3.407   | 140.123 | –58.263 | 0.097      | 0.086      | 23     | 10.4     | 1.0      | 0.1             | 12.2     | 2.2             | 1.84          | 0.11                 | PL  | ... | ...   | 1FGL J0127.0+0322                      | ... | agu   | NVSS J012713+032259   | ...  |
| J0128.0+6330 | 22.003 | 63.505  | 126.998 | 0.922   | 0.255      | 0.206      | –66    | 5.0      | 0.9      | 0.2             | 14.7     | 2.8             | 2.57          | 0.13                 | PL  | ... | 4,8   | ...                                    | ... | †     | ...                   | ...  |
| J0128.4+4431 | 22.117 | 44.530  | 129.852 | –17.843 | 0.281      | 0.138      | 13     | 6.0      | 0.6      | 0.1             | 7.6      | 1.4             | 2.25          | 0.13                 | PL  | T   | 9     | 1FGL J0128.6+4439                      | ... | bzq   | GB6 J0128+4439        | ...  |
| J0129.4+2618 | 22.369 | 26.310  | 133.451 | –35.784 | 0.333      | 0.195      | 61     | 4.9      | 0.5      | 0.1             | 7.5      | 1.5             | 2.56          | 0.15                 | PL  | ... | ...   | ...                                    | ... | ...   | ...                   | ...  |
| J0131.1+6121 | 22.785 | 61.356  | 127.673 | –1.150  | 0.041      | 0.040      | –77    | 16.1     | 2.7      | 0.3             | 31.3     | 3.1             | 1.91          | 0.08                 | PL  | T   | ...   | 1FGL J0131.2+6121                      | ... | agu   | 1RXS J013106.4+612035 | ...  |
| J0132.8–1654 | 23.214 | –16.902 | 168.191 | –75.988 | 0.070      | 0.063      | –70    | 25.5     | 2.1      | 0.2             | 29.5     | 1.6             | 2.45          | 0.05                 | PL  | T   | ...   | 1FGL J0132.6–1655                      | ... | bzq   | PKS 0130–17           | ...  |
| J0133.4–4408 | 23.364 | –44.142 | 279.235 | –71.002 | 0.116      | 0.103      | –20    | 5.6      | 0.4      | 0.1             | 5.0      | 1.2             | 2.07          | 0.17                 | PL  | ... | ...   | ...                                    | ... | ...   | ...                   | ...  |
| J0134.4+2636 | 23.621 | 26.616  | 134.731 | –35.268 | 0.094      | 0.082      | –69    | 8.0      | 0.9      | 0.2             | 10.2     | 2.0             | 1.86          | 0.12                 | PL  | ... | ...   | 1FGL J0134.4+2632                      | ... | agu   | 1RXS J013427.2+263846 | ...  |
| J0136.5+3905 | 24.143 | 39.089  | 132.425 | –22.949 | 0.032      | 0.029      | –86    | 33.3     | 4.5      | 0.3             | 61.9     | 5.0             | 1.69          | 0.04                 | PL  | ... | ...   | 1FGL J0136.5+3905<br>0FGL J0136.6+3903 | ... | bzb   | B3 0133+388           | ...  |
| J0136.9+4751 | 24.240 | 47.861  | 130.785 | –14.315 | 0.031      | 0.030      | 56     | 51.9     | 7.2      | 0.3             | 76.2     | 2.7             | 2.29          | ...                  | LP  | T   | ...   | 1FGL J0137.0+4751<br>0FGL J0137.1+4751 | ... | bzq   | OC 457                | ...  |
| J0137.6–2430 | 24.406 | –24.509 | 201.356 | –79.286 | 0.092      | 0.088      | 60     | 13.9     | 1.0      | 0.1             | 14.2     | 1.3             | 2.42          | 0.08                 | PL  | T   | ...   | 1FGL J0137.5–2428                      | ... | bzq   | PKS 0135–247          | ...  |
| J0137.7+5811 | 24.443 | 58.199  | 129.022 | –4.124  | 0.100      | 0.089      | 65     | 7.3      | 1.1      | 0.2             | 13.3     | 2.0             | 2.33          | 0.12                 | PL  | ... | 4     | 1FGL J0137.8+5814                      | ... | agu   | 1RXS J013748.0+581422 | ...  |
| J0141.5–0928 | 25.396 | –9.481  | 159.140 | –68.750 | 0.063      | 0.059      | –58    | 15.8     | 1.6      | 0.2             | 18.2     | 2.0             | 2.03          | 0.07                 | PL  | ... | ...   | 1FGL J0141.7–0929                      | ... | bzb   | PKS 0139–09           | ...  |
| J0143.6–5844 | 25.917 | –58.745 | 290.468 | –57.102 | 0.064      | 0.056      | –47    | 14.2     | 1.2      | 0.2             | 16.1     | 2.5             | 1.74          | 0.09                 | PL  | ... | ...   | 1FGL J0143.9–5845                      | ... | ...   | ...                   | ...  |
| J0144.6+2704 | 26.156 | 27.079  | 137.286 | –34.306 | 0.049      | 0.045      | 81     | 27.2     | 3.4      | 0.2             | 38.5     | 2.3             | 2.17          | 0.04                 | PL  | T   | ...   | 1FGL J0144.6+2703<br>0FGL J0144.5+2709 | ... | bzb   | TXS 0141+268          | ...  |
| J0145.1–2732 | 26.279 | –27.548 | 218.032 | –78.078 | 0.078      | 0.077      | –67    | 28.8     | 2.1      | 0.2             | 33.7     | 1.6             | 2.58          | 0.05                 | PL  | T   | ...   | 1FGL J0144.9–2732<br>0FGL J0145.1–2728 | ... | bzq   | PKS 0142–278          | ...  |
| J0146.6–5206 | 26.674 | –52.108 | 284.116 | –62.955 | 0.147      | 0.118      | –73    | 4.3      | 0.3      | 0.1             | 3.8      | 1.1             | 2.03          | 0.24                 | PL  | ... | ...   | ...                                    | ... | agu   | PKS 0144–522          | ...  |
| J0148.6+0127 | 27.152 | 1.463   | 150.917 | –58.268 | 0.107      | 0.099      | –87    | 5.4      | 0.5      | 0.1             | 5.3      | 1.3             | 2.02          | 0.20                 | PL  | ... | ...   | ...                                    | ... | agu   | PMN J0148+0129        | ...  |
| J0152.6+0148 | 28.163 | 1.800   | 152.366 | –57.531 | 0.070      | 0.062      | –29    | 8.9      | 0.8      | 0.1             | 9.6      | 2.0             | 1.79          | 0.14                 | PL  | ... | ...   | ...                                    | P   | bzb   | PMN J0152+0146        | ...  |
| J0153.9+0823 | 28.489 | 8.396   | 148.212 | –51.381 | 0.061      | 0.055      | –83    | 15.4     | 1.8      | 0.2             | 21.7     | 2.7             | 1.86          | 0.07                 | PL  | ... | ...   | 1FGL J0154.1+0823                      | ... | bzb   | GB6 J0154+0823        | ...  |
| J0154.9+4434 | 28.733 | 44.573  | 134.679 | –16.846 | 0.090      | 0.079      | 68     | 4.7      | 0.4      | 0.1             | 4.4      | 1.3             | 2.01          | 0.26                 | PL  | ... | ...   | 1FGL J0155.0+4433                      | ... | bzb   | GB6 J0154+4433        | ...  |
| J0156.4+3909 | 29.108 | 39.165  | 136.463 | –21.993 | 0.168      | 0.121      | –63    | 7.9      | 0.7      | 0.1             | 9.2      | 1.3             | 2.40          | 0.12                 | PL  | T   | ...   | ...                                    | ... | agu   | MG4 J015630+3913      | ...  |
| J0156.5–2419 | 29.139 | –24.327 | 205.745 | –75.081 | 0.121      | 0.107      | –32    | 5.0      | 0.4      | 0.1             | 4.6      | 1.4             | 1.79          | 0.19                 | PL  | T   | ...   | ...                                    | ... | agu   | TXS 0154–244          | ...  |

Table 1—Continued

| Name 2FGL     | R.A.   | Decl.   | $l$     | $b$     | $\theta_1$ | $\theta_2$ | $\phi$ | $\sigma$ | $F_{35}$ | $\Delta F_{35}$ | $S_{25}$ | $\Delta S_{25}$ | $\Gamma_{25}$ | $\Delta \Gamma_{25}$ | Mod | Var | Flags | $\gamma$ -ray Assoc. | TeV | Class | ID or Assoc.          | Ref. |
|---------------|--------|---------|---------|---------|------------|------------|--------|----------|----------|-----------------|----------|-----------------|---------------|----------------------|-----|-----|-------|----------------------|-----|-------|-----------------------|------|
| J0157.2–5259  | 29.317 | –52.994 | 282.073 | –61.386 | 0.101      | 0.090      | –32    | 6.5      | 0.5      | 0.1             | 6.7      | 1.8             | 1.75          | 0.17                 | PL  | ... | ...   | 1FGL J0157.0–5259    | ... | agu   | 1RXS J015658.6–530208 | ...  |
| J0158.0–4609  | 29.500 | –46.154 | 272.613 | –66.860 | 0.166      | 0.134      | 48     | 6.8      | 0.5      | 0.1             | 6.8      | 1.1             | 2.36          | 0.14                 | PL  | ... | ...   | 1FGL J0157.5–4613    | ... | bzq   | PMN J0157–4614        | ...  |
| J0158.3–3931  | 29.576 | –39.530 | 258.918 | –71.380 | 0.104      | 0.095      | 49     | 9.3      | 0.9      | 0.1             | 10.1     | 1.6             | 2.07          | 0.11                 | PL  | ... | ...   | 1FGL J0158.0–3931    | ... | bzb   | PMN J0158–3932        | ...  |
| J0158.4+0107  | 29.606 | 1.125   | 155.327 | –57.471 | 0.205      | 0.152      | –55    | 4.8      | 0.4      | 0.1             | 5.8      | 1.2             | 2.49          | 0.19                 | PL  | ... | ...   | ...                  | ... | ...   | ...                   | ...  |
| J0158.6+8558  | 29.671 | 85.967  | 124.201 | 23.262  | 0.180      | 0.154      | –87    | 4.2      | 0.4      | 0.1             | 5.5      | 1.2             | 2.52          | 0.17                 | PL  | ... | ...   | ...                  | ... | ...   | ...                   | ...  |
| J0159.5+1046  | 29.899 | 10.777  | 148.761 | –48.646 | 0.092      | 0.079      | –73    | 9.8      | 1.1      | 0.2             | 11.9     | 1.6             | 2.15          | 0.11                 | PL  | ... | ...   | 1FGL J0159.5+1047    | ... | bzb   | RX J0159.5+1047       | ...  |
| J0159.6–2741  | 29.912 | –27.696 | 219.014 | –74.863 | 0.138      | 0.119      | –11    | 7.0      | 0.6      | 0.1             | 6.4      | 1.2             | 2.12          | 0.13                 | PL  | ... | ...   | 1FGL J0159.7–2741    | ... | bzb   | PMN J0159–2739        | ...  |
| J0200.4–4105  | 30.105 | –41.096 | 261.910 | –70.098 | 0.112      | 0.100      | –23    | 4.4      | 0.3      | 0.1             | 4.1      | 1.3             | 1.82          | 0.23                 | PL  | ... | ...   | ...                  | ... | ...   | ...                   | ...  |
| J0201.5–6626  | 30.392 | –66.448 | 292.314 | –49.210 | 0.179      | 0.163      | –44    | 4.4      | 0.4      | 0.1             | 4.6      | 1.1             | 2.25          | 0.18                 | PL  | T   | 2     | ...                  | ... | agu   | PMN J0201–6638        | ...  |
| J0203.6+7235  | 30.922 | 72.592  | 128.345 | 10.484  | 0.078      | 0.072      | 14     | 7.2      | 1.0      | 0.2             | 11.1     | 1.9             | 2.02          | 0.13                 | PL  | T   | ...   | 1FGL J0203.5+7234    | ... | bzb   | S5 0159+723           | ...  |
| J0204.0+3045  | 31.014 | 30.754  | 140.864 | –29.576 | 0.170      | 0.163      | –65    | 6.7      | 0.6      | 0.1             | 8.8      | 1.4             | 2.46          | 0.13                 | PL  | ... | ...   | 1FGL J0203.5+3044    | ... | bzq   | B2 0200+30            | ...  |
| J0205.0+1514  | 31.256 | 15.235  | 147.988 | –44.027 | 0.135      | 0.109      | –15    | 8.6      | 0.8      | 0.1             | 10.2     | 1.4             | 2.28          | 0.11                 | PL  | T   | ...   | 1FGL J0204.5+1516    | ... | agn   | 4C +15.05             | ...  |
|               |        |         |         |         |            |            |        |          |          |                 |          |                 |               |                      |     |     |       | 3EG J0204+1458       |     |       |                       |      |
|               |        |         |         |         |            |            |        |          |          |                 |          |                 |               |                      |     |     |       | EGR J0204+1505       |     |       |                       |      |
| J0205.3–1657  | 31.329 | –16.965 | 185.993 | –70.129 | 0.164      | 0.109      | 24     | 12.8     | 0.7      | 0.1             | 14.1     | 1.3             | 2.68          | 0.09                 | PL  | T   | ...   | 1FGL J0205.0–1702    | ... | bzq   | PKS 0202–17           | ...  |
|               |        |         |         |         |            |            |        |          |          |                 |          |                 |               |                      |     |     |       | 0FGL J0204.8–1704    |     |       |                       |      |
| J0205.4+3211  | 31.364 | 32.194  | 140.662 | –28.116 | 0.209      | 0.191      | –27    | 6.0      | 0.5      | 0.1             | 8.7      | 1.5             | 2.66          | 0.14                 | PL  | ... | ...   | 1FGL J0205.3+3217    | ... | bzq   | B2 0202+31            | ...  |
| J0205.8+6448  | 31.454 | 64.810  | 130.744 | 3.072   | 0.041      | 0.037      | –72    | 27.4     | 5.5      | 0.3             | 53.7     | 2.7             | 2.35          | ...                  | EC  | ... | ...   | 1FGL J0205.6+6449    | ... | PSR   | PSR J0205+6449        | ...  |
| J0206.5–1149  | 31.649 | –11.829 | 175.642 | –66.656 | 0.093      | 0.090      | –86    | 8.2      | 0.7      | 0.1             | 7.4      | 1.3             | 2.09          | 0.14                 | PL  | T   | ...   | ...                  | ... | bzq   | PMN J0206–1150        | ...  |
| J0207.9–6832  | 31.985 | –68.538 | 292.798 | –47.056 | 0.132      | 0.114      | –73    | 4.6      | 0.3      | 0.1             | 4.6      | 1.1             | 2.43          | 0.20                 | PL  | ... | ...   | ...                  | ... | agu   | PKS 0206–688          | ...  |
| J0209.5–5229  | 32.376 | –52.500 | 278.342 | –60.741 | 0.063      | 0.054      | –56    | 14.1     | 1.5      | 0.2             | 16.7     | 2.2             | 1.91          | 0.09                 | PL  | ... | ...   | 1FGL J0209.3–5229    | ... | bzb   | 1RXS J020922.2–522920 | ...  |
| J0210.7–5102  | 32.696 | –51.035 | 276.122 | –61.763 | 0.046      | 0.043      | 22     | 35.8     | 3.8      | 0.2             | 49.9     | 2.1             | 2.40          | 0.04                 | PL  | T   | ...   | 1FGL J0210.6–5101    | ... | agu   | PKS 0208–512          | ...  |
|               |        |         |         |         |            |            |        |          |          |                 |          |                 |               |                      |     |     |       | 0FGL J0210.8–5100    |     |       |                       |      |
|               |        |         |         |         |            |            |        |          |          |                 |          |                 |               |                      |     |     |       | 3EG J0210–5055       |     |       |                       |      |
|               |        |         |         |         |            |            |        |          |          |                 |          |                 |               |                      |     |     |       | EGR J0210–5058       |     |       |                       |      |
| J0211.2+1050  | 32.806 | 10.837  | 152.595 | –47.388 | 0.054      | 0.052      | –81    | 20.3     | 2.6      | 0.2             | 29.2     | 2.2             | 2.17          | 0.05                 | PL  | T   | ...   | 1FGL J0211.2+1049    | ... | bzb   | MG1 J021114+1051      | ...  |
| J0212.1+5318  | 33.039 | 53.305  | 134.938 | –7.674  | 0.084      | 0.075      | –84    | 15.1     | 2.6      | 0.3             | 15.0     | 1.6             | 2.07          | ...                  | LP  | ... | ...   | 1FGL J0212.3+5319    | ... | ...   | ...                   | ...  |
| J0213.1+2245  | 33.295 | 22.756  | 146.496 | –36.348 | 0.080      | 0.077      | –50    | 9.2      | 1.0      | 0.2             | 11.6     | 1.8             | 2.03          | 0.11                 | PL  | ... | ...   | 1FGL J0213.2+2244    | ... | bzb   | MG3 J021252+2246      | ...  |
| J0214.5+6251c | 33.637 | 62.853  | 132.251 | 1.495   | 0.134      | 0.119      | –6     | 4.1      | 1.0      | 0.2             | 12.2     | 3.1             | 2.26          | 0.14                 | PL  | ... | 6     | ...                  | ... | †     | ...                   | ...  |
| J0216.9–6630  | 34.238 | –66.514 | 290.278 | –48.460 | 0.133      | 0.105      | –47    | 7.4      | 0.7      | 0.1             | 7.7      | 1.5             | 1.94          | 0.14                 | PL  | ... | ...   | 1FGL J0217.9–6630    | ... | bzb   | RBS 0300              | ...  |
| J0217.4+0836  | 34.350 | 8.612   | 156.169 | –48.633 | 0.076      | 0.067      | –80    | 13.5     | 1.6      | 0.2             | 17.8     | 2.3             | 1.94          | 0.09                 | PL  | T   | ...   | 1FGL J0217.2+0834    | ... | bzb   | ZS 0214+083           | ...  |
| J0217.5–0813  | 34.382 | –8.220  | 174.071 | –62.205 | 0.319      | 0.231      | 18     | 4.1      | 0.4      | 0.1             | 4.6      | 1.1             | 2.27          | 0.19                 | PL  | ... | ...   | 1FGL J0217.0–0829    | ... | bzq   | PKS 0214–085          | ...  |
| J0217.7+7353  | 34.431 | 73.899  | 128.917 | 12.038  | 0.146      | 0.122      | 60     | 8.5      | 0.7      | 0.2             | 17.1     | 1.9             | 2.82          | 0.11                 | PL  | T   | 4     | 1FGL J0217.8+7353    | ... | bzq   | S5 0212+73            | ...  |
| J0217.9+0143  | 34.483 | 1.730   | 162.199 | –54.410 | 0.037      | 0.035      | 21     | 42.3     | 5.7      | 0.3             | 63.7     | 2.9             | 2.15          | 0.03                 | PL  | T   | ...   | 1FGL J0217.9+0144    | ... | bzq   | PKS 0215+015          | ...  |
|               |        |         |         |         |            |            |        |          |          |                 |          |                 |               |                      |     |     |       | 0FGL J0217.8+0146    |     |       |                       |      |

Table 1—Continued

| Name 2FGL     | R.A.   | Decl.   | $l$     | $b$     | $\theta_1$ | $\theta_2$ | $\phi$ | $\sigma$ | $F_{35}$ | $\Delta F_{35}$ | $S_{25}$ | $\Delta S_{25}$ | $\Gamma_{25}$ | $\Delta \Gamma_{25}$ | Mod | Var | Flags | $\gamma$ -ray Assoc. | TeV | Class | ID or Assoc.          | Ref. |
|---------------|--------|---------|---------|---------|------------|------------|--------|----------|----------|-----------------|----------|-----------------|---------------|----------------------|-----|-----|-------|----------------------|-----|-------|-----------------------|------|
| J0218.1+4233  | 34.527 | 42.553  | 139.504 | -17.512 | 0.047      | 0.041      | -84    | 26.7     | 4.9      | 0.3             | 47.1     | 2.9             | 2.35          | ...                  | EC  | T   | ...   | 1FGL J0218.1+4232    | ... | PSR   | PSR J0218+4232        | ...  |
| J0218.7+6208c | 34.680 | 62.140  | 132.937 | 0.975   | 0.078      | 0.072      | -54    | 10.5     | 2.4      | 0.6             | 38.4     | 4.1             | 2.37          | ...                  | LP  | ... | 5,6   | ...                  | ... | †     | ...                   | ...  |
| J0219.1-1725  | 34.780 | -17.426 | 191.883 | -67.564 | 0.148      | 0.143      | -18    | 4.3      | 0.4      | 0.1             | 4.8      | 1.4             | 1.92          | 0.21                 | PL  | ... | ...   | ...                  | ... | bzb   | 1RXS J021905.8-172503 | ...  |
| J0219.2+3641  | 34.812 | 36.688  | 141.927 | -22.923 | 0.111      | 0.104      | -71    | 7.1      | 0.8      | 0.1             | 13.3     | 2.2             | 2.61          | 0.12                 | PL  | T   | 5     | ...                  | ... | agu   | MG3 J021846+3641      | ...  |
| J0221.0+3555  | 35.267 | 35.930  | 142.600 | -23.495 | 0.034      | 0.034      | -33    | 34.7     | 5.3      | 0.3             | 63.2     | 2.8             | 2.28          | 0.04                 | PL  | T   | ...   | 1FGL J0221.0+3555    | ... | bzq   | S4 0218+35            | ...  |
|               |        |         |         |         |            |            |        |          |          |                 |          |                 |               |                      |     |     |       | 0FGL J0220.9+3607    |     |       |                       |      |
| J0221.2+2516  | 35.321 | 25.271  | 147.351 | -33.305 | 0.148      | 0.116      | -48    | 4.4      | 0.4      | 0.1             | 5.1      | 1.6             | 1.78          | 0.17                 | PL  | ... | ...   | ...                  | ... | ...   | ...                   | ...  |
| J0221.3+6025c | 35.342 | 60.430  | 133.810 | -0.528  | 0.110      | 0.102      | 27     | 4.6      | 1.2      | 0.3             | 17.3     | 3.7             | 2.45          | 0.11                 | PL  | ... | 6     | ...                  | ... | ...   | ...                   | ...  |
| J0221.4+6257c | 35.373 | 62.961  | 132.962 | 1.856   | 0.118      | 0.096      | -71    | 9.5      | 2.8      | 0.4             | 21.4     | 3.2             | 2.32          | ...                  | LP  | ... | 6     | 1FGL J0220.0+6257    | ... | †     | ...                   | ...  |
| J0222.0-1615  | 35.518 | -16.264 | 190.233 | -66.367 | 0.153      | 0.139      | 62     | 6.9      | 0.6      | 0.1             | 8.1      | 1.3             | 2.47          | 0.12                 | PL  | ... | ...   | 1FGL J0222.1-1618    | ... | bzq   | PKS 0219-164          | ...  |
| J0222.6+4302  | 35.662 | 43.036  | 140.141 | -16.767 | 0.014      | 0.014      | 31     | 95.0     | 25.6     | 0.6             | 257.5    | 9.2             | 1.91          | ...                  | LP  | T   | ...   | 1FGL J0222.6+4302    | P   | BZB   | 3C 66A                | 2    |
|               |        |         |         |         |            |            |        |          |          |                 |          |                 |               |                      |     |     |       | 0FGL J0222.6+4302    |     |       |                       |      |
|               |        |         |         |         |            |            |        |          |          |                 |          |                 |               |                      |     |     |       | 3EG J0222+4253       |     |       |                       |      |
|               |        |         |         |         |            |            |        |          |          |                 |          |                 |               |                      |     |     |       | EGR J0223+4300       |     |       |                       |      |
| J0222.7+6820  | 35.699 | 68.345  | 131.229 | 6.957   | 0.081      | 0.077      | 2      | 5.1      | 0.8      | 0.2             | 8.4      | 1.9             | 2.13          | 0.17                 | PL  | ... | 1     | ...                  | ... | ...   | ...                   | ...  |
| J0223.0-1118  | 35.761 | -11.314 | 181.060 | -63.298 | 0.105      | 0.088      | -11    | 5.2      | 0.3      | 0.1             | 4.9      | 1.8             | 1.56          | 0.22                 | PL  | ... | ...   | 1FGL J0223.0-1118    | ... | agu   | 1RXS J022314.6-111741 | ...  |
| J0224.0+6204  | 36.023 | 62.077  | 133.549 | 1.130   | 0.056      | 0.050      | -44    | 14.4     | 8.5      | 0.7             | 59.2     | 6.5             | 2.19          | ...                  | LP  | ... | ...   | 1FGL J0224.0+6201c   | ... | ...   | ...                   | ...  |
| J0225.9+6154c | 36.495 | 61.904  | 133.818 | 1.046   | 0.076      | 0.075      | 84     | 4.9      | 1.9      | 0.5             | 21.1     | 6.0             | 2.14          | 0.15                 | PL  | ... | 6     | 3EG J0229+6151       | ... | ...   | ...                   | ...  |
| J0226.1+0943  | 36.542 | 9.719   | 158.103 | -46.582 | 0.120      | 0.104      | -20    | 6.5      | 0.7      | 0.1             | 7.6      | 1.5             | 2.10          | 0.15                 | PL  | T   | ...   | 1FGL J0226.3+0937    | ... | ...   | ...                   | ...  |
| J0226.5-4444  | 36.632 | -44.734 | 261.977 | -64.095 | 0.134      | 0.113      | -3     | 5.6      | 0.4      | 0.1             | 6.0      | 2.1             | 1.57          | 0.27                 | PL  | ... | 1     | ...                  | ... | agu   | RBS 0318              | ...  |
| J0227.2+6029c | 36.815 | 60.487  | 134.471 | -0.220  | 0.097      | 0.086      | 79     | 6.1      | 1.6      | 0.3             | 20.8     | 4.0             | 2.38          | 0.11                 | PL  | ... | 6     | ...                  | ... | ...   | ...                   | ...  |
| J0227.3+0203  | 36.844 | 2.066   | 165.106 | -52.766 | 0.133      | 0.100      | 29     | 5.0      | 0.4      | 0.1             | 5.0      | 1.4             | 1.86          | 0.20                 | PL  | ... | ...   | ...                  | ... | bzb   | RX J0227.2+0201       | ...  |
| J0227.7+2249  | 36.950 | 22.825  | 150.232 | -34.888 | 0.115      | 0.102      | -9     | 6.5      | 0.7      | 0.1             | 8.2      | 1.7             | 2.00          | 0.14                 | PL  | T   | ...   | ...                  | ... | ...   | ...                   | ...  |
| J0229.3-3644  | 37.343 | -36.734 | 243.952 | -67.197 | 0.099      | 0.078      | 38     | 16.2     | 1.2      | 0.1             | 18.2     | 1.4             | 2.53          | 0.07                 | PL  | T   | ...   | 1FGL J0229.3-3644    | ... | bzq   | PKS 0227-369          | ...  |
|               |        |         |         |         |            |            |        |          |          |                 |          |                 |               |                      |     |     |       | 0FGL J0229.5-3640    |     |       |                       |      |
| J0230.8+4031  | 37.718 | 40.521  | 142.627 | -18.517 | 0.099      | 0.088      | -30    | 18.1     | 1.4      | 0.2             | 24.4     | 1.6             | 2.63          | 0.06                 | PL  | T   | ...   | 1FGL J0230.8+4031    | ... | bzq   | B3 0227+403           | ...  |
| J0233.9+6238c | 38.475 | 62.635  | 134.402 | 2.068   | 0.194      | 0.100      | 45     | 8.9      | 1.8      | 0.3             | 27.9     | 3.5             | 2.53          | 0.09                 | PL  | ... | 6,9   | ...                  | ... | ...   | ...                   | ...  |
| J0237.1-6136  | 39.294 | -61.615 | 283.165 | -51.262 | 0.057      | 0.053      | 81     | 28.9     | 2.8      | 0.2             | 35.3     | 1.8             | 2.33          | 0.04                 | PL  | T   | ...   | 1FGL J0238.3-6132    | ... | bzq   | PKS 0235-618          | 3    |
| J0237.5-3603  | 39.382 | -36.062 | 241.198 | -65.804 | 0.092      | 0.076      | 57     | 5.5      | 0.4      | 0.1             | 5.7      | 2.0             | 1.56          | 0.22                 | PL  | ... | 8     | 1FGL J0237.5-3603    | ... | bzb   | RBS 0334              | ...  |
| J0237.8+2846  | 39.472 | 28.778  | 149.482 | -28.549 | 0.054      | 0.051      | 28     | 36.5     | 3.8      | 0.3             | 47.6     | 1.9             | 2.44          | ...                  | LP  | T   | ...   | 1FGL J0237.9+2848    | ... | bzq   | 4C +28.07             | ...  |
|               |        |         |         |         |            |            |        |          |          |                 |          |                 |               |                      |     |     |       | 0FGL J0238.4+2855    |     |       |                       |      |
| J0237.9+5238  | 39.497 | 52.638  | 138.839 | -6.912  | 0.116      | 0.096      | -71    | 7.5      | 1.1      | 0.2             | 12.5     | 1.9             | 2.22          | 0.11                 | PL  | ... | ...   | ...                  | ... | ...   | ...                   | ...  |
| J0238.2-3905  | 39.565 | -39.096 | 248.031 | -64.767 | 0.121      | 0.110      | -67    | 5.1      | 0.4      | 0.1             | 5.2      | 1.8             | 1.67          | 0.18                 | PL  | ... | ...   | ...                  | ... | agu   | 1RXS J023800.5-390505 | ...  |
| J0238.6-3117  | 39.657 | -31.284 | 229.457 | -66.304 | 0.082      | 0.078      | -14    | 10.6     | 1.0      | 0.1             | 11.9     | 2.1             | 1.85          | 0.11                 | PL  | ... | ...   | 1FGL J0238.6-3117    | ... | bzb   | 1RXS J023832.6-311658 | ...  |
| J0238.7+1637  | 39.675 | 16.624  | 156.780 | -39.096 | 0.020      | 0.020      | -9     | 91.8     | 18.7     | 0.5             | 181.4    | 5.4             | 2.12          | ...                  | LP  | T   | ...   | 1FGL J0238.6+1637    | ... | BZB   | AO 0235+164           | ...  |

Table 1—Continued

| Name 2FGL     | R.A.   | Decl.   | $l$     | $b$     | $\theta_1$ | $\theta_2$ | $\phi$ | $\sigma$ | $F_{35}$ | $\Delta F_{35}$ | $S_{25}$ | $\Delta S_{25}$ | $\Gamma_{25}$ | $\Delta \Gamma_{25}$ | Mod | Var | Flags | $\gamma$ -ray Assoc.                                   | TeV | Class               | ID or Assoc.        | Ref. |
|---------------|--------|---------|---------|---------|------------|------------|--------|----------|----------|-----------------|----------|-----------------|---------------|----------------------|-----|-----|-------|--------------------------------------------------------|-----|---------------------|---------------------|------|
|               |        |         |         |         |            |            |        |          |          |                 |          |                 |               |                      |     |     |       | 0FGL J0238.6+1636<br>3EG J0237+1635                    |     |                     |                     |      |
| J0239.5+1324  | 39.887 | 13.413  | 159.241 | -41.712 | 0.100      | 0.089      | 80     | 6.1      | 0.7      | 0.1             | 8.1      | 1.7             | 1.96          | 0.15                 | PL  | ... | ...   | 1FGL J0239.5+1324                                      | ... | ...                 | ...                 | ...  |
| J0240.5+6113  | 40.130 | 61.225  | 135.677 | 1.082   | 0.013      | 0.013      | 13     | 134.0    | 47.8     | 0.8             | 499.5    | 6.5             | 2.30          | ...                  | LP  | T   | ...   | 1FGL J0240.5+6113                                      | P   | HMB                 | LS I+61 303         | ...  |
|               |        |         |         |         |            |            |        |          |          |                 |          |                 |               |                      |     |     |       | 0FGL J0240.3+6113<br>EGR J0240+6112<br>1AGL J0242+6111 |     |                     |                     |      |
| J0241.3+6548  | 40.335 | 65.808  | 133.878 | 5.300   | 0.079      | 0.063      | -7     | 7.6      | 1.1      | 0.2             | 12.6     | 2.3             | 1.97          | 0.16                 | PL  | ... | ...   | ...                                                    | ... | agu                 | NVSS J024121+654311 | ...  |
| J0242.5+0006  | 40.650 | 0.104   | 171.953 | -51.860 | 0.161      | 0.123      | 8      | 5.6      | 0.5      | 0.1             | 5.7      | 1.2             | 2.15          | 0.17                 | PL  | ... | ...   | 1FGL J0242.7+0007                                      | ... | sbq                 | NGC 1068            | ...  |
| J0242.9+7118  | 40.726 | 71.313  | 131.689 | 10.361  | 0.091      | 0.088      | 54     | 5.6      | 0.7      | 0.2             | 8.4      | 1.9             | 1.90          | 0.16                 | PL  | ... | ...   | 1FGL J0243.5+7116                                      | ... | bzb                 | S5 0238+711         | ...  |
| J0245.1+2406  | 41.295 | 24.113  | 153.716 | -31.873 | 0.148      | 0.130      | 87     | 11.3     | 1.1      | 0.2             | 17.2     | 1.7             | 2.54          | 0.08                 | PL  | T   | ...   | 1FGL J0245.4+2413                                      | ... | bzq                 | B2 0242+23          | ...  |
| J0245.9-4652  | 41.478 | -46.871 | 261.871 | -60.099 | 0.040      | 0.039      | -70    | 48.2     | 4.5      | 0.3             | 62.0     | 2.1             | 2.43          | 0.03                 | PL  | T   | ...   | 1FGL J0245.9-4652                                      | ... | bzq                 | PKS 0244-470        | ...  |
|               |        |         |         |         |            |            |        |          |          |                 |          |                 |               |                      |     |     |       | 0FGL J0245.6-4656                                      |     |                     |                     |      |
| J0248.1+6021  | 42.042 | 60.357  | 136.888 | 0.687   | 0.064      | 0.063      | -9     | 17.3     | 5.0      | 0.4             | 47.4     | 4.2             | 2.48          | ...                  | EC  | T   | ...   | 1FGL J0248.3+6021                                      | ... | PSR                 | PSR J0248+6021      | ...  |
| J0248.5+5131  | 42.130 | 51.523  | 140.791 | -7.243  | 0.105      | 0.084      | 89     | 6.5      | 0.9      | 0.2             | 10.2     | 2.2             | 1.87          | 0.15                 | PL  | ... | ...   | 1FGL J0248.7+5127                                      | ... | ...                 | ...                 | ...  |
| J0248.6+8440  | 42.164 | 84.671  | 125.752 | 22.453  | 0.144      | 0.118      | 13     | 4.8      | 0.4      | 0.1             | 5.1      | 1.5             | 1.78          | 0.18                 | PL  | ... | ...   | ...                                                    | agu | NVSS J024948+843556 | ...                 |      |
| J0250.6+1713  | 42.662 | 17.222  | 159.437 | -37.060 | 0.066      | 0.059      | -9     | 9.1      | 1.0      | 0.2             | 11.6     | 2.2             | 1.84          | 0.17                 | PL  | ... | ...   | 1FGL J0250.4+1715                                      | ... | bzq                 | NVSS J025037+171209 | ...  |
| J0250.7+5631  | 42.691 | 56.525  | 138.875 | -2.607  | 0.119      | 0.099      | -89    | 5.5      | 1.1      | 0.2             | 12.4     | 2.4             | 2.25          | 0.13                 | PL  | ... | 4     | 1FGL J0251.5+5634                                      | ... | agu                 | NVSS J025047+562935 | ...  |
| J0251.0+2557  | 42.761 | 25.966  | 153.962 | -29.603 | 0.163      | 0.150      | 23     | 4.5      | 0.5      | 0.1             | 6.5      | 1.4             | 2.35          | 0.14                 | PL  | ... | ...   | ...                                                    | ... | ...                 | ...                 | ...  |
| J0252.7-2218  | 43.195 | -22.313 | 209.724 | -62.096 | 0.039      | 0.036      | 60     | 46.0     | 5.0      | 0.3             | 56.1     | 2.4             | 2.33          | ...                  | LP  | T   | ...   | 1FGL J0252.8-2219                                      | ... | bzq                 | PKS 0250-225        | ...  |
| J0253.4+3218  | 43.360 | 32.313  | 150.902 | -23.849 | 0.078      | 0.069      | -80    | 8.5      | 0.9      | 0.2             | 10.7     | 1.9             | 1.92          | 0.12                 | PL  | T   | ...   | ...                                                    | agu | MG3 J025334+3217    | ...                 |      |
| J0253.5+5107  | 43.391 | 51.122  | 141.682 | -7.249  | 0.092      | 0.082      | -67    | 11.3     | 1.8      | 0.2             | 24.2     | 2.3             | 2.44          | 0.07                 | PL  | T   | ...   | 1FGL J0254.2+5107                                      | ... | bzq                 | NVSS J025357+510256 | ...  |
| J0253.9+5908  | 43.476 | 59.135  | 138.078 | -0.087  | 0.186      | 0.184      | 61     | 5.0      | 1.1      | 0.2             | 14.9     | 2.8             | 2.38          | 0.11                 | PL  | ... | 4     | ...                                                    | ... | ...                 | ...                 | ...  |
| J0257.7-1213  | 44.438 | -12.229 | 192.454 | -56.886 | 0.184      | 0.159      | -17    | 6.4      | 0.5      | 0.1             | 7.2      | 1.2             | 2.39          | 0.14                 | PL  | T   | ...   | 1FGL J0257.8-1204                                      | ... | bzq                 | PB 09399            | ...  |
| J0257.9+2025c | 44.480 | 20.423  | 159.006 | -33.443 | 0.141      | 0.111      | 30     | 4.1      | 0.7      | 0.2             | 7.7      | 1.8             | 2.19          | 0.17                 | PL  | ... | 6     | 1FGL J0258.0+2033                                      | ... | bzb                 | MG3 J025805+2029    | ...  |
| J0259.5+0740  | 44.900 | 7.682   | 169.255 | -43.369 | 0.151      | 0.139      | -12    | 5.3      | 0.6      | 0.1             | 8.3      | 1.6             | 2.39          | 0.14                 | PL  | T   | ...   | 1FGL J0259.5+0743                                      | ... | bzq                 | PKS 0256+075        | ...  |
| J0302.7-7919  | 45.679 | -79.325 | 295.811 | -35.919 | 0.128      | 0.118      | -76    | 6.6      | 0.6      | 0.1             | 7.3      | 1.4             | 2.20          | 0.13                 | PL  | T   | ...   | ...                                                    | ... | PMN J0303-7914      | ...                 |      |
| J0303.4-2407  | 45.868 | -24.128 | 214.641 | -60.172 | 0.026      | 0.025      | -86    | 47.0     | 6.7      | 0.3             | 76.6     | 4.2             | 1.94          | 0.03                 | PL  | T   | ...   | 1FGL J0303.5-2406                                      | ... | bzb                 | PKS 0301-243        | ...  |
|               |        |         |         |         |            |            |        |          |          |                 |          |                 |               |                      |     |     |       | 0FGL J0303.7-2410                                      |     |                     |                     |      |
| J0303.5+4713  | 45.879 | 47.219  | 145.001 | -9.914  | 0.063      | 0.059      | -20    | 14.2     | 1.8      | 0.2             | 21.6     | 2.0             | 2.24          | 0.07                 | PL  | T   | ...   | 1FGL J0303.1+4711                                      | ... | bzb                 | 4C +47.08           | ...  |
| J0303.5-6209  | 45.883 | -62.161 | 280.233 | -48.736 | 0.088      | 0.079      | -67    | 13.6     | 1.1      | 0.1             | 16.1     | 1.5             | 2.48          | 0.08                 | PL  | T   | ...   | 1FGL J0303.4-6209                                      | ... | bzq                 | PKS 0302-623        | ...  |
| J0303.5+6822  | 45.887 | 68.370  | 134.655 | 8.559   | 0.166      | 0.115      | -53    | 8.3      | 0.9      | 0.2             | 18.4     | 2.2             | 2.77          | 0.11                 | PL  | ... | 4     | ...                                                    | ... | agu                 | TXS 0259+681        | ...  |
| J0304.5-2836  | 46.142 | -28.606 | 223.680 | -60.634 | 0.092      | 0.081      | -45    | 6.0      | 0.4      | 0.1             | 5.5      | 1.9             | 1.62          | 0.21                 | PL  | ... | ...   | ...                                                    | ... | bzb                 | RBS 0385            | ...  |
| J0305.0-1602  | 46.259 | -16.036 | 200.151 | -57.146 | 0.122      | 0.098      | -30    | 5.3      | 0.3      | 0.1             | 5.6      | 2.0             | 1.50          | 0.22                 | PL  | ... | ...   | 1FGL J0305.2-1601                                      | ... | ...                 | ...                 | ...  |
| J0307.4+4915  | 46.858 | 49.254  | 144.550 | -7.825  | 0.073      | 0.063      | -88    | 9.4      | 1.4      | 0.2             | 15.8     | 2.3             | 2.02          | 0.10                 | PL  | ... | ...   | 1FGL J0307.5+4916                                      | ... | ...                 | ...                 | ...  |

Table 1—Continued

| Name 2FGL     | R.A.   | Decl.   | $l$     | $b$     | $\theta_1$ | $\theta_2$ | $\phi$ | $\sigma$ | $F_{35}$ | $\Delta F_{35}$ | $S_{25}$ | $\Delta S_{25}$ | $\Gamma_{25}$ | $\Delta \Gamma_{25}$ | Mod | Var | Flags    | $\gamma$ -ray Assoc. | TeV | Class | ID or Assoc.          | Ref. |
|---------------|--------|---------|---------|---------|------------|------------|--------|----------|----------|-----------------|----------|-----------------|---------------|----------------------|-----|-----|----------|----------------------|-----|-------|-----------------------|------|
| J0308.3+7442  | 47.080 | 74.709  | 131.734 | 14.227  | 0.061      | 0.059      | 66     | 15.2     | 2.8      | 0.3             | 11.6     | 1.0             | 2.07          | ...                  | LP  | ... | 12       | 1FGL J0308.6+7442    | ... | psr   | PSR J0308+7442        | ...  |
| J0308.7+5954  | 47.180 | 59.916  | 139.355 | 1.496   | 0.202      | 0.170      | 65     | 4.4      | 1.0      | 0.2             | 12.0     | 2.6             | 2.23          | 0.13                 | PL  | ... | 4        | ...                  | ... | ...   | ...                   | ...  |
| J0309.1+1027  | 47.290 | 10.459  | 169.229 | -39.725 | 0.090      | 0.084      | -5     | 10.7     | 1.5      | 0.2             | 17.9     | 2.0             | 2.26          | 0.08                 | PL  | T   | ...      | ...                  | ... | bzq   | PKS 0306+102          | ...  |
| J0309.3-0743  | 47.337 | -7.731  | 188.677 | -52.030 | 0.107      | 0.098      | -64    | 4.2      | 0.3      | 0.1             | 5.2      | 2.0             | 1.56          | 0.22                 | PL  | ... | ...      | ...                  | ... | agu   | NVSS J030943-074427   | ...  |
| J0310.0-6058  | 47.523 | -60.980 | 278.103 | -48.925 | 0.088      | 0.086      | 29     | 13.9     | 1.1      | 0.1             | 17.3     | 1.5             | 2.56          | 0.08                 | PL  | T   | ...      | 1FGL J0310.1-6058    | ... | bzq   | PKS 0308-611          | ...  |
| J0310.2-5013  | 47.570 | -50.230 | 263.583 | -54.934 | 0.087      | 0.081      | 23     | 7.3      | 0.6      | 0.1             | 7.4      | 1.9             | 1.74          | 0.15                 | PL  | T   | ...      | ...                  | ... | agu   | SUMSS J031034-501633  | ...  |
| J0310.7+3813  | 47.692 | 38.221  | 150.912 | -16.966 | 0.136      | 0.110      | -79    | 5.0      | 0.6      | 0.1             | 6.9      | 1.5             | 2.25          | 0.16                 | PL  | T   | ...      | 1FGL J0310.6+3812    | ... | bzq   | B3 0307+38            | ...  |
| J0312.5-0914  | 48.141 | -9.250  | 191.452 | -52.220 | 0.141      | 0.105      | 39     | 5.8      | 0.7      | 0.1             | 7.6      | 1.5             | 2.22          | 0.14                 | PL  | ... | 2        | ...                  | ... | ...   | ...                   | ...  |
| J0312.6+0132  | 48.166 | 1.546   | 178.506 | -45.539 | 0.085      | 0.070      | 43     | 13.2     | 1.5      | 0.2             | 17.4     | 1.7             | 2.26          | 0.08                 | PL  | T   | ...      | 1FGL J0312.6+0131    | ... | bzq   | PKS 0310+013          | ...  |
| J0312.8+2013  | 48.203 | 20.228  | 162.507 | -31.569 | 0.100      | 0.098      | -12    | 4.4      | 0.4      | 0.1             | 5.6      | 1.8             | 1.70          | 0.23                 | PL  | ... | ...      | ...                  | ... | ...   | ...                   | ...  |
| J0314.2-5106  | 48.565 | -51.103 | 264.399 | -53.966 | 0.148      | 0.127      | -4     | 6.2      | 0.6      | 0.1             | 6.8      | 1.3             | 2.24          | 0.16                 | PL  | T   | ...      | 1FGL J0315.6-5109    | ... | bzb   | PMN J0314-5104        | ...  |
| J0315.8-1024  | 48.969 | -10.403 | 193.753 | -52.141 | 0.143      | 0.131      | -31    | 6.6      | 0.8      | 0.1             | 8.5      | 1.5             | 2.18          | 0.13                 | PL  | T   | ...      | 1FGL J0315.9-1033    | ... | bzq   | PKS 0313-107          | ...  |
| J0315.8-2611  | 48.973 | -26.185 | 219.636 | -57.822 | 0.113      | 0.091      | 7      | 7.5      | 0.6      | 0.1             | 7.5      | 1.7             | 1.87          | 0.14                 | PL  | ... | ...      | 1FGL J0315.9-2609    | ... | bzb   | RBS 0405              | ...  |
| J0316.1-6434  | 49.031 | -64.568 | 281.500 | -46.081 | 0.115      | 0.103      | -35    | 7.9      | 0.7      | 0.1             | 8.1      | 1.5             | 1.98          | 0.15                 | PL  | ... | ...      | 1FGL J0316.3-6438    | ... | ...   | ...                   | ...  |
| J0316.1+0904  | 49.048 | 9.082   | 172.098 | -39.592 | 0.050      | 0.048      | 78     | 15.9     | 2.3      | 0.2             | 28.2     | 3.4             | 1.81          | 0.07                 | PL  | T   | ...      | 1FGL J0316.1+0904    | ... | bzb   | GB6 J0316+0904        | ...  |
| J0316.6+4119  | 49.169 | 41.322  | 150.179 | -13.741 | 0.072      | 0.070      | -65    | 4.4      | 0.9      | 0.2             | 9.8      | 2.6             | 2.10          | 0.19                 | PL  | ... | 5        | ...                  | P   | rdg   | IC 310 $\infty$       | ...  |
| J0318.0+0255  | 49.508 | 2.927   | 178.361 | -43.617 | 0.131      | 0.100      | 80     | 6.8      | 0.8      | 0.2             | 9.2      | 1.6             | 2.13          | 0.12                 | PL  | ... | ...      | 1FGL J0318.1+0254    | ... | ...   | ...                   | ...  |
| J0319.6+1849  | 49.909 | 18.827  | 165.009 | -31.679 | 0.063      | 0.054      | -69    | 11.5     | 1.1      | 0.2             | 17.0     | 3.3             | 1.55          | 0.11                 | PL  | T   | ...      | 1FGL J0319.7+1847    | P   | bzb   | RBS 0413              | ...  |
| J0319.8+4130  | 49.965 | 41.513  | 150.585 | -13.254 | 0.017      | 0.017      | -41    | 65.1     | 18.8     | 0.5             | 173.7    | 6.2             | 2.03          | ...                  | LP  | T   | ...      | 1FGL J0319.7+4130    | P   | rdg   | NGC 1275              | ...  |
|               |        |         |         |         |            |            |        |          |          |                 |          |                 |               |                      |     |     |          | 0FGL J0320.0+4131    |     |       |                       |      |
| J0322.0+2336  | 50.516 | 23.611  | 162.096 | -27.579 | 0.065      | 0.053      | 27     | 11.4     | 1.4      | 0.2             | 15.8     | 2.0             | 2.09          | 0.12                 | PL  | ... | ...      | 1FGL J0322.1+2336    | ... | bzb   | MG3 J032201+2336      | ...  |
| J0322.4-3717  | 50.600 | -37.292 | 240.326 | -56.738 | 0.202      | 0.181      | -74    | 5.6      | 0.5      | 0.1             | 6.0      | 1.2             | 2.16          | 0.15                 | PL  | ... | ...      | ...                  | ... | rdg   | For A                 | ...  |
| J0323.6-0108  | 50.900 | -1.150  | 183.955 | -45.230 | 0.112      | 0.097      | 62     | 7.1      | 0.5      | 0.1             | 9.0      | 2.6             | 1.49          | 0.18                 | PL  | ... | ...      | 1FGL J0323.7-0106    | ... | bzb   | BZB J0323-0111        | ...  |
| J0324.8+3408  | 51.210 | 34.143  | 155.777 | -18.768 | 0.154      | 0.150      | -88    | 10.1     | 0.3      | 0.1             | 14.2     | 1.6             | 2.79          | ...                  | LP  | T   | ...      | 1FGL J0325.0+3403    | ... | sey   | 1H 0323+342           | ...  |
| J0325.1-5635  | 51.295 | -56.587 | 270.857 | -49.863 | 0.111      | 0.099      | 47     | 6.8      | 0.6      | 0.1             | 6.6      | 1.2             | 2.19          | 0.16                 | PL  | ... | ...      | 1FGL J0325.6-5626    | ... | agu   | 1RXS J032521.8-563543 | ...  |
| J0325.6-1650  | 51.424 | -16.836 | 204.968 | -52.951 | 0.164      | 0.128      | -88    | 6.7      | 0.7      | 0.1             | 7.8      | 1.7             | 1.97          | 0.16                 | PL  | T   | ...      | 1FGL J0325.9-1649    | ... | bzb   | RBS 0421              | ...  |
| J0326.1+2226  | 51.536 | 22.439  | 163.751 | -27.914 | 0.144      | 0.130      | 86     | 15.2     | 1.1      | 0.2             | 24.0     | 2.0             | 2.70          | ...                  | LP  | T   | ...      | 1FGL J0325.9+2219    | ... | bzq   | TXS 0322+222          | ...  |
| J0326.1+0224  | 51.545 | 2.413   | 180.744 | -42.446 | 0.076      | 0.069      | -55    | 10.8     | 1.3      | 0.2             | 14.3     | 2.0             | 2.06          | 0.10                 | PL  | T   | ...      | 1FGL J0326.2+0222    | ... | bzb   | 1H 0323+022           | ...  |
| J0330.3+5816c | 52.584 | 58.271  | 142.580 | 1.596   | 0.182      | 0.144      | -88    | 6.7      | 0.7      | 0.2             | 15.7     | 2.2             | 2.47          | ...                  | LP  | ... | 1,4,6,12 | ...                  | ... | ...   | ...                   | ...  |
| J0332.1+6309  | 53.031 | 63.156  | 139.955 | 5.726   | 0.097      | 0.074      | -33    | 5.5      | 0.9      | 0.2             | 10.4     | 2.2             | 2.07          | 0.13                 | PL  | ... | ...      | 1FGL J0332.0+6310    | ... | ...   | ...                   | ...  |
| J0332.5-1118  | 53.132 | -11.305 | 198.199 | -49.047 | 0.174      | 0.135      | 82     | 5.1      | 0.5      | 0.1             | 6.0      | 1.2             | 2.41          | 0.15                 | PL  | T   | ...      | ...                  | ... | agu   | NVSS J033223-111951   | ...  |
| J0333.7+2918  | 53.431 | 29.308  | 160.486 | -21.487 | 0.070      | 0.064      | -49    | 10.5     | 1.5      | 0.2             | 16.8     | 2.4             | 1.92          | 0.10                 | PL  | ... | ...      | 1FGL J0333.7+2919    | ... | agu   | TXS 0330+291          | ...  |
| J0334.2-4008  | 53.560 | -40.148 | 244.777 | -54.072 | 0.038      | 0.036      | 9      | 38.3     | 4.3      | 0.3             | 49.3     | 2.5             | 2.19          | 0.04                 | PL  | T   | ...      | 1FGL J0334.2-4010    | ... | bzb   | PKS 0332-403          | ...  |
|               |        |         |         |         |            |            |        |          |          |                 |          |                 |               |                      |     |     |          | 0FGL J0334.1-4006    |     |       |                       |      |
| J0334.3+6538  | 53.579 | 65.640  | 138.694 | 7.884   | 0.075      | 0.073      | 19     | 6.3      | 0.8      | 0.2             | 10.2     | 2.2             | 1.82          | 0.14                 | PL  | ... | ...      | 1FGL J0334.3+6536    | ... | agu   | TXS 0329+654          | ...  |



Table 1—Continued

| Name 2FGL     | R.A.   | Decl.   | $l$     | $b$     | $\theta_1$ | $\theta_2$ | $\phi$ | $\sigma$ | $F_{35}$ | $\Delta F_{35}$ | $S_{25}$ | $\Delta S_{25}$ | $\Gamma_{25}$ | $\Delta \Gamma_{25}$ | Mod | Var | Flags | $\gamma$ -ray Assoc. | TeV | Class | ID or Assoc.          | Ref. |
|---------------|--------|---------|---------|---------|------------|------------|--------|----------|----------|-----------------|----------|-----------------|---------------|----------------------|-----|-----|-------|----------------------|-----|-------|-----------------------|------|
| J0334.3–3728  | 53.585 | –37.469 | 240.220 | –54.361 | 0.052      | 0.048      | –60    | 28.3     | 3.4      | 0.2             | 38.3     | 2.9             | 1.99          | 0.05                 | PL  | T   | ...   | 1FGL J0334.4–3727    | ... | bzb   | PMN J0334–3725        | ...  |
| J0335.3–4501  | 53.846 | –45.029 | 252.743 | –52.883 | 0.074      | 0.068      | –76    | 9.0      | 0.7      | 0.1             | 8.3      | 1.7             | 1.84          | 0.13                 | PL  | ... | ...   | 1FGL J0335.5–4501    | ... | agu   | 1RXS J033514.5–445929 | ...  |
| J0336.0+7504  | 54.002 | 75.079  | 133.060 | 15.548  | 0.093      | 0.075      | –57    | 9.2      | 1.1      | 0.2             | 12.0     | 1.6             | 2.15          | 0.09                 | PL  | ... | ...   | 1FGL J0334.2+7501    | ... | ...   | ...                   | ...  |
| J0337.0+3200c | 54.273 | 32.014  | 159.296 | –18.918 | 0.203      | 0.182      | –14    | 6.7      | 1.1      | 0.2             | 18.0     | 2.6             | 2.59          | 0.10                 | PL  | ... | 6     | ...                  | ... | bzq   | NRAO 140              | ...  |
| J0338.2+1306  | 54.570 | 13.115  | 173.470 | –32.929 | 0.106      | 0.095      | 8      | 5.8      | 0.6      | 0.2             | 9.6      | 2.7             | 1.54          | 0.17                 | PL  | T   | ...   | ...                  | ... | ...   | ...                   | ...  |
| J0339.2–1734  | 54.824 | –17.579 | 208.052 | –50.226 | 0.092      | 0.082      | –2     | 6.3      | 0.6      | 0.1             | 7.4      | 1.8             | 1.83          | 0.16                 | PL  | ... | ...   | 1FGL J0339.1–1734    | ... | agn   | PKS 0336–177          | ...  |
| J0339.4–0144  | 54.871 | –1.744  | 187.959 | –42.441 | 0.108      | 0.099      | 21     | 14.0     | 1.3      | 0.2             | 19.3     | 1.6             | 2.48          | 0.07                 | PL  | T   | ...   | 1FGL J0339.2–0143    | ... | bzq   | PKS 0336–01           | ...  |
|               |        |         |         |         |            |            |        |          |          |                 |          |                 |               |                      |     |     |       | 3EG J0340–0201       |     |       |                       |      |
|               |        |         |         |         |            |            |        |          |          |                 |          |                 |               |                      |     |     |       | EGR J0338–0203       |     |       |                       |      |
| J0340.4+4131  | 55.103 | 41.528  | 153.778 | –11.007 | 0.054      | 0.050      | 45     | 20.3     | 3.9      | 0.3             | 20.8     | 1.8             | 1.98          | ...                  | EC  | ... | ...   | 1FGL J0340.4+4130    | ... | PSR   | PSR J0340+4130        | ...  |
| J0340.5+5307  | 55.149 | 53.131  | 146.755 | –1.731  | 0.146      | 0.124      | 84     | 16.3     | 0.7      | 0.2             | 40.1     | 2.7             | 2.83          | ...                  | LP  | ... | ...   | 1FGL J0341.5+5304    | ... | ...   | ...                   | ...  |
| J0340.6–2113  | 55.152 | –21.230 | 213.651 | –51.149 | 0.164      | 0.134      | 1      | 6.7      | 0.5      | 0.1             | 7.5      | 1.3             | 2.43          | 0.14                 | PL  | ... | ...   | ...                  | ... | bzb   | PKS 0338–214          | ...  |
| J0340.7–2421  | 55.187 | –24.353 | 218.508 | –51.949 | 0.172      | 0.143      | –45    | 4.2      | 0.4      | 0.1             | 4.7      | 1.2             | 2.23          | 0.21                 | PL  | ... | ...   | ...                  | ... | ...   | ...                   | ...  |
| J0341.8+3148c | 55.466 | 31.806  | 160.265 | –18.443 | 0.130      | 0.099      | 80     | 7.6      | 1.6      | 0.2             | 19.5     | 2.8             | 2.31          | 0.09                 | PL  | ... | 6     | ...                  | ... | ...   | ...                   | ...  |
| J0342.4+3859  | 55.603 | 38.986  | 155.682 | –12.778 | 0.087      | 0.071      | –64    | 9.3      | 1.1      | 0.2             | 13.7     | 1.8             | 2.31          | 0.10                 | PL  | T   | ...   | 1FGL J0342.2+3859    | ... | bzq   | GB6 J0342+3858        | ...  |
| J0345.2–2356  | 56.317 | –23.944 | 218.266 | –50.850 | 0.114      | 0.108      | –15    | 9.6      | 0.8      | 0.1             | 11.4     | 1.5             | 2.47          | 0.10                 | PL  | T   | ...   | 1FGL J0345.2–2355    | ... | ...   | ...                   | ...  |
| J0348.6–2750  | 57.152 | –27.849 | 224.570 | –50.920 | 0.123      | 0.099      | 5      | 8.4      | 0.6      | 0.1             | 8.0      | 1.2             | 2.32          | 0.13                 | PL  | ... | ...   | 1FGL J0348.5–2751    | ... | bzq   | PKS 0346–27           | ...  |
| J0350.0–2104  | 57.518 | –21.073 | 214.448 | –48.996 | 0.087      | 0.071      | 14     | 25.0     | 2.2      | 0.2             | 28.4     | 1.7             | 2.47          | ...                  | LP  | T   | ...   | 1FGL J0349.9–2104    | ... | bzq   | PKS 0347–211          | ...  |
|               |        |         |         |         |            |            |        |          |          |                 |          |                 |               |                      |     |     |       | 0FGL J0349.8–2102    |     |       |                       |      |
| J0353.2+5653  | 58.321 | 56.889  | 145.867 | 2.347   | 0.162      | 0.109      | 90     | 4.6      | 0.8      | 0.2             | 9.4      | 2.2             | 2.11          | 0.14                 | PL  | ... | ...   | 1FGL J0352.8+5658    | ... | ...   | ...                   | ...  |
| J0354.1+8010  | 58.540 | 80.169  | 130.405 | 20.067  | 0.081      | 0.068      | –56    | 12.3     | 1.2      | 0.1             | 13.7     | 1.4             | 2.25          | 0.08                 | PL  | T   | ...   | 1FGL J0354.6+8009    | ... | bzb   | S5 0346+80            | ...  |
| J0357.0–4950  | 59.257 | –49.845 | 258.567 | –48.100 | 0.119      | 0.104      | –77    | 4.9      | 0.4      | 0.1             | 4.8      | 1.5             | 1.74          | 0.18                 | PL  | ... | ...   | 1FGL J0357.1–4949    | ... | bzb   | PKS 0355–500          | ...  |
| J0357.8+3205  | 59.472 | 32.097  | 162.758 | –15.999 | 0.037      | 0.036      | –71    | 49.7     | 8.7      | 0.4             | 65.2     | 2.1             | 2.21          | ...                  | EC  | ... | ...   | 1FGL J0357.8+3205    | ... | PSR   | LAT PSR J0357+3205    | ...  |
|               |        |         |         |         |            |            |        |          |          |                 |          |                 |               |                      |     |     |       | 0FGL J0357.5+3205    |     |       |                       |      |
| J0359.1+6003  | 59.775 | 60.055  | 144.408 | 5.259   | 0.110      | 0.097      | 86     | 8.8      | 1.5      | 0.2             | 18.4     | 2.3             | 2.30          | 0.08                 | PL  | T   | ...   | ...                  | ... | bzq   | TXS 0354+599          | ...  |
| J0359.5+5410  | 59.891 | 54.180  | 148.291 | 0.844   | 0.071      | 0.067      | –46    | 13.5     | 3.8      | 0.4             | 25.8     | 2.6             | 2.25          | ...                  | LP  | ... | ...   | 1FGL J0359.5+5410    | ... | ...   | ...                   | ...  |
| J0401.6–3153  | 60.418 | –31.890 | 231.371 | –48.663 | 0.396      | 0.193      | –84    | 4.5      | 0.3      | 0.1             | 4.9      | 1.1             | 2.52          | 0.22                 | PL  | ... | 8,9   | 1FGL J0401.3–3152    | ... | bzq   | PKS 0400–319          | ...  |
| J0402.0–2616  | 60.500 | –26.281 | 223.080 | –47.694 | 0.131      | 0.109      | –17    | 5.7      | 0.5      | 0.1             | 5.7      | 1.2             | 2.13          | 0.16                 | PL  | ... | ...   | 1FGL J0402.1–2618    | ... | bzb   | PKS 0359–264          | ...  |
| J0403.9–3604  | 60.986 | –36.070 | 237.722 | –48.473 | 0.038      | 0.036      | –33    | 66.5     | 5.6      | 0.3             | 83.4     | 2.2             | 2.51          | ...                  | LP  | T   | ...   | 1FGL J0403.9–3603    | ... | bzq   | PKS 0402–362          | ...  |
| J0404.0+3843  | 61.019 | 38.724  | 159.136 | –10.248 | 0.211      | 0.187      | –36    | 4.5      | 0.7      | 0.2             | 10.7     | 2.1             | 2.56          | 0.15                 | PL  | ... | 4     | ...                  | ... | ...   | ...                   | ...  |
| J0404.6+5822  | 61.174 | 58.367  | 146.066 | 4.463   | 0.182      | 0.158      | –39    | 4.5      | 0.8      | 0.2             | 10.6     | 2.2             | 2.44          | 0.13                 | PL  | ... | 4     | ...                  | ... | ...   | ...                   | ...  |
| J0405.8–1309  | 61.454 | –13.165 | 205.833 | –42.610 | 0.163      | 0.155      | 2      | 5.0      | 0.5      | 0.1             | 5.8      | 1.2             | 2.35          | 0.16                 | PL  | ... | ...   | 1FGL J0405.6–1309    | ... | bzq   | PKS 0403–13           | ...  |
| J0407.3–3826  | 61.825 | –38.436 | 241.279 | –47.828 | 0.068      | 0.062      | –78    | 21.4     | 2.0      | 0.2             | 25.1     | 1.7             | 2.34          | 0.06                 | PL  | T   | ...   | 1FGL J0407.4–3827    | ... | bzq   | PKS 0405–385          | ...  |
|               |        |         |         |         |            |            |        |          |          |                 |          |                 |               |                      |     |     |       | 0FGL J0407.6–3829    |     |       |                       |      |
| J0407.7+0740  | 61.929 | 7.682   | 183.932 | –31.124 | 0.172      | 0.166      | 59     | 5.9      | 0.7      | 0.2             | 9.9      | 1.7             | 2.44          | 0.14                 | PL  | ... | ...   | 1FGL J0407.5+0749    | ... | bzq   | TXS 0404+075          | ...  |

Table 1—Continued

| Name 2FGL     | R.A.   | Decl.   | $l$     | $b$     | $\theta_1$ | $\theta_2$ | $\phi$ | $\sigma$ | $F_{35}$ | $\Delta F_{35}$ | $S_{25}$ | $\Delta S_{25}$ | $\Gamma_{25}$ | $\Delta \Gamma_{25}$ | Mod | Var | Flags | $\gamma$ -ray Assoc.                                     | TeV | Class | ID or Assoc.     | Ref. |
|---------------|--------|---------|---------|---------|------------|------------|--------|----------|----------|-----------------|----------|-----------------|---------------|----------------------|-----|-----|-------|----------------------------------------------------------|-----|-------|------------------|------|
| J0409.5+0509  | 62.388 | 5.157   | 186.614 | -32.299 | 0.147      | 0.137      | -81    | 5.4      | 0.6      | 0.1             | 9.5      | 1.8             | 2.54          | 0.14                 | PL  | ... | ...   | ...                                                      | ... | ...   | ...              | ...  |
| J0409.8-0357  | 62.464 | -3.966  | 195.867 | -37.367 | 0.101      | 0.095      | -13    | 7.6      | 0.8      | 0.1             | 8.9      | 1.5             | 2.14          | 0.14                 | PL  | T   | ...   | 1FGL J0409.9-0357                                        | ... | ...   | ...              | ...  |
| J0413.5-5332  | 63.384 | -53.549 | 262.782 | -44.664 | 0.087      | 0.076      | 72     | 13.9     | 1.1      | 0.1             | 15.3     | 1.4             | 2.41          | 0.09                 | PL  | T   | ...   | 1FGL J0413.4-5334<br>0FGL J0412.9-5341                   | ... | bzq   | PMN J0413-5332   | ...  |
| J0414.9-0855  | 63.732 | -8.921  | 202.127 | -38.722 | 0.151      | 0.143      | 10     | 4.1      | 0.3      | 0.1             | 5.8      | 2.6             | 1.41          | 0.43                 | PL  | ... | ...   | ...                                                      | ... | ...   | ...              | ...  |
| J0415.2+5518  | 63.800 | 55.301  | 149.210 | 3.190   | 0.123      | 0.118      | 4      | 5.4      | 1.1      | 0.2             | 13.2     | 2.5             | 2.29          | 0.13                 | PL  | ... | 1     | ...                                                      | ... | ...   | ...              | ...  |
| J0416.0-4355  | 64.012 | -43.931 | 249.197 | -45.921 | 0.200      | 0.155      | 44     | 5.4      | 0.4      | 0.1             | 5.6      | 1.1             | 2.37          | 0.16                 | PL  | ... | ...   | ...                                                      | ... | ...   | ...              | ...  |
| J0416.7-1849  | 64.193 | -18.830 | 214.298 | -42.335 | 0.088      | 0.075      | -88    | 12.4     | 1.2      | 0.2             | 13.5     | 1.6             | 2.20          | 0.09                 | PL  | ... | ...   | 1FGL J0416.5-1851<br>3EG J0412-1853<br>EGR J0413-1851    | ... | bzq   | PKS 0414-189     | ...  |
| J0416.8+0105  | 64.209 | 1.092   | 191.806 | -33.166 | 0.078      | 0.071      | 40     | 6.8      | 0.7      | 0.1             | 7.8      | 1.6             | 1.98          | 0.16                 | PL  | ... | ...   | 1FGL J0416.8+0107                                        | P   | bzb   | 1ES 0414+009     | ...  |
| J0418.9+6636  | 64.747 | 66.603  | 141.529 | 11.559  | 0.094      | 0.075      | -63    | 9.1      | 1.4      | 0.2             | 15.7     | 2.0             | 2.20          | 0.09                 | PL  | ... | ...   | ...                                                      | ... | ...   | ...              | ...  |
| J0420.9-3743  | 65.230 | -37.721 | 240.301 | -45.137 | 0.133      | 0.112      | 82     | 5.8      | 0.6      | 0.1             | 7.7      | 1.6             | 2.39          | 0.17                 | PL  | ... | ...   | ...                                                      | ... | ...   | ...              | ...  |
| J0422.1-0645  | 65.529 | -6.757  | 200.791 | -36.128 | 0.105      | 0.102      | 79     | 7.5      | 0.7      | 0.1             | 9.1      | 1.4             | 2.39          | 0.12                 | PL  | T   | ...   | 1FGL J0422.0-0647                                        | ... | bzq   | PMN J0422-0643   | ...  |
| J0423.2-0120  | 65.807 | -1.342  | 195.285 | -33.147 | 0.033      | 0.031      | -62    | 46.4     | 6.6      | 0.3             | 80.6     | 2.9             | 2.30          | 0.03                 | PL  | T   | ...   | 1FGL J0423.2-0118<br>0FGL J0423.1-0112<br>3EG J0422-0102 | ... | BZQ   | PKS 0420-01      | ...  |
| J0423.4+5612  | 65.862 | 56.206  | 149.400 | 4.649   | 0.194      | 0.126      | -56    | 4.5      | 0.6      | 0.2             | 8.4      | 2.4             | 1.70          | 0.29                 | PL  | ... | 9     | ...                                                      | ... | ...   | ...              | ...  |
| J0423.8+4149  | 65.953 | 41.829  | 159.694 | -5.402  | 0.037      | 0.035      | -71    | 17.8     | 2.9      | 0.3             | 36.3     | 3.8             | 1.80          | 0.06                 | PL  | ... | ...   | 1FGL J0423.8+4148                                        | ... | bzb   | 4C +41.11        | ...  |
| J0424.3-5332  | 66.100 | -53.538 | 262.235 | -43.099 | 0.170      | 0.124      | -84    | 6.4      | 0.6      | 0.1             | 6.2      | 1.2             | 2.13          | 0.18                 | PL  | ... | ...   | ...                                                      | ... | agu   | PMN J0425-5331   | ...  |
| J0424.7+0034  | 66.193 | 0.572   | 193.615 | -31.795 | 0.084      | 0.075      | -5     | 15.2     | 1.9      | 0.2             | 22.6     | 2.0             | 2.30          | 0.07                 | PL  | T   | ...   | 1FGL J0424.8+0036                                        | ... | bzb   | PKS 0422+00      | ...  |
| J0426.6+0509c | 66.669 | 5.155   | 189.515 | -28.844 | 0.216      | 0.161      | -31    | 7.4      | 0.7      | 0.2             | 13.1     | 1.8             | 2.66          | 0.12                 | PL  | ... | 6     | 1FGL J0427.5+0515                                        | ... | bzq   | PKS 0423+051     | ...  |
| J0426.7+5434  | 66.688 | 54.581  | 150.895 | 3.852   | 0.110      | 0.089      | -57    | 17.0     | 3.0      | 0.3             | 34.7     | 2.6             | 2.41          | ...                  | LP  | ... | ...   | 1FGL J0426.5+5437                                        | ... | ...   | ...              | ...  |
| J0427.2-6705  | 66.821 | -67.097 | 279.188 | -38.595 | 0.192      | 0.128      | 87     | 6.2      | 0.5      | 0.1             | 6.8      | 1.2             | 2.40          | 0.14                 | PL  | ... | ...   | ...                                                      | ... | ...   | ...              | ...  |
| J0428.0-3845  | 67.014 | -38.762 | 241.837 | -43.779 | 0.195      | 0.123      | 14     | 6.6      | 0.7      | 0.2             | 21.5     | 3.1             | 2.95          | 0.14                 | PL  | ... | 2,5   | ...                                                      | ... | ...   | ...              | ...  |
| J0428.6-3756  | 67.171 | -37.933 | 240.701 | -43.616 | 0.014      | 0.014      | -66    | 104.7    | 31.1     | 0.7             | 286.0    | 8.3             | 2.04          | ...                  | LP  | T   | ...   | 1FGL J0428.6-3756<br>0FGL J0428.7-3755                   | ... | bzb   | PKS 0426-380     | ...  |
| J0430.2+3508c | 67.564 | 35.149  | 165.451 | -9.088  | 0.144      | 0.126      | -57    | 7.0      | 1.3      | 0.2             | 16.8     | 2.4             | 2.38          | 0.09                 | PL  | ... | 6     | 1FGL J0430.3+3511c                                       | ... | ...   | ...              | ...  |
| J0430.4-2507  | 67.605 | -25.124 | 223.623 | -41.201 | 0.112      | 0.103      | 38     | 4.5      | 0.4      | 0.1             | 4.5      | 1.2             | 2.20          | 0.19                 | PL  | ... | ...   | 1FGL J0430.4-2509                                        | ... | bzb   | PMN J0430-2507   | ...  |
| J0431.5+3622  | 67.890 | 36.381  | 164.715 | -8.059  | 0.147      | 0.105      | 57     | 4.5      | 0.9      | 0.2             | 9.7      | 2.4             | 2.11          | 0.14                 | PL  | ... | ...   | ...                                                      | ... | ...   | ...              | ...  |
| J0433.4-6029  | 68.363 | -60.484 | 270.831 | -40.176 | 0.117      | 0.107      | -2     | 11.5     | 0.9      | 0.1             | 13.0     | 1.3             | 2.49          | 0.09                 | PL  | T   | ...   | ...                                                      | ... | agu   | PKS 0432-606     | ...  |
| J0433.5+2905  | 68.389 | 29.086  | 170.518 | -12.622 | 0.042      | 0.041      | 3      | 21.6     | 4.3      | 0.3             | 47.9     | 3.4             | 2.04          | 0.05                 | PL  | T   | ...   | 1FGL J0433.5+2905<br>3EG J0433+2908<br>EGR J0433+2906    | ... | bzb   | MG2 J043337+2905 | ...  |
| J0433.7+3233  | 68.449 | 32.556  | 167.901 | -10.285 | 0.152      | 0.110      | 50     | 4.3      | 0.6      | 0.2             | 7.2      | 2.1             | 1.78          | 0.21                 | PL  | ... | 2     | 1FGL J0433.5+3230                                        | ... | bzq   | MG2 J043338+3236 | ...  |

Table 1—Continued

| Name 2FGL     | R.A.   | Decl.   | $l$     | $b$     | $\theta_1$ | $\theta_2$ | $\phi$ | $\sigma$ | $F_{35}$ | $\Delta F_{35}$ | $S_{25}$ | $\Delta S_{25}$ | $\Gamma_{25}$ | $\Delta \Gamma_{25}$ | Mod | Var | Flags | $\gamma$ -ray Assoc. | TeV | Class | ID or Assoc.           | Ref. |
|---------------|--------|---------|---------|---------|------------|------------|--------|----------|----------|-----------------|----------|-----------------|---------------|----------------------|-----|-----|-------|----------------------|-----|-------|------------------------|------|
| J0433.9–5726  | 68.478 | –57.442 | 266.943 | –40.904 | 0.097      | 0.081      | –88    | 7.3      | 0.6      | 0.1             | 7.1      | 1.8             | 1.75          | 0.16                 | PL  | ... | ...   | ...                  | ... | agu   | 1RXS J043431.8–572718  | ...  |
| J0434.1–2014  | 68.542 | –20.238 | 217.849 | –38.940 | 0.171      | 0.129      | 12     | 7.0      | 0.7      | 0.1             | 8.0      | 1.4             | 2.22          | 0.13                 | PL  | T   | ...   | 1FGL J0434.1–2018    | ... | bzb   | TXS 0431–203           | ...  |
| J0435.1–2341  | 68.775 | –23.690 | 222.187 | –39.787 | 0.213      | 0.195      | –5     | 4.2      | 0.4      | 0.1             | 5.4      | 1.2             | 2.45          | 0.17                 | PL  | ... | ...   | ...                  | ... | agu   | PMN J0434–2342         | ...  |
| J0436.2+6759  | 69.065 | 67.985  | 141.635 | 13.720  | 0.122      | 0.109      | –3     | 4.4      | 0.5      | 0.1             | 5.8      | 1.5             | 2.15          | 0.17                 | PL  | ... | ...   | ...                  | ... | agu   | GB6 J0437+6757         | ...  |
| J0437.3–4712  | 69.328 | –47.207 | 253.333 | –41.958 | 0.074      | 0.066      | 66     | 23.2     | 2.3      | 0.2             | 18.4     | 1.3             | 2.31          | ...                  | EC  | ... | ...   | 1FGL J0437.2–4715    | ... | PSR   | PSR J0437–4715         | ...  |
| J0438.0–7331  | 69.515 | –73.528 | 286.088 | –35.168 | 0.111      | 0.085      | 22     | 6.1      | 0.4      | 0.1             | 7.4      | 2.4             | 1.44          | 0.20                 | PL  | ... | ...   | ...                  | ... | ...   | ...                    | ...  |
| J0438.8–4521  | 69.722 | –45.365 | 250.843 | –41.781 | 0.097      | 0.085      | –36    | 12.0     | 1.1      | 0.1             | 12.9     | 1.4             | 2.31          | 0.09                 | PL  | T   | ...   | ...                  | ... | agu   | PKS 0437–454           | ...  |
| J0439.0–1252  | 69.760 | –12.867 | 209.809 | –35.125 | 0.216      | 0.170      | 21     | 4.4      | 0.5      | 0.1             | 5.9      | 1.3             | 2.35          | 0.17                 | PL  | ... | ...   | 1FGL J0438.8–1250    | ... | bzq   | PKS 0436–129           | ...  |
| J0439.8–1858  | 69.974 | –18.982 | 216.920 | –37.248 | 0.063      | 0.061      | –28    | 8.3      | 0.6      | 0.1             | 8.0      | 1.8             | 1.79          | 0.15                 | PL  | T   | ...   | 1FGL J0439.8–1857    | ... | ...   | ...                    | ...  |
| J0440.1–3211  | 70.026 | –32.188 | 233.361 | –40.639 | 0.194      | 0.150      | –24    | 4.3      | 0.3      | 0.1             | 5.4      | 2.2             | 1.52          | 0.21                 | PL  | ... | ...   | ...                  | ... | agu   | PKS 0437–322           | ...  |
| J0440.4+1433  | 70.104 | 14.562  | 183.324 | –20.574 | 0.167      | 0.135      | 24     | 4.5      | 0.7      | 0.2             | 9.2      | 2.0             | 2.35          | 0.14                 | PL  | ... | ...   | ...                  | ... | agu   | TXS 0437+145           | ...  |
| J0440.5+2554c | 70.146 | 25.903  | 174.044 | –13.501 | 0.236      | 0.199      | –79    | 4.9      | 1.0      | 0.2             | 13.6     | 2.5             | 2.40          | 0.11                 | PL  | ... | 2,6   | ...                  | ... | ...   | ...                    | ...  |
| J0440.9+2749  | 70.243 | 27.824  | 172.586 | –12.205 | 0.099      | 0.088      | 7      | 6.3      | 0.9      | 0.2             | 10.2     | 2.2             | 1.85          | 0.15                 | PL  | ... | ...   | 1FGL J0440.6+2748    | ... | bzb   | B2 0437+27B            | ...  |
| J0442.7–0017  | 70.686 | –0.293  | 197.212 | –28.440 | 0.039      | 0.037      | –47    | 51.3     | 5.9      | 0.3             | 81.6     | 2.5             | 2.44          | 0.03                 | PL  | T   | ...   | 1FGL J0442.7–0019    | ... | bzq   | PKS 0440–00            | ...  |
|               |        |         |         |         |            |            |        |          |          |                 |          |                 |               |                      |     |     |       | 3EG J0442–0033       |     |       |                        |      |
|               |        |         |         |         |            |            |        |          |          |                 |          |                 |               |                      |     |     |       | EGR J0442+0027       |     |       |                        |      |
| J0448.5–1633  | 72.133 | –16.550 | 215.031 | –34.456 | 0.064      | 0.062      | 82     | 9.8      | 0.9      | 0.1             | 10.7     | 1.9             | 1.91          | 0.12                 | PL  | ... | ...   | 1FGL J0448.5–1633    | ... | bzb   | RBS 0589               | ...  |
| J0448.6–2118  | 72.159 | –21.302 | 220.500 | –36.085 | 0.247      | 0.171      | –47    | 4.2      | 0.4      | 0.1             | 5.4      | 1.3             | 2.33          | 0.18                 | PL  | ... | ...   | ...                  | ... | bzq   | PKS 0446–212           | ...  |
| J0448.9+1121  | 72.243 | 11.363  | 187.400 | –20.765 | 0.079      | 0.071      | –87    | 26.3     | 3.4      | 0.3             | 42.3     | 2.2             | 2.44          | ...                  | LP  | T   | ...   | 1FGL J0448.6+1118    | ... | bzq   | PKS 0446+11            | ...  |
|               |        |         |         |         |            |            |        |          |          |                 |          |                 |               |                      |     |     |       | 3EG J0450+1105       |     |       |                        |      |
| J0449.4–4350  | 72.371 | –43.838 | 248.809 | –39.906 | 0.020      | 0.019      | 84     | 66.5     | 11.4     | 0.4             | 135.6    | 6.1             | 1.86          | 0.02                 | PL  | T   | ...   | 1FGL J0449.5–4350    | P   | bzb   | PKS 0447–439           | ...  |
|               |        |         |         |         |            |            |        |          |          |                 |          |                 |               |                      |     |     |       | 0FGL J0449.7–4348    |     |       |                        |      |
| J0451.8–7011  | 72.958 | –70.199 | 281.815 | –35.403 | 0.182      | 0.152      | –54    | 4.5      | 0.6      | 0.1             | 6.8      | 1.6             | 2.19          | 0.14                 | PL  | ... | ...   | ...                  | ... | gal   | LMC field <sup>a</sup> | ...  |
| J0453.1–2807  | 73.279 | –28.121 | 229.003 | –37.041 | 0.077      | 0.069      | 69     | 28.0     | 1.9      | 0.2             | 35.0     | 1.6             | 2.66          | 0.05                 | PL  | T   | ...   | 1FGL J0453.2–2805    | ... | bzq   | PKS 0451–28            | ...  |
| J0455.8–6920  | 73.969 | –69.349 | 280.692 | –35.333 | 0.151      | 0.137      | 66     | 5.6      | 0.7      | 0.2             | 9.1      | 1.7             | 2.33          | 0.12                 | PL  | ... | 10    | ...                  | ... | gal   | LMC field <sup>a</sup> | ...  |
| J0456.1–4613  | 74.041 | –46.218 | 251.906 | –38.759 | 0.112      | 0.100      | 45     | 19.5     | 1.4      | 0.2             | 24.2     | 1.5             | 2.62          | 0.06                 | PL  | ... | 2     | 1FGL J0455.6–4618    | ... | bzq   | PKS 0454–46            | ...  |
|               |        |         |         |         |            |            |        |          |          |                 |          |                 |               |                      |     |     |       | 3EG J0458–4635       |     |       |                        |      |
| J0456.5+2658  | 74.126 | 26.972  | 175.461 | –10.049 | 0.108      | 0.099      | –24    | 8.5      | 1.5      | 0.2             | 18.4     | 2.4             | 2.34          | 0.08                 | PL  | T   | ...   | ...                  | ... | agu   | MG2 J045613+2702       | ...  |
| J0456.5–3132  | 74.140 | –31.537 | 233.386 | –37.084 | 0.155      | 0.138      | 16     | 6.3      | 0.5      | 0.1             | 6.4      | 1.1             | 2.42          | 0.14                 | PL  | T   | ...   | 1FGL J0456.4–3132    | ... | bzq   | PMN J0456–3135         | ...  |
| J0457.0–2325  | 74.268 | –23.427 | 223.727 | –34.896 | 0.018      | 0.018      | 11     | 126.2    | 22.7     | 0.5             | 221.2    | 4.4             | 2.21          | ...                  | LP  | T   | ...   | 1FGL J0457.0–2325    | ... | bzq   | PKS 0454–234           | ...  |
|               |        |         |         |         |            |            |        |          |          |                 |          |                 |               |                      |     |     |       | 0FGL J0457.1–2325    |     |       |                        |      |
|               |        |         |         |         |            |            |        |          |          |                 |          |                 |               |                      |     |     |       | 3EG J0456–2338       |     |       |                        |      |
|               |        |         |         |         |            |            |        |          |          |                 |          |                 |               |                      |     |     |       | EGR J0456–2334       |     |       |                        |      |
| J0458.4+0654  | 74.602 | 6.904   | 192.758 | –21.314 | 0.153      | 0.141      | 85     | 5.5      | 0.6      | 0.1             | 8.4      | 1.7             | 2.44          | 0.16                 | PL  | T   | 4     | 1FGL J0457.9+0649    | ... | ...   | ...                    | ...  |
| J0501.2–0155  | 75.319 | –1.931  | 201.406 | –25.254 | 0.130      | 0.107      | 33     | 10.2     | 0.9      | 0.1             | 13.6     | 1.5             | 2.52          | 0.10                 | PL  | ... | ...   | 1FGL J0501.0–0200    | ... | bzq   | S3 0458–02             | ...  |

Table 1—Continued

| Name              | 2FGL   | R.A.    | Decl.   | $l$     | $b$   | $\theta_1$ | $\theta_2$ | $\phi$ | $\sigma$ | $F_{35}$ | $\Delta F_{35}$ | $S_{25}$ | $\Delta S_{25}$ | $\Gamma_{25}$ | $\Delta \Gamma_{25}$ | Mod | Var | Flags             | $\gamma$ -ray Assoc. | TeV | Class                 | ID or Assoc. | Ref. |
|-------------------|--------|---------|---------|---------|-------|------------|------------|--------|----------|----------|-----------------|----------|-----------------|---------------|----------------------|-----|-----|-------------------|----------------------|-----|-----------------------|--------------|------|
| 3EG J0500–0159    |        |         |         |         |       |            |            |        |          |          |                 |          |                 |               |                      |     |     |                   |                      |     |                       |              |      |
| J0502.5+0607      | 75.641 | 6.120   | 194.060 | −20.862 | 0.217 | 0.189      | −7         | 4.2    | 0.5      | 0.1      | 7.6             | 1.9      | 2.46            | 0.17          | PL                   | ... | ... | 3EG J0459+0544    | ...                  | bzq | PKS 0459+060          | ...          |      |
| J0503.2+4643      | 75.818 | 46.717  | 160.635 | 3.126   | 0.181 | 0.128      | 48         | 5.8    | 1.1      | 0.2      | 13.7            | 2.4      | 2.33            | 0.10          | PL                   | T   | ... | ...               | ...                  | †   | ...                   | ...          |      |
| J0503.3+4517      | 75.847 | 45.287  | 161.784 | 2.273   | 0.090 | 0.087      | 6          | 5.9    | 1.1      | 0.2      | 12.6            | 2.7      | 1.85            | 0.14          | PL                   | ... | ... | 1FGL J0503.2+4526 | ...                  | agu | 1RXS J050339.8+451715 | ...          |      |
| J0505.4+0419      | 76.353 | 4.328   | 196.093 | −21.202 | 0.123 | 0.114      | −65        | 5.8    | 0.8      | 0.2      | 8.5             | 1.8      | 2.15            | 0.15          | PL                   | ... | 5   | 1FGL J0505.2+0420 | ...                  | bzb | MG1 J050533+0415      | ...          |      |
| J0505.5+0501      | 76.385 | 5.032   | 195.467 | −20.808 | 0.100 | 0.092      | 37         | 8.9    | 1.3      | 0.2      | 16.4            | 2.4      | 2.35            | 0.10          | PL                   | T   | ... | ...               | ...                  | bzq | PKS 0502+049          | ...          |      |
| J0505.8−0411      | 76.451 | −4.199  | 204.206 | −25.351 | 0.182 | 0.138      | 25         | 5.1    | 0.6      | 0.1      | 6.9             | 1.5      | 2.21            | 0.14          | PL                   | ... | ... | 1FGL J0505.8−0416 | ...                  | bzq | S3 0503−04            | ...          |      |
| J0505.9+6116      | 76.490 | 61.274  | 149.063 | 12.115  | 0.089 | 0.087      | 28         | 5.0    | 0.6      | 0.2      | 7.2             | 1.8      | 1.84            | 0.16          | PL                   | ... | ... | 1FGL J0505.9+6121 | ...                  | agu | NVSS J050558+611336   | ...          |      |
| J0506.5−0901      | 76.629 | −9.024  | 209.093 | −27.388 | 0.246 | 0.227      | −73        | 4.7    | 0.6      | 0.1      | 6.7             | 1.5      | 2.24            | 0.16          | PL                   | ... | ... | ...               | ...                  | bzb | 1WGA J0506.6−0857     | ...          |      |
| J0506.7−5435      | 76.697 | −54.593 | 262.434 | −36.799 | 0.077 | 0.068      | 79         | 7.8    | 0.5      | 0.1      | 8.0             | 2.3      | 1.52            | 0.17          | PL                   | ... | ... | 1FGL J0506.9−5435 | ...                  | agu | 1ES 0505−546          | ...          |      |
| J0507.5−6102      | 76.884 | −61.043 | 270.388 | −35.994 | 0.092 | 0.087      | 85         | 14.0   | 1.3      | 0.2      | 16.6            | 1.6      | 2.36            | 0.08          | PL                   | T   | ... | 1FGL J0507.3−6103 | ...                  | bzq | PMN J0507−6104        | ...          |      |
| J0508.0+6737      | 77.013 | 67.625  | 143.800 | 15.900  | 0.025 | 0.023      | −69        | 26.2   | 2.4      | 0.2      | 42.3            | 4.6      | 1.49            | 0.07          | PL                   | T   | ... | 1FGL J0507.9+6738 | P                    | bzb | 1ES 0502+675          | ...          |      |
| 0FGL J0507.9+6739 |        |         |         |         |       |            |            |        |          |          |                 |          |                 |               |                      |     |     |                   |                      |     |                       |              |      |
| J0508.1−1936      | 77.046 | −19.616 | 220.440 | −31.206 | 0.199 | 0.166      | 51         | 4.4    | 0.4      | 0.1      | 5.2             | 1.2      | 2.43            | 0.17          | PL                   | ... | ... | ...               | ...                  | agu | PMN J0508−1936        | ...          |      |
| J0509.2+1013      | 77.311 | 10.221  | 191.337 | −17.267 | 0.112 | 0.090      | −78        | 9.5    | 1.3      | 0.2      | 15.9            | 2.0      | 2.33            | 0.09          | PL                   | ... | ... | 1FGL J0509.2+1015 | ...                  | bzq | PKS 0506+101          | ...          |      |
| J0509.4+0542      | 77.368 | 5.700   | 195.405 | −19.623 | 0.040 | 0.035      | 75         | 30.2   | 4.9      | 0.3      | 54.9            | 3.3      | 2.06            | 0.04          | PL                   | T   | ... | 1FGL J0509.3+0540 | ...                  | bzb | TXS 0506+056          | ...          |      |
| EGR J0509+0550    |        |         |         |         |       |            |            |        |          |          |                 |          |                 |               |                      |     |     |                   |                      |     |                       |              |      |
| J0509.9+1802      | 77.493 | 18.034  | 184.702 | −12.790 | 0.109 | 0.085      | −2         | 8.5    | 1.2      | 0.2      | 15.1            | 2.0      | 2.29            | 0.10          | PL                   | T   | ... | 1FGL J0510.0+1800 | ...                  | bzq | PKS 0507+17           | ...          |      |
| J0512.9+4040      | 78.245 | 40.671  | 166.533 | 0.918   | 0.108 | 0.095      | −35        | 5.1    | 0.8      | 0.2      | 9.7             | 2.3      | 1.89            | 0.12          | PL                   | ... | ... | ...               | ...                  | agu | B3 0509+406           | ...          |      |
| J0515.0−4411      | 78.754 | −44.199 | 249.585 | −35.344 | 0.228 | 0.211      | 10         | 5.4    | 0.4      | 0.1      | 7.1             | 1.3      | 2.62            | 0.15          | PL                   | ... | ... | 1FGL J0515.6−4404 | ...                  | ... | ...                   | ...          |      |
| J0515.5+7355      | 78.887 | 73.928  | 138.525 | 19.758  | 0.147 | 0.124      | 41         | 4.8    | 0.4      | 0.1      | 5.2             | 1.6      | 1.63            | 0.21          | PL                   | ... | ... | 1FGL J0515.2+7355 | ...                  | bzb | GB6 J0516+7350        | ...          |      |
| J0515.9+1528      | 78.985 | 15.469  | 187.704 | −13.035 | 0.059 | 0.054      | −28        | 10.1   | 1.4      | 0.2      | 15.5            | 2.4      | 1.94            | 0.10          | PL                   | ... | ... | 1FGL J0515.9+1528 | ...                  | bzb | GB6 J0515+1527        | ...          |      |
| J0516.5−4601      | 79.137 | −46.020 | 251.836 | −35.222 | 0.223 | 0.192      | −72        | 5.0    | 0.4      | 0.1      | 6.1             | 1.3      | 2.47            | 0.18          | PL                   | ... | ... | ...               | ...                  | bzq | PKS 0514−459          | ...          |      |
| J0516.7+2634      | 79.200 | 26.569  | 178.494 | −6.631  | 0.116 | 0.109      | −47        | 8.1    | 1.2      | 0.2      | 20.2            | 2.5      | 2.58            | 0.09          | PL                   | ... | ... | ...               | ...                  | ... | ...                   | ...          |      |
| J0516.8−6207      | 79.219 | −62.118 | 271.507 | −34.746 | 0.044 | 0.042      | 64         | 26.5   | 3.1      | 0.2      | 34.9            | 2.2      | 2.15            | 0.05          | PL                   | T   | ... | 1FGL J0516.7−6207 | ...                  | bzb | PKS 0516−621          | ...          |      |
| 0FGL J0516.2−6200 |        |         |         |         |       |            |            |        |          |          |                 |          |                 |               |                      |     |     |                   |                      |     |                       |              |      |
| 3EG J0512−6150    |        |         |         |         |       |            |            |        |          |          |                 |          |                 |               |                      |     |     |                   |                      |     |                       |              |      |
| J0517.0+4532      | 79.251 | 45.544  | 162.993 | 4.350   | 0.151 | 0.106      | 83         | 5.7    | 1.0      | 0.2      | 10.6            | 2.1      | 2.13            | 0.11          | PL                   | T   | 4   | ...               | ...                  | bzq | 4C +45.08             | ...          |      |
| J0517.5+0900      | 79.385 | 9.011   | 193.546 | −16.184 | 0.118 | 0.096      | −2         | 9.0    | 1.3      | 0.2      | 16.3            | 2.1      | 2.32            | 0.09          | PL                   | ... | 10  | 1FGL J0517.6+0857 | ...                  | bzq | PMN J0517+0858        | ...          |      |
| J0521.4−1736      | 80.362 | −17.612 | 219.603 | −27.552 | 0.170 | 0.146      | −85        | 5.1    | 0.5      | 0.1      | 6.3             | 1.3      | 2.45            | 0.15          | PL                   | ... | 1   | ...               | ...                  | bzq | CGRaBS J0521−1737     | ...          |      |
| J0521.7+2113      | 80.449 | 21.220  | 183.603 | −8.699  | 0.024 | 0.023      | −41        | 39.0   | 9.0      | 0.4      | 103.3           | 5.2      | 1.93            | 0.03          | PL                   | T   | ... | 1FGL J0521.7+2114 | P                    | bzb | VER J0521+211         | ...          |      |
| J0521.9+0108      | 80.492 | 1.145   | 201.244 | −19.238 | 0.201 | 0.114      | 46         | 4.6    | 0.4      | 0.1      | 6.0             | 2.1      | 1.59            | 0.23          | PL                   | ... | ... | 1FGL J0521.6+0103 | ...                  | bzq | PKS 0519+01           | ...          |      |
| J0523.0−3628      | 80.769 | −36.469 | 240.625 | −32.696 | 0.044 | 0.042      | −0         | 45.8   | 4.9      | 0.3      | 65.9            | 2.3      | 2.42            | 0.03          | PL                   | T   | ... | 1FGL J0522.8−3632 | ...                  | AGN | PKS 0521−36           | 4            |      |
| J0523.3−2530      | 80.828 | −25.503 | 228.228 | −29.844 | 0.066 | 0.059      | −42        | 18.5   | 2.0      | 0.2      | 21.8            | 2.0      | 2.12            | 0.07          | PL                   | ... | ... | 1FGL J0523.5−2529 | ...                  | ... | ...                   | ...          |      |
| J0524.1+2843      | 81.031 | 28.718  | 177.636 | −4.078  | 0.101 | 0.086      | −73        | 6.1    | 1.0      | 0.2      | 12.2            | 2.2      | 2.26            | 0.12          | PL                   | ... | ... | 1FGL J0524.1+2842 | ...                  | ... | ...                   | ...          |      |

Table 1—Continued

| Name 2FGL     | R.A.   | Decl.   | $l$     | $b$     | $\theta_1$ | $\theta_2$ | $\phi$ | $\sigma$ | $F_{35}$ | $\Delta F_{35}$ | $S_{25}$ | $\Delta S_{25}$ | $\Gamma_{25}$ | $\Delta \Gamma_{25}$ | Mod | Var | Flags | $\gamma$ -ray Assoc.                                                                          | TeV | Class | ID or Assoc.               | Ref |
|---------------|--------|---------|---------|---------|------------|------------|--------|----------|----------|-----------------|----------|-----------------|---------------|----------------------|-----|-----|-------|-----------------------------------------------------------------------------------------------|-----|-------|----------------------------|-----|
| J0525.5–6011  | 81.394 | –60.196 | 269.070 | –33.886 | 0.157      | 0.131      | –24    | 4.9      | 0.4      | 0.1             | 5.2      | 1.4             | 1.90          | 0.19                 | PL  | ... | ...   | ...                                                                                           | ... | agu   | SUMSS J052542–601341       | ... |
| J0526.1–4829  | 81.548 | –48.483 | 254.960 | –33.767 | 0.075      | 0.072      | –8     | 12.4     | 1.5      | 0.2             | 17.0     | 1.9             | 2.20          | 0.09                 | PL  | T   | ...   | 1FGL J0526.3–4829                                                                             | ... | bzq   | PKS 0524–485               | ... |
| J0526.6–6825e | 81.650 | –68.420 | 278.843 | –32.850 | ...        | ...        | ...    | 65.2     | 19.6     | 0.6             | 185.2    | 7.5             | 2.17          | ...                  | EC  | T   | ...   | ...                                                                                           | ... | GAL   | LMC                        | 5   |
| J0526.6+2248  | 81.659 | 22.806  | 182.893 | –6.889  | 0.107      | 0.101      | 55     | 7.1      | 1.0      | 0.3             | 26.3     | 4.0             | 2.88          | 0.16                 | PL  | ... | 1     | ...                                                                                           | ... | ...   | ...                        | ... |
| J0526.6+4308  | 81.665 | 43.147  | 165.955 | 4.421   | 0.577      | 0.316      | 50     | 4.4      | 0.8      | 0.2             | 10.2     | 2.1             | 2.38          | 0.12                 | PL  | ... | 4,9   | ...                                                                                           | ... | †     | ...                        | ... |
| J0526.8+6326  | 81.718 | 63.437  | 148.556 | 15.326  | 0.171      | 0.131      | 42     | 4.2      | 0.5      | 0.1             | 5.8      | 1.3             | 2.21          | 0.15                 | PL  | ... | ...   | ...                                                                                           | ... | agu   | GB6 J0526+6317             | ... |
| J0529.2+0935  | 82.301 | 9.597   | 194.581 | –13.423 | 0.099      | 0.092      | –43    | 6.7      | 0.9      | 0.2             | 12.3     | 2.0             | 2.45          | 0.12                 | PL  | ... | 1,4   | ...                                                                                           | ... | agu   | GB6 J0529+0934             | ... |
| J0529.3+3821  | 82.349 | 38.353  | 170.242 | 2.200   | 0.124      | 0.116      | –76    | 4.6      | 1.0      | 0.2             | 11.2     | 2.6             | 2.09          | 0.12                 | PL  | ... | 4     | ...                                                                                           | ... | ...   | ...                        | ... |
| J0530.8–0517c | 82.703 | –5.283  | 208.376 | –20.325 | 0.276      | 0.202      | –55    | 5.7      | 0.9      | 0.2             | 7.9      | 2.0             | 2.51          | ...                  | LP  | ... | 1,6   | ...                                                                                           | ... | bzq   | PMN J0529–0519             | ... |
| J0530.8+1333  | 82.714 | 13.553  | 191.339 | –11.018 | 0.096      | 0.084      | –86    | 20.4     | 2.6      | 0.3             | 39.1     | 2.4             | 2.55          | ...                  | LP  | T   | ...   | 1FGL J0531.0+1331<br>0FGL J0531.0+1331<br>3EG J0530+1323<br>EGR J0530+1331                    | ... | bzq   | PKS 0528+134               | ... |
| J0531.8–3831  | 82.951 | –38.519 | 243.400 | –31.405 | 0.202      | 0.161      | –14    | 5.3      | 0.4      | 0.1             | 7.5      | 1.5             | 2.61          | 0.15                 | PL  | ... | 2     | ...                                                                                           | ... | bzq   | PMN J0532–3848             | ... |
| J0531.8–8324  | 82.967 | –83.408 | 295.830 | –29.192 | 0.096      | 0.084      | –75    | 10.0     | 1.3      | 0.2             | 14.8     | 1.9             | 2.15          | 0.09                 | PL  | T   | ...   | 1FGL J0533.0–8324                                                                             | ... | bzq   | PKS 0541–834               | ... |
| J0532.0–4826  | 83.011 | –48.444 | 255.008 | –32.797 | 0.046      | 0.044      | 90     | 23.1     | 3.0      | 0.2             | 33.8     | 2.4             | 2.13          | 0.05                 | PL  | T   | ...   | ...                                                                                           | ... | agu   | PMN J0531–4827             | ... |
| J0532.5–7223  | 83.140 | –72.393 | 283.379 | –31.699 | 0.169      | 0.135      | 38     | 4.5      | 0.4      | 0.1             | 6.5      | 1.5             | 2.55          | 0.19                 | PL  | ... | ...   | ...                                                                                           | ... | agu   | PMN J0533–7216             | ... |
| J0532.7+0733  | 83.188 | 7.559   | 196.843 | –13.709 | 0.052      | 0.046      | –84    | 26.8     | 4.1      | 0.3             | 50.4     | 2.7             | 2.31          | 0.04                 | PL  | T   | ...   | 1FGL J0532.9+0733                                                                             | ... | bzq   | OG 050                     | ... |
| J0533.0+4823  | 83.261 | 48.394  | 162.131 | 8.206   | 0.059      | 0.057      | 19     | 19.6     | 2.9      | 0.2             | 35.2     | 2.3             | 2.31          | 0.05                 | PL  | T   | ...   | 1FGL J0533.0+4825<br>3EG J0533+4751                                                           | ... | bzq   | TXS 0529+483               | ... |
| J0533.3–6651  | 83.331 | –66.852 | 276.896 | –32.427 | 0.234      | 0.200      | 34     | 5.6      | 0.9      | 0.2             | 10.2     | 1.8             | 2.27          | 0.14                 | PL  | ... | ...   | ...                                                                                           | ... | gal   | LMC field <sup>a</sup>     | ... |
| J0533.9+6759  | 83.490 | 67.998  | 144.773 | 18.191  | 0.089      | 0.077      | –73    | 11.1     | 1.5      | 0.2             | 8.4      | 1.4             | 2.03          | ...                  | LP  | ... | ...   | 1FGL J0533.9+6758                                                                             | ... | ...   | ...                        | ... |
| J0534.5+2201  | 83.632 | 22.020  | 184.553 | –5.783  | 0.007      | 0.007      | –86    | 376.6    | 182.7    | 1.5             | 1891.4   | 16.0            | 2.19          | ...                  | EC  | T   | ...   | 1FGL J0534.5+2200<br>0FGL J0534.6+2201<br>3EG J0534+2200<br>EGR J0534+2159<br>1AGL J0535+2205 | P   | PSR   | PSR J0534+2200<br>PWN Crab | ... |
| J0534.8–0548c | 83.719 | –5.812  | 209.363 | –19.663 | 0.119      | 0.101      | –20    | 6.0      | 1.6      | 0.3             | 18.8     | 3.3             | 2.22          | 0.12                 | PL  | ... | 2,6   | ...                                                                                           | ... | ...   | ...                        | ... |
| J0534.9–0450c | 83.725 | –4.839  | 208.446 | –19.216 | 0.148      | 0.120      | –1     | 4.9      | 1.1      | 0.3             | 12.9     | 2.8             | 2.15          | 0.13                 | PL  | ... | 6     | ...                                                                                           | ... | ...   | ...                        | ... |
| J0536.2–3348  | 84.056 | –33.810 | 238.311 | –29.477 | 0.066      | 0.055      | 11     | 22.1     | 2.1      | 0.2             | 27.2     | 1.7             | 2.39          | 0.06                 | PL  | T   | ...   | 1FGL J0536.2–3348                                                                             | ... | bzb   | 1RXS J053629.4–334302      | ... |
| J0537.7–5716  | 84.433 | –57.274 | 265.530 | –32.391 | 0.109      | 0.096      | –19    | 4.9      | 0.4      | 0.1             | 5.2      | 1.7             | 1.73          | 0.21                 | PL  | ... | ...   | 1FGL J0537.7–5717                                                                             | ... | agu   | SUMSS J053748–571828       | ... |
| J0538.1+2718  | 84.539 | 27.306  | 180.517 | –2.258  | 0.096      | 0.092      | –14    | 5.8      | 1.3      | 0.3             | 15.4     | 2.9             | 2.25          | 0.12                 | PL  | ... | 4     | 1FGL J0538.6+2717                                                                             | ... | †     | ...                        | ... |
| J0538.5–3909  | 84.629 | –39.152 | 244.429 | –30.252 | 0.096      | 0.081      | 33     | 6.5      | 0.6      | 0.1             | 6.9      | 1.4             | 2.18          | 0.15                 | PL  | ... | ...   | 1FGL J0538.4–3910                                                                             | ... | agu   | 1RXS J053810.0–390839      | ... |
| J0538.5–0534c | 84.647 | –5.574  | 209.580 | –18.731 | 0.208      | 0.170      | –42    | 9.3      | 0.9      | 0.2             | 19.8     | 2.4             | 2.53          | ...                  | LP  | ... | 6,12  | ...                                                                                           | ... | ...   | ...                        | ... |
| J0538.8–4405  | 84.706 | –44.084 | 250.080 | –31.092 | 0.013      | 0.013      | –20    | 165.0    | 37.1     | 0.7             | 368.2    | 7.9             | 2.09          | ...                  | LP  | T   | ...   | 1FGL J0538.8–4404                                                                             | ... | BZB   | PKS 0537–441               | ... |

Table 1—Continued

| Name 2FGL     | R.A.   | Decl.   | $l$     | $b$     | $\theta_1$ | $\theta_2$ | $\phi$ | $\sigma$ | $F_{35}$ | $\Delta F_{35}$ | $S_{25}$ | $\Delta S_{25}$ | $\Gamma_{25}$ | $\Delta \Gamma_{25}$ | Mod | Var | Flags  | $\gamma$ -ray Assoc. | TeV | Class | ID or Assoc.          | Ref. |
|---------------|--------|---------|---------|---------|------------|------------|--------|----------|----------|-----------------|----------|-----------------|---------------|----------------------|-----|-----|--------|----------------------|-----|-------|-----------------------|------|
|               |        |         |         |         |            |            |        |          |          |                 |          |                 |               |                      |     |     |        | 0FGL J0538.8–4403    |     |       |                       |      |
|               |        |         |         |         |            |            |        |          |          |                 |          |                 |               |                      |     |     |        | 3EG J0540–4402       |     |       |                       |      |
|               |        |         |         |         |            |            |        |          |          |                 |          |                 |               |                      |     |     |        | EGR J0540–4358       |     |       |                       |      |
|               |        |         |         |         |            |            |        |          |          |                 |          |                 |               |                      |     |     |        | 1AGL J0538–4424      |     |       |                       |      |
| J0539.3–0323  | 84.830 | –3.397  | 207.627 | –17.577 | 0.157      | 0.122      | 19     | 5.0      | 0.9      | 0.2             | 10.7     | 2.3             | 2.32          | 0.13                 | PL  | ... | ...    | ...                  | ... | ...   | ...                   | ...  |
| J0539.3–2841  | 84.846 | –28.697 | 232.936 | –27.410 | 0.154      | 0.123      | 39     | 11.8     | 0.6      | 0.1             | 14.4     | 1.3             | 2.83          | 0.10                 | PL  | T   | ...    | 1FGL J0539.1–2847    | ... | bzq   | PKS 0537–286          | ...  |
| J0540.1–7554  | 85.049 | –75.904 | 287.310 | –30.567 | 0.161      | 0.127      | –77    | 4.1      | 0.4      | 0.1             | 5.2      | 1.3             | 2.22          | 0.18                 | PL  | ... | ...    | ...                  | ... | ...   | ...                   | ...  |
| J0540.3+3549c | 85.091 | 35.818  | 173.560 | 2.672   | 0.180      | 0.125      | –45    | 11.4     | 2.7      | 0.4             | 24.7     | 2.5             | 2.32          | ...                  | LP  | ... | 6      | 1FGL J0541.1+3542c   | ... | ...   | ...                   | ...  |
| J0540.4+5822  | 85.107 | 58.382  | 153.938 | 14.243  | 0.061      | 0.059      | –75    | 7.9      | 0.8      | 0.2             | 10.1     | 1.9             | 1.84          | 0.13                 | PL  | ... | ...    | ...                  | ... | agu   | GB6 J0540+5823        | ...  |
| J0540.4–5415  | 85.109 | –54.253 | 261.979 | –31.911 | 0.166      | 0.115      | 15     | 9.2      | 0.8      | 0.1             | 12.6     | 1.5             | 2.57          | 0.10                 | PL  | T   | ...    | ...                  | ... | bzq   | PKS 0539–543          | ...  |
| J0541.8–0203c | 85.454 | –2.061  | 206.690 | –16.406 | 0.143      | 0.120      | 26     | 9.5      | 2.3      | 0.4             | 19.0     | 2.6             | 2.22          | ...                  | LP  | ... | 6      | 1FGL J0541.9–0204c   | ... | ...   | ...                   | ...  |
| J0543.2–0120c | 85.811 | –1.336  | 206.195 | –15.752 | 0.147      | 0.120      | 2      | 5.5      | 1.4      | 0.3             | 15.5     | 3.1             | 2.19          | 0.11                 | PL  | ... | 1,5,6  | ...                  | ... | ...   | ...                   | ...  |
| J0543.9–5532  | 85.992 | –55.534 | 263.513 | –31.472 | 0.042      | 0.038      | 49     | 17.7     | 1.9      | 0.2             | 25.2     | 3.2             | 1.74          | 0.08                 | PL  | ... | ...    | 1FGL J0543.8–5531    | ... | bzb   | 1RXS J054357.3–553206 | ...  |
| J0545.6+6018  | 86.411 | 60.314  | 152.502 | 15.744  | 0.073      | 0.069      | 49     | 7.9      | 0.9      | 0.1             | 9.8      | 1.7             | 1.95          | 0.11                 | PL  | ... | ...    | 1FGL J0545.6+6022    | ... | ...   | ...                   | ...  |
| J0547.1+0020c | 86.800 | 0.335   | 205.149 | –14.095 | 0.142      | 0.124      | –2     | 11.3     | 2.0      | 0.3             | 23.0     | 2.4             | 2.40          | ...                  | LP  | ... | 6      | 1FGL J0547.0+0020c   | ... | ...   | ...                   | ...  |
| J0547.4+3722  | 86.870 | 37.381  | 172.969 | 4.705   | 0.143      | 0.124      | –77    | 4.4      | 0.7      | 0.2             | 10.1     | 2.2             | 2.42          | 0.15                 | PL  | ... | 4      | ...                  | ... | ...   | ...                   | ...  |
| J0547.5–0141c | 86.881 | –1.687  | 207.034 | –14.970 | 0.296      | 0.191      | –67    | 6.1      | 0.7      | 0.2             | 13.1     | 2.2             | 2.42          | ...                  | LP  | ... | 1,6,12 | ...                  | ... | ...   | ...                   | ...  |
| J0553.9+3104  | 88.487 | 31.079  | 179.087 | 2.647   | 0.116      | 0.106      | –10    | 11.1     | 2.6      | 0.3             | 13.9     | 1.7             | 2.15          | ...                  | LP  | ... | ...    | 1FGL J0553.9+3105    | ... | †     | ...                   | ...  |
| J0555.9–4348  | 88.976 | –43.804 | 250.405 | –28.018 | 0.178      | 0.144      | –0     | 5.0      | 0.6      | 0.1             | 6.3      | 1.4             | 2.11          | 0.17                 | PL  | ... | ...    | ...                  | ... | ...   | ...                   | ...  |
| J0558.2–3837  | 89.558 | –38.625 | 244.851 | –26.398 | 0.111      | 0.098      | –49    | 7.3      | 0.7      | 0.1             | 8.3      | 1.4             | 2.25          | 0.15                 | PL  | ... | ...    | 1FGL J0557.6–3831    | ... | bzb   | EXO 0556.4–3838       | ...  |
| J0558.7–7501  | 89.683 | –75.031 | 286.131 | –29.532 | 0.135      | 0.098      | 43     | 6.5      | 0.7      | 0.1             | 8.3      | 1.6             | 2.09          | 0.14                 | PL  | ... | ...    | 1FGL J0559.2–7500    | ... | bzb   | PKS 0600–749          | ...  |
| J0600.8–1949  | 90.216 | –19.830 | 225.702 | –19.751 | 0.225      | 0.181      | –44    | 5.1      | 0.5      | 0.1             | 7.0      | 1.4             | 2.39          | 0.15                 | PL  | ... | ...    | 1FGL J0600.5–2006    | ... | ...   | ...                   | ...  |
| J0600.9+3839  | 90.241 | 38.651  | 173.190 | 7.641   | 0.085      | 0.074      | 58     | 5.1      | 0.7      | 0.2             | 7.4      | 1.9             | 2.04          | 0.21                 | PL  | ... | ...    | 1FGL J0600.9+3838    | ... | ...   | ...                   | ...  |
| J0601.1–7037  | 90.295 | –70.623 | 281.060 | –29.629 | 0.051      | 0.049      | 37     | 28.1     | 3.6      | 0.2             | 34.9     | 2.1             | 2.29          | ...                  | LP  | T   | ...    | 1FGL J0600.7–7037    | ... | bzq   | PKS 0601–70           | ...  |
| J0602.3+5315  | 90.589 | 53.251  | 160.101 | 14.608  | 0.151      | 0.110      | 69     | 6.3      | 0.6      | 0.1             | 8.1      | 1.9             | 1.75          | 0.17                 | PL  | ... | ...    | ...                  | ... | agu   | GB6 J0601+5315        | ...  |
| J0602.7–4011  | 90.678 | –40.184 | 246.776 | –25.956 | 0.117      | 0.089      | 23     | 9.6      | 1.1      | 0.2             | 12.4     | 1.8             | 2.11          | 0.11                 | PL  | ... | ...    | 1FGL J0603.0–4012    | ... | ...   | ...                   | ...  |
| J0604.2–4817  | 91.054 | –48.294 | 255.700 | –27.488 | 0.067      | 0.065      | 56     | 7.7      | 0.7      | 0.1             | 8.2      | 1.9             | 1.82          | 0.15                 | PL  | ... | ...    | 1FGL J0604.2–4817    | ... | agu   | 1ES 0602–482          | ...  |
| J0605.0+0001  | 91.258 | 0.032   | 207.556 | –10.295 | 0.084      | 0.078      | –9     | 4.9      | 0.6      | 0.2             | 7.4      | 2.0             | 1.89          | 0.18                 | PL  | ... | ...    | 1FGL J0605.1+0005    | ... | agu   | GB6 J0604+0000        | ...  |
| J0605.3+3758  | 91.347 | 37.980  | 174.204 | 8.083   | 0.124      | 0.101      | 1      | 7.6      | 1.4      | 0.2             | 7.1      | 1.4             | 2.12          | ...                  | LP  | ... | ...    | 1FGL J0605.3+3800    | ... | ...   | ...                   | ...  |
| J0607.4+4739  | 91.870 | 47.658  | 165.639 | 12.872  | 0.060      | 0.053      | 67     | 17.0     | 2.2      | 0.2             | 24.7     | 2.3             | 2.05          | 0.06                 | PL  | ... | ...    | 1FGL J0607.2+4739    | ... | bzb   | TXS 0603+476          | ...  |
| J0607.5–0618c | 91.881 | –6.306  | 213.604 | –12.623 | 0.190      | 0.166      | –1     | 7.6      | 0.9      | 0.3             | 12.9     | 2.0             | 2.41          | ...                  | LP  | ... | 6      | 1FGL J0608.1–0630c   | ... | ...   | ...                   | ...  |
| J0608.0–1521  | 92.003 | –15.367 | 222.112 | –16.407 | 0.072      | 0.069      | 87     | 19.7     | 2.3      | 0.2             | 28.6     | 2.0             | 2.45          | ...                  | LP  | T   | ...    | 1FGL J0608.0–1521    | ... | bzq   | PMN J0608–1520        | ...  |
| J0608.0–0836  | 92.015 | –8.611  | 215.788 | –13.522 | 0.068      | 0.062      | –44    | 11.6     | 1.8      | 0.2             | 22.7     | 2.4             | 2.36          | 0.08                 | PL  | T   | ...    | 1FGL J0608.2–0837    | ... | bzq   | PKS 0605–08           | ...  |
| J0608.3+2037  | 92.085 | 20.632  | 189.767 | 0.285   | 0.113      | 0.104      | –71    | 12.5     | 3.3      | 0.5             | 28.9     | 2.8             | 2.28          | ...                  | LP  | ... | ...    | 1FGL J0608.3+2038c   | ... | ...   | ...                   | ...  |
| J0609.4–0248  | 92.375 | –2.812  | 210.646 | –10.610 | 0.086      | 0.070      | 12     | 7.9      | 1.0      | 0.2             | 11.9     | 2.5             | 1.79          | 0.15                 | PL  | ... | ...    | 1FGL J0609.3–0244    | ... | agu   | NVSS J060915–024754   | ...  |

Table 1—Continued

| Name 2FGL     | R.A.   | Decl.   | $l$     | $b$     | $\theta_1$ | $\theta_2$ | $\phi$ | $\sigma$ | $F_{35}$ | $\Delta F_{35}$ | $S_{25}$ | $\Delta S_{25}$ | $\Gamma_{25}$ | $\Delta \Gamma_{25}$ | Mod | Var | Flags | $\gamma$ -ray Assoc. | TeV | Class | ID or Assoc.               |
|---------------|--------|---------|---------|---------|------------|------------|--------|----------|----------|-----------------|----------|-----------------|---------------|----------------------|-----|-----|-------|----------------------|-----|-------|----------------------------|
| J0609.6–1847  | 92.424 | –18.788 | 225.552 | –17.426 | 0.227      | 0.170      | –34    | 4.5      | 0.6      | 0.1             | 6.4      | 1.5             | 2.20          | 0.17                 | PL  | ... | ...   | ...                  | ... | bzb   | PMN J0610–1847             |
| J0610.3–2059  | 92.584 | –20.990 | 227.741 | –18.153 | 0.112      | 0.104      | 15     | 8.6      | 1.1      | 0.2             | 8.2      | 1.7             | 2.23          | ...                  | EC  | ... | ...   | 1FGL J0610.7–2059    | ... | PSR   | PSR J0610–2100             |
| J0611.0+4321  | 92.751 | 43.352  | 169.864 | 11.504  | 0.127      | 0.110      | –11    | 4.5      | 0.5      | 0.1             | 6.0      | 1.6             | 1.95          | 0.21                 | PL  | ... | ...   | ...                  | ... | agu   | B3 0607+434                |
| J0611.8–6059  | 92.960 | –60.984 | 270.090 | –28.227 | 0.142      | 0.122      | 87     | 5.8      | 0.5      | 0.1             | 6.6      | 1.3             | 2.36          | 0.16                 | PL  | ... | ...   | ...                  | ... | bzq   | PKS 0609–609               |
| J0612.8+4122  | 93.213 | 41.368  | 171.828 | 10.920  | 0.039      | 0.036      | 10     | 24.2     | 3.6      | 0.3             | 40.4     | 2.9             | 2.03          | 0.05                 | PL  | T   | ...   | 1FGL J0612.7+4120    | ... | bzb   | B3 0609+413                |
| J0613.8–0200  | 93.457 | –2.013  | 210.424 | –9.284  | 0.047      | 0.045      | 45     | 23.0     | 5.0      | 0.3             | 30.7     | 2.3             | 2.06          | ...                  | EC  | ... | ...   | 1FGL J0613.7–0200    | ... | PSR   | PSR J0613–0200             |
|               |        |         |         |         |            |            |        |          |          |                 |          |                 |               |                      |     |     |       | 0FGL J0613.9–0202    |     |       |                            |
| J0614.1–3329  | 93.540 | –33.484 | 240.486 | –21.825 | 0.021      | 0.021      | –30    | 79.9     | 18.3     | 0.5             | 110.9    | 3.3             | 1.86          | ...                  | EC  | ... | ...   | 1FGL J0614.1–3328    | ... | PSR   | PSR J0614–3329             |
|               |        |         |         |         |            |            |        |          |          |                 |          |                 |               |                      |     |     |       | 0FGL J0614.3–3330    |     |       |                            |
|               |        |         |         |         |            |            |        |          |          |                 |          |                 |               |                      |     |     |       | 3EG J0616–3310       |     |       |                            |
|               |        |         |         |         |            |            |        |          |          |                 |          |                 |               |                      |     |     |       | EGR J0615–3308       |     |       |                            |
| J0616.6+2425  | 94.151 | 24.421  | 187.353 | 3.775   | 0.237      | 0.171      | –76    | 4.1      | 0.9      | 0.2             | 10.9     | 2.6             | 2.27          | 0.13                 | PL  | ... | 11    | ...                  | ... | ...   | ...                        |
| J0616.9+5701  | 94.241 | 57.028  | 157.401 | 18.057  | 0.055      | 0.053      | 55     | 11.5     | 1.2      | 0.2             | 13.4     | 2.0             | 1.90          | 0.10                 | PL  | ... | ...   | 1FGL J0616.9+5701    | ... | bzb   | 87GB 061258.1+570222       |
| J0617.2+2234e | 94.310 | 22.580  | 189.048 | 3.034   | ...        | ...        | ...    | 132.9    | 65.1     | 1.0             | 519.4    | 9.2             | 1.97          | ...                  | LP  | ... | ...   | 1FGL J0617.2+2233    | E   | SNR   | SNR G189.1–03.0            |
|               |        |         |         |         |            |            |        |          |          |                 |          |                 |               |                      |     |     |       | 0FGL J0617.4+2234    |     |       | IC 443                     |
|               |        |         |         |         |            |            |        |          |          |                 |          |                 |               |                      |     |     |       | 3EG J0617+2238       |     |       |                            |
|               |        |         |         |         |            |            |        |          |          |                 |          |                 |               |                      |     |     |       | EGR J0617+2238       |     |       |                            |
|               |        |         |         |         |            |            |        |          |          |                 |          |                 |               |                      |     |     |       | 1AGL J0617+2236      |     |       |                            |
| J0617.6–1716  | 94.413 | –17.281 | 224.913 | –15.086 | 0.093      | 0.070      | –75    | 10.6     | 1.4      | 0.2             | 15.9     | 2.3             | 1.96          | 0.10                 | PL  | ... | ...   | 1FGL J0617.7–1718    | ... | bzb   | CRATES J061733.67–171522.8 |
| J0620.8–2556  | 95.224 | –25.939 | 233.521 | –17.806 | 0.191      | 0.137      | 14     | 6.4      | 0.7      | 0.1             | 8.3      | 1.5             | 2.16          | 0.13                 | PL  | T   | 2     | ...                  | ... | ...   | ...                        |
| J0621.2+2508  | 95.315 | 25.139  | 187.213 | 5.045   | 0.111      | 0.103      | –34    | 5.4      | 1.0      | 0.2             | 11.1     | 2.2             | 2.10          | 0.12                 | PL  | ... | 11    | 1FGL J0621.5+2508    | ... | ...   | ...                        |
| J0621.9+3750  | 95.488 | 37.839  | 175.841 | 10.926  | 0.103      | 0.081      | 68     | 14.7     | 1.8      | 0.2             | 14.5     | 1.4             | 2.33          | ...                  | LP  | ... | ...   | 1FGL J0622.2+3751    | ... | agu   | GB6 J0621+3750             |
| J0622.9+3326  | 95.749 | 33.440  | 179.942 | 9.169   | 0.045      | 0.042      | –2     | 23.4     | 4.0      | 0.3             | 44.4     | 2.9             | 2.13          | 0.04                 | PL  | T   | ...   | ...                  | ... | agu   | B2 0619+33                 |
| J0625.2+4441  | 96.324 | 44.685  | 169.757 | 14.397  | 0.083      | 0.074      | 21     | 8.3      | 0.8      | 0.1             | 9.5      | 1.7             | 1.91          | 0.14                 | PL  | ... | ...   | 1FGL J0625.4+4440    | ... | bzb   | GB6 J0625+4440             |
| J0626.8–4258  | 96.706 | –42.971 | 251.055 | –22.372 | 0.148      | 0.119      | –18    | 4.7      | 0.4      | 0.1             | 5.9      | 1.8             | 1.70          | 0.20                 | PL  | ... | ...   | 1FGL J0626.6–4254    | ... | agu   | 1RXS J062635.9–42581       |
| J0627.1–3528  | 96.777 | –35.479 | 243.445 | –19.965 | 0.067      | 0.064      | 45     | 12.6     | 1.5      | 0.2             | 17.2     | 2.3             | 1.93          | 0.09                 | PL  | ... | ...   | 1FGL J0627.3–3530    | ... | rdg   | PKS 0625–35                |
| J0628.9–6246  | 97.228 | –62.771 | 272.363 | –26.450 | 0.117      | 0.100      | 75     | 6.2      | 0.6      | 0.1             | 7.4      | 1.7             | 1.87          | 0.17                 | PL  | ... | ...   | ...                  | ... | agu   | PKS 0628–627               |
| J0629.3–2001  | 97.349 | –20.030 | 228.679 | –13.678 | 0.062      | 0.059      | 84     | 17.4     | 2.5      | 0.2             | 28.3     | 2.3             | 2.19          | 0.06                 | PL  | T   | ...   | 1FGL J0629.6–2000    | ... | bzb   | PKS 0627–199               |
| J0630.9–2406  | 97.734 | –24.108 | 232.678 | –15.000 | 0.039      | 0.037      | –81    | 24.2     | 3.4      | 0.3             | 42.0     | 4.0             | 1.79          | 0.06                 | PL  | ... | ...   | 1FGL J0630.9–2406    | ... | bzb   | TXS 0628–240               |
| J0631.5+1035  | 97.883 | 10.595  | 201.248 | 0.456   | 0.048      | 0.044      | 66     | 19.8     | 5.9      | 0.4             | 38.5     | 3.0             | 2.07          | ...                  | EC  | ... | ...   | 1FGL J0631.4+1037    | ... | PSR   | PSR J0631+1036             |
|               |        |         |         |         |            |            |        |          |          |                 |          |                 |               |                      |     |     |       | 0FGL J0631.8+1034    |     |       |                            |
| J0631.6+0640  | 97.920 | 6.676   | 204.740 | –1.323  | 0.087      | 0.067      | 71     | 10.6     | 4.2      | 0.5             | 29.6     | 4.1             | 2.15          | ...                  | LP  | ... | 5     | 3EG J0631+0642       | ... | †     | ...                        |
| J0631.7+0428  | 97.938 | 4.477   | 206.700 | –2.322  | 0.298      | 0.161      | –80    | 10.2     | 3.3      | 0.4             | 26.9     | 3.4             | 2.29          | ...                  | LP  | ... | 9     | ...                  | ... | ...   | ...                        |
| J0633.7+0633  | 98.432 | 6.556   | 205.081 | –0.927  | 0.029      | 0.028      | 88     | 34.1     | 15.4     | 0.7             | 92.0     | 5.4             | 2.10          | ...                  | EC  | ... | ...   | 1FGL J0633.7+0632    | ... | PSR   | LAT PSR J0633+0632         |
|               |        |         |         |         |            |            |        |          |          |                 |          |                 |               |                      |     |     |       | 0FGL J0633.5+0634    |     |       |                            |

Table 1—Continued

| Name 2FGL     | R.A.    | Decl.   | $l$     | $b$     | $\theta_1$ | $\theta_2$ | $\phi$ | $\sigma$ | $F_{35}$ | $\Delta F_{35}$ | $S_{25}$ | $\Delta S_{25}$ | $\Gamma_{25}$ | $\Delta \Gamma_{25}$ | Mod | Var | Flags  | $\gamma$ -ray Assoc.                                                                          | TeV | Class | ID or Assoc.              | R   |
|---------------|---------|---------|---------|---------|------------|------------|--------|----------|----------|-----------------|----------|-----------------|---------------|----------------------|-----|-----|--------|-----------------------------------------------------------------------------------------------|-----|-------|---------------------------|-----|
| J0633.8+7132  | 98.472  | 71.548  | 143.185 | 24.267  | 0.254      | 0.218      | 25     | 4.7      | 0.4      | 0.1             | 6.6      | 1.3             | 2.62          | 0.16                 | PL  | T   | ...    | EGR J0633+0646                                                                                | ... | agu   | GB6 J0636+7138            | ... |
| J0633.9+1746  | 98.479  | 17.774  | 195.132 | 4.270   | 0.006      | 0.006      | -87    | 791.0    | 729.0    | 3.0             | 4315.1   | 15.1            | 1.87          | ...                  | EC  | ... | 10     | 1FGL J0633.9+1746<br>0FGL J0634.0+1745<br>3EG J0633+1751<br>EGR J0633+1750<br>1AGL J0634+1748 | E   | PSR   | PSR J0633+1746<br>Geminga | ... |
| J0634.3+0356c | 98.586  | 3.944   | 207.471 | -1.994  | 0.279      | 0.177      | -23    | 5.4      | 1.9      | 0.4             | 22.4     | 4.2             | 2.26          | 0.10                 | PL  | ... | 5,6,9  | 1FGL J0634.3+0402c                                                                            | ... | ...   | ...                       | ... |
| J0635.0-2334  | 98.751  | -23.577 | 232.561 | -13.935 | 0.152      | 0.120      | 88     | 4.1      | 0.5      | 0.1             | 5.8      | 1.5             | 2.19          | 0.16                 | PL  | ... | ...    | ...                                                                                           | ... | bzq   | CGRaBS J0634-2335         | ... |
| J0635.5-7516  | 98.889  | -75.274 | 286.371 | -27.173 | 0.082      | 0.078      | 33     | 20.9     | 1.7      | 0.2             | 31.0     | 1.8             | 2.65          | 0.06                 | PL  | T   | ...    | 1FGL J0636.1-7521                                                                             | ... | bzq   | PKS 0637-75               | ... |
| J0636.0+0554  | 99.006  | 5.906   | 205.921 | -0.720  | 0.275      | 0.202      | 66     | 9.0      | 1.4      | 0.3             | 26.4     | 3.2             | 2.47          | ...                  | LP  | ... | 2,5,12 | ...                                                                                           | ... | †     | ...                       | ... |
| J0637.0+0416c | 99.262  | 4.271   | 207.490 | -1.245  | 0.217      | 0.153      | 82     | 7.8      | 2.4      | 0.4             | 20.3     | 3.3             | 2.32          | ...                  | LP  | ... | 6      | ...                                                                                           | ... | ...   | ...                       | ... |
| J0637.8+0737  | 99.474  | 7.622   | 204.610 | 0.481   | 0.148      | 0.109      | 3      | 7.2      | 1.0      | 0.3             | 17.7     | 2.8             | 2.47          | ...                  | LP  | ... | ...    | ...                                                                                           | ... | †     | ...                       | ... |
| J0641.1+1006c | 100.294 | 10.104  | 202.773 | 2.337   | 0.165      | 0.115      | 18     | 9.9      | 1.9      | 0.4             | 23.8     | 3.0             | 2.42          | ...                  | LP  | ... | 6      | ...                                                                                           | ... | ...   | ...                       | ... |
| J0641.2+7315  | 100.322 | 73.251  | 141.481 | 25.169  | 0.161      | 0.118      | -45    | 7.8      | 0.7      | 0.1             | 9.1      | 1.3             | 2.40          | 0.12                 | PL  | T   | 2      | 1FGL J0639.9+7325                                                                             | ... | ...   | ...                       | ... |
| J0642.9+0319  | 100.733 | 3.325   | 209.004 | -0.373  | 0.134      | 0.106      | -58    | 7.7      | 0.6      | 0.2             | 17.8     | 2.3             | 2.46          | ...                  | LP  | ... | 1,12   | ...                                                                                           | ... | ...   | ...                       | ... |
| J0643.2+0858  | 100.815 | 8.982   | 204.008 | 2.283   | 0.073      | 0.065      | 41     | 15.8     | 3.5      | 0.3             | 37.8     | 3.2             | 2.41          | ...                  | LP  | T   | ...    | 1FGL J0643.2+0859<br>0FGL J0643.2+0858                                                        | ... | bzq   | PMN J0643+0857            | ... |
| J0644.2-6713  | 101.053 | -67.220 | 277.532 | -25.549 | 0.052      | 0.049      | 71     | 20.8     | 2.5      | 0.2             | 27.8     | 2.1             | 2.16          | 0.05                 | PL  | T   | ...    | ...                                                                                           | ... | agu   | PKS 0644-671              | ... |
| J0644.6+6034  | 101.170 | 60.575  | 155.067 | 22.598  | 0.107      | 0.087      | -41    | 9.3      | 0.9      | 0.1             | 10.0     | 1.4             | 2.11          | 0.10                 | PL  | ... | ...    | 1FGL J0645.5+6033                                                                             | ... | ...   | ...                       | ... |
| J0647.7+0032  | 101.932 | 0.537   | 212.032 | -0.580  | 0.141      | 0.121      | 51     | 9.8      | 1.2      | 0.3             | 19.2     | 2.1             | 2.34          | ...                  | LP  | ... | 8,12   | 1FGL J0647.3+0031                                                                             | ... | ...   | ...                       | ... |
| J0647.7-5132  | 101.941 | -51.543 | 261.004 | -21.465 | 0.161      | 0.123      | 58     | 4.5      | 0.3      | 0.1             | 4.9      | 2.1             | 1.55          | 0.31                 | PL  | ... | ...    | ...                                                                                           | ... | agu   | 1RXS J064710.1-513546     | ... |
| J0647.8-6102  | 101.956 | -61.035 | 270.942 | -23.938 | 0.088      | 0.075      | -7     | 7.1      | 0.8      | 0.1             | 8.6      | 1.5             | 2.19          | 0.13                 | PL  | ... | ...    | 1FGL J0648.6-6052                                                                             | ... | agu   | PMN J0647-6058            | ... |
| J0648.7-1739  | 102.197 | -17.666 | 228.478 | -8.522  | 0.120      | 0.097      | 56     | 7.6      | 1.3      | 0.2             | 15.7     | 2.4             | 2.30          | 0.10                 | PL  | T   | ...    | 1FGL J0648.7-1740                                                                             | ... | bzq   | TXS 0646-176              | ... |
| J0648.9+1516  | 102.225 | 15.281  | 198.992 | 6.354   | 0.048      | 0.047      | -56    | 12.8     | 1.6      | 0.2             | 20.4     | 3.1             | 1.74          | 0.11                 | PL  | ... | ...    | 1FGL J0648.8+1516                                                                             | P   | bzb   | VER J0648+152             | ... |
| J0649.7-3138  | 102.438 | -31.644 | 241.528 | -14.170 | 0.088      | 0.079      | -50    | 6.5      | 0.6      | 0.2             | 8.8      | 2.3             | 1.69          | 0.17                 | PL  | ... | ...    | ...                                                                                           | ... | agu   | 1RXS J064933.8-313914     | ... |
| J0650.4-1632  | 102.619 | -16.548 | 227.642 | -7.669  | 0.243      | 0.135      | -60    | 4.4      | 0.9      | 0.2             | 10.9     | 2.4             | 2.30          | 0.12                 | PL  | ... | 8,9    | 1FGL J0650.6-1635                                                                             | ... | agu   | PKS 0648-16               | ... |
| J0650.7+2505  | 102.699 | 25.096  | 190.242 | 11.020  | 0.045      | 0.043      | 19     | 16.9     | 1.8      | 0.2             | 27.2     | 3.9             | 1.59          | 0.08                 | PL  | ... | ...    | 1FGL J0650.7+2503                                                                             | ... | bzb   | 1ES 0647+250              | ... |
| J0653.7+2818  | 103.436 | 28.306  | 187.536 | 12.950  | 0.096      | 0.089      | 43     | 5.7      | 0.5      | 0.1             | 6.4      | 1.6             | 1.90          | 0.15                 | PL  | ... | ...    | ...                                                                                           | ... | agu   | NVSS J065345+282010       | ... |
| J0654.2+4514  | 103.568 | 45.244  | 171.199 | 19.363  | 0.048      | 0.045      | 59     | 28.9     | 3.5      | 0.2             | 41.3     | 2.2             | 2.28          | 0.04                 | PL  | T   | ...    | 1FGL J0654.3+4514<br>0FGL J0654.3+4513                                                        | ... | bzq   | B3 0650+453               | ... |
| J0654.5+5043  | 103.649 | 50.718  | 165.680 | 21.144  | 0.044      | 0.041      | 5      | 23.7     | 2.8      | 0.2             | 31.1     | 2.4             | 2.04          | 0.05                 | PL  | T   | ...    | 1FGL J0654.4+5042<br>0FGL J0654.3+5042                                                        | ... | bzq   | GB6 J0654+5042            | ... |
| J0656.2-0320  | 104.058 | -3.340  | 216.451 | -0.458  | 0.073      | 0.071      | 10     | 17.2     | 3.5      | 0.4             | 40.8     | 2.9             | 2.44          | ...                  | LP  | T   | ...    | 1FGL J0656.2-0321                                                                             | ... | bzq   | TXS 0653-033              | ... |
| J0658.4+0633  | 104.612 | 6.556   | 207.882 | 4.537   | 0.135      | 0.116      | 26     | 4.4      | 0.7      | 0.2             | 8.0      | 1.8             | 2.31          | 0.15                 | PL  | ... | ...    | 1FGL J0658.5+0641                                                                             | ... | ...   | ...                       | ... |



Table 1—Continued

| Name 2FGL     | R.A.    | Decl.   | $l$     | $b$     | $\theta_1$ | $\theta_2$ | $\phi$ | $\sigma$ | $F_{35}$ | $\Delta F_{35}$ | $S_{25}$ | $\Delta S_{25}$ | $\Gamma_{25}$ | $\Delta \Gamma_{25}$ | Mod | Var | Flags | $\gamma$ -ray Assoc. | TeV | Class | ID or Assoc.          | Ref |
|---------------|---------|---------|---------|---------|------------|------------|--------|----------|----------|-----------------|----------|-----------------|---------------|----------------------|-----|-----|-------|----------------------|-----|-------|-----------------------|-----|
| J0659.7+1417  | 104.933 | 14.294  | 201.051 | 8.267   | 0.112      | 0.104      | -11    | 17.8     | 0.6      | 0.2             | 24.7     | 1.8             | 2.77          | ...                  | EC  | ... | ...   | 1FGL J0659.8+1414    | ... | PSR   | PSR J0659+1414        | ... |
| J0700.3+1710  | 105.077 | 17.181  | 198.480 | 9.648   | 0.181      | 0.139      | 36     | 6.5      | 0.6      | 0.1             | 9.5      | 1.6             | 2.50          | 0.13                 | PL  | T   | ...   | ...                  | ... | agu   | TXS 0657+172          | ... |
| J0700.3-6611  | 105.089 | -66.185 | 276.771 | -23.777 | 0.038      | 0.036      | 8      | 28.5     | 3.9      | 0.3             | 43.9     | 3.0             | 2.01          | 0.04                 | PL  | ... | ...   | 1FGL J0700.4-6611    | ... | bzb   | PKS 0700-661          | ... |
|               |         |         |         |         |            |            |        |          |          |                 |          |                 |               |                      |     |     |       | 0FGL J0700.0-6611    |     |       |                       |     |
| J0701.7-4630  | 105.446 | -46.516 | 256.761 | -17.650 | 0.115      | 0.096      | 65     | 14.4     | 1.5      | 0.2             | 15.6     | 1.5             | 2.40          | ...                  | LP  | T   | ...   | 1FGL J0702.0-4628    | ... | bzq   | PKS 0700-465          | ... |
| J0702.7-1951  | 105.686 | -19.861 | 231.935 | -6.525  | 0.100      | 0.089      | 67     | 5.8      | 1.0      | 0.2             | 11.8     | 2.6             | 1.86          | 0.12                 | PL  | ... | ...   | 1FGL J0702.2-1954    | ... | agu   | TXS 0700-197          | ... |
| J0703.1-3912  | 105.777 | -39.210 | 249.813 | -14.664 | 0.159      | 0.132      | -32    | 4.5      | 0.5      | 0.1             | 5.9      | 1.6             | 1.97          | 0.16                 | PL  | ... | ...   | ...                  | ... | agu   | NVSS J070312-391418   | ... |
| J0705.3-1043c | 106.344 | -10.720 | 224.053 | -1.814  | 0.273      | 0.173      | 59     | 4.1      | 1.2      | 0.3             | 15.6     | 3.4             | 2.37          | 0.12                 | PL  | ... | 4,5,6 | 1FGL J0705.9-1051c   | ... | ...   | ...                   | ... |
| J0706.5+3744  | 106.639 | 37.742  | 179.497 | 18.996  | 0.059      | 0.059      | 2      | 10.7     | 1.0      | 0.2             | 13.6     | 2.5             | 1.73          | 0.11                 | PL  | ... | ...   | 1FGL J0706.5+3744    | ... | bzb   | GB6 J0706+3744        | ... |
| J0706.5+7741  | 106.645 | 77.699  | 136.768 | 27.260  | 0.086      | 0.067      | -12    | 11.7     | 1.0      | 0.1             | 11.5     | 1.5             | 2.00          | 0.08                 | PL  | ... | ...   | 1FGL J0707.3+7742    | ... | agu   | NVSS J070651+774137   | ... |
| J0706.7-4845  | 106.698 | -48.759 | 259.276 | -17.674 | 0.217      | 0.130      | 44     | 7.8      | 0.9      | 0.1             | 10.2     | 1.6             | 2.27          | 0.11                 | PL  | ... | ...   | 1FGL J0706.3-4849    | ... | agu   | PMN J0705-4847        | ... |
| J0708.5-1020c | 107.125 | -10.349 | 224.076 | -0.962  | 0.181      | 0.167      | -16    | 6.2      | 1.4      | 0.4             | 15.6     | 3.0             | 2.36          | ...                  | LP  | ... | 4,5,6 | ...                  | ... | ...   | ...                   | ... |
| J0709.0+2236  | 107.274 | 22.600  | 194.341 | 13.797  | 0.194      | 0.149      | -85    | 5.2      | 0.6      | 0.1             | 6.7      | 1.4             | 2.27          | 0.15                 | PL  | T   | 11    | ...                  | ... | agu   | GB6 J0708+2241        | ... |
| J0709.3-0256  | 107.342 | -2.948  | 217.605 | 2.638   | 0.152      | 0.128      | -84    | 10.5     | 1.3      | 0.3             | 17.9     | 2.0             | 2.49          | ...                  | LP  | ... | ...   | ...                  | ... | agu   | PMN J0709-0255        | ... |
| J0710.5+5908  | 107.629 | 59.139  | 157.405 | 25.429  | 0.045      | 0.043      | 19     | 12.3     | 0.8      | 0.1             | 13.3     | 2.6             | 1.53          | 0.12                 | PL  | ... | ...   | 1FGL J0710.6+5911    | P   | bzb   | 1H 0658+595           | ... |
| J0710.8+4733  | 107.702 | 47.562  | 169.758 | 22.782  | 0.190      | 0.137      | 54     | 9.2      | 0.8      | 0.1             | 12.0     | 1.4             | 2.49          | 0.10                 | PL  | T   | ...   | 1FGL J0711.4+4731    | ... | bzb   | S4 0707+47            | ... |
| J0712.9+5032  | 108.228 | 50.537  | 166.728 | 23.889  | 0.067      | 0.061      | -57    | 15.5     | 1.7      | 0.2             | 19.2     | 2.0             | 2.06          | 0.07                 | PL  | T   | ...   | 1FGL J0712.7+5033    | ... | bzb   | GB6 J0712+5033        | ... |
|               |         |         |         |         |            |            |        |          |          |                 |          |                 |               |                      |     |     |       | 0FGL J0712.9+5034    |     |       |                       |     |
| J0713.5-0952  | 108.390 | -9.874  | 224.231 | 0.362   | 0.326      | 0.296      | 62     | 7.1      | 1.2      | 0.3             | 17.7     | 2.7             | 2.56          | ...                  | LP  | ... | ...   | 1FGL J0713.7-0950    | ... | ...   | ...                   | ... |
| J0714.0+1933  | 108.512 | 19.565  | 197.678 | 13.610  | 0.043      | 0.041      | -16    | 35.8     | 5.2      | 0.3             | 46.2     | 2.3             | 2.22          | ...                  | LP  | T   | ...   | 1FGL J0714.0+1935    | ... | bzq   | MG2 J071354+1934      | ... |
|               |         |         |         |         |            |            |        |          |          |                 |          |                 |               |                      |     |     |       | 0FGL J0714.2+1934    |     |       |                       |     |
| J0718.7-4320  | 109.680 | -43.343 | 254.934 | -13.657 | 0.043      | 0.039      | 0      | 18.9     | 2.5      | 0.2             | 28.8     | 3.0             | 1.88          | 0.06                 | PL  | ... | ...   | 1FGL J0718.7-4320    | ... | bzb   | PMN J0718-4319        | ... |
| J0719.2-5000  | 109.806 | -50.015 | 261.289 | -16.273 | 0.118      | 0.103      | 83     | 6.3      | 0.7      | 0.1             | 8.6      | 1.6             | 2.21          | 0.13                 | PL  | T   | ...   | 1FGL J0718.8-4958    | ... | ...   | ...                   | ... |
| J0719.3+3306  | 109.827 | 33.108  | 185.056 | 19.847  | 0.027      | 0.026      | -27    | 52.0     | 8.3      | 0.4             | 69.8     | 3.3             | 2.06          | ...                  | LP  | T   | ...   | 1FGL J0719.3+3306    | ... | bzq   | B2 0716+33            | ... |
|               |         |         |         |         |            |            |        |          |          |                 |          |                 |               |                      |     |     |       | 0FGL J0719.4+3302    |     |       |                       |     |
| J0721.2-0223  | 110.320 | -2.395  | 218.487 | 5.532   | 0.143      | 0.100      | 68     | 4.6      | 0.4      | 0.2             | 6.1      | 2.0             | 1.66          | 0.25                 | PL  | ... | ...   | ...                  | ... | agu   | 1RXS J072114.5-022047 | ... |
| J0721.5+0404c | 110.380 | 4.068   | 212.724 | 8.542   | 0.227      | 0.179      | 68     | 5.1      | 0.6      | 0.1             | 8.5      | 1.6             | 2.52          | 0.13                 | PL  | T   | 6     | 1FGL J0721.4+0401    | ... | bzq   | PMN J0721+0406        | ... |
| J0721.9+7120  | 110.476 | 71.350  | 143.974 | 28.019  | 0.016      | 0.015      | 28     | 115.2    | 18.3     | 0.4             | 183.4    | 5.3             | 2.08          | ...                  | LP  | T   | ...   | 1FGL J0721.9+7120    | P   | bzb   | S5 0716+71            | ... |
|               |         |         |         |         |            |            |        |          |          |                 |          |                 |               |                      |     |     |       | 0FGL J0722.0+7120    |     |       |                       |     |
|               |         |         |         |         |            |            |        |          |          |                 |          |                 |               |                      |     |     |       | 3EG J0721+7120       |     |       |                       |     |
|               |         |         |         |         |            |            |        |          |          |                 |          |                 |               |                      |     |     |       | EGR J0723+7134       |     |       |                       |     |
|               |         |         |         |         |            |            |        |          |          |                 |          |                 |               |                      |     |     |       | 1AGL J0722+7125      |     |       |                       |     |
| J0723.9+2901  | 110.997 | 29.031  | 189.482 | 19.356  | 0.138      | 0.130      | -20    | 8.0      | 0.7      | 0.1             | 9.6      | 1.4             | 2.40          | 0.13                 | PL  | T   | ...   | 1FGL J0723.6+2908    | ... | ...   | ...                   | ... |
| J0725.3+1426  | 111.331 | 14.443  | 203.628 | 13.928  | 0.028      | 0.027      | 34     | 57.6     | 9.6      | 0.4             | 91.0     | 3.5             | 2.18          | ...                  | LP  | T   | ...   | ...                  | ... | BZQ   | 4C +14.23             | 8   |
| J0725.6+2159  | 111.400 | 21.990  | 196.499 | 17.056  | 0.163      | 0.127      | -45    | 6.6      | 0.5      | 0.1             | 8.8      | 1.4             | 2.59          | 0.14                 | PL  | T   | 1,11  | ...                  | ... | bzq   | TXS 0723+220          | ... |

Table 1—Continued

| Name 2FGL    | R.A.    | Decl.   | $l$     | $b$     | $\theta_1$ | $\theta_2$ | $\phi$ | $\sigma$ | $F_{35}$ | $\Delta F_{35}$ | $S_{25}$ | $\Delta S_{25}$ | $\Gamma_{25}$ | $\Delta \Gamma_{25}$ | Mod | Var | Flags | $\gamma$ -ray Assoc.                                                       | TeV | Class | ID or Assoc.          | Ref. |
|--------------|---------|---------|---------|---------|------------|------------|--------|----------|----------|-----------------|----------|-----------------|---------------|----------------------|-----|-----|-------|----------------------------------------------------------------------------|-----|-------|-----------------------|------|
| J0725.8–0549 | 111.451 | –5.821  | 222.059 | 4.935   | 0.105      | 0.087      | –23    | 4.1      | 0.4      | 0.1             | 5.3      | 1.8             | 1.78          | 0.24                 | PL  | ... | ...   | ...                                                                        | ... | ...   | ...                   | ...  |
| J0726.0–0053 | 111.511 | –0.899  | 217.706 | 7.279   | 0.097      | 0.079      | 39     | 9.2      | 1.1      | 0.2             | 12.9     | 1.7             | 2.27          | 0.10                 | PL  | ... | ...   | 1FGL J0725.9–0053                                                          | ... | agu   | PKS 0723–008          | ...  |
| J0727.0–4726 | 111.765 | –47.447 | 259.404 | –14.047 | 0.221      | 0.183      | –60    | 7.8      | 1.1      | 0.2             | 13.3     | 1.8             | 2.34          | 0.09                 | PL  | ... | ...   | 3EG J0724–4713<br>EGR J0726–4715                                           | ... | bzq   | PMN J0726–4728        | ...  |
| J0729.9+3304 | 112.486 | 33.076  | 185.884 | 21.936  | 0.100      | 0.087      | 85     | 5.8      | 0.5      | 0.1             | 6.2      | 1.6             | 1.89          | 0.18                 | PL  | ... | ...   | 1FGL J0730.0+3305                                                          | ... | bzb   | 1RXS J073026.0+330727 | ...  |
| J0730.2–1141 | 112.572 | –11.696 | 227.773 | 3.130   | 0.019      | 0.019      | –86    | 92.6     | 22.0     | 0.6             | 228.8    | 4.7             | 2.28          | ...                  | LP  | T   | ...   | 1FGL J0730.3–1141<br>0FGL J0730.4–1142                                     | ... | bzq   | PKS 0727–11           | ...  |
| J0730.6–6607 | 112.674 | –66.118 | 277.667 | –20.825 | 0.103      | 0.082      | 43     | 5.3      | 0.3      | 0.1             | 6.6      | 2.4             | 1.34          | 0.28                 | PL  | ... | 1     | ...                                                                        | ... | agu   | PMN J0730–6602        | ...  |
| J0733.9+5023 | 113.485 | 50.400  | 167.675 | 27.126  | 0.154      | 0.121      | –74    | 7.4      | 0.7      | 0.1             | 8.2      | 1.3             | 2.35          | 0.12                 | PL  | T   | ...   | ...                                                                        | ... | bzq   | TXS 0730+504          | ...  |
| J0734.2–7706 | 113.571 | –77.115 | 289.049 | –24.055 | 0.116      | 0.109      | –71    | 8.1      | 1.0      | 0.2             | 13.0     | 1.8             | 2.37          | 0.10                 | PL  | T   | ...   | 1FGL J0734.1–7715                                                          | ... | agu   | PKS 0736–770          | ...  |
| J0734.6–1558 | 113.670 | –15.972 | 232.039 | 2.006   | 0.056      | 0.054      | –27    | 26.1     | 5.8      | 0.4             | 53.7     | 2.7             | 2.33          | ...                  | EC  | ... | ...   | 1FGL J0734.7–1557                                                          | ... | PSR   | LAT PSR J0734–1559    | ...  |
| J0737.1–3235 | 114.294 | –32.587 | 246.859 | –5.562  | 0.141      | 0.125      | –67    | 6.9      | 1.3      | 0.2             | 16.6     | 2.5             | 2.33          | 0.11                 | PL  | T   | ...   | 1FGL J0737.4–3239                                                          | ... | ...   | ...                   | ...  |
| J0737.5–8246 | 114.385 | –82.774 | 295.086 | –25.467 | 0.099      | 0.090      | –62    | 4.4      | 0.3      | 0.1             | 6.0      | 2.4             | 1.35          | 0.30                 | PL  | ... | ...   | ...                                                                        | ... | ...   | ...                   | ...  |
| J0738.0+1742 | 114.524 | 17.703  | 201.847 | 18.064  | 0.035      | 0.033      | 80     | 36.8     | 5.2      | 0.3             | 57.4     | 3.2             | 2.05          | 0.03                 | PL  | ... | ...   | 1FGL J0738.2+1741<br>0FGL J0738.2+1738<br>3EG J0737+1721<br>EGR J0737+1720 | ... | bzb   | PKS 0735+17<br>18     | ...  |
| J0739.2+0138 | 114.819 | 1.648   | 216.960 | 11.389  | 0.066      | 0.061      | –63    | 26.2     | 2.5      | 0.2             | 34.3     | 1.8             | 2.48          | ...                  | LP  | T   | ...   | 1FGL J0739.1+0138                                                          | ... | bzq   | PKS 0736+01           | ...  |
| J0742.4–2821 | 115.624 | –28.366 | 243.728 | –2.499  | 0.206      | 0.154      | 41     | 6.4      | 1.6      | 0.3             | 11.8     | 2.1             | 2.26          | ...                  | EC  | ... | 4     | 1FGL J0742.8–2822                                                          | ... | PSR   | PSR J0742–2822        | ...  |
| J0742.6+5442 | 115.652 | 54.713  | 163.068 | 29.081  | 0.061      | 0.058      | –74    | 25.1     | 2.5      | 0.2             | 30.8     | 1.8             | 2.31          | 0.05                 | PL  | T   | ...   | 1FGL J0742.2+5443<br>3EG J0743+5447<br>EGR J0743+5438                      | ... | bzq   | GB6 J0742+5444        | ...  |
| J0742.7–3113 | 115.678 | –31.225 | 246.240 | –3.872  | 0.188      | 0.155      | 43     | 5.2      | 1.1      | 0.2             | 12.7     | 2.5             | 2.27          | 0.13                 | PL  | ... | 4     | 1FGL J0743.0–3110                                                          | ... | ...   | ...                   | ...  |
| J0744.1–2523 | 116.048 | –25.399 | 241.341 | –0.696  | 0.080      | 0.076      | 24     | 12.4     | 3.0      | 0.3             | 22.0     | 2.3             | 2.24          | ...                  | LP  | ... | ...   | 1FGL J0744.1–2523                                                          | ... | ...   | ...                   | ...  |
| J0745.0+7436 | 116.275 | 74.602  | 140.219 | 29.633  | 0.120      | 0.093      | 24     | 7.9      | 0.6      | 0.1             | 7.7      | 1.6             | 1.80          | 0.14                 | PL  | ... | ...   | 1FGL J0745.2+7438                                                          | ... | bzb   | MS 0737.9+7441        | ...  |
| J0745.5+7910 | 116.399 | 79.178  | 134.995 | 29.143  | 0.125      | 0.115      | –6     | 5.5      | 0.4      | 0.1             | 4.7      | 1.0             | 2.23          | 0.14                 | PL  | ... | ...   | ...                                                                        | ... | ...   | ...                   | ...  |
| J0745.9+8512 | 116.486 | 85.209  | 128.215 | 28.158  | 0.132      | 0.087      | 24     | 5.0      | 0.3      | 0.1             | 4.5      | 1.4             | 1.68          | 0.18                 | PL  | ... | ...   | ...                                                                        | ... | agu   | NVSS J074715+851208   | ...  |
| J0746.0–0222 | 116.523 | –2.369  | 221.392 | 11.023  | 0.150      | 0.088      | –54    | 7.3      | 0.7      | 0.1             | 9.7      | 2.4             | 1.67          | 0.15                 | PL  | ... | ...   | ...                                                                        | ... | ...   | ...                   | ...  |
| J0746.5–0713 | 116.637 | –7.217  | 225.768 | 8.800   | 0.151      | 0.139      | –50    | 4.7      | 0.6      | 0.1             | 7.0      | 1.7             | 1.99          | 0.15                 | PL  | ... | ...   | 1FGL J0746.5–0711                                                          | ... | agu   | PMN J0746–0709        | ...  |
| J0746.5–4758 | 116.646 | –47.972 | 261.391 | –11.345 | 0.090      | 0.084      | 84     | 4.8      | 0.6      | 0.2             | 6.7      | 1.8             | 1.95          | 0.17                 | PL  | ... | ...   | ...                                                                        | ... | agu   | CRATES J0746–4754     | ...  |
| J0746.6+2549 | 116.668 | 25.829  | 194.590 | 22.946  | 0.200      | 0.163      | 61     | 11.1     | 0.6      | 0.1             | 14.1     | 1.4             | 2.85          | 0.11                 | PL  | T   | ...   | 1FGL J0746.6+2548                                                          | ... | bzq   | B2 0743+25            | ...  |
| J0747.2–1654 | 116.806 | –16.905 | 234.334 | 4.166   | 0.371      | 0.226      | 19     | 4.6      | 0.7      | 0.2             | 10.1     | 2.0             | 2.53          | 0.13                 | PL  | ... | 9     | ...                                                                        | ... | agu   | TXS 0745–165          | ...  |
| J0747.5–3305 | 116.889 | –33.092 | 248.374 | –3.911  | 0.124      | 0.101      | 74     | 9.0      | 2.6      | 0.4             | 17.7     | 2.6             | 2.23          | ...                  | LP  | ... | 3     | 1FGL J0747.4–3303                                                          | ... | agu   | PKS 0745–330          | ...  |
| J0747.7+4501 | 116.949 | 45.029  | 174.130 | 28.406  | 0.301      | 0.224      | –65    | 4.6      | 0.5      | 0.1             | 5.7      | 1.2             | 2.24          | 0.16                 | PL  | ... | ...   | ...                                                                        | ... | bzq   | B3 0745+453           | ...  |
| J0748.5–2204 | 117.139 | –22.075 | 238.968 | 1.837   | 0.214      | 0.171      | –36    | 5.2      | 0.9      | 0.2             | 13.0     | 2.3             | 2.49          | 0.12                 | PL  | ... | 4     | ...                                                                        | ... | ...   | ...                   | ...  |

Table 1—Continued

| Name 2FGL     | R.A.    | Decl.   | $l$     | $b$     | $\theta_1$ | $\theta_2$ | $\phi$ | $\sigma$ | $F_{35}$ | $\Delta F_{35}$ | $S_{25}$ | $\Delta S_{25}$ | $\Gamma_{25}$ | $\Delta \Gamma_{25}$ | Mod | Var | Flags | $\gamma$ -ray Assoc. | TeV | Class | ID or Assoc.        | Ref. |
|---------------|---------|---------|---------|---------|------------|------------|--------|----------|----------|-----------------|----------|-----------------|---------------|----------------------|-----|-----|-------|----------------------|-----|-------|---------------------|------|
| J0750.6+1230  | 117.652 | 12.514  | 208.137 | 18.702  | 0.102      | 0.092      | 32     | 15.8     | 1.5      | 0.2             | 20.1     | 1.6             | 2.42          | 0.07                 | PL  | T   | ...   | 1FGL J0750.6+1235    | ... | bzq   | OI 280              | ...  |
| J0751.1+1809  | 117.780 | 18.152  | 202.702 | 21.088  | 0.069      | 0.063      | 27     | 18.3     | 2.6      | 0.2             | 14.6     | 1.4             | 2.06          | ...                  | EC  | ... | ...   | 1FGL J0751.1+1807    | ... | PSR   | PSR J0751+1807      | ...  |
| J0753.0+5352  | 118.264 | 53.869  | 164.217 | 30.510  | 0.074      | 0.066      | -66    | 12.3     | 1.2      | 0.1             | 13.1     | 1.7             | 2.01          | 0.09                 | PL  | ... | ...   | 1FGL J0752.8+5353    | ... | bzb   | 4C +54.15           | ...  |
| J0753.2-1634  | 118.318 | -16.576 | 234.781 | 5.582   | 0.387      | 0.167      | -48    | 4.3      | 0.6      | 0.1             | 6.5      | 1.6             | 2.12          | 0.18                 | PL  | ... | 9     | ...                  | ... | ...   | ...                 | ...  |
| J0753.2+1937  | 118.320 | 19.623  | 201.452 | 22.124  | 0.168      | 0.162      | -84    | 4.5      | 0.3      | 0.1             | 7.0      | 1.4             | 2.89          | 0.19                 | PL  | T   | 11    | ...                  | ... | ...   | ...                 | ...  |
| J0754.4-1147  | 118.603 | -11.786 | 230.755 | 8.237   | 0.089      | 0.074      | -2     | 10.2     | 1.4      | 0.2             | 15.9     | 2.3             | 1.98          | 0.09                 | PL  | ... | ...   | 1FGL J0754.4-1147    | ... | bzb   | TXS 0752-116        | ...  |
| J0754.8+4824  | 118.715 | 48.410  | 170.539 | 30.162  | 0.082      | 0.074      | -37    | 12.2     | 1.1      | 0.1             | 12.9     | 1.5             | 2.19          | 0.09                 | PL  | ... | ...   | ...                  | ... | bzb   | GB1 0751+485        | ...  |
| J0756.3-6433  | 119.077 | -64.563 | 277.270 | -17.759 | 0.077      | 0.074      | -63    | 4.5      | 0.3      | 0.2             | 4.4      | 1.5             | 1.78          | 0.32                 | PL  | ... | ...   | ...                  | ... | ...   | ...                 | ...  |
| J0757.1+0957  | 119.288 | 9.963   | 211.298 | 19.074  | 0.058      | 0.052      | -54    | 18.9     | 2.0      | 0.2             | 23.4     | 1.9             | 2.19          | 0.06                 | PL  | T   | ...   | 1FGL J0757.2+0956    | ... | bzb   | PKS 0754+100        | ...  |
| J0758.0-2615c | 119.501 | -26.257 | 243.664 | 1.539   | 0.239      | 0.188      | -30    | 5.1      | 0.9      | 0.2             | 11.5     | 2.2             | 2.35          | 0.11                 | PL  | ... | 1,6,9 | ...                  | ... | ...   | ...                 | ...  |
| J0758.8-1448  | 119.724 | -14.808 | 233.943 | 7.648   | 0.156      | 0.124      | 46     | 5.8      | 0.7      | 0.1             | 8.3      | 1.6             | 2.25          | 0.13                 | PL  | ... | ...   | 1FGL J0758.6-1450    | ... | ...   | ...                 | ...  |
| J0801.5+4401  | 120.388 | 44.028  | 175.764 | 30.640  | 0.145      | 0.137      | 42     | 6.3      | 0.6      | 0.1             | 6.7      | 1.2             | 2.26          | 0.14                 | PL  | ... | ...   | 1FGL J0800.5+4407    | ... | bzb   | B3 0757+441         | ...  |
| J0802.6-0940  | 120.664 | -9.668  | 229.930 | 11.052  | 0.107      | 0.098      | -7     | 5.2      | 0.5      | 0.1             | 5.9      | 1.6             | 1.97          | 0.21                 | PL  | ... | ...   | ...                  | ... | ...   | ...                 | ...  |
| J0802.7-5615  | 120.692 | -56.259 | 270.042 | -13.167 | 0.128      | 0.112      | 56     | 5.3      | 0.7      | 0.2             | 8.8      | 1.7             | 2.25          | 0.13                 | PL  | ... | ...   | 1FGL J0802.4-5622    | ... | ...   | ...                 | ...  |
| J0803.2-0339  | 120.804 | -3.654  | 224.650 | 14.157  | 0.091      | 0.074      | 39     | 11.5     | 1.2      | 0.2             | 13.8     | 2.0             | 1.97          | 0.10                 | PL  | T   | ...   | 1FGL J0803.1-0339    | ... | ...   | ...                 | ...  |
| J0805.2-0121  | 121.312 | -1.356  | 222.822 | 15.714  | 0.194      | 0.159      | -41    | 4.7      | 0.5      | 0.1             | 5.3      | 1.3             | 2.14          | 0.16                 | PL  | T   | ...   | ...                  | ... | bzq   | PKS B0805-010       | ...  |
| J0805.3+7535  | 121.342 | 75.588  | 138.881 | 30.788  | 0.057      | 0.049      | -70    | 16.9     | 1.5      | 0.1             | 20.2     | 2.7             | 1.68          | 0.07                 | PL  | T   | ...   | 1FGL J0804.7+7534    | ... | bzb   | RX J0805.4+7534     | ...  |
| J0805.5+6145  | 121.387 | 61.755  | 155.027 | 32.380  | 0.125      | 0.109      | -59    | 18.0     | 1.0      | 0.1             | 20.2     | 1.3             | 2.74          | 0.07                 | PL  | T   | ...   | 1FGL J0806.2+6148    | ... | bzq   | TXS 0800+618        | ...  |
| J0807.0-6511  | 121.774 | -65.189 | 278.402 | -17.028 | 0.186      | 0.134      | 65     | 4.4      | 0.2      | 0.1             | 5.8      | 2.5             | 1.10          | 0.41                 | PL  | ... | ...   | ...                  | ... | ...   | ...                 | ...  |
| J0807.1-0543  | 121.782 | -5.723  | 227.002 | 13.988  | 0.069      | 0.065      | 51     | 11.8     | 1.3      | 0.2             | 14.9     | 1.9             | 2.10          | 0.10                 | PL  | ... | ...   | 1FGL J0807.0-0544    | ... | bzb   | PKS 0804-05         | ...  |
| J0808.2-0750  | 122.059 | -7.850  | 229.037 | 13.160  | 0.021      | 0.020      | -29    | 71.3     | 15.0     | 0.5             | 136.3    | 5.2             | 2.04          | ...                  | LP  | T   | ...   | 1FGL J0808.2-0750    | ... | bzq   | PKS 0805-07         | ...  |
| J0809.8+5218  | 122.460 | 52.308  | 166.255 | 32.913  | 0.043      | 0.038      | -79    | 22.8     | 2.4      | 0.2             | 27.9     | 2.5             | 1.94          | 0.06                 | PL  | T   | ...   | 1FGL J0809.5+5219    | P   | bzb   | 1ES 0806+524        | ...  |
| J0811.1-7527  | 122.791 | -75.466 | 288.252 | -21.423 | 0.041      | 0.038      | 30     | 20.7     | 2.7      | 0.2             | 35.5     | 3.9             | 1.71          | 0.06                 | PL  | ... | ...   | 1FGL J0811.1-7527    | ... | bzb   | PMN J0810-7530      | ...  |
| J0811.4+0149  | 122.874 | 1.832   | 220.666 | 18.604  | 0.097      | 0.076      | 60     | 12.9     | 1.3      | 0.2             | 14.8     | 1.6             | 2.26          | 0.08                 | PL  | ... | ...   | 1FGL J0811.2+0148    | ... | bzb   | OJ 014              | ...  |
| J0812.6+6511  | 123.153 | 65.184  | 150.898 | 32.918  | 0.144      | 0.113      | -81    | 4.1      | 0.4      | 0.1             | 4.3      | 1.2             | 2.12          | 0.21                 | PL  | ... | 5     | ...                  | ... | agu   | GB6 J0812+6508      | ...  |
| J0814.0-1006  | 123.503 | -10.115 | 231.785 | 13.227  | 0.146      | 0.113      | -32    | 7.9      | 1.1      | 0.2             | 13.2     | 1.9             | 2.23          | 0.11                 | PL  | ... | ...   | 1FGL J0814.5-1011    | ... | bzb   | NVSS J081411-101208 | ...  |
| J0814.7+6429  | 123.682 | 64.486  | 151.698 | 33.216  | 0.066      | 0.065      | 74     | 13.4     | 1.3      | 0.1             | 15.3     | 1.5             | 2.26          | 0.08                 | PL  | T   | ...   | 1FGL J0815.0+6434    | ... | bzb   | GB6 J0814+6431      | ...  |
| J0816.4-1311  | 124.109 | -13.190 | 234.789 | 12.123  | 0.038      | 0.036      | -85    | 21.2     | 2.8      | 0.2             | 34.1     | 3.6             | 1.80          | 0.06                 | PL  | T   | ...   | 1FGL J0816.4-1311    | ... | bzb   | PMN J0816-1311      | ...  |
| J0816.5+5739  | 124.125 | 57.652  | 159.862 | 33.913  | 0.079      | 0.072      | -62    | 10.8     | 1.0      | 0.1             | 10.9     | 1.6             | 1.98          | 0.11                 | PL  | T   | ...   | 1FGL J0816.7+5739    | ... | bzb   | SBS 0812+578        | ...  |
| J0816.7-2420  | 124.189 | -24.347 | 244.332 | 6.140   | 0.107      | 0.093      | -44    | 8.1      | 1.0      | 0.2             | 11.8     | 1.7             | 2.32          | 0.10                 | PL  | T   | ...   | ...                  | ... | agu   | PMN J0816-2421      | ...  |
| J0816.9+2049  | 124.250 | 20.823  | 202.456 | 27.742  | 0.212      | 0.183      | -64    | 5.7      | 0.4      | 0.1             | 7.3      | 1.3             | 2.60          | 0.15                 | PL  | ... | ...   | ...                  | ... | bzb   | BZB J0816+2051      | ...  |
| J0817.9+3238  | 124.486 | 32.650  | 189.536 | 31.479  | 0.117      | 0.101      | 0      | 5.7      | 0.5      | 0.1             | 5.7      | 1.2             | 2.19          | 0.15                 | PL  | ... | ...   | ...                  | ... | bzb   | RX J0817.9+3243     | ...  |
| J0818.2-0935  | 124.559 | -9.593  | 231.882 | 14.388  | 0.079      | 0.073      | -81    | 11.7     | 1.5      | 0.2             | 16.9     | 2.1             | 2.04          | 0.09                 | PL  | ... | ...   | 1FGL J0818.0-0938    | ... | bzb   | TXS 0815-094        | ...  |
| J0818.2+4223  | 124.573 | 42.398  | 178.206 | 33.409  | 0.029      | 0.028      | 56     | 51.0     | 7.2      | 0.3             | 80.9     | 3.2             | 2.14          | 0.03                 | PL  | T   | 10    | 1FGL J0818.2+4222    | ... | bzb   | S4 0814+42          | ...  |
|               |         |         |         |         |            |            |        |          |          |                 |          |                 |               |                      |     |     |       | 0FGL J0818.3+4222    |     |       |                     |      |

Table 1—Continued

| Name 2FGL     | R.A.    | Decl.   | $l$     | $b$    | $\theta_1$ | $\theta_2$ | $\phi$ | $\sigma$ | $F_{35}$ | $\Delta F_{35}$ | $S_{25}$ | $\Delta S_{25}$ | $\Gamma_{25}$ | $\Delta \Gamma_{25}$ | Mod | Var | Flags | $\gamma$ -ray Assoc. | TeV | Class | ID or Assoc.           |
|---------------|---------|---------|---------|--------|------------|------------|--------|----------|----------|-----------------|----------|-----------------|---------------|----------------------|-----|-----|-------|----------------------|-----|-------|------------------------|
| J0819.3+2750  | 124.826 | 27.844  | 195.032 | 30.488 | 0.158      | 0.146      | −76    | 4.5      | 0.4      | 0.1             | 4.3      | 1.1             | 2.26          | 0.22                 | PL  | ... | ...   | ...                  | ... | bzb   | 5C 07.119              |
| J0819.6−0803  | 124.906 | −8.056  | 230.706 | 15.478 | 0.153      | 0.122      | −8     | 4.4      | 0.3      | 0.1             | 5.3      | 2.0             | 1.58          | 0.24                 | PL  | ... | ...   | ...                  | ... | bzb   | RX J0819.2−0756        |
| J0821.0−4254  | 125.250 | −42.914 | 260.208 | −3.565 | 0.099      | 0.078      | 26     | 4.8      | 1.5      | 0.4             | 17.3     | 4.2             | 1.99          | 0.14                 | PL  | ... | 5     | ...                  | ... | †     | ...                    |
| J0823.0−4246  | 125.766 | −42.770 | 260.305 | −3.173 | 0.085      | 0.073      | −61    | 10.2     | 5.7      | 0.6             | 40.9     | 4.7             | 2.09          | ...                  | LP  | ... | 3     | 1FGL J0823.3−4248    | ... | †     | ...                    |
| J0823.0+4041  | 125.767 | 40.687  | 180.394 | 34.053 | 0.116      | 0.097      | 67     | 7.2      | 0.7      | 0.1             | 8.3      | 1.4             | 2.30          | 0.14                 | PL  | T   | ...   | ...                  | ... | agu   | B3 0819+408            |
| J0823.4−4305  | 125.858 | −43.092 | 260.608 | −3.301 | 0.116      | 0.085      | 56     | 5.1      | 1.4      | 0.4             | 17.4     | 4.2             | 1.76          | 0.17                 | PL  | ... | 5     | ...                  | ... | †     | ...                    |
| J0824.7+3914  | 126.175 | 39.245  | 182.173 | 34.144 | 0.164      | 0.159      | −10    | 5.5      | 0.4      | 0.1             | 7.2      | 1.3             | 2.64          | 0.17                 | PL  | ... | ...   | ...                  | ... | bzq   | 4C +39.23              |
| J0824.9+5552  | 126.234 | 55.877  | 161.959 | 35.139 | 0.106      | 0.099      | 5      | 14.0     | 0.8      | 0.1             | 15.7     | 1.3             | 2.68          | 0.08                 | PL  | T   | ...   | 1FGL J0825.0+5555    | ... | bzq   | OJ 535                 |
|               |         |         |         |        |            |            |        |          |          |                 |          |                 |               |                      |     |     |       | 0FGL J0824.9+5551    |     |       |                        |
| J0825.9+0308  | 126.478 | 3.144   | 221.241 | 22.398 | 0.119      | 0.097      | −32    | 7.2      | 0.7      | 0.1             | 7.6      | 1.5             | 1.97          | 0.17                 | PL  | ... | ...   | 1FGL J0825.9+0309    | ... | bzb   | PKS 0823+033           |
| J0825.9−2229  | 126.481 | −22.499 | 243.970 | 8.916  | 0.040      | 0.036      | −33    | 30.3     | 4.5      | 0.3             | 50.5     | 3.1             | 2.08          | 0.04                 | PL  | T   | ...   | 1FGL J0825.8−2230    | ... | bzb   | PKS 0823−223           |
|               |         |         |         |        |            |            |        |          |          |                 |          |                 |               |                      |     |     |       | 0FGL J0826.0−2228    |     |       |                        |
| J0825.9−3216  | 126.485 | −32.275 | 252.042 | 3.329  | 0.124      | 0.101      | −84    | 6.9      | 1.0      | 0.2             | 13.0     | 2.0             | 2.40          | 0.11                 | PL  | T   | ...   | 1FGL J0825.9−3216    | ... | agu   | PKS 0823−321           |
| J0830.5+2407  | 127.646 | 24.122  | 200.067 | 31.796 | 0.100      | 0.091      | −67    | 17.3     | 1.1      | 0.1             | 20.9     | 1.4             | 2.67          | 0.07                 | PL  | T   | ...   | 1FGL J0830.5+2407    | ... | bzq   | S3 0827+24             |
|               |         |         |         |        |            |            |        |          |          |                 |          |                 |               |                      |     |     |       | 3EG J0829+2413       |     |       |                        |
|               |         |         |         |        |            |            |        |          |          |                 |          |                 |               |                      |     |     |       | EGR J0829+2415       |     |       | 20                     |
| J0831.9+0429  | 127.987 | 4.486   | 220.719 | 24.357 | 0.038      | 0.037      | 56     | 38.4     | 5.0      | 0.3             | 46.6     | 2.6             | 2.18          | ...                  | LP  | T   | ...   | 1FGL J0831.6+0429    | ... | bzb   | PKS 0829+046           |
| J0833.1−4511e | 128.287 | −45.190 | 263.332 | −3.106 | ...        | ...        | ...    | ...      | 18.3     | ...             | 244.8    | ...             | 2.41          | ...                  | PL  | ... | 5     | ...                  | ... | PWN   | Vela−X                 |
| J0834.3+4400  | 128.587 | 44.012  | 176.628 | 36.489 | 0.097      | 0.086      | 24     | 6.2      | 0.5      | 0.1             | 5.3      | 1.2             | 2.04          | 0.19                 | PL  | ... | ...   | ...                  | ... | bzb   | B3 0831+442            |
| J0834.3+4221  | 128.592 | 42.366  | 178.666 | 36.354 | 0.128      | 0.123      | −45    | 8.0      | 0.7      | 0.1             | 8.8      | 1.3             | 2.33          | 0.13                 | PL  | ... | ...   | 1FGL J0834.4+4221    | ... | bzq   | OJ 451                 |
| J0835.3−4510  | 128.839 | −45.179 | 263.556 | −2.787 | 0.006      | 0.006      | 20     | 1027.8   | 1357.9   | 4.1             | 9209.4   | 22.7            | 1.97          | ...                  | EC  | ... | 10    | 1FGL J0835.3−4510    | E   | PSR   | PSR J0835−4510         |
|               |         |         |         |        |            |            |        |          |          |                 |          |                 |               |                      |     |     |       | 0FGL J0835.4−4510    |     |       | Vela                   |
|               |         |         |         |        |            |            |        |          |          |                 |          |                 |               |                      |     |     |       | 3EG J0834−4511       |     |       |                        |
|               |         |         |         |        |            |            |        |          |          |                 |          |                 |               |                      |     |     |       | EGR J0834−4512       |     |       |                        |
|               |         |         |         |        |            |            |        |          |          |                 |          |                 |               |                      |     |     |       | 1AGL J0835−4509      |     |       |                        |
| J0838.8−2828  | 129.714 | −28.476 | 250.599 | 7.816  | 0.100      | 0.077      | 78     | 8.2      | 1.1      | 0.2             | 12.2     | 2.0             | 2.00          | 0.10                 | PL  | ... | ...   | 1FGL J0838.6−2828    | ... | ...   | ...                    |
| J0839.4+1802  | 129.863 | 18.036  | 207.626 | 31.696 | 0.137      | 0.128      | 8      | 4.9      | 0.4      | 0.1             | 5.4      | 1.2             | 2.46          | 0.20                 | PL  | T   | 11    | ...                  | ... | bzb   | TXS 0836+182           |
| J0839.6+0059  | 129.900 | 0.998   | 225.085 | 24.362 | 0.105      | 0.093      | −1     | 8.3      | 0.8      | 0.1             | 9.1      | 1.4             | 2.21          | 0.11                 | PL  | T   | ...   | 1FGL J0839.5+0059    | ... | bzq   | PKS 0837+012           |
| J0839.7+3541  | 129.947 | 35.689  | 187.068 | 36.524 | 0.168      | 0.134      | −22    | 5.0      | 0.4      | 0.1             | 5.1      | 1.4             | 1.92          | 0.18                 | PL  | ... | ...   | ...                  | ... | bzb   | FIRST J083943.3+354001 |
| J0840.7+1310  | 130.191 | 13.180  | 212.993 | 30.122 | 0.142      | 0.135      | 10     | 8.0      | 0.8      | 0.1             | 9.6      | 1.4             | 2.36          | 0.11                 | PL  | T   | ...   | 1FGL J0840.8+1310    | ... | rdg   | 3C 207                 |
| J0841.3−3556  | 130.340 | −35.939 | 256.894 | 3.720  | 0.053      | 0.048      | 45     | 12.2     | 1.7      | 0.2             | 23.6     | 3.7             | 1.66          | 0.09                 | PL  | T   | ...   | 1FGL J0841.4−3558    | ... | ...   | ...                    |
| J0841.6+7052  | 130.420 | 70.880  | 143.550 | 34.451 | 0.113      | 0.104      | −15    | 16.0     | 0.7      | 0.1             | 21.0     | 1.4             | 2.95          | 0.07                 | PL  | T   | ...   | 1FGL J0842.2+7054    | ... | bzq   | 4C +71.07              |
|               |         |         |         |        |            |            |        |          |          |                 |          |                 |               |                      |     |     |       | 3EG J0845+7049       |     |       |                        |
| J0842.9−4721  | 130.741 | −47.365 | 266.094 | −3.070 | 0.120      | 0.116      | 49     | 12.4     | 1.4      | 0.2             | 42.0     | 3.7             | 2.60          | ...                  | LP  | ... | 12    | ...                  | ... | †     | ...                    |
| J0843.6+6715  | 130.903 | 67.259  | 147.746 | 35.612 | 0.108      | 0.087      | 47     | 7.4      | 0.6      | 0.1             | 6.6      | 1.2             | 2.02          | 0.13                 | PL  | ... | ...   | 1FGL J0843.4+6718    | ... | ...   | ...                    |

Table 1—Continued

| Name 2FGL    | R.A.    | Decl.   | $l$     | $b$    | $\theta_1$ | $\theta_2$ | $\phi$ | $\sigma$ | $F_{35}$ | $\Delta F_{35}$ | $S_{25}$ | $\Delta S_{25}$ | $\Gamma_{25}$ | $\Delta \Gamma_{25}$ | Mod | Var | Flags    | $\gamma$ -ray Assoc. | TeV | Class | ID or Assoc.          | Ref. |
|--------------|---------|---------|---------|--------|------------|------------|--------|----------|----------|-----------------|----------|-----------------|---------------|----------------------|-----|-----|----------|----------------------|-----|-------|-----------------------|------|
| J0843.9+5312 | 130.982 | 53.209  | 165.060 | 38.054 | 0.099      | 0.093      | -62    | 6.7      | 0.5      | 0.1             | 6.0      | 1.1             | 2.09          | 0.15                 | PL  | ... | ...      | 1FGL J0844.0+5314    | ... | bzb   | BZB J0844+5312        | ...  |
| J0844.8-5459 | 131.210 | -54.987 | 272.313 | -7.526 | 0.091      | 0.078      | -57    | 10.3     | 1.7      | 0.2             | 18.6     | 2.4             | 2.07          | 0.08                 | PL  | ... | ...      | 1FGL J0845.0-5459    | ... | agu   | PMN J0845-5458        | ...  |
| J0844.9+6214 | 131.230 | 62.249  | 153.753 | 36.902 | 0.180      | 0.155      | -32    | 4.1      | 0.4      | 0.1             | 4.8      | 1.1             | 2.42          | 0.18                 | PL  | ... | ...      | ...                  | ... | ...   | ...                   | ...  |
| J0846.0+2820 | 131.511 | 28.348  | 196.336 | 36.305 | 0.272      | 0.174      | 79     | 4.1      | 0.3      | 0.1             | 5.1      | 1.2             | 2.51          | 0.20                 | PL  | ... | ...      | ...                  | ... | ...   | ...                   | ...  |
| J0846.7-4053 | 131.696 | -40.898 | 261.451 | 1.485  | 0.166      | 0.139      | -65    | 5.3      | 1.4      | 0.3             | 19.9     | 3.6             | 2.48          | 0.12                 | PL  | T   | 1,4      | ...                  | ... | ...   | ...                   | ...  |
| J0847.0-2334 | 131.754 | -23.570 | 247.737 | 12.230 | 0.142      | 0.123      | 69     | 7.6      | 1.0      | 0.2             | 10.9     | 1.7             | 2.19          | 0.11                 | PL  | ... | ...      | 1FGL J0846.9-2334    | ... | agn   | PMN J0847-2337        | ...  |
| J0847.2+1134 | 131.813 | 11.573  | 215.451 | 30.902 | 0.089      | 0.077      | 75     | 7.8      | 0.5      | 0.1             | 9.3      | 2.6             | 1.48          | 0.16                 | PL  | ... | ...      | 1FGL J0847.2+1134    | ... | bzb   | RX J0847.1+1133       | ...  |
| J0848.1-0703 | 132.028 | -7.053  | 233.770 | 21.993 | 0.189      | 0.161      | 27     | 4.1      | 0.4      | 0.1             | 4.4      | 1.3             | 1.96          | 0.23                 | PL  | ... | ...      | ...                  | ... | bzb   | TXS 0845-068          | ...  |
| J0848.5-4535 | 132.127 | -45.587 | 265.297 | -1.216 | 0.111      | 0.100      | -11    | 11.5     | 3.1      | 0.6             | 43.9     | 4.6             | 2.35          | ...                  | LP  | T   | ...      | ...                  | E   | †     | ...                   | ...  |
| J0848.7-4324 | 132.188 | -43.407 | 263.632 | 0.192  | 0.152      | 0.112      | -89    | 15.5     | 2.8      | 0.4             | 54.4     | 3.9             | 2.52          | ...                  | LP  | T   | 1,12     | ...                  | ... | ...   | ...                   | ...  |
| J0849.0+0455 | 132.269 | 4.922   | 222.528 | 28.330 | 0.153      | 0.118      | -27    | 6.1      | 0.6      | 0.1             | 8.1      | 2.3             | 1.68          | 0.19                 | PL  | ... | ...      | 1FGL J0848.6+0504    | ... | bzb   | TXS 0846+051          | ...  |
| J0849.2+6606 | 132.316 | 66.103  | 148.943 | 36.455 | 0.088      | 0.083      | -61    | 6.7      | 0.5      | 0.1             | 6.0      | 1.3             | 1.96          | 0.16                 | PL  | ... | ...      | 1FGL J0849.3+6607    | ... | bzb   | GB6 J0848+6605        | ...  |
| J0849.8+4852 | 132.472 | 48.868  | 170.536 | 39.252 | 0.069      | 0.067      | 24     | 19.2     | 1.8      | 0.2             | 21.0     | 1.7             | 2.22          | 0.06                 | PL  | T   | ...      | 1FGL J0849.9+4852    | ... | bzb   | GB6 J0850+4855        | ...  |
| J0849.9-3540 | 132.478 | -35.669 | 257.761 | 5.247  | 0.093      | 0.081      | -0     | 8.9      | 1.5      | 0.2             | 17.2     | 2.5             | 2.03          | 0.09                 | PL  | T   | ...      | 1FGL J0849.6-3540    | ... | agu   | PMN J0849-3541        | ...  |
| J0850.1-4846 | 132.545 | -48.772 | 267.948 | -3.007 | 0.130      | 0.112      | 51     | 7.6      | 0.5      | 0.1             | 24.5     | 3.2             | 2.60          | ...                  | LP  | ... | 1,4,5,12 | ...                  | ... | ...   | ...                   | ...  |
| J0850.2-1212 | 132.551 | -12.216 | 238.658 | 19.535 | 0.044      | 0.040      | 57     | 33.9     | 4.6      | 0.3             | 42.6     | 2.5             | 2.18          | ...                  | LP  | T   | ...      | 1FGL J0850.0-1213    | ... | bzq   | BZQ J0850-1213        | ...  |
|              |         |         |         |        |            |            |        |          |          |                 |          |                 |               |                      |     |     |          | 3EG J0852-1216       |     |       |                       |      |
|              |         |         |         |        |            |            |        |          |          |                 |          |                 |               |                      |     |     |          | EGR J0852-1224       |     |       |                       |      |
| J0851.7-4635 | 132.941 | -46.592 | 266.433 | -1.416 | 0.152      | 0.129      | 40     | 5.5      | 1.7      | 0.5             | 19.4     | 5.3             | 2.06          | 0.22                 | PL  | ... | ...      | ...                  | E   | †     | ...                   | ...  |
| J0852.4-5756 | 133.124 | -57.945 | 275.317 | -8.535 | 0.089      | 0.086      | -72    | 8.8      | 1.3      | 0.2             | 15.0     | 2.0             | 2.17          | 0.09                 | PL  | T   | ...      | ...                  | ... | agu   | PMN J0852-5755        | ...  |
| J0853.1-3659 | 133.278 | -36.989 | 259.196 | 4.910  | 0.163      | 0.108      | -57    | 4.6      | 0.8      | 0.2             | 9.4      | 2.3             | 1.88          | 0.15                 | PL  | ... | ...      | ...                  | ... | agu   | NVSS J085310-365820   | ...  |
| J0853.5-4711 | 133.396 | -47.199 | 267.099 | -1.566 | 0.130      | 0.108      | 88     | 7.0      | 2.1      | 0.4             | 24.0     | 5.2             | 2.15          | 0.17                 | PL  | ... | ...      | ...                  | E   | †     | ...                   | ...  |
| J0854.7-4501 | 133.695 | -45.029 | 265.570 | -0.010 | 0.068      | 0.062      | 34     | 13.6     | 5.3      | 0.5             | 41.3     | 4.7             | 2.25          | ...                  | LP  | T   | ...      | 1FGL J0854.6-4504    | ... | ...   | ...                   | ...  |
| J0854.8+2005 | 133.713 | 20.098  | 206.828 | 35.826 | 0.040      | 0.039      | 62     | 27.2     | 3.5      | 0.2             | 41.3     | 2.3             | 2.23          | 0.04                 | PL  | T   | ...      | 1FGL J0854.8+2006    | ... | BZB   | OJ 287                | ...  |
|              |         |         |         |        |            |            |        |          |          |                 |          |                 |               |                      |     |     |          | 0FGL J0855.4+2009    |     |       |                       |      |
|              |         |         |         |        |            |            |        |          |          |                 |          |                 |               |                      |     |     |          | 3EG J0853+1941       |     |       |                       |      |
|              |         |         |         |        |            |            |        |          |          |                 |          |                 |               |                      |     |     |          | EGR J0853+2015       |     |       |                       |      |
| J0855.1-0712 | 133.789 | -7.211  | 234.956 | 23.365 | 0.219      | 0.206      | -66    | 4.2      | 0.3      | 0.1             | 5.5      | 1.2             | 2.62          | 0.20                 | PL  | ... | ...      | ...                  | ... | agu   | 3C 209                | ...  |
| J0855.4-4625 | 133.868 | -46.432 | 266.720 | -0.824 | 0.111      | 0.099      | 15     | 6.2      | 2.2      | 0.4             | 24.6     | 5.2             | 2.15          | 0.16                 | PL  | ... | ...      | ...                  | E   | †     | ...                   | ...  |
| J0856.0+7136 | 134.009 | 71.608  | 142.254 | 35.306 | 0.222      | 0.140      | -18    | 4.8      | 0.4      | 0.1             | 5.8      | 1.2             | 2.54          | 0.17                 | PL  | ... | ...      | ...                  | ... | agu   | GB6 J0856+7146        | ...  |
| J0856.3+2058 | 134.076 | 20.978  | 205.939 | 36.437 | 0.152      | 0.126      | 84     | 6.1      | 0.7      | 0.1             | 8.0      | 1.6             | 2.14          | 0.14                 | PL  | ... | ...      | 1FGL J0856.6+2103    | ... | bzb   | TXS 0853+211          | ...  |
| J0856.6-1105 | 134.173 | -11.096 | 238.652 | 21.479 | 0.048      | 0.046      | 11     | 22.9     | 2.9      | 0.2             | 32.1     | 2.6             | 2.05          | 0.05                 | PL  | ... | ...      | 1FGL J0856.6-1105    | ... | bzb   | CRATES J0856-1105     | ...  |
| J0858.0-4815 | 134.505 | -48.261 | 268.392 | -1.684 | 0.174      | 0.111      | 88     | 14.1     | 3.5      | 0.5             | 48.7     | 4.4             | 2.47          | ...                  | LP  | ... | 2,9      | ...                  | ... | ...   | ...                   | ...  |
| J0858.1-1952 | 134.533 | -19.876 | 246.333 | 16.526 | 0.120      | 0.107      | 21     | 7.0      | 0.8      | 0.2             | 10.8     | 1.7             | 2.41          | 0.12                 | PL  | T   | ...      | ...                  | ... | agu   | PKS 0855-19           | ...  |
| J0858.2-3129 | 134.569 | -31.489 | 255.625 | 9.250  | 0.147      | 0.122      | 31     | 4.3      | 0.3      | 0.1             | 7.6      | 3.0             | 1.12          | 0.34                 | PL  | ... | ...      | ...                  | ... | agu   | 1RXS J085802.6-313043 | ...  |

Table 1—Continued

| Name 2FGL     | R.A.    | Decl.   | $l$     | $b$    | $\theta_1$ | $\theta_2$ | $\phi$ | $\sigma$ | $F_{35}$ | $\Delta F_{35}$ | $S_{25}$ | $\Delta S_{25}$ | $\Gamma_{25}$ | $\Delta \Gamma_{25}$ | Mod | Var | Flags | $\gamma$ -ray Assoc.                   | TeV | Class | ID or Assoc.          | Ref. |
|---------------|---------|---------|---------|--------|------------|------------|--------|----------|----------|-----------------|----------|-----------------|---------------|----------------------|-----|-----|-------|----------------------------------------|-----|-------|-----------------------|------|
| J0858.3–4333  | 134.584 | –43.560 | 264.866 | 1.428  | 0.148      | 0.142      | 86     | 14.1     | 3.3      | 0.6             | 44.2     | 3.9             | 2.45          | ...                  | LP  | ... | ...   | 3EG J0859–4257                         | ... | ...   | ...                   | ...  |
| J0859.4–2532  | 134.871 | –25.536 | 251.117 | 13.246 | 0.126      | 0.117      | –48    | 4.6      | 0.6      | 0.2             | 6.5      | 1.7             | 2.06          | 0.18                 | PL  | ... | ...   | ...                                    | ... | ...   | ...                   | ...  |
| J0900.5–4441c | 135.150 | –44.688 | 265.984 | 0.994  | 0.151      | 0.113      | 48     | 5.7      | 2.0      | 0.4             | 25.3     | 4.6             | 2.35          | 0.11                 | PL  | ... | 4,5,6 | ...                                    | ... | ...   | ...                   | ...  |
| J0900.9+6736  | 135.248 | 67.613  | 146.713 | 37.099 | 0.156      | 0.128      | 32     | 6.3      | 0.5      | 0.1             | 6.9      | 1.2             | 2.47          | 0.13                 | PL  | ... | ...   | ...                                    | ... | ...   | ...                   | ...  |
| J0901.7–4655  | 135.429 | –46.921 | 267.790 | –0.334 | 0.128      | 0.103      | 63     | 12.5     | 4.0      | 0.5             | 40.1     | 4.2             | 2.38          | ...                  | LP  | ... | 2,5   | ...                                    | ... | ...   | ...                   | ...  |
| J0902.4+2050  | 135.611 | 20.848  | 206.673 | 37.752 | 0.096      | 0.082      | –71    | 9.3      | 0.9      | 0.1             | 10.2     | 1.7             | 2.01          | 0.11                 | PL  | ... | ...   | 1FGL J0902.4+2050                      | ... | bzb   | NVSS J090226+205045   | ...  |
| J0902.8–4741c | 135.710 | –47.696 | 268.497 | –0.705 | 0.100      | 0.098      | 82     | 7.0      | 3.3      | 0.5             | 13.7     | 2.2             | 2.22          | ...                  | LP  | ... | 6,12  | 1FGL J0902.5–4731c                     | ... | ...   | ...                   | ...  |
| J0903.4+4651  | 135.869 | 46.859  | 173.027 | 41.625 | 0.150      | 0.124      | 86     | 5.4      | 0.4      | 0.1             | 5.1      | 1.1             | 2.27          | 0.18                 | PL  | ... | ...   | ...                                    | ... | bzq   | S4 0859+47            | ...  |
| J0903.6+4238  | 135.922 | 42.636  | 178.681 | 41.763 | 0.144      | 0.125      | 35     | 5.4      | 0.4      | 0.1             | 5.3      | 1.1             | 2.28          | 0.19                 | PL  | ... | 1     | ...                                    | ... | agn   | S4 0900+42            | ...  |
| J0904.0–4823c | 136.014 | –48.394 | 269.154 | –1.018 | 0.168      | 0.138      | –40    | 4.1      | 1.7      | 0.4             | 22.5     | 5.3             | 2.37          | 0.12                 | PL  | ... | 4,5,6 | ...                                    | ... | ...   | ...                   | ...  |
| J0904.8–3513  | 136.225 | –35.222 | 259.400 | 7.867  | 0.115      | 0.102      | 28     | 9.4      | 1.3      | 0.2             | 18.0     | 2.1             | 2.45          | 0.09                 | PL  | T   | ...   | 1FGL J0904.7–3514<br>3EG J0903–3531    | ... | agu   | NVSS J090442–351423   | ...  |
| J0904.9–5735  | 136.241 | –57.584 | 276.124 | –7.033 | 0.065      | 0.059      | –23    | 10.4     | 1.6      | 0.2             | 17.5     | 2.4             | 1.98          | 0.09                 | PL  | T   | ...   | 1FGL J0905.1–5736                      | ... | agn   | PKS 0903–57           | ...  |
| J0905.6+1357  | 136.403 | 13.964  | 215.039 | 35.964 | 0.061      | 0.055      | 65     | 14.2     | 1.5      | 0.2             | 17.8     | 2.6             | 1.81          | 0.10                 | PL  | ... | ...   | 1FGL J0905.5+1356                      | ... | bzb   | MG1 J090534+1358      | ...  |
| J0906.2–0906  | 136.571 | –9.114  | 238.381 | 24.550 | 0.086      | 0.077      | 31     | 8.1      | 0.8      | 0.1             | 8.7      | 1.7             | 1.99          | 0.13                 | PL  | ... | ...   | 1FGL J0906.4–0903                      | ... | agu   | PMN J0906–0905        | ...  |
| J0907.9–4716c | 136.989 | –47.273 | 268.762 | 0.220  | 0.112      | 0.096      | 89     | 7.5      | 2.4      | 0.4             | 30.9     | 4.5             | 2.38          | 0.09                 | PL  | ... | 4,5,6 | ...                                    | ... | ...   | ...                   | ...  |
| J0908.5–4913  | 137.148 | –49.218 | 270.266 | –1.018 | 0.559      | 0.301      | 24     | 11.6     | 3.4      | 0.6             | 44.6     | 4.7             | 3.01          | ...                  | EC  | ... | 2,9   | 1FGL J0906.3–4855c                     | ... | PSR   | PSR J0908–4913        | ...  |
| J0908.7–2119  | 137.193 | –21.318 | 249.138 | 17.569 | 0.126      | 0.124      | –42    | 4.3      | 0.5      | 0.1             | 7.0      | 1.7             | 2.37          | 0.17                 | PL  | ... | ...   | 1FGL J0908.7–2119                      | ... | agu   | NVSS J090858–211854   | ...  |
| J0909.1+0121  | 137.285 | 1.366   | 228.935 | 30.922 | 0.057      | 0.052      | –51    | 22.8     | 3.2      | 0.2             | 43.8     | 3.0             | 2.49          | ...                  | LP  | T   | ...   | 1FGL J0909.0+0126                      | ... | bzq   | PKS 0906+01           | ...  |
| J0909.2+2308  | 137.318 | 23.149  | 204.481 | 39.962 | 0.089      | 0.069      | –82    | 8.3      | 0.9      | 0.2             | 11.4     | 2.4             | 1.71          | 0.15                 | PL  | ... | ...   | 1FGL J0909.2+2310                      | ... | bzb   | RX J0908.9+2311       | ...  |
| J0909.6+0158  | 137.417 | 1.973   | 228.406 | 31.348 | 0.152      | 0.123      | 67     | 5.1      | 0.7      | 0.2             | 10.5     | 2.6             | 2.50          | 0.17                 | PL  | ... | 5     | 0FGL J0909.7+0145                      | ... | bzb   | PKS 0907+022          | ...  |
| J0909.7–0229  | 137.433 | –2.497  | 232.801 | 28.992 | 0.071      | 0.064      | 30     | 19.2     | 2.0      | 0.2             | 23.5     | 1.8             | 2.28          | 0.06                 | PL  | T   | ...   | 1FGL J0909.6–0229                      | ... | bzq   | PKS 0907–023          | ...  |
| J0910.4–5050  | 137.603 | –50.847 | 271.659 | –1.911 | 0.209      | 0.155      | –56    | 12.4     | 2.8      | 0.4             | 47.2     | 4.0             | 2.60          | 0.06                 | PL  | T   | ...   | 1FGL J0910.4–5055<br>0FGL J0910.2–5044 | ... | agu   | AT20G J0910–5048      | ...  |
| J0910.6+3329  | 137.654 | 33.495  | 191.114 | 42.467 | 0.081      | 0.078      | 57     | 11.1     | 1.0      | 0.1             | 11.9     | 1.9             | 1.94          | 0.11                 | PL  | ... | ...   | 1FGL J0910.7+3332                      | ... | bzb   | Ton 1015              | ...  |
| J0910.9+2246  | 137.747 | 22.780  | 205.093 | 40.233 | 0.092      | 0.079      | –2     | 8.9      | 1.2      | 0.2             | 14.1     | 1.8             | 2.25          | 0.09                 | PL  | T   | ...   | 1FGL J0911.0+2247                      | ... | bzq   | TXS 0907+230          | ...  |
| J0912.1+4126  | 138.043 | 41.442  | 180.314 | 43.331 | 0.107      | 0.091      | –30    | 6.9      | 0.5      | 0.1             | 6.4      | 1.2             | 2.30          | 0.17                 | PL  | T   | ...   | 1FGL J0912.3+4127                      | ... | bzq   | B3 0908+416B          | ...  |
| J0912.5+2758  | 138.132 | 27.974  | 198.548 | 41.896 | 0.147      | 0.103      | –29    | 4.5      | 0.2      | 0.1             | 5.0      | 2.4             | 1.20          | 0.37                 | PL  | ... | ...   | 1FGL J0912.6+2756                      | ... | bzb   | 1RXS J091211.9+275955 | ...  |
| J0912.9–2102  | 138.236 | –21.040 | 249.569 | 18.494 | 0.069      | 0.060      | –31    | 7.3      | 0.8      | 0.2             | 9.3      | 1.9             | 1.94          | 0.15                 | PL  | ... | ...   | ...                                    | ... | bzb   | MRC 0910–208          | ...  |
| J0913.0+1553  | 138.251 | 15.893  | 213.683 | 38.361 | 0.229      | 0.188      | –66    | 4.1      | 0.4      | 0.1             | 5.0      | 1.3             | 2.25          | 0.26                 | PL  | T   | 11    | ...                                    | ... | bzb   | BZB J0912+1555        | ...  |
| J0914.1–4756  | 138.542 | –47.936 | 269.962 | 0.531  | 0.150      | 0.139      | 83     | 11.2     | 2.4      | 0.6             | 36.8     | 4.1             | 2.42          | ...                  | LP  | ... | 1     | ...                                    | ... | ...   | ...                   | ...  |
| J0915.8+2932  | 138.963 | 29.544  | 196.666 | 42.928 | 0.049      | 0.044      | 12     | 19.9     | 2.1      | 0.2             | 24.8     | 2.7             | 1.87          | 0.06                 | PL  | ... | ...   | 1FGL J0915.7+2931                      | ... | bzb   | B2 0912+29            | ...  |
| J0917.0+3900  | 139.265 | 39.003  | 183.714 | 44.223 | 0.162      | 0.137      | 81     | 5.9      | 0.4      | 0.1             | 6.0      | 1.1             | 2.53          | 0.16                 | PL  | ... | ...   | ...                                    | ... | bzq   | S4 0913+39            | ...  |
| J0919.3–2203  | 139.850 | –22.057 | 251.416 | 18.969 | 0.189      | 0.140      | 62     | 4.3      | 0.5      | 0.1             | 5.3      | 1.5             | 2.00          | 0.20                 | PL  | ... | ...   | ...                                    | ... | agu   | NVSS J091922–220757   | ...  |
| J0920.9+4441  | 140.236 | 44.697  | 175.703 | 44.811 | 0.028      | 0.027      | 55     | 75.9     | 9.1      | 0.3             | 95.0     | 2.7             | 2.27          | ...                  | LP  | T   | ...   | 1FGL J0920.9+4441                      | ... | bzq   | S4 0917+44            | ...  |

Table 1—Continued

| Name 2FGL         | R.A.    | Decl.   | $l$     | $b$     | $\theta_1$ | $\theta_2$ | $\phi$ | $\sigma$ | $F_{35}$ | $\Delta F_{35}$ | $S_{25}$ | $\Delta S_{25}$ | $\Gamma_{25}$ | $\Delta \Gamma_{25}$ | Mod | Var | Flags  | $\gamma$ -ray Assoc. | TeV | Class | ID or Assoc.          | Ref.  |
|-------------------|---------|---------|---------|---------|------------|------------|--------|----------|----------|-----------------|----------|-----------------|---------------|----------------------|-----|-----|--------|----------------------|-----|-------|-----------------------|-------|
| 0FGL J0921.2+4437 |         |         |         |         |            |            |        |          |          |                 |          |                 |               |                      |     |     |        |                      |     |       |                       |       |
| J0921.9+2335      | 140.486 | 23.585  | 205.014 | 42.875  | 0.235      | 0.139      | 75     | 5.0      | 0.5      | 0.1             | 5.9      | 1.9             | 1.74          | 0.20                 | PL  | ... | 9      | 1FGL J0922.0+2337    | ... | bzb   | NVSS J092145+233548   | ...   |
| J0921.9+6216      | 140.493 | 62.278  | 152.163 | 41.029  | 0.114      | 0.094      | 82     | 12.5     | 0.8      | 0.1             | 12.2     | 1.2             | 2.51          | 0.09                 | PL  | T   | ...    | ...                  | ... | bzq   | OK 630                | ...   |
| J0922.2-5214c     | 140.558 | -52.244 | 273.942 | -1.563  | 0.195      | 0.179      | 2      | 9.3      | 1.1      | 0.3             | 22.5     | 2.5             | 2.43          | ...                  | LP  | ... | 1,6,12 | ...                  | ... | ...   | ...                   | ...   |
| J0922.7+0435      | 140.679 | 4.596   | 227.688 | 35.486  | 0.166      | 0.116      | 79     | 5.1      | 0.5      | 0.1             | 6.0      | 1.3             | 2.25          | 0.17                 | PL  | ... | ...    | ...                  | ... | agu   | GB6 J0922+0433        | ...   |
| J0923.2+4125      | 140.817 | 41.431  | 180.292 | 45.411  | 0.108      | 0.089      | 71     | 12.6     | 1.0      | 0.1             | 12.6     | 1.4             | 2.31          | 0.09                 | PL  | T   | ...    | 1FGL J0923.2+4121    | ... | bzq   | B3 0920+416           | ...   |
| J0923.5+1508      | 140.895 | 15.138  | 215.853 | 40.422  | 0.185      | 0.137      | 23     | 4.2      | 0.4      | 0.1             | 4.7      | 1.2             | 2.33          | 0.21                 | PL  | T   | 11     | ...                  | ... | ...   | ...                   | ...   |
| J0924.0+2819      | 141.017 | 28.322  | 198.804 | 44.457  | 0.192      | 0.125      | -25    | 9.1      | 0.6      | 0.1             | 10.1     | 1.2             | 2.64          | 0.12                 | PL  | T   | ...    | 1FGL J0924.2+2812    | ... | bzq   | B2 0920+28            | ...   |
| J0927.9-2041      | 141.977 | -20.695 | 251.736 | 21.355  | 0.277      | 0.213      | 8      | 6.9      | 0.6      | 0.1             | 9.1      | 1.4             | 2.53          | 0.12                 | PL  | T   | ...    | ...                  | ... | bzq   | PKS 0925-203          | ...   |
| J0928.8-3530      | 142.223 | -35.505 | 263.016 | 11.227  | 0.128      | 0.115      | -76    | 4.4      | 0.6      | 0.1             | 6.3      | 1.7             | 1.94          | 0.16                 | PL  | ... | ...    | 1FGL J0929.0-3531    | ... | ...   | ...                   | ...   |
| J0929.5+5009      | 142.396 | 50.162  | 167.737 | 45.485  | 0.112      | 0.087      | -13    | 8.1      | 0.7      | 0.1             | 8.1      | 1.5             | 1.98          | 0.14                 | PL  | T   | ...    | 1FGL J0929.4+5000    | ... | bzb   | GB6 J0929+5013        | ...   |
| J0930.4+8611      | 142.617 | 86.197  | 126.291 | 29.520  | 0.072      | 0.068      | -48    | 10.5     | 1.0      | 0.1             | 11.5     | 1.6             | 2.05          | 0.09                 | PL  | T   | 9      | ...                  | ... | bzb   | S5 0916+864           | ...   |
| J0934.0-6231      | 143.509 | -62.526 | 282.239 | -7.879  | 0.074      | 0.062      | 18     | 13.0     | 2.5      | 0.3             | 12.5     | 1.6             | 1.88          | ...                  | LP  | ... | ...    | 1FGL J0933.9-6228    | ... | ...   | ...                   | ...   |
| J0934.7+3932      | 143.677 | 39.535  | 182.957 | 47.640  | 0.332      | 0.221      | 63     | 4.2      | 0.4      | 0.1             | 4.5      | 1.1             | 2.34          | 0.19                 | PL  | ... | ...    | 1FGL J0934.5+3929    | ... | bzb   | GB6 J0934+3926        | ...   |
| J0937.6+5009      | 144.425 | 50.153  | 167.338 | 46.755  | 0.144      | 0.124      | -60    | 7.0      | 0.5      | 0.1             | 6.9      | 1.1             | 2.50          | 0.15                 | PL  | T   | ...    | 1FGL J0937.7+5005    | ... | bzq   | GB6 J0937+5008        | ...   |
| J0937.9-1434      | 144.479 | -14.580 | 248.489 | 27.213  | 0.134      | 0.125      | 24     | 4.1      | 0.4      | 0.1             | 4.6      | 1.4             | 1.89          | 0.19                 | PL  | ... | 8      | ...                  | ... | ...   | ...                   | ...   |
| J0939.1-1734      | 144.789 | -17.579 | 251.190 | 25.418  | 0.111      | 0.093      | 60     | 9.9      | 1.1      | 0.2             | 12.2     | 1.6             | 2.22          | 0.10                 | PL  | T   | ...    | ...                  | ... | agu   | TXS 0936-173          | ...   |
| J0940.3-2827      | 145.091 | -28.457 | 259.746 | 17.977  | 0.137      | 0.110      | 34     | 6.3      | 0.7      | 0.1             | 8.5      | 1.5             | 2.32          | 0.13                 | PL  | T   | ...    | ...                  | ... | agu   | TXS 0937-282          | ...   |
| J0940.8-6105      | 145.213 | -61.086 | 281.865 | -6.271  | 0.173      | 0.112      | 24     | 4.4      | 0.7      | 0.2             | 8.4      | 2.0             | 2.15          | 0.13                 | PL  | ... | ...    | ...                  | ... | agu   | MRC 0939-608          | ...   |
| J0941.4+2724      | 145.358 | 27.416  | 201.165 | 48.046  | 0.162      | 0.126      | 79     | 6.6      | 0.5      | 0.1             | 6.3      | 1.1             | 2.32          | 0.14                 | PL  | ... | ...    | 1FGL J0941.2+2722    | ... | bzq   | MG2 J094148+2728      | ...   |
| J0941.4+6148      | 145.358 | 61.805  | 151.536 | 43.311  | 0.128      | 0.119      | 54     | 6.8      | 0.6      | 0.1             | 6.4      | 1.2             | 2.08          | 0.14                 | PL  | ... | ...    | 1FGL J0941.2+6149    | ... | bzb   | RX J0940.3+6148       | ...   |
| J0941.9-0755      | 145.490 | -7.928  | 243.397 | 32.284  | 0.145      | 0.130      | -73    | 4.6      | 0.4      | 0.1             | 5.0      | 1.6             | 1.86          | 0.17                 | PL  | T   | ...    | ...                  | ... | agu   | PMN J0942-0800        | ...   |
| J0942.8-7558      | 145.712 | -75.976 | 292.214 | -17.200 | 0.292      | 0.163      | 67     | 4.9      | 0.7      | 0.2             | 9.7      | 1.9             | 2.44          | 0.14                 | PL  | ... | 9      | 1FGL J0940.2-7605    | ... | rdg   | PKS 0943-76           | ...   |
| J0945.9+5751      | 146.482 | 57.864  | 156.229 | 45.458  | 0.107      | 0.099      | 41     | 7.6      | 0.6      | 0.1             | 6.3      | 1.1             | 2.16          | 0.14                 | PL  | ... | ...    | 1FGL J0945.6+5754    | ... | bzb   | GB6 J0945+5757        | ...   |
| J0946.2+0104      | 146.553 | 1.068   | 235.359 | 38.551  | 0.113      | 0.088      | 38     | 4.6      | 0.3      | 0.1             | 5.3      | 1.9             | 1.57          | 0.26                 | PL  | ... | ...    | ...                  | ... | bzb   | RXS J094620.5+010459  | ...   |
| J0946.5+1015      | 146.648 | 10.259  | 225.010 | 43.412  | 0.140      | 0.119      | 57     | 11.9     | 1.0      | 0.1             | 14.1     | 1.4             | 2.48          | 0.09                 | PL  | T   | ...    | 1FGL J0946.6+1012    | ... | bzq   | TXS 0943+105          | ...   |
| J0946.9-2541      | 146.738 | -25.697 | 258.852 | 20.987  | 0.218      | 0.168      | 72     | 4.8      | 0.6      | 0.1             | 6.2      | 1.5             | 2.08          | 0.16                 | PL  | ... | ...    | ...                  | ... | agu   | 1RXS J094709.2-254056 | ...   |
| J0948.8+4040      | 147.202 | 40.678  | 180.971 | 50.262  | 0.117      | 0.116      | 41     | 6.6      | 0.4      | 0.1             | 6.6      | 1.1             | 2.56          | 0.16                 | PL  | ... | ...    | ...                  | ... | bzq   | 4C +40.24             | ...   |
| J0948.8+0020      | 147.221 | 0.350   | 236.602 | 38.685  | 0.081      | 0.069      | 57     | 24.1     | 2.2      | 0.2             | 38.9     | 1.8             | 2.60          | ...                  | LP  | T   | ...    | 1FGL J0949.0+0021    | ... | SEY   | PMN J0948+0022        | 10,11 |
| 0FGL J0948.3+0019 |         |         |         |         |            |            |        |          |          |                 |          |                 |               |                      |     |     |        |                      |     |       |                       |       |
| J0950.1+4554      | 147.541 | 45.906  | 172.870 | 49.725  | 0.153      | 0.115      | 61     | 6.2      | 0.5      | 0.1             | 6.2      | 1.8             | 1.68          | 0.18                 | PL  | ... | ...    | ...                  | ... | bzb   | US 1015               | ...   |
| J0952.7-3717      | 148.189 | -37.294 | 267.881 | 13.134  | 0.267      | 0.204      | 45     | 4.9      | 0.6      | 0.1             | 8.3      | 1.6             | 2.41          | 0.13                 | PL  | ... | ...    | ...                  | ... | ...   | ...                   | ...   |
| J0953.1-0839      | 148.275 | -8.667  | 246.194 | 33.912  | 0.045      | 0.043      | -53    | 19.9     | 2.3      | 0.2             | 29.0     | 3.3             | 1.78          | 0.06                 | PL  | T   | ...    | 1FGL J0953.0-0838    | ... | bzb   | PMN J0953-0840        | ...   |
| J0953.6-1504      | 148.407 | -15.077 | 251.841 | 29.658  | 0.153      | 0.122      | -61    | 6.7      | 0.8      | 0.1             | 9.0      | 1.7             | 2.00          | 0.12                 | PL  | ... | ...    | 1FGL J0953.6-1505    | ... | ...   | ...                   | ...   |
| J0953.9-7659      | 148.475 | -76.991 | 293.428 | -17.524 | 0.114      | 0.099      | -7     | 4.5      | 0.7      | 0.2             | 7.3      | 1.9             | 2.11          | 0.19                 | PL  | ... | ...    | ...                  | ... | agu   | 1RXS J095306.1-765755 | ...   |

Table 1—Continued

| Name 2FGL     | R.A.    | Decl.   | $l$     | $b$    | $\theta_1$ | $\theta_2$ | $\phi$ | $\sigma$ | $F_{35}$ | $\Delta F_{35}$ | $S_{25}$ | $\Delta S_{25}$ | $\Gamma_{25}$ | $\Delta \Gamma_{25}$ | Mod | Var | Flags | $\gamma$ -ray Assoc. | TeV | Class | ID or Assoc.          | Ref. |
|---------------|---------|---------|---------|--------|------------|------------|--------|----------|----------|-----------------|----------|-----------------|---------------|----------------------|-----|-----|-------|----------------------|-----|-------|-----------------------|------|
| J0955.0–3949  | 148.763 | –39.824 | 269.885 | 11.470 | 0.120      | 0.091      | –8     | 11.4     | 1.5      | 0.2             | 18.9     | 2.0             | 2.35          | 0.07                 | PL  | ... | ...   | 1FGL J0955.2–3949    | ... | ...   | ...                   | ...  |
| J0955.9+6936  | 148.982 | 69.615  | 141.475 | 40.608 | 0.086      | 0.072      | 70     | 12.5     | 1.0      | 0.1             | 12.2     | 1.3             | 2.28          | 0.09                 | PL  | ... | ...   | 1FGL J0956.5+6938    | P   | sbq   | M 82                  | ...  |
| J0956.9+2516  | 149.239 | 25.281  | 205.480 | 51.015 | 0.109      | 0.098      | 18     | 14.5     | 1.3      | 0.2             | 16.6     | 1.5             | 2.39          | 0.07                 | PL  | T   | ...   | 1FGL J0956.9+2513    | ... | bzq   | OK 290                | ...  |
| J0957.6–1350  | 149.404 | –13.849 | 251.602 | 31.207 | 0.176      | 0.140      | 67     | 7.7      | 0.7      | 0.1             | 10.0     | 1.4             | 2.46          | 0.11                 | PL  | T   | ...   | ...                  | ... | bzq   | PMN J0957–1350        | ...  |
| J0957.7+5522  | 149.433 | 55.382  | 158.592 | 47.941 | 0.020      | 0.019      | –22    | 75.2     | 11.2     | 0.4             | 103.0    | 4.8             | 1.95          | ...                  | LP  | ... | ...   | 1FGL J0957.7+5523    | ... | bzq   | 4C +55.17             | ...  |
|               |         |         |         |        |            |            |        |          |          |                 |          |                 |               |                      |     |     |       | 0FGL J0957.6+5522    |     |       |                       |      |
|               |         |         |         |        |            |            |        |          |          |                 |          |                 |               |                      |     |     |       | EGR J0957+5513       |     |       |                       |      |
| J0957.7+4735  | 149.440 | 47.588  | 169.838 | 50.593 | 0.217      | 0.171      | 26     | 5.3      | 0.3      | 0.1             | 5.1      | 1.0             | 2.54          | 0.16                 | PL  | ... | ...   | ...                  | ... | bzq   | OK 492                | ...  |
| J0958.6+6533  | 149.652 | 65.557  | 145.770 | 43.121 | 0.090      | 0.069      | –89    | 16.8     | 1.4      | 0.2             | 18.2     | 1.4             | 2.42          | 0.07                 | PL  | T   | ...   | 1FGL J1000.1+6539    | ... | bzb   | S4 0954+65            | ...  |
|               |         |         |         |        |            |            |        |          |          |                 |          |                 |               |                      |     |     |       | 3EG J0958+6533       |     |       |                       |      |
|               |         |         |         |        |            |            |        |          |          |                 |          |                 |               |                      |     |     |       | EGR J0956+6524       |     |       |                       |      |
| J0958.6–2446  | 149.671 | –24.768 | 260.287 | 23.464 | 0.495      | 0.182      | 79     | 4.2      | 0.5      | 0.1             | 5.5      | 1.3             | 2.28          | 0.18                 | PL  | ... | 8,9   | ...                  | ... | agu   | TXS 0956–244          | ...  |
| J1001.0+2913  | 150.250 | 29.229  | 199.443 | 52.587 | 0.107      | 0.088      | –11    | 11.8     | 1.0      | 0.1             | 12.1     | 1.4             | 2.22          | 0.09                 | PL  | T   | ...   | 1FGL J1000.9+2915    | ... | bzb   | GB6 J1001+2911        | ...  |
| J1003.0+2219  | 150.762 | 22.322  | 210.620 | 51.636 | 0.148      | 0.129      | 74     | 4.8      | 0.4      | 0.1             | 5.0      | 1.2             | 2.24          | 0.16                 | PL  | ... | ...   | ...                  | ... | bzb   | 1RXS J100235.8+221609 | ...  |
| J1007.1–2157  | 151.793 | –21.950 | 259.851 | 26.867 | 0.136      | 0.082      | –76    | 10.6     | 0.9      | 0.1             | 13.8     | 1.5             | 2.53          | 0.10                 | PL  | ... | ...   | 1FGL J1007.1–2157    | ... | bzq   | PKS 1004+217          | ...  |
| J1007.7+0621  | 151.932 | 6.353   | 233.471 | 45.952 | 0.098      | 0.088      | 75     | 9.9      | 1.0      | 0.1             | 12.1     | 1.5             | 2.29          | 0.10                 | PL  | T   | ...   | 1FGL J1007.9+0619    | ... | bzb   | MG1 J100820+0621      | ...  |
| J1008.6+0028  | 152.166 | 0.473   | 240.361 | 42.730 | 0.212      | 0.183      | –59    | 4.4      | 0.5      | 0.1             | 5.2      | 1.4             | 2.05          | 0.18                 | PL  | ... | ...   | ...                  | ... | agu   | PKS 1005+007          | ...  |
| J1009.7–3123  | 152.440 | –31.392 | 266.865 | 19.930 | 0.180      | 0.156      | 51     | 6.6      | 0.8      | 0.2             | 9.8      | 1.7             | 2.24          | 0.14                 | PL  | ... | ...   | ...                  | P   | bzb   | 1RXS J101015.9–311909 | ...  |
| J1010.7–5643c | 152.691 | –56.727 | 282.206 | –0.465 | 0.150      | 0.128      | 40     | 8.7      | 2.7      | 0.6             | 33.5     | 4.3             | 2.50          | ...                  | LP  | ... | 4,6   | 3EG J1014–5705       | ... | ...   | ...                   | ...  |
| J1010.8–0158  | 152.719 | –1.972  | 243.399 | 41.627 | 0.138      | 0.128      | –76    | 5.7      | 0.6      | 0.1             | 6.3      | 1.3             | 2.13          | 0.14                 | PL  | ... | ...   | 1FGL J1011.0–0156    | ... | bzq   | PKS 1008–01           | ...  |
| J1012.1–4236  | 153.046 | –42.606 | 274.218 | 11.215 | 0.179      | 0.136      | –69    | 4.2      | 0.6      | 0.2             | 6.8      | 1.8             | 1.98          | 0.16                 | PL  | ... | ...   | ...                  | ... | ...   | ...                   | ...  |
| J1012.1+0631  | 153.048 | 6.522   | 234.145 | 46.972 | 0.097      | 0.089      | 12     | 6.9      | 0.7      | 0.1             | 7.8      | 1.5             | 2.14          | 0.15                 | PL  | T   | ...   | 1FGL J1012.2+0634    | ... | bzb   | NRAO 350              | ...  |
| J1012.5+4227  | 153.144 | 42.451  | 176.984 | 54.381 | 0.127      | 0.109      | 22     | 4.8      | 0.4      | 0.1             | 4.4      | 1.3             | 1.87          | 0.20                 | PL  | ... | ...   | ...                  | ... | bzb   | B3 1009+427           | ...  |
| J1012.6+2440  | 153.172 | 24.678  | 207.739 | 54.362 | 0.045      | 0.044      | 77     | 34.8     | 4.3      | 0.3             | 38.7     | 2.2             | 2.24          | ...                  | LP  | T   | ...   | 1FGL J1012.7+2440    | ... | bzq   | MG2 J101241+2439      | ...  |
|               |         |         |         |        |            |            |        |          |          |                 |          |                 |               |                      |     |     |       | 0FGL J1012.9+2435    |     |       |                       |      |
| J1013.6+3434  | 153.403 | 34.575  | 190.580 | 55.545 | 0.165      | 0.129      | –37    | 4.1      | 0.3      | 0.1             | 3.9      | 1.1             | 2.09          | 0.21                 | PL  | ... | ...   | ...                  | ... | ...   | ...                   | ...  |
| J1014.1+2306  | 153.537 | 23.108  | 210.491 | 54.312 | 0.285      | 0.251      | –11    | 5.3      | 0.5      | 0.1             | 7.1      | 1.4             | 2.54          | 0.16                 | PL  | ... | ...   | ...                  | ... | bzq   | 4C +23.24             | ...  |
| J1015.1+4925  | 153.788 | 49.432  | 165.527 | 52.726 | 0.024      | 0.023      | 17     | 54.1     | 7.8      | 0.3             | 72.6     | 4.6             | 1.85          | ...                  | LP  | T   | ...   | 1FGL J1015.1+4927    | P   | bzb   | 1H 1013+498           | ...  |
|               |         |         |         |        |            |            |        |          |          |                 |          |                 |               |                      |     |     |       | 0FGL J1015.2+4927    |     |       |                       |      |
| J1016.0+0513  | 154.014 | 5.229   | 236.507 | 47.040 | 0.035      | 0.034      | –57    | 27.2     | 4.4      | 0.3             | 48.9     | 3.1             | 2.08          | 0.05                 | PL  | T   | ...   | 1FGL J1016.1+0514    | ... | bzq   | TXS 1013+054          | ...  |
|               |         |         |         |        |            |            |        |          |          |                 |          |                 |               |                      |     |     |       | 0FGL J1015.9+0515    |     |       |                       |      |
| J1016.1+5600  | 154.031 | 56.003  | 155.962 | 49.970 | 0.258      | 0.214      | 21     | 4.6      | 0.2      | 0.1             | 5.0      | 1.1             | 2.78          | 0.24                 | PL  | ... | ...   | ...                  | ... | ...   | ...                   | ...  |
| J1016.2–0638  | 154.062 | –6.638  | 249.155 | 39.514 | 0.210      | 0.186      | –18    | 4.7      | 0.4      | 0.1             | 6.2      | 1.3             | 2.49          | 0.17                 | PL  | ... | ...   | ...                  | ... | agu   | PMN J1015–0626        | ...  |
| J1016.4–4244  | 154.122 | –42.746 | 274.960 | 11.555 | 0.146      | 0.121      | 80     | 4.3      | 0.6      | 0.2             | 6.8      | 2.0             | 1.81          | 0.18                 | PL  | ... | ...   | ...                  | ... | ...   | ...                   | ...  |
| J1016.5–5858  | 154.125 | –58.973 | 284.107 | –1.886 | 0.053      | 0.050      | –71    | 10.5     | 7.0      | 0.8             | 51.3     | 10.0            | 2.26          | ...                  | EC  | ... | 5     | 3EG J1013–5915       | ... | PSR   | PSR J1016–5857        | ...  |



Table 1—Continued

| Name 2FGL     | R.A.    | Decl.   | $l$     | $b$     | $\theta_1$ | $\theta_2$ | $\phi$ | $\sigma$ | $F_{35}$ | $\Delta F_{35}$ | $S_{25}$ | $\Delta S_{25}$ | $\Gamma_{25}$ | $\Delta \Gamma_{25}$ | Mod | Var | Flags  | $\gamma$ -ray Assoc. | TeV | Class | ID or Assoc.          | Ref. |
|---------------|---------|---------|---------|---------|------------|------------|--------|----------|----------|-----------------|----------|-----------------|---------------|----------------------|-----|-----|--------|----------------------|-----|-------|-----------------------|------|
| J1017.0+3531  | 154.271 | 35.528  | 188.828 | 56.214  | 0.456      | 0.306      | −46    | 4.4      | 0.2      | 0.1             | 6.1      | 1.2             | 2.89          | 0.20                 | PL  | ... | ...    | 1FGL J1016.2+3548    | ... | bzq   | B2 1015+35B           | ...  |
| J1018.3−3119  | 154.599 | −31.322 | 268.392 | 21.096  | 0.246      | 0.193      | −35    | 6.3      | 0.6      | 0.1             | 10.1     | 1.6             | 2.66          | 0.13                 | PL  | ... | ...    | ...                  | ... | bzq   | PKS 1016−311          | ...  |
| J1018.6+0531  | 154.659 | 5.524   | 236.694 | 47.735  | 0.216      | 0.144      | −30    | 5.8      | 0.8      | 0.2             | 11.6     | 2.2             | 2.51          | 0.13                 | PL  | T   | 5      | ...                  | ... | bzq   | TXS 1015+057          | ...  |
| J1019.0+5915  | 154.752 | 59.264  | 151.404 | 48.577  | 0.158      | 0.120      | −59    | 4.8      | 0.3      | 0.1             | 3.8      | 0.9             | 2.18          | 0.19                 | PL  | ... | ...    | ...                  | ... | bzb   | TXS 1015+594          | ...  |
| J1019.0−5856  | 154.759 | −58.942 | 284.362 | −1.678  | 0.023      | 0.022      | −75    | 31.9     | 25.6     | 1.0             | 252.7    | 11.2            | 2.32          | ...                  | LP  | ... | ...    | 0FGL J1018.2−5858    | ... | HMB   | 1FGL J1018.6−5856     | ...  |
| J1019.8+6322  | 154.960 | 63.370  | 146.397 | 46.253  | 0.184      | 0.165      | −41    | 4.1      | 0.3      | 0.1             | 3.7      | 0.9             | 2.18          | 0.19                 | PL  | ... | ...    | ...                  | ... | bzb   | GB6 J1019+6319        | ...  |
| J1020.0−6029  | 155.006 | −60.497 | 285.319 | −2.911  | 0.256      | 0.162      | 89     | 5.7      | 1.0      | 0.4             | 15.5     | 3.4             | 2.60          | ...                  | LP  | ... | 1,4,5  | ...                  | ... | ...   | ...                   | ...  |
| J1021.6+8021  | 155.416 | 80.363  | 130.035 | 34.600  | 0.109      | 0.099      | −87    | 5.6      | 0.4      | 0.1             | 5.1      | 1.1             | 2.29          | 0.15                 | PL  | ... | ...    | ...                  | ... | agu   | WN B1016.6+8038       | ...  |
| J1022.7−5741  | 155.675 | −57.699 | 284.090 | −0.374  | 0.048      | 0.046      | 72     | 15.4     | 18.8     | 1.3             | 142.6    | 15.0            | 2.25          | ...                  | EC  | ... | 3,5,10 | ...                  | E   | PSR   | PSR J1023−5746        | ...  |
| J1023.1−0115  | 155.782 | −1.256  | 245.380 | 44.418  | 0.124      | 0.095      | −54    | 7.1      | 0.7      | 0.1             | 8.1      | 1.8             | 1.88          | 0.13                 | PL  | ... | ...    | 1FGL J1022.8−0115    | ... | bzb   | RX J1022.7−0112       | ...  |
| J1023.5−5749c | 155.876 | −57.832 | 284.252 | −0.429  | 0.044      | 0.039      | −69    | 7.4      | 6.7      | 1.3             | 75.1     | 14.3            | 2.10          | 0.08                 | PL  | ... | 3,6,10 | 0FGL J1024.0−5754    | E   | ...   | ...                   | ...  |
| J1023.6+2959  | 155.909 | 29.995  | 198.981 | 57.559  | 0.070      | 0.066      | −79    | 4.1      | 0.1      | 0.1             | 3.5      | 1.9             | 1.28          | 0.49                 | PL  | ... | ...    | ...                  | ... | bzb   | RX J1023.6+3001       | ...  |
| J1023.6+3947  | 155.921 | 39.794  | 180.838 | 56.972  | 0.144      | 0.128      | 84     | 8.0      | 0.6      | 0.1             | 7.9      | 1.1             | 2.44          | 0.12                 | PL  | T   | ...    | 1FGL J1023.6+3937    | ... | bzq   | 4C +40.25             | ...  |
| J1023.6+0040  | 155.924 | 0.677   | 243.432 | 45.784  | 0.184      | 0.175      | 1      | 6.0      | 0.3      | 0.1             | 5.4      | 1.0             | 2.49          | ...                  | LP  | ... | 12     | ...                  | ... | psr   | PSR J1023+0038        | ...  |
| J1023.8−3248  | 155.950 | −32.807 | 270.312 | 20.552  | 0.221      | 0.197      | 24     | 4.1      | 0.4      | 0.1             | 6.7      | 1.5             | 2.60          | 0.17                 | PL  | ... | ...    | ...                  | ... | bzq   | PKS 1021−323          | ...  |
| J1023.8−4335  | 155.966 | −43.595 | 276.583 | 11.599  | 0.059      | 0.054      | 70     | 12.2     | 1.5      | 0.2             | 18.1     | 2.7             | 1.82          | 0.09                 | PL  | ... | ...    | 1FGL J1024.0−4332    | ... | bzb   | RX J1023.8−4336       | ...  |
| J1024.6−0719  | 156.161 | −7.322  | 251.702 | 40.516  | 0.249      | 0.171      | 79     | 5.0      | 0.7      | 0.2             | 2.9      | 0.7             | 2.18          | ...                  | EC  | ... | ...    | 1FGL J1024.6−0718    | ... | PSR   | PSR J1024−0719        | ...  |
| J1026.3−8546  | 156.584 | −85.776 | 300.205 | −23.697 | 0.106      | 0.083      | 64     | 8.0      | 0.9      | 0.2             | 10.8     | 2.1             | 1.86          | 0.13                 | PL  | ... | ...    | 1FGL J1028.7−8543    | ... | bzb   | PKS 1029−85           | ...  |
| J1026.7−1749  | 156.696 | −17.826 | 260.887 | 32.986  | 0.092      | 0.088      | 66     | 6.9      | 0.7      | 0.1             | 8.5      | 1.8             | 1.93          | 0.14                 | PL  | ... | ...    | 1FGL J1027.1−1747    | ... | bzb   | 1RXS J102658.5−174905 | ...  |
| J1027.4−5730c | 156.864 | −57.511 | 284.530 | 0.123   | 0.087      | 0.077      | 67     | 12.5     | 6.6      | 0.7             | 63.8     | 6.8             | 2.35          | ...                  | LP  | ... | 2,5,6  | ...                  | ... | ...   | ...                   | ...  |
| J1028.5−5819  | 157.127 | −58.332 | 285.077 | −0.505  | 0.020      | 0.019      | −63    | 53.2     | 32.8     | 0.9             | 244.7    | 8.3             | 2.19          | ...                  | EC  | ... | ...    | 1FGL J1028.4−5819    | ... | PSR   | PSR J1028−5819        | ...  |
|               |         |         |         |         |            |            |        |          |          |                 |          |                 |               |                      |     |     |        | 0FGL J1028.6−5817    |     |       |                       |      |
|               |         |         |         |         |            |            |        |          |          |                 |          |                 |               |                      |     |     |        | 3EG J1027−5817       |     |       |                       |      |
| J1029.5−2022  | 157.381 | −20.373 | 263.343 | 31.377  | 0.146      | 0.138      | −18    | 4.3      | 0.5      | 0.1             | 5.1      | 1.4             | 2.00          | 0.20                 | PL  | ... | ...    | ...                  | ... | ...   | ...                   | ...  |
| J1029.9+7437  | 157.479 | 74.618  | 134.364 | 39.207  | 0.138      | 0.110      | 54     | 9.2      | 0.7      | 0.1             | 9.4      | 1.2             | 2.37          | 0.11                 | PL  | ... | ...    | ...                  | ... | agu   | S5 1027+74            | ...  |
| J1030.4−6015  | 157.610 | −60.255 | 286.282 | −2.023  | 0.173      | 0.141      | 65     | 6.1      | 0.7      | 0.2             | 21.5     | 3.6             | 2.56          | ...                  | LP  | ... | 1,12   | ...                  | ... | ...   | ...                   | ...  |
| J1031.0+5053  | 157.761 | 50.895  | 161.471 | 54.402  | 0.064      | 0.056      | 44     | 14.2     | 1.2      | 0.1             | 14.1     | 2.1             | 1.81          | 0.09                 | PL  | ... | ...    | 1FGL J1031.0+5051    | ... | bzb   | 1ES 1028+511          | ...  |
| J1032.6+3733  | 158.173 | 37.561  | 184.395 | 59.102  | 0.123      | 0.117      | 67     | 10.2     | 0.9      | 0.1             | 10.3     | 1.3             | 2.22          | 0.11                 | PL  | ... | ...    | 1FGL J1032.7+3737    | ... | bzb   | B3 1029+378           | ...  |
| J1032.9−8401  | 158.228 | −84.020 | 299.267 | −22.161 | 0.115      | 0.106      | −12    | 4.2      | 0.6      | 0.1             | 6.3      | 1.6             | 2.21          | 0.16                 | PL  | ... | ...    | ...                  | ... | ...   | ...                   | ...  |
| J1033.2+4117  | 158.300 | 41.286  | 177.342 | 58.388  | 0.078      | 0.068      | −11    | 15.7     | 1.1      | 0.1             | 15.7     | 1.3             | 2.44          | 0.08                 | PL  | T   | ...    | 1FGL J1033.2+4116    | ... | bzq   | S4 1030+41            | ...  |
| J1033.5−5032  | 158.375 | −50.548 | 281.701 | 6.549   | 0.080      | 0.070      | 35     | 5.8      | 0.6      | 0.2             | 8.4      | 2.3             | 1.70          | 0.15                 | PL  | ... | ...    | 1FGL J1033.5−5033    | ... | ...   | ...                   | ...  |
| J1033.9+6050  | 158.484 | 60.835  | 147.796 | 49.126  | 0.040      | 0.035      | 17     | 44.1     | 4.2      | 0.2             | 49.4     | 2.0             | 2.24          | 0.03                 | PL  | T   | 10     | 1FGL J1033.8+6048    | ... | BZQ   | S4 1030+61            | 12   |
|               |         |         |         |         |            |            |        |          |          |                 |          |                 |               |                      |     |     |        | 0FGL J1034.0+6051    |     |       |                       |      |
| J1036.1−6722  | 159.039 | −67.372 | 290.448 | −7.840  | 0.062      | 0.058      | −49    | 17.8     | 3.5      | 0.3             | 19.9     | 1.8             | 2.09          | ...                  | LP  | T   | ...    | 1FGL J1036.2−6719    | ... | ...   | ...                   | ...  |
| J1036.4−5828c | 159.113 | −58.481 | 286.050 | −0.106  | 0.103      | 0.085      | 23     | 4.5      | 2.2      | 0.5             | 26.5     | 6.1             | 2.29          | 0.11                 | PL  | ... | 6      | ...                  | ... | ...   | ...                   | ...  |

Table 1—Continued

| Name 2FGL     | R.A.    | Decl.   | $l$     | $b$     | $\theta_1$ | $\theta_2$ | $\phi$ | $\sigma$ | $F_{35}$ | $\Delta F_{35}$ | $S_{25}$ | $\Delta S_{25}$ | $\Gamma_{25}$ | $\Delta \Gamma_{25}$ | Mod | Var | Flags | $\gamma$ -ray Assoc.                                                         | TeV | Class | ID or Assoc.         | Ref. |
|---------------|---------|---------|---------|---------|------------|------------|--------|----------|----------|-----------------|----------|-----------------|---------------|----------------------|-----|-----|-------|------------------------------------------------------------------------------|-----|-------|----------------------|------|
| J1037.5–2820  | 159.392 | –28.347 | 270.279 | 25.906  | 0.097      | 0.083      | –80    | 13.9     | 1.0      | 0.2             | 18.6     | 1.6             | 2.65          | 0.08                 | PL  | T   | ...   | 1FGL J1037.7–2820                                                            | ... | bzq   | PKS B1035–281        | ...  |
| J1037.6+5712  | 159.418 | 57.209  | 151.767 | 51.769  | 0.040      | 0.038      | –2     | 28.7     | 2.9      | 0.2             | 33.3     | 2.7             | 1.91          | 0.05                 | PL  | ... | ...   | 1FGL J1037.7+5711                                                            | ... | bzb   | GB6 J1037+5711       | ...  |
| J1038.2–2423  | 159.556 | –24.384 | 267.945 | 29.290  | 0.164      | 0.128      | 8      | 5.9      | 0.6      | 0.1             | 7.3      | 1.3             | 2.31          | 0.14                 | PL  | ... | ...   | ...                                                                          | ... | ...   | ...                  | ...  |
| J1038.6–5850c | 159.655 | –58.840 | 286.471 | –0.280  | 0.090      | 0.084      | –41    | 5.4      | 2.4      | 0.5             | 27.0     | 5.8             | 2.15          | 0.11                 | PL  | T   | 5,6   | ...                                                                          | ... | ...   | ...                  | ...  |
| J1040.7+0614  | 160.182 | 6.246   | 240.877 | 52.588  | 0.101      | 0.095      | –65    | 13.7     | 1.1      | 0.2             | 16.5     | 1.5             | 2.52          | 0.08                 | PL  | T   | ...   | 1FGL J1040.5+0616                                                            | ... | bzq   | 4C +06.41            | ...  |
| J1042.6+8053  | 160.658 | 80.887  | 128.826 | 34.716  | 0.211      | 0.139      | 87     | 4.6      | 0.5      | 0.1             | 7.1      | 1.7             | 2.54          | 0.15                 | PL  | T   | ...   | 1FGL J1048.7+8054                                                            | ... | bzq   | S5 1039+81           | ...  |
| J1043.1+2404  | 160.779 | 24.082  | 211.701 | 60.988  | 0.090      | 0.085      | 35     | 10.0     | 1.0      | 0.1             | 10.8     | 1.6             | 2.07          | 0.10                 | PL  | ... | ...   | 1FGL J1043.1+2404                                                            | ... | bzb   | B2 1040+24A          | ...  |
| J1044.5–5737  | 161.138 | –57.626 | 286.577 | 1.160   | 0.030      | 0.029      | –62    | 43.6     | 17.4     | 0.6             | 148.6    | 4.8             | 2.29          | ...                  | EC  | T   | ...   | 1FGL J1044.5–5737                                                            | ... | PSR   | LAT PSR J1044–5737   | ...  |
| J1045.0–5941  | 161.251 | –59.692 | 287.595 | –0.639  | 0.024      | 0.023      | –42    | 36.1     | 23.6     | 0.9             | 188.7    | 7.8             | 2.14          | ...                  | LP  | ... | ...   | 1AGL J1043–5749<br>1FGL J1045.2–5942<br>0FGL J1045.6–5937<br>1AGL J1043–5936 | ... | ...   | Eta Carinae          | ...  |
| J1045.5–2931  | 161.375 | –29.521 | 272.607 | 25.833  | 0.103      | 0.087      | 53     | 9.1      | 0.9      | 0.1             | 11.3     | 1.5             | 2.39          | 0.12                 | PL  | T   | ...   | ...                                                                          | ... | agu   | PKS B1043–291        | ...  |
| J1046.8–6005c | 161.707 | –60.086 | 287.980 | –0.882  | 0.129      | 0.089      | 30     | 4.9      | 2.3      | 0.5             | 26.0     | 5.9             | 2.04          | 0.13                 | PL  | ... | 5,6   | 1AGL J1043–5936                                                              | ... | ...   | ...                  | ...  |
| J1047.7–6216  | 161.949 | –62.283 | 289.093 | –2.780  | 0.080      | 0.071      | –44    | 14.1     | 3.4      | 0.4             | 37.5     | 3.3             | 2.42          | ...                  | LP  | ... | 3     | ...                                                                          | ... | agu   | PMN J1047–6217       | ...  |
| J1048.2–5831  | 162.070 | –58.530 | 287.432 | 0.586   | 0.021      | 0.020      | 23     | 55.3     | 28.1     | 0.8             | 205.1    | 6.6             | 2.16          | ...                  | EC  | T   | ...   | 1FGL J1048.2–5832<br>0FGL J1047.6–5834<br>3EG J1048–5840<br>EGR J1048–5839   | ... | PSR   | PSR J1048–5832       | ...  |
| J1048.3+7144  | 162.087 | 71.738  | 135.445 | 42.271  | 0.050      | 0.046      | –63    | 23.4     | 2.4      | 0.2             | 30.4     | 1.8             | 2.34          | 0.05                 | PL  | T   | ...   | 1FGL J1048.8+7145                                                            | ... | bzq   | S5 1044+71           | ...  |
| J1048.6+2336  | 162.160 | 23.602  | 213.293 | 62.107  | 0.168      | 0.155      | –23    | 5.6      | 0.6      | 0.1             | 6.6      | 1.3             | 2.23          | 0.15                 | PL  | ... | ...   | 1FGL J1048.7+2335                                                            | ... | bzb   | NVSS J104900+233821  | ...  |
| J1049.4+1551  | 162.371 | 15.853  | 228.380 | 59.579  | 0.105      | 0.094      | –2     | 4.6      | 0.3      | 0.1             | 4.0      | 1.2             | 1.86          | 0.24                 | PL  | ... | ...   | ...                                                                          | ... | agu   | GB6 J1049+1548       | ...  |
| J1049.7+7240  | 162.429 | 72.683  | 134.561 | 41.585  | 0.134      | 0.114      | 62     | 5.9      | 0.6      | 0.1             | 7.0      | 1.4             | 2.35          | 0.16                 | PL  | ... | ...   | 1FGL J1048.5+7239                                                            | ... | bzb   | GB6 J1047+7238       | ...  |
| J1050.3–5922c | 162.594 | –59.370 | 288.053 | –0.042  | 0.157      | 0.137      | –65    | 7.3      | 4.0      | 0.6             | 27.0     | 5.4             | 2.27          | ...                  | LP  | ... | 1,5,6 | ...                                                                          | ... | ...   | ...                  | ...  |
| J1051.3+3938  | 162.831 | 39.647  | 178.528 | 62.159  | 0.157      | 0.125      | –50    | 4.3      | 0.3      | 0.1             | 4.9      | 1.9             | 1.56          | 0.22                 | PL  | ... | ...   | ...                                                                          | ... | bzb   | PB 00667             | ...  |
| J1051.8+0107  | 162.968 | 1.131   | 250.094 | 51.301  | 0.119      | 0.117      | –48    | 5.0      | 0.5      | 0.1             | 5.6      | 1.4             | 2.08          | 0.19                 | PL  | ... | ...   | 1FGL J1051.9+0106                                                            | ... | bzb   | BZB J1051+0103       | ...  |
| J1053.6+4928  | 163.417 | 49.473  | 160.288 | 58.236  | 0.060      | 0.052      | 11     | 11.8     | 0.9      | 0.1             | 11.8     | 2.2             | 1.75          | 0.12                 | PL  | ... | ...   | 1FGL J1053.6+4927<br>0FGL J1053.7+4926                                       | ... | bzb   | GB6 J1053+4930       | ...  |
| J1054.5+2212  | 163.635 | 22.215  | 216.972 | 63.056  | 0.056      | 0.050      | 61     | 17.1     | 1.6      | 0.2             | 18.3     | 1.7             | 2.15          | 0.08                 | PL  | T   | ...   | 1FGL J1054.5+2212<br>0FGL J1054.5+2212                                       | ... | bzb   | 87GB 105148.6+222705 | ...  |
| J1056.0–5853  | 164.002 | –58.888 | 288.490 | 0.709   | 0.137      | 0.118      | 42     | 12.0     | 4.1      | 0.5             | 37.0     | 4.0             | 2.36          | ...                  | LP  | ... | 3     | ...                                                                          | ... | ...   | ...                  | ...  |
| J1056.2–6021  | 164.072 | –60.359 | 289.153 | –0.605  | 0.095      | 0.088      | 84     | 12.5     | 6.1      | 0.6             | 46.9     | 5.2             | 2.27          | ...                  | LP  | ... | ...   | ...                                                                          | ... | ...   | ...                  | ...  |
| J1057.0–8004  | 164.267 | –80.083 | 297.951 | –18.336 | 0.068      | 0.066      | –39    | 19.8     | 2.8      | 0.2             | 24.8     | 2.0             | 2.28          | ...                  | LP  | T   | ...   | 1FGL J1058.1–8006<br>0FGL J1100.2–8000                                       | ... | bzb   | PKS 1057–79          | ...  |
| J1057.1+7001  | 164.284 | 70.017  | 136.084 | 44.077  | 0.176      | 0.154      | 9      | 9.9      | 0.6      | 0.1             | 10.5     | 1.2             | 2.64          | 0.10                 | PL  | T   | ...   | ...                                                                          | ... | bzq   | S5 1053+70           | ...  |

Table 1—Continued

| Name 2FGL     | R.A.    | Decl.   | $l$     | $b$     | $\theta_1$ | $\theta_2$ | $\phi$ | $\sigma$ | $F_{35}$ | $\Delta F_{35}$ | $S_{25}$ | $\Delta S_{25}$ | $\Gamma_{25}$ | $\Delta \Gamma_{25}$ | Mod | Var | Flags   | $\gamma$ -ray Assoc.                                                                          | TeV | Class | ID or Assoc.     | Ref. |
|---------------|---------|---------|---------|---------|------------|------------|--------|----------|----------|-----------------|----------|-----------------|---------------|----------------------|-----|-----|---------|-----------------------------------------------------------------------------------------------|-----|-------|------------------|------|
| J1057.9–5226  | 164.496 | –52.448 | 285.985 | 6.650   | 0.014      | 0.014      | 14     | 133.7    | 50.0     | 0.9             | 293.2    | 4.2             | 2.01          | ...                  | EC  | ... | ...     | 1FGL J1057.9–5226<br>0FGL J1058.1–5225<br>3EG J1058–5234<br>EGR J1058–5221<br>1AGL J1058–5239 | ... | PSR   | PSR J1057–5226   | ...  |
| J1058.4+0133  | 164.615 | 1.566   | 251.501 | 52.768  | 0.038      | 0.036      | 15     | 31.5     | 5.1      | 0.3             | 59.1     | 2.9             | 2.22          | 0.04                 | PL  | T   | ...     | 1FGL J1058.4+0134<br>0FGL J1057.8+0138                                                        | ... | bzb   | 4C +01.28        | ...  |
| J1058.6+5628  | 164.666 | 56.480  | 149.575 | 54.421  | 0.028      | 0.026      | –56    | 42.8     | 4.8      | 0.2             | 54.7     | 3.3             | 1.93          | 0.03                 | PL  | T   | ...     | 1FGL J1058.6+5628<br>0FGL J1058.9+5629                                                        | ... | bzb   | TXS 1055+567     | ...  |
| J1058.7–6621  | 164.682 | –66.366 | 291.961 | –5.926  | 0.136      | 0.099      | 57     | 5.6      | 1.0      | 0.2             | 11.1     | 2.2             | 2.23          | 0.14                 | PL  | ... | ...     | ...                                                                                           | ... | ...   | ...              | ...  |
| J1059.0+0222  | 164.767 | 2.374   | 250.741 | 53.452  | 0.164      | 0.140      | 40     | 4.7      | 0.6      | 0.2             | 7.8      | 1.9             | 2.29          | 0.18                 | PL  | ... | 5       | ...                                                                                           | ... | agu   | GB6 J1059+0224   | ...  |
| J1059.3–6118c | 164.827 | –61.313 | 289.891 | –1.313  | 0.240      | 0.173      | 40     | 4.4      | 1.9      | 0.4             | 24.8     | 5.5             | 2.36          | 0.12                 | PL  | ... | 4,5,6,9 | 3EG J1102–6103<br>EGR J1058–6101                                                              | ... | ...   | ...              | ...  |
| J1059.3–1132  | 164.833 | –11.541 | 264.124 | 42.727  | 0.063      | 0.059      | –1     | 19.4     | 2.2      | 0.2             | 24.4     | 2.0             | 2.17          | 0.06                 | PL  | T   | ...     | 1FGL J1059.3–1132                                                                             | ... | bzb   | PKS B1056–113    | ...  |
| J1059.4+8113  | 164.859 | 81.231  | 127.931 | 34.782  | 0.091      | 0.086      | –35    | 10.1     | 0.8      | 0.1             | 13.6     | 1.6             | 2.58          | 0.09                 | PL  | T   | ...     | ...                                                                                           | ... | bzq   | S5 1053+81       | ...  |
| J1059.9–2051  | 164.988 | –20.867 | 270.733 | 34.941  | 0.167      | 0.144      | 20     | 4.2      | 0.4      | 0.1             | 5.0      | 1.3             | 2.19          | 0.19                 | PL  | ... | 4       | ...                                                                                           | ... | ...   | ...              | ...  |
| J1100.9+4014  | 165.233 | 40.247  | 175.938 | 63.696  | 0.140      | 0.096      | –61    | 7.6      | 0.6      | 0.1             | 8.7      | 2.2             | 1.60          | 0.17                 | PL  | ... | 8       | ...                                                                                           | ... | bzb   | RX J1100.3+4019  | ...  |
| J1102.1–6308c | 165.549 | –63.148 | 290.957 | –2.845  | 0.156      | 0.144      | 41     | 5.1      | 1.1      | 0.2             | 21.4     | 3.8             | 2.71          | 0.12                 | PL  | T   | 1,6,10  | ...                                                                                           | ... | ...   | ...              | ...  |
| J1103.4–2330  | 165.874 | –23.503 | 273.165 | 33.055  | 0.137      | 0.121      | 61     | 5.2      | 0.5      | 0.1             | 6.1      | 1.7             | 1.80          | 0.21                 | PL  | ... | ...     | 1FGL J1103.7–2329                                                                             | P   | bzb   | 1ES 1101–232     | ...  |
| J1103.9–5356  | 165.994 | –53.940 | 287.428 | 5.665   | 0.045      | 0.042      | 35     | 22.1     | 4.4      | 0.3             | 49.5     | 3.3             | 2.11          | 0.05                 | PL  | T   | ...     | 1FGL J1103.9–5355                                                                             | ... | agu   | PKS 1101–536     | ...  |
| J1104.3+0729  | 166.089 | 7.491   | 245.716 | 57.915  | 0.142      | 0.113      | –17    | 8.1      | 0.8      | 0.1             | 9.2      | 1.4             | 2.20          | 0.12                 | PL  | ... | ...     | 1FGL J1104.4+0734                                                                             | ... | bzb   | MG1 J110424+0730 | ...  |
| J1104.4+3812  | 166.120 | 38.213  | 179.818 | 65.035  | 0.011      | 0.011      | –4     | 131.5    | 29.7     | 0.6             | 375.7    | 10.5            | 1.77          | 0.01                 | PL  | T   | ...     | 1FGL J1104.4+3812<br>0FGL J1104.5+3811<br>3EG J1104+3809<br>EGR J1104+3813<br>1AGL J1104+3754 | P   | bzb   | Mkn 421          | ...  |
| J1104.7–6036  | 166.193 | –60.614 | 290.210 | –0.405  | 0.053      | 0.048      | 41     | 16.9     | 8.5      | 0.6             | 64.0     | 6.4             | 2.27          | ...                  | LP  | ... | 3       | 3EG J1102–6103<br>1AGL J1108–6103                                                             | ... | ...   | ...              | ...  |
| J1105.4–7622  | 166.368 | –76.371 | 296.691 | –14.800 | 0.124      | 0.113      | 85     | 5.1      | 0.7      | 0.2             | 9.7      | 1.9             | 2.43          | 0.14                 | PL  | ... | 4       | ...                                                                                           | ... | ...   | ...              | ...  |
| J1105.6–6114  | 166.409 | –61.236 | 290.554 | –0.933  | 0.137      | 0.108      | 25     | 10.0     | 5.0      | 0.6             | 43.8     | 5.6             | 2.34          | ...                  | LP  | ... | 2,5     | 3EG J1102–6103<br>1AGL J1108–6103                                                             | ... | ...   | ...              | ...  |
| J1106.1+2814  | 166.536 | 28.235  | 204.061 | 66.709  | 0.104      | 0.088      | –60    | 10.4     | 0.9      | 0.1             | 10.3     | 1.3             | 2.23          | 0.10                 | PL  | T   | ...     | 1FGL J1106.5+2809                                                                             | ... | bzq   | MG2 J110606+2812 | ...  |
| J1106.3–3643  | 166.599 | –36.720 | 280.520 | 21.538  | 0.156      | 0.132      | 65     | 5.9      | 0.7      | 0.1             | 8.0      | 1.5             | 2.20          | 0.14                 | PL  | ... | ...     | ...                                                                                           | ... | agu   | PMN J1106–3647   | ...  |
| J1107.2–4448  | 166.820 | –44.807 | 284.188 | 14.241  | 0.150      | 0.118      | –4     | 10.6     | 0.9      | 0.2             | 17.1     | 1.7             | 2.67          | 0.10                 | PL  | T   | ...     | ...                                                                                           | ... | bzq   | PKS 1104–445     | ...  |
| J1107.5+0223  | 166.878 | 2.386   | 253.331 | 54.918  | 0.112      | 0.098      | 32     | 6.3      | 0.6      | 0.1             | 7.2      | 1.5             | 2.11          | 0.16                 | PL  | ... | ...     | ...                                                                                           | ... | bzb   | BZB J1107+0222   | ...  |

Table 1—Continued

| Name 2FGL     | R.A.    | Decl.   | $l$     | $b$    | $\theta_1$ | $\theta_2$ | $\phi$ | $\sigma$ | $F_{35}$ | $\Delta F_{35}$ | $S_{25}$ | $\Delta S_{25}$ | $\Gamma_{25}$ | $\Delta \Gamma_{25}$ | Mod | Var | Flags | $\gamma$ -ray Assoc. | TeV | Class | ID or Assoc.          | Ref. |
|---------------|---------|---------|---------|--------|------------|------------|--------|----------|----------|-----------------|----------|-----------------|---------------|----------------------|-----|-----|-------|----------------------|-----|-------|-----------------------|------|
| J1107.8+1505  | 166.961 | 15.086  | 234.231 | 63.087 | 0.091      | 0.085      | -34    | 7.2      | 0.6      | 0.1             | 6.9      | 1.6             | 1.86          | 0.14                 | PL  | ... | ...   | 1FGL J1107.8+1502    | ... | bzb   | 87GB 110510.0+151723  | ...  |
| J1109.3+2414  | 167.349 | 24.240  | 214.370 | 66.870 | 0.123      | 0.116      | 57     | 4.1      | 0.3      | 0.1             | 4.0      | 1.5             | 1.71          | 0.24                 | PL  | ... | ...   | ...                  | ... | bzb   | 1ES 1106+244          | ...  |
| J1110.1-1835  | 167.535 | -18.585 | 271.916 | 38.111 | 0.109      | 0.096      | -20    | 7.7      | 0.8      | 0.1             | 9.3      | 1.8             | 1.96          | 0.12                 | PL  | ... | ...   | 1FGL J1110.2-1839    | ... | bzb   | CRATES J1110-1835     | ...  |
| J1110.2+7134  | 167.557 | 71.580  | 133.641 | 43.382 | 0.111      | 0.098      | 86     | 4.6      | 0.3      | 0.1             | 3.5      | 1.0             | 2.10          | 0.22                 | PL  | ... | ...   | 1FGL J1109.9+7134    | ... | bzb   | 87GB 110723.4+715023  | ...  |
| J1112.1-6040  | 168.031 | -60.672 | 291.063 | -0.109 | 0.033      | 0.033      | -2     | 22.8     | 12.6     | 0.8             | 77.9     | 6.6             | 2.10          | ...                  | LP  | ... | ...   | 1FGL J1112.1-6041c   | ... | †     | ...                   | ...  |
|               |         |         |         |        |            |            |        |          |          |                 |          |                 |               |                      |     |     |       | 1AGL J1108-6103      |     |       |                       |      |
| J1112.4+3450  | 168.108 | 34.850  | 186.778 | 67.493 | 0.087      | 0.066      | -65    | 19.3     | 1.7      | 0.2             | 21.6     | 1.5             | 2.37          | 0.06                 | PL  | T   | ...   | 1FGL J1112.8+3444    | ... | bzq   | TXS 1109+350          | ...  |
| J1112.5-6105  | 168.135 | -61.091 | 291.267 | -0.479 | 0.062      | 0.055      | -63    | 11.3     | 5.6      | 0.6             | 63.5     | 7.5             | 2.16          | 0.07                 | PL  | ... | ...   | 1AGL J1108-6103      | ... | psr   | PSR J1112-6103        | ...  |
| J1115.0-0701  | 168.760 | -7.027  | 265.109 | 48.636 | 0.094      | 0.087      | -0     | 4.6      | 0.3      | 0.1             | 4.7      | 1.8             | 1.60          | 0.28                 | PL  | ... | ...   | ...                  | ... | ...   | ...                   | ...  |
| J1117.2-4844  | 169.303 | -48.742 | 287.344 | 11.257 | 0.204      | 0.152      | -53    | 6.3      | 0.8      | 0.2             | 10.3     | 1.7             | 2.40          | 0.12                 | PL  | ... | 2,4   | ...                  | ... | agu   | CRATES J1117-4838     | ...  |
| J1117.2+2013  | 169.305 | 20.227  | 225.633 | 67.395 | 0.044      | 0.041      | -76    | 18.9     | 1.9      | 0.2             | 25.1     | 3.3             | 1.70          | 0.07                 | PL  | T   | ...   | 1FGL J1117.1+2013    | ... | bzb   | RBS 0958              | ...  |
| J1117.2-5341  | 169.316 | -53.697 | 289.159 | 6.638  | 0.111      | 0.106      | 82     | 4.8      | 0.6      | 0.2             | 7.2      | 1.9             | 1.92          | 0.18                 | PL  | ... | ...   | 1FGL J1117.0-5339    | ... | ...   | ...                   | ...  |
| J1118.0+5354  | 169.507 | 53.916  | 149.217 | 58.184 | 0.060      | 0.057      | -18    | 11.0     | 0.8      | 0.1             | 9.5      | 1.6             | 1.91          | 0.12                 | PL  | ... | ...   | 1FGL J1118.0+5354    | ... | bzb   | BZB J1117+5355        | ...  |
| J1118.1-4629  | 169.546 | -46.486 | 286.664 | 13.419 | 0.173      | 0.162      | 15     | 6.4      | 0.6      | 0.1             | 10.6     | 1.7             | 2.62          | 0.12                 | PL  | ... | ...   | ...                  | ... | bzq   | PKS 1116-46           | ...  |
| J1118.8-6128  | 169.703 | -61.473 | 292.107 | -0.564 | 0.057      | 0.048      | -47    | 19.6     | 9.0      | 0.6             | 79.1     | 5.8             | 2.30          | ...                  | EC  | ... | ...   | 1FGL J1119.4-6127c   | E   | PSR   | PSR J1119-6127        | ...  |
| J1118.9-6027c | 169.736 | -60.466 | 291.770 | 0.386  | 0.154      | 0.125      | -77    | 8.6      | 2.6      | 0.4             | 27.7     | 4.1             | 2.46          | ...                  | LP  | ... | 1,5,6 | ...                  | ... | ...   | ...                   | ...  |
| J1120.0-2204  | 170.002 | -22.081 | 276.495 | 36.054 | 0.063      | 0.059      | -86    | 20.5     | 2.5      | 0.2             | 18.0     | 1.6             | 2.20          | ...                  | LP  | ... | ...   | 1FGL J1119.9-2205    | ... | ...   | ...                   | ...  |
| J1120.4+0710  | 170.117 | 7.172   | 251.527 | 60.610 | 0.089      | 0.078      | -80    | 8.9      | 0.9      | 0.1             | 9.9      | 1.7             | 1.98          | 0.11                 | PL  | ... | ...   | 1FGL J1120.4+0710    | ... | bzq   | MG1 J112039+0704      | ...  |
| J1121.0+4211  | 170.261 | 42.186  | 167.831 | 66.211 | 0.054      | 0.052      | -34    | 14.4     | 1.2      | 0.1             | 17.6     | 3.0             | 1.61          | 0.09                 | PL  | ... | ...   | 1FGL J1121.0+4209    | ... | bzb   | RBS 0970              | ...  |
| J1121.5-0554  | 170.387 | -5.912  | 266.271 | 50.449 | 0.049      | 0.048      | 64     | 30.6     | 3.9      | 0.3             | 47.2     | 2.3             | 2.30          | 0.04                 | PL  | T   | 10    | 1FGL J1121.5-0554    | ... | bzq   | PKS 1118-05           | 13   |
| J1123.3-2527  | 170.838 | -25.466 | 279.043 | 33.287 | 0.203      | 0.128      | 8      | 4.5      | 0.5      | 0.1             | 5.5      | 1.5             | 1.94          | 0.16                 | PL  | ... | ...   | 1FGL J1123.6-2528    | ... | ...   | ...                   | ...  |
| J1124.2-3654  | 171.051 | -36.906 | 284.139 | 22.762 | 0.078      | 0.068      | 72     | 12.1     | 1.7      | 0.2             | 18.5     | 2.2             | 2.09          | 0.08                 | PL  | ... | ...   | 1FGL J1124.4-3654    | ... | psr   | PSR J1124-36          | ...  |
| J1124.2+2338  | 171.074 | 23.648  | 218.120 | 70.040 | 0.128      | 0.112      | -74    | 8.2      | 0.6      | 0.1             | 8.3      | 1.2             | 2.41          | 0.12                 | PL  | ... | ...   | 1FGL J1123.9+2339    | ... | bzq   | OM 235                | ...  |
| J1124.6-5913  | 171.175 | -59.222 | 292.028 | 1.801  | 0.049      | 0.043      | 28     | 24.4     | 7.2      | 0.4             | 67.4     | 4.3             | 2.36          | ...                  | EC  | ... | ...   | ...                  | ... | PSR   | PSR J1124-5916        | ...  |
| J1125.0-5821  | 171.272 | -58.361 | 291.793 | 2.631  | 0.151      | 0.138      | 47     | 4.8      | 1.1      | 0.2             | 12.9     | 2.9             | 2.20          | 0.16                 | PL  | ... | ...   | ...                  | ... | psr   | PSR J1125-5825        | ...  |
| J1125.2+4933  | 171.317 | 49.553  | 153.573 | 62.135 | 0.123      | 0.107      | -85    | 4.1      | 0.3      | 0.1             | 3.3      | 1.1             | 1.88          | 0.28                 | PL  | ... | ...   | ...                  | ... | bzb   | GB6 J1124+4933        | ...  |
| J1125.6-3559  | 171.420 | -35.999 | 284.089 | 23.715 | 0.134      | 0.095      | 52     | 6.5      | 0.8      | 0.2             | 9.3      | 1.9             | 1.93          | 0.13                 | PL  | T   | ...   | 1FGL J1125.5-3559    | ... | bzb   | PMN J1125-3556        | ...  |
| J1126.0-0743  | 171.502 | -7.721  | 269.196 | 49.473 | 0.094      | 0.090      | -78    | 4.6      | 0.4      | 0.1             | 4.9      | 1.7             | 1.67          | 0.21                 | PL  | ... | ...   | 1FGL J1126.0-0741    | ... | bzb   | 1RXS J112551.6-074219 | ...  |
| J1126.6-1856  | 171.661 | -18.946 | 276.601 | 39.551 | 0.060      | 0.055      | 28     | 30.1     | 3.4      | 0.2             | 43.2     | 2.1             | 2.36          | 0.04                 | PL  | T   | ...   | 1FGL J1126.8-1854    | ... | bzq   | PKS 1124-186          | ...  |
| J1127.6+3622  | 171.908 | 36.370  | 180.228 | 69.991 | 0.107      | 0.089      | -59    | 8.7      | 0.7      | 0.1             | 8.5      | 1.3             | 2.24          | 0.13                 | PL  | T   | ...   | ...                  | ... | bzq   | MG2 J112758+3620      | ...  |
| J1129.0-0532  | 172.269 | -5.539  | 268.509 | 51.742 | 0.140      | 0.128      | 18     | 8.1      | 0.6      | 0.1             | 12.4     | 1.6             | 2.70          | 0.12                 | PL  | T   | ...   | 1FGL J1129.2-0528    | ... | ...   | ...                   | ...  |
| J1129.5+3758  | 172.379 | 37.971  | 175.539 | 69.686 | 0.145      | 0.096      | 85     | 11.1     | 1.0      | 0.1             | 11.9     | 1.4             | 2.26          | 0.10                 | PL  | ... | ...   | 1FGL J1129.3+3757    | ... | ...   | ...                   | ...  |
| J1130.3-1448  | 172.580 | -14.803 | 275.330 | 43.679 | 0.083      | 0.076      | 84     | 24.9     | 1.8      | 0.2             | 34.6     | 1.7             | 2.70          | 0.05                 | PL  | T   | ...   | 1FGL J1130.2-1447    | ... | bzq   | PKS 1127-14           | ...  |
|               |         |         |         |        |            |            |        |          |          |                 |          |                 |               |                      |     |     |       | 0FGL J1129.8-1443    |     |       |                       |      |
| J1130.9+5809  | 172.731 | 58.163  | 141.830 | 55.912 | 0.112      | 0.092      | -59    | 6.4      | 0.4      | 0.1             | 4.7      | 0.9             | 2.19          | 0.26                 | PL  | ... | ...   | ...                  | ... | bzb   | BZB J1131+5809        | ...  |

Table 1—Continued

| Name 2FGL     | R.A.    | Decl.   | $l$     | $b$     | $\theta_1$ | $\theta_2$ | $\phi$ | $\sigma$ | $F_{35}$ | $\Delta F_{35}$ | $S_{25}$ | $\Delta S_{25}$ | $\Gamma_{25}$ | $\Delta \Gamma_{25}$ | Mod | Var | Flags                                      | $\gamma$ -ray Assoc.                                     | TeV | Class         | ID or Assoc.          | Ref. |
|---------------|---------|---------|---------|---------|------------|------------|--------|----------|----------|-----------------|----------|-----------------|---------------|----------------------|-----|-----|--------------------------------------------|----------------------------------------------------------|-----|---------------|-----------------------|------|
| J1132.9+0033  | 173.226 | 0.559   | 264.326 | 57.422  | 0.088      | 0.071      | −2     | 16.7     | 1.8      | 0.2             | 20.8     | 1.9             | 2.18          | 0.07                 | PL  | T   | ...<br>1FGL J1133.1+0033<br>3EG J1133+0033 | ...                                                      | bzb | PKS B1130+008 | ...                   |      |
| J1134.4−7415  | 173.620 | −74.260 | 297.685 | −12.177 | 0.156      | 0.135      | 58     | 4.4      | 0.7      | 0.2             | 8.1      | 1.8             | 2.25          | 0.13                 | PL  | ... | ...                                        | ...                                                      | ... | agu           | PKS 1133−739          | ...  |
| J1135.2−6829  | 173.820 | −68.496 | 296.018 | −6.653  | 0.177      | 0.134      | 52     | 5.7      | 0.8      | 0.2             | 11.7     | 2.0             | 2.51          | 0.13                 | PL  | ... | 1,4                                        | ...                                                      | ... | agu           | PKS 1133−681          | ...  |
| J1135.3−6054  | 173.850 | −60.914 | 293.821 | 0.606   | 0.054      | 0.050      | 18     | 18.9     | 6.1      | 0.5             | 52.4     | 3.7             | 2.33          | ...                  | EC  | ... | ...                                        | 1FGL J1134.8−6055                                        | ... | PSR           | LAT PSR J1135−6055    | ...  |
| J1136.3+6736  | 174.081 | 67.607  | 133.483 | 47.953  | 0.078      | 0.077      | 26     | 8.6      | 0.6      | 0.1             | 8.4      | 1.9             | 1.68          | 0.12                 | PL  | ... | ...                                        | 1FGL J1136.2+6739                                        | ... | bzb           | RX J1136.5+6737       | ...  |
| J1136.7+7009  | 174.178 | 70.164  | 131.876 | 45.645  | 0.049      | 0.045      | −7     | 15.0     | 1.1      | 0.1             | 14.9     | 2.2             | 1.74          | 0.08                 | PL  | ... | ...                                        | 1FGL J1136.6+7009                                        | P   | bzb           | Mkn 180               | ...  |
| J1137.0+2553  | 174.267 | 25.893  | 212.961 | 73.332  | 0.108      | 0.089      | −68    | 5.0      | 0.3      | 0.1             | 4.8      | 1.9             | 1.44          | 0.25                 | PL  | ... | ...                                        | 1FGL J1136.9+2551                                        | ... | bzb           | RX J1136.8+2551       | ...  |
| J1138.8−6233c | 174.702 | −62.559 | 294.675 | −0.857  | 0.181      | 0.117      | −33    | 4.9      | 2.0      | 0.4             | 22.7     | 4.5             | 2.18          | 0.11                 | PL  | ... | 4,6,9                                      | ...                                                      | ... | ...           | ...                   | ...  |
| J1141.0+6803  | 175.254 | 68.053  | 132.608 | 47.731  | 0.083      | 0.075      | 90     | 6.2      | 0.3      | 0.1             | 5.7      | 1.9             | 1.45          | 0.20                 | PL  | ... | 1,5                                        | ...                                                      | ... | agu           | NVSS J114118+680429   | ...  |
| J1141.7−1404  | 175.439 | −14.074 | 278.474 | 45.463  | 0.105      | 0.091      | −68    | 5.9      | 0.6      | 0.1             | 6.8      | 1.6             | 1.89          | 0.15                 | PL  | ... | ...                                        | 1FGL J1141.8−1403                                        | ... | agu           | 1RXS J114142.2−140757 | ...  |
| J1141.9+1550  | 175.495 | 15.844  | 244.395 | 70.331  | 0.102      | 0.089      | 35     | 7.8      | 0.7      | 0.1             | 8.3      | 1.5             | 2.07          | 0.14                 | PL  | ... | ...                                        | 1FGL J1141.8+1549                                        | ... | bzb           | MG1 J114208+1547      | ...  |
| J1142.9+0121  | 175.735 | 1.354   | 267.559 | 59.437  | 0.091      | 0.079      | −38    | 11.0     | 1.2      | 0.2             | 13.2     | 1.8             | 2.02          | 0.10                 | PL  | T   | ...                                        | 1FGL J1142.7+0127                                        | ... | psr           | PSR J1142+01          | ...  |
| J1143.1+6119  | 175.798 | 61.324  | 136.768 | 53.933  | 0.105      | 0.090      | −78    | 9.0      | 0.8      | 0.1             | 8.3      | 1.3             | 2.07          | 0.12                 | PL  | ... | ...                                        | ...                                                      | ... | bzb           | 87GB 114026.7+613850  | ...  |
| J1146.8−3812  | 176.721 | −38.207 | 289.213 | 22.939  | 0.087      | 0.078      | −70    | 14.1     | 1.6      | 0.2             | 19.5     | 1.8             | 2.31          | 0.07                 | PL  | T   | ...                                        | 1FGL J1146.9−3812                                        | ... | bzq           | PKS 1144+379          | ...  |
| J1146.9+4000  | 176.737 | 40.006  | 164.887 | 71.448  | 0.065      | 0.061      | 46     | 23.3     | 2.0      | 0.2             | 25.9     | 1.6             | 2.35          | 0.05                 | PL  | T   | ...                                        | 0FGL J1146.7−3808<br>1FGL J1146.8+4004                   | ... | bzq           | S4 1144+40            | ...  |
| J1147.7−0724  | 176.940 | −7.400  | 276.597 | 52.185  | 0.089      | 0.080      | −50    | 15.1     | 1.7      | 0.2             | 20.2     | 1.8             | 2.30          | 0.07                 | PL  | T   | ...                                        | 1FGL J1147.7−0722                                        | ... | bzq           | PKS 1145−071          | ...  |
| J1150.1+2419  | 177.536 | 24.330  | 220.982 | 75.925  | 0.089      | 0.084      | 45     | 13.7     | 1.3      | 0.2             | 14.9     | 1.6             | 2.19          | 0.08                 | PL  | ... | ...                                        | 1FGL J1150.2+2419                                        | ... | bzb           | B2 1147+24            | ...  |
| J1150.5+4154  | 177.631 | 41.910  | 159.135 | 70.674  | 0.045      | 0.043      | −43    | 21.4     | 2.2      | 0.2             | 28.6     | 3.2             | 1.76          | 0.06                 | PL  | ... | ...                                        | 1FGL J1150.5+4152                                        | ... | bzb           | RBS 1040              | ...  |
| J1151.5−1347  | 177.877 | −13.785 | 281.508 | 46.579  | 0.077      | 0.074      | 7      | 5.7      | 0.4      | 0.1             | 5.7      | 1.7             | 1.71          | 0.21                 | PL  | ... | ...                                        | 1FGL J1151.4−1345                                        | ... | bzb           | PMN J1151−1347        | ...  |
| J1151.5+5857  | 177.880 | 58.958  | 136.912 | 56.515  | 0.051      | 0.047      | 76     | 11.2     | 0.8      | 0.1             | 9.6      | 1.7             | 1.79          | 0.13                 | PL  | ... | ...                                        | 1FGL J1151.6+5857                                        | ... | bzb           | TXS 1148+592          | ...  |
| J1152.4−0840  | 178.112 | −8.674  | 279.117 | 51.449  | 0.101      | 0.092      | 63     | 10.0     | 1.2      | 0.2             | 13.3     | 1.8             | 2.17          | 0.11                 | PL  | ... | ...                                        | 1FGL J1152.2−0836                                        | ... | bzq           | PKS B1149−084         | ...  |
| J1153.2+4935  | 178.305 | 49.599  | 145.511 | 64.899  | 0.118      | 0.114      | −6     | 11.8     | 0.8      | 0.1             | 11.6     | 1.2             | 2.52          | 0.09                 | PL  | T   | ...                                        | ...                                                      | ... | BZQ OM 484    | 14                    |      |
| J1154.0−0010  | 178.525 | −0.169  | 273.810 | 59.421  | 0.065      | 0.060      | −45    | 9.4      | 0.8      | 0.1             | 9.7      | 1.9             | 1.86          | 0.15                 | PL  | T   | ...                                        | 1FGL J1154.0−0008                                        | ... | bzb           | 1RXS J115404.9−001008 | ...  |
| J1154.1−3242  | 178.544 | −32.713 | 289.221 | 28.630  | 0.080      | 0.075      | 54     | 9.5      | 1.1      | 0.2             | 12.4     | 1.9             | 2.03          | 0.10                 | PL  | ... | ...                                        | 1FGL J1154.2−3242                                        | ... | agu           | PKS 1151−324          | ...  |
| J1154.4+6019  | 178.624 | 60.320  | 135.319 | 55.418  | 0.168      | 0.123      | 22     | 7.5      | 0.4      | 0.1             | 9.5      | 1.3             | 2.78          | 0.13                 | PL  | T   | ...                                        | 1FGL J1152.1+6027                                        | ... | bzq           | RX J1154.0+6022       | ...  |
| J1156.7−0751  | 179.187 | −7.851  | 280.259 | 52.596  | 0.260      | 0.239      | −29    | 4.3      | 0.5      | 0.1             | 6.6      | 1.6             | 2.49          | 0.20                 | PL  | ... | ...                                        | 1FGL J1156.7−0751                                        | ... | ...           | ...                   | ...  |
| J1158.8+0939  | 179.709 | 9.651   | 265.073 | 68.564  | 0.155      | 0.139      | −44    | 6.7      | 0.7      | 0.1             | 7.4      | 1.4             | 2.14          | 0.14                 | PL  | T   | ...                                        | ...                                                      | ... | bzb           | GB6 J1158+0937        | ...  |
| J1159.0−2226  | 179.756 | −22.439 | 287.326 | 38.839  | 0.097      | 0.084      | 19     | 9.7      | 1.3      | 0.2             | 16.2     | 2.1             | 2.35          | 0.10                 | PL  | T   | 5                                          | ...                                                      | ... | agu           | PKS 1156−221          | ...  |
| J1159.3−2142  | 179.837 | −21.701 | 287.173 | 39.571  | 0.072      | 0.068      | −84    | 12.3     | 1.6      | 0.2             | 20.3     | 2.2             | 2.33          | 0.09                 | PL  | T   | ...                                        | 1FGL J1159.4−2149                                        | ... | bzq           | PMN J1159−2142        | ...  |
| J1159.5+2914  | 179.878 | 29.247  | 199.411 | 78.370  | 0.032      | 0.030      | 58     | 52.4     | 6.0      | 0.3             | 73.1     | 2.5             | 2.29          | 0.03                 | PL  | T   | ...                                        | 0FGL J1159.2+2912<br>3EG J1200+2847<br>1FGL J1159.4+2914 | ... | bzq           | Ton 599               | ...  |
| J1200.0+0159  | 180.013 | 1.996   | 274.669 | 62.014  | 0.142      | 0.133      | −39    | 6.0      | 0.6      | 0.1             | 6.6      | 1.3             | 2.20          | 0.15                 | PL  | ... | ...                                        | 1FGL J1159.8+0200                                        | ... | agu           | GB6 J1200+0202        | ...  |

Table 1—Continued

| Name 2FGL     | R.A.    | Decl.   | $l$     | $b$    | $\theta_1$ | $\theta_2$ | $\phi$ | $\sigma$ | $F_{35}$ | $\Delta F_{35}$ | $S_{25}$ | $\Delta S_{25}$ | $\Gamma_{25}$ | $\Delta \Gamma_{25}$ | Mod | Var | Flags | $\gamma$ -ray Assoc. | TeV | Class | ID or Assoc.          | Ref. |
|---------------|---------|---------|---------|--------|------------|------------|--------|----------|----------|-----------------|----------|-----------------|---------------|----------------------|-----|-----|-------|----------------------|-----|-------|-----------------------|------|
| J1203.2+6030  | 180.821 | 60.511  | 133.410 | 55.627 | 0.092      | 0.088      | −58    | 9.4      | 0.8      | 0.1             | 8.7      | 1.4             | 1.99          | 0.13                 | PL  | ... | ...   | 1FGL J1202.9+6032    | ... | bzb   | SBS 1200+608          | ...  |
| J1203.6−6243c | 180.924 | −62.719 | 297.493 | −0.352 | 0.075      | 0.069      | 80     | 9.8      | 5.1      | 0.6             | 42.0     | 6.3             | 2.35          | ...                  | LP  | ... | 5,6   | ...                  | ... | ...   | ...                   | ...  |
| J1204.2+1144  | 181.058 | 11.741  | 264.892 | 71.038 | 0.133      | 0.105      | 54     | 7.4      | 0.8      | 0.1             | 8.3      | 1.5             | 2.06          | 0.13                 | PL  | ... | ...   | 1FGL J1204.4+1139    | ... | bzb   | 1RXS J120413.0+114549 | ...  |
| J1204.3−0711  | 181.095 | −7.187  | 282.881 | 53.843 | 0.133      | 0.115      | −15    | 7.1      | 0.8      | 0.1             | 8.4      | 1.5             | 2.13          | 0.16                 | PL  | ... | ...   | 1FGL J1204.3−0714    | ... | bzb   | 1RXS J120417.0−070959 | ...  |
| J1206.0−2638  | 181.519 | −26.637 | 290.521 | 35.139 | 0.224      | 0.136      | −16    | 8.6      | 0.8      | 0.1             | 14.3     | 1.8             | 2.67          | 0.11                 | PL  | T   | ...   | 1FGL J1205.9−2637    | ... | bzq   | PKS 1203−26           | ...  |
| J1207.3−5055  | 181.838 | −50.931 | 295.874 | 11.336 | 0.150      | 0.122      | 85     | 5.8      | 0.8      | 0.2             | 9.5      | 1.8             | 2.18          | 0.12                 | PL  | ... | ...   | 1FGL J1207.0−5055    | ... | ...   | ...                   | ...  |
| J1208.5−6240  | 182.139 | −62.674 | 298.034 | −0.211 | 0.063      | 0.060      | −41    | 11.7     | 6.6      | 0.7             | 52.7     | 8.6             | 2.28          | ...                  | LP  | ... | ...   | ...                  | ... | ...   | ...                   | ...  |
| J1208.6−2257  | 182.156 | −22.956 | 290.246 | 38.859 | 0.420      | 0.227      | −37    | 4.4      | 0.4      | 0.1             | 7.1      | 1.5             | 2.59          | 0.18                 | PL  | ... | 9     | ...                  | ... | ...   | ...                   | ...  |
| J1208.8+5441  | 182.215 | 54.691  | 135.802 | 61.361 | 0.063      | 0.059      | −33    | 26.1     | 1.8      | 0.2             | 26.4     | 1.4             | 2.47          | 0.05                 | PL  | T   | ...   | 1FGL J1209.3+5444    | ... | bzq   | TXS 1206+549          | ...  |
| J1209.6+4121  | 182.403 | 41.354  | 151.384 | 73.384 | 0.091      | 0.088      | −45    | 6.2      | 0.4      | 0.1             | 6.7      | 2.0             | 1.58          | 0.17                 | PL  | ... | ...   | 1FGL J1209.4+4119    | ... | bzb   | B3 1206+416           | ...  |
| J1209.7+1807  | 182.443 | 18.122  | 253.939 | 76.838 | 0.213      | 0.149      | 49     | 4.9      | 0.4      | 0.1             | 5.8      | 1.2             | 2.46          | 0.17                 | PL  | ... | ...   | 1FGL J1209.7+1806    | ... | bzq   | MG1 J120953+1809      | ...  |
| J1213.2−2616  | 183.301 | −26.274 | 292.352 | 35.811 | 0.128      | 0.096      | −1     | 5.1      | 0.5      | 0.1             | 7.3      | 1.7             | 2.41          | 0.19                 | PL  | ... | ...   | ...                  | ... | bzb   | RBS 1080              | ...  |
| J1214.0−6237  | 183.505 | −62.620 | 298.645 | −0.060 | 0.078      | 0.059      | 81     | 13.5     | 7.0      | 0.6             | 59.4     | 6.5             | 2.26          | ...                  | LP  | ... | 5     | 1FGL J1213.7−6240c   | ... | snr   | SNR G298.6−00.0       | ...  |
| J1214.1−4410  | 183.527 | −44.167 | 295.900 | 18.194 | 0.161      | 0.117      | 41     | 6.0      | 0.8      | 0.2             | 9.1      | 1.6             | 2.25          | 0.12                 | PL  | ... | ...   | 1FGL J1213.6−4424    | ... | ...   | ...                   | ...  |
| J1214.6+1309  | 183.660 | 13.163  | 269.481 | 73.596 | 0.247      | 0.190      | 89     | 6.1      | 0.5      | 0.1             | 7.6      | 1.3             | 2.57          | 0.14                 | PL  | ... | ...   | ...                  | ... | bzq   | 4C +13.46             | ...  |
| J1214.8+1653  | 183.724 | 16.900  | 261.490 | 76.732 | 0.111      | 0.096      | 8      | 6.0      | 0.5      | 0.1             | 6.2      | 1.3             | 2.18          | 0.15                 | PL  | ... | ...   | ...                  | ... | bzq   | TXS 1214+171          | ...  |
| J1214.9+5004  | 183.729 | 50.081  | 137.433 | 66.006 | 0.095      | 0.087      | 82     | 6.7      | 0.5      | 0.1             | 5.5      | 1.2             | 2.00          | 0.17                 | PL  | T   | ...   | 1FGL J1214.9+5004    | ... | bzb   | BZB J1215+5002        | ...  |
| J1217.8+3006  | 184.467 | 30.109  | 188.926 | 82.056 | 0.031      | 0.029      | −66    | 33.6     | 5.5      | 0.3             | 61.2     | 3.5             | 2.02          | 0.04                 | PL  | T   | ...   | 1FGL J1217.7+3007    | P   | bzb   | 1ES 1215+303          | ...  |
|               |         |         |         |        |            |            |        |          |          |                 |          |                 |               |                      |     |     |       | 0FGL J1218.0+3006    |     |       |                       |      |
| J1218.5−0122  | 184.637 | −1.383  | 286.102 | 60.410 | 0.090      | 0.084      | 16     | 13.1     | 1.6      | 0.2             | 17.7     | 2.0             | 2.10          | 0.08                 | PL  | T   | ...   | 1FGL J1218.4−0128    | ... | bzb   | PKS 1216−010          | ...  |
| J1218.8−4827  | 184.713 | −48.467 | 297.374 | 14.053 | 0.152      | 0.137      | 46     | 5.0      | 0.6      | 0.1             | 8.4      | 1.8             | 2.40          | 0.15                 | PL  | ... | 4,5   | ...                  | ... | agu   | PMN J1219−4826        | ...  |
| J1219.2+7107  | 184.818 | 71.130  | 126.651 | 45.766 | 0.176      | 0.134      | 31     | 5.2      | 0.4      | 0.1             | 4.4      | 0.9             | 2.27          | 0.16                 | PL  | ... | ...   | 1FGL J1221.5+7106    | ... | bzq   | S5 1217+71            | ...  |
| J1219.7+0201  | 184.928 | 2.017   | 284.756 | 63.764 | 0.176      | 0.165      | −60    | 4.6      | 0.4      | 0.1             | 7.1      | 1.7             | 2.66          | 0.19                 | PL  | ... | ...   | ...                  | ... | bzq   | PKS 1217+02           | ...  |
| J1219.8−0310  | 184.951 | −3.174  | 287.576 | 58.751 | 0.128      | 0.126      | −62    | 5.9      | 0.6      | 0.1             | 7.4      | 1.8             | 1.86          | 0.15                 | PL  | ... | ...   | 1FGL J1219.8−0309    | ... | bzb   | 1RXS J121946.0−031419 | ...  |
| J1221.3+3010  | 185.348 | 30.179  | 186.329 | 82.739 | 0.036      | 0.035      | 88     | 20.4     | 2.8      | 0.3             | 37.8     | 4.1             | 1.71          | 0.07                 | PL  | T   | ...   | 1FGL J1221.3+3008    | P   | bzb   | PG 1218+304           | ...  |
| J1221.4−0633  | 185.358 | −6.553  | 289.680 | 55.545 | 0.136      | 0.103      | 90     | 8.3      | 0.8      | 0.1             | 10.6     | 1.5             | 2.37          | 0.12                 | PL  | ... | ...   | 1FGL J1221.4−0635    | ... | ...   | ...                   | ...  |
| J1221.4+2814  | 185.374 | 28.239  | 201.691 | 83.280 | 0.031      | 0.030      | 10     | 40.6     | 5.5      | 0.3             | 61.7     | 3.3             | 2.02          | 0.03                 | PL  | T   | ...   | 1FGL J1221.5+2814    | P   | bzb   | W Comae               | ...  |
|               |         |         |         |        |            |            |        |          |          |                 |          |                 |               |                      |     |     |       | 0FGL J1221.7+2814    |     |       |                       |      |
|               |         |         |         |        |            |            |        |          |          |                 |          |                 |               |                      |     |     |       | 1AGL J1222+2851      |     |       |                       |      |
| J1222.4+0413  | 185.616 | 4.223   | 284.870 | 66.073 | 0.092      | 0.080      | −69    | 18.3     | 1.3      | 0.2             | 28.0     | 1.9             | 2.77          | 0.07                 | PL  | T   | ...   | 1FGL J1222.5+0415    | ... | bzq   | 4C +04.42             | ...  |
| J1223.3+7954  | 185.846 | 79.910  | 124.470 | 37.134 | 0.096      | 0.082      | 20     | 4.2      | 0.2      | 0.1             | 3.3      | 1.5             | 1.36          | 0.33                 | PL  | ... | ...   | ...                  | ... | ...   | ...                   | ...  |
| J1223.9+8043  | 185.977 | 80.725  | 124.306 | 36.330 | 0.081      | 0.070      | −89    | 12.0     | 1.1      | 0.1             | 13.3     | 1.4             | 2.26          | 0.08                 | PL  | T   | ...   | 1FGL J1224.8+8044    | ... | bzb   | S5 1221+80            | ...  |
| J1224.4+2436  | 186.106 | 24.602  | 234.002 | 83.420 | 0.068      | 0.062      | −40    | 7.7      | 0.6      | 0.1             | 7.0      | 1.3             | 2.03          | 0.19                 | PL  | ... | ...   | ...                  | ... | bzb   | MS 1221.8+2452        | ...  |
| J1224.9+2122  | 186.226 | 21.380  | 255.070 | 81.660 | 0.014      | 0.013      | 24     | 182.4    | 35.4     | 0.6             | 372.9    | 5.9             | 2.23          | ...                  | LP  | T   | ...   | 1FGL J1224.7+2121    | P   | BZQ   | 4C +21.35             | ...  |
|               |         |         |         |        |            |            |        |          |          |                 |          |                 |               |                      |     |     |       | 3EG J1224+2118       |     |       |                       |      |

Table 1—Continued

| Name 2FGL    | R.A.    | Decl.   | $l$     | $b$     | $\theta_1$ | $\theta_2$ | $\phi$ | $\sigma$ | $F_{35}$ | $\Delta F_{35}$ | $S_{25}$ | $\Delta S_{25}$ | $\Gamma_{25}$ | $\Delta \Gamma_{25}$ | Mod | Var | Flags | $\gamma$ -ray Assoc.                                                                          | TeV | Class | ID or Assoc.         | Ref. |
|--------------|---------|---------|---------|---------|------------|------------|--------|----------|----------|-----------------|----------|-----------------|---------------|----------------------|-----|-----|-------|-----------------------------------------------------------------------------------------------|-----|-------|----------------------|------|
| J1225.0+4335 | 186.255 | 43.594  | 139.191 | 72.691  | 0.198      | 0.166      | 46     | 6.5      | 0.4      | 0.1             | 6.6      | 1.1             | 2.52          | 0.15                 | PL  | ... | ...   | 1FGL J1225.8+4336<br>3EG J1227+4302                                                           | ... | bzb   | B3 1222+438          | ...  |
| J1226.0+2953 | 186.521 | 29.896  | 185.018 | 83.782  | 0.070      | 0.064      | 27     | 12.9     | 1.7      | 0.2             | 9.1      | 1.3             | 1.98          | ...                  | LP  | T   | ...   | 1FGL J1226.0+2954                                                                             | ... | ...   | ...                  | ...  |
| J1226.7–1331 | 186.676 | –13.523 | 293.764 | 48.908  | 0.074      | 0.070      | 57     | 9.9      | 1.3      | 0.2             | 14.1     | 2.2             | 1.97          | 0.12                 | PL  | T   | ...   | 1FGL J1226.7–1332                                                                             | ... | bzb   | PMN J1226–1328       | ...  |
| J1226.9+4940 | 186.739 | 49.674  | 133.089 | 66.969  | 0.264      | 0.202      | –74    | 5.0      | 0.5      | 0.1             | 6.5      | 1.5             | 2.39          | 0.20                 | PL  | ... | 5,8   | ...                                                                                           | ... | bzq   | 87GB 122531.6+494958 | ...  |
| J1227.7–4853 | 186.928 | –48.891 | 298.920 | 13.795  | 0.059      | 0.051      | 3      | 24.3     | 3.5      | 0.3             | 33.4     | 2.3             | 2.33          | ...                  | LP  | ... | ...   | 1FGL J1227.9–4852                                                                             | ... | ...   | ...                  | ...  |
| J1228.6+4857 | 187.170 | 48.953  | 132.826 | 67.735  | 0.086      | 0.079      | –38    | 8.5      | 0.7      | 0.1             | 9.8      | 1.5             | 2.39          | 0.13                 | PL  | T   | ...   | 1FGL J1228.2+4855                                                                             | ... | bzq   | TXS 1226+492         | ...  |
| J1228.7–8310 | 187.179 | –83.171 | 302.213 | –20.331 | 0.178      | 0.166      | 9      | 4.5      | 0.5      | 0.1             | 8.0      | 1.6             | 2.62          | 0.16                 | PL  | ... | 4     | 3EG J1249–8330                                                                                | ... | agu   | PKS 1221–82          | ...  |
| J1229.1+0202 | 187.277 | 2.042   | 289.954 | 64.349  | 0.022      | 0.021      | 75     | 140.6    | 15.1     | 0.4             | 272.0    | 3.4             | 2.62          | ...                  | LP  | T   | ...   | 1FGL J1229.1+0203<br>0FGL J1229.1+0202<br>3EG J1229+0210<br>EGR J1229+0203<br>1AGL J1228+0142 | ... | BZQ   | 3C 273               | ...  |
| J1230.2+2517 | 187.561 | 25.291  | 232.876 | 84.905  | 0.132      | 0.104      | –78    | 9.4      | 0.9      | 0.1             | 10.5     | 1.4             | 2.27          | 0.11                 | PL  | T   | ...   | 1FGL J1230.4+2520                                                                             | ... | bzb   | ON 246               | ...  |
| J1230.2–5258 | 187.575 | –52.979 | 299.707 | 9.761   | 0.144      | 0.141      | 30     | 4.1      | 0.6      | 0.2             | 7.4      | 1.8             | 2.21          | 0.18                 | PL  | ... | ...   | ...                                                                                           | ... | agu   | PMN J1229–5303       | ...  |
| J1230.8+1224 | 187.701 | 12.406  | 283.744 | 74.504  | 0.066      | 0.061      | 62     | 16.7     | 1.7      | 0.2             | 19.6     | 1.8             | 2.17          | 0.07                 | PL  | ... | ...   | 1FGL J1230.8+1223                                                                             | P   | rdg   | M 87                 | ...  |
| J1231.1–6512 | 187.793 | –65.212 | 300.808 | –2.424  | 0.125      | 0.117      | –13    | 8.1      | 1.9      | 0.3             | 18.5     | 2.7             | 2.36          | ...                  | LP  | ... | 4     | ...                                                                                           | ... | ...   | ...                  | ...  |
| J1231.2–1411 | 187.815 | –14.187 | 295.557 | 48.396  | 0.023      | 0.022      | 75     | 73.3     | 17.7     | 0.5             | 105.7    | 3.1             | 1.95          | ...                  | EC  | ... | ...   | 1FGL J1231.1–1410<br>0FGL J1231.5–1410<br>EGR J1231–1412                                      | ... | PSR   | PSR J1231–1411       | ...  |
| J1231.3–5112 | 187.837 | –51.210 | 299.724 | 11.536  | 0.157      | 0.128      | –3     | 10.1     | 1.1      | 0.2             | 13.5     | 1.8             | 2.51          | ...                  | LP  | T   | ...   | 1FGL J1232.2–5118                                                                             | ... | ...   | ...                  | ...  |
| J1231.6+1417 | 187.917 | 14.291  | 282.199 | 76.361  | 0.132      | 0.114      | –11    | 6.3      | 0.6      | 0.1             | 7.0      | 1.4             | 2.15          | 0.16                 | PL  | ... | 2     | ...                                                                                           | ... | bzb   | GB6 J1231+1421       | ...  |
| J1231.7+2848 | 187.937 | 28.809  | 190.658 | 85.340  | 0.039      | 0.036      | –59    | 29.0     | 3.5      | 0.2             | 41.7     | 3.4             | 1.87          | 0.05                 | PL  | T   | ...   | 1FGL J1231.6+2850                                                                             | ... | bzb   | B2 1229+29           | ...  |
| J1233.7–0145 | 188.437 | –1.763  | 293.844 | 60.797  | 0.110      | 0.102      | 79     | 9.7      | 1.0      | 0.2             | 12.2     | 1.6             | 2.23          | 0.11                 | PL  | ... | ...   | 1FGL J1233.6–0146                                                                             | ... | bzb   | BZB J1233–0144       | ...  |
| J1234.0–5733 | 188.515 | –57.553 | 300.593 | 5.240   | 0.101      | 0.080      | –0     | 7.9      | 1.6      | 0.2             | 18.2     | 2.6             | 2.17          | 0.10                 | PL  | ... | ...   | 1FGL J1234.0–5736                                                                             | ... | agu   | PMN J1234–5736       | ...  |
| J1236.1–6155 | 189.041 | –61.923 | 301.136 | 0.896   | 0.147      | 0.128      | 54     | 5.1      | 1.8      | 0.4             | 23.9     | 4.4             | 2.40          | 0.11                 | PL  | ... | 4,5   | ...                                                                                           | ... | ...   | ...                  | ...  |
| J1238.1–1953 | 189.527 | –19.892 | 298.655 | 42.869  | 0.142      | 0.121      | 1      | 4.9      | 0.5      | 0.1             | 5.9      | 1.3             | 2.29          | 0.18                 | PL  | ... | ...   | ...                                                                                           | ... | agu   | PMN J1238–1959       | ...  |
| J1239.5+0443 | 189.880 | 4.730   | 295.180 | 67.422  | 0.041      | 0.040      | –25    | 36.7     | 4.5      | 0.3             | 55.0     | 2.4             | 2.32          | 0.04                 | PL  | T   | ...   | 1FGL J1239.5+0443<br>3EG J1236+0457<br>EGR J1237+0434<br>1AGL J1238+0406                      | ... | bzq   | MG1 J123931+0443     | ...  |
| J1239.5+0728 | 189.885 | 7.478   | 294.217 | 70.148  | 0.116      | 0.111      | 20     | 4.4      | 0.4      | 0.1             | 4.8      | 1.5             | 1.89          | 0.19                 | PL  | ... | ...   | ...                                                                                           | ... | agu   | PKS 1236+077         | ...  |
| J1240.6–7151 | 190.163 | –71.866 | 302.083 | –9.012  | 0.078      | 0.071      | 15     | 8.2      | 1.1      | 0.2             | 13.2     | 2.5             | 1.82          | 0.16                 | PL  | ... | ...   | 1FGL J1240.3–7154                                                                             | ... | ...   | ...                  | ...  |
| J1241.6–1457 | 190.405 | –14.957 | 299.398 | 47.847  | 0.159      | 0.127      | 16     | 4.6      | 0.5      | 0.1             | 5.2      | 1.4             | 1.98          | 0.19                 | PL  | ... | ...   | ...                                                                                           | ... | bzb   | RX J1241.8–1455      | ...  |
| J1243.1+3627 | 190.780 | 36.451  | 133.128 | 80.513  | 0.046      | 0.042      | 84     | 19.3     | 1.9      | 0.2             | 25.5     | 3.3             | 1.70          | 0.07                 | PL  | ... | ...   | 1FGL J1243.1+3627                                                                             | ... | bzb   | Ton 116              | ...  |

Table 1—Continued

| Name 2FGL     | R.A.    | Decl.   | $l$     | $b$    | $\theta_1$ | $\theta_2$ | $\phi$ | $\sigma$ | $F_{35}$ | $\Delta F_{35}$ | $S_{25}$ | $\Delta S_{25}$ | $\Gamma_{25}$ | $\Delta \Gamma_{25}$ | Mod | Var | Flags | $\gamma$ -ray Assoc.                                                                          | TeV | Class | ID or Assoc.          | Ref. |
|---------------|---------|---------|---------|--------|------------|------------|--------|----------|----------|-----------------|----------|-----------------|---------------|----------------------|-----|-----|-------|-----------------------------------------------------------------------------------------------|-----|-------|-----------------------|------|
| J1243.9–6232  | 190.982 | –62.541 | 302.067 | 0.318  | 0.097      | 0.088      | 56     | 5.3      | 2.2      | 0.4             | 26.6     | 4.9             | 2.31          | 0.10                 | PL  | ... | 3,4   | ...                                                                                           | ... | ...   | ...                   | ...  |
| J1245.1+5708  | 191.279 | 57.134  | 124.646 | 59.973 | 0.093      | 0.088      | 67     | 6.5      | 0.5      | 0.1             | 5.4      | 1.1             | 2.11          | 0.17                 | PL  | ... | ...   | ...                                                                                           | ... | bzb   | 1RXS J124510.5+571020 | ...  |
| J1246.7–2546  | 191.681 | –25.783 | 301.602 | 37.077 | 0.030      | 0.029      | 58     | 56.7     | 8.7      | 0.4             | 88.9     | 3.1             | 2.26          | ...                  | LP  | T   | ...   | 1FGL J1246.7–2545<br>0FGL J1246.6–2544                                                        | ... | bzq   | PKS 1244–255          | ...  |
| J1248.2+5820  | 192.063 | 58.350  | 123.738 | 58.773 | 0.033      | 0.032      | –61    | 36.1     | 4.1      | 0.2             | 46.7     | 3.0             | 1.95          | 0.04                 | PL  | ... | ...   | 1FGL J1248.2+5820                                                                             | ... | bzb   | PG 1246+586           | ...  |
| J1248.6–5510  | 192.158 | –55.174 | 302.528 | 7.696  | 0.189      | 0.150      | –78    | 5.2      | 0.8      | 0.2             | 11.3     | 2.1             | 2.47          | 0.13                 | PL  | ... | 1     | ...                                                                                           | ... | ...   | ...                   | ...  |
| J1249.5–2811  | 192.379 | –28.183 | 302.417 | 34.686 | 0.091      | 0.079      | 52     | 5.4      | 0.5      | 0.1             | 5.9      | 1.5             | 1.96          | 0.18                 | PL  | ... | ...   | 1FGL J1249.3–2812                                                                             | ... | ...   | ...                   | ...  |
| J1249.9+3705  | 192.477 | 37.090  | 124.692 | 80.033 | 0.095      | 0.078      | 58     | 9.0      | 0.7      | 0.1             | 10.5     | 2.5             | 1.58          | 0.13                 | PL  | ... | ...   | 1FGL J1249.8+3706                                                                             | ... | bzb   | RX J1249.8+3708       | ...  |
| J1251.2+1045  | 192.812 | 10.757  | 302.769 | 73.628 | 0.155      | 0.117      | 50     | 4.4      | 0.4      | 0.1             | 5.0      | 1.4             | 1.93          | 0.20                 | PL  | T   | ...   | 1FGL J1251.3+1044                                                                             | ... | bzb   | 1RXS J125117.4+103914 | ...  |
| J1253.1+5302  | 193.276 | 53.047  | 122.360 | 64.080 | 0.038      | 0.036      | 17     | 32.9     | 3.7      | 0.2             | 42.0     | 2.8             | 1.97          | 0.04                 | PL  | T   | ...   | 1FGL J1253.0+5301<br>0FGL J1253.4+5300                                                        | ... | bzb   | S4 1250+53            | ...  |
| J1254.1+6237  | 193.537 | 62.620  | 122.395 | 54.506 | 0.104      | 0.099      | 31     | 5.0      | 0.3      | 0.1             | 3.6      | 0.9             | 2.02          | 0.21                 | PL  | ... | ...   | 1FGL J1254.0+6236                                                                             | ... | bzb   | BZB J1253+6242        | ...  |
| J1254.2–2203  | 193.571 | –22.052 | 303.804 | 40.815 | 0.147      | 0.125      | 83     | 5.4      | 0.7      | 0.2             | 8.3      | 1.7             | 2.26          | 0.14                 | PL  | ... | ...   | ...                                                                                           | ... | ...   | ...                   | ...  |
| J1254.4+2209  | 193.611 | 22.156  | 310.921 | 84.981 | 0.084      | 0.082      | –32    | 7.7      | 0.7      | 0.1             | 7.7      | 1.5             | 1.99          | 0.13                 | PL  | ... | ...   | 1FGL J1254.4+2209                                                                             | ... | bzb   | TXS 1252+224          | ...  |
| J1255.8–5828  | 193.964 | –58.472 | 303.512 | 4.395  | 0.357      | 0.237      | 30     | 4.5      | 0.8      | 0.2             | 12.4     | 2.5             | 2.51          | 0.13                 | PL  | ... | 4     | ...                                                                                           | ... | ...   | ...                   | ...  |
| J1256.1–0547  | 194.042 | –5.794  | 305.097 | 57.058 | 0.017      | 0.016      | 29     | 147.8    | 25.6     | 0.6             | 298.4    | 4.8             | 2.34          | ...                  | LP  | T   | ...   | 1FGL J1256.2–0547<br>0FGL J1256.1–0547<br>3EG J1255–0549<br>EGR J1256–0552<br>1AGL J1256–0549 | P   | BZQ   | 3C 279                | 15   |
| J1256.5–1145  | 194.139 | –11.753 | 304.928 | 51.099 | 0.083      | 0.076      | –21    | 8.4      | 0.9      | 0.2             | 10.4     | 1.7             | 2.03          | 0.13                 | PL  | ... | ...   | 1FGL J1256.5–1148                                                                             | ... | agn   | PMN J1256–1146        | ...  |
| J1257.0+3650  | 194.252 | 36.839  | 116.358 | 80.218 | 0.107      | 0.086      | –71    | 9.2      | 0.8      | 0.1             | 9.0      | 1.5             | 2.01          | 0.11                 | PL  | T   | ...   | 1FGL J1256.9+3650                                                                             | ... | bzb   | 1RXS J125716.0+364713 | ...  |
| J1258.2+3231  | 194.563 | 32.523  | 108.031 | 84.406 | 0.197      | 0.159      | –34    | 6.0      | 0.4      | 0.1             | 7.1      | 1.3             | 2.55          | 0.15                 | PL  | T   | ...   | 1FGL J1258.3+3227                                                                             | ... | bzq   | ON 393                | ...  |
| J1258.4–1801  | 194.608 | –18.032 | 305.276 | 44.808 | 0.103      | 0.087      | 47     | 9.6      | 0.8      | 0.1             | 13.2     | 1.5             | 2.54          | 0.11                 | PL  | T   | ...   | 1FGL J1258.4–1802                                                                             | ... | bzq   | PKS B1256–177         | ...  |
| J1258.8–2223  | 194.718 | –22.384 | 305.192 | 40.455 | 0.079      | 0.075      | 4      | 14.6     | 2.0      | 0.2             | 24.5     | 2.2             | 2.30          | 0.07                 | PL  | T   | ...   | 1FGL J1258.7–2221<br>EGR J1259–2209                                                           | ... | bzq   | PKS 1256–220          | ...  |
| J1259.8–3749  | 194.968 | –37.831 | 304.770 | 25.011 | 0.127      | 0.088      | –25    | 5.5      | 0.6      | 0.1             | 7.4      | 1.8             | 1.91          | 0.17                 | PL  | ... | ...   | 1FGL J1300.9–3745                                                                             | ... | ...   | ...                   | ...  |
| J1301.5+0835  | 195.391 | 8.584   | 310.762 | 71.302 | 0.103      | 0.089      | –81    | 7.8      | 0.8      | 0.1             | 8.4      | 1.5             | 2.08          | 0.12                 | PL  | ... | ...   | 1FGL J1301.8+0837                                                                             | ... | psr   | PSR J1301+08          | ...  |
| J1301.6+3331  | 195.423 | 33.523  | 104.479 | 83.234 | 0.148      | 0.118      | 1      | 6.5      | 0.6      | 0.1             | 6.4      | 1.2             | 2.18          | 0.17                 | PL  | T   | ...   | ...                                                                                           | ... | agu   | 5C 12.170             | ...  |
| J1302.4–3257  | 195.603 | –32.954 | 305.587 | 29.861 | 0.088      | 0.080      | –39    | 15.3     | 2.3      | 0.2             | 16.9     | 1.9             | 2.13          | ...                  | LP  | ... | ...   | 1FGL J1302.3–3255                                                                             | ... | psr   | PSR J1302–32          | ...  |
| J1303.1+2435  | 195.776 | 24.598  | 349.624 | 86.354 | 0.049      | 0.046      | –83    | 26.3     | 3.0      | 0.2             | 24.0     | 2.0             | 2.11          | ...                  | LP  | T   | ...   | 1FGL J1303.0+2433                                                                             | ... | bzb   | MG2 J130304+2434      | ...  |
| J1303.5–4622  | 195.883 | –46.375 | 305.107 | 16.446 | 0.194      | 0.127      | 38     | 4.8      | 0.7      | 0.2             | 7.6      | 1.6             | 2.21          | 0.14                 | PL  | ... | ...   | 1FGL J1304.0–4622                                                                             | ... | bzq   | PMN J1303–4621        | ...  |
| J1303.7–6316c | 195.943 | –63.268 | 304.319 | –0.430 | 0.105      | 0.082      | 68     | 5.8      | 2.5      | 0.5             | 27.4     | 5.2             | 2.10          | 0.13                 | PL  | ... | 6     | ...                                                                                           | E   | ...   | ...                   | ...  |
| J1303.8–5537  | 195.965 | –55.623 | 304.699 | 7.206  | 0.170      | 0.145      | 56     | 9.6      | 1.2      | 0.2             | 21.1     | 2.3             | 2.65          | 0.09                 | PL  | ... | ...   | ...                                                                                           | ... | agu   | PMN J1303–5540        | ...  |
| J1304.1–2415  | 196.032 | –24.264 | 306.630 | 38.517 | 0.097      | 0.085      | 16     | 6.8      | 0.8      | 0.2             | 9.7      | 2.1             | 1.86          | 0.13                 | PL  | ... | ...   | ...                                                                                           | ... | agu   | 1RXS J130343.6–241506 | ...  |



Table 1—Continued

| Name 2FGL     | R.A.    | Decl.   | $l$     | $b$    | $\theta_1$ | $\theta_2$ | $\phi$ | $\sigma$ | $F_{35}$ | $\Delta F_{35}$ | $S_{25}$ | $\Delta S_{25}$ | $\Gamma_{25}$ | $\Delta \Gamma_{25}$ | Mod | Var | Flags     | $\gamma$ -ray Assoc.                                     | TeV | Class | ID or Assoc.          | Ref. |     |
|---------------|---------|---------|---------|--------|------------|------------|--------|----------|----------|-----------------|----------|-----------------|---------------|----------------------|-----|-----|-----------|----------------------------------------------------------|-----|-------|-----------------------|------|-----|
| J1304.3–4353  | 196.096 | −43.896 | 305.397 | 18.914 | 0.039      | 0.037      | −55    | 23.1     | 3.7      | 0.3             | 43.2     | 3.6             | 1.90          | 0.05                 | PL  | T   | ...       | 1FGL J1304.3–4352<br>3EG J1300–4406                      | ... | agu   | 1RXS J130421.2–435308 | ...  |     |
| J1305.0+1152  | 196.272 | 11.870  | 315.451 | 74.409 | 0.197      | 0.173      | 55     | 5.0      | 0.5      | 0.1             | 6.3      | 1.3             | 2.21          | 0.15                 | PL  | ... | ...       | ...                                                      | ... | ...   | ...                   | ...  |     |
| J1305.1–2110  | 196.300 | −21.175 | 307.223 | 41.582 | 0.096      | 0.086      | −61    | 5.2      | 0.6      | 0.1             | 7.0      | 1.6             | 2.20          | 0.17                 | PL  | ... | 1         | ...                                                      | ... | agu   | PKS B1302–208         | ...  |     |
| J1305.7+7854  | 196.426 | 78.916  | 122.060 | 38.189 | 0.173      | 0.124      | −9     | 4.8      | 0.3      | 0.1             | 4.3      | 1.0             | 2.35          | 0.20                 | PL  | ... | ...       | 1FGL J1306.0+7852                                        | ... | bzb   | S5 1304+79            | ...  |     |
| J1305.8–4925  | 196.461 | −49.427 | 305.339 | 13.377 | 0.184      | 0.118      | −17    | 4.7      | 0.8      | 0.2             | 8.4      | 1.9             | 2.10          | 0.15                 | PL  | ... | 4         | 1FGL J1305.4–4928                                        | ... | sbg   | NGC 4945              | ...  |     |
| J1306.2–6044  | 196.567 | −60.740 | 304.745 | 2.079  | 0.057      | 0.055      | −0     | 15.5     | 5.5      | 0.5             | 38.3     | 3.6             | 2.16          | ...                  | LP  | ... | ...       | 1FGL J1306.4–6038<br>3EG J1308–6112                      | ... | ...   | ...                   | ...  |     |
| J1306.9–4028  | 196.745 | −40.471 | 306.127 | 22.305 | 0.173      | 0.127      | 7      | 5.0      | 0.7      | 0.2             | 8.3      | 1.6             | 2.33          | 0.13                 | PL  | ... | 3         | 1FGL J1307.0–4030                                        | ... | sey   | ESO 323–77            | ...  |     |
| J1307.5–4300  | 196.899 | −43.007 | 306.070 | 19.766 | 0.048      | 0.042      | −82    | 14.9     | 2.0      | 0.2             | 24.9     | 3.3             | 1.77          | 0.08                 | PL  | ... | ...       | 1FGL J1307.6–4259                                        | ... | agu   | 1RXS J130737.8–425940 | ...  |     |
| J1307.6–6704  | 196.901 | −67.076 | 304.510 | −4.254 | 0.096      | 0.078      | −33    | 11.5     | 2.1      | 0.3             | 28.7     | 2.8             | 2.45          | 0.07                 | PL  | T   | ...       | 1FGL J1307.3–6701                                        | ... | agu   | PKS 1304–668          | ...  |     |
| J1308.5+3547  | 197.125 | 35.793  | 101.240 | 80.605 | 0.104      | 0.094      | −76    | 12.7     | 1.1      | 0.1             | 13.1     | 1.4             | 2.28          | 0.09                 | PL  | T   | ...       | 1FGL J1308.5+3550                                        | ... | bzq   | 5C 12.291             | ...  |     |
| J1309.3+1154  | 197.338 | 11.911  | 319.243 | 74.213 | 0.147      | 0.131      | −63    | 4.4      | 0.5      | 0.1             | 5.3      | 1.5             | 1.91          | 0.19                 | PL  | ... | ...       | 1FGL J1309.2+1156                                        | ... | bzb   | 4C +12.46             | ...  |     |
| J1309.4+4304  | 197.367 | 43.078  | 111.174 | 73.636 | 0.043      | 0.041      | −89    | 19.0     | 1.8      | 0.2             | 21.4     | 2.5             | 1.84          | 0.07                 | PL  | ... | ...       | 1FGL J1309.5+4304                                        | ... | bzb   | B3 1307+433           | ...  |     |
| J1309.6–6230c | 197.412 | −62.513 | 305.032 | 0.285  | 0.192      | 0.127      | −7     | 6.1      | 3.1      | 0.5             | 35.6     | 5.7             | 2.22          | 0.09                 | PL  | ... | 3,4,5,6,9 | 1FGL J1309.9–6229c                                       | ... | ...   | ...                   |      | ... |
| J1310.6+3222  | 197.674 | 32.381  | 85.593  | 83.289 | 0.039      | 0.036      | 43     | 46.0     | 5.3      | 0.3             | 52.4     | 2.6             | 2.22          | ...                  | LP  | T   | ...       | 1FGL J1310.6+3222<br>0FGL J1310.6+3220                   | ... | bzq   | OP 313 $\gamma$       | ...  |     |
| J1310.9+0036  | 197.740 | 0.607   | 313.759 | 63.068 | 0.110      | 0.096      | −77    | 4.6      | 0.4      | 0.2             | 6.1      | 2.3             | 1.52          | 0.33                 | PL  | ... | ...       | ...                                                      | ... | bzb   | RX J1311.1+0035       | ...  |     |
| J1311.7–3429  | 197.943 | −34.489 | 307.686 | 28.195 | 0.034      | 0.033      | −56    | 43.1     | 7.7      | 0.4             | 61.7     | 2.9             | 2.19          | ...                  | LP  | ... | ...       | 1FGL J1311.7–3429<br>0FGL J1311.9–3419<br>3EG J1314–3431 | ... | ...   | ...                   | ...  |     |
| J1312.0–6458  | 198.006 | −64.973 | 305.109 | −2.188 | 0.698      | 0.313      | −89    | 4.5      | 1.1      | 0.3             | 17.2     | 3.5             | 2.55          | 0.13                 | PL  | ... | 4,8,9     | ...                                                      | ... | ...   | ...                   | ...  |     |
| J1312.4–2157  | 198.123 | −21.954 | 309.372 | 40.654 | 0.061      | 0.055      | 87     | 15.6     | 2.2      | 0.2             | 24.2     | 2.5             | 2.02          | 0.07                 | PL  | T   | ...       | 1FGL J1312.4–2156                                        | ... | bzb   | PKS 1309–216          | ...  |     |
| J1312.7+0051  | 198.183 | 0.854   | 314.821 | 63.233 | 0.063      | 0.062      | 14     | 14.4     | 2.5      | 0.3             | 13.5     | 1.6             | 2.00          | ...                  | LP  | ... | ...       | 1FGL J1312.6+0048                                        | ... | psr   | PSR J1312+00          | ...  |     |
| J1312.8+4828  | 198.212 | 48.472  | 113.323 | 68.255 | 0.025      | 0.023      | −68    | 67.4     | 9.0      | 0.3             | 83.3     | 3.4             | 2.11          | ...                  | LP  | T   | ...       | 1FGL J1312.4+4827                                        | ... | bzq   | GB 1310+487           | ...  |     |
| J1312.9–2351  | 198.242 | −23.860 | 309.248 | 38.748 | 0.170      | 0.122      | 89     | 5.7      | 0.7      | 0.2             | 8.7      | 2.1             | 1.85          | 0.16                 | PL  | ... | ...       | ...                                                      | ... | ...   | ...                   | ...  |     |
| J1313.0–0425  | 198.259 | −4.423  | 313.136 | 58.020 | 0.239      | 0.156      | 56     | 4.1      | 0.4      | 0.1             | 5.5      | 1.3             | 2.37          | 0.18                 | PL  | ... | ...       | ...                                                      | ... | bzq   | PKS B1310–041         | ...  |     |
| J1314.5–5330  | 198.641 | −53.516 | 306.411 | 9.199  | 0.164      | 0.123      | 50     | 9.3      | 1.6      | 0.2             | 21.7     | 2.5             | 2.43          | 0.08                 | PL  | T   | ...       | 1FGL J1314.9–5338                                        | ... | agu   | PMN J1315–5334        | ...  |     |
| J1314.6+2348  | 198.655 | 23.807  | 1.799   | 83.803 | 0.077      | 0.068      | −88    | 15.0     | 1.4      | 0.2             | 16.1     | 1.7             | 2.08          | 0.08                 | PL  | ... | ...       | 1FGL J1314.7+2346                                        | ... | bzb   | TXS 1312+240          | ...  |     |
| J1315.6–0730  | 198.915 | −7.510  | 313.404 | 54.869 | 0.108      | 0.091      | −54    | 6.1      | 0.6      | 0.1             | 7.2      | 1.7             | 1.92          | 0.17                 | PL  | T   | 11        | 1FGL J1315.6–0729                                        | ... | ...   | ...                   | ...  |     |
| J1315.9–3339  | 198.992 | −33.663 | 308.763 | 28.931 | 0.070      | 0.063      | −66    | 17.7     | 2.6      | 0.2             | 31.3     | 2.3             | 2.31          | 0.06                 | PL  | T   | ...       | 1FGL J1316.1–3341                                        | ... | bzq   | PKS 1313–333          | ...  |     |
| J1317.2–6304  | 199.310 | −63.078 | 305.848 | −0.352 | 0.127      | 0.098      | −56    | 11.6     | 5.4      | 0.6             | 45.3     | 4.6             | 2.30          | ...                  | LP  | ... | 2         | ...                                                      | ... | ...   | ...                   | ...  |     |
| J1317.9+3426  | 199.497 | 34.435  | 86.616  | 80.737 | 0.173      | 0.159      | −79    | 4.2      | 0.3      | 0.1             | 4.3      | 1.0             | 2.38          | 0.18                 | PL  | T   | ...       | 1FGL J1317.8+3425                                        | ... | bzq   | S4 1315+34            | ...  |     |
| J1318.9–1228  | 199.745 | −12.476 | 313.389 | 49.835 | 0.147      | 0.134      | 38     | 4.8      | 0.5      | 0.1             | 6.1      | 1.4             | 2.30          | 0.20                 | PL  | ... | ...       | ...                                                      | ... | agu   | PMN J1318–1235        | ...  |     |
| J1320.1–5756  | 200.048 | −57.942 | 306.754 | 4.716  | 0.115      | 0.105      | −84    | 5.6      | 0.9      | 0.2             | 14.5     | 2.5             | 2.56          | 0.13                 | PL  | ... | 1,4       | ...                                                      | ... | ...   | ...                   | ...  |     |

Table 1—Continued

| Name 2FGL     | R.A.    | Decl.   | $l$     | $b$    | $\theta_1$ | $\theta_2$ | $\phi$ | $\sigma$ | $F_{35}$ | $\Delta F_{35}$ | $S_{25}$ | $\Delta S_{25}$ | $\Gamma_{25}$ | $\Delta \Gamma_{25}$ | Mod | Var | Flags | $\gamma$ -ray Assoc. | TeV | Class | ID or Assoc.          | Ref. |
|---------------|---------|---------|---------|--------|------------|------------|--------|----------|----------|-----------------|----------|-----------------|---------------|----------------------|-----|-----|-------|----------------------|-----|-------|-----------------------|------|
| J1321.1+2215  | 200.298 | 22.253  | 358.732 | 81.670 | 0.110      | 0.096      | −31    | 12.7     | 1.3      | 0.2             | 15.3     | 1.6             | 2.29          | 0.08                 | PL  | T   | ...   | 1FGL J1321.1+2214    | ... | bzq   | TXS 1318+225          | ...  |
| J1322.6+8313  | 200.666 | 83.227  | 121.827 | 33.834 | 0.128      | 0.101      | 32     | 5.6      | 0.4      | 0.1             | 6.1      | 1.1             | 2.59          | 0.16                 | PL  | T   | 4     | 1FGL J1321.3+8310    | ... | bzq   | S5 1322+83            | ...  |
| J1322.7−0938  | 200.697 | −9.636  | 315.679 | 52.458 | 0.173      | 0.140      | −84    | 5.6      | 0.5      | 0.1             | 7.8      | 1.4             | 2.62          | 0.17                 | PL  | T   | 11    | 1FGL J1322.7−0943    | ... | bzq   | PKS B1319−093         | ...  |
| J1323.0+2941  | 200.762 | 29.695  | 55.049  | 82.592 | 0.064      | 0.055      | 79     | 14.6     | 1.4      | 0.2             | 15.3     | 1.7             | 2.07          | 0.08                 | PL  | T   | ...   | 1FGL J1323.1+2942    | ... | agu   | 4C +29.48             | ...  |
| J1324.0−4330e | 201.000 | −43.500 | 309.168 | 18.977 | ...        | ...        | ...    | 16.2     | 3.8      | 0.4             | 62.1     | 4.0             | 2.58          | 0.06                 | PL  | ... | 5     | 3EG J1324−4314       | ... | RDG   | Cen A Lobes           | 16   |
| J1324.4−5411  | 201.121 | −54.196 | 307.806 | 8.363  | 0.185      | 0.180      | 21     | 4.9      | 0.9      | 0.2             | 12.2     | 2.5             | 2.39          | 0.14                 | PL  | ... | 4,5   | ...                  | ... | ...   | ...                   | ...  |
| J1325.6−4300  | 201.418 | −43.015 | 309.558 | 19.416 | 0.064      | 0.056      | 34     | 27.4     | 3.0      | 0.2             | 64.7     | 2.8             | 2.76          | 0.05                 | PL  | ... | ...   | 1FGL J1325.6−4300    | P   | RDG   | Cen A Core            | 17   |
|               |         |         |         |        |            |            |        |          |          |                 |          |                 |               |                      |     |     |       | 0FGL J1325.4−4303    |     |       |                       |      |
|               |         |         |         |        |            |            |        |          |          |                 |          |                 |               |                      |     |     |       | 3EG J1324−4314       |     |       |                       |      |
| J1326.4−4729  | 201.605 | −47.498 | 309.036 | 14.959 | 0.104      | 0.089      | −2     | 7.7      | 2.0      | 0.3             | 12.0     | 2.0             | 2.18          | ...                  | LP  | ... | ...   | ...                  | ... | glc   | Omega Cen             | ...  |
| J1326.7−5254  | 201.700 | −52.915 | 308.325 | 9.586  | 0.062      | 0.058      | −36    | 19.7     | 3.9      | 0.3             | 45.1     | 3.0             | 2.23          | 0.05                 | PL  | T   | ...   | 1FGL J1327.0−5257    | ... | bzb   | PMN J1326−5256        | ...  |
|               |         |         |         |        |            |            |        |          |          |                 |          |                 |               |                      |     |     |       | 0FGL J1326.6−5302    |     |       |                       |      |
| J1326.8+2210  | 201.716 | 22.173  | 3.228   | 80.552 | 0.076      | 0.072      | −9     | 19.8     | 1.9      | 0.2             | 26.5     | 1.7             | 2.47          | 0.06                 | PL  | T   | ...   | 1FGL J1326.6+2213    | ... | bzq   | B2 1324+22            | ...  |
| J1328.5−4728  | 202.148 | −47.471 | 309.416 | 14.932 | 0.052      | 0.048      | 87     | 9.4      | 1.0      | 0.2             | 15.7     | 3.3             | 1.57          | 0.17                 | PL  | ... | ...   | 1FGL J1328.2−4729    | ... | ...   | ...                   | ...  |
| J1329.2−5608  | 202.320 | −56.136 | 308.220 | 6.347  | 0.085      | 0.074      | −86    | 16.7     | 3.7      | 0.3             | 34.2     | 3.0             | 2.32          | ...                  | LP  | T   | ...   | 1FGL J1329.2−5605    | ... | agu   | PMN J1329−5608        | ...  |
|               |         |         |         |        |            |            |        |          |          |                 |          |                 |               |                      |     |     |       | 0FGL J1328.8−5604    |     |       |                       |      |
| J1329.3−0528  | 202.341 | −5.476  | 320.044 | 56.131 | 0.189      | 0.163      | −26    | 4.8      | 0.7      | 0.2             | 9.7      | 2.5             | 2.44          | 0.20                 | PL  | ... | ...   | ...                  | ... | agn   | 1RXS J132928.0−053132 | ...  |
| J1329.5−3448  | 202.400 | −34.802 | 311.751 | 27.415 | 0.175      | 0.151      | −74    | 4.2      | 0.4      | 0.1             | 6.0      | 1.4             | 2.43          | 0.19                 | PL  | ... | 4     | ...                  | ... | ...   | ...                   | ...  |
| J1329.7−6108  | 202.435 | −61.142 | 307.539 | 1.386  | 0.089      | 0.078      | 37     | 5.7      | 1.7      | 0.3             | 20.7     | 3.6             | 2.27          | 0.10                 | PL  | ... | 3,4   | ...                  | ... | ...   | ...                   | ...  |
| J1330.1−7002  | 202.546 | −70.046 | 306.252 | −7.424 | 0.040      | 0.038      | −9     | 34.5     | 6.4      | 0.3             | 61.7     | 2.9             | 2.28          | ...                  | LP  | T   | ...   | 1FGL J1330.7−7006    | ... | agu   | PKS 1326−697          | ...  |
| J1330.9+7001  | 202.739 | 70.032  | 118.029 | 46.719 | 0.091      | 0.082      | 5      | 7.3      | 0.5      | 0.1             | 6.2      | 1.5             | 1.76          | 0.15                 | PL  | ... | ...   | 1FGL J1331.0+6957    | ... | bzb   | NVSS J133025+700141   | ...  |
| J1332.0−0508  | 203.015 | −5.136  | 321.371 | 56.274 | 0.042      | 0.041      | 26     | 35.8     | 5.0      | 0.3             | 75.6     | 3.3             | 2.54          | ...                  | LP  | T   | ...   | 1FGL J1331.9−0506    | ... | bzq   | PKS 1329−049          | ...  |
|               |         |         |         |        |            |            |        |          |          |                 |          |                 |               |                      |     |     |       | 0FGL J1331.7−0506    |     |       |                       |      |
| J1332.5−1255  | 203.139 | −12.923 | 318.219 | 48.724 | 0.056      | 0.051      | −32    | 26.7     | 3.5      | 0.2             | 45.8     | 2.4             | 2.38          | 0.04                 | PL  | T   | ...   | 1FGL J1332.6−1255    | ... | bzq   | PMN J1332−1256        | ...  |
| J1332.7+4725  | 203.187 | 47.417  | 103.905 | 68.156 | 0.226      | 0.219      | 20     | 4.5      | 0.3      | 0.1             | 4.9      | 1.1             | 2.54          | 0.18                 | PL  | T   | ...   | 1FGL J1332.9+4728    | ... | bzq   | B3 1330+476           | ...  |
| J1332.7+2726  | 203.188 | 27.450  | 37.306  | 80.818 | 0.158      | 0.141      | 4      | 5.2      | 0.4      | 0.1             | 5.0      | 1.1             | 2.28          | 0.16                 | PL  | T   | ...   | ...                  | ... | bzq   | MG2 J133305+2725      | ...  |
| J1333.5+5058  | 203.385 | 50.968  | 107.223 | 64.857 | 0.085      | 0.082      | −58    | 15.0     | 1.0      | 0.1             | 15.1     | 1.3             | 2.48          | 0.08                 | PL  | T   | ...   | 1FGL J1333.2+5056    | ... | bzq   | CLASS J1333+5057      | ...  |
|               |         |         |         |        |            |            |        |          |          |                 |          |                 |               |                      |     |     |       | 0FGL J1333.3+5058    |     |       |                       |      |
| J1335.3−4058  | 203.843 | −40.980 | 311.803 | 21.133 | 0.141      | 0.119      | −53    | 4.6      | 0.6      | 0.2             | 7.1      | 1.7             | 2.13          | 0.18                 | PL  | ... | ...   | ...                  | ... | ...   | ...                   | ...  |
| J1335.4−5658  | 203.875 | −56.971 | 308.937 | 5.386  | 0.140      | 0.121      | −55    | 6.0      | 1.3      | 0.2             | 16.7     | 2.9             | 2.35          | 0.11                 | PL  | T   | 1     | ...                  | ... | ...   | ...                   | ...  |
| J1337.7−1257  | 204.427 | −12.955 | 320.041 | 48.374 | 0.064      | 0.062      | −22    | 14.4     | 1.8      | 0.2             | 24.4     | 2.1             | 2.44          | 0.07                 | PL  | T   | ...   | 1FGL J1337.7−1255    | ... | bzq   | PKS 1335−127          | ...  |
|               |         |         |         |        |            |            |        |          |          |                 |          |                 |               |                      |     |     |       | EGR J1337−1310       |     |       |                       |      |
| J1338.9+1152  | 204.737 | 11.883  | 341.411 | 71.113 | 0.072      | 0.068      | −12    | 9.4      | 0.9      | 0.1             | 9.8      | 1.8             | 1.93          | 0.12                 | PL  | ... | ...   | 1FGL J1338.9+1153    | ... | bzb   | BZB J1338+1153        | ...  |
| J1339.2−2348  | 204.805 | −23.813 | 316.793 | 37.769 | 0.157      | 0.123      | 38     | 5.6      | 0.6      | 0.1             | 7.3      | 1.5             | 2.31          | 0.15                 | PL  | ... | 4     | ...                  | ... | ...   | ...                   | ...  |
| J1340.5−0412  | 205.129 | −4.208  | 325.512 | 56.497 | 0.144      | 0.132      | −62    | 4.3      | 0.4      | 0.1             | 4.8      | 1.4             | 1.95          | 0.21                 | PL  | ... | ...   | 1FGL J1340.5−0413    | ... | ...   | ...                   | ...  |

Table 1—Continued

| Name 2FGL     | R.A.    | Decl.   | $l$     | $b$    | $\theta_1$ | $\theta_2$ | $\phi$ | $\sigma$ | $F_{35}$ | $\Delta F_{35}$ | $S_{25}$ | $\Delta S_{25}$ | $\Gamma_{25}$ | $\Delta \Gamma_{25}$ | Mod | Var | Flags | $\gamma$ -ray Assoc. | TeV | Class | ID or Assoc.           | Ref. |
|---------------|---------|---------|---------|--------|------------|------------|--------|----------|----------|-----------------|----------|-----------------|---------------|----------------------|-----|-----|-------|----------------------|-----|-------|------------------------|------|
| J1340.5+4407  | 205.132 | 44.124  | 95.956  | 70.343 | 0.126      | 0.109      | 81     | 4.9      | 0.4      | 0.1             | 4.7      | 1.4             | 1.80          | 0.24                 | PL  | ... | ...   | 1FGL J1340.6+4406    | ... | bzb   | RX J1340.4+4410        | ...  |
| J1341.3–2048  | 205.334 | –20.802 | 318.348 | 40.571 | 0.198      | 0.179      | –55    | 5.8      | 0.5      | 0.1             | 8.9      | 1.5             | 2.63          | 0.13                 | PL  | T   | ...   | 1FGL J1341.1–2045    | ... | bzq   | PKS B1339–206          | ...  |
| J1344.2–1723  | 206.068 | –17.396 | 320.477 | 43.669 | 0.042      | 0.039      | –85    | 30.8     | 5.0      | 0.3             | 41.6     | 2.6             | 2.13          | ...                  | LP  | T   | ...   | 1FGL J1344.2–1723    | ... | bzq   | PMN J1344–1723         | ...  |
| J1345.4+4453  | 206.371 | 44.897  | 95.147  | 69.204 | 0.060      | 0.058      | 6      | 23.3     | 2.1      | 0.2             | 30.1     | 1.6             | 2.47          | 0.05                 | PL  | T   | ...   | 1FGL J1345.4+4453    | ... | bzq   | B3 1343+451            | ...  |
| J1345.8–3356  | 206.460 | –33.941 | 315.648 | 27.584 | 0.177      | 0.115      | –62    | 5.4      | 0.6      | 0.1             | 7.2      | 1.4             | 2.29          | 0.18                 | PL  | ... | 1     | ...                  | ... | ...   | ...                    | ...  |
| J1345.9+0706  | 206.490 | 7.100   | 338.278 | 66.156 | 0.102      | 0.099      | 4      | 6.3      | 0.6      | 0.1             | 7.1      | 1.4             | 2.13          | 0.14                 | PL  | T   | ...   | 1FGL J1346.0+0703    | ... | bzq   | TXS 1343+073           | ...  |
| J1346.0–2605  | 206.505 | –26.094 | 317.956 | 35.181 | 0.185      | 0.127      | –74    | 5.0      | 0.6      | 0.1             | 6.7      | 1.4             | 2.24          | 0.15                 | PL  | ... | ...   | ...                  | ... | ...   | ...                    | ...  |
| J1346.6–6027  | 206.663 | –60.466 | 309.690 | 1.679  | 0.119      | 0.090      | 55     | 5.4      | 1.9      | 0.3             | 23.0     | 4.3             | 2.33          | 0.12                 | PL  | ... | 1,4   | ...                  | ... | rdg   | Cen B                  | ...  |
| J1347.0–2956  | 206.759 | –29.945 | 317.047 | 31.398 | 0.110      | 0.105      | 41     | 5.0      | 0.4      | 0.1             | 7.5      | 2.8             | 1.36          | 0.30                 | PL  | ... | ...   | ...                  | ... | ...   | ...                    | ...  |
| J1347.7–3752  | 206.927 | –37.883 | 315.023 | 23.664 | 0.091      | 0.084      | 7      | 8.0      | 0.9      | 0.2             | 11.1     | 1.6             | 2.32          | 0.12                 | PL  | T   | ...   | 1FGL J1347.8–3751    | ... | bzq   | PMN J1347–3750         | ...  |
| J1349.9–6222  | 207.481 | –62.381 | 309.653 | –0.275 | 0.072      | 0.068      | –58    | 11.4     | 6.6      | 0.7             | 54.5     | 5.8             | 2.24          | ...                  | LP  | ... | 2     | ...                  | ... | ...   | ...                    | ...  |
| J1350.8+3035  | 207.713 | 30.589  | 51.347  | 76.550 | 0.143      | 0.127      | –51    | 8.8      | 0.6      | 0.1             | 8.8      | 1.2             | 2.45          | 0.11                 | PL  | T   | ...   | 1FGL J1351.0+3035    | ... | bzq   | B2 1348+30B            | ...  |
| J1351.1+0032  | 207.784 | 0.543   | 333.725 | 59.797 | 0.156      | 0.108      | 1      | 8.2      | 0.8      | 0.1             | 9.6      | 1.4             | 2.29          | 0.11                 | PL  | T   | ...   | ...                  | ... | bzq   | PKS 1348+007           | ...  |
| J1351.1–2749  | 207.787 | –27.833 | 318.730 | 33.200 | 0.176      | 0.143      | 17     | 4.4      | 0.5      | 0.1             | 6.4      | 1.5             | 2.38          | 0.17                 | PL  | T   | 4     | ...                  | ... | ...   | ...                    | ...  |
| J1351.3–2909  | 207.846 | –29.158 | 318.361 | 31.911 | 0.119      | 0.109      | 54     | 6.0      | 0.7      | 0.1             | 8.5      | 1.6             | 2.32          | 0.13                 | PL  | T   | ...   | ...                  | ... | agu   | PKS 1348–289           | ...  |
| J1351.4+1115  | 207.867 | 11.256  | 347.454 | 68.765 | 0.073      | 0.068      | –79    | 7.2      | 0.4      | 0.1             | 7.6      | 2.4             | 1.46          | 0.19                 | PL  | ... | ...   | 1FGL J1351.5+1115    | ... | bzb   | RX J1351.5+1115        | ...  |
| J1352.6–4413  | 208.171 | –44.230 | 314.362 | 17.278 | 0.119      | 0.107      | 74     | 5.3      | 0.6      | 0.1             | 7.2      | 1.6             | 2.13          | 0.17                 | PL  | ... | ...   | ...                  | ... | bzb   | PKS 1349–439           | ...  |
| J1353.3+1435  | 208.328 | 14.598  | 355.028 | 70.906 | 0.106      | 0.102      | –58    | 6.0      | 0.5      | 0.1             | 6.3      | 1.2             | 2.26          | 0.17                 | PL  | ... | ...   | 1FGL J1353.3+1434    | ... | bzb   | OP 186                 | ...  |
| J1353.5–6640  | 208.382 | –66.681 | 309.033 | –4.548 | 0.067      | 0.060      | 57     | 7.0      | 0.9      | 0.2             | 11.7     | 2.5             | 1.80          | 0.17                 | PL  | ... | ...   | 1FGL J1353.6–6640    | ... | ...   | ...                    | ...  |
| J1354.5+3703  | 208.642 | 37.051  | 73.531  | 73.388 | 0.180      | 0.155      | –66    | 6.1      | 0.5      | 0.1             | 6.0      | 1.2             | 2.14          | 0.15                 | PL  | ... | ...   | ...                  | ... | bzb   | FIRST J135426.6+370654 | ...  |
| J1354.7–1047  | 208.695 | –10.791 | 327.093 | 49.086 | 0.140      | 0.109      | 39     | 14.6     | 1.3      | 0.2             | 20.1     | 1.6             | 2.57          | 0.08                 | PL  | T   | ...   | 1FGL J1354.9–1041    | ... | bzq   | PKS 1352–104           | ...  |
|               |         |         |         |        |            |            |        |          |          |                 |          |                 |               |                      |     |     |       | 0FGL J1355.0–1044    |     |       |                        |      |
| J1356.0–6436  | 209.019 | –64.612 | 309.793 | –2.605 | 0.116      | 0.095      | –16    | 11.8     | 2.5      | 0.4             | 33.8     | 3.5             | 2.52          | ...                  | EC  | ... | ...   | ...                  | E   | PSR   | PSR J1357–6429         | ...  |
| J1358.0+0137  | 209.515 | 1.617   | 337.775 | 59.903 | 0.263      | 0.206      | –76    | 4.6      | 0.5      | 0.1             | 6.0      | 1.3             | 2.28          | 0.16                 | PL  | ... | ...   | ...                  | ... | bzb   | RX J1357.6+0128        | ...  |
| J1358.1+7644  | 209.532 | 76.746  | 118.025 | 39.740 | 0.098      | 0.093      | –74    | 11.0     | 0.8      | 0.1             | 10.1     | 1.1             | 2.30          | 0.10                 | PL  | T   | ...   | 1FGL J1358.1+7646    | ... | bzq   | S5 1357+76             | ...  |
| J1358.8–6027c | 209.713 | –60.457 | 311.154 | 1.334  | 0.108      | 0.084      | –64    | 5.5      | 2.3      | 0.4             | 27.6     | 5.1             | 2.27          | 0.10                 | PL  | ... | 2,4,6 | ...                  | ... | ...   | ...                    | ...  |
| J1359.4+5541  | 209.852 | 55.689  | 104.324 | 58.916 | 0.154      | 0.129      | –20    | 10.8     | 0.5      | 0.1             | 10.5     | 1.1             | 2.70          | 0.11                 | PL  | T   | ...   | 1FGL J1359.1+5539    | ... | bzq   | 87GB 135720.6+555936   | ...  |
| J1359.9–3746  | 209.987 | –37.777 | 317.595 | 23.136 | 0.089      | 0.067      | 16     | 6.4      | 0.6      | 0.2             | 8.7      | 2.4             | 1.63          | 0.17                 | PL  | ... | ...   | 1FGL J1400.1–3743    | ... | bzb   | PMN J1359–3746         | ...  |
| J1400.2–2412  | 210.075 | –24.211 | 322.433 | 36.039 | 0.164      | 0.115      | –28    | 4.3      | 0.5      | 0.1             | 5.5      | 1.5             | 2.01          | 0.16                 | PL  | ... | ...   | ...                  | ... | ...   | ...                    | ...  |
| J1400.6–5601  | 210.170 | –56.020 | 312.551 | 5.553  | 0.117      | 0.100      | 12     | 9.2      | 1.9      | 0.3             | 15.0     | 2.3             | 2.36          | ...                  | LP  | T   | ...   | 1FGL J1400.9–5559    | ... | agu   | PMN J1400–5605         | ...  |
| J1400.7–1438  | 210.185 | –14.649 | 326.962 | 44.964 | 0.155      | 0.134      | 82     | 5.6      | 0.7      | 0.1             | 8.3      | 1.5             | 2.33          | 0.14                 | PL  | ... | ...   | ...                  | ... | ...   | ...                    | ...  |
| J1404.0–5244  | 211.014 | –52.739 | 313.931 | 8.575  | 0.172      | 0.156      | 19     | 4.3      | 0.9      | 0.2             | 10.1     | 2.2             | 2.24          | 0.13                 | PL  | ... | ...   | ...                  | ... | ...   | ...                    | ...  |
| J1405.1+0405  | 211.296 | 4.084   | 343.529 | 61.002 | 0.205      | 0.186      | 32     | 4.5      | 0.5      | 0.1             | 5.9      | 1.6             | 1.90          | 0.17                 | PL  | ... | ...   | ...                  | ... | bzq   | PKS 1402+044           | ...  |
| J1405.5–6121  | 211.375 | –61.364 | 311.686 | 0.242  | 0.057      | 0.047      | –37    | 15.8     | 12.9     | 0.9             | 105.9    | 8.7             | 2.24          | ...                  | LP  | ... | 2     | 1FGL J1405.1–6123c   | ... | ...   | ...                    | ...  |
| J1406.2–2510  | 211.557 | –25.170 | 323.593 | 34.683 | 0.068      | 0.064      | –87    | 7.7      | 0.7      | 0.1             | 10.1     | 2.5             | 1.63          | 0.16                 | PL  | ... | ...   | 1FGL J1406.2–2510    | ... | agu   | NVSS J140609–250808    | ...  |

Table 1—Continued

| Name 2FGL     | R.A.    | Decl.   | $l$     | $b$    | $\theta_1$ | $\theta_2$ | $\phi$ | $\sigma$ | $F_{35}$ | $\Delta F_{35}$ | $S_{25}$ | $\Delta S_{25}$ | $\Gamma_{25}$ | $\Delta \Gamma_{25}$ | Mod | Var | Flags | $\gamma$ -ray Assoc. | TeV | Class | ID or Assoc.          | Ref. |
|---------------|---------|---------|---------|--------|------------|------------|--------|----------|----------|-----------------|----------|-----------------|---------------|----------------------|-----|-----|-------|----------------------|-----|-------|-----------------------|------|
| J1407.4–2948  | 211.857 | –29.816 | 322.011 | 30.224 | 0.352      | 0.235      | –4     | 5.3      | 0.5      | 0.1             | 7.8      | 1.4             | 2.51          | 0.13                 | PL  | ... | 2     | 1FGL J1407.9–2928    | ... | ...   | ...                   | ...  |
| J1407.5–4257  | 211.884 | –42.966 | 317.437 | 17.752 | 0.092      | 0.083      | 77     | 5.8      | 0.7      | 0.2             | 8.2      | 1.9             | 1.91          | 0.14                 | PL  | ... | ...   | 1FGL J1407.5–4256    | ... | agu   | CGRaBS J1407–4302     | ...  |
| J1407.6–5937c | 211.915 | –59.627 | 312.439 | 1.830  | 0.187      | 0.109      | 29     | 4.8      | 1.7      | 0.4             | 20.7     | 4.3             | 2.27          | 0.13                 | PL  | ... | 4,6   | ...                  | ... | ...   | ...                   | ...  |
| J1408.8–0751  | 212.208 | –7.866  | 333.851 | 50.301 | 0.077      | 0.069      | –79    | 17.5     | 1.7      | 0.2             | 23.7     | 1.7             | 2.43          | 0.06                 | PL  | T   | ...   | 1FGL J1408.9–0751    | ... | bzq   | PKS B1406–076         | ...  |
|               |         |         |         |        |            |            |        |          |          |                 |          |                 |               |                      |     |     |       | 3EG J1409–0745       |     |       |                       |      |
| J1409.9–6129  | 212.497 | –61.494 | 312.162 | –0.038 | 0.098      | 0.062      | 79     | 7.4      | 5.7      | 0.9             | 54.1     | 10.9            | 2.11          | ...                  | EC  | ... | 2,4,5 | 1FGL J1410.3–6128c   | ... | PSR   | PSR J1410–6132        | ...  |
|               |         |         |         |        |            |            |        |          |          |                 |          |                 |               |                      |     |     |       | 3EG J1410–6147       |     |       |                       |      |
|               |         |         |         |        |            |            |        |          |          |                 |          |                 |               |                      |     |     |       | 1AGL J1412–6149      |     |       |                       |      |
| J1410.3+2811  | 212.600 | 28.199  | 41.021  | 72.502 | 0.150      | 0.122      | –2     | 4.6      | 0.3      | 0.1             | 5.6      | 2.0             | 1.52          | 0.23                 | PL  | ... | ...   | ...                  | ... | bzb   | BZB J1410+2820        | ...  |
| J1410.4+7411  | 212.607 | 74.198  | 115.839 | 41.825 | 0.078      | 0.069      | –52    | 9.1      | 0.6      | 0.1             | 7.4      | 1.3             | 1.93          | 0.15                 | PL  | ... | ...   | ...                  | ... | ...   | ...                   | ...  |
| J1411.9–5744  | 212.992 | –57.742 | 313.537 | 3.462  | 0.116      | 0.116      | –29    | 4.9      | 1.2      | 0.3             | 14.9     | 3.1             | 2.33          | 0.13                 | PL  | ... | 4     | ...                  | ... | †     | ...                   | ...  |
| J1413.4–6204  | 213.359 | –62.075 | 312.372 | –0.716 | 0.025      | 0.023      | 4      | 34.7     | 25.5     | 1.0             | 164.4    | 7.7             | 2.11          | ...                  | EC  | ... | ...   | 1FGL J1413.4–6205    | ... | PSR   | LAT PSR J1413–6205    | ...  |
|               |         |         |         |        |            |            |        |          |          |                 |          |                 |               |                      |     |     |       | 0FGL J1413.1–6203    |     |       |                       |      |
|               |         |         |         |        |            |            |        |          |          |                 |          |                 |               |                      |     |     |       | EGRc J1414–6224      |     |       |                       |      |
|               |         |         |         |        |            |            |        |          |          |                 |          |                 |               |                      |     |     |       | 1AGL J1412–6149      |     |       |                       |      |
| J1414.1–5450  | 213.540 | –54.835 | 314.736 | 6.130  | 0.199      | 0.165      | 17     | 5.3      | 0.9      | 0.2             | 14.1     | 2.5             | 2.53          | 0.12                 | PL  | ... | 4,8   | ...                  | ... | ...   | ...                   | ...  |
| J1415.7–6520  | 213.929 | –65.338 | 311.580 | –3.891 | 0.128      | 0.106      | 32     | 4.5      | 1.0      | 0.2             | 12.0     | 2.8             | 2.27          | 0.15                 | PL  | ... | 4     | ...                  | ... | ...   | ...                   | ...  |
| J1416.0+1323  | 214.006 | 13.387  | 2.319   | 65.934 | 0.183      | 0.136      | –82    | 5.8      | 0.4      | 0.1             | 7.2      | 1.3             | 2.60          | 0.15                 | PL  | T   | ...   | ...                  | ... | agu   | PKS B1413+135         | ...  |
| J1416.3–2415  | 214.090 | –24.256 | 326.604 | 34.682 | 0.131      | 0.109      | 9      | 4.4      | 0.3      | 0.1             | 5.3      | 2.1             | 1.43          | 0.28                 | PL  | ... | ...   | ...                  | ... | agu   | NVSS J141612–241812   | ...  |
| J1417.5–4404  | 214.376 | –44.079 | 318.850 | 16.116 | 0.144      | 0.112      | –15    | 6.6      | 0.8      | 0.2             | 10.9     | 1.8             | 2.39          | 0.13                 | PL  | ... | ...   | 1FGL J1417.7–4407    | ... | ...   | ...                   | ...  |
| J1417.7–5028  | 214.430 | –50.470 | 316.681 | 10.084 | 0.202      | 0.125      | –0     | 5.0      | 0.9      | 0.2             | 10.1     | 2.1             | 2.25          | 0.13                 | PL  | ... | ...   | 1FGL J1417.7–5030    | ... | ...   | ...                   | ...  |
| J1418.1+2539  | 214.534 | 25.655  | 33.507  | 70.552 | 0.202      | 0.140      | –90    | 4.6      | 0.4      | 0.1             | 5.0      | 1.3             | 1.98          | 0.19                 | PL  | ... | ...   | 1FGL J1417.8+2541    | ... | bzb   | BZB J1417+2543        | ...  |
| J1418.4–0234  | 214.603 | –2.574  | 341.563 | 53.644 | 0.046      | 0.041      | 40     | 18.8     | 2.2      | 0.2             | 29.2     | 3.7             | 1.70          | 0.07                 | PL  | T   | ...   | 1FGL J1418.3–0235    | ... | bzb   | BZB J1418–0233        | ...  |
| J1418.7–6058  | 214.691 | –60.978 | 313.326 | 0.119  | 0.020      | 0.020      | 86     | 27.8     | 43.1     | 2.0             | 316.9    | 17.2            | 2.20          | ...                  | EC  | ... | 2     | 1FGL J1418.7–6057    | E   | PSR   | LAT PSR J1418–6058    | ...  |
|               |         |         |         |        |            |            |        |          |          |                 |          |                 |               |                      |     |     |       | 0FGL J1418.8–6058    |     |       |                       |      |
|               |         |         |         |        |            |            |        |          |          |                 |          |                 |               |                      |     |     |       | 1AGL J1419–6055      |     |       |                       |      |
| J1419.4+3820  | 214.857 | 38.344  | 69.829  | 68.448 | 0.186      | 0.163      | 74     | 7.8      | 0.5      | 0.1             | 8.2      | 1.2             | 2.65          | 0.14                 | PL  | ... | ...   | ...                  | ... | bzq   | B3 1417+385           | ...  |
| J1419.4–0835  | 214.866 | –8.596  | 336.848 | 48.393 | 0.132      | 0.119      | –83    | 7.0      | 0.7      | 0.1             | 8.4      | 1.5             | 2.17          | 0.12                 | PL  | T   | ...   | ...                  | ... | agu   | NVSS J141922–083830   | ...  |
| J1419.4+7730  | 214.870 | 77.511  | 116.981 | 38.581 | 0.106      | 0.089      | –11    | 5.1      | 0.3      | 0.1             | 3.8      | 1.2             | 1.78          | 0.24                 | PL  | ... | ...   | 1FGL J1419.7+7731    | ... | agu   | 1RXS J141901.8+773229 | ...  |
| J1420.1–6047  | 215.027 | –60.797 | 313.541 | 0.235  | 0.038      | 0.037      | 42     | 12.1     | 18.9     | 1.8             | 145.9    | 16.6            | 2.26          | ...                  | EC  | ... | 5     | 1FGL J1420.1–6048    | E   | PSR   | PSR J1420–6048        | ...  |
|               |         |         |         |        |            |            |        |          |          |                 |          |                 |               |                      |     |     |       | 3EG J1420–6038       |     |       |                       |      |
|               |         |         |         |        |            |            |        |          |          |                 |          |                 |               |                      |     |     |       | EGR J1418–6040       |     |       |                       |      |
|               |         |         |         |        |            |            |        |          |          |                 |          |                 |               |                      |     |     |       | 1AGL J1419–6055      |     |       |                       |      |
| J1420.2+5422  | 215.067 | 54.376  | 98.181  | 58.275 | 0.109      | 0.091      | –63    | 10.9     | 0.8      | 0.1             | 9.8      | 1.1             | 2.37          | 0.11                 | PL  | ... | ...   | 1FGL J1421.0+5421    | ... | bzb   | OQ 530                | ...  |
| J1421.1–1117  | 215.277 | –11.299 | 335.400 | 45.843 | 0.207      | 0.148      | 87     | 4.7      | 0.6      | 0.1             | 6.5      | 1.5             | 2.14          | 0.16                 | PL  | ... | ...   | ...                  | ... | agu   | PMN J1420–1118        | ...  |

Table 1—Continued

| Name 2FGL     | R.A.    | Decl.   | $l$     | $b$     | $\theta_1$ | $\theta_2$ | $\phi$ | $\sigma$ | $F_{35}$ | $\Delta F_{35}$ | $S_{25}$ | $\Delta S_{25}$ | $\Gamma_{25}$ | $\Delta \Gamma_{25}$ | Mod | Var | Flags  | $\gamma$ -ray Assoc.                                  | TeV | Class | ID or Assoc.       | Ref. |
|---------------|---------|---------|---------|---------|------------|------------|--------|----------|----------|-----------------|----------|-----------------|---------------|----------------------|-----|-----|--------|-------------------------------------------------------|-----|-------|--------------------|------|
| J1422.3–6841  | 215.579 | –68.696 | 311.064 | –7.272  | 0.130      | 0.113      | –56    | 7.0      | 0.9      | 0.2             | 15.0     | 2.2             | 2.58          | 0.12                 | PL  | ... | ...    | ...                                                   | ... | ...   | ...                | ...  |
| J1422.5–6137c | 215.635 | –61.623 | 313.535 | –0.641  | 0.044      | 0.040      | –35    | 12.2     | 5.9      | 0.7             | 30.4     | 3.1             | 1.92          | ...                  | LP  | ... | 3,6,12 | ...                                                   | ... | ...   | ...                | ...  |
| J1423.9–7842  | 215.982 | –78.715 | 307.533 | –16.679 | 0.159      | 0.118      | –20    | 4.9      | 0.6      | 0.1             | 7.0      | 1.7             | 2.03          | 0.14                 | PL  | T   | ...    | 1FGL J1424.5–7847                                     | ... | ...   | ...                | ...  |
| J1424.2–1752  | 216.054 | –17.880 | 332.080 | 39.683  | 0.088      | 0.072      | 54     | 6.5      | 0.7      | 0.1             | 8.1      | 1.7             | 1.97          | 0.16                 | PL  | ... | ...    | ...                                                   | ... | ...   | ...                | ...  |
| J1425.1+3615  | 216.299 | 36.265  | 63.458  | 68.140  | 0.092      | 0.077      | 44     | 10.5     | 0.9      | 0.1             | 10.4     | 1.4             | 2.14          | 0.11                 | PL  | ... | ...    | 1FGL J1425.0+3614                                     | ... | bzb   | BZB J1424+3615     | ...  |
| J1426.1+3406  | 216.543 | 34.100  | 57.660  | 68.519  | 0.105      | 0.094      | –33    | 6.1      | 0.5      | 0.1             | 5.9      | 1.6             | 1.83          | 0.18                 | PL  | ... | ...    | 1FGL J1426.0+3403                                     | ... | bzb   | BZB J1426+3404     | ...  |
| J1427.0+2347  | 216.760 | 23.795  | 29.479  | 68.199  | 0.020      | 0.019      | 89     | 64.1     | 11.5     | 0.4             | 144.5    | 6.8             | 1.78          | 0.02                 | PL  | T   | ...    | 1FGL J1426.9+2347<br>0FGL J1427.1+2347                | P   | bzb   | PKS 1424+240       | ...  |
| J1427.4–3306  | 216.854 | –33.104 | 325.125 | 25.598  | 0.164      | 0.128      | 31     | 9.5      | 0.9      | 0.2             | 13.6     | 1.6             | 2.48          | 0.10                 | PL  | ... | ...    | ...                                                   | ... | bzb   | PKS B1424–328      | ...  |
| J1427.6–6048c | 216.903 | –60.804 | 314.396 | –0.091  | 0.095      | 0.082      | 70     | 5.9      | 2.8      | 1.0             | 32.5     | 5.6             | 2.22          | ...                  | LP  | ... | 2,4,6  | ...                                                   | E   | ...   | ...                | ...  |
| J1428.0–4206  | 217.012 | –42.104 | 321.468 | 17.264  | 0.023      | 0.023      | 16     | 68.3     | 14.7     | 0.5             | 130.9    | 4.3             | 2.13          | ...                  | LP  | T   | ...    | 1FGL J1428.2–4204<br>3EG J1429–4217<br>EGR J1428–4240 | ... | BZQ   | PKS B1424–418      | ...  |
| J1428.6+4240  | 217.154 | 42.673  | 77.472  | 64.887  | 0.050      | 0.045      | –47    | 13.1     | 0.8      | 0.1             | 16.8     | 3.6             | 1.32          | 0.12                 | PL  | ... | ...    | 1FGL J1428.7+4239                                     | P   | bzb   | H 1426+428         | ...  |
| J1430.0–5909  | 217.511 | –59.166 | 315.280 | 1.321   | 0.039      | 0.037      | 50     | 26.5     | 11.6     | 0.6             | 94.8     | 4.9             | 2.30          | ...                  | EC  | ... | ...    | 1FGL J1429.9–5911                                     | ... | PSR   | LAT PSR J1429–5911 | ...  |
| J1433.8+4205  | 218.453 | 42.086  | 75.192  | 64.331  | 0.125      | 0.105      | –70    | 7.0      | 0.5      | 0.1             | 6.4      | 1.1             | 2.26          | 0.14                 | PL  | T   | ...    | 1FGL J1433.9+4204                                     | ... | bzq   | B3 1432+422        | ...  |
| J1435.1+2022  | 218.786 | 20.368  | 22.606  | 65.378  | 0.172      | 0.148      | 20     | 5.4      | 0.5      | 0.1             | 6.3      | 1.2             | 2.35          | 0.16                 | PL  | ... | ...    | ...                                                   | ... | bzb   | CRATES J1435+2021  | ...  |
| J1436.9+2319  | 219.233 | 23.329  | 29.750  | 65.887  | 0.141      | 0.110      | 4      | 5.2      | 0.4      | 0.1             | 5.9      | 1.3             | 2.41          | 0.18                 | PL  | ... | ...    | 1FGL J1436.9+2314                                     | ... | bzq   | PKS B1434+235      | ...  |
| J1437.1+5640  | 219.276 | 56.676  | 97.728  | 54.974  | 0.056      | 0.048      | –20    | 8.0      | 0.5      | 0.1             | 7.8      | 2.1             | 1.53          | 0.16                 | PL  | ... | ...    | 1FGL J1437.0+5640                                     | ... | bzb   | BZB J1436+5639     | ...  |
| J1437.2–5211  | 219.308 | –52.191 | 318.913 | 7.367   | 0.196      | 0.146      | –88    | 4.9      | 0.9      | 0.2             | 12.1     | 2.3             | 2.43          | 0.13                 | PL  | ... | 4      | ...                                                   | ... | ...   | ...                | ...  |
| J1438.7+3712  | 219.684 | 37.208  | 63.715  | 65.270  | 0.069      | 0.063      | –47    | 21.1     | 1.9      | 0.2             | 23.0     | 1.6             | 2.28          | 0.06                 | PL  | T   | ...    | 1FGL J1438.7+3711                                     | ... | bzq   | B2 1436+37B        | ...  |
| J1439.2+3932  | 219.802 | 39.536  | 68.841  | 64.442  | 0.147      | 0.123      | 46     | 5.5      | 0.4      | 0.1             | 5.6      | 1.7             | 1.69          | 0.17                 | PL  | ... | ...    | 1FGL J1439.2+3930                                     | ... | bzb   | PG 1437+398        | ...  |
| J1440.3–1540  | 220.076 | –15.669 | 337.851 | 39.709  | 0.175      | 0.135      | 16     | 4.1      | 0.5      | 0.1             | 6.5      | 1.5             | 2.40          | 0.16                 | PL  | ... | 11     | 1FGL J1441.7–1538                                     | ... | bzb   | PKS 1437–153       | ...  |
| J1440.3+4948  | 220.099 | 49.816  | 87.710  | 59.198  | 0.266      | 0.170      | –54    | 4.6      | 0.3      | 0.1             | 4.7      | 1.1             | 2.45          | 0.21                 | PL  | ... | ...    | ...                                                   | ... | bzb   | GB6 J1439+4958     | ...  |
| J1440.9+0611  | 220.248 | 6.189   | 359.097 | 56.593  | 0.069      | 0.057      | –86    | 10.4     | 1.1      | 0.2             | 12.2     | 1.6             | 2.16          | 0.11                 | PL  | T   | ...    | 1FGL J1440.9+0613                                     | ... | bzb   | PMN J1440+0610     | ...  |
| J1441.1–3304  | 220.282 | –33.070 | 328.008 | 24.406  | 0.249      | 0.149      | –28    | 5.4      | 0.4      | 0.1             | 8.5      | 1.5             | 2.76          | 0.17                 | PL  | T   | 4      | ...                                                   | ... | bzq   | PKS 1438–328       | ...  |
| J1441.6–5956  | 220.414 | –59.937 | 316.332 | 0.036   | 0.167      | 0.098      | –71    | 7.0      | 3.8      | 0.6             | 43.2     | 6.2             | 2.20          | 0.08                 | PL  | ... | 2,10   | 1FGL J1442.0–6000c                                    | ... | †     | ...                | ...  |
| J1442.0+4352  | 220.522 | 43.877  | 77.160  | 62.159  | 0.109      | 0.072      | –13    | 7.4      | 0.5      | 0.1             | 7.5      | 2.0             | 1.62          | 0.15                 | PL  | ... | ...    | 1FGL J1442.1+4348                                     | ... | bzb   | BZB J1442+4348     | ...  |
| J1442.7+1159  | 220.688 | 11.996  | 8.291   | 59.842  | 0.086      | 0.075      | –59    | 6.5      | 0.5      | 0.1             | 8.9      | 2.9             | 1.41          | 0.18                 | PL  | ... | ...    | 1FGL J1442.8+1158                                     | P   | bzb   | IES 1440+122       | ...  |
| J1443.9–3908  | 220.985 | –39.135 | 325.643 | 18.725  | 0.037      | 0.036      | 26     | 21.2     | 3.2      | 0.3             | 41.3     | 4.1             | 1.77          | 0.06                 | PL  | ... | ...    | 1FGL J1444.0–3906                                     | ... | bzb   | PKS 1440–389       | ...  |
| J1444.1+2500  | 221.029 | 25.015  | 34.548  | 64.661  | 0.109      | 0.093      | 73     | 9.4      | 0.9      | 0.1             | 10.2     | 1.6             | 2.03          | 0.12                 | PL  | ... | ...    | 1FGL J1443.8+2457                                     | ... | bzq   | PKS 1441+25        | ...  |
| J1446.6–5753  | 221.662 | –57.894 | 317.775 | 1.619   | 0.170      | 0.136      | –7     | 10.8     | 1.5      | 0.4             | 32.0     | 3.6             | 2.53          | ...                  | LP  | ... | 1,4    | ...                                                   | ... | ...   | ...                | ...  |
| J1446.8–4701  | 221.708 | –47.030 | 322.535 | 11.402  | 0.124      | 0.103      | 51     | 7.2      | 1.2      | 0.2             | 12.9     | 2.1             | 2.13          | 0.11                 | PL  | ... | ...    | 1FGL J1446.8–4702                                     | ... | ...   | ...                | ...  |
| J1448.0+3608  | 222.002 | 36.137  | 60.256  | 63.725  | 0.070      | 0.066      | 10     | 12.8     | 1.2      | 0.2             | 13.9     | 2.0             | 1.89          | 0.09                 | PL  | T   | ...    | 1FGL J1447.9+3608                                     | ... | bzb   | RBS 1432           | ...  |
| J1451.0+5159  | 222.751 | 51.991  | 89.097  | 56.554  | 0.089      | 0.084      | –69    | 7.1      | 0.7      | 0.1             | 8.0      | 1.5             | 2.11          | 0.13                 | PL  | ... | 5      | 1FGL J1451.0+5204                                     | ... | bzb   | BZB J1450+5201     | ...  |

Table 1—Continued

| Name 2FGL     | R.A.    | Decl.   | $l$     | $b$    | $\theta_1$ | $\theta_2$ | $\phi$ | $\sigma$ | $F_{35}$ | $\Delta F_{35}$ | $S_{25}$ | $\Delta S_{25}$ | $\Gamma_{25}$ | $\Delta \Gamma_{25}$ | Mod | Var | Flags | $\gamma$ -ray Assoc. | TeV | Class | ID or Assoc.       | Ref. |
|---------------|---------|---------|---------|--------|------------|------------|--------|----------|----------|-----------------|----------|-----------------|---------------|----------------------|-----|-----|-------|----------------------|-----|-------|--------------------|------|
| J1454.4+5123  | 223.622 | 51.400  | 87.656  | 56.458 | 0.051      | 0.049      | 58     | 18.5     | 2.0      | 0.2             | 22.4     | 2.1             | 2.04          | 0.07                 | PL  | ... | ...   | 1FGL J1454.6+5125    | ... | bzb   | TXS 1452+516       | ...  |
| J1456.7–6247c | 224.200 | –62.788 | 316.715 | –3.321 | 0.200      | 0.143      | 78     | 4.4      | 1.2      | 0.3             | 14.9     | 3.3             | 2.32          | 0.14                 | PL  | ... | 6     | ...                  | ... | ...   | ...                | ...  |
| J1457.4–3540  | 224.363 | –35.671 | 329.886 | 20.521 | 0.026      | 0.026      | 21     | 66.5     | 11.9     | 0.4             | 120.7    | 3.5             | 2.27          | ...                  | LP  | T   | ...   | 1FGL J1457.5–3540    | ... | BZQ   | PKS 1454–354       | 18   |
|               |         |         |         |        |            |            |        |          |          |                 |          |                 |               |                      |     |     |       | 0FGL J1457.6–3538    |     |       |                    |      |
|               |         |         |         |        |            |            |        |          |          |                 |          |                 |               |                      |     |     |       | 3EG J1500–3509       |     |       |                    |      |
| J1458.5–2121  | 224.643 | –21.362 | 338.533 | 32.579 | 0.150      | 0.116      | 77     | 4.1      | 0.5      | 0.1             | 6.5      | 1.5             | 2.28          | 0.18                 | PL  | ... | ...   | ...                  | ... | ...   | ...                | ...  |
| J1459.4–6054  | 224.857 | –60.913 | 317.867 | –1.808 | 0.033      | 0.031      | 22     | 37.9     | 13.9     | 0.6             | 121.7    | 4.5             | 2.32          | ...                  | EC  | ... | ...   | 1FGL J1459.4–6053    | ... | PSR   | LAT PSR J1459–6053 | ...  |
|               |         |         |         |        |            |            |        |          |          |                 |          |                 |               |                      |     |     |       | 0FGL J1459.4–6056    |     |       |                    |      |
| J1501.0+2238  | 225.275 | 22.639  | 31.462  | 60.336 | 0.049      | 0.042      | 79     | 17.5     | 1.9      | 0.2             | 23.9     | 3.0             | 1.77          | 0.07                 | PL  | T   | ...   | 1FGL J1501.1+2237    | ... | bzb   | MS 1458.8+2249     | ...  |
| J1502.1+5548  | 225.534 | 55.816  | 92.704  | 52.951 | 0.157      | 0.150      | –41    | 6.8      | 0.4      | 0.1             | 7.7      | 1.1             | 2.65          | 0.13                 | PL  | T   | ...   | ...                  | ... | ...   | ...                | ...  |
| J1502.4+4804  | 225.615 | 48.077  | 81.249  | 57.071 | 0.173      | 0.139      | –89    | 9.5      | 0.6      | 0.1             | 10.1     | 1.2             | 2.63          | 0.11                 | PL  | T   | ...   | 1FGL J1503.3+4759    | ... | ...   | ...                | ...  |
| J1503.7–1541  | 225.941 | –15.700 | 343.738 | 36.477 | 0.098      | 0.095      | 7      | 7.7      | 0.9      | 0.2             | 11.8     | 2.4             | 1.80          | 0.15                 | PL  | ... | ...   | 1FGL J1503.5–1544    | ... | bzb   | RBS 1457           | ...  |
|               |         |         |         |        |            |            |        |          |          |                 |          |                 |               |                      |     |     |       | 3EG J1504–1537       |     |       |                    |      |
|               |         |         |         |        |            |            |        |          |          |                 |          |                 |               |                      |     |     |       | EGR J1504–1539       |     |       |                    |      |
| J1503.9–5800c | 225.995 | –58.008 | 319.767 | 0.465  | 0.100      | 0.084      | –21    | 6.2      | 2.9      | 0.5             | 35.9     | 6.0             | 2.31          | 0.10                 | PL  | ... | 6     | 1FGL J1503.4–5805c   | E   | ...   | ...                | ...  |
| J1504.3+1029  | 226.095 | 10.488  | 11.366  | 54.585 | 0.013      | 0.013      | –53    | 116.1    | 40.1     | 0.7             | 382.2    | 7.3             | 2.21          | ...                  | LP  | T   | ...   | 1FGL J1504.4+1029    | ... | BZQ   | PKS 1504+106       | 19   |
|               |         |         |         |        |            |            |        |          |          |                 |          |                 |               |                      |     |     |       | 0FGL J1504.4+1030    |     |       |                    |      |
| J1504.9–3433  | 226.249 | –34.564 | 331.907 | 20.685 | 0.142      | 0.120      | –64    | 5.1      | 0.7      | 0.2             | 8.5      | 1.8             | 2.24          | 0.16                 | PL  | ... | ...   | 1FGL J1505.1–3435    | ... | bzb   | PMN J1505–3432     | ...  |
|               |         |         |         |        |            |            |        |          |          |                 |          |                 |               |                      |     |     |       | 3EG J1500–3509       |     |       |                    |      |
| J1505.1+0324  | 226.292 | 3.407   | 2.200   | 50.220 | 0.102      | 0.088      | –26    | 14.5     | 1.4      | 0.2             | 20.5     | 1.7             | 2.51          | 0.07                 | PL  | ... | ...   | 1FGL J1505.0+0328    | ... | sey   | PKS 1502+036       | ...  |
| J1506.0+3729  | 226.506 | 37.489  | 61.609  | 59.927 | 0.127      | 0.113      | 37     | 10.7     | 0.7      | 0.1             | 10.8     | 1.2             | 2.57          | 0.10                 | PL  | T   | ...   | 1FGL J1505.8+3725    | ... | bzq   | B2 1504+37         | ...  |
| J1506.6+0806  | 226.673 | 8.102   | 8.556   | 52.781 | 0.161      | 0.120      | 23     | 5.4      | 0.6      | 0.1             | 6.7      | 1.6             | 1.96          | 0.16                 | PL  | ... | ...   | ...                  | ... | bzb   | PMN J1506+0814     | ...  |
| J1506.9+1052  | 226.748 | 10.868  | 12.506  | 54.245 | 0.105      | 0.098      | –42    | 4.1      | 0.7      | 0.2             | 17.8     | 4.6             | 2.85          | 0.18                 | PL  | ... | 5     | ...                  | ... | ...   | ...                | ...  |
| J1507.0–6223  | 226.752 | –62.397 | 317.936 | –3.542 | 0.143      | 0.094      | 18     | 4.6      | 1.0      | 0.3             | 12.2     | 3.0             | 1.87          | 0.20                 | PL  | ... | ...   | ...                  | E   | ...   | ...                | ...  |
| J1508.5+2709  | 227.144 | 27.150  | 40.981  | 59.588 | 0.131      | 0.104      | –27    | 5.0      | 0.4      | 0.1             | 4.6      | 1.2             | 1.97          | 0.27                 | PL  | ... | ...   | ...                  | ... | bzb   | RBS 1467           | ...  |
| J1508.5–4957  | 227.149 | –49.951 | 324.359 | 7.127  | 0.113      | 0.097      | 61     | 7.6      | 1.3      | 0.2             | 22.8     | 3.0             | 2.61          | 0.09                 | PL  | T   | 5     | ...                  | ... | agu   | PMN J1508–4953     | ...  |
| J1508.9–4342  | 227.227 | –43.708 | 327.636 | 12.472 | 0.249      | 0.181      | –55    | 4.5      | 0.5      | 0.1             | 9.5      | 1.9             | 2.65          | 0.14                 | PL  | T   | ...   | ...                  | ... | bzq   | PMN J1509–4340     | ...  |
| J1509.6–5850  | 227.403 | –58.835 | 319.997 | –0.619 | 0.037      | 0.035      | 14     | 22.1     | 14.5     | 0.8             | 109.4    | 9.0             | 2.28          | ...                  | EC  | ... | ...   | 1FGL J1509.4–5850    | ... | PSR   | PSR J1509–5850     | ...  |
|               |         |         |         |        |            |            |        |          |          |                 |          |                 |               |                      |     |     |       | 0FGL J1509.5–5848    |     |       |                    |      |
|               |         |         |         |        |            |            |        |          |          |                 |          |                 |               |                      |     |     |       | 1AGL J1506–5859      |     |       |                    |      |
| J1509.7+5556  | 227.443 | 55.935  | 91.829  | 52.014 | 0.081      | 0.078      | –76    | 6.3      | 0.4      | 0.1             | 5.0      | 1.4             | 1.76          | 0.21                 | PL  | ... | ...   | 1FGL J1509.4+5602    | ... | bzb   | SBS 1508+561       | ...  |
| J1510.9–0545  | 227.726 | –5.759  | 353.874 | 42.905 | 0.076      | 0.072      | 5      | 12.6     | 2.2      | 0.2             | 30.9     | 3.0             | 2.44          | 0.06                 | PL  | T   | ...   | 1FGL J1511.1–0545    | ... | bzq   | PKS 1508–05        | ...  |
|               |         |         |         |        |            |            |        |          |          |                 |          |                 |               |                      |     |     |       | 0FGL J1511.2–0536    |     |       |                    |      |
| J1510.9–5808c | 227.735 | –58.138 | 320.500 | –0.107 | 0.109      | 0.082      | –26    | 4.4      | 2.6      | 0.5             | 33.8     | 7.7             | 2.38          | 0.12                 | PL  | ... | 4,5,6 | 1FGL J1510.8–5804c   | ... | ...   | ...                | ...  |
| J1511.8–0513  | 227.967 | –5.223  | 354.620 | 43.121 | 0.084      | 0.070      | –85    | 7.8      | 1.2      | 0.2             | 14.2     | 2.5             | 2.22          | 0.12                 | PL  | T   | 5     | 1FGL J1511.8–0513    | ... | ...   | ...                | ...  |

Table 1—Continued

| Name 2FGL     | R.A.    | Decl.   | $l$     | $b$     | $\theta_1$ | $\theta_2$ | $\phi$ | $\sigma$ | $F_{35}$ | $\Delta F_{35}$ | $S_{25}$ | $\Delta S_{25}$ | $\Gamma_{25}$ | $\Delta \Gamma_{25}$ | Mod | Var | Flags  | $\gamma$ -ray Assoc.                                                                          | TeV | Class | ID or Assoc.         | Ref.  |
|---------------|---------|---------|---------|---------|------------|------------|--------|----------|----------|-----------------|----------|-----------------|---------------|----------------------|-----|-----|--------|-----------------------------------------------------------------------------------------------|-----|-------|----------------------|-------|
| J1512.2+0201  | 228.070 | 2.023   | 2.323   | 47.970  | 0.066      | 0.063      | 75     | 14.3     | 1.8      | 0.2             | 20.3     | 2.0             | 2.17          | 0.08                 | PL  | ... | ...    | 1FGL J1512.3+0201                                                                             | ... | bzq   | PKS 1509+022         | ...   |
| J1512.5−6247c | 228.149 | −62.785 | 318.294 | −4.203  | 0.179      | 0.150      | 70     | 7.4      | 0.6      | 0.2             | 22.5     | 2.8             | 2.54          | ...                  | LP  | ... | 1,6,12 | ...                                                                                           | ... | ...   | ...                  | ...   |
| J1512.8−0906  | 228.207 | −9.103  | 351.283 | 40.138  | 0.014      | 0.014      | −38    | 202.4    | 40.6     | 0.7             | 510.5    | 6.0             | 2.39          | ...                  | LP  | T   | ...    | 1FGL J1512.8−0906<br>0FGL J1512.7−0905<br>3EG J1512−0849<br>EGR J1512−0857<br>1AGL J1511−0908 | P   | BZQ   | PKS 1510−08          | 20,21 |
| J1513.5−2546  | 228.381 | −25.767 | 338.897 | 27.007  | 0.156      | 0.149      | 43     | 4.4      | 0.7      | 0.2             | 7.3      | 1.7             | 2.15          | 0.14                 | PL  | ... | ...    | 3EG J1517−2538                                                                                | ... | ...   | ...                  | ...   |
| J1513.6−3233  | 228.402 | −32.565 | 334.681 | 21.400  | 0.122      | 0.116      | 18     | 11.3     | 1.6      | 0.2             | 20.6     | 2.1             | 2.41          | 0.08                 | PL  | T   | ...    | ...                                                                                           | ... | bzq   | PKS 1510−324         | ...   |
| J1513.9−2256  | 228.481 | −22.947 | 340.858 | 29.238  | 0.131      | 0.122      | −88    | 4.3      | 0.6      | 0.2             | 6.6      | 1.8             | 1.96          | 0.24                 | PL  | ... | ...    | ...                                                                                           | ... | ...   | ...                  | ...   |
| J1514.0−5915e | 228.507 | −59.256 | 320.270 | −1.271  | ...        | ...        | ...    | ...      | 2.9      | ...             | 45.6     | ...             | 1.57          | ...                  | PL  | ... | 4,5    | ...                                                                                           | E   | PWN   | MSH 15−52 PWN        | 22    |
| J1514.1−4946  | 228.544 | −49.773 | 325.229 | 6.817   | 0.036      | 0.034      | 10     | 26.1     | 7.0      | 0.4             | 42.7     | 3.5             | 2.05          | ...                  | LP  | ... | ...    | 1FGL J1514.1−4945<br>0FGL J1514.3−4946                                                        | ... | psr   | PSR J1514−49         | ...   |
| J1514.6−4751  | 228.657 | −47.850 | 326.311 | 8.416   | 0.072      | 0.061      | 74     | 11.7     | 2.1      | 0.2             | 24.5     | 2.5             | 2.25          | 0.07                 | PL  | T   | ...    | 1FGL J1514.1−4745                                                                             | ... | agu   | PMN J1514−4748       | ...   |
| J1514.6+4449  | 228.659 | 44.823  | 74.274  | 56.452  | 0.124      | 0.112      | −46    | 8.7      | 0.8      | 0.1             | 9.2      | 1.3             | 2.29          | 0.12                 | PL  | T   | ...    | 1FGL J1514.7+4447                                                                             | ... | bzq   | BZQ J1514+4450       | ...   |
| J1516.9+1925  | 229.248 | 19.425  | 27.806  | 55.824  | 0.155      | 0.136      | −68    | 4.9      | 0.5      | 0.1             | 6.6      | 1.3             | 2.46          | 0.16                 | PL  | ... | ...    | 1FGL J1516.9+1928                                                                             | ... | bzb   | PKS 1516+197         | ...   |
| J1517.2+3645  | 229.317 | 36.764  | 59.580  | 57.818  | 0.157      | 0.132      | 24     | 4.1      | 0.3      | 0.1             | 3.9      | 1.0             | 2.13          | 0.19                 | PL  | T   | ...    | ...                                                                                           | ... | ...   | ...                  | ...   |
| J1517.7−2421  | 229.435 | −24.360 | 340.698 | 27.582  | 0.037      | 0.035      | −6     | 29.2     | 5.2      | 0.3             | 57.3     | 3.5             | 2.05          | 0.04                 | PL  | ... | ...    | 1FGL J1517.8−2423<br>0FGL J1517.9−2423                                                        | P   | bzb   | AP Librae            | ...   |
| J1518.0+6526  | 229.517 | 65.437  | 102.249 | 45.358  | 0.076      | 0.072      | −25    | 9.6      | 0.7      | 0.1             | 9.8      | 2.0             | 1.66          | 0.13                 | PL  | ... | ...    | 1FGL J1517.8+6530                                                                             | ... | bzb   | 1H 1515+660          | ...   |
| J1518.2−2733  | 229.552 | −27.561 | 338.678 | 24.940  | 0.103      | 0.089      | −72    | 6.7      | 1.0      | 0.2             | 11.3     | 2.1             | 2.05          | 0.14                 | PL  | ... | ...    | ...                                                                                           | ... | agu   | TXS 1515−273         | ...   |
| J1518.4−5233  | 229.614 | −52.566 | 324.319 | 4.092   | 0.106      | 0.088      | 61     | 5.6      | 1.3      | 0.2             | 14.2     | 2.8             | 1.99          | 0.11                 | PL  | ... | ...    | 1FGL J1518.0−5233                                                                             | ... | ...   | ...                  | ...   |
| J1520.8−0349  | 230.221 | −3.833  | 358.115 | 42.478  | 0.089      | 0.079      | −56    | 8.7      | 1.1      | 0.2             | 13.1     | 2.4             | 1.84          | 0.12                 | PL  | ... | ...    | 1FGL J1521.0−0350                                                                             | ... | bzb   | NVSS J152048−034850  | ...   |
| J1520.9+4209  | 230.241 | 42.164  | 69.088  | 56.127  | 0.286      | 0.195      | −84    | 7.3      | 0.3      | 0.1             | 5.1      | 0.8             | 2.65          | ...                  | LP  | ... | 12     | 1FGL J1519.7+4216                                                                             | ... | bzq   | B3 1518+423          | ...   |
| J1521.8−5735  | 230.458 | −57.598 | 322.016 | −0.409  | 0.055      | 0.050      | 67     | 16.7     | 8.9      | 0.7             | 65.0     | 5.4             | 2.28          | ...                  | LP  | ... | ...    | 1FGL J1521.8−5734c                                                                            | ... | †     | ...                  | ...   |
| J1522.0+4348  | 230.506 | 43.805  | 71.816  | 55.508  | 0.254      | 0.230      | −27    | 5.4      | 0.2      | 0.1             | 7.7      | 1.3             | 2.99          | 0.16                 | PL  | T   | ...    | ...                                                                                           | ... | bzq   | B3 1520+437          | ...   |
| J1522.1+3144  | 230.542 | 31.744  | 50.176  | 57.023  | 0.019      | 0.019      | 55     | 131.4    | 17.6     | 0.5             | 213.7    | 3.7             | 2.37          | ...                  | LP  | T   | ...    | 1FGL J1522.1+3143<br>0FGL J1522.2+3143                                                        | ... | bzq   | B2 1520+31           | ...   |
| J1522.7−2731  | 230.676 | −27.523 | 339.586 | 24.380  | 0.053      | 0.048      | −35    | 20.3     | 3.5      | 0.3             | 40.9     | 2.8             | 2.22          | 0.05                 | PL  | T   | ...    | 1FGL J1522.6−2732                                                                             | ... | bzb   | PKS 1519−273         | ...   |
| J1528.0−5841  | 232.007 | −58.691 | 322.094 | −1.771  | 0.103      | 0.084      | 49     | 7.3      | 2.4      | 0.4             | 31.8     | 4.3             | 2.42          | 0.09                 | PL  | ... | 1      | ...                                                                                           | ... | ...   | ...                  | ...   |
| J1531.0+5725  | 232.753 | 57.431  | 91.356  | 48.751  | 0.153      | 0.125      | −11    | 4.8      | 0.4      | 0.1             | 4.2      | 1.0             | 2.08          | 0.21                 | PL  | ... | ...    | ...                                                                                           | ... | bzb   | 87GB 152947.5+574636 | ...   |
| J1535.4+3720  | 233.861 | 37.335  | 59.962  | 54.153  | 0.160      | 0.132      | −43    | 5.0      | 0.4      | 0.1             | 5.1      | 1.1             | 2.15          | 0.16                 | PL  | ... | ...    | ...                                                                                           | ... | bzb   | RGB J1534+372        | ...   |
| J1536.4−4949  | 234.124 | −49.829 | 328.205 | 4.767   | 0.028      | 0.026      | 0      | 40.3     | 12.0     | 0.5             | 94.6     | 4.5             | 2.09          | ...                  | LP  | ... | ...    | 1FGL J1536.5−4949<br>0FGL J1536.7−4947                                                        | ... | ...   | ...                  | ...   |
| J1537.4−7957  | 234.356 | −79.961 | 309.967 | −19.439 | 0.122      | 0.111      | 28     | 5.3      | 0.7      | 0.2             | 7.7      | 1.6             | 2.19          | 0.16                 | PL  | ... | ...    | ...                                                                                           | ... | agu   | PMN J1537−7958       | ...   |

Table 1—Continued

| Name 2FGL     | R.A.    | Decl.   | $l$     | $b$     | $\theta_1$ | $\theta_2$ | $\phi$ | $\sigma$ | $F_{35}$ | $\Delta F_{35}$ | $S_{25}$ | $\Delta S_{25}$ | $\Gamma_{25}$ | $\Delta \Gamma_{25}$ | Mod | Var | Flags  | $\gamma$ -ray Assoc.                   | TeV | Class | ID or Assoc.          | Ref. |
|---------------|---------|---------|---------|---------|------------|------------|--------|----------|----------|-----------------|----------|-----------------|---------------|----------------------|-----|-----|--------|----------------------------------------|-----|-------|-----------------------|------|
| J1538.1+8159  | 234.530 | 81.988  | 116.590 | 32.970  | 0.069      | 0.063      | −80    | 7.6      | 0.4      | 0.1             | 7.3      | 2.0             | 1.48          | 0.16                 | PL  | ... | ...    | 1FGL J1536.6+8200                      | ... | bzb   | 1ES 1544+820          | ...  |
| J1539.2−3325  | 234.813 | −33.428 | 338.743 | 17.529  | 0.072      | 0.067      | 54     | 10.8     | 2.3      | 0.3             | 10.6     | 1.5             | 1.85          | ...                  | LP  | ... | ...    | 1FGL J1539.0−3328                      | ... | ...   | ...                   | ...  |
| J1539.3−4636  | 234.835 | −46.611 | 330.511 | 7.074   | 0.439      | 0.240      | −16    | 6.9      | 1.1      | 0.2             | 17.9     | 2.7             | 2.60          | 0.11                 | PL  | ... | 4,8,9  | ...                                    | ... | ...   | ...                   | ...  |
| J1539.5+2747  | 234.896 | 27.791  | 43.951  | 52.879  | 0.114      | 0.097      | 11     | 6.8      | 0.6      | 0.1             | 7.2      | 1.5             | 1.99          | 0.13                 | PL  | T   | ...    | 1FGL J1539.7+2747                      | ... | bzq   | MG2 J153938+2744      | ...  |
| J1540.4+1438  | 235.102 | 14.644  | 24.053  | 48.828  | 0.232      | 0.181      | 13     | 4.6      | 0.5      | 0.1             | 6.3      | 1.4             | 2.28          | 0.19                 | PL  | ... | ...    | ...                                    | ... | bzb   | 4C +14.60             | ...  |
| J1542.9+6129  | 235.729 | 61.489  | 95.383  | 45.401  | 0.026      | 0.025      | −17    | 51.7     | 6.4      | 0.3             | 71.7     | 3.4             | 1.97          | 0.03                 | PL  | T   | ...    | 1FGL J1542.9+6129<br>0FGL J1543.1+6130 | ... | bzb   | GB6 J1542+6129        | ...  |
| J1543.7−0241  | 235.934 | −2.692  | 4.167   | 38.901  | 0.236      | 0.203      | 71     | 4.3      | 0.6      | 0.2             | 8.1      | 1.7             | 2.46          | 0.14                 | PL  | ... | ...    | 1FGL J1544.0−0252                      | ... | ...   | ...                   | ...  |
| J1544.1−2554  | 236.042 | −25.912 | 344.751 | 22.610  | 0.178      | 0.136      | −14    | 8.5      | 1.2      | 0.2             | 16.0     | 2.0             | 2.40          | 0.10                 | PL  | ... | ...    | ...                                    | ... | ...   | ...                   | ...  |
| J1544.5−1126  | 236.139 | −11.446 | 356.170 | 32.994  | 0.142      | 0.120      | 57     | 5.8      | 0.8      | 0.2             | 10.0     | 1.8             | 2.35          | 0.12                 | PL  | T   | ...    | 1FGL J1544.5−1127                      | ... | ...   | ...                   | ...  |
| J1546.1+0820  | 236.527 | 8.342   | 16.829  | 44.678  | 0.104      | 0.083      | 8      | 4.9      | 0.3      | 0.1             | 5.4      | 2.0             | 1.57          | 0.21                 | PL  | ... | ...    | ...                                    | ... | bzb   | 1RXS J154604.6+081912 | ...  |
| J1548.3+1453  | 237.088 | 14.900  | 25.586  | 47.183  | 0.082      | 0.072      | 56     | 10.4     | 1.1      | 0.2             | 13.1     | 1.7             | 2.22          | 0.11                 | PL  | ... | ...    | 1FGL J1548.6+1451                      | ... | ...   | ...                   | ...  |
| J1548.8−2251  | 237.212 | −22.862 | 347.841 | 24.157  | 0.077      | 0.063      | 23     | 8.5      | 1.2      | 0.2             | 13.9     | 2.4             | 1.93          | 0.13                 | PL  | ... | ...    | 1FGL J1548.7−2250                      | ... | bzb   | PMN J1548−2251        | ...  |
| J1549.5+0237  | 237.388 | 2.627   | 10.869  | 40.897  | 0.073      | 0.062      | 61     | 16.6     | 1.8      | 0.2             | 25.5     | 1.9             | 2.46          | 0.07                 | PL  | T   | ...    | 1FGL J1549.3+0235                      | ... | bzq   | PKS 1546+027          | ...  |
| J1549.7−0657  | 237.432 | −6.965  | 1.226   | 35.031  | 0.114      | 0.094      | −62    | 5.5      | 0.7      | 0.2             | 8.3      | 1.7             | 2.10          | 0.13                 | PL  | ... | ...    | 1FGL J1549.7−0659                      | ... | psr   | PSR J1549−06          | ...  |
| J1550.7+0526  | 237.687 | 5.434   | 14.224  | 42.187  | 0.120      | 0.112      | 59     | 9.0      | 1.0      | 0.2             | 12.6     | 1.6             | 2.32          | 0.11                 | PL  | ... | ...    | 1FGL J1550.7+0527                      | ... | bzq   | 4C +05.44             | ...  |
| J1551.0−4636  | 237.770 | −46.608 | 332.111 | 5.835   | 0.162      | 0.128      | −43    | 7.1      | 0.5      | 0.2             | 16.6     | 2.5             | 2.62          | ...                  | LP  | ... | 1,4,12 | ...                                    | ... | ...   | ...                   | ...  |
| J1551.3−5333c | 237.837 | −53.562 | 327.756 | 0.406   | 0.119      | 0.080      | −24    | 5.7      | 5.4      | 0.9             | 33.7     | 7.1             | 2.05          | ...                  | LP  | ... | 3,5,6  | ...                                    | ... | ...   | ...                   | ...  |
| J1551.9+0855  | 237.975 | 8.925   | 18.526  | 43.724  | 0.121      | 0.099      | −9     | 5.0      | 0.6      | 0.1             | 6.2      | 1.5             | 2.00          | 0.16                 | PL  | ... | ...    | 1FGL J1551.7+0851                      | ... | bzb   | TXS 1549+089          | ...  |
| J1552.8−4824  | 238.212 | −48.410 | 331.197 | 4.251   | 0.241      | 0.147      | 18     | 6.6      | 0.6      | 0.2             | 19.3     | 2.9             | 2.53          | ...                  | LP  | ... | 4,12   | ...                                    | ... | ...   | ...                   | ...  |
| J1552.8−5609  | 238.214 | −56.152 | 326.290 | −1.739  | 0.046      | 0.043      | 52     | 15.3     | 5.0      | 0.4             | 56.8     | 5.1             | 1.93          | 0.06                 | PL  | ... | ...    | 1FGL J1552.4−5609                      | ... | †     | ...                   | ...  |
| J1553.2−2424  | 238.322 | −24.404 | 347.501 | 22.337  | 0.165      | 0.134      | −56    | 4.4      | 0.6      | 0.2             | 8.6      | 1.9             | 2.45          | 0.17                 | PL  | ... | ...    | 1FGL J1553.4−2425                      | ... | agu   | PKS 1550−242          | ...  |
| J1553.5−3116  | 238.383 | −31.273 | 342.614 | 17.231  | 0.065      | 0.059      | −25    | 7.1      | 0.7      | 0.2             | 11.3     | 2.8             | 1.57          | 0.14                 | PL  | ... | ...    | 1FGL J1553.5−3116                      | ... | bzb   | 1RXS J155333.4−311841 | ...  |
| J1553.5+1255  | 238.388 | 12.929  | 23.767  | 45.211  | 0.044      | 0.042      | 72     | 33.0     | 4.9      | 0.3             | 42.1     | 2.3             | 2.23          | ...                  | LP  | T   | ...    | 1FGL J1553.4+1255<br>0FGL J1553.4+1255 | ... | bzq   | PKS 1551+130          | ...  |
| J1553.5−0324  | 238.396 | −3.401  | 5.385   | 36.530  | 0.170      | 0.115      | −15    | 5.2      | 0.9      | 0.2             | 10.4     | 2.1             | 2.22          | 0.14                 | PL  | ... | ...    | ...                                    | ... | ...   | ...                   | ...  |
| J1554.4−5317c | 238.624 | −53.289 | 328.292 | 0.320   | 0.089      | 0.075      | −5     | 7.9      | 7.7      | 1.0             | 56.2     | 7.9             | 2.10          | ...                  | LP  | ... | 6      | 1FGL J1554.8−5312c                     | ... | ...   | ...                   | ...  |
| J1555.7+1111  | 238.942 | 11.190  | 21.917  | 43.953  | 0.015      | 0.015      | 88     | 69.2     | 14.0     | 0.5             | 197.4    | 9.2             | 1.67          | 0.02                 | PL  | T   | ...    | 1FGL J1555.7+1111<br>0FGL J1555.8+1110 | P   | bzb   | PG 1553+113           | ...  |
| J1558.3+8513  | 239.577 | 85.220  | 118.901 | 30.348  | 0.104      | 0.090      | −90    | 9.2      | 0.6      | 0.1             | 9.7      | 1.2             | 2.52          | 0.11                 | PL  | ... | ...    | ...                                    | ... | agu   | WN B1609.6+8517       | ...  |
| J1558.6−7039  | 239.654 | −70.656 | 317.291 | −13.204 | 0.153      | 0.098      | 84     | 4.6      | 0.6      | 0.1             | 6.6      | 1.6             | 2.10          | 0.17                 | PL  | ... | ...    | ...                                    | ... | agu   | PKS 1552−705          | ...  |
| J1558.9−6428  | 239.737 | −64.483 | 321.474 | −8.594  | 0.088      | 0.081      | −55    | 9.8      | 1.6      | 0.2             | 17.4     | 2.4             | 2.01          | 0.10                 | PL  | ... | ...    | ...                                    | ... | agu   | PMN J1558−6432        | ...  |
| J1559.0+5627  | 239.767 | 56.457  | 87.620  | 45.727  | 0.081      | 0.075      | −88    | 13.3     | 1.3      | 0.1             | 14.2     | 1.6             | 2.10          | 0.09                 | PL  | T   | ...    | 1FGL J1558.9+5627                      | ... | bzb   | TXS 1557+565          | ...  |
| J1600.7−3053  | 240.188 | −30.894 | 344.075 | 16.470  | 0.082      | 0.068      | 32     | 7.5      | 1.0      | 0.2             | 5.5      | 1.0             | 1.90          | ...                  | EC  | ... | ...    | 1FGL J1600.7−3055                      | ... | PSR   | PSR J1600−3053        | ...  |
| J1601.1−4220  | 240.279 | −42.336 | 336.269 | 7.935   | 0.194      | 0.142      | 64     | 7.3      | 1.5      | 0.3             | 20.5     | 2.8             | 2.46          | 0.10                 | PL  | ... | ...    | 1FGL J1601.7−4217c                     | ... | ...   | ...                   | ...  |



Table 1—Continued

| Name 2FGL     | R.A.    | Decl.   | $l$     | $b$     | $\theta_1$ | $\theta_2$ | $\phi$ | $\sigma$ | $F_{35}$ | $\Delta F_{35}$ | $S_{25}$ | $\Delta S_{25}$ | $\Gamma_{25}$ | $\Delta \Gamma_{25}$ | Mod | Var | Flags      | $\gamma$ -ray Assoc.                                  | TeV | Class | ID or Assoc.    | Ref. |
|---------------|---------|---------|---------|---------|------------|------------|--------|----------|----------|-----------------|----------|-----------------|---------------|----------------------|-----|-----|------------|-------------------------------------------------------|-----|-------|-----------------|------|
| J1602.4+2308  | 240.617 | 23.141  | 38.627  | 46.833  | 0.164      | 0.133      | −70    | 5.2      | 0.6      | 0.1             | 6.3      | 1.4             | 2.11          | 0.15                 | PL  | ... | 1          | ...                                                   | ... | ...   | ...             | ...  |
| J1603.8−4904  | 240.971 | −49.078 | 332.149 | 2.561   | 0.024      | 0.023      | −24    | 33.0     | 12.9     | 0.6             | 143.7    | 6.5             | 2.04          | 0.03                 | PL  | T   | ...        | 1FGL J1603.8−4903<br>0FGL J1604.0−4904                | ... | bzb   | PMN J1603−4904  | ...  |
| J1604.5−4442  | 241.141 | −44.716 | 335.147 | 5.741   | 0.060      | 0.054      | −61    | 22.5     | 5.4      | 0.4             | 68.2     | 3.7             | 2.35          | 0.04                 | PL  | T   | ...        | 1FGL J1604.7−4443                                     | ... | agu   | PMN J1604−4441  | ...  |
| J1604.6+5710  | 241.154 | 57.179  | 88.190  | 44.759  | 0.086      | 0.066      | 63     | 19.2     | 1.6      | 0.2             | 24.2     | 1.6             | 2.50          | 0.06                 | PL  | T   | ...        | 1FGL J1604.3+5710                                     | ... | bzq   | GB6 J1604+5714  | ...  |
| J1607.0+1552  | 241.770 | 15.876  | 29.396  | 43.421  | 0.054      | 0.050      | −46    | 19.5     | 2.2      | 0.2             | 25.3     | 1.9             | 2.23          | 0.06                 | PL  | T   | ...        | 1FGL J1607.1+1552<br>3EG J1605+1553<br>EGR J1607+1533 | ... | bzb   | 4C +15.54       | ...  |
| J1608.5+1029  | 242.148 | 10.494  | 23.013  | 40.831  | 0.089      | 0.082      | 84     | 20.0     | 1.6      | 0.2             | 26.1     | 1.7             | 2.60          | ...                  | LP  | T   | ...        | 1FGL J1609.0+1031<br>3EG J1608+1055<br>EGR J1608+1051 | ... | bzq   | 4C +10.45       | ...  |
| J1610.1−4808  | 242.542 | −48.148 | 333.545 | 2.553   | 0.194      | 0.166      | −45    | 9.5      | 1.5      | 0.5             | 40.5     | 4.7             | 2.73          | ...                  | LP  | T   | 1,4        | ...                                                   | ... | ...   | ...             | ...  |
| J1610.6−4002  | 242.664 | −40.043 | 339.171 | 8.416   | 0.309      | 0.191      | 75     | 8.6      | 1.4      | 0.2             | 23.5     | 2.8             | 2.61          | 0.10                 | PL  | ... | 9          | 1FGL J1610.8−3955                                     | ... | bzq   | PMN J1610−3958  | ...  |
| J1610.8−6650  | 242.703 | −66.844 | 320.771 | −11.161 | 0.044      | 0.041      | 28     | 18.5     | 2.6      | 0.2             | 34.9     | 3.9             | 1.70          | 0.06                 | PL  | ... | ...        | 1FGL J1610.6−6649                                     | ... | bzb   | PMN J1610−6649  | ...  |
| J1612.0+1403  | 243.002 | 14.063  | 27.774  | 41.612  | 0.205      | 0.190      | 85     | 4.7      | 0.5      | 0.1             | 6.4      | 1.4             | 2.31          | 0.15                 | PL  | ... | ...        | ...                                                   | ... | ...   | ...             | ...  |
| J1613.4+3409  | 243.372 | 34.159  | 55.068  | 46.415  | 0.174      | 0.121      | 75     | 6.0      | 0.5      | 0.1             | 6.0      | 1.1             | 2.31          | 0.17                 | PL  | ... | ...        | 1FGL J1613.5+3411<br>3EG J1614+3424                   | ... | bzq   | OS 349<br>J1614 | ...  |
| J1614.5−2230  | 243.646 | −22.513 | 352.629 | 20.193  | 0.054      | 0.051      | 52     | 19.0     | 4.5      | 0.4             | 22.7     | 2.1             | 2.05          | ...                  | EC  | T   | ...        | 3EG J1616−2221                                        | ... | PSR   | PSR J1614−2230  | ...  |
| J1614.8+4703  | 243.712 | 47.054  | 73.686  | 45.773  | 0.228      | 0.177      | 9      | 4.6      | 0.3      | 0.1             | 4.8      | 1.1             | 2.45          | 0.22                 | PL  | ... | ...        | ...                                                   | ... | ...   | ...             | ...  |
| J1614.9−5212  | 243.745 | −52.206 | 331.327 | −0.931  | 0.120      | 0.115      | 67     | 4.4      | 2.2      | 0.6             | 25.3     | 6.4             | 1.98          | 0.18                 | PL  | ... | 2          | ...                                                   | ... | ...   | ...             | ...  |
| J1615.0−5051  | 243.758 | −50.852 | 332.268 | 0.043   | 0.088      | 0.074      | 39     | 15.2     | 12.1     | 1.3             | 120.3    | 9.8             | 2.28          | ...                  | LP  | ... | ...        | 0FGL J1615.6−5049                                     | E   | †     | ...             | ...  |
| J1615.2−5138  | 243.801 | −51.635 | 331.747 | −0.542  | 0.056      | 0.047      | 28     | 14.7     | 12.1     | 1.0             | 91.4     | 10.4            | 2.11          | ...                  | LP  | ... | 2          | 1FGL J1614.7−5138c                                    | E   | ...   | ...             | ...  |
| J1616.8−2302  | 244.211 | −23.042 | 352.590 | 19.452  | 0.126      | 0.098      | −43    | 4.9      | 0.8      | 0.2             | 9.5      | 2.4             | 1.90          | 0.18                 | PL  | ... | ...        | ...                                                   | ... | glc   | M80             | ...  |
| J1617.3−5336  | 244.340 | −53.614 | 330.609 | −2.194  | 0.159      | 0.143      | 43     | 4.8      | 1.4      | 0.3             | 21.7     | 4.0             | 2.54          | 0.11                 | PL  | ... | ...        | ...                                                   | ... | ...   | ...             | ...  |
| J1617.5−2657  | 244.394 | −26.957 | 349.693 | 16.663  | 0.147      | 0.117      | 5      | 4.2      | 0.9      | 0.2             | 11.0     | 2.5             | 2.36          | 0.16                 | PL  | ... | ...        | 3EG J1612−2618<br>EGR J1617−2610                      | ... | ...   | ...             | ...  |
| J1617.6−2526c | 244.411 | −25.438 | 350.865 | 17.691  | 0.184      | 0.154      | −41    | 5.8      | 1.1      | 0.2             | 16.3     | 2.7             | 2.52          | 0.11                 | PL  | ... | 6          | EGR J1617−2610                                        | ... | agu   | PMN J1617−2537  | ...  |
| J1617.6−4219  | 244.425 | −42.331 | 338.531 | 5.850   | 0.285      | 0.231      | −27    | 5.8      | 0.8      | 0.2             | 19.3     | 3.2             | 2.80          | 0.13                 | PL  | ... | 4          | ...                                                   | ... | ...   | ...             | ...  |
| J1618.0−5825  | 244.506 | −58.431 | 327.300 | −5.704  | 0.121      | 0.103      | 49     | 5.8      | 0.9      | 0.2             | 14.3     | 2.4             | 2.59          | 0.14                 | PL  | ... | 4          | ...                                                   | ... | ...   | ...             | ...  |
| J1618.2−7718  | 244.562 | −77.301 | 313.438 | −18.879 | 0.078      | 0.071      | 24     | 16.4     | 2.1      | 0.2             | 31.0     | 2.0             | 2.50          | 0.05                 | PL  | T   | ...        | 1FGL J1617.9−7716                                     | ... | bzq   | PKS 1610−77     | ...  |
| J1619.0−4650  | 244.769 | −46.847 | 335.534 | 2.457   | 0.427      | 0.249      | −60    | 10.6     | 1.3      | 0.3             | 38.6     | 4.0             | 2.69          | ...                  | LP  | ... | 1,9,12     | ...                                                   | ... | ...   | ...             | ...  |
| J1619.6−4509  | 244.919 | −45.158 | 336.796 | 3.586   | 0.163      | 0.128      | 82     | 5.5      | 1.7      | 0.3             | 19.6     | 4.0             | 2.25          | 0.14                 | PL  | ... | 1          | ...                                                   | ... | ...   | ...             | ...  |
| J1619.7−5040c | 244.932 | −50.681 | 332.920 | −0.351  | 0.077      | 0.063      | −38    | 6.4      | 5.3      | 0.8             | 63.5     | 10.8            | 2.27          | 0.08                 | PL  | ... | 3,4,5,6,10 | 1FGL J1619.7−5043c                                    | ... | ...   | ...             | ...  |
| J1620.5−2320c | 245.125 | −23.348 | 352.949 | 18.624  | 0.165      | 0.131      | −1     | 4.6      | 1.1      | 0.2             | 12.7     | 2.7             | 2.29          | 0.13                 | PL  | ... | 6          | ...                                                   | ... | ...   | ...             | ...  |
| J1620.6−5111c | 245.166 | −51.194 | 332.664 | −0.820  | 0.130      | 0.095      | −82    | 9.9      | 6.7      | 0.9             | 68.5     | 8.5             | 2.37          | ...                  | LP  | T   | 4,6        | ...                                                   | ... | ...   | ...             | ...  |

Table 1—Continued

| Name 2FGL     | R.A.    | Decl.   | $l$     | $b$     | $\theta_1$ | $\theta_2$ | $\phi$ | $\sigma$ | $F_{35}$ | $\Delta F_{35}$ | $S_{25}$ | $\Delta S_{25}$ | $\Gamma_{25}$ | $\Delta \Gamma_{25}$ | Mod | Var | Flags    | $\gamma$ -ray Assoc.                                     | TeV | Class            | ID or Assoc.   | Ref. |
|---------------|---------|---------|---------|---------|------------|------------|--------|----------|----------|-----------------|----------|-----------------|---------------|----------------------|-----|-----|----------|----------------------------------------------------------|-----|------------------|----------------|------|
| J1620.8–4928  | 245.209 | −49.481 | 333.890 | 0.376   | 0.029      | 0.027      | −51    | 28.0     | 24.8     | 1.1             | 180.8    | 9.7             | 2.20          | ...                  | LP  | ... | ...      | 1FGL J1620.8–4928c<br>1AGL J1624–4946                    | ... | ...              | ...            | ...  |
| J1622.8–5006  | 245.717 | −50.108 | 333.679 | −0.299  | 0.058      | 0.049      | 18     | 11.2     | 9.9      | 1.3             | 54.9     | 11.1            | 2.14          | ...                  | LP  | ... | ...      | 1FGL J1622.9–5008c<br>1AGL J1624–4946                    | ... | ...              | ...            | ...  |
| J1622.8–0314  | 245.721 | −3.243  | 10.708  | 30.708  | 0.143      | 0.112      | 13     | 6.0      | 0.9      | 0.2             | 10.0     | 1.8             | 2.22          | 0.13                 | PL  | ... | ...      | ...                                                      | ... | ...              | ...            | ...  |
| J1623.2+4328  | 245.814 | 43.469  | 68.415  | 44.654  | 0.160      | 0.134      | 67     | 4.7      | 0.3      | 0.1             | 5.1      | 1.1             | 2.58          | 0.22                 | PL  | ... | ...      | ...                                                      | ... | ...              | ...            | ...  |
| J1624.0–4941c | 246.015 | −49.695 | 334.108 | −0.145  | 0.115      | 0.097      | −6     | 5.5      | 7.0      | 1.3             | 28.6     | 5.5             | 2.26          | ...                  | LP  | ... | 4,5,6,12 | 1FGL J1623.7–4943c<br>1AGL J1624–4946                    | ... | ...              | ...            | ...  |
| J1624.1–4040  | 246.041 | −40.673 | 340.571 | 6.161   | 0.065      | 0.054      | 37     | 16.8     | 4.7      | 0.4             | 37.9     | 3.3             | 2.31          | ...                  | LP  | ... | ...      | 1FGL J1624.0–4041                                        | ... | ...              | ...            | ...  |
| J1624.2–2124  | 246.072 | −21.411 | 355.095 | 19.252  | 0.453      | 0.236      | 49     | 8.2      | 0.4      | 0.1             | 15.4     | 1.9             | 2.64          | ...                  | LP  | ... | 8,12     | ...                                                      | ... | ...              | ...            | ...  |
| J1624.4+1123  | 246.117 | 11.391  | 26.279  | 37.732  | 0.373      | 0.251      | 14     | 4.4      | 0.4      | 0.1             | 6.9      | 1.5             | 2.65          | 0.18                 | PL  | ... | 8        | ...                                                      | agu | MG1 J162441+1111 | ...            | ...  |
| J1625.2–0020  | 246.303 | −0.335  | 13.920  | 31.831  | 0.057      | 0.051      | 73     | 20.5     | 3.9      | 0.3             | 16.1     | 1.3             | 1.97          | ...                  | LP  | ... | 12       | 1FGL J1625.3–0019                                        | ... | ...              | ...            | ...  |
| J1625.7–2526  | 246.428 | −25.441 | 352.145 | 16.344  | 0.046      | 0.039      | 70     | 30.1     | 8.2      | 0.5             | 82.1     | 4.2             | 2.34          | ...                  | LP  | T   | ...      | 1FGL J1625.7–2524<br>0FGL J1625.8–2527<br>3EG J1626–2519 | ... | bzq              | PKS 1622–253   | ...  |
| J1626.0–7636  | 246.516 | −76.604 | 314.298 | −18.746 | 0.091      | 0.082      | 1      | 5.4      | 0.5      | 0.1             | 6.0      | 1.7             | 1.79          | 0.21                 | PL  | ... | ...      | ...                                                      | agu | PKS 1619–765     | ...            | ...  |
| J1626.1–2948  | 246.529 | −29.809 | 348.856 | 13.346  | 0.093      | 0.082      | 11     | 13.0     | 2.4      | 0.3             | 30.0     | 2.7             | 2.34          | 0.07                 | PL  | T   | ...      | 1FGL J1626.2–2956<br>3EG J1625–2955<br>EGR J1625–2958    | ... | BZQ              | PKS 1622–29    | ...  |
| J1626.4–4408  | 246.609 | −44.144 | 338.365 | 3.444   | 0.129      | 0.096      | −57    | 9.8      | 2.4      | 0.3             | 39.2     | 4.2             | 2.58          | 0.08                 | PL  | ... | ...      | ...                                                      | ... | ...              | ...            | ...  |
| J1627.0–2425c | 246.760 | −24.429 | 353.144 | 16.789  | 0.118      | 0.084      | −86    | 14.4     | 5.0      | 0.5             | 42.5     | 4.3             | 2.28          | ...                  | LP  | ... | 6        | 0FGL J1625.9–2423<br>3EG J1627–2419                      | ... | agu              | PMN J1626–2426 | ...  |
| J1627.8+3219  | 246.966 | 32.321  | 52.988  | 43.215  | 0.129      | 0.103      | 61     | 7.7      | 0.7      | 0.1             | 8.2      | 1.6             | 2.00          | 0.12                 | PL  | ... | ...      | 1FGL J1627.6+3218                                        | ... | ...              | ...            | ...  |
| J1628.1–4857c | 247.045 | −48.960 | 335.102 | −0.114  | 0.191      | 0.108      | 60     | 12.6     | 6.5      | 1.1             | 92.6     | 7.8             | 2.48          | ...                  | LP  | ... | 2,4,5,6  | ...                                                      | ... | †                | ...            | ...  |
| J1628.3–3206  | 247.086 | −32.105 | 347.455 | 11.442  | 0.128      | 0.110      | −55    | 8.3      | 1.8      | 0.3             | 12.4     | 1.9             | 2.23          | ...                  | LP  | ... | ...      | 1FGL J1627.8–3204                                        | ... | psr              | PSR J1628–32   | ...  |
| J1629.4+8236  | 247.355 | 82.614  | 115.901 | 31.242  | 0.126      | 0.092      | −16    | 12.2     | 1.1      | 0.1             | 13.1     | 1.4             | 2.20          | 0.07                 | PL  | ... | 2        | 3EG J1621+8203                                           | ... | rdg              | NGC 6251       | ...  |
| J1629.6–6141  | 247.411 | −61.696 | 325.955 | −9.017  | 0.162      | 0.111      | 37     | 10.7     | 1.3      | 0.2             | 21.3     | 2.1             | 2.58          | 0.08                 | PL  | T   | ...      | 1FGL J1629.5–6147                                        | ... | bzq              | PMN J1629–6133 | ...  |
| J1630.1–4615  | 247.540 | −46.258 | 337.289 | 1.508   | 0.137      | 0.128      | −18    | 11.3     | 3.0      | 0.7             | 49.1     | 5.2             | 2.50          | ...                  | LP  | ... | 1        | ...                                                      | ... | ...              | ...            | ...  |
| J1630.2–4752  | 247.565 | −47.874 | 336.127 | 0.385   | 0.073      | 0.066      | 80     | 5.1      | 3.1      | 0.9             | 35.8     | 8.4             | 1.89          | 0.17                 | PL  | ... | 2        | ...                                                      | E   | ...              | ...            | ...  |
| J1630.3+3732  | 247.596 | 37.549  | 60.201  | 43.257  | 0.085      | 0.077      | −26    | 10.4     | 1.2      | 0.2             | 5.2      | 0.8             | 2.23          | ...                  | LP  | ... | 12       | 1FGL J1630.5+3735                                        | ... | ...              | ...            | ...  |
| J1630.4+5218  | 247.613 | 52.303  | 80.344  | 42.443  | 0.087      | 0.070      | 37     | 10.8     | 1.0      | 0.1             | 10.6     | 1.5             | 2.03          | 0.10                 | PL  | ... | ...      | 1FGL J1630.2+5220                                        | ... | bzb              | TXS 1629+524   | ...  |
| J1631.0–1050  | 247.754 | −10.844 | 5.057   | 24.638  | 0.219      | 0.191      | 55     | 4.4      | 0.8      | 0.2             | 10.0     | 2.1             | 2.38          | 0.14                 | PL  | ... | ...      | 1FGL J1630.3–1042<br>3EG J1631–1018                      | ... | ...              | ...            | ...  |
| J1631.6–2819  | 247.907 | −28.320 | 350.823 | 13.446  | 0.271      | 0.221      | 24     | 4.6      | 0.7      | 0.2             | 12.9     | 2.5             | 2.66          | 0.13                 | PL  | ... | ...      | ...                                                      | ... | ...              | ...            | ...  |
| J1631.7–4720c | 247.926 | −47.345 | 336.679 | 0.570   | 0.100      | 0.083      | 70     | 8.4      | 6.2      | 0.8             | 70.7     | 9.2             | 2.21          | 0.07                 | PL  | ... | 5,6,10   | ...                                                      | ... | †                | ...            | ...  |

Table 1—Continued

| Name 2FGL     | R.A.    | Decl.   | $l$     | $b$    | $\theta_1$ | $\theta_2$ | $\phi$ | $\sigma$ | $F_{35}$ | $\Delta F_{35}$ | $S_{25}$ | $\Delta S_{25}$ | $\Gamma_{25}$ | $\Delta \Gamma_{25}$ | Mod | Var | Flags | $\gamma$ -ray Assoc.                                     | TeV | Class | ID or Assoc.        | Ref. |
|---------------|---------|---------|---------|--------|------------|------------|--------|----------|----------|-----------------|----------|-----------------|---------------|----------------------|-----|-----|-------|----------------------------------------------------------|-----|-------|---------------------|------|
| J1632.4–4820c | 248.114 | –48.336 | 336.041 | –0.198 | 0.103      | 0.064      | 78     | 7.0      | 5.2      | 0.8             | 58.5     | 9.3             | 2.10          | 0.09                 | PL  | ... | 4,6   | ...                                                      | ... | psr   | PSR J1632–4818      | ...  |
| J1632.4–4753c | 248.114 | –47.891 | 336.366 | 0.105  | 0.064      | 0.059      | –48    | 8.8      | 8.2      | 1.1             | 90.9     | 12.5            | 2.05          | 0.08                 | PL  | ... | 2,6   | ...                                                      | E   | ...   | ...                 | ...  |
| J1632.6–2328c | 248.155 | –23.473 | 354.769 | 16.448 | 0.144      | 0.121      | 37     | 6.2      | 1.3      | 0.3             | 17.6     | 2.8             | 2.39          | 0.10                 | PL  | ... | 1,6   | ...                                                      | ... | ...   | ...                 | ...  |
| J1634.4–4743c | 248.615 | –47.733 | 336.711 | –0.034 | 0.060      | 0.057      | –58    | 8.1      | 7.9      | 1.4             | 52.7     | 10.2            | 1.93          | ...                  | LP  | ... | 5,6   | ...                                                      | ... | ...   | ...                 | ...  |
| J1635.2+3810  | 248.809 | 38.171  | 61.135  | 42.343 | 0.025      | 0.024      | 18     | 75.8     | 11.6     | 0.4             | 144.4    | 3.1             | 2.41          | ...                  | LP  | T   | ...   | 1FGL J1635.0+3808<br>0FGL J1635.2+3809<br>3EG J1635+3813 | ... | bzq   | 4C +38.41           | ...  |
| J1635.4–4717c | 248.850 | –47.297 | 337.140 | 0.143  | 0.112      | 0.070      | –15    | 7.7      | 6.7      | 1.1             | 73.9     | 11.8            | 2.06          | 0.10                 | PL  | ... | 5,6,8 | 1FGL J1635.7–4715c                                       | E   | †     | ...                 | ...  |
| J1636.3–4740c | 249.090 | –47.683 | 336.964 | –0.236 | 0.069      | 0.054      | 44     | 13.3     | 15.5     | 1.3             | 113.8    | 11.5            | 2.23          | ...                  | LP  | ... | 2,6   | 1FGL J1636.4–4737c                                       | ... | ...   | ...                 | ...  |
| J1636.6–0841  | 249.158 | –8.694  | 7.867   | 24.785 | 0.196      | 0.164      | –12    | 4.8      | 0.8      | 0.2             | 10.2     | 2.1             | 2.42          | 0.14                 | PL  | ... | ...   | ...                                                      | ... | ...   | ...                 | ...  |
| J1637.7+4714  | 249.434 | 47.244  | 73.376  | 41.884 | 0.076      | 0.063      | 30     | 21.8     | 1.8      | 0.2             | 24.3     | 1.5             | 2.41          | 0.06                 | PL  | T   | ...   | 1FGL J1637.9+4707                                        | ... | bzq   | 4C +47.44           | ...  |
| J1637.9–3451  | 249.477 | –34.866 | 346.725 | 8.113  | 0.087      | 0.078      | –31    | 5.7      | 0.8      | 0.2             | 11.3     | 2.9             | 1.65          | 0.18                 | PL  | ... | ...   | ...                                                      | ... | agu   | NVSS J163750–344915 | ...  |
| J1638.0–4703c | 249.512 | –47.053 | 337.623 | –0.026 | 0.063      | 0.051      | 49     | 13.6     | 14.6     | 1.2             | 112.8    | 12.2            | 2.26          | ...                  | LP  | ... | 5,6   | 3EG J1639–4702<br>1AGL J1639–4702                        | ... | ...   | ...                 | ...  |
| J1639.7–5504  | 249.941 | –55.070 | 331.808 | –5.561 | 0.098      | 0.086      | 53     | 5.9      | 0.8      | 0.2             | 17.5     | 2.8             | 2.79          | 0.14                 | PL  | ... | 1,4   | ...                                                      | ... | ...   | ...                 | ...  |
| J1639.8–5145  | 249.951 | –51.765 | 334.297 | –3.378 | 0.084      | 0.069      | 35     | 12.8     | 3.3      | 0.3             | 45.4     | 4.0             | 2.45          | 0.07                 | PL  | ... | ...   | 3EG J1638–5155<br>EGR J1638–5157                         | ... | ...   | ...                 | 43   |
| J1639.8–4921c | 249.964 | –49.363 | 336.101 | –1.790 | 0.179      | 0.130      | 18     | 4.4      | 2.1      | 0.4             | 25.1     | 6.0             | 2.29          | 0.14                 | PL  | ... | 6     | ...                                                      | ... | ...   | ...                 | ...  |
| J1640.5–4633  | 250.137 | –46.552 | 338.282 | –0.011 | 0.068      | 0.053      | 2      | 11.7     | 9.2      | 0.9             | 104.9    | 10.1            | 2.19          | 0.06                 | PL  | ... | 3     | 1FGL J1640.8–4634c<br>3EG J1639–4702<br>1AGL J1639–4702  | E   | †     | ...                 | ...  |
| J1640.7+3945  | 250.179 | 39.757  | 63.350  | 41.380 | 0.047      | 0.044      | –42    | 18.1     | 3.8      | 0.3             | 48.9     | 3.9             | 2.36          | 0.06                 | PL  | T   | ...   | 0FGL J1641.4+3939<br>EGR J1642+3940                      | ... | BZQ   | NRAO 512            | ...  |
| J1641.0+1141  | 250.250 | 11.697  | 28.759  | 34.201 | 0.142      | 0.115      | 50     | 4.3      | 0.5      | 0.1             | 5.3      | 1.5             | 2.03          | 0.22                 | PL  | ... | ...   | 1FGL J1641.0+1143                                        | ... | agn   | MG1 J164058+1144    | ...  |
| J1641.6–0614  | 250.412 | –6.249  | 10.866  | 25.152 | 0.103      | 0.098      | 54     | 6.1      | 1.1      | 0.2             | 14.4     | 2.8             | 2.37          | 0.13                 | PL  | ... | ...   | ...                                                      | ... | bzb   | TXS 1639–062        | ...  |
| J1641.8–5319  | 250.466 | –53.326 | 333.329 | –4.643 | 0.151      | 0.128      | 41     | 6.2      | 1.4      | 0.3             | 19.6     | 3.2             | 2.46          | 0.11                 | PL  | ... | ...   | ...                                                      | ... | ...   | ...                 | ...  |
| J1642.9+3949  | 250.748 | 39.829  | 63.480  | 40.947 | 0.054      | 0.049      | 33     | 16.5     | 3.4      | 0.3             | 49.3     | 3.9             | 2.49          | 0.06                 | PL  | T   | 5     | EGR J1642+3940                                           | ... | BZQ   | 3C 345              | ...  |
| J1643.3–4928  | 250.846 | –49.468 | 336.401 | –2.290 | 0.203      | 0.138      | –26    | 5.9      | 2.6      | 0.4             | 33.4     | 6.4             | 2.38          | 0.10                 | PL  | ... | ...   | ...                                                      | ... | ...   | ...                 | ...  |
| J1643.5–0641  | 250.884 | –6.694  | 10.748  | 24.515 | 0.106      | 0.090      | 10     | 5.9      | 1.2      | 0.2             | 13.3     | 2.7             | 2.14          | 0.16                 | PL  | ... | 5     | 1FGL J1643.5–0646                                        | ... | bzb   | NVSS J164328–064619 | ...  |
| J1645.7–2148c | 251.438 | –21.816 | 358.093 | 15.147 | 0.222      | 0.147      | 89     | 7.3      | 1.5      | 0.3             | 12.6     | 2.0             | 2.34          | ...                  | LP  | ... | 6     | 1FGL J1645.0–2155c                                       | ... | ...   | ...                 | ...  |
| J1646.7–1333  | 251.682 | –13.551 | 5.160   | 19.942 | 0.119      | 0.104      | –58    | 4.3      | 0.5      | 0.2             | 6.9      | 2.2             | 1.75          | 0.25                 | PL  | ... | ...   | ...                                                      | ... | ...   | ...                 | ...  |
| J1647.0+4351  | 251.769 | 43.858  | 68.824  | 40.340 | 0.180      | 0.144      | 89     | 4.4      | 0.3      | 0.1             | 4.5      | 1.0             | 2.47          | 0.19                 | PL  | ... | ...   | ...                                                      | ... | ...   | ...                 | ...  |
| J1647.5+4950  | 251.881 | 49.840  | 76.655  | 40.085 | 0.084      | 0.081      | 35     | 16.2     | 1.2      | 0.1             | 17.3     | 1.3             | 2.48          | 0.07                 | PL  | T   | ...   | 1FGL J1647.4+4948                                        | ... | agn   | SBS 1646+499        | ...  |
| J1648.1–4930  | 252.046 | –49.505 | 336.880 | –2.907 | 0.161      | 0.093      | –74    | 4.6      | 1.5      | 0.4             | 16.1     | 4.1             | 2.07          | 0.17                 | PL  | ... | 4,5   | ...                                                      | ... | ...   | ...                 | ...  |
| J1648.4–4612  | 252.104 | –46.200 | 339.434 | –0.809 | 0.069      | 0.048      | –44    | 9.8      | 8.0      | 1.0             | 55.9     | 8.7             | 2.11          | ...                  | EC  | ... | 5     | 1FGL J1648.4–4609c                                       | E   | PSR   | PSR J1648–4611      | ...  |

Table 1—Continued

| Name 2FGL     | R.A.    | Decl.   | $l$     | $b$     | $\theta_1$ | $\theta_2$ | $\phi$ | $\sigma$ | $F_{35}$ | $\Delta F_{35}$ | $S_{25}$ | $\Delta S_{25}$ | $\Gamma_{25}$ | $\Delta \Gamma_{25}$ | Mod | Var | Flags        | $\gamma$ -ray Assoc. | TeV | Class | ID or Assoc.          |
|---------------|---------|---------|---------|---------|------------|------------|--------|----------|----------|-----------------|----------|-----------------|---------------|----------------------|-----|-----|--------------|----------------------|-----|-------|-----------------------|
| J1649.2–3004  | 252.305 | –30.070 | 351.989 | 9.385   | 0.186      | 0.119      | 55     | 5.2      | 1.1      | 0.2             | 12.5     | 2.7             | 1.94          | 0.13                 | PL  | ... | ...          | 0FGL J1648.1–4606    | ... | ...   | ...                   |
| J1649.6+5238  | 252.420 | 52.646  | 80.253  | 39.497  | 0.109      | 0.099      | 56     | 7.9      | 0.7      | 0.1             | 7.9      | 1.2             | 2.26          | 0.12                 | PL  | ... | ...          | 1FGL J1649.6+5241    | ... | bzb   | 87GB 164812.2+524023  |
| J1650.1–5044  | 252.540 | –50.744 | 336.130 | –3.944  | 0.038      | 0.034      | –83    | 24.0     | 7.0      | 0.4             | 81.1     | 4.4             | 2.24          | 0.04                 | PL  | T   | ...          | 1FGL J1650.4–5042    | ... | agu   | PMN J1650–5044        |
| J1650.6–4603c | 252.652 | –46.055 | 339.790 | –1.006  | 0.057      | 0.051      | –39    | 11.8     | 11.1     | 1.0             | 74.0     | 8.4             | 2.13          | ...                  | LP  | ... | 6            | 1FGL J1651.5–4602c   | E   | ...   | ...                   |
| J1650.8+0830  | 252.708 | 8.508   | 26.604  | 30.635  | 0.180      | 0.158      | 37     | 7.3      | 0.7      | 0.1             | 11.8     | 1.6             | 2.59          | 0.12                 | PL  | T   | ...          | EGR J1652–4552       | ... | bzq   | MG1 J165034+0824      |
| J1651.8–4439c | 252.957 | –44.658 | 341.003 | –0.281  | 0.236      | 0.146      | 88     | 6.5      | 3.4      | 0.7             | 42.8     | 6.2             | 2.19          | ...                  | LP  | ... | 3,4,6,8,9,12 | ...                  | ... | ...   | ...                   |
| J1652.5–4351c | 253.131 | –43.854 | 341.702 | 0.134   | 0.090      | 0.080      | –79    | 7.8      | 7.0      | 0.9             | 37.0     | 5.9             | 2.12          | ...                  | LP  | ... | 3,4,6        | 1FGL J1652.8–4350c   | ... | ...   | ...                   |
| J1653.6–0159  | 253.402 | –1.996  | 16.593  | 24.931  | 0.060      | 0.055      | 67     | 22.5     | 4.2      | 0.3             | 34.3     | 2.5             | 2.24          | ...                  | LP  | ... | ...          | 1FGL J1653.6–0158    | ... | ...   | ...                   |
| J1653.9+3945  | 253.481 | 39.763  | 63.605  | 38.849  | 0.019      | 0.019      | –63    | 54.8     | 8.8      | 0.3             | 114.4    | 6.3             | 1.74          | 0.03                 | PL  | T   | ...          | 0FGL J1653.4–0200    | ... | ...   | ...                   |
| J1653.9–4627c | 253.492 | –46.462 | 339.844 | –1.714  | 0.106      | 0.092      | –74    | 6.5      | 3.2      | 0.6             | 35.3     | 6.2             | 2.04          | 0.10                 | PL  | ... | 6            | 3EG J1652–0223       | ... | ...   | ...                   |
| J1656.1–3256  | 254.049 | –32.940 | 350.665 | 6.431   | 0.192      | 0.184      | 73     | 8.5      | 1.0      | 0.2             | 24.9     | 2.9             | 2.86          | 0.10                 | PL  | T   | ...          | 1FGL J1653.9+3945    | P   | BZB   | Mkn 501               |
| J1656.4–0738  | 254.124 | –7.648  | 11.811  | 21.308  | 0.129      | 0.120      | –83    | 4.7      | 0.8      | 0.2             | 10.8     | 2.2             | 2.48          | 0.16                 | PL  | ... | 4            | 0FGL J1653.9+3946    | ... | ...   | ...                   |
| J1656.5+6012  | 254.126 | 60.201  | 89.631  | 37.468  | 0.140      | 0.128      | 79     | 4.9      | 0.4      | 0.1             | 4.5      | 1.0             | 2.36          | 0.21                 | PL  | ... | 4            | 3EG J1655–4554       | ... | ...   | ...                   |
| J1656.9–2008  | 254.233 | –20.150 | 1.095   | 14.077  | 0.101      | 0.081      | 35     | 6.6      | 1.1      | 0.2             | 13.5     | 2.9             | 1.79          | 0.14                 | PL  | ... | ...          | 1FGL J1656.2–3257    | ... | bzq   | Swift J1656.3–3302    |
| J1657.1–1027  | 254.280 | –10.454 | 9.404   | 19.630  | 0.239      | 0.159      | 10     | 5.7      | 1.0      | 0.2             | 13.3     | 2.3             | 2.42          | 0.12                 | PL  | ... | ...          | 1FGL J1656.9+6017    | ... | agu   | 1RXS J165604.4+601702 |
| J1657.5–4652  | 254.391 | –46.875 | 339.909 | –2.453  | 0.097      | 0.080      | –4     | 7.3      | 3.1      | 0.5             | 35.5     | 5.9             | 2.23          | 0.09                 | PL  | ... | 4            | 1FGL J1656.9–1033    | ... | agu   | PMN J1657–1021        |
| J1657.9+4809  | 254.482 | 48.161  | 74.392  | 38.453  | 0.095      | 0.084      | –62    | 15.2     | 1.2      | 0.1             | 16.6     | 1.3             | 2.47          | 0.07                 | PL  | T   | ...          | ...                  | ... | ...   | ...                   |
| J1658.1–4743  | 254.540 | –47.733 | 339.298 | –3.065  | 0.110      | 0.093      | –4     | 6.1      | 2.2      | 0.4             | 28.6     | 5.0             | 2.38          | 0.10                 | PL  | ... | 4            | ...                  | ... | bzq   | 4C +48.41             |
| J1658.4–5322  | 254.617 | –53.368 | 334.879 | –6.583  | 0.089      | 0.074      | 18     | 15.4     | 2.9      | 0.3             | 29.3     | 2.5             | 2.45          | ...                  | EC  | ... | ...          | 1FGL J1658.8–5317    | ... | PSR   | PSR J1658–5324        |
| J1659.2–0142  | 254.823 | –1.715  | 17.661  | 23.859  | 0.126      | 0.116      | –52    | 5.7      | 1.0      | 0.2             | 10.7     | 2.2             | 2.05          | 0.14                 | PL  | ... | ...          | ...                  | ... | ...   | ...                   |
| J1700.2+6831  | 255.062 | 68.517  | 99.578  | 35.191  | 0.042      | 0.040      | 69     | 37.9     | 3.8      | 0.2             | 50.0     | 1.9             | 2.40          | 0.03                 | PL  | T   | ...          | 1FGL J1700.1+6830    | ... | bzq   | TXS 1700+685          |
| J1700.8–4912  | 255.221 | –49.211 | 338.410 | –4.332  | 0.183      | 0.150      | 21     | 4.3      | 1.2      | 0.3             | 16.1     | 3.6             | 2.41          | 0.13                 | PL  | ... | 4            | ...                  | ... | ...   | ...                   |
| J1701.2–3007  | 255.314 | –30.122 | 353.573 | 7.306   | 0.064      | 0.057      | 30     | 13.5     | 2.9      | 0.3             | 33.3     | 3.0             | 2.24          | 0.06                 | PL  | ... | ...          | 1FGL J1701.1–3005    | ... | glc   | NGC 6266              |
| J1702.5–5654  | 255.639 | –56.915 | 332.388 | –9.197  | 0.073      | 0.069      | –61    | 21.0     | 3.3      | 0.3             | 34.8     | 2.4             | 2.39          | ...                  | LP  | ... | ...          | 1FGL J1702.4–5653    | ... | ...   | ...                   |
| J1703.2–6217  | 255.802 | –62.296 | 328.019 | –12.445 | 0.067      | 0.062      | 52     | 24.7     | 3.3      | 0.3             | 44.8     | 2.3             | 2.43          | 0.04                 | PL  | T   | ...          | 1FGL J1702.7–6217    | ... | bzq   | CGRaBS J1703–6212     |
| J1704.3+1235  | 256.082 | 12.597  | 32.512  | 29.391  | 0.110      | 0.098      | –11    | 5.3      | 0.6      | 0.1             | 6.7      | 1.5             | 2.19          | 0.17                 | PL  | ... | ...          | 3EG J1659–6251       | ... | ...   | ...                   |
| J1704.6–0529  | 256.162 | –5.496  | 14.920  | 20.753  | 0.108      | 0.091      | –8     | 7.9      | 1.4      | 0.2             | 17.1     | 2.4             | 2.35          | 0.10                 | PL  | ... | ...          | ...                  | ... | ...   | ...                   |
| J1704.9–4618  | 256.248 | –46.304 | 341.143 | –3.111  | 0.258      | 0.179      | –75    | 9.3      | 1.5      | 0.3             | 33.3     | 3.9             | 4.59          | ...                  | LP  | ... | 1,4,8,12     | ...                  | ... | ...   | ...                   |
| J1708.4+1003c | 257.101 | 10.056  | 30.368  | 27.416  | 0.142      | 0.125      | 86     | 4.7      | 0.4      | 0.1             | 8.0      | 1.6             | 2.65          | 0.16                 | PL  | ... | 6            | ...                  | ... | ...   | ...                   |

Table 1—Continued

| Name 2FGL     | R.A.    | Decl.   | $l$     | $b$     | $\theta_1$ | $\theta_2$ | $\phi$ | $\sigma$ | $F_{35}$ | $\Delta F_{35}$ | $S_{25}$ | $\Delta S_{25}$ | $\Gamma_{25}$ | $\Delta \Gamma_{25}$ | Mod | Var | Flags | $\gamma$ -ray Assoc.                                                                          | TeV | Class | ID or Assoc.   | Ref. |
|---------------|---------|---------|---------|---------|------------|------------|--------|----------|----------|-----------------|----------|-----------------|---------------|----------------------|-----|-----|-------|-----------------------------------------------------------------------------------------------|-----|-------|----------------|------|
| J1709.0–0821  | 257.253 | –8.356  | 12.957  | 18.318  | 0.230      | 0.192      | –45    | 5.4      | 1.0      | 0.2             | 14.2     | 2.5             | 2.47          | 0.11                 | PL  | ... | ...   | 3EG J1709–0828                                                                                | ... | ...   | ...            | ...  |
| J1709.7–4429  | 257.433 | –44.485 | 343.101 | –2.689  | 0.008      | 0.008      | –25    | 256.8    | 191.4    | 1.7             | 1351.0   | 10.7            | 2.03          | ...                  | EC  | T   | ...   | 1FGL J1709.7–4429<br>0FGL J1709.7–4428<br>3EG J1710–4439<br>EGR J1710–4435<br>1AGL J1709–4428 | E   | PSR   | PSR J1709–4429 | ...  |
| J1709.7+4319  | 257.449 | 43.322  | 68.406  | 36.205  | 0.054      | 0.052      | –43    | 23.6     | 2.2      | 0.2             | 27.2     | 1.7             | 2.31          | 0.05                 | PL  | T   | ...   | 1FGL J1709.6+4320                                                                             | ... | bzq   | B3 1708+433    | ...  |
| J1710.0–0323  | 257.523 | –3.393  | 17.594  | 20.683  | 0.256      | 0.193      | 23     | 6.9      | 1.0      | 0.2             | 15.9     | 2.3             | 2.56          | 0.11                 | PL  | ... | ...   | ...                                                                                           | ... | ...   | ...            | ...  |
| J1710.5–5020  | 257.635 | –50.342 | 338.440 | –6.257  | 0.160      | 0.112      | 10     | 8.3      | 0.7      | 0.2             | 16.8     | 2.1             | 2.46          | ...                  | LP  | ... | 12    | ...                                                                                           | ... | ...   | ...            | ...  |
| J1712.4–3941  | 258.111 | –39.687 | 347.269 | –0.257  | 0.121      | 0.107      | 65     | 5.1      | 2.3      | 0.6             | 29.3     | 6.3             | 1.75          | 0.17                 | PL  | ... | ...   | 1FGL J1711.7–3944c                                                                            | E   | †     | ...            | ...  |
| J1714.0+0751  | 258.501 | 7.863   | 28.841  | 25.213  | 0.122      | 0.105      | 77     | 8.5      | 1.4      | 0.2             | 9.4      | 1.6             | 2.21          | ...                  | EC  | ... | ...   | 1FGL J1713.9+0750                                                                             | ... | PSR   | PSR J1713+0747 | ...  |
| J1714.5–3829  | 258.630 | –38.492 | 348.473 | 0.118   | 0.045      | 0.038      | –28    | 19.2     | 14.7     | 0.9             | 107.3    | 8.0             | 2.13          | ...                  | LP  | ... | ...   | 1FGL J1714.5–3830c<br>0FGL J1714.7–3827<br>3EG J1714–3857                                     | E   | †     | ...            | ...  |
| J1714.8+6836  | 258.719 | 68.616  | 99.308  | 33.870  | 0.123      | 0.100      | 78     | 12.0     | 1.2      | 0.2             | 7.8      | 1.1             | 2.29          | ...                  | LP  | T   | ...   | ...                                                                                           | ... | bzq   | S4 1716+68     | ...  |
| J1715.4–4024c | 258.873 | –40.401 | 347.031 | –1.147  | 0.088      | 0.069      | 54     | 7.5      | 3.3      | 0.5             | 36.9     | 5.5             | 2.13          | 0.10                 | PL  | ... | 6     | ...                                                                                           | E   | agu   | PMN J1715–4025 | ...  |
| J1716.6–0526c | 259.171 | –5.441  | 16.621  | 18.223  | 0.194      | 0.147      | 64     | 6.8      | 0.5      | 0.1             | 13.1     | 1.9             | 2.44          | ...                  | LP  | ... | 6,12  | ...                                                                                           | ... | ...   | ...            | ...  |
| J1717.3–2809  | 259.345 | –28.161 | 357.255 | 5.615   | 0.186      | 0.120      | –11    | 5.1      | 1.2      | 0.3             | 17.4     | 3.2             | 2.45          | 0.13                 | PL  | ... | 2,4   | 3EG J1717–2737                                                                                | ... | ...   | ...            | ...  |
| J1717.5–5802  | 259.383 | –58.035 | 332.635 | –11.487 | 0.151      | 0.129      | –42    | 7.0      | 0.9      | 0.2             | 13.2     | 2.0             | 2.50          | 0.12                 | PL  | ... | ...   | ...                                                                                           | ... | psr   | PSR J1717–5800 | ...  |
| J1717.7–3342  | 259.441 | –33.717 | 352.744 | 2.356   | 0.051      | 0.047      | –55    | 24.2     | 8.7      | 0.6             | 92.9     | 4.8             | 2.39          | ...                  | LP  | T   | ...   | 1FGL J1717.9–3343<br>3EG J1718–3313                                                           | ... | bzb   | TXS 1714–336   | ...  |
| J1718.1–3725  | 259.537 | –37.428 | 349.755 | 0.153   | 0.073      | 0.055      | 13     | 6.0      | 3.3      | 0.6             | 36.5     | 6.7             | 1.98          | 0.11                 | PL  | ... | 3     | 1FGL J1717.9–3729c                                                                            | ... | †     | ...            | ...  |
| J1718.3–3827  | 259.585 | –38.454 | 348.938 | –0.469  | 0.064      | 0.054      | –11    | 16.0     | 11.2     | 0.8             | 88.4     | 7.3             | 2.31          | ...                  | EC  | T   | ...   | 1FGL J1718.2–3825                                                                             | E   | PSR   | PSR J1718–3825 | ...  |
| J1718.4–3056  | 259.606 | –30.948 | 355.093 | 3.833   | 0.112      | 0.087      | –49    | 5.4      | 1.5      | 0.3             | 17.9     | 3.6             | 2.24          | 0.12                 | PL  | ... | ...   | ...                                                                                           | ... | agu   | PMN J1718–3056 | ...  |
| J1719.3+1744  | 259.830 | 17.743  | 39.526  | 28.071  | 0.047      | 0.043      | 85     | 17.6     | 2.2      | 0.2             | 26.7     | 3.0             | 1.84          | 0.06                 | PL  | T   | ...   | 1FGL J1719.2+1745<br>0FGL J1719.3+1746                                                        | ... | bzb   | PKS 1717+177   | ...  |
| J1721.0+0711  | 260.257 | 7.194   | 29.034  | 23.357  | 0.138      | 0.120      | 25     | 7.3      | 1.0      | 0.2             | 13.1     | 2.0             | 2.36          | 0.11                 | PL  | ... | ...   | 1FGL J1721.1+0713                                                                             | ... | ...   | ...            | ...  |
| J1721.5–0718c | 260.383 | –7.301  | 15.602  | 16.232  | 0.136      | 0.122      | –79    | 6.0      | 1.0      | 0.3             | 10.6     | 2.0             | 2.26          | ...                  | LP  | ... | 1,4,6 | ...                                                                                           | ... | ...   | ...            | ...  |
| J1722.5–0420  | 260.645 | –4.344  | 18.399  | 17.516  | 0.137      | 0.110      | 47     | 9.0      | 1.9      | 0.3             | 16.8     | 2.2             | 2.27          | ...                  | LP  | ... | ...   | 1FGL J1722.4–0421                                                                             | ... | ...   | ...            | ...  |
| J1722.7+1013  | 260.682 | 10.230  | 32.221  | 24.305  | 0.056      | 0.049      | 40     | 15.7     | 2.3      | 0.2             | 26.6     | 2.3             | 2.23          | 0.06                 | PL  | T   | ...   | 1FGL J1722.5+1012                                                                             | ... | bzq   | TXS 1720+102   | ...  |
| J1724.0+4003  | 261.008 | 40.061  | 64.875  | 33.161  | 0.069      | 0.062      | –3     | 21.0     | 2.1      | 0.2             | 25.8     | 1.7             | 2.34          | 0.06                 | PL  | T   | ...   | 1FGL J1724.0+4002                                                                             | ... | bzq   | S4 1722+40     | ...  |
| J1724.9–0508c | 261.244 | –5.145  | 17.989  | 16.597  | 0.113      | 0.094      | 86     | 4.4      | 0.9      | 0.2             | 10.1     | 2.6             | 2.01          | 0.16                 | PL  | ... | 4,5,6 | 1FGL J1725.2–0509                                                                             | ... | ...   | ...            | ...  |
| J1725.0+1151  | 261.268 | 11.865  | 34.115  | 24.472  | 0.039      | 0.037      | 56     | 21.9     | 3.7      | 0.3             | 42.3     | 3.5             | 1.93          | 0.06                 | PL  | ... | ...   | 1FGL J1725.0+1151                                                                             | ... | bzb   | 1H 1720+117    | ...  |
| J1725.1–7714  | 261.277 | –77.248 | 315.710 | –21.869 | 0.171      | 0.139      | –88    | 7.2      | 0.8      | 0.2             | 12.7     | 1.8             | 2.57          | 0.11                 | PL  | T   | ...   | ...                                                                                           | ... | agu   | PKS 1716–771   | ...  |
| J1725.2+5853  | 261.301 | 58.891  | 87.503  | 34.012  | 0.132      | 0.118      | 72     | 6.4      | 0.5      | 0.1             | 6.2      | 1.1             | 2.26          | 0.17                 | PL  | T   | ...   | 1FGL J1725.5+5854                                                                             | ... | bzb   | 7C 1724+5854   | ...  |

Table 1—Continued

| Name 2FGL     | R.A.    | Decl.   | $l$     | $b$    | $\theta_1$ | $\theta_2$ | $\phi$ | $\sigma$ | $F_{35}$ | $\Delta F_{35}$ | $S_{25}$ | $\Delta S_{25}$ | $\Gamma_{25}$ | $\Delta \Gamma_{25}$ | Mod | Var | Flags     | $\gamma$ -ray Assoc. | TeV | Class | ID or Assoc.        | Ref. |
|---------------|---------|---------|---------|--------|------------|------------|--------|----------|----------|-----------------|----------|-----------------|---------------|----------------------|-----|-----|-----------|----------------------|-----|-------|---------------------|------|
| J1726.6–3545  | 261.670 | –35.764 | 352.096 | –0.314 | 0.158      | 0.110      | 23     | 8.4      | 4.4      | 0.9             | 42.2     | 5.4             | 2.29          | ...                  | LP  | ... | 1,4       | ...                  | ... | ...   | ...                 | ...  |
| J1727.1+4531  | 261.785 | 45.524  | 71.441  | 33.338 | 0.077      | 0.072      | 25     | 21.5     | 1.5      | 0.2             | 25.1     | 1.5             | 2.58          | 0.06                 | PL  | T   | ...       | 1FGL J1727.3+4525    | ... | bzq   | S4 1726+45          | ...  |
| J1727.1–0704  | 261.797 | –7.080  | 16.546  | 15.142 | 0.192      | 0.156      | 11     | 4.1      | 1.0      | 0.2             | 11.9     | 2.7             | 2.23          | 0.13                 | PL  | ... | ...       | ...                  | ... | glc   | IC 1257             | ...  |
| J1727.3–4611  | 261.842 | –46.189 | 343.476 | –6.205 | 0.223      | 0.151      | –23    | 4.1      | 0.9      | 0.2             | 12.0     | 2.6             | 2.45          | 0.13                 | PL  | ... | 4         | ...                  | ... | †     | ...                 | ...  |
| J1727.6+0647  | 261.918 | 6.794   | 29.443  | 21.703 | 0.178      | 0.162      | 58     | 4.8      | 0.6      | 0.2             | 9.2      | 1.9             | 2.52          | 0.14                 | PL  | ... | 4,8       | ...                  | ... | ...   | ...                 | ...  |
| J1727.8–2308  | 261.960 | –23.145 | 2.761   | 6.471  | 0.084      | 0.072      | 35     | 5.8      | 1.5      | 0.3             | 18.4     | 3.4             | 2.30          | 0.11                 | PL  | ... | 4         | ...                  | ... | ...   | ...                 | ...  |
| J1727.9+1220  | 261.982 | 12.346  | 34.912  | 24.037 | 0.144      | 0.121      | 33     | 4.4      | 0.7      | 0.2             | 7.8      | 2.0             | 2.09          | 0.20                 | PL  | T   | ...       | ...                  | ... | bzq   | PKS 1725+123        | ...  |
| J1728.0–2737c | 262.008 | –27.632 | 359.022 | 3.967  | 0.152      | 0.122      | 9      | 5.4      | 1.7      | 0.3             | 26.3     | 4.8             | 2.52          | 0.11                 | PL  | ... | 2,4,6     | ...                  | ... | ...   | ...                 | ...  |
| J1728.2+5015  | 262.061 | 50.261  | 77.117  | 33.550 | 0.069      | 0.065      | 23     | 9.0      | 0.8      | 0.1             | 9.7      | 1.9             | 1.83          | 0.13                 | PL  | ... | ...       | 1FGL J1727.9+5010    | ... | bzb   | I Zw 187            | ...  |
| J1728.2+0429  | 262.069 | 4.489   | 27.313  | 20.525 | 0.134      | 0.121      | 48     | 10.6     | 1.3      | 0.2             | 19.5     | 2.0             | 2.53          | 0.08                 | PL  | T   | ...       | 1FGL J1728.2+0431    | ... | bzq   | PKS 1725+044        | ...  |
|               |         |         |         |        |            |            |        |          |          |                 |          |                 |               |                      |     |     |           | 3EG J1727+0429       |     |       |                     |      |
|               |         |         |         |        |            |            |        |          |          |                 |          |                 |               |                      |     |     |           | EGR J1727+0416       |     |       |                     |      |
| J1729.5–0854  | 262.381 | –8.907  | 15.230  | 13.709 | 0.204      | 0.184      | 57     | 10.2     | 1.1      | 0.2             | 19.3     | 2.0             | 2.50          | ...                  | LP  | ... | 12        | ...                  | ... | ...   | ...                 | ...  |
| J1730.5–3350  | 262.636 | –33.844 | 354.134 | 0.090  | ...        | ...        | ...    | 6.1      | 1.7      | 0.6             | 36.6     | 5.5             | 2.35          | ...                  | EC  | ... | 2,4       | ...                  | ... | PSR   | PSR J1730–3350      | ...  |
| J1730.6–2409  | 262.654 | –24.161 | 2.254   | 5.384  | 0.155      | 0.091      | –90    | 8.7      | 3.0      | 0.4             | 20.8     | 3.0             | 2.25          | ...                  | LP  | ... | ...       | 1FGL J1730.4–2406    | ... | ...   | ...                 | ...  |
| J1730.6–0353  | 262.660 | –3.895  | 19.853  | 15.999 | 0.115      | 0.101      | 14     | 7.1      | 1.7      | 0.3             | 8.3      | 1.8             | 2.07          | ...                  | LP  | ... | ...       | 1FGL J1730.7–0352    | ... | ...   | ...                 | ...  |
| J1730.7+0023  | 262.685 | 0.395   | 23.786  | 18.064 | 0.060      | 0.057      | 14     | 14.1     | 2.2      | 0.2             | 27.3     | 2.4             | 2.31          | 0.07                 | PL  | T   | ...       | ...                  | ... | bzq   | PKS 1728+004        | ...  |
| J1730.8+5427  | 262.725 | 54.466  | 82.171  | 33.307 | 0.241      | 0.167      | –43    | 4.6      | 0.3      | 0.1             | 5.4      | 1.2             | 2.69          | 0.18                 | PL  | ... | ...       | ...                  | ... | ...   | ...                 | ...  |
| J1731.3+3718  | 262.826 | 37.302  | 61.982  | 31.255 | 0.243      | 0.178      | 4      | 5.3      | 0.6      | 0.1             | 6.6      | 1.4             | 2.09          | 0.14                 | PL  | ... | ...       | 1FGL J1730.8+3716    | ... | bzb   | GB6 J1730+3714      | ...  |
| J1731.6–3234c | 262.902 | –32.583 | 355.310 | 0.596  | 0.093      | 0.086      | 37     | 5.8      | 4.9      | 0.8             | 29.0     | 6.0             | 2.20          | ...                  | LP  | T   | 3,4,6     | ...                  | ... | †     | ...                 | ...  |
| J1731.8–3004  | 262.970 | –30.073 | 357.443 | 1.921  | 0.065      | 0.058      | –73    | 7.7      | 3.2      | 0.5             | 37.8     | 5.6             | 2.26          | 0.09                 | PL  | ... | ...       | 1FGL J1732.0–2957    | ... | agu   | NVSS J173146–300309 | ...  |
| J1731.9–2703c | 262.989 | –27.065 | 359.975 | 3.549  | 0.138      | 0.119      | –30    | 7.0      | 2.6      | 0.4             | 32.1     | 5.0             | 2.30          | 0.10                 | PL  | ... | 4,6       | ...                  | ... | ...   | ...                 | ...  |
| J1732.5–3131  | 263.135 | –31.519 | 356.309 | 1.013  | 0.021      | 0.021      | 73     | 45.9     | 37.2     | 1.1             | 211.6    | 7.5             | 2.10          | ...                  | EC  | ... | ...       | 1FGL J1732.5–3131    | ... | PSR   | LAT PSR J1732–3131  | ...  |
|               |         |         |         |        |            |            |        |          |          |                 |          |                 |               |                      |     |     |           | EGR J1732–3126       |     |       |                     |      |
| J1733.1–1307  | 263.279 | –13.128 | 12.001  | 10.772 | 0.078      | 0.070      | 41     | 18.4     | 3.1      | 0.3             | 41.0     | 2.8             | 2.49          | ...                  | LP  | T   | ...       | 1FGL J1733.0–1308    | ... | bzq   | PKS 1730–13         | ...  |
|               |         |         |         |        |            |            |        |          |          |                 |          |                 |               |                      |     |     |           | 3EG J1733–1313       |     |       |                     |      |
| J1733.2–2913c | 263.304 | –29.227 | 358.312 | 2.139  | 0.178      | 0.121      | 30     | 5.6      | 2.5      | 0.5             | 29.4     | 5.7             | 2.26          | 0.12                 | PL  | ... | 2,6       | ...                  | ... | ...   | ...                 | ...  |
| J1733.4–2812c | 263.359 | –28.203 | 359.197 | 2.655  | 0.149      | 0.114      | –62    | 6.2      | 2.3      | 0.4             | 30.6     | 5.5             | 2.39          | 0.11                 | PL  | ... | 1,4,5,6,8 | ...                  | ... | ...   | ...                 | ...  |
| J1734.3+3858  | 263.577 | 38.981  | 64.043  | 31.018 | 0.044      | 0.043      | –77    | 30.5     | 3.6      | 0.2             | 41.6     | 2.2             | 2.24          | 0.04                 | PL  | T   | ...       | 1FGL J1734.4+3859    | ... | bzq   | B2 1732+38A         | ...  |
| J1734.7–2533  | 263.687 | –25.561 | 1.583   | 3.837  | 0.153      | 0.135      | 46     | 10.4     | 1.8      | 0.3             | 32.9     | 3.4             | 2.44          | ...                  | LP  | T   | 2,12      | ...                  | ... | ...   | ...                 | ...  |
| J1735.9+2033  | 263.999 | 20.552  | 44.068  | 25.433 | 0.070      | 0.061      | 24     | 10.3     | 0.9      | 0.2             | 14.1     | 2.9             | 1.55          | 0.12                 | PL  | ... | ...       | 1FGL J1735.7+2031    | ... | bzb   | NVSS J173605+203301 | ...  |
| J1736.0–4443  | 264.011 | –44.722 | 345.545 | –6.694 | 0.075      | 0.066      | –28    | 9.7      | 2.0      | 0.3             | 23.0     | 2.7             | 2.24          | 0.08                 | PL  | ... | 3,10      | 1FGL J1735.9–4438    | ... | glc   | NGC 6388            | ...  |
| J1736.6+0626  | 264.164 | 6.435   | 30.165  | 19.547 | 0.204      | 0.178      | –4     | 6.8      | 0.7      | 0.2             | 13.2     | 1.9             | 2.66          | 0.12                 | PL  | T   | 4         | 1FGL J1736.3+0628    | ... | bzq   | MG1 J173624+0632    | ...  |
| J1737.2–3213  | 264.307 | –32.222 | 356.257 | –0.205 | 0.109      | 0.093      | 19     | 8.4      | 5.7      | 0.9             | 50.6     | 6.5             | 2.24          | ...                  | LP  | ... | 4,5       | 1AGL J1736–3235      | ... | †     | ...                 | ...  |
| J1738.9+8716  | 264.734 | 87.273  | 119.998 | 27.946 | 0.070      | 0.066      | –0     | 12.3     | 1.2      | 0.1             | 13.6     | 1.6             | 2.07          | 0.08                 | PL  | T   | ...       | 1FGL J1739.4+8717    | ... | ...   | ...                 | ...  |

Table 1—Continued

| Name 2FGL     | R.A.    | Decl.   | $l$     | $b$     | $\theta_1$ | $\theta_2$ | $\phi$ | $\sigma$ | $F_{35}$ | $\Delta F_{35}$ | $S_{25}$ | $\Delta S_{25}$ | $\Gamma_{25}$ | $\Delta \Gamma_{25}$ | Mod | Var | Flags    | $\gamma$ -ray Assoc.                                  | TeV | Class | ID or Assoc.          | Ref |
|---------------|---------|---------|---------|---------|------------|------------|--------|----------|----------|-----------------|----------|-----------------|---------------|----------------------|-----|-----|----------|-------------------------------------------------------|-----|-------|-----------------------|-----|
| J1738.9–2908  | 264.736 | –29.140 | 359.058 | 1.132   | 0.245      | 0.107      | 28     | 15.3     | 6.8      | 0.8             | 79.1     | 6.5             | 2.43          | ...                  | LP  | ... | 2,8,9    | 3EG J1736–2908                                        | ... | †     | ...                   | ... |
| J1739.5+4955  | 264.886 | 49.929  | 76.891  | 31.717  | 0.080      | 0.071      | 27     | 12.6     | 1.2      | 0.2             | 13.9     | 1.5             | 2.20          | 0.09                 | PL  | T   | ...      | EGR J1740+4946                                        | ... | bzq   | S4 1738+49            | ... |
| J1739.6–2726  | 264.916 | –27.434 | 0.587   | 1.906   | 0.199      | 0.113      | –30    | 15.2     | 5.6      | 0.7             | 56.6     | 5.0             | 2.40          | ...                  | LP  | ... | 2        | ...                                                   | ... | ...   | ...                   | ... |
| J1740.2+5212  | 265.060 | 52.201  | 79.566  | 31.806  | 0.063      | 0.059      | 32     | 30.8     | 2.5      | 0.2             | 37.4     | 1.7             | 2.50          | 0.04                 | PL  | T   | ...      | 1FGL J1740.0+5209<br>3EG J1738+5203<br>EGR J1740+5213 | ... | bzq   | 4C +51.37             | ... |
| J1740.3+4738  | 265.089 | 47.645  | 74.247  | 31.330  | 0.131      | 0.101      | 15     | 6.1      | 0.6      | 0.1             | 6.3      | 1.3             | 2.09          | 0.15                 | PL  | ... | ...      | ...                                                   | ... | bzq   | S4 1738+47            | ... |
| J1740.4–3054c | 265.105 | –30.911 | 357.728 | –0.081  | 0.164      | 0.100      | 5      | 11.0     | 9.5      | 0.9             | 70.2     | 7.8             | 2.26          | ...                  | LP  | ... | 6        | 1FGL J1740.3–3053c<br>0FGL J1741.4–3046               | ... | †     | ...                   | ... |
| J1741.0+1347  | 265.251 | 13.794  | 37.764  | 21.727  | 0.150      | 0.124      | 50     | 4.1      | 0.5      | 0.1             | 5.7      | 1.6             | 1.93          | 0.19                 | PL  | ... | ...      | ...                                                   | ... | ...   | ...                   | ... |
| J1741.1–6750  | 265.284 | –67.850 | 325.236 | –18.724 | 0.170      | 0.142      | 8      | 5.0      | 0.5      | 0.1             | 7.5      | 1.5             | 2.52          | 0.16                 | PL  | ... | ...      | ...                                                   | ... | ...   | ...                   | ... |
| J1741.9–2054  | 265.476 | –20.908 | 6.413   | 4.914   | 0.034      | 0.033      | 75     | 47.3     | 16.2     | 0.6             | 122.3    | 4.1             | 2.30          | ...                  | EC  | T   | ...      | 0FGL J1742.1–2054<br>3EG J1741–2050                   | ... | PSR   | LAT PSR J1741–2054    | ... |
| J1742.0–2540c | 265.508 | –25.673 | 2.363   | 2.388   | 0.120      | 0.095      | –71    | 6.1      | 2.3      | 0.4             | 26.6     | 4.6             | 2.20          | 0.09                 | PL  | ... | 3,4,6,10 | ...                                                   | ... | ...   | ...                   | ... |
| J1742.1+5948  | 265.528 | 59.808  | 88.526  | 31.834  | 0.094      | 0.082      | –20    | 6.7      | 0.5      | 0.1             | 6.1      | 1.1             | 2.23          | 0.17                 | PL  | ... | ...      | 1FGL J1742.1+5947                                     | ... | bzb   | RGB 1742+597          | ... |
| J1742.5–3323  | 265.642 | –33.396 | 355.858 | –1.779  | 0.144      | 0.101      | 24     | 10.5     | 5.0      | 0.6             | 35.7     | 5.2             | 2.37          | ...                  | LP  | ... | ...      | ...                                                   | ... | ...   | ...                   | ... |
| J1743.2–2304  | 265.800 | –23.072 | 4.720   | 3.526   | 0.188      | 0.108      | 41     | 7.2      | 2.0      | 0.3             | 27.2     | 3.9             | 2.43          | 0.09                 | PL  | T   | ...      | 3EG J1741–2312                                        | ... | ...   | ...                   | ... |
| J1743.9–3039c | 265.989 | –30.654 | 358.347 | –0.590  | 0.088      | 0.063      | 5      | 4.8      | 3.7      | 0.8             | 41.6     | 10.1            | 2.18          | 0.12                 | PL  | T   | 6        | 1AGL J1746–3017                                       | ... | ...   | ...                   | ... |
| J1744.1+1934  | 266.044 | 19.579  | 43.850  | 23.290  | 0.088      | 0.076      | –0     | 6.4      | 0.6      | 0.1             | 9.4      | 2.5             | 1.62          | 0.15                 | PL  | ... | ...      | 1FGL J1744.2+1934                                     | ... | bzb   | S3 1741+19            | ... |
| J1744.1–7620  | 266.046 | –76.342 | 317.092 | –22.476 | 0.056      | 0.052      | 88     | 20.8     | 3.8      | 0.3             | 20.0     | 1.9             | 2.08          | ...                  | LP  | ... | ...      | 1FGL J1743.8–7620                                     | ... | ...   | ...                   | ... |
| J1744.6–1135  | 266.153 | –11.587 | 14.805  | 9.151   | 0.068      | 0.060      | 72     | 18.1     | 4.8      | 0.4             | 35.6     | 2.7             | 2.29          | ...                  | EC  | ... | ...      | 1FGL J1744.4–1134                                     | ... | PSR   | PSR J1744–1134        | ... |
| J1745.1–1729  | 266.277 | –17.498 | 9.736   | 6.035   | 0.122      | 0.109      | –26    | 6.9      | 1.7      | 0.3             | 19.1     | 3.1             | 2.07          | 0.11                 | PL  | ... | ...      | ...                                                   | ... | agu   | 1RXS J174459.5–172640 | ... |
| J1745.5–0751  | 266.385 | –7.852  | 18.206  | 10.820  | 0.076      | 0.074      | –84    | 5.8      | 1.0      | 0.2             | 12.8     | 2.9             | 1.80          | 0.15                 | PL  | ... | ...      | 1FGL J1745.6–0751                                     | ... | bzb   | TXS 1742–078          | ... |
| J1745.5–3028c | 266.385 | –30.482 | 358.672 | –0.791  | 0.115      | 0.085      | –44    | 4.9      | 4.3      | 0.9             | 48.7     | 11.2            | 2.20          | 0.11                 | PL  | ... | 2,4,5,6  | 3EG J1744–3011<br>1AGL J1746–3017                     | E   | †     | ...                   | ... |
| J1745.6+1015  | 266.403 | 10.265  | 34.844  | 19.229  | 0.120      | 0.093      | –6     | 8.6      | 1.2      | 0.2             | 15.4     | 2.1             | 2.34          | 0.10                 | PL  | ... | ...      | 1FGL J1745.5+1018                                     | ... | psr   | PSR J1745+10          | ... |
| J1745.6+0203  | 266.414 | 2.066   | 27.158  | 15.559  | 0.204      | 0.174      | 3      | 4.2      | 0.8      | 0.2             | 9.8      | 2.2             | 2.32          | 0.14                 | PL  | ... | ...      | ...                                                   | ... | ...   | ...                   | ... |
| J1745.6–2858  | 266.423 | –28.979 | 359.973 | –0.036  | 0.016      | 0.016      | 27     | 43.1     | 77.4     | 2.0             | 575.6    | 17.6            | 2.15          | ...                  | LP  | ... | 2        | ...                                                   | ... | †     | ...                   | ... |
| J1746.0+2316  | 266.514 | 23.275  | 47.786  | 24.221  | 0.408      | 0.367      | 56     | 5.1      | 0.3      | 0.1             | 8.3      | 1.5             | 2.87          | 0.17                 | PL  | ... | 1,4      | ...                                                   | ... | bzq   | TXS 1742+228          | ... |
| J1746.5–3238  | 266.644 | –32.644 | 356.940 | –2.103  | 0.064      | 0.051      | –55    | 20.4     | 9.3      | 0.6             | 81.2     | 5.9             | 2.36          | ...                  | LP  | ... | ...      | 1FGL J1746.7–3233                                     | ... | ...   | ...                   | ... |
| J1746.6–2851c | 266.669 | –28.859 | 0.187   | –0.158  | 0.080      | 0.070      | –16    | 5.9      | 6.6      | 1.4             | 73.3     | 15.5            | 2.01          | 0.10                 | PL  | ... | 1,5,6    | 1FGL J1746.4–2849c<br>3EG J1746–2851                  | ... | ...   | ...                   | ... |
| J1747.1–3000  | 266.788 | –30.014 | 359.253 | –0.845  | 0.034      | 0.032      | –88    | 27.0     | 25.0     | 1.1             | 225.6    | 11.3            | 2.35          | ...                  | EC  | ... | 2        | 1AGL J1746–3017                                       | ... | PSR   | PSR J1747–2958        | ... |
| J1747.2–3507  | 266.818 | –35.125 | 354.888 | –3.509  | 0.179      | 0.142      | –73    | 5.9      | 1.4      | 0.3             | 23.4     | 3.8             | 2.61          | 0.12                 | PL  | ... | 4,8      | ...                                                   | ... | ...   | ...                   | ... |
| J1747.3–2825c | 266.850 | –28.431 | 0.634   | –0.071  | 0.058      | 0.052      | 61     | 10.6     | 14.3     | 1.4             | 69.3     | 9.0             | 2.15          | ...                  | LP  | ... | 5,6      | ...                                                   | ... | ...   | ...                   | ... |

Table 1—Continued

| Name 2FGL     | R.A.    | Decl.   | $l$     | $b$     | $\theta_1$ | $\theta_2$ | $\phi$ | $\sigma$ | $F_{35}$ | $\Delta F_{35}$ | $S_{25}$ | $\Delta S_{25}$ | $\Gamma_{25}$ | $\Delta \Gamma_{25}$ | Mod | Var | Flags | $\gamma$ -ray Assoc.                                  | TeV | Class | ID or Assoc.           | Ref. |
|---------------|---------|---------|---------|---------|------------|------------|--------|----------|----------|-----------------|----------|-----------------|---------------|----------------------|-----|-----|-------|-------------------------------------------------------|-----|-------|------------------------|------|
| J1747.5–4036  | 266.878 | –40.607 | 350.186 | –6.359  | 0.097      | 0.090      | 19     | 5.8      | 1.2      | 0.2             | 14.4     | 2.6             | 2.21          | 0.12                 | PL  | ... | ...   | 1FGL J1747.4–4035                                     | ... | psr   | PSR J1747–4036         | ...  |
| J1747.6+0324  | 266.923 | 3.403   | 28.634  | 15.724  | 0.145      | 0.116      | 82     | 5.8      | 1.0      | 0.2             | 12.0     | 2.2             | 2.23          | 0.12                 | PL  | ... | ...   | ...                                                   | ... | ...   | ...                    | ...  |
| J1748.0–2447  | 267.001 | –24.785 | 3.826   | 1.699   | 0.038      | 0.035      | –27    | 23.3     | 12.2     | 0.7             | 76.7     | 4.7             | 2.13          | ...                  | LP  | ... | 10    | 1FGL J1747.9–2448                                     | E   | glc   | Terzan 5               | ...  |
| J1748.6–2913  | 267.163 | –29.231 | 0.092   | –0.720  | 0.067      | 0.056      | 44     | 14.4     | 13.2     | 1.1             | 109.7    | 10.6            | 2.33          | ...                  | LP  | ... | 3,5   | 1FGL J1748.3–2916c                                    | ... | ...   | ...                    | ...  |
| J1748.7–2020  | 267.185 | –20.349 | 7.722   | 3.834   | 0.096      | 0.085      | 13     | 10.6     | 2.8      | 0.3             | 42.2     | 4.2             | 2.52          | 0.07                 | PL  | ... | ...   | 1FGL J1748.7–2020                                     | ... | glc   | NGC 6440               | ...  |
| J1748.8+3418  | 267.210 | 34.303  | 59.627  | 27.084  | 0.166      | 0.163      | –69    | 6.7      | 0.6      | 0.1             | 7.8      | 1.3             | 2.45          | 0.15                 | PL  | ... | ...   | ...                                                   | ... | ...   | ...                    | ...  |
| J1748.8+7006  | 267.217 | 70.111  | 100.539 | 30.692  | 0.051      | 0.050      | 34     | 20.8     | 2.1      | 0.2             | 23.7     | 1.9             | 2.04          | 0.06                 | PL  | ... | ...   | 1FGL J1748.5+7004                                     | ... | bzb   | S4 1749+70             | ...  |
| J1748.9–3923  | 267.240 | –39.388 | 351.384 | –5.979  | 0.126      | 0.110      | 56     | 4.3      | 1.1      | 0.2             | 11.9     | 2.7             | 2.15          | 0.16                 | PL  | ... | ...   | ...                                                   | ... | ...   | ...                    | ...  |
| J1749.1+0515  | 267.295 | 5.263   | 30.532  | 16.238  | 0.164      | 0.142      | –82    | 4.6      | 0.7      | 0.2             | 9.9      | 2.1             | 2.49          | 0.14                 | PL  | ... | 4,5   | ...                                                   | ... | ...   | ...                    | ...  |
| J1749.1+4323  | 267.297 | 43.392  | 69.671  | 29.128  | 0.072      | 0.067      | –59    | 13.5     | 1.3      | 0.2             | 15.0     | 1.6             | 2.22          | 0.08                 | PL  | ... | ...   | 1FGL J1749.0+4323                                     | ... | bzb   | B3 1747+433            | ...  |
| J1749.7–3134c | 267.435 | –31.577 | 358.200 | –2.127  | 0.132      | 0.114      | –11    | 4.7      | 2.1      | 0.4             | 27.7     | 5.6             | 2.42          | 0.11                 | PL  | ... | 4,5,6 | ...                                                   | ... | ...   | ...                    | ...  |
| J1751.5+0938  | 267.876 | 9.640   | 34.906  | 17.650  | 0.051      | 0.047      | –7     | 25.4     | 4.6      | 0.3             | 41.3     | 2.7             | 2.24          | ...                  | LP  | T   | ...   | 1FGL J1751.5+0937<br>0FGL J1751.5+0935                | ... | bzb   | OT 081                 | ...  |
| J1753.8–5012  | 268.453 | –50.204 | 342.269 | –12.041 | 0.114      | 0.097      | 14     | 12.1     | 1.5      | 0.2             | 18.8     | 2.0             | 2.44          | ...                  | LP  | T   | ...   | 1FGL J1754.0–5002                                     | ... | agu   | PMN J1753–5015         | ...  |
| J1753.8–4446  | 268.463 | –44.778 | 347.119 | –9.446  | 0.110      | 0.101      | 78     | 5.8      | 1.0      | 0.2             | 11.7     | 2.1             | 2.24          | 0.12                 | PL  | ... | ...   | ...                                                   | ... | ...   | ...                    | ...  |
| J1754.1–2930  | 268.537 | –29.509 | 0.464   | –1.891  | 0.173      | 0.095      | 12     | 9.1      | 3.6      | 0.5             | 38.3     | 5.3             | 2.45          | ...                  | LP  | T   | 2,4   | ...                                                   | ... | ...   | ...                    | ...  |
| J1754.3+3212  | 268.584 | 32.203  | 57.746  | 25.385  | 0.047      | 0.045      | 5      | 20.1     | 2.4      | 0.2             | 26.4     | 2.4             | 2.02          | 0.06                 | PL  | T   | ...   | 1FGL J1754.3+3212                                     | ... | bzb   | RX J1754.1+3212        | ...  |
| J1754.4–2538c | 268.617 | –25.646 | 3.833   | 0.002   | 0.108      | 0.090      | 87     | 4.3      | 4.1      | 0.9             | 16.9     | 4.2             | 1.93          | ...                  | LP  | ... | 2,4,6 | 1FGL J1754.5–2537c                                    | ... | ...   | ...                    | ...  |
| J1755.5–6423  | 268.892 | –64.391 | 329.194 | –18.563 | 0.215      | 0.162      | 60     | 4.5      | 0.5      | 0.1             | 6.5      | 1.5             | 2.48          | 0.16                 | PL  | ... | 4     | ...                                                   | ... | agu   | PMN J1754–6423         | ...  |
| J1756.5+5523  | 269.138 | 55.393  | 83.507  | 29.683  | 0.083      | 0.071      | –4     | 6.7      | 0.5      | 0.1             | 6.8      | 1.6             | 1.79          | 0.17                 | PL  | ... | ...   | 1FGL J1756.6+5524                                     | ... | bzb   | 1RXS J175615.5+552217  | ...  |
| J1757.5–6028  | 269.377 | –60.473 | 333.031 | –17.128 | 0.086      | 0.077      | 37     | 5.8      | 0.7      | 0.1             | 7.2      | 1.6             | 2.03          | 0.15                 | PL  | ... | ...   | ...                                                   | ... | ...   | ...                    | ...  |
| J1758.8–2402c | 269.714 | –24.045 | 5.717   | –0.055  | 0.118      | 0.085      | 81     | 8.5      | 8.5      | 1.0             | 53.1     | 7.2             | 2.00          | ...                  | LP  | T   | 3,5,6 | ...                                                   | E   | ...   | ...                    | ...  |
| J1759.2–3853  | 269.810 | –38.900 | 352.806 | –7.467  | 0.135      | 0.115      | –33    | 4.3      | 1.1      | 0.2             | 11.9     | 2.8             | 2.18          | 0.15                 | PL  | ... | ...   | EGR J1758–3923                                        | ... | ...   | ...                    | ...  |
| J1759.2–4819  | 269.824 | –48.319 | 344.400 | –11.951 | 0.103      | 0.072      | –10    | 9.0      | 1.4      | 0.2             | 15.8     | 2.1             | 2.18          | 0.10                 | PL  | T   | ...   | ...                                                   | ... | agu   | PMN J1758–4820         | ...  |
| J1759.4–2954  | 269.858 | –29.913 | 0.689   | –3.087  | 0.186      | 0.161      | 5      | 5.3      | 1.7      | 0.3             | 22.9     | 4.3             | 2.40          | 0.12                 | PL  | ... | ...   | ...                                                   | ... | ...   | ...                    | ...  |
| J1759.5–0521  | 269.893 | –5.354  | 22.142  | 8.991   | 0.127      | 0.110      | –85    | 4.7      | 1.0      | 0.3             | 16.3     | 3.3             | 2.57          | 0.14                 | PL  | ... | 4     | ...                                                   | ... | ...   | ...                    | ...  |
| J1800.5+7829  | 270.147 | 78.483  | 110.057 | 29.072  | 0.033      | 0.032      | 28     | 42.5     | 4.4      | 0.2             | 51.7     | 2.1             | 2.23          | 0.03                 | PL  | T   | ...   | 1FGL J1800.4+7827<br>0FGL J1802.2+7827                | ... | bzb   | S5 1803+784            | ...  |
| J1800.8–2400  | 270.203 | –24.011 | 5.969   | –0.426  | 0.069      | 0.054      | –15    | 8.8      | 6.2      | 0.9             | 71.4     | 9.7             | 1.90          | 0.08                 | PL  | ... | 3,5   | 1FGL J1800.5–2359c                                    | E   | ...   | ...                    | ...  |
| J1801.3–2326e | 270.340 | –23.440 | 6.527   | –0.251  | ...        | ...        | ...    | 49.3     | 59.0     | 1.5             | 424.6    | 11.1            | 2.12          | ...                  | LP  | ... | 10    | 0FGL J1801.6–2327<br>3EG J1800–2338<br>EGR J1800–2328 | ... | SNR   | SNR G006.4–00.1<br>W28 | 24   |
| J1801.7+4405  | 270.434 | 44.086  | 70.966  | 27.052  | 0.186      | 0.159      | 34     | 6.5      | 0.4      | 0.1             | 8.0      | 1.3             | 2.66          | 0.14                 | PL  | ... | ...   | ...                                                   | ... | bzq   | S4 1800+44             | ...  |
| J1802.3–2445c | 270.589 | –24.763 | 5.489   | –1.103  | 0.134      | 0.104      | 55     | 9.6      | 4.4      | 1.0             | 49.8     | 5.8             | 2.32          | ...                  | LP  | ... | 4,5,6 | ...                                                   | ... | †     | ...                    | ...  |
| J1802.6–3940  | 270.664 | –39.679 | 352.437 | –8.421  | 0.022      | 0.022      | 51     | 61.4     | 16.9     | 0.5             | 165.0    | 4.9             | 2.23          | ...                  | LP  | T   | ...   | 1FGL J1802.5–3939                                     | ... | bzq   | PMN J1802–3940         | ...  |



Table 1—Continued

| Name 2FGL     | R.A.    | Decl.   | $l$     | $b$     | $\theta_1$ | $\theta_2$ | $\phi$ | $\sigma$ | $F_{35}$ | $\Delta F_{35}$ | $S_{25}$ | $\Delta S_{25}$ | $\Gamma_{25}$ | $\Delta \Gamma_{25}$ | Mod | Var | Flags         | $\gamma$ -ray Assoc. | TeV | Class | ID or Assoc.         |
|---------------|---------|---------|---------|---------|------------|------------|--------|----------|----------|-----------------|----------|-----------------|---------------|----------------------|-----|-----|---------------|----------------------|-----|-------|----------------------|
|               |         |         |         |         |            |            |        |          |          |                 |          |                 |               |                      |     |     |               | 0FGL J1802.6–3939    |     |       |                      |
|               |         |         |         |         |            |            |        |          |          |                 |          |                 |               |                      |     |     |               | 3EG J1800–3955       |     |       |                      |
|               |         |         |         |         |            |            |        |          |          |                 |          |                 |               |                      |     |     |               | EGR J1758–3923       |     |       |                      |
| J1802.8–6706  | 270.710 | −67.108 | 326.855 | −20.317 | 0.173      | 0.132      | −7     | 4.3      | 0.5      | 0.1             | 5.9      | 1.4             | 2.25          | 0.17                 | PL  | ... | ...           | ...                  | ... | ...   | ...                  |
| J1803.3–2148  | 270.832 | −21.804 | 8.174   | 0.162   | 0.045      | 0.038      | 61     | 15.5     | 15.1     | 1.1             | 108.7    | 9.3             | 2.16          | ...                  | LP  | ... | 5             | 1FGL J1803.1–2147c   | ... | ...   | ...                  |
|               |         |         |         |         |            |            |        |          |          |                 |          |                 |               |                      |     |     |               | 1AGL J1805–2143      |     |       |                      |
| J1803.6+2523c | 270.907 | 25.396  | 51.471  | 21.227  | 0.331      | 0.255      | −30    | 5.7      | 0.4      | 0.1             | 9.4      | 1.5             | 2.83          | 0.15                 | PL  | T   | 4,6           | ...                  | ... | agu   | TXS 1801+253         |
| J1805.0–0845  | 271.270 | −8.752  | 19.796  | 6.161   | 0.111      | 0.103      | −13    | 5.9      | 1.5      | 0.3             | 18.6     | 3.3             | 2.31          | 0.11                 | PL  | ... | 4             | 1FGL J1807.0–0906    | ... | ...   | ...                  |
| J1805.6–2136e | 271.408 | −21.612 | 8.604   | −0.211  | ...        | ...        | ...    | 23.1     | 28.5     | 1.4             | 200.5    | 11.9            | 2.10          | ...                  | LP  | ... | ...           | 0FGL J1805.3–2138    | ... | SNR   | SNR G008.7–00.1      |
|               |         |         |         |         |            |            |        |          |          |                 |          |                 |               |                      |     |     |               | 1AGL J1805–2143      |     |       | W30                  |
| J1805.8+0612  | 271.464 | 6.213   | 33.330  | 12.954  | 0.112      | 0.083      | −41    | 7.9      | 1.3      | 0.2             | 14.5     | 2.2             | 2.11          | 0.10                 | PL  | ... | ...           | 1FGL J1806.2+0609    | ... | ...   | ...                  |
| J1806.7+6948  | 271.679 | 69.800  | 100.104 | 29.178  | 0.039      | 0.036      | 24     | 32.9     | 3.8      | 0.2             | 43.6     | 2.2             | 2.19          | 0.04                 | PL  | T   | ...           | 1FGL J1807.0+6945    | ... | bzb   | 3C 371               |
| J1807.7–0419  | 271.939 | −4.328  | 24.034  | 7.684   | 0.128      | 0.111      | −83    | 6.7      | 0.5      | 0.2             | 19.6     | 2.9             | 2.62          | ...                  | LP  | ... | 1,4,12        | ...                  | ... | ...   | ...                  |
| J1808.3–3356  | 272.092 | −33.935 | 358.084 | −6.696  | 0.130      | 0.103      | −70    | 6.8      | 1.4      | 0.2             | 17.2     | 2.6             | 2.31          | 0.10                 | PL  | ... | ...           | ...                  | ... | ...   | ...                  |
| J1808.5–2037c | 272.140 | −20.619 | 9.804   | −0.323  | 0.117      | 0.098      | −9     | 8.8      | 3.3      | 0.6             | 76.7     | 8.0             | 2.33          | ...                  | LP  | ... | 2,4,5,6,10,12 | ...                  | ... | ...   | ...                  |
| J1808.6–1950c | 272.154 | −19.850 | 10.483  | 0.038   | 0.078      | 0.074      | 52     | 7.8      | 7.1      | 0.9             | 53.6     | 8.2             | 2.18          | ...                  | LP  | ... | 4,6           | 1FGL J1808.5–1954c   | ... | glc   | 2MS-GC01             |
| J1809.4+2042  | 272.368 | 20.712  | 47.388  | 18.231  | 0.127      | 0.094      | 18     | 5.4      | 0.6      | 0.1             | 6.4      | 1.6             | 2.17          | 0.24                 | PL  | ... | 10            | ...                  | ... | agu   | RX J1809.3+2041      |
| J1809.7+2909  | 272.444 | 29.164  | 55.771  | 21.266  | 0.075      | 0.070      | 85     | 10.3     | 1.2      | 0.2             | 13.0     | 1.8             | 2.04          | 0.11                 | PL  | ... | ...           | 1FGL J1809.6+2908    | ... | bzb   | MG2 J180948+2910     |
| J1809.8–2332  | 272.468 | −23.546 | 7.389   | −2.006  | 0.013      | 0.013      | −0     | 99.9     | 69.0     | 1.2             | 493.3    | 8.7             | 2.13          | ...                  | EC  | ... | ...           | 1FGL J1809.8–2332    | ... | PSR   | LAT PSR J1809–2332   |
|               |         |         |         |         |            |            |        |          |          |                 |          |                 |               |                      |     |     |               | 3EG J1809–2328       |     |       |                      |
|               |         |         |         |         |            |            |        |          |          |                 |          |                 |               |                      |     |     |               | 1AGL J1809–2332      |     |       |                      |
| J1810.7+1742  | 272.691 | 17.703  | 44.618  | 16.759  | 0.082      | 0.072      | −46    | 18.3     | 2.5      | 0.2             | 25.5     | 2.1             | 2.41          | ...                  | LP  | ... | ...           | 1FGL J1810.3+1741    | ... | psr   | PSR J1810+17         |
| J1810.8+1606  | 272.720 | 16.102  | 43.105  | 16.081  | 0.103      | 0.095      | −7     | 7.2      | 1.1      | 0.2             | 12.1     | 2.0             | 2.13          | 0.12                 | PL  | ... | ...           | 1FGL J1811.0+1607    | ... | bzb   | 87GB 180835.5+160714 |
| J1811.0+5340  | 272.774 | 53.670  | 81.878  | 27.366  | 0.130      | 0.094      | −7     | 6.0      | 0.6      | 0.1             | 6.3      | 1.4             | 1.94          | 0.15                 | PL  | ... | ...           | ...                  | ... | agu   | 87GB 181007.0+533142 |
| J1811.1–1905c | 272.796 | −19.093 | 11.438  | −0.126  | 0.079      | 0.067      | −29    | 11.4     | 3.1      | 0.5             | 69.9     | 6.2             | 2.34          | ...                  | LP  | ... | 4,6,10,12     | 1FGL J1810.9–1905c   | ... | †     | ...                  |
| J1811.3–2421  | 272.833 | −24.365 | 6.831   | −2.692  | 0.192      | 0.143      | 42     | 6.4      | 1.6      | 0.4             | 28.2     | 4.7             | 2.39          | ...                  | LP  | ... | 1,4,5,12      | ...                  | ... | ...   | ...                  |
| J1811.3+0339  | 272.834 | 3.657   | 31.623  | 10.585  | 0.079      | 0.071      | 14     | 6.7      | 0.9      | 0.2             | 12.2     | 2.7             | 1.73          | 0.14                 | PL  | ... | ...           | 1FGL J1811.3+0340    | ... | bzb   | NVSS J181118+034113  |
| J1813.4–1246  | 273.358 | −12.771 | 17.245  | 2.434   | 0.024      | 0.023      | 2      | 53.3     | 26.8     | 0.8             | 245.5    | 6.7             | 2.33          | ...                  | EC  | ... | ...           | 1FGL J1813.3–1246    | ... | PSR   | LAT PSR J1813–1246   |
|               |         |         |         |         |            |            |        |          |          |                 |          |                 |               |                      |     |     |               | 0FGL J1813.5–1248    |     |       |                      |
| J1813.5+3143  | 273.395 | 31.722  | 58.654  | 21.360  | 0.068      | 0.062      | −42    | 14.9     | 1.8      | 0.2             | 20.0     | 2.0             | 2.11          | 0.07                 | PL  | ... | ...           | 1FGL J1813.4+3141    | ... | bzb   | B2 1811+31           |
| J1813.6–2821  | 273.404 | −28.354 | 3.559   | −5.042  | 0.125      | 0.121      | −39    | 4.4      | 1.0      | 0.2             | 13.2     | 2.8             | 2.43          | 0.15                 | PL  | ... | 4             | ...                  | ... | ...   | ...                  |
| J1813.7–1139c | 273.435 | −11.659 | 18.259  | 2.899   | 0.148      | 0.119      | 17     | 9.5      | 2.0      | 0.4             | 37.9     | 4.4             | 2.38          | ...                  | LP  | ... | 4,5,6,12      | ...                  | ... | ...   | ...                  |
| J1813.7+0617  | 273.435 | 6.293   | 34.296  | 11.235  | 0.161      | 0.102      | −8     | 5.9      | 0.9      | 0.2             | 10.7     | 2.2             | 1.97          | 0.13                 | PL  | T   | ...           | ...                  | ... | bzb   | TXS 1811+062         |
| J1814.1–1735c | 273.539 | −17.592 | 13.093  | −0.024  | 0.079      | 0.070      | 11     | 13.1     | 9.1      | 1.0             | 84.2     | 7.9             | 2.33          | ...                  | LP  | ... | 4,6           | 1FGL J1814.0–1736c   | ... | ...   | ...                  |
|               |         |         |         |         |            |            |        |          |          |                 |          |                 |               |                      |     |     |               | 0FGL J1814.3–1739    |     |       |                      |

Table 1—Continued

| Name 2FGL     | R.A.    | Decl.   | $l$     | $b$     | $\theta_1$ | $\theta_2$ | $\phi$ | $\sigma$ | $F_{35}$ | $\Delta F_{35}$ | $S_{25}$ | $\Delta S_{25}$ | $\Gamma_{25}$ | $\Delta \Gamma_{25}$ | Mod | Var | Flags        | $\gamma$ -ray Assoc.                                                        | TeV | Class | ID or Assoc.          |
|---------------|---------|---------|---------|---------|------------|------------|--------|----------|----------|-----------------|----------|-----------------|---------------|----------------------|-----|-----|--------------|-----------------------------------------------------------------------------|-----|-------|-----------------------|
| J1815.6–6407  | 273.916 | −64.131 | 330.325 | −20.483 | 0.173      | 0.127      | 26     | 5.9      | 0.6      | 0.1             | 8.5      | 1.5             | 2.46          | 0.14                 | PL  | ... | ...          | 1AGL J1815–1732<br>3EG J1813–6419<br>EGR J1814–6423                         | ... | agu   | PMN J1814–6412        |
| J1816.5+4511  | 274.149 | 45.199  | 72.854  | 24.741  | 0.083      | 0.072      | −90    | 13.0     | 1.4      | 0.2             | 15.3     | 1.8             | 2.11          | 0.08                 | PL  | ... | ...          | 1FGL J1816.7+4509                                                           | ... | ...   | ...                   |
| J1816.7–4942  | 274.187 | −49.701 | 344.410 | −15.128 | 0.098      | 0.085      | −87    | 8.9      | 1.2      | 0.2             | 14.0     | 1.9             | 2.26          | 0.09                 | PL  | T   | ...          | ...                                                                         | ... | agu   | PMN J1816–4943        |
| J1817.6–1651c | 274.410 | −16.861 | 14.132  | −0.408  | 0.200      | 0.144      | −65    | 6.2      | 2.0      | 0.6             | 43.6     | 6.8             | 2.38          | ...                  | LP  | ... | 3,4,5,6,8,12 | 1FGL J1817.6–1651c                                                          | ... | ...   | ...                   |
| J1818.6+0903  | 274.668 | 9.057   | 37.374  | 11.362  | 0.097      | 0.079      | −84    | 10.6     | 1.8      | 0.2             | 22.6     | 2.6             | 2.32          | 0.08                 | PL  | T   | ...          | 1FGL J1818.1+0905                                                           | ... | bzq   | MG1 J181841+0903      |
| J1818.7+2138  | 274.690 | 21.643  | 49.173  | 16.602  | 0.161      | 0.126      | 1      | 4.1      | 0.5      | 0.1             | 6.0      | 1.6             | 2.29          | 0.20                 | PL  | ... | ...          | ...                                                                         | ... | agu   | MG2 J181902+2132      |
| J1819.3–1523  | 274.836 | −15.392 | 15.620  | −0.072  | 0.120      | 0.088      | 27     | 19.3     | 9.2      | 1.1             | 111.1    | 7.1             | 2.42          | ...                  | LP  | ... | ...          | 1FGL J1819.4–1518c                                                          | ... | ...   | ...                   |
| J1820.6+3625  | 275.153 | 36.423  | 63.937  | 21.516  | 0.112      | 0.103      | −14    | 5.4      | 0.4      | 0.1             | 5.1      | 1.5             | 1.80          | 0.25                 | PL  | ... | ...          | ...                                                                         | ... | agu   | NVSS J182021+362343   |
| J1820.6–3219  | 275.162 | −32.323 | 0.726   | −8.227  | 0.228      | 0.144      | 54     | 4.5      | 1.0      | 0.2             | 11.5     | 2.5             | 2.14          | 0.12                 | PL  | ... | ...          | 1FGL J1820.5–3216                                                           | ... | ...   | ...                   |
| J1821.8+0830  | 275.460 | 8.508   | 37.224  | 10.418  | 0.151      | 0.128      | −74    | 4.6      | 0.8      | 0.2             | 11.2     | 2.5             | 2.42          | 0.14                 | PL  | ... | ...          | ...                                                                         | ... | ...   | ...                   |
| J1823.1–1338c | 275.786 | −13.639 | 17.599  | −0.059  | 0.067      | 0.054      | 6      | 10.4     | 11.8     | 1.2             | 91.6     | 10.7            | 2.22          | ...                  | LP  | ... | 6            | 1FGL J1823.2–1336c                                                          | ... | ...   | ...                   |
| J1823.4–3014  | 275.852 | −30.248 | 2.864   | −7.811  | 0.130      | 0.101      | −16    | 6.7      | 1.4      | 0.2             | 15.8     | 2.7             | 2.16          | ...                  | EC  | ... | 4            | 1FGL J1823.4–3009                                                           | ... | PSR   | PSR J1823–3021A       |
| J1823.6–3453  | 275.921 | −34.897 | 358.682 | −9.944  | 0.050      | 0.047      | −27    | 11.9     | 1.6      | 0.2             | 22.3     | 3.5             | 1.69          | 0.10                 | PL  | ... | ...          | 1FGL J1823.5–3454                                                           | ... | agu   | NVSS J182338–345412   |
| J1823.7+6856  | 275.949 | 68.935  | 99.179  | 27.645  | 0.108      | 0.098      | 82     | 8.8      | 0.8      | 0.1             | 9.7      | 1.3             | 2.34          | 0.11                 | PL  | ... | ...          | ...                                                                         | ... | bzb   | 7CG J1823+6856        |
| J1823.8+4312  | 275.965 | 43.214  | 71.139  | 22.959  | 0.147      | 0.129      | −7     | 4.6      | 0.4      | 0.1             | 5.6      | 1.2             | 2.34          | 0.17                 | PL  | ... | ...          | ...                                                                         | ... | agu   | 1RXS J182418.7+430954 |
| J1824.0+5650  | 276.001 | 56.838  | 85.723  | 26.094  | 0.055      | 0.053      | 42     | 27.7     | 2.6      | 0.2             | 35.9     | 1.8             | 2.43          | 0.04                 | PL  | T   | ...          | 1FGL J1824.0+5651                                                           | ... | bzb   | 4C +56.27             |
| J1824.5–1351e | 276.130 | −13.852 | 17.567  | −0.454  | ...        | ...        | ...    | 10.1     | 13.5     | 2.2             | 184.2    | 20.7            | 1.69          | 0.09                 | PL  | ... | ...          | ...                                                                         | ... | PWN   | HESS J1825–137        |
| J1824.5+1013  | 276.147 | 10.225  | 39.095  | 10.563  | 0.101      | 0.088      | −58    | 4.6      | 0.7      | 0.2             | 7.7      | 1.9             | 2.09          | 0.16                 | PL  | ... | ...          | 1FGL J1824.6+1013                                                           | ... | ...   | ...                   |
| J1824.8–2449  | 276.203 | −24.827 | 7.864   | −5.615  | 0.103      | 0.095      | 30     | 11.4     | 2.8      | 0.3             | 24.3     | 3.3             | 2.39          | ...                  | LP  | ... | ...          | 1FGL J1824.5–2449                                                           | ... | glc   | NGC 6626              |
| J1825.1–5231  | 276.287 | −52.530 | 342.242 | −17.454 | 0.068      | 0.066      | 23     | 15.9     | 2.4      | 0.2             | 18.5     | 1.8             | 2.19          | ...                  | LP  | T   | ...          | ...                                                                         | ... | agu   | PKS 1821–525          |
| J1826.1–1256  | 276.535 | −12.948 | 18.551  | −0.380  | 0.019      | 0.018      | 64     | 52.2     | 53.4     | 1.4             | 361.1    | 10.0            | 2.19          | ...                  | EC  | ... | ...          | 1FGL J1826.1–1256<br>0FGL J1825.9–1256<br>3EG J1826–1302<br>1AGL J1826–1246 | ... | PSR   | LAT PSR J1826–1256    |
| J1826.3–1450  | 276.589 | −14.837 | 16.904  | −1.307  | 0.029      | 0.027      | 66     | 22.8     | 21.2     | 1.1             | 229.3    | 11.4            | 2.41          | ...                  | LP  | ... | ...          | 1FGL J1826.2–1450<br>0FGL J1826.3–1451                                      | P   | HMB   | LS 5039               |
| J1827.4–0846  | 276.858 | −8.775  | 22.392  | 1.283   | 0.074      | 0.066      | −43    | 6.3      | 2.5      | 0.5             | 28.1     | 5.1             | 2.05          | 0.10                 | PL  | ... | 4            | ...                                                                         | ... | ...   | ...                   |
| J1827.4–1445c | 276.866 | −14.755 | 17.102  | −1.505  | 0.093      | 0.066      | 56     | 4.6      | 2.8      | 0.8             | 31.4     | 8.7             | 2.05          | 0.16                 | PL  | ... | 6            | ...                                                                         | ... | ...   | ...                   |
| J1827.6+1149  | 276.915 | 11.819  | 40.889  | 10.580  | 0.150      | 0.141      | 69     | 5.1      | 0.8      | 0.2             | 10.6     | 2.1             | 2.43          | 0.14                 | PL  | ... | 1            | ...                                                                         | ... | ...   | ...                   |
| J1828.3–1124c | 277.099 | −11.414 | 20.165  | −0.154  | 0.142      | 0.109      | 9      | 7.6      | 4.4      | 0.8             | 40.9     | 5.3             | 2.13          | ...                  | LP  | ... | 2,4,6,12     | 1FGL J1827.9–1128c                                                          | ... | †     | ...                   |
| J1828.7+3231  | 277.181 | 32.528  | 60.634  | 18.629  | 0.159      | 0.130      | 84     | 5.5      | 0.7      | 0.1             | 7.7      | 1.5             | 2.24          | 0.13                 | PL  | ... | ...          | ...                                                                         | ... | ...   | ...                   |
| J1829.1+2725  | 277.295 | 27.424  | 55.693  | 16.655  | 0.173      | 0.134      | −26    | 8.3      | 0.8      | 0.2             | 12.8     | 1.6             | 2.53          | 0.10                 | PL  | ... | ...          | ...                                                                         | ... | agu   | 87GB 182712.0+272717  |
| J1829.1–0340c | 277.295 | −3.673  | 27.118  | 3.262   | 0.162      | 0.120      | −64    | 4.2      | 1.8      | 0.4             | 21.6     | 4.7             | 2.32          | 0.11                 | PL  | ... | 3,6          | ...                                                                         | ... | ...   | ...                   |

Table 1—Continued

| Name 2FGL     | R.A.    | Decl.   | $l$     | $b$     | $\theta_1$ | $\theta_2$ | $\phi$ | $\sigma$ | $F_{35}$ | $\Delta F_{35}$ | $S_{25}$ | $\Delta S_{25}$ | $\Gamma_{25}$ | $\Delta \Gamma_{25}$ | Mod | Var | Flags       | $\gamma$ -ray Assoc. | TeV | Class | ID or Assoc.          |
|---------------|---------|---------|---------|---------|------------|------------|--------|----------|----------|-----------------|----------|-----------------|---------------|----------------------|-----|-----|-------------|----------------------|-----|-------|-----------------------|
| J1829.2+5402  | 277.321 | 54.049  | 82.860  | 24.806  | 0.066      | 0.060      | -70    | 8.4      | 0.7      | 0.1             | 8.0      | 1.6             | 1.88          | 0.13                 | PL  | ... | ...         | 1FGL J1829.8+5404    | ... | bzb   | 1RXS J182925.7+540255 |
| J1829.3-2419  | 277.330 | -24.323 | 8.785   | -6.296  | 0.109      | 0.088      | -36    | 6.5      | 1.5      | 0.3             | 16.7     | 3.0             | 2.18          | 0.17                 | PL  | ... | ...         | 1FGL J1829.3-2423    | ... | agu   | 1RXS J182853.8-241746 |
| J1829.7+4846  | 277.449 | 48.770  | 77.263  | 23.468  | 0.075      | 0.067      | 25     | 14.1     | 1.4      | 0.2             | 17.2     | 1.5             | 2.34          | 0.07                 | PL  | T   | ...         | 1FGL J1829.8+4845    | ... | rdg   | 3C 380                |
| J1829.8-0204c | 277.452 | -2.077  | 28.610  | 3.858   | 0.127      | 0.115      | -62    | 6.6      | 3.5      | 0.6             | 20.3     | 3.7             | 1.97          | ...                  | LP  | ... | 6           | ...                  | ... | ...   | ...                   |
| J1830.0+1325  | 277.515 | 13.421  | 42.615  | 10.746  | 0.130      | 0.117      | -78    | 4.7      | 0.8      | 0.2             | 8.6      | 2.1             | 2.02          | 0.19                 | PL  | ... | ...         | ...                  | ... | agu   | MG1 J183001+1323      |
| J1830.1+0617  | 277.543 | 6.292   | 36.145  | 7.582   | 0.066      | 0.055      | -14    | 13.3     | 2.8      | 0.3             | 31.9     | 3.0             | 2.21          | 0.07                 | PL  | T   | ...         | 1FGL J1830.1+0618    | ... | bzq   | TXS 1827+062          |
|               |         |         |         |         |            |            |        |          |          |                 |          |                 |               |                      |     |     |             | 0FGL J1830.3+0617    |     |       |                       |
| J1830.2-4441  | 277.570 | -44.689 | 350.122 | -15.209 | 0.089      | 0.083      | 89     | 13.1     | 1.6      | 0.2             | 21.7     | 1.9             | 2.45          | 0.07                 | PL  | T   | ...         | ...                  | ... | agu   | PMN J1830-4441        |
| J1830.4-1634  | 277.609 | -16.578 | 15.815  | -2.984  | 0.102      | 0.086      | 29     | 8.3      | 2.1      | 0.3             | 38.1     | 4.9             | 2.66          | 0.10                 | PL  | ... | 4           | ...                  | ... | ...   | ...                   |
| J1830.9-3132  | 277.736 | -31.545 | 2.416   | -9.836  | 0.113      | 0.106      | -59    | 4.1      | 0.7      | 0.2             | 8.4      | 2.2             | 1.98          | 0.15                 | PL  | ... | ...         | ...                  | ... | ...   | ...                   |
| J1831.2-1518  | 277.816 | -15.303 | 17.040  | -2.572  | 0.206      | 0.156      | -30    | 4.9      | 1.6      | 0.4             | 33.1     | 6.3             | 2.76          | 0.14                 | PL  | ... | 4,5         | ...                  | ... | ...   | ...                   |
| J1832.0-0200  | 278.003 | -2.016  | 28.918  | 3.397   | 0.102      | 0.093      | 79     | 9.2      | 3.2      | 0.5             | 45.6     | 4.6             | 2.03          | ...                  | LP  | T   | 12          | 1FGL J1831.5-0200c   | ... | ...   | ...                   |
| J1832.2-6502  | 278.065 | -65.038 | 330.001 | -22.458 | 0.140      | 0.111      | 46     | 5.2      | 0.6      | 0.1             | 6.9      | 1.6             | 1.95          | 0.14                 | PL  | ... | ...         | 1FGL J1833.2-6502    | ... | ...   | ...                   |
| J1832.7-5700  | 278.177 | -57.010 | 338.222 | -20.054 | 0.111      | 0.102      | -49    | 7.1      | 0.8      | 0.2             | 10.0     | 1.6             | 2.30          | 0.13                 | PL  | ... | ...         | 1FGL J1832.6-5700    | ... | bzb   | PMN J1832-5659        |
| J1833.1-0437c | 278.297 | -4.630  | 26.729  | 1.934   | 0.183      | 0.111      | -85    | 7.9      | 0.9      | 0.2             | 39.5     | 5.0             | 2.49          | ...                  | LP  | ... | 3,4,6,10,12 | ...                  | ... | ...   | ...                   |
| J1833.6-1032  | 278.403 | -10.539 | 21.534  | -0.884  | 0.082      | 0.057      | -29    | 13.9     | 10.2     | 0.9             | 62.8     | 5.7             | 2.22          | ...                  | EC  | ... | 3,4         | 1FGL J1833.5-1034    | ... | PSR   | PSR J1833-1034        |
| J1833.6-2104  | 278.413 | -21.075 | 12.153  | -5.716  | 0.029      | 0.028      | 32     | 67.1     | 11.9     | 0.5             | 205.5    | 4.3             | 2.62          | ...                  | LP  | T   | ...         | 1FGL J1833.6-2103    | ... | bzq   | PKS 1830-211          |
|               |         |         |         |         |            |            |        |          |          |                 |          |                 |               |                      |     |     |             | 0FGL J1833.4-2106    |     |       |                       |
|               |         |         |         |         |            |            |        |          |          |                 |          |                 |               |                      |     |     |             | 3EG J1832-2110       |     |       |                       |
| J1834.3-0848  | 278.578 | -8.815  | 23.143  | -0.242  | 0.074      | 0.057      | 43     | 12.6     | 11.4     | 1.0             | 79.3     | 7.3             | 2.08          | ...                  | LP  | ... | 3           | ...                  | E   | †     | ...                   |
| J1834.7-0705c | 278.693 | -7.096  | 24.721  | 0.449   | 0.073      | 0.068      | -15    | 10.5     | 8.8      | 1.0             | 98.4     | 11.1            | 2.12          | 0.06                 | PL  | ... | 3,6,10      | 1FGL J1834.7-0709c   | ... | †     | ...                   |
| J1835.4+1036  | 278.859 | 10.610  | 40.634  | 8.337   | 0.164      | 0.141      | -49    | 4.2      | 0.7      | 0.2             | 9.9      | 2.2             | 2.48          | 0.17                 | PL  | ... | 4           | ...                  | ... | ...   | ...                   |
| J1835.4+1349  | 278.859 | 13.826  | 43.562  | 9.745   | 0.151      | 0.124      | 82     | 5.3      | 0.8      | 0.2             | 12.2     | 2.3             | 2.49          | 0.14                 | PL  | ... | 1,4         | 1FGL J1835.3+1345    | ... | ...   | ...                   |
| J1835.5-0649  | 278.899 | -6.831  | 25.050  | 0.389   | 0.081      | 0.075      | 15     | 5.2      | 4.1      | 1.0             | 46.0     | 9.9             | 1.96          | 0.13                 | PL  | ... | 2           | ...                  | ... | ...   | ...                   |
| J1835.6-3258  | 278.908 | -32.969 | 1.542   | -11.344 | 0.114      | 0.105      | 51     | 7.0      | 1.5      | 0.3             | 6.6      | 1.2             | 2.06          | ...                  | LP  | ... | ...         | 1FGL J1835.3-3255    | ... | glc   | NGC 6652              |
| J1836.2+5926  | 279.065 | 59.434  | 88.886  | 24.997  | 0.009      | 0.009      | -38    | 303.7    | 99.9     | 1.0             | 602.9    | 5.1             | 1.93          | ...                  | EC  | ... | ...         | 0FGL J1836.2+5924    | ... | PSR   | LAT PSR J1836+5925    |
|               |         |         |         |         |            |            |        |          |          |                 |          |                 |               |                      |     |     |             | 1AGL J1836+5923      |     |       |                       |
| J1836.2+3137  | 279.074 | 31.617  | 60.358  | 16.803  | 0.134      | 0.115      | -89    | 6.3      | 0.8      | 0.2             | 9.9      | 1.7             | 2.28          | 0.13                 | PL  | T   | ...         | 1FGL J1836.3+3135    | ... | bzb   | RX J1836.2+3136       |
| J1836.8-0623c | 279.220 | -6.386  | 25.593  | 0.310   | 0.085      | 0.077      | 37     | 9.7      | 8.9      | 1.0             | 79.9     | 9.9             | 2.25          | ...                  | LP  | ... | 4,5,6       | ...                  | ... | agu   | VERA J1837-0628       |
| J1837.3-0700c | 279.347 | -7.011  | 25.095  | -0.089  | 0.088      | 0.082      | 59     | 8.2      | 7.6      | 1.3             | 60.9     | 8.5             | 2.09          | ...                  | LP  | ... | 4,5,6       | 1FGL J1837.5-0659c   | E   | ...   | ...                   |
| J1837.9+3821  | 279.478 | 38.353  | 67.089  | 18.911  | 0.262      | 0.173      | 32     | 4.8      | 0.4      | 0.1             | 6.7      | 1.3             | 2.68          | 0.17                 | PL  | ... | 4           | ...                  | ... | ...   | ...                   |
| J1838.7+4759  | 279.696 | 47.994  | 76.898  | 21.820  | 0.067      | 0.060      | -11    | 12.1     | 1.2      | 0.2             | 15.8     | 2.6             | 1.72          | 0.10                 | PL  | T   | ...         | 1FGL J1838.6+4756    | ... | bzb   | GB6 J1838+4802        |
| J1839.0-0102  | 279.765 | -1.035  | 30.598  | 2.281   | 0.119      | 0.105      | 6      | 9.6      | 1.5      | 0.3             | 36.7     | 4.0             | 2.40          | ...                  | LP  | ... | 4,12        | ...                  | ... | ...   | ...                   |
| J1839.0-0539  | 279.766 | -5.656  | 26.490  | 0.163   | 0.027      | 0.026      | -75    | 23.6     | 29.4     | 1.5             | 235.4    | 16.5            | 2.21          | ...                  | LP  | ... | ...         | ...                  | E   | ...   | ...                   |
| J1839.3-0558c | 279.827 | -5.980  | 26.230  | -0.039  | 0.069      | 0.056      | -30    | 9.4      | 12.3     | 1.4             | 99.2     | 15.3            | 2.18          | ...                  | LP  | ... | 2,5,6       | ...                  | ... | ...   | ...                   |

Table 1—Continued

| Name 2FGL     | R.A.    | Decl.   | $l$     | $b$     | $\theta_1$ | $\theta_2$ | $\phi$ | $\sigma$ | $F_{35}$ | $\Delta F_{35}$ | $S_{25}$ | $\Delta S_{25}$ | $\Gamma_{25}$ | $\Delta \Gamma_{25}$ | Mod | Var | Flags      | $\gamma$ -ray Assoc. | TeV | Class | ID or Assoc.       | Ref |
|---------------|---------|---------|---------|---------|------------|------------|--------|----------|----------|-----------------|----------|-----------------|---------------|----------------------|-----|-----|------------|----------------------|-----|-------|--------------------|-----|
| J1839.7–0334c | 279.946 | −3.571  | 28.426  | 0.960   | 0.173      | 0.145      | −61    | 6.3      | 2.5      | 0.5             | 41.5     | 6.4             | 4.14          | ...                  | LP  | ... | 4,5,6,12   | ...                  | ... | †     | ...                | ... |
| J1840.3–0413c | 280.083 | −4.232  | 27.901  | 0.535   | 0.153      | 0.116      | −83    | 6.3      | 5.8      | 0.9             | 33.6     | 6.5             | 2.01          | ...                  | LP  | ... | 1,4,5,6    | EGR J1838–0420       | ... | †     | ...                | ... |
| J1841.2–0459c | 280.305 | −4.996  | 27.323  | −0.011  | 0.128      | 0.063      | −22    | 11.8     | 10.1     | 0.9             | 81.2     | 9.0             | 2.20          | ...                  | LP  | T   | 6          | ...                  | E   | †     | ...                | ... |
| J1841.7+3221  | 280.435 | 32.352  | 61.521  | 16.010  | 0.081      | 0.070      | −53    | 10.6     | 1.4      | 0.2             | 15.2     | 2.1             | 2.03          | 0.10                 | PL  | ... | ...        | 1FGL J1841.9+3220    | ... | bzb   | RX J1841.7+3218    | ... |
| J1842.3+2740  | 280.582 | 27.671  | 57.108  | 14.068  | 0.147      | 0.129      | −29    | 4.9      | 0.7      | 0.1             | 7.6      | 1.6             | 2.20          | 0.14                 | PL  | ... | ...        | ...                  | ... | ...   | ...                | ... |
| J1842.3–5839  | 280.588 | −58.660 | 336.966 | −21.784 | 0.090      | 0.085      | 48     | 6.0      | 0.6      | 0.1             | 7.6      | 1.9             | 1.79          | 0.18                 | PL  | ... | ...        | 1FGL J1842.3–5845    | ... | ...   | ...                | ... |
| J1842.8–0359c | 280.722 | −3.990  | 28.408  | 0.079   | 0.076      | 0.069      | 90     | 6.0      | 6.4      | 1.1             | 35.5     | 8.4             | 2.02          | ...                  | LP  | ... | 4,5,6      | 1FGL J1842.9–0359c   | ... | ...   | ...                | ... |
| J1843.7–0312c | 280.928 | −3.216  | 29.190  | 0.250   | 0.131      | 0.095      | 61     | 8.3      | 7.3      | 1.0             | 58.2     | 8.9             | 2.23          | ...                  | LP  | ... | 4,6        | ...                  | ... | ...   | ...                | ... |
| J1844.3+1548  | 281.076 | 15.810  | 46.316  | 8.678   | 0.069      | 0.062      | −28    | 12.5     | 1.9      | 0.2             | 26.2     | 2.4             | 2.43          | 0.08                 | PL  | ... | 3          | 1FGL J1844.1+1547    | ... | ...   | ...                | ... |
| J1844.3–0343c | 281.097 | −3.732  | 28.808  | −0.136  | 0.077      | 0.062      | 3      | 8.6      | 9.4      | 1.2             | 56.9     | 9.6             | 2.12          | ...                  | LP  | ... | 6          | 1FGL J1844.2–0342c   | ... | ...   | ...                | ... |
|               |         |         |         |         |            |            |        |          |          |                 |          |                 |               |                      |     |     |            | 0FGL J1844.1–0335    | ... | ...   | ...                | ... |
| J1844.7+5716  | 281.189 | 57.272  | 86.848  | 23.430  | 0.271      | 0.237      | 19     | 4.1      | 0.4      | 0.1             | 6.0      | 1.4             | 2.49          | 0.16                 | PL  | ... | ...        | ...                  | ... | agu   | TXS 1843+571       | ... |
| J1844.9–1116  | 281.241 | −11.277 | 22.151  | −3.699  | 0.190      | 0.179      | 57     | 8.4      | 0.8      | 0.2             | 23.2     | 2.8             | 2.67          | ...                  | LP  | ... | 2,12       | 1FGL J1845.9–1133    | ... | ...   | ...                | ... |
| J1846.4+0920  | 281.610 | 9.339   | 40.702  | 5.344   | 0.045      | 0.043      | 64     | 18.1     | 4.9      | 0.4             | 29.8     | 2.9             | 2.12          | ...                  | EC  | T   | ...        | 1FGL J1846.4+0919    | ... | PSR   | LAT PSR J1846+0919 | ... |
| J1846.6–2519  | 281.653 | −25.320 | 9.627   | −10.258 | 0.228      | 0.187      | −86    | 7.2      | 1.1      | 0.2             | 16.6     | 2.4             | 2.49          | 0.11                 | PL  | ... | 4          | ...                  | ... | ...   | ...                | ... |
| J1847.2–0236  | 281.809 | −2.611  | 30.130  | −0.257  | 0.114      | 0.074      | −87    | 13.8     | 9.7      | 1.0             | 91.7     | 8.0             | 2.32          | ...                  | LP  | ... | 4          | 1FGL J1846.8–0233c   | ... | ...   | ...                | ... |
| J1848.2–0139c | 282.070 | −1.651  | 31.104  | −0.051  | 0.100      | 0.093      | −66    | 11.4     | 10.3     | 1.0             | 120.6    | 11.2            | 2.41          | ...                  | LP  | ... | 3,6,10     | 1FGL J1848.1–0145c   | E   | ...   | ...                | ... |
|               |         |         |         |         |            |            |        |          |          |                 |          |                 |               |                      |     |     |            | 0FGL J1848.6–0138    | ... | ...   | ...                | ... |
| J1848.5+3216  | 282.127 | 32.274  | 62.019  | 14.661  | 0.095      | 0.089      | −40    | 7.7      | 1.5      | 0.2             | 20.0     | 3.0             | 2.38          | 0.09                 | PL  | T   | ...        | 0FGL J1847.8+3223    | ... | BZQ   | B2 1846+32A        | 26  |
| J1848.6+3241  | 282.170 | 32.690  | 62.429  | 14.790  | 0.123      | 0.110      | 11     | 5.0      | 1.0      | 0.2             | 13.8     | 2.9             | 2.43          | 0.12                 | PL  | ... | 5          | ...                  | ... | agu   | B2 1846+32B        | ... |
| J1849.3–0055  | 282.328 | −0.917  | 31.874  | 0.055   | 0.068      | 0.058      | 78     | 9.0      | 7.9      | 1.0             | 49.4     | 9.0             | 2.19          | ...                  | LP  | ... | ...        | 1FGL J1849.0–0055c   | ... | †     | ...                | ... |
| J1849.4+6706  | 282.350 | 67.104  | 97.504  | 25.033  | 0.027      | 0.026      | 22     | 60.4     | 7.4      | 0.3             | 73.1     | 2.6             | 2.23          | ...                  | LP  | T   | ...        | 1FGL J1849.3+6705    | ... | bzq   | S4 1849+67         | ... |
|               |         |         |         |         |            |            |        |          |          |                 |          |                 |               |                      |     |     |            | 0FGL J1849.4+6706    | ... | ...   | ...                | ... |
|               |         |         |         |         |            |            |        |          |          |                 |          |                 |               |                      |     |     |            | 1AGL J1846+6714      | ... | ...   | ...                | ... |
| J1849.5+2744  | 282.383 | 27.745  | 57.841  | 12.640  | 0.124      | 0.104      | −77    | 5.4      | 0.7      | 0.2             | 8.3      | 1.7             | 2.15          | 0.13                 | PL  | ... | ...        | ...                  | ... | bzb   | MG2 J184929+2748   | ... |
| J1849.7–4310  | 282.432 | −43.182 | 352.947 | −17.890 | 0.082      | 0.080      | 9      | 9.1      | 1.3      | 0.2             | 14.0     | 2.1             | 2.02          | 0.09                 | PL  | ... | ...        | 1FGL J1849.6–4314    | ... | bzb   | PMN J1849–4314     | ... |
| J1849.9–0125c | 282.493 | −1.426  | 31.497  | −0.325  | 0.094      | 0.081      | 61     | 7.5      | 7.7      | 1.0             | 60.3     | 10.2            | 2.24          | ...                  | LP  | ... | 2,4,5,6    | 1FGL J1849.7–0121c   | ... | ...   | ...                | ... |
| J1850.7–0014c | 282.691 | −0.248  | 32.635  | 0.036   | 0.191      | 0.161      | 26     | 9.2      | 4.3      | 0.9             | 77.6     | 8.8             | 2.52          | ...                  | LP  | T   | 3,4,5,6,10 | 1FGL J1850.2–0019c   | ... | †     | ...                | ... |
| J1852.5+4856  | 283.132 | 48.938  | 78.605  | 19.939  | 0.049      | 0.047      | 80     | 26.7     | 2.9      | 0.2             | 34.3     | 1.9             | 2.28          | 0.04                 | PL  | T   | ...        | 1FGL J1852.5+4853    | ... | bzq   | S4 1851+48         | ... |
| J1852.7+0047c | 283.183 | 0.788   | 33.781  | 0.071   | 0.187      | 0.131      | −13    | 5.6      | 1.8      | 0.5             | 45.0     | 7.4             | 2.20          | ...                  | LP  | ... | 3,4,5,6,12 | 1FGL J1853.1+0032c   | ... | †     | ...                | ... |
| J1852.8+0156c | 283.205 | 1.934   | 34.811  | 0.574   | 0.100      | 0.094      | 25     | 7.3      | 5.6      | 0.8             | 38.1     | 5.9             | 2.11          | ...                  | LP  | ... | 1,4,6      | ...                  | ... | ...   | ...                | ... |
| J1855.9+0121e | 283.990 | 1.355   | 34.654  | −0.388  | ...        | ...        | ...    | 57.6     | 79.6     | 1.8             | 548.9    | 13.3            | 2.10          | ...                  | LP  | T   | ...        | 3EG J1856+0114       | ... | SNR   | SNR G034.7–00.4    | 27  |
|               |         |         |         |         |            |            |        |          |          |                 |          |                 |               |                      |     |     |            | 1AGL J1857+0137      | ... | W44   | ...                | ... |
| J1856.2+0450c | 284.060 | 4.838   | 37.785  | 1.139   | 0.129      | 0.104      | −70    | 12.3     | 3.7      | 0.8             | 65.3     | 6.0             | 2.47          | ...                  | LP  | ... | 5,6        | ...                  | ... | ...   | ...                | ... |
| J1857.2+0055c | 284.312 | 0.931   | 34.423  | −0.868  | 0.065      | 0.052      | 53     | 12.2     | 10.6     | 1.1             | 60.1     | 7.0             | 1.93          | ...                  | LP  | ... | 5,6        | ...                  | ... | ...   | ...                | ... |

Table 1—Continued

| Name 2FGL     | R.A.    | Decl.   | $l$     | $b$     | $\theta_1$ | $\theta_2$ | $\phi$ | $\sigma$ | $F_{35}$ | $\Delta F_{35}$ | $S_{25}$ | $\Delta S_{25}$ | $\Gamma_{25}$ | $\Delta \Gamma_{25}$ | Mod | Var | Flags   | $\gamma$ -ray Assoc. | TeV | Class | ID or Assoc.          | Ref. |
|---------------|---------|---------|---------|---------|------------|------------|--------|----------|----------|-----------------|----------|-----------------|---------------|----------------------|-----|-----|---------|----------------------|-----|-------|-----------------------|------|
| J1857.6+0211  | 284.419 | 2.187   | 35.590  | -0.390  | 0.067      | 0.055      | 52     | 17.8     | 14.4     | 1.0             | 98.7     | 7.4             | 2.16          | ...                  | LP  | ... | 2       | EGR J1856+0235       | E   | ...   | ...                   | ...  |
| J1857.8+0355c | 284.469 | 3.925   | 37.159  | 0.359   | 0.162      | 0.113      | 4      | 11.6     | 9.2      | 0.9             | 53.2     | 7.6             | 2.29          | ...                  | LP  | ... | 2,6     | 1FGL J1857.9+0352c   | ... | ...   | ...                   | ...  |
| J1858.1-2510  | 284.545 | -25.170 | 10.885  | -12.570 | 0.152      | 0.146      | -80    | 8.4      | 1.3      | 0.2             | 17.4     | 2.2             | 2.42          | 0.09                 | PL  | T   | ...     | ...                  | ... | agu   | PMN J1858-2511        | ...  |
| J1858.3-2218  | 284.589 | -22.311 | 13.560  | -11.418 | 0.105      | 0.098      | 83     | 6.2      | 1.0      | 0.2             | 11.6     | 2.1             | 2.14          | 0.12                 | PL  | ... | 10      | 1FGL J1858.1-2218    | ... | ...   | ...                   | ...  |
| J1858.5+0129c | 284.625 | 1.493   | 35.066  | -0.890  | 0.190      | 0.126      | -81    | 7.0      | 6.8      | 1.0             | 36.2     | 6.3             | 1.95          | ...                  | LP  | ... | 4,5,6   | 1AGL J1857+0137      | ... | ...   | ...                   | ...  |
| J1859.3+0312c | 284.845 | 3.210   | 36.695  | -0.301  | 0.114      | 0.090      | -49    | 6.3      | 4.3      | 1.1             | 38.1     | 6.5             | 4.75          | ...                  | LP  | T   | 1,4,5,6 | ...                  | ... | ...   | ...                   | ...  |
| J1901.1+0427  | 285.298 | 4.458   | 38.010  | -0.133  | 0.116      | 0.092      | -52    | 16.3     | 9.9      | 1.0             | 90.6     | 6.9             | 2.31          | ...                  | LP  | T   | ...     | 1AGL J1901+0429      | ... | ...   | ...                   | ...  |
| J1902.0-5109  | 285.508 | -51.161 | 345.586 | -22.394 | 0.074      | 0.061      | 6      | 19.4     | 3.0      | 0.3             | 21.8     | 1.7             | 2.21          | ...                  | EC  | ... | ...     | 1FGL J1902.0-5110    | ... | PSR   | PSR J1902-5105        | ...  |
| J1902.3-1106  | 285.588 | -11.103 | 24.227  | -7.435  | 0.180      | 0.137      | 64     | 5.6      | 1.0      | 0.2             | 15.5     | 2.6             | 2.53          | 0.13                 | PL  | ... | 1,4     | ...                  | ... | ...   | ...                   | ...  |
| J1902.5-6746  | 285.639 | -67.776 | 327.788 | -26.004 | 0.126      | 0.111      | -82    | 8.2      | 0.7      | 0.1             | 10.6     | 1.4             | 2.49          | 0.10                 | PL  | T   | ...     | 1FGL J1902.3-6802    | ... | bzq   | PMN J1903-6749        | ...  |
| J1902.7-7053  | 285.682 | -70.897 | 324.342 | -26.437 | 0.111      | 0.107      | -0     | 9.9      | 1.1      | 0.2             | 12.9     | 1.6             | 2.23          | 0.10                 | PL  | ... | ...     | 1FGL J1901.6-7051    | ... | ...   | ...                   | ...  |
| J1903.3+5539  | 285.840 | 55.666  | 85.963  | 20.514  | 0.040      | 0.037      | -66    | 27.5     | 3.5      | 0.2             | 39.5     | 2.9             | 1.94          | 0.04                 | PL  | ... | ...     | 1FGL J1903.0+5539    | ... | bzb   | TXS 1902+556          | ...  |
| J1904.8-0705  | 286.220 | -7.096  | 28.120  | -6.206  | 0.128      | 0.104      | 33     | 10.3     | 1.9      | 0.3             | 27.6     | 2.9             | 2.48          | 0.08                 | PL  | ... | ...     | 1FGL J1904.4-0703    | ... | ...   | ...                   | ...  |
| J1904.9-3720c | 286.231 | -37.334 | 359.783 | -18.552 | 0.156      | 0.121      | -61    | 8.4      | 1.3      | 0.3             | 10.1     | 1.5             | 2.23          | ...                  | LP  | ... | 2,6     | 1FGL J1903.8-3718c   | ... | ...   | ...                   | ...  |
| J1906.5+0720  | 286.647 | 7.343   | 41.189  | -0.002  | 0.057      | 0.047      | -3     | 24.0     | 14.3     | 1.0             | 129.6    | 6.7             | 2.30          | ...                  | LP  | ... | ...     | 1FGL J1906.6+0716c   | ... | ...   | ...                   | ...  |
| J1907.9+0602  | 286.986 | 6.034   | 40.183  | -0.903  | 0.021      | 0.020      | -69    | 54.8     | 37.7     | 1.0             | 281.7    | 7.4             | 2.20          | ...                  | EC  | ... | 2       | 1FGL J1907.9+0602    | E   | PSR   | LAT PSR J1907+0602    | ...  |
| J1908.8-0132  | 287.204 | -1.550  | 33.533  | -4.573  | 0.116      | 0.097      | -12    | 7.4      | 1.4      | 0.2             | 22.9     | 3.1             | 2.60          | 0.10                 | PL  | ... | 10      | 1AGL J1908+0614      | ... | ...   | ...                   | ...  |
| J1911.0+0905  | 287.764 | 9.094   | 43.253  | -0.175  | 0.025      | 0.024      | 81     | 33.0     | 22.3     | 0.9             | 174.5    | 7.9             | 2.11          | ...                  | LP  | T   | 10      | 1FGL J1910.9+0906c   | P   | snr   | SNR G043.3-00.2       | ...  |
| J1911.1-2005  | 287.791 | -20.097 | 16.892  | -13.211 | 0.045      | 0.043      | 4      | 31.9     | 5.7      | 0.3             | 65.4     | 3.0             | 2.41          | ...                  | LP  | T   | ...     | 0FGL J1911.0+0905    | ... | bzq   | PKS B1908-201         | ...  |
| J1911.5-1908  | 287.893 | -19.135 | 17.832  | -12.900 | 0.155      | 0.106      | 86     | 4.7      | 0.7      | 0.2             | 8.4      | 2.1             | 1.91          | 0.20                 | PL  | ... | ...     | 1FGL J1911.2-2007    | ... | ...   | ...                   | ...  |
| J1912.0+1609  | 288.013 | 16.160  | 49.635  | 2.873   | 0.101      | 0.096      | -13    | 6.0      | 1.3      | 0.3             | 22.9     | 3.8             | 2.61          | 0.11                 | PL  | ... | 1,4     | 0FGL J1911.2-2011    | ... | agu   | PMN J1911-1908        | ...  |
| J1913.4+4440  | 288.353 | 44.670  | 75.784  | 15.069  | 0.110      | 0.095      | -11    | 4.1      | 0.3      | 0.1             | 4.7      | 1.7             | 1.69          | 0.21                 | PL  | ... | ...     | 3EG J1911-2000       | ... | agu   | 87GB 190942.8+160617  | ...  |
| J1913.8-1237  | 288.451 | -12.630 | 24.080  | -10.622 | 0.278      | 0.250      | -20    | 4.2      | 0.7      | 0.2             | 10.6     | 2.2             | 2.47          | 0.15                 | PL  | ... | 4       | EGR J1912-2000       | ... | ...   | 1RXS J191401.9+443849 | ...  |
| J1914.0+1436  | 288.520 | 14.604  | 48.480  | 1.721   | 0.155      | 0.127      | -51    | 7.4      | 0.9      | 0.2             | 28.1     | 3.9             | 4.74          | ...                  | LP  | ... | 1,4,12  | ...                  | ... | ...   | ...                   | ...  |
| J1914.4+0951c | 288.619 | 9.851   | 44.314  | -0.572  | 0.128      | 0.103      | 19     | 5.5      | 2.8      | 0.9             | 29.6     | 5.6             | 2.31          | ...                  | LP  | ... | 4,6     | ...                  | ... | ...   | ...                   | ...  |
| J1916.1+1106  | 289.045 | 11.109  | 45.624  | -0.358  | 0.164      | 0.097      | 80     | 7.1      | 1.3      | 0.3             | 39.2     | 5.2             | 2.32          | ...                  | LP  | T   | 3,4,12  | 1FGL J1916.0+1110c   | ... | †     | ...                   | ...  |
| J1917.0-3027  | 289.269 | -30.456 | 7.506   | -18.468 | 0.102      | 0.089      | -65    | 6.1      | 0.9      | 0.2             | 9.8      | 2.0             | 2.00          | 0.14                 | PL  | ... | ...     | 1FGL J1916.9-3028    | ... | ...   | ...                   | ...  |
| J1917.6-1921  | 289.423 | -19.350 | 18.243  | -14.305 | 0.049      | 0.044      | -42    | 19.6     | 3.2      | 0.3             | 37.3     | 3.4             | 1.91          | 0.06                 | PL  | T   | ...     | 1FGL J1917.7-1922    | ... | bzb   | 1H 1914-194           | ...  |
| J1918.2-4110  | 289.571 | -41.175 | 356.797 | -22.241 | 0.056      | 0.051      | -86    | 16.8     | 2.5      | 0.2             | 30.5     | 3.4             | 1.84          | 0.06                 | PL  | ... | ...     | 1FGL J1918.4-4108    | ... | bzb   | PMN J1918-4111        | ...  |
| J1919.5-7324  | 289.883 | -73.409 | 321.637 | -27.909 | 0.223      | 0.210      | 89     | 4.4      | 0.3      | 0.1             | 7.6      | 1.6             | 2.78          | 0.18                 | PL  | ... | ...     | ...                  | ... | ...   | ...                   | ...  |

Table 1—Continued

| Name 2FGL     | R.A.    | Decl.   | $l$     | $b$     | $\theta_1$ | $\theta_2$ | $\phi$ | $\sigma$ | $F_{35}$ | $\Delta F_{35}$ | $S_{25}$ | $\Delta S_{25}$ | $\Gamma_{25}$ | $\Delta \Gamma_{25}$ | Mod | Var | Flags    | $\gamma$ -ray Assoc. | TeV | Class | ID or Assoc.          | Ref. |
|---------------|---------|---------|---------|---------|------------|------------|--------|----------|----------|-----------------|----------|-----------------|---------------|----------------------|-----|-----|----------|----------------------|-----|-------|-----------------------|------|
| J1921.1+1436c | 290.292 | 14.600  | 49.278  | 0.202   | 0.114      | 0.104      | 62     | 8.2      | 4.1      | 1.0             | 50.3     | 6.9             | 2.35          | ...                  | LP  | ... | 2,5,6    | 1AGL J1922+1351      | ... | ...   | ...                   | ...  |
| J1921.3+0131  | 290.332 | 1.520   | 37.713  | -5.947  | 0.128      | 0.115      | -24    | 7.6      | 1.5      | 0.2             | 20.6     | 2.8             | 2.43          | 0.09                 | PL  | ... | 3        | 1FGL J1921.2+0132    | ... | ...   | ...                   | ...  |
| J1921.3-1231  | 290.338 | -12.529 | 24.984  | -12.240 | 0.096      | 0.091      | 11     | 6.6      | 1.0      | 0.2             | 11.6     | 2.1             | 2.11          | 0.12                 | PL  | ... | ...      | 1FGL J1921.1-1234    | ... | bzb   | TXS 1918-126          | ...  |
| J1921.9-1608  | 290.495 | -16.138 | 21.695  | -13.906 | 0.052      | 0.049      | 11     | 12.6     | 1.6      | 0.2             | 20.8     | 3.2             | 1.74          | 0.10                 | PL  | ... | ...      | 1FGL J1922.0-1608    | ... | bzb   | PMN J1921-1607        | ...  |
| J1922.6-7454  | 290.662 | -74.908 | 319.943 | -28.146 | 0.084      | 0.082      | 19     | 5.7      | 0.6      | 0.1             | 6.3      | 1.5             | 2.03          | 0.21                 | PL  | ... | ...      | ...                  | ... | agu   | SUMSS J192240-745348  | ...  |
| J1923.2+1408e | 290.818 | 14.145  | 49.116  | -0.462  | ...        | ...        | ...    | 50.1     | 39.2     | 1.1             | 318.6    | 10.2            | 2.08          | ...                  | LP  | ... | ...      | 0FGL J1923.0+1411    | ... | SNR   | W51C                  | 28   |
|               |         |         |         |         |            |            |        |          |          |                 |          |                 |               |                      |     |     |          | 1AGL J1922+1351      | ... |       | W51C                  |      |
| J1923.4+2013  | 290.866 | 20.226  | 54.500  | 2.368   | 0.406      | 0.230      | 44     | 5.7      | 1.3      | 0.3             | 23.5     | 3.8             | 2.66          | 0.12                 | PL  | ... | 1,4,9    | ...                  | ... | ...   | ...                   | ...  |
| J1923.5-2105  | 290.884 | -21.087 | 17.168  | -16.259 | 0.030      | 0.029      | -51    | 47.2     | 8.3      | 0.4             | 81.4     | 3.4             | 2.24          | ...                  | LP  | T   | ...      | 1FGL J1923.5-2104    | ... | bzq   | TXS 1920-211          | ...  |
|               |         |         |         |         |            |            |        |          |          |                 |          |                 |               |                      |     |     |          | 0FGL J1923.3-2101    | ... |       |                       |      |
| J1924.8+1724c | 291.211 | 17.417  | 52.178  | 0.753   | 0.141      | 0.119      | -56    | 7.5      | 3.9      | 0.6             | 26.4     | 4.7             | 2.24          | ...                  | LP  | ... | 2,6      | 1FGL J1925.0+1720c   | ... | ...   | ...                   | ...  |
| J1924.8-2912  | 291.217 | -29.216 | 9.371   | -19.601 | 0.067      | 0.058      | -16    | 23.0     | 3.0      | 0.3             | 41.3     | 2.3             | 2.43          | 0.05                 | PL  | T   | ...      | 1FGL J1925.2-2919    | ... | bzq   | PKS B1921-293         | ...  |
| J1924.9-1036  | 291.236 | -10.609 | 27.145  | -12.204 | 0.119      | 0.107      | -84    | 8.8      | 1.5      | 0.2             | 17.6     | 2.3             | 2.27          | 0.09                 | PL  | ... | ...      | ...                  | ... | ...   | ...                   | ...  |
| J1925.7-7836c | 291.450 | -78.602 | 315.748 | -28.246 | 0.136      | 0.102      | -88    | 6.0      | 0.7      | 0.2             | 9.5      | 1.7             | 2.41          | 0.14                 | PL  | ... | 1,6      | ...                  | ... | ...   | ...                   | ...  |
| J1927.0+6153  | 291.768 | 61.898  | 93.307  | 19.713  | 0.038      | 0.034      | -68    | 18.8     | 2.2      | 0.2             | 26.1     | 2.7             | 1.84          | 0.07                 | PL  | T   | ...      | 1FGL J1926.8+6153    | ... | bzb   | 1RXS J192649.5+615445 | ...  |
| J1927.5+6117  | 291.898 | 61.284  | 92.722  | 19.434  | 0.080      | 0.075      | 43     | 7.5      | 0.9      | 0.2             | 9.5      | 1.7             | 2.08          | 0.12                 | PL  | ... | 5        | ...                  | ... | bzb   | S4 1926+61            | ...  |
| J1928.8+1740c | 292.223 | 17.680  | 52.869  | 0.029   | 0.125      | 0.077      | -11    | 6.6      | 1.5      | 0.4             | 33.4     | 5.0             | 2.25          | ...                  | LP  | ... | 3,4,6,12 | 1FGL J1929.0+1741c   | ... | psr   | PSR J1928+1746        | ...  |
|               |         |         |         |         |            |            |        |          |          |                 |          |                 |               |                      |     |     |          | 3EG J1928+1733       | ... |       |                       |      |
| J1931.1+0938  | 292.776 | 9.640   | 46.058  | -4.287  | 0.045      | 0.042      | -40    | 16.2     | 3.1      | 0.3             | 39.3     | 3.2             | 2.36          | 0.07                 | PL  | T   | 3        | 1FGL J1931.2+0939    | ... | bzb   | RX J1931.1+0937       | ...  |
| J1931.8+1325  | 292.959 | 13.428  | 49.476  | -2.631  | 0.309      | 0.262      | 77     | 5.8      | 0.4      | 0.1             | 18.1     | 2.9             | 2.55          | ...                  | LP  | ... | 1,4,12   | ...                  | ... | ...   | ...                   | ...  |
| J1932.1+1913  | 293.042 | 19.224  | 54.596  | 0.090   | 0.068      | 0.062      | -38    | 18.4     | 7.6      | 0.6             | 64.7     | 4.5             | 2.33          | ...                  | LP  | ... | 2        | 1FGL J1932.1+1914c   | ... | †     | ...                   | ...  |
| J1933.3+0722  | 293.339 | 7.381   | 44.330  | -5.852  | 0.074      | 0.072      | -13    | 7.6      | 1.2      | 0.2             | 16.7     | 2.6             | 2.47          | 0.12                 | PL  | ... | 4        | 1FGL J1933.3+0723    | ... | agu   | 1RXS J193320.3+072616 | ...  |
| J1936.5-0855  | 294.144 | -8.933  | 29.975  | -14.055 | 0.227      | 0.164      | 29     | 4.8      | 0.8      | 0.2             | 10.1     | 2.1             | 2.42          | 0.14                 | PL  | ... | ...      | ...                  | ... | ...   | ...                   | ...  |
| J1936.8-4721  | 294.214 | -47.357 | 351.132 | -27.008 | 0.068      | 0.064      | 44     | 7.2      | 0.7      | 0.2             | 10.0     | 2.5             | 1.64          | 0.16                 | PL  | ... | ...      | 1FGL J1936.9-4720    | ... | bzb   | PMN J1936-4719        | ...  |
| J1936.9+8402  | 294.239 | 84.041  | 116.441 | 25.804  | 0.162      | 0.141      | 24     | 4.6      | 0.4      | 0.1             | 4.7      | 1.1             | 2.03          | 0.15                 | PL  | ... | ...      | ...                  | ... | agu   | 6C B194425+834912     | ...  |
| J1937.2-3955  | 294.320 | -39.933 | 359.200 | -25.359 | 0.104      | 0.091      | 74     | 10.0     | 1.1      | 0.2             | 16.1     | 1.8             | 2.47          | 0.09                 | PL  | T   | ...      | 1FGL J1938.2-3957    | ... | bzq   | PKS 1933-400          | ...  |
| J1940.8-6213  | 295.210 | -62.226 | 334.460 | -29.482 | 0.168      | 0.150      | -1     | 6.8      | 0.6      | 0.1             | 9.3      | 1.4             | 2.49          | 0.12                 | PL  | T   | ...      | ...                  | ... | agu   | PKS 1936-623          | ...  |
| J1941.6+7218  | 295.417 | 72.315  | 104.272 | 22.065  | 0.186      | 0.120      | 77     | 10.5     | 1.0      | 0.2             | 12.3     | 1.6             | 2.48          | ...                  | LP  | T   | ...      | 1FGL J1941.6+7214    | ... | agu   | 87GB 194202.1+721428  | ...  |
| J1942.5-1024  | 295.644 | -10.402 | 29.267  | -16.024 | 0.187      | 0.165      | 21     | 4.9      | 0.7      | 0.2             | 10.5     | 2.2             | 2.54          | 0.14                 | PL  | ... | ...      | ...                  | ... | sey   | NGC 6814              | ...  |
| J1942.7-8049c | 295.681 | -80.821 | 313.155 | -28.793 | 0.210      | 0.141      | -6     | 7.3      | 1.0      | 0.2             | 13.4     | 1.9             | 2.40          | 0.10                 | PL  | ... | 2,6      | ...                  | ... | ...   | ...                   | ...  |
| J1942.8+1033  | 295.706 | 10.558  | 48.262  | -6.372  | 0.039      | 0.037      | 14     | 16.9     | 2.8      | 0.3             | 34.0     | 3.7             | 1.82          | 0.07                 | PL  | ... | ...      | 1FGL J1942.7+1033    | ... | agu   | 1RXS J194246.3+103339 | ...  |
| J1942.9-3528  | 295.737 | -35.481 | 4.276   | -25.226 | 0.179      | 0.169      | -79    | 4.8      | 0.8      | 0.2             | 8.8      | 1.8             | 2.21          | 0.15                 | PL  | ... | ...      | ...                  | ... | ...   | ...                   | ...  |
| J1944.3+7325  | 296.093 | 73.423  | 105.468 | 22.266  | 0.157      | 0.144      | -62    | 4.5      | 0.5      | 0.1             | 6.9      | 1.6             | 2.52          | 0.16                 | PL  | ... | 5        | ...                  | ... | ...   | ...                   | ...  |
| J1946.1-3115  | 296.548 | -31.260 | 8.943   | -24.623 | 0.147      | 0.128      | 73     | 4.6      | 0.7      | 0.2             | 8.6      | 1.8             | 2.29          | 0.15                 | PL  | ... | ...      | 1FGL J1946.1-3118    | ... | bzb   | PKS 1942-313          | ...  |
| J1946.4-5402  | 296.602 | -54.046 | 343.900 | -29.554 | 0.111      | 0.091      | -54    | 12.2     | 1.7      | 0.2             | 9.9      | 1.3             | 2.15          | ...                  | LP  | ... | ...      | 1FGL J1946.7-5404    | ... | ...   | ...                   | ...  |

Table 1—Continued

| Name 2FGL     | R.A.    | Decl.   | $l$     | $b$     | $\theta_1$ | $\theta_2$ | $\phi$ | $\sigma$ | $F_{35}$ | $\Delta F_{35}$ | $S_{25}$ | $\Delta S_{25}$ | $\Gamma_{25}$ | $\Delta \Gamma_{25}$ | Mod | Var | Flags  | $\gamma$ -ray Assoc. | TeV | Class | ID or Assoc.          | Ref. |
|---------------|---------|---------|---------|---------|------------|------------|--------|----------|----------|-----------------|----------|-----------------|---------------|----------------------|-----|-----|--------|----------------------|-----|-------|-----------------------|------|
| J1946.7–1118  | 296.677 | −11.311 | 28.861  | −17.329 | 0.185      | 0.171      | −29    | 4.8      | 0.8      | 0.2             | 9.6      | 2.0             | 2.31          | 0.14                 | PL  | ... | ...    | ...                  | ... | ...   | ...                   | ...  |
| J1947.8–0739  | 296.972 | −7.663  | 32.426  | −16.014 | 0.207      | 0.168      | 88     | 6.5      | 0.9      | 0.2             | 12.6     | 2.0             | 2.49          | 0.12                 | PL  | ... | ...    | ...                  | ... | ...   | ...                   | ...  |
| J1949.4–1457  | 297.374 | −14.958 | 25.663  | −19.463 | 0.151      | 0.145      | 27     | 5.2      | 0.8      | 0.2             | 9.3      | 1.8             | 2.30          | 0.13                 | PL  | ... | ...    | ...                  | ... | ...   | ...                   | ...  |
| J1949.7+2405  | 297.437 | 24.086  | 60.841  | −1.055  | 0.178      | 0.158      | 85     | 6.9      | 1.8      | 0.4             | 18.6     | 2.7             | 2.17          | ...                  | LP  | ... | 1,4,12 | ...                  | ... | ...   | ...                   | ...  |
| J1949.9+0907  | 297.476 | 9.123   | 47.861  | −8.595  | 0.177      | 0.117      | −15    | 5.4      | 0.7      | 0.2             | 10.7     | 2.1             | 2.47          | 0.15                 | PL  | ... | 1      | 1FGL J1950.0+0904    | ... | agu   | 1RXS J194934.1+090655 | ...  |
| J1950.3+1223  | 297.579 | 12.395  | 50.782  | −7.064  | 0.177      | 0.136      | 5      | 9.5      | 1.2      | 0.2             | 21.7     | 2.4             | 2.65          | 0.09                 | PL  | ... | ...    | 1FGL J1950.4+1226    | ... | ...   | ...                   | ...  |
| J1952.6–3252  | 298.156 | −32.869 | 7.689   | −26.403 | 0.727      | 0.519      | 6      | 4.4      | 0.6      | 0.2             | 8.2      | 1.8             | 2.44          | 0.15                 | PL  | ... | 8,9    | ...                  | ... | ...   | ...                   | ...  |
| J1953.0+3253  | 298.254 | 32.887  | 68.778  | 2.820   | 0.023      | 0.023      | 67     | 56.4     | 21.1     | 0.7             | 141.8    | 4.1             | 2.13          | ...                  | EC  | ... | ...    | 1FGL J1952.9+3252    | ... | PSR   | PSR J1952+3252        | ...  |
|               |         |         |         |         |            |            |        |          |          |                 |          |                 |               |                      |     |     |        | 0FGL J1953.2+3249    |     |       |                       |      |
| J1954.3+2836  | 298.580 | 28.609  | 65.251  | 0.381   | 0.031      | 0.028      | 36     | 34.8     | 16.7     | 0.7             | 110.5    | 4.8             | 2.15          | ...                  | EC  | ... | ...    | 1FGL J1954.3+2836    | ... | PSR   | LAT PSR J1954+2836    | ...  |
|               |         |         |         |         |            |            |        |          |          |                 |          |                 |               |                      |     |     |        | 0FGL J1954.4+2838    |     |       |                       |      |
| J1954.4–1607  | 298.614 | −16.131 | 25.030  | −21.028 | 0.226      | 0.171      | −79    | 4.5      | 0.7      | 0.2             | 8.0      | 1.9             | 2.13          | 0.15                 | PL  | ... | ...    | ...                  | ... | agu   | 1RXS J195500.6–160328 | ...  |
| J1954.6–1122  | 298.671 | −11.381 | 29.666  | −19.131 | 0.073      | 0.062      | −74    | 18.8     | 2.9      | 0.3             | 34.7     | 2.5             | 2.25          | 0.05                 | PL  | T   | ...    | 1FGL J1954.8–1124    | ... | bzq   | TXS 1951–115          | ...  |
| J1955.0–5639  | 298.775 | −56.654 | 341.009 | −31.002 | 0.077      | 0.074      | 29     | 5.1      | 0.5      | 0.1             | 6.3      | 1.7             | 1.88          | 0.19                 | PL  | ... | 1      | ...                  | ... | agu   | 1RXS J195503.1–564031 | ...  |
| J1955.2+1356  | 298.807 | 13.936  | 52.731  | −7.326  | 0.077      | 0.075      | −37    | 12.5     | 1.9      | 0.2             | 24.7     | 2.3             | 2.40          | 0.08                 | PL  | T   | ...    | 1FGL J1954.8+1402    | ... | bzq   | 87GB 195252.4+135009  | ...  |
| J1955.9–0241  | 298.983 | −2.700  | 37.969  | −15.567 | 0.194      | 0.167      | 38     | 5.7      | 0.7      | 0.2             | 11.7     | 2.0             | 2.58          | 0.13                 | PL  | ... | 1      | 1FGL J1956.2–0238    | ... | ...   | ...                   | ...  |
| J1957.9+5033  | 299.481 | 50.555  | 84.606  | 10.975  | 0.065      | 0.064      | 54     | 25.5     | 3.4      | 0.3             | 28.1     | 1.7             | 2.35          | ...                  | EC  | ... | ...    | 1FGL J1957.6+5033    | ... | PSR   | LAT PSR J1957+5033    | ...  |
| J1958.2–3848  | 299.554 | −38.806 | 1.530   | −29.012 | 0.059      | 0.056      | −49    | 24.5     | 3.1      | 0.2             | 39.0     | 2.2             | 2.36          | 0.05                 | PL  | T   | ...    | 1FGL J1958.4–3847    | ... | bzq   | PKS 1954–388          | ...  |
| J1958.4–3012  | 299.619 | −30.212 | 10.938  | −26.823 | 0.088      | 0.081      | −38    | 5.0      | 0.6      | 0.2             | 7.0      | 1.9             | 1.86          | 0.24                 | PL  | ... | ...    | 1FGL J1958.4–3013    | ... | bzb   | 1RXS J195815.6–301119 | ...  |
| J1958.6+4020  | 299.650 | 40.350  | 75.774  | 5.698   | 0.171      | 0.137      | 71     | 5.5      | 1.0      | 0.2             | 12.0     | 2.3             | 2.30          | 0.15                 | PL  | ... | 1      | ...                  | ... | ...   | ...                   | ...  |
| J1958.6+2845  | 299.664 | 28.762  | 65.876  | −0.353  | 0.031      | 0.030      | −56    | 32.3     | 14.8     | 0.7             | 95.3     | 4.7             | 2.14          | ...                  | EC  | ... | ...    | 1FGL J1958.6+2845    | ... | PSR   | LAT PSR J1958+2846    | ...  |
|               |         |         |         |         |            |            |        |          |          |                 |          |                 |               |                      |     |     |        | 3EG J1958+2909       |     |       |                       |      |
| J1958.9+3844  | 299.731 | 38.740  | 74.423  | 4.811   | 0.217      | 0.159      | −54    | 5.7      | 1.0      | 0.2             | 15.3     | 2.6             | 2.52          | 0.13                 | PL  | T   | 4      | ...                  | ... | agu   | MG2 J195919+3847      | ...  |
| J1959.1–4245  | 299.786 | −42.760 | 357.123 | −29.989 | 0.067      | 0.063      | −58    | 22.1     | 2.5      | 0.2             | 32.9     | 2.0             | 2.41          | 0.05                 | PL  | T   | ...    | 1FGL J1959.3–4241    | ... | bzq   | PMN J1959–4246        | ...  |
| J1959.5+2047  | 299.899 | 20.791  | 59.184  | −4.701  | 0.073      | 0.072      | 14     | 12.4     | 2.7      | 0.3             | 16.7     | 1.9             | 2.25          | ...                  | EC  | ... | ...    | 1FGL J1959.6+2047    | ... | PSR   | PSR J1959+2048        | ...  |
| J1959.6–2931  | 299.919 | −29.519 | 11.767  | −26.864 | 0.195      | 0.171      | 84     | 4.5      | 0.7      | 0.2             | 10.7     | 2.0             | 2.58          | 0.13                 | PL  | ... | ...    | ...                  | ... | agu   | PMN J2000–2931        | ...  |
| J1959.9+4212  | 299.978 | 42.210  | 77.503  | 6.448   | 0.140      | 0.114      | −42    | 4.6      | 0.8      | 0.2             | 8.9      | 2.2             | 2.13          | 0.16                 | PL  | ... | 8      | ...                  | ... | agu   | MG4 J195957+4213      | ...  |
| J1959.9–4727  | 299.988 | −47.455 | 351.772 | −30.876 | 0.057      | 0.055      | 53     | 12.5     | 1.4      | 0.2             | 18.8     | 3.1             | 1.71          | 0.09                 | PL  | ... | ...    | 1FGL J1959.7–4730    | ... | agu   | SUMSS J195945–472519  | ...  |
| J1959.9+3336c | 299.991 | 33.601  | 70.143  | 1.948   | 0.144      | 0.115      | 31     | 7.5      | 1.5      | 0.3             | 21.0     | 2.9             | 2.35          | ...                  | LP  | ... | 4,6,12 | ...                  | ... | ...   | ...                   | ...  |
| J2000.0+6509  | 300.020 | 65.157  | 98.016  | 17.666  | 0.026      | 0.025      | 85     | 40.4     | 5.9      | 0.3             | 66.9     | 3.6             | 1.94          | 0.03                 | PL  | T   | ...    | 1FGL J2000.0+6508    | P   | bzb   | 1ES 1959+650          | ...  |
|               |         |         |         |         |            |            |        |          |          |                 |          |                 |               |                      |     |     |        | 0FGL J2000.2+6506    |     |       |                       |      |
| J2000.8–1751  | 300.217 | −17.857 | 23.961  | −23.113 | 0.080      | 0.076      | 65     | 17.0     | 2.5      | 0.2             | 32.0     | 2.4             | 2.38          | 0.06                 | PL  | T   | ...    | 1FGL J2000.9–1749    | ... | bzq   | PKS 1958–179          | ...  |
| J2001.1+4352  | 300.288 | 43.879  | 79.060  | 7.118   | 0.020      | 0.020      | 80     | 47.2     | 11.8     | 0.4             | 136.1    | 6.0             | 1.90          | 0.03                 | PL  | T   | ...    | 1FGL J2001.1+4351    | P   | bzb   | MAGIC J2001+435       | ...  |
|               |         |         |         |         |            |            |        |          |          |                 |          |                 |               |                      |     |     |        | 0FGL J2001.0+4352    |     |       |                       |      |
| J2001.7+7042  | 300.430 | 70.704  | 103.348 | 19.973  | 0.087      | 0.080      | 55     | 6.2      | 0.8      | 0.2             | 9.3      | 1.8             | 2.18          | 0.13                 | PL  | ... | ...    | 1FGL J2001.9+7040    | ... | bzb   | TXS 2001+705          | ...  |

Table 1—Continued

| Name 2FGL     | R.A.    | Decl.   | $l$     | $b$     | $\theta_1$ | $\theta_2$ | $\phi$ | $\sigma$ | $F_{35}$ | $\Delta F_{35}$ | $S_{25}$ | $\Delta S_{25}$ | $\Gamma_{25}$ | $\Delta \Gamma_{25}$ | Mod | Var | Flags | $\gamma$ -ray Assoc.                   | TeV | Class | ID or Assoc.        | Ref. |
|---------------|---------|---------|---------|---------|------------|------------|--------|----------|----------|-----------------|----------|-----------------|---------------|----------------------|-----|-----|-------|----------------------------------------|-----|-------|---------------------|------|
| J2002.8–2150  | 300.717 | −21.843 | 20.094  | −25.024 | 0.147      | 0.138      | 45     | 4.1      | 0.5      | 0.1             | 6.0      | 1.6             | 2.06          | 0.19                 | PL  | ... | ...   | ...                                    | ... | ...   | ...                 | ...  |
| J2004.4+3339c | 301.120 | 33.662  | 70.693  | 1.182   | 0.070      | 0.061      | 72     | 9.1      | 2.9      | 0.4             | 32.2     | 4.3             | 2.04          | 0.08                 | PL  | ... | 3,6   | 1FGL J2004.7+3343                      | ... | ...   | ...                 | ...  |
| J2004.5+7754  | 301.129 | 77.916  | 110.480 | 22.797  | 0.143      | 0.102      | −90    | 10.0     | 1.1      | 0.1             | 12.5     | 1.5             | 2.22          | 0.09                 | PL  | T   | ...   | 1FGL J2006.0+7751                      | ... | bzb   | S5 2007+77          | ...  |
| J2004.6+7004  | 301.173 | 70.074  | 102.861 | 19.474  | 0.063      | 0.056      | 37     | 9.5      | 1.2      | 0.2             | 13.1     | 2.0             | 1.97          | 0.11                 | PL  | T   | ...   | 1FGL J2004.8+7004                      | ... | ...   | ...                 | ...  |
| J2006.2–0929  | 301.572 | −9.492  | 32.780  | −20.905 | 0.422      | 0.283      | −13    | 4.8      | 0.6      | 0.2             | 8.7      | 1.7             | 2.43          | 0.13                 | PL  | ... | 9     | ...                                    | ... | ...   | ...                 | ...  |
| J2006.5–2256  | 301.639 | −22.949 | 19.275  | −26.208 | 0.166      | 0.138      | −35    | 6.4      | 0.8      | 0.2             | 11.2     | 1.8             | 2.49          | 0.12                 | PL  | T   | ...   | 1FGL J2006.6–2302<br>3EG J2006–2321    | ... | ...   | ...                 | ...  |
| J2006.9–1734  | 301.734 | −17.582 | 24.842  | −24.343 | 0.170      | 0.159      | −1     | 4.7      | 0.6      | 0.1             | 9.6      | 2.0             | 2.59          | 0.15                 | PL  | ... | 4,5   | ...                                    | ... | ...   | ...                 | ...  |
| J2007.9–4430  | 301.992 | −44.515 | 355.408 | −31.849 | 0.107      | 0.103      | 76     | 6.8      | 0.7      | 0.1             | 9.4      | 1.5             | 2.47          | 0.12                 | PL  | ... | ...   | 1FGL J2007.9–4430                      | ... | sey   | PKS 2004–447        | ...  |
| J2009.1–0339  | 302.281 | −3.660  | 38.666  | −18.932 | 0.189      | 0.181      | 87     | 5.9      | 0.9      | 0.2             | 10.8     | 1.9             | 2.35          | 0.12                 | PL  | ... | 1     | ...                                    | ... | ...   | ...                 | ...  |
| J2009.2–1505  | 302.318 | −15.087 | 27.599  | −23.888 | 0.159      | 0.154      | 69     | 6.5      | 0.2      | 0.1             | 9.0      | 1.4             | 2.78          | ...                  | LP  | ... | 12    | ...                                    | ... | ...   | ...                 | ...  |
| J2009.5–4850  | 302.375 | −48.834 | 350.372 | −32.614 | 0.032      | 0.031      | −52    | 25.9     | 3.8      | 0.3             | 48.1     | 4.3             | 1.78          | 0.05                 | PL  | T   | ...   | 1FGL J2009.5–4849<br>0FGL J2009.4–4850 | P   | BZB   | PKS 2005–489        | ...  |
| J2009.7+7225  | 302.437 | 72.418  | 105.284 | 20.157  | 0.086      | 0.082      | 29     | 12.3     | 1.4      | 0.2             | 17.5     | 1.8             | 2.30          | 0.08                 | PL  | T   | ...   | 1FGL J2009.1+7228                      | ... | bzb   | 4C +72.28           | ...  |
| J2009.8+2747  | 302.457 | 27.795  | 66.370  | −2.948  | 0.377      | 0.345      | 4      | 4.6      | 0.8      | 0.2             | 11.7     | 2.3             | 2.41          | ...                  | LP  | ... | 4,12  | ...                                    | ... | ...   | ...                 | ...  |
| J2012.1+4630  | 303.035 | 46.508  | 82.339  | 6.866   | 0.042      | 0.037      | 45     | 14.2     | 2.6      | 0.3             | 28.8     | 3.1             | 1.97          | 0.07                 | PL  | T   | ...   | 1FGL J2012.2+4629                      | ... | bzb   | 7C 2010–5619        | ...  |
| J2012.4+3955c | 303.120 | 39.929  | 76.833  | 3.229   | 0.107      | 0.097      | −55    | 8.6      | 2.0      | 0.4             | 23.3     | 3.3             | 2.42          | ...                  | LP  | ... | 6     | ...                                    | ... | ...   | ...                 | ...  |
| J2013.8+4115c | 303.454 | 41.260  | 78.087  | 3.749   | 0.123      | 0.105      | −62    | 8.6      | 2.5      | 0.4             | 26.4     | 3.8             | 2.35          | ...                  | LP  | ... | 6     | ...                                    | ... | ...   | ...                 | ...  |
| J2014.0–0046  | 303.517 | −0.771  | 41.973  | −18.668 | 0.116      | 0.083      | 84     | 7.1      | 1.0      | 0.2             | 11.4     | 2.3             | 1.89          | 0.15                 | PL  | ... | 2     | 1FGL J2014.5–0047                      | ... | bzb   | PMN J2014–0047      | ...  |
| J2014.7+0646  | 303.685 | 6.781   | 48.928  | −15.091 | 0.116      | 0.108      | −75    | 4.8      | 0.5      | 0.2             | 6.8      | 2.0             | 1.74          | 0.23                 | PL  | ... | ...   | 1FGL J2014.4+0647                      | ... | agu   | NVSS J201431+064849 | ...  |
| J2015.1–0137  | 303.778 | −1.620  | 41.315  | −19.301 | 0.090      | 0.073      | 12     | 8.3      | 1.2      | 0.2             | 13.8     | 2.0             | 2.25          | 0.11                 | PL  | ... | ...   | 1FGL J2015.3–0129                      | ... | bzb   | PKS 2012–017        | ...  |
| J2015.6+3709  | 303.924 | 37.162  | 74.873  | 1.176   | 0.040      | 0.035      | −87    | 27.4     | 12.0     | 0.6             | 120.4    | 6.1             | 2.37          | ...                  | LP  | T   | ...   | 1FGL J2015.7+3708<br>3EG J2016+3657    | ... | agu   | MG2 J201534+3710    | ...  |
| J2016.3–0904  | 304.078 | −9.070  | 34.343  | −22.953 | 0.053      | 0.050      | 23     | 14.8     | 1.9      | 0.2             | 21.2     | 2.3             | 2.05          | 0.08                 | PL  | ... | ...   | 1FGL J2016.2–0903                      | ... | bzb   | PMN J2016–0903      | ...  |
| J2017.3+0603  | 304.350 | 6.054   | 48.626  | −16.030 | 0.033      | 0.032      | 74     | 31.2     | 6.4      | 0.4             | 37.8     | 2.5             | 1.88          | ...                  | EC  | ... | ...   | 1FGL J2017.3+0603<br>0FGL J2017.2+0602 | ... | PSR   | PSR J2017+0603      | ...  |
| J2017.4–3215  | 304.350 | −32.265 | 9.940   | −31.274 | 0.170      | 0.147      | −3     | 5.4      | 0.5      | 0.2             | 9.4      | 1.6             | 2.65          | 0.17                 | PL  | ... | 1     | ...                                    | ... | ...   | ...                 | ...  |
| J2017.5–1618  | 304.395 | −16.309 | 27.222  | −26.206 | 0.107      | 0.096      | −33    | 9.2      | 1.1      | 0.2             | 12.9     | 1.8             | 2.18          | 0.11                 | PL  | ... | ...   | 1FGL J2017.9–1621<br>3EG J2020–1545    | ... | ...   | ...                 | ...  |
| J2018.0+3626  | 304.511 | 36.448  | 74.545  | 0.387   | 0.059      | 0.050      | −53    | 18.5     | 11.1     | 0.7             | 75.0     | 6.3             | 2.28          | ...                  | LP  | ... | ...   | ...                                    | E   | ...   | ...                 | ...  |
| J2018.2+3850c | 304.565 | 38.841  | 76.549  | 1.697   | 0.075      | 0.060      | 61     | 8.4      | 2.7      | 0.4             | 31.2     | 4.8             | 2.18          | 0.10                 | PL  | ... | 6     | ...                                    | ... | agu   | TXS 2016+386        | ...  |
| J2019.1+4040  | 304.779 | 40.681  | 78.163  | 2.595   | 0.102      | 0.052      | 33     | 10.3     | 4.7      | 0.8             | 55.1     | 7.4             | 1.88          | 0.10                 | PL  | ... | 2,8,9 | ...                                    | E   | †     | ...                 | ...  |
| J2020.0+4159  | 305.016 | 41.993  | 79.349  | 3.188   | 0.127      | 0.110      | −85    | 9.4      | 2.5      | 0.9             | 40.0     | 4.9             | 2.41          | ...                  | LP  | ... | 4     | ...                                    | ... | ...   | ...                 | ...  |
| J2021.0+3651  | 305.270 | 36.863  | 75.231  | 0.119   | 0.013      | 0.013      | 34     | 95.0     | 67.6     | 1.2             | 488.8    | 8.5             | 2.17          | ...                  | EC  | ... | ...   | 1FGL J2021.0+3651<br>0FGL J2020.8+3649 | E   | PSR   | PSR J2021+3651      | ...  |



Table 1—Continued

| Name 2FGL     | R.A.    | Decl.   | $l$     | $b$     | $\theta_1$ | $\theta_2$ | $\phi$ | $\sigma$ | $F_{35}$ | $\Delta F_{35}$ | $S_{25}$ | $\Delta S_{25}$ | $\Gamma_{25}$ | $\Delta \Gamma_{25}$ | Mod | Var | Flags        | $\gamma$ -ray Assoc. | TeV | Class | ID or Assoc.         |
|---------------|---------|---------|---------|---------|------------|------------|--------|----------|----------|-----------------|----------|-----------------|---------------|----------------------|-----|-----|--------------|----------------------|-----|-------|----------------------|
| J2021.5+0632  | 305.391 | 6.542   | 49.614  | -16.671 | 0.138      | 0.108      | 24     | 5.2      | 0.7      | 0.2             | 8.3      | 1.8             | 2.15          | 0.15                 | PL  | ... | ...          | 1AGL J2021+3652      | ... | ...   | ...                  |
| J2021.5+4026  | 305.392 | 40.441  | 78.228  | 2.075   | 0.010      | 0.010      | -41    | 129.7    | 122.6    | 1.5             | 928.2    | 10.2            | 2.15          | ...                  | EC  | ... | ...          | 1FGL J2021.5+4026    | ... | PSR   | LAT PSR J2021+4026   |
|               |         |         |         |         |            |            |        |          |          |                 |          |                 |               |                      |     |     |              | 0FGL J2021.5+4026    |     |       |                      |
|               |         |         |         |         |            |            |        |          |          |                 |          |                 |               |                      |     |     |              | 1AGL J2022+4032      |     |       |                      |
| J2022.3-4518  | 305.584 | -45.308 | 354.823 | -34.468 | 0.247      | 0.152      | 28     | 4.4      | 0.5      | 0.1             | 6.0      | 1.3             | 2.31          | 0.15                 | PL  | ... | ...          | 1FGL J2022.5-4532    | ... | bzb   | PMN J2022-4513       |
| J2022.5+7614  | 305.636 | 76.243  | 109.334 | 21.160  | 0.097      | 0.085      | 67     | 13.4     | 1.5      | 0.2             | 18.5     | 1.7             | 2.32          | 0.07                 | PL  | T   | ...          | ...                  | ... | bzb   | S5 2023+760          |
| J2022.8+3843c | 305.709 | 38.723  | 76.957  | 0.894   | 0.134      | 0.125      | -18    | 10.0     | 2.3      | 0.4             | 41.8     | 4.5             | 2.52          | ...                  | LP  | ... | 2,4,6,12     | ...                  | ... | snr   | SNR G076.9+01.0      |
| J2023.4-1137  | 305.859 | -11.630 | 32.620  | -25.628 | 0.081      | 0.076      | 61     | 9.3      | 1.1      | 0.2             | 12.5     | 1.9             | 2.07          | 0.11                 | PL  | ... | ...          | 1FGL J2023.7-1141    | ... | bzq   | PMN J2023-1140       |
| J2025.1+3341  | 306.282 | 33.695  | 73.105  | -2.371  | 0.061      | 0.059      | 82     | 12.4     | 4.1      | 0.4             | 47.6     | 4.8             | 2.44          | ...                  | LP  | T   | ...          | ...                  | ... | agu   | B2 2023+33           |
| J2025.6-0736  | 306.416 | -7.605  | 36.889  | -24.388 | 0.029      | 0.029      | 31     | 63.2     | 10.1     | 0.4             | 107.5    | 3.2             | 2.32          | ...                  | LP  | T   | ...          | 1FGL J2025.6-0735    | ... | bzq   | PKS 2023-07          |
|               |         |         |         |         |            |            |        |          |          |                 |          |                 |               |                      |     |     |              | 0FGL J2025.6-0736    |     |       |                      |
|               |         |         |         |         |            |            |        |          |          |                 |          |                 |               |                      |     |     |              | 3EG J2025-0744       |     |       |                      |
|               |         |         |         |         |            |            |        |          |          |                 |          |                 |               |                      |     |     |              | 1AGL J2026-0732      |     |       |                      |
| J2028.3+3332  | 307.098 | 33.542  | 73.375  | -3.014  | 0.040      | 0.036      | -68    | 25.8     | 10.2     | 0.6             | 60.8     | 4.6             | 2.21          | ...                  | LP  | ... | ...          | ...                  | ... | ...   | ...                  |
| J2029.4+4924  | 307.367 | 49.407  | 86.391  | 6.087   | 0.071      | 0.066      | 22     | 15.6     | 4.1      | 0.4             | 27.7     | 2.7             | 2.24          | ...                  | LP  | T   | ...          | 1FGL J2029.2+4924    | ... | bzb   | MC J202932+4925      |
| J2030.0+3640  | 307.512 | 36.680  | 76.120  | -1.452  | 0.044      | 0.042      | 11     | 17.1     | 7.4      | 0.6             | 37.0     | 3.5             | 2.10          | ...                  | EC  | ... | ...          | 1FGL J2030.0+3641    | ... | PSR   | PSR J2030+3641       |
| J2030.3-0622  | 307.593 | -6.373  | 38.678  | -24.878 | 0.084      | 0.082      | 56     | 10.4     | 0.9      | 0.1             | 17.7     | 1.9             | 2.73          | 0.10                 | PL  | T   | ...          | 1FGL J2030.3-0617    | ... | bzq   | TXS 2027-065         |
| J2030.7+4417  | 307.675 | 44.284  | 82.343  | 2.921   | 0.068      | 0.065      | -3     | 18.6     | 6.7      | 0.5             | 56.2     | 4.0             | 2.32          | ...                  | LP  | ... | ...          | 1FGL J2030.9+4411    | ... | ...   | ...                  |
| J2031.0+1938  | 307.773 | 19.641  | 62.269  | -11.527 | 0.116      | 0.101      | 89     | 6.6      | 0.8      | 0.1             | 8.8      | 1.9             | 1.88          | 0.15                 | PL  | ... | ...          | ...                  | ... | agu   | RX J2030.8+1935      |
| J2031.4-1842  | 307.868 | -18.703 | 26.103  | -30.172 | 0.288      | 0.225      | -89    | 4.1      | 0.3      | 0.1             | 6.6      | 1.5             | 2.78          | 0.23                 | PL  | T   | 4,8,9,11     | ...                  | ... | ...   | ...                  |
| J2031.7+1223  | 307.940 | 12.389  | 56.165  | -15.703 | 0.160      | 0.133      | -85    | 9.7      | 1.2      | 0.2             | 16.2     | 1.9             | 2.40          | 0.09                 | PL  | T   | ...          | 1FGL J2031.5+1219    | ... | bzb   | PKS 2029+121         |
|               |         |         |         |         |            |            |        |          |          |                 |          |                 |               |                      |     |     |              | EGR J2032+1226       |     |       |                      |
| J2032.1+4049  | 308.044 | 40.828  | 79.713  | 0.662   | 0.109      | 0.078      | -10    | 13.6     | 3.8      | 0.9             | 102.2    | 8.4             | 2.48          | ...                  | LP  | T   | 2            | 1AGL J2032+4102      | ... | HMB   | Cyg X-3              |
| J2032.2+4126  | 308.062 | 41.437  | 80.212  | 1.011   | 0.023      | 0.021      | -21    | 36.8     | 21.8     | 0.9             | 143.7    | 8.9             | 2.10          | ...                  | EC  | ... | ...          | 1FGL J2032.2+4127    | E   | PSR   | LAT PSR J2032+4127   |
|               |         |         |         |         |            |            |        |          |          |                 |          |                 |               |                      |     |     |              | 0FGL J2032.2+4122    |     |       |                      |
|               |         |         |         |         |            |            |        |          |          |                 |          |                 |               |                      |     |     |              | 1AGL J2032+4102      |     |       |                      |
| J2033.6+3927  | 308.411 | 39.452  | 78.773  | -0.382  | 0.117      | 0.090      | -74    | 13.0     | 0.7      | 0.1             | 61.2     | 4.7             | 2.77          | ...                  | LP  | ... | 4,12         | 1FGL J2032.8+3928    | ... | ...   | ...                  |
| J2034.7-4201  | 308.687 | -42.031 | 359.088 | -36.392 | 0.093      | 0.090      | -89    | 4.7      | 0.5      | 0.1             | 5.3      | 1.4             | 2.03          | 0.20                 | PL  | ... | ...          | 1FGL J2034.6-4202    | ... | ...   | ...                  |
| J2034.9+3632  | 308.739 | 36.535  | 76.587  | -2.331  | 0.084      | 0.075      | 29     | 5.5      | 1.5      | 0.3             | 17.0     | 3.3             | 2.03          | 0.11                 | PL  | ... | ...          | 1FGL J2034.7+3639    | ... | ...   | ...                  |
| J2035.4+1058  | 308.851 | 10.972  | 55.435  | -17.224 | 0.099      | 0.087      | -48    | 14.4     | 1.5      | 0.2             | 24.3     | 2.0             | 2.55          | 0.07                 | PL  | T   | ...          | 1FGL J2035.4+1100    | ... | bzq   | PKS 2032+107         |
| J2036.0+4224c | 309.021 | 42.415  | 81.422  | 1.023   | 0.170      | 0.120      | -58    | 6.1      | 0.6      | 0.2             | 39.9     | 6.1             | 2.54          | ...                  | LP  | ... | 3,4,5,6,12   | ...                  | ... | ...   | ...                  |
| J2036.6+6551  | 309.166 | 65.857  | 100.650 | 14.760  | 0.106      | 0.085      | 48     | 4.9      | 0.6      | 0.1             | 6.5      | 1.6             | 2.00          | 0.16                 | PL  | ... | ...          | 1FGL J2038.1+6552    | ... | bzb   | 87GB 203539.4+654245 |
| J2038.0+4145c | 309.524 | 41.754  | 81.121  | 0.326   | 0.223      | 0.170      | 89     | 8.8      | 1.1      | 0.3             | 54.2     | 6.6             | 2.64          | ...                  | LP  | ... | 3,4,5,6,8,12 | ...                  | ... | ...   | ...                  |
| J2039.1-1046  | 309.786 | -10.779 | 35.312  | -28.764 | 0.055      | 0.049      | -8     | 17.5     | 2.2      | 0.2             | 24.8     | 2.5             | 1.99          | 0.07                 | PL  | T   | ...          | 1FGL J2039.0-1047    | ... | bzb   | TXS 2036-109         |

Table 1—Continued

| Name 2FGL     | R.A.    | Decl.   | $l$     | $b$     | $\theta_1$ | $\theta_2$ | $\phi$ | $\sigma$ | $F_{35}$ | $\Delta F_{35}$ | $S_{25}$ | $\Delta S_{25}$ | $\Gamma_{25}$ | $\Delta \Gamma_{25}$ | Mod | Var | Flags    | $\gamma$ -ray Assoc. | TeV | Class | ID or Assoc.        |
|---------------|---------|---------|---------|---------|------------|------------|--------|----------|----------|-----------------|----------|-----------------|---------------|----------------------|-----|-----|----------|----------------------|-----|-------|---------------------|
| J2039.6+5218  | 309.913 | 52.314  | 89.704  | 6.511   | 0.082      | 0.072      | 5      | 4.1      | 0.4      | 0.2             | 6.9      | 2.4             | 1.50          | 0.26                 | PL  | ... | ...      | ...                  | ... | bzb   | 1ES 2037+521        |
| J2039.8−5620  | 309.965 | −56.341 | 341.192 | −37.178 | 0.066      | 0.064      | 4      | 17.6     | 2.2      | 0.2             | 24.9     | 2.0             | 2.19          | 0.06                 | PL  | ... | 10       | 1FGL J2039.4−5621    | ... | ...   | ...                 |
| J2040.1+4105c | 310.050 | 41.084  | 80.829  | −0.394  | 0.156      | 0.106      | 16     | 4.5      | 1.9      | 0.4             | 30.1     | 6.1             | 2.54          | 0.13                 | PL  | ... | 4,5,6    | ...                  | ... | ...   | ...                 |
| J2040.2−7109  | 310.058 | −71.151 | 323.278 | −34.261 | 0.129      | 0.117      | −34    | 4.5      | 0.4      | 0.1             | 4.9      | 1.3             | 2.03          | 0.22                 | PL  | ... | ...      | ...                  | ... | agu   | PKS 2035−714        |
| J2041.2+4735  | 310.322 | 47.594  | 86.101  | 3.434   | 0.092      | 0.086      | −66    | 11.7     | 3.6      | 0.4             | 28.8     | 3.1             | 2.30          | ...                  | LP  | ... | ...      | ...                  | ... | ...   | ...                 |
| J2041.5+5003  | 310.376 | 50.066  | 88.085  | 4.916   | 0.153      | 0.136      | −66    | 4.2      | 1.2      | 0.3             | 15.3     | 3.5             | 2.33          | 0.12                 | PL  | ... | 4,5      | ...                  | ... | †     | ...                 |
| J2042.0+4252c | 310.508 | 42.872  | 82.451  | 0.433   | 0.220      | 0.188      | 47     | 9.9      | 0.8      | 0.2             | 47.1     | 4.9             | 2.70          | ...                  | LP  | ... | 2,4,6,12 | ...                  | ... | ...   | ...                 |
| J2042.1+2428  | 310.533 | 24.470  | 67.788  | −10.798 | 0.097      | 0.084      | −49    | 6.2      | 0.6      | 0.1             | 8.1      | 2.1             | 1.73          | 0.17                 | PL  | ... | ...      | 1FGL J2042.2+2427    | ... | bzb   | MG2 J204208+2426    |
| J2042.8−7317  | 310.714 | −73.299 | 320.735 | −33.797 | 0.138      | 0.111      | −14    | 5.1      | 0.5      | 0.1             | 5.7      | 1.3             | 2.28          | 0.21                 | PL  | ... | ...      | 1FGL J2043.0−7317    | ... | ...   | ...                 |
| J2043.2+1711  | 310.809 | 17.184  | 61.897  | −15.296 | 0.049      | 0.047      | −34    | 27.0     | 4.6      | 0.3             | 29.4     | 1.9             | 2.05          | ...                  | EC  | ... | ...      | 1FGL J2043.2+1709    | ... | PSR   | PSR J2043+1710      |
| J2043.3+5105  | 310.838 | 51.099  | 89.085  | 5.317   | 0.156      | 0.140      | 49     | 10.9     | 1.8      | 0.3             | 24.2     | 2.5             | 2.44          | ...                  | LP  | T   | 2,12     | ...                  | ... | †     | ...                 |
| J2043.7+2743  | 310.947 | 27.724  | 70.655  | −9.137  | 0.121      | 0.107      | 23     | 8.8      | 1.4      | 0.2             | 9.3      | 1.6             | 2.30          | ...                  | EC  | ... | ...      | 1FGL J2043.7+2740    | ... | PSR   | PSR J2043+2740      |
| J2044.4−4757  | 311.123 | −47.961 | 351.729 | −38.379 | 0.146      | 0.136      | −52    | 7.3      | 0.8      | 0.1             | 9.6      | 1.6             | 2.22          | 0.12                 | PL  | ... | ...      | ...                  | ... | ...   | ...                 |
| J2046.0+4954  | 311.523 | 49.913  | 88.420  | 4.241   | 0.112      | 0.097      | −83    | 9.3      | 2.4      | 0.4             | 25.3     | 3.4             | 2.35          | ...                  | LP  | ... | ...      | 1FGL J2046.0+4954    | ... | †     | ...                 |
| J2046.2−4259  | 311.565 | −42.988 | 358.090 | −38.580 | 0.135      | 0.120      | 42     | 4.1      | 0.4      | 0.1             | 4.9      | 1.3             | 2.08          | 0.20                 | PL  | ... | ...      | ...                  | ... | ...   | †...                |
| J2046.7+1055  | 311.689 | 10.925  | 57.020  | −19.570 | 0.152      | 0.131      | 48     | 6.2      | 0.8      | 0.2             | 9.4      | 1.7             | 2.26          | 0.13                 | PL  | ... | ...      | 1FGL J2047.6+1055    | ... | psr   | PSR J2047+10        |
| J2047.9+4536c | 312.000 | 45.615  | 85.263  | 1.303   | 0.219      | 0.157      | 53     | 6.7      | 0.6      | 0.2             | 21.7     | 3.1             | 2.60          | ...                  | LP  | ... | 1,4,6,12 | ...                  | ... | ...   | ...                 |
| J2049.8+1001  | 312.453 | 10.021  | 56.674  | −20.700 | 0.148      | 0.131      | −29    | 8.4      | 1.0      | 0.2             | 13.1     | 1.8             | 2.38          | 0.10                 | PL  | T   | ...      | 1FGL J2049.7+1003    | ... | agu   | PKS 2047+098        |
| J2050.0+0408  | 312.503 | 4.150   | 51.391  | −23.957 | 0.110      | 0.094      | 40     | 7.3      | 0.8      | 0.1             | 9.2      | 1.7             | 2.03          | 0.13                 | PL  | ... | ...      | 1FGL J2050.1+0407    | ... | bzb   | PKS 2047+039        |
| J2051.0+3040e | 312.750 | 30.670  | 73.985  | −8.563  | ...        | ...        | ...    | 27.7     | 11.4     | 0.6             | 77.2     | 3.8             | 2.08          | ...                  | EC  | T   | ...      | ...                  | ... | SNR   | SNR G074.0−08.5     |
| Cygnus Loop   |         |         |         |         |            |            |        |          |          |                 |          |                 |               |                      |     |     |          |                      |     |       |                     |
| J2051.8+5054  | 312.955 | 50.906  | 89.769  | 4.156   | 0.092      | 0.091      | −0     | 6.4      | 1.8      | 0.3             | 21.1     | 3.5             | 2.23          | 0.10                 | PL  | ... | 4,5      | 1FGL J2052.2+5059    | ... | ...   | ...                 |
| J2053.2+1212c | 313.323 | 12.212  | 59.114  | −20.154 | 0.121      | 0.110      | −42    | 5.2      | 0.6      | 0.1             | 7.3      | 1.5             | 2.35          | 0.16                 | PL  | ... | 6        | ...                  | ... | ...   | ...                 |
| J2055.4−0023  | 313.861 | −0.398  | 47.870  | −27.487 | 0.097      | 0.082      | 69     | 5.2      | 0.4      | 0.1             | 8.1      | 3.0             | 1.35          | 0.23                 | PL  | ... | ...      | 1FGL J2055.5−0023    | ... | bzb   | 1RXS J205528.2−0021 |
| J2055.8+2539  | 313.960 | 25.664  | 70.690  | −12.526 | 0.037      | 0.037      | 87     | 45.1     | 9.2      | 0.4             | 55.9     | 2.1             | 2.12          | ...                  | EC  | ... | ...      | 1FGL J2055.8+2539    | ... | PSR   | LAT PSR J2055+2539  |
|               |         |         |         |         |            |            |        |          |          |                 |          |                 |               |                      |     |     |          | 0FGL J2055.5+2540    |     |       |                     |
| J2055.8+4754  | 313.967 | 47.909  | 87.891  | 1.728   | 0.216      | 0.098      | 73     | 4.4      | 1.1      | 0.3             | 12.0     | 3.0             | 2.13          | 0.14                 | PL  | ... | 4,9      | ...                  | ... | ...   | ...                 |
| J2056.2−4715  | 314.068 | −47.255 | 352.580 | −40.381 | 0.029      | 0.028      | 90     | 65.9     | 8.6      | 0.4             | 100.8    | 3.0             | 2.35          | ...                  | LP  | T   | ...      | 1FGL J2056.3−4714    | ... | bzq   | PKS 2052−47         |
|               |         |         |         |         |            |            |        |          |          |                 |          |                 |               |                      |     |     |          | 0FGL J2056.1−4715    |     |       |                     |
|               |         |         |         |         |            |            |        |          |          |                 |          |                 |               |                      |     |     |          | 3EG J2055−4716       |     |       |                     |
| J2056.7+4939  | 314.181 | 49.655  | 89.313  | 2.752   | 0.069      | 0.064      | −13    | 5.8      | 1.2      | 0.3             | 14.2     | 3.3             | 1.91          | 0.16                 | PL  | ... | ...      | 1FGL J2056.7+4938    | ... | agu   | RGB J2056+496       |
| J2102.2+4546  | 315.560 | 45.775  | 86.991  | −0.492  | 0.097      | 0.092      | −70    | 11.1     | 2.7      | 0.3             | 27.3     | 3.2             | 2.45          | ...                  | LP  | T   | 3        | ...                  | ... | NOV   | V407 Cyg            |
| J2103.3+4357c | 315.832 | 43.962  | 85.763  | −1.840  | 0.149      | 0.121      | −15    | 8.0      | 1.6      | 0.3             | 25.2     | 3.1             | 2.57          | 0.09                 | PL  | ... | 1,4,6    | ...                  | ... | ...   | ...                 |
| J2103.4+4706  | 315.856 | 47.115  | 88.128  | 0.245   | 0.226      | 0.117      | −70    | 5.5      | 1.5      | 0.3             | 17.0     | 3.3             | 2.03          | 0.12                 | PL  | ... | 1,8,9    | ...                  | ... | agu   | GB6 J2102+4702      |
| J2103.5−1112  | 315.896 | −11.203 | 37.863  | −34.371 | 0.188      | 0.138      | −27    | 5.0      | 0.6      | 0.1             | 6.7      | 1.5             | 2.15          | 0.16                 | PL  | ... | ...      | ...                  | ... | ...   | ...                 |

Table 1—Continued

| Name 2FGL     | R.A.    | Decl.   | $l$     | $b$     | $\theta_1$ | $\theta_2$ | $\phi$ | $\sigma$ | $F_{35}$ | $\Delta F_{35}$ | $S_{25}$ | $\Delta S_{25}$ | $\Gamma_{25}$ | $\Delta \Gamma_{25}$ | Mod | Var | Flags | $\gamma$ -ray Assoc. | TeV | Class | ID or Assoc.          | Ref. |
|---------------|---------|---------|---------|---------|------------|------------|--------|----------|----------|-----------------|----------|-----------------|---------------|----------------------|-----|-----|-------|----------------------|-----|-------|-----------------------|------|
| J2103.6–6236  | 315.921 | –62.610 | 332.639 | –38.920 | 0.076      | 0.065      | –8     | 12.8     | 1.3      | 0.2             | 14.8     | 2.0             | 1.93          | 0.09                 | PL  | ... | ...   | 1FGL J2103.9–6237    | ... | agu   | PMN J2103–6232        | ...  |
| J2104.9+3555  | 316.240 | 35.930  | 79.944  | –7.408  | 0.112      | 0.103      | –82    | 5.4      | 0.8      | 0.2             | 9.5      | 1.9             | 2.35          | 0.14                 | PL  | ... | 1,4   | ...                  | ... | ...   | ...                   | ...  |
| J2107.6+2506  | 316.909 | 25.106  | 71.990  | –14.938 | 0.199      | 0.179      | –52    | 4.2      | 0.5      | 0.1             | 7.1      | 1.6             | 2.40          | 0.16                 | PL  | ... | ...   | ...                  | ... | ...   | ...                   | ...  |
| J2107.8+3652  | 316.963 | 36.882  | 81.051  | –7.208  | 0.095      | 0.080      | 52     | 5.0      | 0.6      | 0.2             | 6.6      | 1.8             | 1.89          | 0.19                 | PL  | ... | ...   | ...                  | ... | ...   | ...                   | ...  |
| J2107.9+5207c | 316.987 | 52.119  | 92.334  | 3.056   | 0.123      | 0.111      | 19     | 12.9     | 3.2      | 0.6             | 36.0     | 3.3             | 2.34          | ...                  | LP  | ... | 2,6   | 1FGL J2107.5+5202c   | ... | ...   | ...                   | ...  |
| J2108.6–1603  | 317.159 | –16.062 | 32.982  | –37.453 | 0.246      | 0.185      | 90     | 4.1      | 0.4      | 0.1             | 5.9      | 1.4             | 2.59          | 0.21                 | PL  | ... | 11    | ...                  | ... | agu   | NVSS J210833–160724   | ...  |
| J2108.7–0246  | 317.180 | –2.780  | 47.451  | –31.556 | 0.114      | 0.093      | 26     | 4.6      | 0.4      | 0.1             | 4.9      | 1.7             | 1.74          | 0.20                 | PL  | ... | ...   | 1FGL J2108.5–0249    | ... | bzb   | TXS 2106–030          | ...  |
| J2108.9–6636  | 317.229 | –66.603 | 327.573 | –38.171 | 0.099      | 0.085      | 33     | 7.1      | 0.6      | 0.1             | 7.2      | 1.6             | 1.88          | 0.15                 | PL  | T   | ...   | 1FGL J2108.6–6646    | ... | agu   | PKS 2104–668          | ...  |
| J2109.9+0807  | 317.498 | 8.131   | 58.085  | –25.868 | 0.121      | 0.116      | 55     | 7.3      | 1.0      | 0.2             | 12.0     | 1.8             | 2.27          | 0.11                 | PL  | T   | ...   | 1FGL J2110.0+0811    | ... | bzq   | PMN J2110+0810        | ...  |
| J2110.3+3822  | 317.590 | 38.369  | 82.495  | –6.575  | 0.127      | 0.115      | 83     | 4.6      | 0.7      | 0.2             | 7.4      | 1.8             | 2.08          | 0.19                 | PL  | ... | ...   | 1FGL J2110.3+3820    | ... | ...   | ...                   | ...  |
| J2111.3+4605  | 317.834 | 46.094  | 88.292  | –1.447  | 0.043      | 0.041      | 18     | 22.2     | 6.4      | 0.4             | 38.8     | 3.1             | 2.07          | ...                  | LP  | ... | ...   | 1FGL J2111.3+4607    | ... | ...   | ...                   | ...  |
|               |         |         |         |         |            |            |        |          |          |                 |          |                 |               |                      |     |     |       | 0FGL J2110.8+4608    |     |       |                       |      |
| J2112.3–4832  | 318.088 | –48.542 | 350.590 | –42.971 | 0.168      | 0.141      | –62    | 5.6      | 0.4      | 0.1             | 7.7      | 1.4             | 2.70          | 0.16                 | PL  | ... | 1     | ...                  | ... | ...   | ...                   | ...  |
| J2112.5+0818  | 318.146 | 8.311   | 58.665  | –26.283 | 0.120      | 0.113      | 25     | 4.7      | 0.6      | 0.2             | 6.6      | 1.7             | 1.94          | 0.19                 | PL  | ... | ...   | ...                  | ... | agu   | 1RXS J211242.5+081831 | ...  |
| J2112.5–3042  | 318.149 | –30.711 | 14.931  | –42.448 | 0.055      | 0.050      | 73     | 19.7     | 3.4      | 0.3             | 18.9     | 2.0             | 2.00          | ...                  | LP  | ... | ...   | 1FGL J2112.5–3044    | ... | ...   | ...                   | ...  |
| J2114.1+5440  | 318.539 | 54.673  | 94.839  | 4.121   | 0.233      | 0.123      | 53     | 4.3      | 1.2      | 0.3             | 13.6     | 2.9             | 2.25          | 0.14                 | PL  | ... | ...   | ...                  | ... | ...   | ...                   | ...  |
| J2115.3+2932  | 318.848 | 29.547  | 76.603  | –13.303 | 0.103      | 0.090      | –2     | 11.1     | 1.3      | 0.2             | 16.7     | 1.8             | 2.33          | 0.08                 | PL  | T   | ...   | 1FGL J2115.5+2937    | ... | bzq   | B2 2113+29            | ...  |
| J2115.4+1213  | 318.859 | 12.220  | 62.596  | –24.504 | 0.145      | 0.114      | –6     | 5.1      | 0.5      | 0.1             | 6.8      | 1.4             | 2.38          | 0.19                 | PL  | ... | ...   | ...                  | ... | ...   | ...                   | ...  |
| J2116.2+3339  | 319.052 | 33.662  | 79.817  | –10.642 | 0.039      | 0.037      | –74    | 20.3     | 2.8      | 0.2             | 34.9     | 3.6             | 1.80          | 0.06                 | PL  | T   | ...   | 1FGL J2116.1+3338    | ... | bzb   | B2 2114+33            | ...  |
| J2117.5+3730  | 319.385 | 37.515  | 82.843  | –8.192  | 0.105      | 0.093      | –90    | 10.5     | 1.8      | 0.2             | 10.8     | 1.6             | 2.14          | ...                  | LP  | ... | ...   | 1FGL J2116.8+3729    | ... | ...   | ...                   | ...  |
| J2120.6–1301  | 320.152 | –13.030 | 37.983  | –38.914 | 0.180      | 0.147      | 83     | 6.7      | 0.6      | 0.1             | 9.2      | 1.5             | 2.47          | 0.13                 | PL  | ... | ...   | 1FGL J2120.2–1259    | ... | agu   | NVSS J212035–125443   | ...  |
| J2121.0+1901  | 320.263 | 19.032  | 69.254  | –21.245 | 0.051      | 0.048      | 80     | 19.5     | 2.3      | 0.2             | 26.9     | 2.1             | 2.20          | 0.06                 | PL  | ... | ...   | 1FGL J2120.9+1901    | ... | bzq   | OX 131                | ...  |
| J2124.0–1513  | 321.023 | –15.223 | 35.813  | –40.569 | 0.256      | 0.238      | –0     | 4.2      | 0.3      | 0.1             | 6.4      | 1.5             | 2.71          | 0.22                 | PL  | T   | 11    | ...                  | ... | ...   | ...                   | ...  |
| J2124.6–3357  | 321.160 | –33.965 | 10.942  | –45.418 | 0.037      | 0.035      | –21    | 37.8     | 7.4      | 0.4             | 37.0     | 1.9             | 1.94          | ...                  | EC  | ... | ...   | 1FGL J2124.7–3358    | ... | PSR   | PSR J2124–3358        | ...  |
|               |         |         |         |         |            |            |        |          |          |                 |          |                 |               |                      |     |     |       | 0FGL J2124.7–3358    |     |       |                       |      |
| J2125.0–4632  | 321.265 | –46.546 | 352.994 | –45.338 | 0.165      | 0.149      | 44     | 6.9      | 0.7      | 0.1             | 9.0      | 1.4             | 2.44          | 0.12                 | PL  | T   | ...   | ...                  | ... | ...   | ...                   | ...  |
| J2127.8+3614  | 321.970 | 36.238  | 83.392  | –10.560 | 0.085      | 0.075      | 47     | 8.7      | 1.1      | 0.2             | 13.9     | 2.6             | 1.74          | 0.12                 | PL  | ... | ...   | ...                  | ... | bzb   | B2 2125+35            | ...  |
| J2128.7+5824  | 322.177 | 58.406  | 98.911  | 5.334   | 0.199      | 0.139      | 54     | 8.4      | 0.6      | 0.3             | 17.3     | 2.2             | 2.52          | ...                  | LP  | ... | 4     | ...                  | ... | ...   | ...                   | ...  |
| J2129.8–0428  | 322.467 | –4.482  | 48.934  | –36.963 | 0.143      | 0.120      | 16     | 7.7      | 0.8      | 0.1             | 9.2      | 1.6             | 2.12          | 0.11                 | PL  | ... | ...   | 1FGL J2129.8–0427    | ... | psr   | PSR J2129–04          | ...  |
| J2131.0–5417  | 322.772 | –54.291 | 341.980 | –44.712 | 0.224      | 0.167      | 51     | 9.0      | 0.6      | 0.1             | 11.7     | 1.4             | 2.74          | 0.12                 | PL  | T   | ...   | ...                  | ... | ...   | ...                   | ...  |
| J2131.6–0914  | 322.922 | –9.242  | 43.925  | –39.688 | 0.091      | 0.081      | –10    | 7.5      | 0.8      | 0.1             | 8.5      | 1.5             | 2.09          | 0.16                 | PL  | ... | ...   | 1FGL J2131.7–0914    | ... | bzb   | RBS 1752              | ...  |
| J2132.5+2605  | 323.139 | 26.085  | 76.691  | –18.439 | 0.140      | 0.119      | –53    | 5.8      | 0.7      | 0.1             | 7.7      | 1.5             | 2.21          | 0.14                 | PL  | ... | ...   | ...                  | ... | ...   | ...                   | ...  |
| J2133.5–6431  | 323.376 | –64.533 | 328.735 | –41.323 | 0.123      | 0.116      | –18    | 6.2      | 0.7      | 0.1             | 8.6      | 1.5             | 2.30          | 0.12                 | PL  | ... | ...   | 1FGL J2134.3–6429    | ... | ...   | ...                   | ...  |
| J2133.8–0154  | 323.466 | –1.906  | 52.319  | –36.449 | 0.118      | 0.108      | –10    | 9.4      | 1.0      | 0.2             | 11.7     | 1.5             | 2.32          | 0.10                 | PL  | ... | ...   | 1FGL J2134.0–0203    | ... | bzb   | PKS 2131–021          | ...  |
| J2133.9+6645  | 323.491 | 66.750  | 105.165 | 10.963  | 0.129      | 0.080      | –45    | 6.7      | 1.0      | 0.2             | 11.2     | 2.1             | 1.94          | 0.13                 | PL  | ... | ...   | ...                  | ... | ...   | ...                   | ...  |

Table 1—Continued

| Name 2FGL    | R.A.    | Decl.   | $l$     | $b$     | $\theta_1$ | $\theta_2$ | $\phi$ | $\sigma$ | $F_{35}$ | $\Delta F_{35}$ | $S_{25}$ | $\Delta S_{25}$ | $\Gamma_{25}$ | $\Delta \Gamma_{25}$ | Mod | Var | Flags | $\gamma$ -ray Assoc. | TeV | Class | ID or Assoc.        | Ref. |
|--------------|---------|---------|---------|---------|------------|------------|--------|----------|----------|-----------------|----------|-----------------|---------------|----------------------|-----|-----|-------|----------------------|-----|-------|---------------------|------|
| J2134.5–6513 | 323.643 | –65.228 | 327.839 | –41.118 | 0.111      | 0.105      | –3     | 4.5      | 0.4      | 0.1             | 4.8      | 1.4             | 1.96          | 0.23                 | PL  | ... | ...   | ...                  | ... | agu   | PKS 2130–654        | ...  |
| J2134.6–2130 | 323.653 | –21.500 | 28.952  | –45.082 | 0.111      | 0.092      | –47    | 7.2      | 0.8      | 0.1             | 8.5      | 1.6             | 2.00          | 0.14                 | PL  | ... | ...   | 1FGL J2134.5–2130    | ... | ...   | ...                 | ...  |
| J2135.6–4959 | 323.919 | –49.992 | 347.675 | –46.476 | 0.191      | 0.128      | 37     | 11.3     | 0.9      | 0.1             | 14.2     | 1.4             | 2.58          | 0.10                 | PL  | ... | ...   | 1FGL J2135.8–4957    | ... | bzq   | PMN J2135–5006      | ...  |
| J2139.1–2054 | 324.786 | –20.916 | 30.204  | –45.912 | 0.134      | 0.106      | 2      | 4.1      | 0.3      | 0.1             | 5.3      | 2.4             | 1.39          | 0.28                 | PL  | ... | ...   | ...                  | ... | bzb   | RBS 1769            | ...  |
| J2139.3–4236 | 324.841 | –42.608 | 358.291 | –48.317 | 0.035      | 0.034      | –29    | 39.1     | 5.6      | 0.3             | 62.0     | 3.2             | 2.10          | 0.03                 | PL  | T   | ...   | 1FGL J2139.3–4235    | ... | bzb   | MH 2136–428         | ...  |
|              |         |         |         |         |            |            |        |          |          |                 |          |                 |               |                      |     |     |       | 0FGL J2139.4–4238    |     |       |                     |      |
| J2139.8+4714 | 324.954 | 47.242  | 92.599  | –4.028  | 0.071      | 0.066      | –41    | 15.5     | 3.2      | 0.3             | 22.2     | 2.1             | 2.31          | ...                  | LP  | ... | ...   | 1FGL J2139.9+4715    | ... | ...   | ...                 | ...  |
| J2141.7–3739 | 325.439 | –37.659 | 5.738   | –49.052 | 0.103      | 0.100      | 40     | 5.8      | 0.6      | 0.1             | 7.3      | 1.3             | 2.39          | 0.15                 | PL  | ... | ...   | ...                  | ... | bzq   | PKS 2138–377        | ...  |
| J2143.2–3929 | 325.822 | –39.497 | 2.914   | –49.295 | 0.115      | 0.095      | –42    | 6.6      | 0.7      | 0.1             | 8.0      | 1.8             | 1.85          | 0.16                 | PL  | ... | ...   | 1FGL J2143.1–3927    | ... | bzb   | PMN J2143–3929      | ...  |
| J2143.5+1743 | 325.879 | 17.720  | 72.094  | –26.079 | 0.047      | 0.043      | –86    | 44.0     | 4.5      | 0.3             | 72.7     | 2.3             | 2.58          | 0.03                 | PL  | T   | ...   | 1FGL J2143.4+1742    | ... | bzq   | OX 169              | ...  |
|              |         |         |         |         |            |            |        |          |          |                 |          |                 |               |                      |     |     |       | 0FGL J2143.2+1741    |     |       |                     |      |
| J2144.8–3356 | 326.214 | –33.940 | 11.467  | –49.595 | 0.061      | 0.059      | 30     | 19.4     | 2.1      | 0.2             | 24.4     | 1.9             | 2.25          | 0.06                 | PL  | T   | ...   | 1FGL J2145.4–3358    | ... | bzq   | PMN J2145–3357      | ...  |
| J2146.5–1530 | 326.627 | –15.510 | 38.346  | –45.656 | 0.330      | 0.265      | 31     | 4.9      | 0.4      | 0.1             | 7.3      | 1.4             | 2.61          | 0.16                 | PL  | ... | ...   | ...                  | ... | bzq   | PKS 2143–156        | ...  |
| J2146.6–1345 | 326.659 | –13.751 | 40.650  | –44.970 | 0.054      | 0.050      | 14     | 12.5     | 1.2      | 0.2             | 16.9     | 3.1             | 1.64          | 0.11                 | PL  | T   | ...   | 1FGL J2146.6–1345    | ... | bzb   | NVSS J214637–134359 | ...  |
| J2147.3+0930 | 326.835 | 9.515   | 65.846  | –32.283 | 0.052      | 0.051      | 9      | 35.9     | 3.5      | 0.2             | 52.4     | 2.1             | 2.51          | 0.04                 | PL  | T   | ...   | 1FGL J2147.2+0929    | ... | bzq   | PKS 2144+092        | ...  |
|              |         |         |         |         |            |            |        |          |          |                 |          |                 |               |                      |     |     |       | 0FGL J2147.1+0931    |     |       |                     |      |
| J2147.4–7534 | 326.869 | –75.579 | 315.816 | –36.556 | 0.048      | 0.044      | –85    | 35.1     | 3.6      | 0.2             | 54.0     | 2.1             | 2.52          | 0.04                 | PL  | T   | ...   | ...                  | ... | bzq   | PKS 2142–75         | ...  |
| J2148.2+0659 | 327.064 | 6.994   | 63.719  | –34.082 | 0.374      | 0.324      | –70    | 5.7      | 0.4      | 0.1             | 8.5      | 1.5             | 2.77          | 0.16                 | PL  | ... | ...   | 1FGL J2148.5+0654    | ... | bzq   | 4C +06.69           | ...  |
| J2149.6+0326 | 327.413 | 3.443   | 60.590  | –36.576 | 0.134      | 0.111      | –48    | 7.4      | 0.8      | 0.1             | 9.2      | 1.6             | 2.10          | 0.12                 | PL  | ... | ...   | 1FGL J2149.7+0327    | ... | bzb   | PKS B2147+031       | ...  |
| J2150.2–1412 | 327.553 | –14.216 | 40.563  | –45.952 | 0.150      | 0.141      | –6     | 4.4      | 0.5      | 0.1             | 5.1      | 1.4             | 2.03          | 0.19                 | PL  | T   | 11    | 1FGL J2150.3–1410    | ... | bzb   | TXS 2147–144        | ...  |
| J2150.8–2738 | 327.703 | –27.645 | 21.404  | –50.132 | 0.193      | 0.169      | –35    | 5.2      | 0.5      | 0.1             | 6.2      | 1.3             | 2.38          | 0.16                 | PL  | T   | 1     | ...                  | ... | bzq   | PMN J2151–2742      | ...  |
| J2151.5–3021 | 327.892 | –30.360 | 17.228  | –50.696 | 0.180      | 0.163      | 79     | 12.4     | 0.6      | 0.1             | 20.5     | 1.8             | 3.00          | 0.09                 | PL  | T   | ...   | ...                  | ... | bzq   | PKS 2149–306        | ...  |
| J2152.4+1735 | 328.102 | 17.590  | 73.648  | –27.686 | 0.109      | 0.106      | –80    | 5.3      | 0.6      | 0.1             | 6.4      | 1.5             | 2.18          | 0.18                 | PL  | ... | ...   | 1FGL J2152.5+1734    | ... | bzb   | S3 2150+17          | ...  |
| J2154.0–1138 | 328.503 | –11.634 | 44.476  | –45.662 | 0.170      | 0.137      | 3      | 10.5     | 0.8      | 0.1             | 13.5     | 1.4             | 2.57          | 0.10                 | PL  | T   | ...   | ...                  | ... | bzq   | PMN J2153–1136      | ...  |
| J2157.4+3129 | 329.365 | 31.499  | 84.780  | –18.195 | 0.079      | 0.074      | –80    | 23.4     | 2.5      | 0.2             | 35.0     | 1.9             | 2.45          | 0.05                 | PL  | T   | ...   | 1FGL J2157.4+3129    | ... | bzq   | B2 2155+31          | ...  |
|              |         |         |         |         |            |            |        |          |          |                 |          |                 |               |                      |     |     |       | 0FGL J2157.5+3125    |     |       |                     |      |
| J2157.9–1501 | 329.483 | –15.023 | 40.610  | –47.986 | 0.113      | 0.096      | 66     | 10.2     | 1.1      | 0.2             | 12.8     | 1.7             | 2.19          | 0.10                 | PL  | T   | ...   | 1FGL J2157.9–1503    | ... | bzq   | PKS 2155–152        | ...  |
| J2158.8–3013 | 329.715 | –30.219 | 17.741  | –52.243 | 0.014      | 0.014      | 44     | 104.0    | 23.5     | 0.6             | 282.8    | 8.9             | 1.84          | 0.02                 | PL  | T   | ...   | 1FGL J2158.8–3013    | P   | bzb   | PKS 2155–304        | ...  |
|              |         |         |         |         |            |            |        |          |          |                 |          |                 |               |                      |     |     |       | 0FGL J2158.8–3014    |     |       |                     |      |
|              |         |         |         |         |            |            |        |          |          |                 |          |                 |               |                      |     |     |       | 3EG J2158–3023       |     |       |                     |      |
|              |         |         |         |         |            |            |        |          |          |                 |          |                 |               |                      |     |     |       | EGR J2200–3015       |     |       |                     |      |
| J2159.9+1023 | 329.983 | 10.398  | 69.104  | –34.000 | 0.214      | 0.160      | 56     | 4.3      | 0.5      | 0.1             | 5.1      | 1.4             | 2.07          | 0.19                 | PL  | ... | ...   | ...                  | ... | bzb   | TXS 2157+102        | ...  |
| J2200.1–6931 | 330.043 | –69.525 | 321.282 | –40.961 | 0.128      | 0.120      | 27     | 7.6      | 0.5      | 0.1             | 8.9      | 1.3             | 2.62          | 0.14                 | PL  | T   | ...   | ...                  | ... | ...   | ...                 | ...  |
| J2201.2+5926 | 330.314 | 59.440  | 102.787 | 3.398   | 0.305      | 0.165      | –58    | 4.6      | 1.1      | 0.2             | 14.2     | 2.9             | 2.40          | 0.12                 | PL  | ... | 4,8,9 | ...                  | ... | ...   | ...                 | ...  |
| J2201.9–8335 | 330.483 | –83.599 | 308.002 | –31.765 | 0.067      | 0.060      | 64     | 24.7     | 2.9      | 0.2             | 34.8     | 2.1             | 2.46          | ...                  | LP  | T   | ...   | 1FGL J2201.6–8327    | ... | bzq   | PKS 2155–83         | ...  |

Table 1—Continued

| Name 2FGL    | R.A.    | Decl.   | $l$     | $b$     | $\theta_1$ | $\theta_2$ | $\phi$ | $\sigma$ | $F_{35}$ | $\Delta F_{35}$ | $S_{25}$ | $\Delta S_{25}$ | $\Gamma_{25}$ | $\Delta \Gamma_{25}$ | Mod | Var | Flags | $\gamma$ -ray Assoc.                                                                          | TeV | Class | ID or Assoc.        | Ref. |
|--------------|---------|---------|---------|---------|------------|------------|--------|----------|----------|-----------------|----------|-----------------|---------------|----------------------|-----|-----|-------|-----------------------------------------------------------------------------------------------|-----|-------|---------------------|------|
| J2202.8+4216 | 330.707 | 42.268  | 92.600  | -10.461 | 0.025      | 0.024      | -61    | 59.3     | 10.5     | 0.4             | 106.6    | 3.3             | 2.26          | ...                  | LP  | T   | ...   | 1FGL J2202.8+4216<br>0FGL J2202.4+4217<br>3EG J2202+4217<br>EGR J2204+4225                    | P   | bzb   | BL Lacertae         | ...  |
| J2203.4+1726 | 330.869 | 17.436  | 75.683  | -29.634 | 0.034      | 0.032      | -60    | 46.5     | 6.5      | 0.3             | 64.2     | 2.9             | 2.23          | ...                  | LP  | T   | ...   | 1FGL J2203.5+1726<br>0FGL J2203.2+1731                                                        | ... | bzq   | PKS 2201+171        | ...  |
| J2204.6+0442 | 331.164 | 4.705   | 64.813  | -38.676 | 0.132      | 0.113      | -10    | 6.7      | 0.6      | 0.1             | 7.5      | 1.3             | 2.23          | 0.12                 | PL  | ... | ...   | 1FGL J2204.6+0442                                                                             | ... | bzb   | 4C +04.77           | ...  |
| J2206.6+6500 | 331.653 | 65.000  | 106.625 | 7.486   | 0.235      | 0.178      | 29     | 12.0     | 1.0      | 0.5             | 21.7     | 2.2             | 2.53          | ...                  | LP  | ... | ...   | ...                                                                                           | ... | bzq   | TXS 2206+650        | ...  |
| J2206.6-0029 | 331.664 | -0.483  | 59.933  | -42.339 | 0.154      | 0.123      | -15    | 5.4      | 0.6      | 0.1             | 6.9      | 1.5             | 2.16          | 0.14                 | PL  | ... | ...   | 1FGL J2207.1-0021                                                                             | ... | bzb   | PMN J2206-0031      | ...  |
| J2208.1-5345 | 332.030 | -53.750 | 339.896 | -49.989 | 0.101      | 0.093      | 55     | 13.8     | 1.2      | 0.2             | 15.5     | 1.4             | 2.42          | 0.09                 | PL  | T   | ...   | 1FGL J2207.8-5344<br>0FGL J2207.0-5347                                                        | ... | bzq   | PKS 2204-54         | ...  |
| J2210.1+5913 | 332.547 | 59.233  | 103.586 | 2.559   | 0.117      | 0.104      | 37     | 5.8      | 1.5      | 0.3             | 18.8     | 3.3             | 2.36          | 0.10                 | PL  | ... | 1,4   | ...                                                                                           | ... | ...   | ...                 | ...  |
| J2211.9+2355 | 332.983 | 23.919  | 82.205  | -26.071 | 0.076      | 0.070      | 71     | 9.2      | 1.0      | 0.2             | 10.9     | 1.8             | 1.99          | 0.11                 | PL  | ... | ...   | 1FGL J2212.1+2358<br>3EG J2209+2401                                                           | ... | bzq   | PKS 2209+236        | ...  |
| J2212.6+0702 | 333.158 | 7.048   | 68.742  | -38.581 | 0.134      | 0.102      | -22    | 9.1      | 1.0      | 0.2             | 11.7     | 1.6             | 2.22          | 0.10                 | PL  | ... | ...   | 1FGL J2212.9+0654                                                                             | ... | ...   | ...                 | ...  |
| J2213.1-2527 | 333.276 | -25.458 | 26.461  | -54.619 | 0.156      | 0.129      | -40    | 9.1      | 0.7      | 0.1             | 10.4     | 1.3             | 2.45          | 0.11                 | PL  | ... | ...   | 1FGL J2213.1-2529                                                                             | ... | bzq   | PKS 2210-25         | ...  |
| J2213.7-4754 | 333.437 | -47.915 | 348.012 | -53.053 | 0.121      | 0.098      | 32     | 4.9      | 0.4      | 0.1             | 4.9      | 1.2             | 2.28          | 0.26                 | PL  | ... | ...   | ...                                                                                           | ... | ...   | ...                 | ...  |
| J2214.7+3000 | 333.691 | 30.013  | 86.879  | -21.679 | 0.039      | 0.039      | 27     | 34.7     | 5.8      | 0.3             | 33.2     | 1.8             | 2.01          | ...                  | EC  | ... | ...   | 1FGL J2214.8+3002<br>0FGL J2214.8+3002                                                        | ... | PSR   | PSR J2214+3000      | ...  |
| J2215.7+5135 | 333.939 | 51.586  | 99.892  | -4.183  | 0.065      | 0.063      | 9      | 11.0     | 1.9      | 0.2             | 10.9     | 1.6             | 2.04          | ...                  | LP  | ... | ...   | 1FGL J2216.1+5139                                                                             | ... | psr   | PSR J2215+51        | ...  |
| J2217.1+2422 | 334.297 | 24.374  | 83.565  | -26.469 | 0.084      | 0.081      | 33     | 8.9      | 0.9      | 0.1             | 10.7     | 1.5             | 2.24          | 0.10                 | PL  | ... | ...   | 1FGL J2217.1+2423                                                                             | ... | bzb   | B2 2214+24B         | ...  |
| J2219.1+1805 | 334.796 | 18.085  | 79.430  | -31.638 | 0.155      | 0.102      | 9      | 5.2      | 0.5      | 0.1             | 5.3      | 1.3             | 2.09          | 0.20                 | PL  | ... | ...   | 1FGL J2219.3+1804                                                                             | ... | bzq   | MG1 J221916+1806    | ...  |
| J2219.6+5850 | 334.913 | 58.835  | 104.370 | 1.545   | 0.181      | 0.102      | -89    | 6.6      | 1.7      | 0.3             | 21.5     | 3.3             | 2.33          | 0.09                 | PL  | ... | 4,5   | ...                                                                                           | ... | ...   | ...                 | ...  |
| J2221.0+6307 | 335.265 | 63.132  | 106.864 | 5.052   | 0.163      | 0.128      | -26    | 11.3     | 1.1      | 0.2             | 23.3     | 2.2             | 2.47          | ...                  | LP  | ... | 2,12  | ...                                                                                           | ... | ...   | ...                 | ...  |
| J2221.6-5223 | 335.421 | -52.384 | 340.408 | -52.421 | 0.091      | 0.086      | -21    | 7.9      | 0.7      | 0.1             | 7.5      | 1.3             | 2.06          | 0.14                 | PL  | ... | ...   | 1FGL J2222.5-5218                                                                             | ... | bzb   | PMN J2221-5224      | ...  |
| J2222.0-3503 | 335.502 | -35.059 | 9.571   | -57.245 | 0.234      | 0.205      | 23     | 4.1      | 0.4      | 0.1             | 4.6      | 1.1             | 2.24          | 0.18                 | PL  | T   | ...   | ...                                                                                           | ... | bzq   | PKS 2220-351        | ...  |
| J2223.4+0104 | 335.860 | 1.070   | 65.256  | -44.599 | 0.085      | 0.072      | -72    | 6.2      | 0.4      | 0.1             | 6.5      | 2.0             | 1.63          | 0.18                 | PL  | ... | ...   | 1FGL J2223.3+0103                                                                             | ... | agu   | NVSS J222329+010226 | ...  |
| J2225.6-0454 | 336.424 | -4.901  | 59.000  | -48.795 | 0.082      | 0.081      | 56     | 21.7     | 2.2      | 0.2             | 30.5     | 1.9             | 2.44          | 0.05                 | PL  | ... | ...   | 1FGL J2225.8-0457                                                                             | ... | bzq   | 3C 446              | ...  |
| J2227.8+0051 | 336.964 | 0.864   | 66.073  | -45.563 | 0.192      | 0.173      | 55     | 4.2      | 0.5      | 0.1             | 5.5      | 1.4             | 2.09          | 0.16                 | PL  | ... | ...   | ...                                                                                           | ... | ...   | ...                 | ...  |
| J2228.6-1633 | 337.168 | -16.551 | 43.216  | -55.363 | 0.114      | 0.088      | -57    | 6.2      | 0.6      | 0.1             | 6.3      | 1.3             | 2.07          | 0.16                 | PL  | ... | ...   | 1FGL J2228.5-1633                                                                             | ... | ...   | ...                 | ...  |
| J2229.0+6114 | 337.267 | 61.246  | 106.651 | 2.959   | 0.017      | 0.016      | 70     | 90.5     | 31.4     | 0.7             | 251.7    | 4.4             | 2.17          | ...                  | EC  | ... | ...   | 1FGL J2229.0+6114<br>0FGL J2229.0+6114<br>3EG J2227+6122<br>EGR J2227+6114<br>1AGL J2231+6109 | E   | PSR   | PSR J2229+6114      | ...  |

Table 1—Continued

| Name 2FGL     | R.A.    | Decl.   | $l$     | $b$     | $\theta_1$ | $\theta_2$ | $\phi$ | $\sigma$ | $F_{35}$ | $\Delta F_{35}$ | $S_{25}$ | $\Delta S_{25}$ | $\Gamma_{25}$ | $\Delta \Gamma_{25}$ | Mod | Var | Flags | $\gamma$ -ray Assoc.                                     | TeV | Class | ID or Assoc.          | Ref. |
|---------------|---------|---------|---------|---------|------------|------------|--------|----------|----------|-----------------|----------|-----------------|---------------|----------------------|-----|-----|-------|----------------------------------------------------------|-----|-------|-----------------------|------|
| J2229.7−0832  | 337.441 | −8.546  | 55.247  | −51.721 | 0.046      | 0.041      | −35    | 48.8     | 4.3      | 0.3             | 68.1     | 2.2             | 2.57          | ...                  | LP  | T   | ...   | 1FGL J2229.7−0832<br>0FGL J2229.8−0829                   | ... | bzq   | PKS 2227−08           | ...  |
| J2231.0+6512  | 337.768 | 65.203  | 108.896 | 6.230   | 0.148      | 0.098      | −11    | 8.3      | 1.5      | 0.2             | 20.3     | 2.6             | 2.42          | 0.08                 | PL  | ... | ...   | ...                                                      | ... | ...   | ...                   | ...  |
| J2232.4+1143  | 338.121 | 11.724  | 77.404  | −38.568 | 0.060      | 0.057      | −87    | 32.3     | 2.9      | 0.2             | 42.1     | 2.0             | 2.54          | ...                  | LP  | T   | ...   | 1FGL J2232.5+1144<br>0FGL J2232.4+1141<br>3EG J2232+1147 | ... | bzq   | CTA 102               | ...  |
| J2234.7+0945  | 338.692 | 9.752   | 76.287  | −40.429 | 0.112      | 0.111      | −7     | 9.7      | 1.1      | 0.2             | 13.0     | 1.7             | 2.23          | 0.10                 | PL  | T   | 3     | 1FGL J2234.8+0944                                        | ... | psr   | PSR J2234+09          | ...  |
| J2234.9−4831  | 338.732 | −48.518 | 344.657 | −56.058 | 0.193      | 0.142      | 6      | 8.3      | 0.6      | 0.1             | 9.2      | 1.2             | 2.55          | 0.13                 | PL  | ... | ...   | 1FGL J2235.7−4817<br>EGR J2233−4812                      | ... | bzq   | PKS 2232−488          | ...  |
| J2236.1−3628  | 339.047 | −36.483 | 6.282   | −59.959 | 0.205      | 0.132      | −70    | 6.8      | 0.6      | 0.1             | 7.2      | 1.3             | 2.23          | 0.14                 | PL  | T   | ...   | ...                                                      | ... | agu   | NVSS J223554−362901   | ...  |
| J2236.4+2828  | 339.102 | 28.476  | 90.120  | −25.659 | 0.037      | 0.037      | 18     | 38.7     | 5.1      | 0.3             | 48.3     | 2.5             | 2.22          | ...                  | LP  | T   | ...   | 1FGL J2236.2+2828                                        | ... | bzb   | B2 2234+28A           | ...  |
| J2236.5−1431  | 339.133 | −14.533 | 47.909  | −56.196 | 0.047      | 0.043      | −55    | 31.5     | 3.9      | 0.3             | 45.1     | 2.4             | 2.24          | 0.04                 | PL  | T   | ...   | 1FGL J2236.4−1432                                        | ... | BZB   | PKS 2233−148          | 29   |
| J2237.2+6316  | 339.307 | 63.270  | 108.498 | 4.223   | 0.135      | 0.112      | 56     | 6.3      | 1.4      | 0.2             | 17.8     | 2.9             | 2.39          | 0.10                 | PL  | ... | 1,4   | ...                                                      | ... | ...   | ...                   | ...  |
| J2237.2−3920  | 339.314 | −39.342 | 0.620   | −59.625 | 0.113      | 0.103      | −38    | 5.7      | 0.5      | 0.1             | 5.3      | 1.2             | 2.07          | 0.17                 | PL  | ... | ...   | 1FGL J2237.2−3919                                        | ... | bzq   | PKS 2234−396          | ...  |
| J2238.4+5902  | 339.608 | 59.049  | 106.552 | 0.474   | 0.044      | 0.040      | 57     | 24.4     | 8.7      | 0.5             | 62.6     | 3.3             | 2.23          | ...                  | EC  | ... | ...   | 1FGL J2238.4+5903                                        | ... | PSR   | LAT PSR J2238+5903    | ...  |
| J2239.8+5825  | 339.966 | 58.427  | 106.413 | −0.160  | 0.147      | 0.128      | 29     | 4.2      | 1.3      | 0.3             | 8.4      | 2.1             | 2.20          | ...                  | EC  | ... | 5     | ...                                                      | ... | PSR   | PSR J2240+5832        | ...  |
| J2241.7−5236  | 340.448 | −52.616 | 337.436 | −54.935 | 0.037      | 0.035      | 42     | 36.0     | 5.5      | 0.3             | 34.1     | 1.9             | 2.00          | ...                  | EC  | ... | ...   | 1FGL J2241.9−5236<br>0FGL J2241.7−5239                   | ... | PSR   | PSR J2241−5236        | ...  |
| J2243.2−2540  | 340.814 | −25.683 | 28.461  | −61.339 | 0.087      | 0.079      | 80     | 16.9     | 1.6      | 0.2             | 19.7     | 1.6             | 2.30          | 0.07                 | PL  | ... | ...   | 1FGL J2243.1−2541                                        | ... | bzb   | PKS 2240−260          | ...  |
| J2243.9+2021  | 340.998 | 20.356  | 86.590  | −33.372 | 0.038      | 0.034      | 69     | 29.4     | 3.9      | 0.3             | 50.6     | 4.3             | 1.75          | 0.05                 | PL  | T   | ...   | 1FGL J2244.0+2021                                        | ... | bzb   | RGB J2243+203         | ...  |
| J2244.1+4059  | 341.029 | 40.988  | 98.497  | −15.765 | 0.066      | 0.058      | 88     | 19.2     | 2.6      | 0.2             | 31.1     | 2.2             | 2.28          | 0.05                 | PL  | T   | ...   | 1FGL J2243.4+4104                                        | ... | bzb   | TXS 2241+406          | ...  |
| J2246.3+1549  | 341.585 | 15.825  | 83.972  | −37.408 | 0.111      | 0.097      | 58     | 8.2      | 1.0      | 0.2             | 18.4     | 3.0             | 2.63          | 0.13                 | PL  | T   | ...   | 1FGL J2246.3+1549<br>3EG J2243+1509                      | ... | ...   | ...                   | ...  |
| J2246.8−5203  | 341.712 | −52.057 | 337.480 | −55.888 | 0.144      | 0.132      | 66     | 4.9      | 0.4      | 0.1             | 6.0      | 1.9             | 1.69          | 0.21                 | PL  | ... | ...   | ...                                                      | ... | agu   | 1RXS J224642.0−520638 | ...  |
| J2247.2−0002  | 341.811 | −0.049  | 70.020  | −49.718 | 0.107      | 0.088      | 53     | 7.5      | 0.8      | 0.1             | 9.1      | 1.6             | 2.13          | 0.12                 | PL  | ... | ...   | 1FGL J2247.3+0000                                        | ... | bzb   | PKS 2244−002          | ...  |
| J2247.8+4412  | 341.969 | 44.211  | 100.717 | −13.266 | 0.100      | 0.080      | 46     | 5.4      | 0.5      | 0.1             | 6.3      | 1.7             | 1.81          | 0.19                 | PL  | ... | 8     | ...                                                      | ... | agu   | NVSS J224753+441317   | ...  |
| J2249.1+5758  | 342.293 | 57.978  | 107.286 | −1.130  | 0.129      | 0.104      | −8     | 5.3      | 1.1      | 0.2             | 12.3     | 2.5             | 1.99          | 0.14                 | PL  | ... | ...   | ...                                                      | ... | ...   | ...                   | ...  |
| J2250.0+3825  | 342.512 | 38.419  | 98.251  | −18.566 | 0.052      | 0.049      | 1      | 10.3     | 1.1      | 0.2             | 13.2     | 2.2             | 1.84          | 0.11                 | PL  | ... | ...   | 1FGL J2250.1+3825                                        | P   | bzb   | B3 2247+381           | ...  |
| J2250.2−4205  | 342.568 | −42.093 | 353.809 | −61.154 | 0.125      | 0.095      | −73    | 6.7      | 0.6      | 0.1             | 7.5      | 2.0             | 1.73          | 0.15                 | PL  | ... | ...   | ...                                                      | ... | agu   | PMN J2250−4206        | ...  |
| J2250.7+6305c | 342.688 | 63.095  | 109.764 | 3.351   | 0.115      | 0.085      | −3     | 5.7      | 1.3      | 0.2             | 16.8     | 3.0             | 2.39          | 0.11                 | PL  | ... | 3,4,6 | ...                                                      | ... | ...   | ...                   | ...  |
| J2250.8−2808  | 342.711 | −28.141 | 23.691  | −63.340 | 0.048      | 0.043      | −45    | 27.6     | 3.4      | 0.2             | 38.3     | 2.3             | 2.20          | 0.05                 | PL  | T   | ...   | 1FGL J2250.8−2809                                        | ... | agn   | PMN J2250−2806        | ...  |
| J2251.1−4927  | 342.782 | −49.464 | 340.731 | −57.896 | 0.169      | 0.115      | 49     | 5.9      | 0.5      | 0.1             | 6.0      | 1.5             | 1.86          | 0.15                 | PL  | ... | 8     | 1FGL J2251.2−4928                                        | ... | ...   | ...                   | ...  |
| J2251.8+4211  | 342.957 | 42.185  | 100.403 | −15.395 | 0.189      | 0.168      | −73    | 4.6      | 0.5      | 0.1             | 8.0      | 1.7             | 2.51          | 0.14                 | PL  | ... | ...   | ...                                                      | ... | ...   | ...                   | ...  |
| J2251.9+4032  | 342.985 | 40.536  | 99.631  | −16.867 | 0.115      | 0.094      | 35     | 8.2      | 1.0      | 0.2             | 11.4     | 1.7             | 2.13          | 0.11                 | PL  | ... | ...   | 1FGL J2251.7+4030                                        | ... | bzb   | CRATES J2251+4030     | ...  |
| J2253.9+1609  | 343.497 | 16.153  | 86.122  | −38.184 | 0.010      | 0.010      | −65    | 339.4    | 96.5     | 1.0             | 1201.7   | 7.8             | 2.38          | ...                  | LP  | T   | ...   | 1FGL J2253.9+1608                                        | ... | BZQ   | 3C 454.3              | ...  |

Table 1—Continued

| Name 2FGL     | R.A.    | Decl.   | $l$     | $b$     | $\theta_1$ | $\theta_2$ | $\phi$ | $\sigma$ | $F_{35}$ | $\Delta F_{35}$ | $S_{25}$ | $\Delta S_{25}$ | $\Gamma_{25}$ | $\Delta \Gamma_{25}$ | Mod | Var | Flags | $\gamma$ -ray Assoc. | TeV | Class | ID or Assoc.          | Ref. |
|---------------|---------|---------|---------|---------|------------|------------|--------|----------|----------|-----------------|----------|-----------------|---------------|----------------------|-----|-----|-------|----------------------|-----|-------|-----------------------|------|
|               |         |         |         |         |            |            |        |          |          |                 |          |                 |               |                      |     |     |       | 0FGL J2254.0+1609    |     |       |                       |      |
|               |         |         |         |         |            |            |        |          |          |                 |          |                 |               |                      |     |     |       | 3EG J2254+1601       |     |       |                       |      |
|               |         |         |         |         |            |            |        |          |          |                 |          |                 |               |                      |     |     |       | EGR J2253+1606       |     |       |                       |      |
|               |         |         |         |         |            |            |        |          |          |                 |          |                 |               |                      |     |     |       | 1AGL J2254+1602      |     |       |                       |      |
| J2254.1+1401  | 343.531 | 14.031  | 84.620  | -39.957 | 0.169      | 0.132      | 48     | 5.5      | 0.8      | 0.2             | 8.7      | 1.9             | 2.22          | 0.15                 | PL  | T   | 10    | ...                  | ... | bzb   | BZB J2253+1404        | ...  |
| J2255.2+2408  | 343.813 | 24.146  | 91.602  | -31.564 | 0.114      | 0.092      | 83     | 9.9      | 1.1      | 0.2             | 12.1     | 1.8             | 2.00          | 0.10                 | PL  | T   | ...   | ...                  | ... | bzb   | BZB J2255+2410        | ...  |
| J2256.4-2009  | 344.112 | -20.154 | 41.580  | -62.826 | 0.116      | 0.092      | -80    | 8.4      | 0.8      | 0.1             | 8.6      | 1.5             | 2.01          | 0.12                 | PL  | ... | ...   | 1FGL J2256.3-2009    | ... | bzb   | PKS 2254-204          | ...  |
| J2256.9-1023  | 344.242 | -10.391 | 59.269  | -58.288 | 0.104      | 0.100      | -85    | 9.0      | 0.9      | 0.1             | 10.1     | 1.4             | 2.19          | 0.10                 | PL  | ... | 10    | 1FGL J2256.9-1024    | ... | psr   | PSR J2256-10          | ...  |
| J2257.5+6222c | 344.387 | 62.383  | 110.154 | 2.371   | 0.142      | 0.117      | 15     | 7.4      | 2.3      | 0.4             | 14.4     | 2.6             | 2.24          | ...                  | LP  | ... | 6     | ...                  | ... | ...   | ...                   | ...  |
| J2257.9-3646  | 344.481 | -36.767 | 3.899   | -64.186 | 0.136      | 0.105      | 23     | 5.3      | 0.4      | 0.1             | 4.9      | 1.4             | 1.89          | 0.19                 | PL  | ... | ...   | 1FGL J2257.9-3643    | ... | ...   | ...                   | ...  |
| J2258.0-2759  | 344.506 | -27.995 | 24.331  | -64.906 | 0.058      | 0.058      | -33    | 29.2     | 2.9      | 0.2             | 35.6     | 1.9             | 2.44          | ...                  | LP  | T   | ...   | 1FGL J2258.0-2757    | ... | bzq   | PKS 2255-282          | ...  |
|               |         |         |         |         |            |            |        |          |          |                 |          |                 |               |                      |     |     |       | EGR J2258-2745       |     |       |                       |      |
| J2258.8-5524  | 344.717 | -55.411 | 330.893 | -55.175 | 0.170      | 0.150      | -24    | 4.3      | 0.4      | 0.1             | 4.4      | 1.4             | 1.81          | 0.24                 | PL  | ... | ...   | 1FGL J2258.9-5525    | ... | bzb   | PMN J2258-5526        | ...  |
| J2259.0-8254  | 344.761 | -82.906 | 306.924 | -33.329 | 0.117      | 0.105      | 21     | 5.5      | 0.7      | 0.1             | 8.1      | 1.6             | 2.32          | 0.15                 | PL  | ... | ...   | 1FGL J2259.9-8255    | ... | ...   | ...                   | ...  |
| J2300.0-3553  | 345.010 | -35.895 | 5.649   | -64.798 | 0.211      | 0.182      | -89    | 4.6      | 0.4      | 0.1             | 5.3      | 1.2             | 2.36          | 0.18                 | PL  | ... | ...   | ...                  | ... | ...   | ...                   | ...  |
| J2300.6+3139  | 345.155 | 31.654  | 96.913  | -25.559 | 0.079      | 0.068      | 33     | 9.1      | 0.8      | 0.1             | 9.6      | 1.7             | 1.91          | 0.12                 | PL  | ... | ...   | 1FGL J2300.4+3138    | ... | bzb   | NVSS J2300.22+313703  | ...  |
| J2302.7+4443  | 345.698 | 44.720  | 103.403 | -13.992 | 0.035      | 0.033      | 24     | 35.9     | 7.2      | 0.4             | 39.9     | 2.1             | 1.94          | ...                  | EC  | ... | ...   | 1FGL J2302.8+4443    | ... | PSR   | PSR J2302+4442        | ...  |
|               |         |         |         |         |            |            |        |          |          |                 |          |                 |               |                      |     |     |       | 0FGL J2302.9+4443    |     |       |                       |      |
| J2304.7+3703  | 346.177 | 37.066  | 100.350 | -21.081 | 0.092      | 0.082      | 86     | 5.5      | 0.5      | 0.1             | 6.5      | 1.9             | 1.66          | 0.20                 | PL  | ... | ...   | 1FGL J2304.3+3709    | ... | bzb   | 1RXS J230437.1+370506 | ...  |
|               |         |         |         |         |            |            |        |          |          |                 |          |                 |               |                      |     |     |       | EGR J2308+3645       |     |       |                       |      |
| J2308.0+1457  | 347.016 | 14.952  | 89.006  | -41.011 | 0.120      | 0.099      | 28     | 9.6      | 1.2      | 0.2             | 14.7     | 1.9             | 2.28          | 0.11                 | PL  | ... | ...   | 1FGL J2307.3+1452    | ... | bzb   | MG1 J230734+1449      | ...  |
| J2309.8-3627  | 347.473 | -36.459 | 3.124   | -66.585 | 0.164      | 0.116      | 35     | 6.5      | 0.6      | 0.1             | 8.0      | 2.2             | 1.65          | 0.16                 | PL  | ... | ...   | 1FGL J2310.0-3627    | ... | agu   | 1RXS J230940.6-363241 | ...  |
| J2310.9+0204  | 347.743 | 2.077   | 79.296  | -52.072 | 0.079      | 0.077      | -46    | 6.1      | 0.5      | 0.1             | 6.0      | 1.3             | 2.07          | 0.17                 | PL  | T   | ...   | 1FGL J2310.9+0204    | ... | bzb   | NVSS J231101+020504   | ...  |
| J2311.0+3425  | 347.771 | 34.430  | 100.420 | -24.017 | 0.042      | 0.040      | 77     | 36.1     | 4.3      | 0.3             | 45.7     | 2.2             | 2.32          | ...                  | LP  | T   | ...   | 1FGL J2311.0+3425    | ... | bzq   | B2 2308+34            | ...  |
| J2314.0+1446  | 348.514 | 14.769  | 90.552  | -41.899 | 0.069      | 0.066      | -24    | 8.6      | 0.8      | 0.2             | 10.0     | 2.0             | 1.81          | 0.14                 | PL  | ... | ...   | 1FGL J2314.1+1444    | ... | bzb   | RGB J2313+147         | ...  |
| J2315.7-5014  | 348.949 | -50.242 | 334.762 | -60.561 | 0.162      | 0.124      | 52     | 7.3      | 0.7      | 0.1             | 7.7      | 1.3             | 2.24          | 0.14                 | PL  | ... | ...   | 1FGL J2315.9-5014    | ... | bzb   | PKS 2312-505          | ...  |
| J2317.3-4534  | 349.331 | -45.569 | 342.115 | -63.748 | 0.113      | 0.099      | 89     | 10.0     | 1.0      | 0.1             | 10.6     | 1.6             | 2.07          | 0.12                 | PL  | ... | ...   | ...                  | ... | agu   | 1RXS J231733.0-453348 | ...  |
| J2319.1-4208  | 349.780 | -42.139 | 348.392 | -65.931 | 0.139      | 0.123      | 47     | 4.4      | 0.3      | 0.1             | 4.8      | 2.1             | 1.59          | 0.42                 | PL  | ... | 8     | ...                  | ... | bzb   | PKS 2316-423          | ...  |
| J2319.3-3830  | 349.833 | -38.513 | 356.511 | -67.644 | 0.190      | 0.145      | -79    | 4.5      | 0.4      | 0.1             | 4.8      | 1.2             | 2.20          | 0.26                 | PL  | ... | ...   | ...                  | ... | ...   | ...                   | ...  |
| J2321.0+2737  | 350.259 | 27.621  | 99.499  | -31.104 | 0.200      | 0.172      | 9      | 6.5      | 0.7      | 0.1             | 8.6      | 1.4             | 2.31          | 0.13                 | PL  | ... | ...   | 1FGL J2321.6+2726    | ... | bzq   | 4C +27.50             | ...  |
| J2322.2+3206  | 350.551 | 32.104  | 101.764 | -27.073 | 0.101      | 0.097      | -86    | 12.4     | 1.4      | 0.2             | 16.6     | 1.7             | 2.27          | 0.08                 | PL  | T   | ...   | 1FGL J2322.0+3208    | ... | bzq   | B2 2319+31            | ...  |
| J2322.6+3435  | 350.672 | 34.588  | 102.903 | -24.808 | 0.075      | 0.063      | -78    | 5.3      | 0.4      | 0.1             | 5.6      | 1.6             | 1.74          | 0.24                 | PL  | ... | ...   | 1FGL J2322.6+3435    | ... | bzb   | TXS 2320+343          | ...  |
| J2323.0-4918  | 350.764 | -49.313 | 334.479 | -62.050 | 0.122      | 0.109      | -1     | 4.2      | 0.3      | 0.1             | 4.2      | 1.4             | 1.80          | 0.24                 | PL  | ... | ...   | 1FGL J2323.0-4919    | ... | agu   | 1RXS J232256.7-491658 | ...  |
| J2323.4+5849  | 350.856 | 58.830  | 111.743 | -2.117  | 0.030      | 0.029      | -21    | 22.8     | 5.8      | 0.4             | 43.3     | 3.8             | 1.81          | ...                  | LP  | ... | ...   | 1FGL J2323.4+5849    | P   | snr   | SNR G111.7-02.1       | ...  |
| J2323.6-0316  | 350.908 | -3.282  | 77.784  | -58.235 | 0.072      | 0.069      | -6     | 21.4     | 2.1      | 0.2             | 27.8     | 1.8             | 2.39          | 0.05                 | PL  | T   | ...   | 1FGL J2323.5-0315    | ... | bzq   | PKS 2320-035          | ...  |

Table 1—Continued

| Name              | 2FGL    | R.A.    | Decl.   | $l$     | $b$   | $\theta_1$ | $\theta_2$ | $\phi$ | $\sigma$ | $F_{35}$ | $\Delta F_{35}$ | $S_{25}$ | $\Delta S_{25}$ | $\Gamma_{25}$ | $\Delta \Gamma_{25}$ | Mod | Var  | Flags             | $\gamma$ -ray Assoc. | TeV | Class                 | ID or Assoc. | Ref. |  |  |  |  |  |  |  |  |  |
|-------------------|---------|---------|---------|---------|-------|------------|------------|--------|----------|----------|-----------------|----------|-----------------|---------------|----------------------|-----|------|-------------------|----------------------|-----|-----------------------|--------------|------|--|--|--|--|--|--|--|--|--|
| 3EG J2321−0328    |         |         |         |         |       |            |            |        |          |          |                 |          |                 |               |                      |     |      |                   |                      |     |                       |              |      |  |  |  |  |  |  |  |  |  |
| J2323.8+4212      | 350.954 | 42.200  | 106.060 | −17.783 | 0.046 | 0.040      | 70         | 20.3   | 2.5      | 0.2      | 29.7            | 2.9      | 1.88            | 0.06          | PL                   | T   | ...  | 1FGL J2323.5+4211 | ...                  | bzb | 1ES 2321+419          | ...          |      |  |  |  |  |  |  |  |  |  |
| J2324.6+0801      | 351.168 | 8.017   | 88.985  | −49.051 | 0.101 | 0.085      | 15         | 6.6    | 0.7      | 0.1      | 7.3             | 1.5      | 2.12            | 0.17          | PL                   | ... | ...  | ...               | ...                  | agu | PMN J2324+0801        | ...          |      |  |  |  |  |  |  |  |  |  |
| J2324.7−4042      | 351.188 | −40.702 | 350.145 | −67.575 | 0.068 | 0.056      | 31         | 12.9   | 1.6      | 0.2      | 19.4            | 2.8      | 1.81            | 0.10          | PL                   | ... | ...  | ...               | ...                  | bzb | 1ES 2322−409          | ...          |      |  |  |  |  |  |  |  |  |  |
| J2325.3+3957      | 351.331 | 39.959  | 105.517 | −19.983 | 0.043 | 0.043      | 57         | 19.1   | 2.3      | 0.2      | 26.1            | 2.4      | 1.99            | 0.06          | PL                   | T   | ...  | 1FGL J2325.2+3957 | ...                  | bzb | B3 2322+396           | ...          |      |  |  |  |  |  |  |  |  |  |
| 0FGL J2325.3+3959 |         |         |         |         |       |            |            |        |          |          |                 |          |                 |               |                      |     |      |                   |                      |     |                       |              |      |  |  |  |  |  |  |  |  |  |
| J2325.3−3557      | 351.349 | −35.957 | 1.813   | −69.715 | 0.058 | 0.053      | −61        | 25.9   | 2.9      | 0.2      | 23.4            | 1.8      | 2.20            | ...           | LP                   | T   | ...  | 1FGL J2325.5−3559 | ...                  | bzq | CTS 0490              | ...          |      |  |  |  |  |  |  |  |  |  |
| J2325.4+1650      | 351.362 | 16.848  | 95.089  | −41.329 | 0.137 | 0.122      | 79         | 4.2    | 0.4      | 0.1      | 4.5             | 1.2      | 2.12            | 0.21          | PL                   | ... | ...  | ...               | ...                  | agu | NVSS J232538+164641   | ...          |      |  |  |  |  |  |  |  |  |  |
| J2325.4−4758      | 351.367 | −47.981 | 335.963 | −63.262 | 0.074 | 0.070      | 58         | 8.7    | 0.9      | 0.1      | 10.2            | 1.6      | 2.24            | 0.15          | PL                   | ... | ...  | 1FGL J2325.6−4758 | ...                  | bzb | PKS 2322−482          | ...          |      |  |  |  |  |  |  |  |  |  |
| J2327.5+0940      | 351.891 | 9.681   | 91.153  | −47.948 | 0.075 | 0.071      | 52         | 24.9   | 2.0      | 0.2      | 36.2            | 2.2      | 2.64            | ...           | LP                   | T   | ...  | 1FGL J2327.7+0943 | ...                  | bzq | PKS 2325+093          | ...          |      |  |  |  |  |  |  |  |  |  |
| 0FGL J2327.3+0947 |         |         |         |         |       |            |            |        |          |          |                 |          |                 |               |                      |     |      |                   |                      |     |                       |              |      |  |  |  |  |  |  |  |  |  |
| J2327.9−4037      | 351.985 | −40.624 | 349.495 | −68.133 | 0.080 | 0.077      | 53         | 9.8    | 1.2      | 0.2      | 17.6            | 1.9      | 2.46            | 0.08          | PL                   | T   | ...  | ...               | ...                  | agu | PKS 2325−408          | ...          |      |  |  |  |  |  |  |  |  |  |
| J2329.2+3755      | 352.308 | 37.926  | 105.536 | −22.153 | 0.059 | 0.057      | −21        | 9.4    | 0.9      | 0.2      | 11.4            | 2.1      | 1.83            | 0.13          | PL                   | ... | ...  | 1FGL J2329.2+3755 | ...                  | bzb | NVSS J232914+375414   | ...          |      |  |  |  |  |  |  |  |  |  |
| J2329.2−4956      | 352.317 | −49.939 | 331.996 | −62.297 | 0.036 | 0.034      | 5          | 46.8   | 5.7      | 0.3      | 65.9            | 2.6      | 2.36            | ...           | LP                   | T   | ...  | 1FGL J2329.2−4954 | ...                  | bzq | PKS 2326−502          | ...          |      |  |  |  |  |  |  |  |  |  |
| J2329.7−4744      | 352.448 | −47.741 | 335.211 | −63.950 | 0.283 | 0.186      | −13        | 4.1    | 0.4      | 0.1      | 6.8             | 1.8      | 2.58            | 0.21          | PL                   | ... | 5    | 1FGL J2330.3−4745 | ...                  | bzq | PKS 2326−477          | ...          |      |  |  |  |  |  |  |  |  |  |
| J2330.2+1107      | 352.552 | 11.131  | 93.000  | −46.965 | 0.385 | 0.281      | −22        | 4.6    | 0.4      | 0.1      | 7.8             | 1.7      | 2.75            | 0.18          | PL                   | ... | 9    | ...               | ...                  | bzq | 4C +10.73             | ...          |      |  |  |  |  |  |  |  |  |  |
| J2330.6−3723      | 352.656 | −37.388 | 356.790 | −70.136 | 0.119 | 0.108      | 31         | 4.8    | 0.4      | 0.1      | 4.4             | 1.2      | 2.09            | 0.22          | PL                   | ... | ...  | ...               | ...                  | bzb | PKS 2327−376          | ...          |      |  |  |  |  |  |  |  |  |  |
| J2330.9−2144      | 352.750 | −21.744 | 44.956  | −70.942 | 0.069 | 0.061      | −6         | 24.0   | 2.2      | 0.2      | 28.7            | 1.7      | 2.39            | 0.05          | PL                   | T   | ...  | 1FGL J2331.0−2145 | ...                  | bzq | PMN J2331−2148        | ...          |      |  |  |  |  |  |  |  |  |  |
| J2331.8−1607      | 352.961 | −16.126 | 59.669  | −68.525 | 0.168 | 0.146      | −42        | 6.2    | 0.6      | 0.1      | 6.7             | 1.3      | 2.13            | 0.13          | PL                   | T   | ...  | ...               | ...                  | bzq | PKS 2329−16           | ...          |      |  |  |  |  |  |  |  |  |  |
| J2332.5−5535      | 353.143 | −55.587 | 324.129 | −58.176 | 0.143 | 0.131      | 16         | 7.2    | 0.6      | 0.1      | 7.1             | 1.3      | 2.10            | 0.14          | PL                   | ... | ...  | 1FGL J2333.0−5535 | ...                  | ... | ...                   | ...          |      |  |  |  |  |  |  |  |  |  |
| J2333.3+6237      | 353.326 | 62.620  | 114.086 | 1.098   | 0.121 | 0.108      | 18         | 4.8    | 1.0      | 0.2      | 13.8            | 2.7      | 2.40            | 0.12          | PL                   | ... | 4,10 | ...               | ...                  | †   | ...                   | ...          |      |  |  |  |  |  |  |  |  |  |
| J2334.3+0734      | 353.581 | 7.580   | 91.904  | −50.587 | 0.136 | 0.125      | 14         | 9.1    | 0.9      | 0.1      | 11.7            | 1.5      | 2.38            | 0.11          | PL                   | T   | ...  | 1FGL J2334.3+0735 | ...                  | bzq | TXS 2331+073          | ...          |      |  |  |  |  |  |  |  |  |  |
| J2334.8+1431      | 353.718 | 14.526  | 96.560  | −44.390 | 0.068 | 0.061      | 22         | 10.9   | 1.1      | 0.2      | 13.2            | 2.2      | 1.82            | 0.10          | PL                   | T   | ...  | 1FGL J2334.7+1429 | ...                  | bzb | BZB J2334+1408        | ...          |      |  |  |  |  |  |  |  |  |  |
| J2336.3−4111      | 354.078 | −41.186 | 345.786 | −69.130 | 0.089 | 0.084      | 5          | 13.5   | 1.3      | 0.2      | 15.3            | 1.6      | 2.23            | 0.08          | PL                   | T   | ...  | ...               | ...                  | bzq | PKS 2333−415          | ...          |      |  |  |  |  |  |  |  |  |  |
| J2338.1−0229      | 354.536 | −2.486  | 84.361  | −59.751 | 0.082 | 0.076      | −10        | 18.9   | 1.7      | 0.2      | 23.9            | 1.7      | 2.44            | 0.06          | PL                   | T   | ...  | 1FGL J2338.3−0231 | ...                  | bzq | PKS 2335−027          | ...          |      |  |  |  |  |  |  |  |  |  |
| J2339.0+2125      | 354.769 | 21.423  | 101.292 | −38.389 | 0.093 | 0.085      | 16         | 5.9    | 0.4      | 0.1      | 5.9             | 1.7      | 1.71            | 0.26          | PL                   | ... | ...  | 1FGL J2339.0+2123 | ...                  | bzb | RX J2338.8+2124       | ...          |      |  |  |  |  |  |  |  |  |  |
| J2339.6−0532      | 354.909 | −5.542  | 81.358  | −62.467 | 0.041 | 0.039      | 24         | 32.2   | 4.8      | 0.3      | 30.5            | 2.3      | 1.97            | ...           | LP                   | ... | ...  | 1FGL J2339.7−0531 | ...                  | ... | ...                   | ...          |      |  |  |  |  |  |  |  |  |  |
| 0FGL J2339.8−0530 |         |         |         |         |       |            |            |        |          |          |                 |          |                 |               |                      |     |      |                   |                      |     |                       |              |      |  |  |  |  |  |  |  |  |  |
| J2341.7+8016      | 355.426 | 80.270  | 119.884 | 17.814  | 0.041 | 0.039      | −82        | 20.5   | 2.6      | 0.2      | 30.9            | 2.8      | 1.87            | 0.05          | PL                   | ... | ...  | 1FGL J2341.6+8015 | ...                  | bzb | 1RXS J234051.4+801513 | ...          |      |  |  |  |  |  |  |  |  |  |
| J2343.3−4752      | 355.836 | −47.869 | 331.049 | −65.372 | 0.151 | 0.133      | 51         | 6.8    | 0.6      | 0.1      | 6.8             | 1.2      | 2.25            | 0.14          | PL                   | ... | 2    | ...               | ...                  | ... | ...                   | ...          |      |  |  |  |  |  |  |  |  |  |
| J2343.6+3437      | 355.904 | 34.627  | 107.421 | −26.193 | 0.125 | 0.093      | −58        | 4.2    | 0.3      | 0.1      | 4.5             | 1.8      | 1.47            | 0.27          | PL                   | ... | ...  | 1FGL J2343.6+3437 | ...                  | bzb | 1RXS J234332.5+343957 | ...          |      |  |  |  |  |  |  |  |  |  |
| J2345.0−1553      | 356.269 | −15.887 | 65.689  | −70.941 | 0.050 | 0.045      | −83        | 29.0   | 4.2      | 0.3      | 48.5            | 2.7      | 2.19            | 0.04          | PL                   | T   | ...  | 1FGL J2344.6−1554 | ...                  | BZQ | PMN J2345−1555        | 30           |      |  |  |  |  |  |  |  |  |  |
| 0FGL J2345.5−1559 |         |         |         |         |       |            |            |        |          |          |                 |          |                 |               |                      |     |      |                   |                      |     |                       |              |      |  |  |  |  |  |  |  |  |  |
| J2347.0+5142      | 356.759 | 51.705  | 112.885 | −9.906  | 0.042 | 0.037      | −15        | 14.5   | 1.5      | 0.2      | 20.6            | 2.9      | 1.72            | 0.08          | PL                   | ... | ...  | 1FGL J2347.1+5142 | P                    | bzb | 1ES 2344+514          | ...          |      |  |  |  |  |  |  |  |  |  |
| J2347.2+0707      | 356.806 | 7.123   | 96.215  | −52.385 | 0.099 | 0.084      | 75         | 7.2    | 0.7      | 0.1      | 8.4             | 1.7      | 1.96            | 0.16          | PL                   | ... | ...  | 1FGL J2347.3+0710 | ...                  | ... | ...                   | ...          |      |  |  |  |  |  |  |  |  |  |



## REFERENCES

- Abdo, A. A., et al. 2009a, *ApJ*, 706, L1
- . 2009b, *ApJ*, 699, 976
- . 2009c, *ApJ*, 697, 934
- . 2009d, *ApJ*, 707, 727
- . 2010a, *Nature*, 463, 919
- . 2010b, *ApJ*, 714, 927
- . 2010c, *A&A*, 523, A46+
- . 2010d, *Science*, 328, 725
- . 2010e, *ApJ*, 721, 1425
- . 2010f, *ApJ*, 718, 348
- . 2010g, *ApJ*, 713, 146
- . 2010h, *Science*, 327, 1103
- . 2010i, *ApJ*, 712, 459
- . 2010j, *A&A*, 512, A7+
- . 2010k, *ApJ*, 710, 810
- . 2011a, *ApJ*, 727, 129
- . 2011b, *ApJ*, 726, 43
- Cheung, C. C., Donato, D., & Reyes, L. C. 2009, *The Astronomer’s Telegram*, 1943, 1
- Cutini, S., & Hays, E. 2009, *The Astronomer’s Telegram*, 2033, 1
- D’Ammando, F., Sokolovsky, K. V., Ciprini, S., & Vetere, L. 2010a, *The Astronomer’s Telegram*, 2628, 1
- D’Ammando, F., Sokolovsky, K. V., Cutini, S., & Vetere, L. 2010b, *The Astronomer’s Telegram*, 2673, 1

Table 1—Continued

| Name 2FGL     | R.A.    | Decl.   | $l$     | $b$     | $\theta_1$ | $\theta_2$ | $\phi$ | $\sigma$ | $F_{35}$ | $\Delta F_{35}$ | $S_{25}$ | $\Delta S_{25}$ | $\Gamma_{25}$ | $\Delta \Gamma_{25}$ | Mod | Var | Flags | $\gamma$ -ray Assoc. | TeV | Class | ID or Assoc.          | Ref. |
|---------------|---------|---------|---------|---------|------------|------------|--------|----------|----------|-----------------|----------|-----------------|---------------|----------------------|-----|-----|-------|----------------------|-----|-------|-----------------------|------|
| J2347.9–1629  | 356.984 | –16.487 | 65.569  | –71.852 | 0.066      | 0.063      | –70    | 13.2     | 1.6      | 0.2             | 19.8     | 2.0             | 2.36          | 0.08                 | PL  | T   | ...   | 1FGL J2348.0–1629    | ... | bzq   | PKS 2345–16           | ...  |
| J2350.2–3002  | 357.557 | –30.039 | 17.105  | –76.263 | 0.085      | 0.080      | 8      | 6.4      | 0.6      | 0.1             | 6.5      | 1.3             | 2.19          | 0.17                 | PL  | ... | ...   | 1FGL J2350.1–3005    | ... | agu   | 1RXS J235035.3–300537 | ...  |
| J2351.6–7558  | 357.913 | –75.979 | 307.653 | –40.597 | 0.126      | 0.102      | –64    | 4.1      | 0.4      | 0.1             | 4.6      | 1.4             | 1.92          | 0.19                 | PL  | ... | ...   | ...                  | ... | ...   | ...                   | ...  |
| J2352.0+1753  | 358.019 | 17.898  | 103.554 | –42.729 | 0.102      | 0.091      | 53     | 8.2      | 0.7      | 0.1             | 8.6      | 1.7             | 1.92          | 0.14                 | PL  | ... | ...   | 1FGL J2352.1+1752    | ... | bzb   | 87GB 234934.7+173227  | ...  |
| J2353.3+6643c | 358.341 | 66.719  | 117.228 | 4.493   | 0.110      | 0.083      | 17     | 5.4      | 1.3      | 0.2             | 15.1     | 3.0             | 2.29          | 0.11                 | PL  | ... | 4,6   | ...                  | ... | ...   | ...                   | ...  |
| J2353.5–3034  | 358.384 | –30.580 | 14.273  | –76.872 | 0.108      | 0.097      | –45    | 6.0      | 0.5      | 0.1             | 5.9      | 1.3             | 2.11          | 0.18                 | PL  | ... | ...   | ...                  | ... | bzb   | PKS 2351–309          | ...  |
| J2354.2–6615  | 358.565 | –66.263 | 311.803 | –49.869 | 0.201      | 0.151      | 78     | 4.9      | 0.4      | 0.1             | 5.0      | 1.1             | 2.15          | 0.16                 | PL  | ... | ...   | 1FGL J2355.9–6613    | ... | ...   | ...                   | ...  |
| J2356.0–5256  | 359.021 | –52.939 | 320.943 | –62.211 | 0.189      | 0.127      | –15    | 11.7     | 0.8      | 0.1             | 13.1     | 1.3             | 2.57          | 0.10                 | PL  | T   | 2     | 1FGL J2356.0–5253    | ... | ...   | ...                   | ...  |
| J2356.1+4034  | 359.028 | 40.581  | 111.712 | –21.082 | 0.186      | 0.102      | 70     | 6.2      | 0.6      | 0.1             | 8.5      | 2.2             | 1.66          | 0.17                 | PL  | ... | ...   | 1FGL J2356.1+4037    | ... | bzb   | NVSS J235612+403648   | ...  |
| J2356.3+0432  | 359.091 | 4.541   | 98.069  | –55.649 | 0.364      | 0.223      | 45     | 4.2      | 0.3      | 0.1             | 5.7      | 1.3             | 2.76          | 0.20                 | PL  | ... | 8,9   | 1FGL J2357.2+0445    | ... | bzq   | MG1 J235704+0447      | ...  |
| J2358.4–1811  | 359.613 | –18.196 | 66.370  | –74.879 | 0.151      | 0.138      | 66     | 4.1      | 0.4      | 0.1             | 4.3      | 1.3             | 1.93          | 0.20                 | PL  | ... | ...   | 1FGL J2358.5–1809    | ... | ...   | ...                   | ...  |
| J2358.9+6325  | 359.745 | 63.422  | 117.105 | 1.145   | 0.337      | 0.259      | –75    | 4.8      | 1.0      | 0.2             | 13.9     | 2.8             | 2.47          | 0.12                 | PL  | ... | 4,5,8 | ...                  | ... | †     | ...                   | ...  |
| J2359.0–3037  | 359.759 | –30.625 | 12.876  | –78.017 | 0.126      | 0.102      | 45     | 7.0      | 0.6      | 0.1             | 7.1      | 1.6             | 1.89          | 0.17                 | PL  | ... | ...   | 1FGL J2359.0–3035    | P   | bzb   | H 2356–309            | ...  |
| J2359.4+6751c | 359.860 | 67.863  | 118.048 | 5.486   | 0.186      | 0.156      | 60     | 7.7      | 1.3      | 0.3             | 17.4     | 2.6             | 2.43          | ...                  | LP  | T   | 1,4,6 | ...                  | ... | ...   | ...                   | ...  |
| J2359.6+6543c | 359.907 | 65.731  | 117.637 | 3.393   | 0.115      | 0.088      | 3      | 7.7      | 1.9      | 0.3             | 22.2     | 3.2             | 2.21          | 0.08                 | PL  | ... | 6     | ...                  | ... | ...   | ...                   | ...  |

References. — 1 Abdo et al. (2010c), 2 Abdo et al. (2011b), 3 D’Ammando et al. (2010b), 4 D’Ammando et al. (2010d), 5 Abdo et al. (2010j), 6 Abdo et al. (2010i), 7 Donato et al. (2010b), 8 Tanaka et al. (2009), 9 Abdo et al. (2010g), 10 Abdo et al. (2009b), 11 Abdo et al. (2009d), 12 D’Ammando et al. (2010a), 13 Cheung et al. (2009), 14 Reyes et al. (2011), 15 Abdo et al. (2010a), 16 Abdo et al. (2010d), 17 Abdo et al. (2010d), 18 Abdo et al. (2009c), 19 Abdo et al. (2010k), 20 Abdo et al. (2010e), 21 Cutini & Hays (2009), 22 Abdo et al. (2010b), 23 Abdo et al. (2011a), 24 Abdo et al. (2010f), 25 Grondin et al. (2011), 26 D’Ammando et al. (2010c), 27 Abdo et al. (2010h), 28 Abdo et al. (2009a), 29 Sokolovsky et al. (2010), 30 Donato et al. (2010a)

Note. — The definitions of the columns are provided in Table 4.

<sup>a</sup>Within the Large Magellanic Cloud on the sky

- D’Ammando, F., Sokolovsky, K. V., & Gelbord, J. 2010c, The Astronomer’s Telegram, 2963, 1
- D’Ammando, F., Sokolovsky, K. V., Iafrate, G., & Stark, M. 2010d, The Astronomer’s Telegram, 2689, 1
- Donato, D., Hauser, M., Wagner, S., Hagen, H., & Atom Team. 2010a, The Astronomer’s Telegram, 2972, 1
- Donato, D., Sokolovsky, K. V., D’Ammando, F., & Schinzel, F. K. 2010b, The Astronomer’s Telegram, 2848, 1
- Grondin, M.-H., et al. 2011, ApJ, 738, 42
- Reyes, L., D’Ammando, F., & Hoversten, E. 2011, The Astronomer’s Telegram, 3353, 1
- Sokolovsky, K. V., Donato, D., Schinzel, F. K., & Kovalev, Y. Y. 2010, The Astronomer’s Telegram, 2589, 1
- Tanaka, Y. T., Donato, D., Cutini, S., Gasparrini, D., & Cheung, C. C. 2009, The Astronomer’s Telegram, 2253, 1
