# Supplementary material for: Fermi Large Area Telescope Second Source Catalog
Source: arXiv:1108.1435 ancillary file (2012-02-23)
Supplement: Supplementary file 2 [file table7_full.pdf]

Table 1. Second LAT Catalog: Spectral Information

|               | 100 MeV – 300 MeV |                |               | 300 MeV – 1 GeV |                |               | 1 GeV – 3 GeV |                |               | 3 GeV – 10 GeV |                |               | 10 GeV – 100 GeV |                |               |
|---------------|-------------------|----------------|---------------|-----------------|----------------|---------------|---------------|----------------|---------------|----------------|----------------|---------------|------------------|----------------|---------------|
| Name 2FGL     | $F_1^a$           | $\Delta F_1^a$ | $\sqrt{TS_1}$ | $F_2^a$         | $\Delta F_2^a$ | $\sqrt{TS_2}$ | $F_3^b$       | $\Delta F_3^b$ | $\sqrt{TS_3}$ | $F_4^c$        | $\Delta F_4^c$ | $\sqrt{TS_4}$ | $F_5^c$          | $\Delta F_5^c$ | $\sqrt{TS_5}$ |
| J0000.9–0748  | 1.4               | 0.0            |               | 1.5             | 0.3            | 0.1           | 5.3           | 0.5            | 0.0           | 2.5            | 2.0            | 0.0           | 2.5              | 0.7            | 0.0           |
| J0001.7–4159  | 1.5               | 0.0            |               | 2.2             | 0.2            | 0.0           | 2.8           | 0.5            | 0.0           | 2.6            | 1.6            | 0.6           | 5.2              | 0.9            | 0.0           |
| J0002.7+6220  | 1.9               | 0.7            |               | 3.5             | 1.3            | 0.2           | 9.2           | 2.6            | 0.4           | 8.7            | 4.1            | 1.1           | 5.2              | 0.5            | 0.0           |
| J0004.2+2208  | 1.6               | 0.0            |               | 2.0             | 0.3            | 0.1           | 4.8           | 0.4            | 0.0           | 1.6            | 1.3            | 0.6           | 3.7              | 0.5            | 0.0           |
| J0004.7–4736  | 2.2               | 0.4            |               | 5.8             | 0.4            | 0.1           | 7.7           | 0.9            | 0.2           | 7.9            | 1.3            | 0.6           | 4.1              | 0.6            | 0.0           |
| J0006.1+3821  | 2.7               | 0.5            |               | 5.9             | 0.5            | 0.1           | 7.0           | 0.9            | 0.2           | 6.2            | 2.3            | 0.0           | 2.8              | 0.6            | 0.0           |
| J0007.0+7303  | 17.9              | 0.6            |               | 37.6            | 11.6           | 0.2           | 96.0          | 49.9           | 0.9           | 122.7          | 149.9          | 4.2           | 91.3             | 12.5           | 1.2           |
| J0007.7+6825c | 2.8               | 0.0            |               | 0.6             | 1.1            | 0.2           | 6.1           | 0.9            | 0.3           | 3.2            | 1.3            | 0.0           | 0.0              | 1.0            | 0.0           |
| J0007.8+4713  | 2.7               | 0.4            |               | 6.6             | 0.6            | 0.1           | 8.4           | 1.5            | 0.2           | 9.5            | 4.9            | 1.0           | 9.3              | 1.2            | 0.5           |
| J0008.7–2344  | 0.5               | 0.0            |               | 0.0             | 0.1            | 0.0           | 0.1           | 0.6            | 0.0           | 3.2            | 1.4            | 0.0           | 1.6              | 1.8            | 0.0           |
| J0009.0+0632  | 2.1               | 0.0            |               | 2.8             | 0.3            | 0.0           | 2.4           | 0.3            | 0.1           | 3.2            | 1.4            | 0.6           | 3.7              | 0.7            | 0.0           |
| J0009.1+5030  | 0.9               | 0.0            |               | 0.3             | 0.4            | 0.1           | 6.0           | 1.5            | 0.2           | 9.6            | 5.9            | 1.1           | 10.6             | 1.9            | 0.6           |
| J0009.9–3206  | 0.7               | 0.0            |               | 0.1             | 0.3            | 0.0           | 3.1           | 0.5            | 0.1           | 5.0            | 1.7            | 0.0           | 1.6              | 0.9            | 0.0           |
| J0010.5+6556c | 2.7               | 0.0            |               | 2.8             | 1.2            | 0.2           | 7.0           | 1.8            | 0.0           | 3.0            | 3.2            | 0.0           | 1.5              | 0.7            | 0.0           |
| J0011.3+0054  | 1.3               | 0.0            |               | 0.8             | 0.3            | 0.1           | 4.9           | 0.5            | 0.1           | 4.4            | 1.9            | 0.0           | 2.0              | 0.6            | 0.0           |
| J0012.9–3954  | 1.5               | 0.0            |               | 2.4             | 0.3            | 0.0           | 2.6           | 0.5            | 0.1           | 4.7            | 2.1            | 0.0           | 3.0              | 1.2            | 0.0           |
| J0013.8+1907  | 1.0               | 0.0            |               | 0.8             | 0.3            | 0.0           | 2.6           | 0.4            | 0.0           | 1.0            | 1.9            | 0.7           | 5.1              | 0.5            | 0.0           |
| J0014.3–0509  | 3.4               | 0.0            |               | 1.7             | 0.5            | 0.0           | 2.7           | 0.8            | 0.0           | 3.1            | 1.5            | 0.0           | 0.5              | 0.9            | 0.0           |
| J0017.4–0018  | 1.9               | 0.5            |               | 4.6             | 0.3            | 0.1           | 4.4           | 0.5            | 0.0           | 2.2            | 1.4            | 0.0           | 1.3              | 0.5            | 0.0           |
| J0017.6–0510  | 3.9               | 0.0            |               | 2.3             | 0.8            | 0.1           | 8.6           | 1.1            | 0.2           | 7.8            | 1.3            | 0.5           | 4.4              | 1.1            | 0.0           |
| J0018.5+2945  | 0.5               | 0.0            |               | 0.0             | 0.1            | 0.0           | 0.0           | 0.2            | 0.0           | 0.6            | 1.5            | 0.0           | 2.1              | 0.8            | 0.4           |
| J0018.8–8154  | 1.3               | 0.0            |               | 0.9             | 0.4            | 0.1           | 4.8           | 0.4            | 0.2           | 3.2            | 2.4            | 0.7           | 5.0              | 1.4            | 0.0           |
| J0019.4–5645  | 1.5               | 0.4            |               | 3.5             | 0.3            | 0.0           | 2.7           | 0.3            | 0.1           | 4.2            | 2.1            | 0.0           | 1.8              | 0.7            | 0.0           |
| J0021.6–2551  | 1.3               | 0.0            |               | 1.8             | 0.2            | 0.0           | 2.9           | 0.7            | 0.2           | 6.9            | 2.2            | 0.7           | 5.9              | 1.5            | 0.0           |
| J0022.2–1853  | 0.5               | 0.0            |               | 0.0             | 0.2            | 0.0           | 1.9           | 0.5            | 0.1           | 5.3            | 2.5            | 0.7           | 6.6              | 1.7            | 0.6           |
| J0022.3–5141  | 1.0               | 0.0            |               | 0.7             | 0.2            | 0.0           | 2.4           | 0.6            | 0.1           | 5.9            | 1.4            | 0.0           | 2.0              | 0.6            | 0.0           |
| J0022.5+0607  | 1.6               | 0.5            |               | 3.9             | 0.6            | 0.1           | 8.9           | 1.8            | 0.2           | 12.6           | 4.6            | 0.9           | 9.5              | 1.3            | 0.5           |
| J0023.2+4454  | 1.7               | 0.4            |               | 4.1             | 0.2            | 0.1           | 3.2           | 0.7            | 0.2           | 5.9            | 1.1            | 0.5           | 3.3              | 0.8            | 0.0           |
| J0023.5+0924  | 1.2               | 0.0            |               | 0.6             | 0.4            | 0.1           | 5.6           | 0.9            | 0.2           | 6.4            | 2.5            | 0.0           | 2.4              | 0.8            | 0.0           |
| J0023.9–7204  | 1.4               | 0.0            |               | 2.8             | 0.9            | 0.1           | 16.3          | 3.4            | 0.3           | 21.5           | 6.3            | 1.1           | 12.3             | 0.8            | 0.0           |
| J0024.5+0346  | 2.0               | 0.0            |               | 2.3             | 0.4            | 0.0           | 3.1           | 0.4            | 0.1           | 3.3            | 2.0            | 0.0           | 2.0              | 1.0            | 0.0           |
| J0029.2–7043  | 2.2               | 0.0            |               | 2.7             | 0.3            | 0.1           | 4.8           | 0.6            | 0.2           | 5.2            | 1.7            | 0.6           | 4.5              | 0.6            | 0.0           |
| J0030.2–4223  | 2.8               | 0.4            |               | 7.5             | 0.5            | 0.1           | 8.6           | 0.9            | 0.2           | 8.2            | 1.2            | 0.5           | 4.1              | 0.9            | 0.0           |
| J0030.4+0450  | 2.8               | 0.5            |               | 8.6             | 2.4            | 0.1           | 34.2          | 8.2            | 0.4           | 38.6           | 12.8           | 1.5           | 19.6             | 1.0            | 0.0           |
| J0031.0+0724  | 1.4               | 0.5            |               | 3.7             | 0.2            | 0.0           | 0.8           | 0.6            | 0.0           | 2.7            | 0.9            | 0.0           | 0.0              | 0.7            | 0.3           |
| J0032.7–5521  | 1.5               | 0.4            |               | 4.2             | 0.6            | 0.1           | 10.5          | 1.3            | 0.2           | 10.5           | 2.3            | 0.7           | 6.7              | 1.6            | 0.0           |
| J0033.5–1921  | 1.1               | 0.0            |               | 1.5             | 0.4            | 0.1           | 8.5           | 2.2            | 0.2           | 16.3           | 9.0            | 1.3           | 15.8             | 3.4            | 0.8           |
| J0034.4–0534  | 1.5               | 0.3            |               | 4.5             | 0.6            | 0.1           | 10.7          | 2.2            | 0.2           | 14.8           | 2.4            | 0.7           | 7.0              | 0.5            | 0.0           |
| J0035.2+1515  | 1.1               | 0.0            |               | 1.0             | 0.2            | 0.0           | 1.1           | 0.7            | 0.2           | 6.2            | 2.7            | 0.7           | 6.7              | 2.0            | 0.6           |
| J0035.8+5951  | 2.9               | 0.0            |               | 2.9             | 0.5            | 0.1           | 4.3           | 1.4            | 0.3           | 5.9            | 5.4            | 1.1           | 7.3              | 3.3            | 0.7           |
| J0037.8+1238  | 1.5               | 0.5            |               | 3.5             | 0.4            | 0.1           | 5.4           | 0.8            | 0.2           | 6.0            | 1.9            | 0.7           | 4.5              | 0.9            | 0.4           |
| J0038.1+0015  | 1.4               | 0.0            |               | 1.9             | 0.2            | 0.0           | 1.5           | 0.3            | 0.0           | 1.1            | 1.5            | 0.6           | 4.3              | 1.1            | 0.0           |
| J0038.3–2457  | 1.9               | 0.4            |               | 5.2             | 0.3            | 0.1           | 5.4           | 0.7            | 0.2           | 7.0            | 2.2            | 0.0           | 2.6              | 1.4            | 0.0           |
| J0038.7–2215  | 0.6               | 0.0            |               | 0.0             | 0.1            | 0.0           | 1.0           | 0.3            | 0.1           | 3.4            | 2.0            | 0.0           | 3.2              | 1.3            | 0.0           |

Table 1—Continued

|               | 100 MeV – 300 MeV |                |               | 300 MeV – 1 GeV |                |               | 1 GeV – 3 GeV |                |               | 3 GeV – 10 GeV |                |               | 10 GeV – 100 GeV |                |               |
|---------------|-------------------|----------------|---------------|-----------------|----------------|---------------|---------------|----------------|---------------|----------------|----------------|---------------|------------------|----------------|---------------|
| Name 2FGL     | $F_1^a$           | $\Delta F_1^a$ | $\sqrt{TS_1}$ | $F_2^a$         | $\Delta F_2^a$ | $\sqrt{TS_2}$ | $F_3^b$       | $\Delta F_3^b$ | $\sqrt{TS_3}$ | $F_4^c$        | $\Delta F_4^c$ | $\sqrt{TS_4}$ | $F_5^c$          | $\Delta F_5^c$ | $\sqrt{TS_5}$ |
| J0038.8+6259  | 1.3               | 0.0            | 0.0           | 0.7             | 0.0            | 2.5           | 1.1           | 0.3            | 3.9           | 5.0            | 1.2            | 6.0           | 0.5              | 0.0            | 0.0           |
| J0039.1+4331  | 0.7               | 0.0            | 0.0           | 0.1             | 0.0            | 0.1           | 0.6           | 0.0            | 2.9           | 1.0            | 0.5            | 3.4           | 1.2              | 0.0            | 2.9           |
| J0042.5+4114  | 1.2               | 0.0            | 1.0           | 0.2             | 0.1            | 3.8           | 0.4           | 0.1            | 3.7           | 1.6            | 0.0            | 1.6           | 1.4              | 0.0            | 2.4           |
| J0043.7+3426  | 1.6               | 0.4            | 4.4           | 0.6             | 0.1            | 8.3           | 1.5           | 0.2            | 10.1          | 3.7            | 0.9            | 7.5           | 1.2              | 0.5            | 5.9           |
| J0044.7–3702  | 1.2               | 0.4            | 3.4           | 0.4             | 0.1            | 6.4           | 0.4           | 0.1            | 4.1           | 1.5            | 0.0            | 1.7           | 0.6              | 0.0            | 0.0           |
| J0045.3+2127  | 2.1               | 0.6            | 5.7           | 0.3             | 0.1            | 4.5           | 0.8           | 0.2            | 6.3           | 5.7            | 1.0            | 11.6          | 1.1              | 0.4            | 6.3           |
| J0045.5+1218  | 1.4               | 0.0            | 1.2           | 0.3             | 0.0            | 2.8           | 0.8           | 0.2            | 6.3           | 2.6            | 0.8            | 5.8           | 1.2              | 0.0            | 3.5           |
| J0046.7–8416  | 1.6               | 0.5            | 3.3           | 0.5             | 0.1            | 5.6           | 0.6           | 0.2            | 4.3           | 1.9            | 0.0            | 2.0           | 0.6              | 0.0            | 0.0           |
| J0047.0–2516  | 1.6               | 0.0            | 2.1           | 0.3             | 0.1            | 5.5           | 0.4           | 0.1            | 3.5           | 1.4            | 0.6            | 4.2           | 0.8              | 0.0            | 0.6           |
| J0047.2+5657  | 2.4               | 0.0            | 2.3           | 0.5             | 0.1            | 5.3           | 1.7           | 0.3            | 8.9           | 5.3            | 1.0            | 8.5           | 0.8              | 0.4            | 4.2           |
| J0047.9+2232  | 2.6               | 0.0            | 3.1           | 0.8             | 0.1            | 11.2          | 1.1           | 0.2            | 8.4           | 2.0            | 0.6            | 5.9           | 1.5              | 0.0            | 3.3           |
| J0048.8–6347  | 0.5               | 0.0            | 0.0           | 0.2             | 0.0            | 2.0           | 0.4           | 0.1            | 4.1           | 1.9            | 0.0            | 3.4           | 0.6              | 0.0            | 1.0           |
| J0049.7–5738  | 1.2               | 0.0            | 0.4           | 0.2             | 0.1            | 4.6           | 0.3           | 0.1            | 3.2           | 1.7            | 0.0            | 2.3           | 1.2              | 0.0            | 3.6           |
| J0050.1–0452  | 1.8               | 0.5            | 4.1           | 0.3             | 0.0            | 2.8           | 0.4           | 0.1            | 3.2           | 1.2            | 0.5            | 3.7           | 0.8              | 0.0            | 0.0           |
| J0050.2+0234  | 2.1               | 0.0            | 3.0           | 0.2             | 0.1            | 3.4           | 0.7           | 0.2            | 6.0           | 2.2            | 0.0            | 3.2           | 0.7              | 0.0            | 0.0           |
| J0050.6–0929  | 3.4               | 0.4            | 8.5           | 1.2             | 0.1            | 17.4          | 3.0           | 0.3            | 18.1          | 6.6            | 1.1            | 12.0          | 1.8              | 0.6            | 7.7           |
| J0051.0–0648  | 1.3               | 0.0            | 0.7           | 0.5             | 0.1            | 7.4           | 1.2           | 0.2            | 8.2           | 1.8            | 0.7            | 4.5           | 1.1              | 0.0            | 2.5           |
| J0051.4–6241  | 1.0               | 0.0            | 0.9           | 0.2             | 0.1            | 3.6           | 0.7           | 0.2            | 7.4           | 5.4            | 1.0            | 11.9          | 1.7              | 0.5            | 7.6           |
| J0055.0–2454  | 0.5               | 0.0            | 0.0           | 0.1             | 0.0            | 0.0           | 0.3           | 0.1            | 3.6           | 2.1            | 0.7            | 5.2           | 0.8              | 0.0            | 1.5           |
| J0056.8–2111  | 1.2               | 0.0            | 1.6           | 0.2             | 0.0            | 1.5           | 0.5           | 0.0            | 2.5           | 1.4            | 0.6            | 4.1           | 1.6              | 0.0            | 3.5           |
| J0057.9+3311  | 1.7               | 0.0            | 2.2           | 0.3             | 0.1            | 4.9           | 0.7           | 0.2            | 5.6           | 1.6            | 0.6            | 4.1           | 0.8              | 0.0            | 0.7           |
| J0057.9–3236  | 1.0               | 0.0            | 1.1           | 0.3             | 0.1            | 5.0           | 0.7           | 0.2            | 7.2           | 2.0            | 0.6            | 5.9           | 0.7              | 0.0            | 1.1           |
| J0059.0–7242e | 3.1               | 0.6            | 6.3           | 1.0             | 0.1            | 9.8           | 2.4           | 0.4            | 8.1           | 8.4            | 1.7            | 6.5           | 1.3              | 0.0            | 0.0           |
| J0059.2–0151  | 0.5               | 0.0            | 0.0           | 0.1             | 0.0            | 0.4           | 0.3           | 0.0            | 1.2           | 1.2            | 0.0            | 0.9           | 0.9              | 0.4            | 4.7           |
| J0059.7–5700  | 2.3               | 0.6            | 5.7           | 0.4             | 0.1            | 6.5           | 0.5           | 0.1            | 4.9           | 2.3            | 0.0            | 2.9           | 0.5              | 0.0            | 0.0           |
| J0100.2+0746  | 1.0               | 0.0            | 0.5           | 0.2             | 0.1            | 4.2           | 1.2           | 0.2            | 8.8           | 6.6            | 1.1            | 12.3          | 2.2              | 0.6            | 9.0           |
| J0101.2–6425  | 0.9               | 0.0            | 1.7           | 0.3             | 0.1            | 7.6           | 1.8           | 0.2            | 14.4          | 3.4            | 0.8            | 7.9           | 0.5              | 0.0            | 0.0           |
| J0102.2+0943  | 1.8               | 0.0            | 2.3           | 0.3             | 0.0            | 2.7           | 0.5           | 0.0            | 2.2           | 1.8            | 0.7            | 4.3           | 1.2              | 0.0            | 3.3           |
| J0102.3+4216  | 2.6               | 0.4            | 6.1           | 0.5             | 0.1            | 7.3           | 0.6           | 0.2            | 4.8           | 1.8            | 0.0            | 2.1           | 0.8              | 0.0            | 0.7           |
| J0102.7+5827  | 3.1               | 0.7            | 5.1           | 1.2             | 0.1            | 10.2          | 2.3           | 0.3            | 9.7           | 5.2            | 1.1            | 7.6           | 1.3              | 0.0            | 2.3           |
| J0102.9+4838  | 1.5               | 0.0            | 0.4           | 0.3             | 0.1            | 3.8           | 2.0           | 0.3            | 9.9           | 4.4            | 1.0            | 7.6           | 0.6              | 0.0            | 1.7           |
| J0103.5+5336  | 0.5               | 0.0            | 0.0           | 0.2             | 0.0            | 0.8           | 0.5           | 0.2            | 3.2           | 2.3            | 0.0            | 2.6           | 1.1              | 0.4            | 5.5           |
| J0103.8+1324  | 0.9               | 0.0            | 0.4           | 0.1             | 0.0            | 0.6           | 0.5           | 0.0            | 2.0           | 1.9            | 0.7            | 5.0           | 0.9              | 0.0            | 2.1           |
| J0105.0–2411  | 1.4               | 0.4            | 3.7           | 0.4             | 0.1            | 6.3           | 0.6           | 0.2            | 5.3           | 2.0            | 0.7            | 4.8           | 0.6              | 0.0            | 0.0           |
| J0105.3+3930  | 1.3               | 0.0            | 1.4           | 0.2             | 0.1            | 3.4           | 0.5           | 0.2            | 4.6           | 1.3            | 0.5            | 4.3           | 0.7              | 0.0            | 0.3           |
| J0106.5+4854  | 2.3               | 0.0            | 0.9           | 0.7             | 0.1            | 7.6           | 2.1           | 0.3            | 10.1          | 8.3            | 1.2            | 12.2          | 0.6              | 0.0            | 0.3           |
| J0108.6+0135  | 11.6              | 0.5            | 28.2          | 3.2             | 0.1            | 39.5          | 5.2           | 0.3            | 29.0          | 10.1           | 1.4            | 16.5          | 1.9              | 0.0            | 3.9           |
| J0109.0+1817  | 1.0               | 0.0            | 0.7           | 0.2             | 0.0            | 1.4           | 0.6           | 0.0            | 2.9           | 1.4            | 0.5            | 4.5           | 1.0              | 0.0            | 2.2           |
| J0109.9+6132  | 10.7              | 0.8            | 15.8          | 3.2             | 0.2            | 20.9          | 4.7           | 0.4            | 15.8          | 4.9            | 1.1            | 6.6           | 0.8              | 0.0            | 1.3           |
| J0110.3+6805  | 2.2               | 0.6            | 3.4           | 0.7             | 0.1            | 5.4           | 1.1           | 0.3            | 4.4           | 3.8            | 0.9            | 6.0           | 1.6              | 0.5            | 6.5           |
| J0112.1+2245  | 5.4               | 0.5            | 13.6          | 1.8             | 0.1            | 24.7          | 5.7           | 0.3            | 31.1          | 15.4           | 1.6            | 21.6          | 3.4              | 0.7            | 11.4          |
| J0112.8+3208  | 6.5               | 0.5            | 15.8          | 1.8             | 0.1            | 23.7          | 3.9           | 0.3            | 22.8          | 7.9            | 1.2            | 13.3          | 1.6              | 0.0            | 3.5           |
| J0113.2–3557  | 1.0               | 0.0            | 1.0           | 0.2             | 0.0            | 2.2           | 0.3           | 0.1            | 3.4           | 1.7            | 0.0            | 2.3           | 1.0              | 0.0            | 1.8           |
| J0113.7+4948  | 1.8               | 0.7            | 3.8           | 0.4             | 0.1            | 4.5           | 0.7           | 0.2            | 4.7           | 2.3            | 0.0            | 2.6           | 0.7              | 0.4            | 4.0           |

Table 1—Continued

|              | 100 MeV – 300 MeV |                |               | 300 MeV – 1 GeV |                |               | 1 GeV – 3 GeV |                |               | 3 GeV – 10 GeV |                |               | 10 GeV – 100 GeV |                |               |
|--------------|-------------------|----------------|---------------|-----------------|----------------|---------------|---------------|----------------|---------------|----------------|----------------|---------------|------------------|----------------|---------------|
| Name 2FGL    | $F_1^a$           | $\Delta F_1^a$ | $\sqrt{TS_1}$ | $F_2^a$         | $\Delta F_2^a$ | $\sqrt{TS_2}$ | $F_3^b$       | $\Delta F_3^b$ | $\sqrt{TS_3}$ | $F_4^c$        | $\Delta F_4^c$ | $\sqrt{TS_4}$ | $F_5^c$          | $\Delta F_5^c$ | $\sqrt{TS_5}$ |
| J0114.7+1326 | 2.3               | 0.5            | 5.6           | 0.3             | 0.1            | 5.7           | 0.9           | 0.2            | 7.1           | 1.9            | 0.6            | 5.6           | 0.9              | 0.4            | 4.2           |
| J0115.4+0358 | 2.0               | 0.0            | 3.0           | 0.4             | 0.1            | 7.0           | 1.1           | 0.2            | 8.5           | 3.9            | 0.9            | 8.1           | 1.0              | 0.4            | 4.8           |
| J0115.7+2518 | 1.4               | 0.0            | 1.5           | 0.4             | 0.1            | 5.4           | 0.8           | 0.2            | 6.1           | 3.5            | 0.9            | 7.5           | 1.1              | 0.4            | 5.7           |
| J0116.0–1134 | 2.6               | 0.4            | 6.5           | 0.8             | 0.1            | 12.6          | 1.2           | 0.2            | 9.2           | 2.4            | 0.8            | 5.5           | 0.6              | 0.0            | 0.0           |
| J0116.6–6153 | 0.7               | 0.0            | 0.2           | 0.1             | 0.0            | 1.0           | 0.4           | 0.0            | 2.2           | 1.5            | 0.0            | 1.9           | 0.7              | 0.3            | 4.9           |
| J0118.6–4631 | 0.8               | 0.0            | 0.6           | 0.2             | 0.0            | 2.7           | 0.2           | 0.0            | 0.4           | 1.1            | 0.5            | 3.8           | 1.3              | 0.0            | 2.8           |
| J0118.8–2142 | 5.0               | 0.4            | 14.4          | 1.8             | 0.1            | 26.7          | 3.3           | 0.3            | 21.2          | 6.5            | 1.1            | 12.3          | 1.8              | 0.0            | 4.0           |
| J0120.4–2700 | 1.9               | 0.3            | 6.0           | 0.9             | 0.1            | 16.0          | 2.8           | 0.3            | 19.8          | 12.3           | 1.5            | 19.3          | 3.4              | 0.7            | 12.7          |
| J0122.6+3425 | 0.6               | 0.0            | 0.0           | 0.1             | 0.0            | 0.0           | 0.5           | 0.0            | 2.0           | 1.4            | 0.0            | 1.4           | 1.2              | 0.4            | 5.8           |
| J0124.5–0621 | 0.7               | 0.0            | 0.0           | 0.3             | 0.1            | 5.3           | 0.4           | 0.2            | 3.4           | 1.2            | 0.6            | 3.2           | 0.7              | 0.0            | 0.0           |
| J0124.6–2322 | 1.9               | 0.0            | 2.7           | 0.2             | 0.1            | 3.9           | 0.6           | 0.2            | 5.2           | 1.6            | 0.0            | 2.5           | 1.6              | 0.0            | 3.0           |
| J0127.2+0324 | 1.1               | 0.0            | 1.2           | 0.2             | 0.1            | 3.4           | 0.6           | 0.1            | 5.5           | 3.5            | 0.9            | 7.4           | 1.0              | 0.4            | 5.3           |
| J0128.0+6330 | 2.7               | 0.0            | 1.0           | 0.8             | 0.2            | 4.4           | 1.4           | 0.0            | 2.2           | 2.5            | 0.0            | 1.1           | 1.1              | 0.0            | 1.7           |
| J0128.4+4431 | 1.2               | 0.0            | 0.9           | 0.3             | 0.1            | 4.8           | 0.7           | 0.0            | 3.1           | 1.9            | 0.7            | 4.3           | 0.5              | 0.0            | 0.0           |
| J0129.4+2618 | 1.6               | 0.5            | 3.5           | 0.3             | 0.1            | 3.7           | 0.6           | 0.2            | 4.6           | 1.3            | 0.0            | 0.9           | 0.5              | 0.0            | 0.0           |
| J0131.1+6121 | 2.7               | 0.8            | 4.0           | 0.5             | 0.1            | 4.2           | 1.2           | 0.3            | 5.1           | 6.2            | 1.2            | 8.5           | 3.8              | 0.8            | 11.4          |
| J0132.8–1654 | 4.1               | 0.4            | 10.8          | 1.1             | 0.1            | 16.5          | 1.8           | 0.2            | 13.4          | 2.4            | 0.8            | 5.7           | 1.4              | 0.0            | 3.1           |
| J0133.4–4408 | 0.6               | 0.0            | 0.0           | 0.2             | 0.0            | 2.6           | 0.4           | 0.1            | 4.2           | 1.7            | 0.0            | 2.7           | 0.9              | 0.0            | 2.4           |
| J0134.4+2636 | 0.9               | 0.0            | 0.0           | 0.3             | 0.0            | 1.7           | 0.6           | 0.2            | 5.2           | 3.0            | 0.8            | 6.2           | 1.6              | 0.0            | 3.1           |
| J0136.5+3905 | 1.7               | 0.3            | 5.3           | 0.4             | 0.1            | 7.7           | 2.5           | 0.2            | 16.1          | 14.7           | 1.6            | 20.5          | 7.2              | 1.0            | 18.1          |
| J0136.9+4751 | 9.1               | 0.5            | 21.0          | 2.8             | 0.1            | 31.6          | 5.9           | 0.4            | 28.0          | 12.4           | 1.5            | 17.5          | 1.3              | 0.5            | 6.2           |
| J0137.6–2430 | 1.9               | 0.4            | 5.2           | 0.5             | 0.1            | 9.1           | 1.0           | 0.2            | 9.3           | 1.2            | 0.0            | 1.4           | 1.2              | 0.0            | 2.2           |
| J0137.7+5811 | 2.6               | 0.0            | 2.3           | 0.5             | 0.1            | 4.6           | 1.1           | 0.0            | 2.8           | 2.4            | 0.8            | 4.1           | 1.6              | 0.0            | 3.2           |
| J0141.5–0928 | 1.4               | 0.0            | 2.1           | 0.5             | 0.1            | 9.0           | 1.1           | 0.2            | 9.5           | 3.9            | 0.9            | 8.4           | 0.8              | 0.4            | 4.9           |
| J0143.6–5844 | 1.0               | 0.0            | 1.0           | 0.2             | 0.1            | 4.2           | 0.8           | 0.2            | 7.7           | 2.3            | 0.7            | 6.6           | 2.2              | 0.6            | 9.5           |
| J0144.6+2704 | 3.3               | 0.4            | 8.1           | 1.0             | 0.1            | 13.6          | 2.9           | 0.3            | 17.3          | 6.7            | 1.1            | 11.9          | 1.1              | 0.4            | 5.0           |
| J0145.1–2732 | 5.8               | 0.5            | 14.6          | 1.3             | 0.1            | 19.3          | 1.9           | 0.2            | 13.7          | 1.8            | 0.7            | 4.8           | 0.8              | 0.0            | 1.2           |
| J0146.6–5206 | 1.1               | 0.0            | 0.6           | 0.2             | 0.0            | 1.4           | 0.4           | 0.0            | 1.8           | 2.2            | 0.0            | 3.0           | 0.9              | 0.0            | 2.7           |
| J0148.6+0127 | 1.7               | 0.0            | 2.6           | 0.2             | 0.1            | 3.3           | 0.4           | 0.0            | 0.6           | 1.2            | 0.6            | 3.5           | 1.5              | 0.0            | 3.9           |
| J0152.6+0148 | 1.0               | 0.0            | 0.0           | 0.2             | 0.0            | 0.7           | 0.7           | 0.2            | 6.7           | 1.9            | 0.7            | 5.1           | 0.8              | 0.4            | 4.8           |
| J0153.9+0823 | 1.3               | 0.0            | 1.3           | 0.3             | 0.1            | 4.9           | 1.4           | 0.2            | 9.8           | 5.2            | 1.0            | 9.8           | 1.6              | 0.6            | 5.9           |
| J0154.9+4434 | 1.4               | 0.0            | 1.6           | 0.3             | 0.0            | 1.9           | 0.4           | 0.0            | 1.3           | 1.6            | 0.0            | 1.5           | 0.7              | 0.3            | 4.6           |
| J0156.4+3909 | 1.8               | 0.0            | 2.4           | 0.4             | 0.1            | 5.8           | 0.5           | 0.2            | 4.3           | 1.3            | 0.6            | 3.4           | 0.5              | 0.0            | 0.0           |
| J0156.5–2419 | 0.7               | 0.0            | 0.2           | 0.2             | 0.0            | 1.6           | 0.3           | 0.1            | 3.3           | 1.3            | 0.0            | 1.3           | 1.5              | 0.0            | 4.6           |
| J0157.2–5259 | 1.3               | 0.0            | 1.2           | 0.1             | 0.0            | 0.9           | 0.4           | 0.0            | 2.2           | 2.8            | 0.7            | 7.3           | 0.7              | 0.0            | 0.0           |
| J0158.0–4609 | 1.4               | 0.0            | 1.7           | 0.3             | 0.1            | 5.1           | 0.5           | 0.1            | 4.9           | 2.2            | 0.0            | 3.0           | 0.5              | 0.0            | 0.0           |
| J0158.3–3931 | 1.0               | 0.0            | 0.5           | 0.3             | 0.1            | 5.8           | 0.7           | 0.2            | 6.3           | 1.4            | 0.6            | 4.0           | 0.8              | 0.4            | 4.3           |
| J0158.4+0107 | 2.0               | 0.0            | 2.7           | 0.2             | 0.1            | 3.6           | 0.5           | 0.0            | 2.3           | 1.7            | 0.0            | 1.9           | 1.3              | 0.0            | 2.9           |
| J0158.6+8558 | 1.4               | 0.0            | 1.4           | 0.3             | 0.0            | 2.8           | 0.5           | 0.1            | 4.6           | 0.7            | 0.0            | 0.0           | 0.6              | 0.0            | 0.0           |
| J0159.5+1046 | 1.5               | 0.4            | 3.5           | 0.3             | 0.1            | 3.9           | 0.7           | 0.2            | 5.0           | 1.7            | 0.7            | 3.8           | 1.1              | 0.4            | 5.9           |
| J0159.6–2741 | 0.6               | 0.0            | 0.0           | 0.2             | 0.1            | 3.7           | 0.6           | 0.2            | 5.4           | 1.4            | 0.5            | 4.9           | 0.5              | 0.0            | 0.0           |
| J0200.4–4105 | 1.0               | 0.0            | 0.8           | 0.1             | 0.0            | 0.4           | 0.3           | 0.1            | 3.2           | 1.9            | 0.0            | 3.3           | 1.0              | 0.0            | 2.6           |
| J0201.5–6626 | 1.5               | 0.0            | 1.4           | 0.2             | 0.1            | 3.9           | 0.3           | 0.1            | 3.5           | 1.4            | 0.0            | 1.5           | 0.9              | 0.0            | 2.2           |
| J0203.6+7235 | 2.3               | 0.0            | 1.6           | 0.5             | 0.0            | 2.4           | 1.1           | 0.0            | 3.1           | 2.6            | 0.8            | 5.2           | 0.9              | 0.4            | 3.7           |

Table 1—Continued

|               | 100 MeV – 300 MeV |                |               | 300 MeV – 1 GeV |                |               | 1 GeV – 3 GeV |                |               | 3 GeV – 10 GeV |                |               | 10 GeV – 100 GeV |                |               |
|---------------|-------------------|----------------|---------------|-----------------|----------------|---------------|---------------|----------------|---------------|----------------|----------------|---------------|------------------|----------------|---------------|
| Name 2FGL     | $F_1^a$           | $\Delta F_1^a$ | $\sqrt{TS_1}$ | $F_2^a$         | $\Delta F_2^a$ | $\sqrt{TS_2}$ | $F_3^b$       | $\Delta F_3^b$ | $\sqrt{TS_3}$ | $F_4^c$        | $\Delta F_4^c$ | $\sqrt{TS_4}$ | $F_5^c$          | $\Delta F_5^c$ | $\sqrt{TS_5}$ |
| J0204.0+3045  | 1.4               | 0.6            | 3.2           | 0.4             | 0.1            | 5.8           | 0.6           | 0.2            | 4.7           | 1.5            | 0.0            | 1.1           | 0.6              | 0.0            | 0.0           |
| J0205.0+1514  | 1.9               | 0.4            | 4.6           | 0.3             | 0.0            | 2.9           | 0.9           | 0.2            | 7.0           | 1.7            | 0.7            | 4.0           | 0.7              | 0.0            | 1.9           |
| J0205.3–1657  | 2.6               | 0.4            | 6.5           | 0.5             | 0.1            | 7.4           | 0.8           | 0.2            | 7.1           | 1.1            | 0.0            | 1.1           | 0.8              | 0.0            | 0.8           |
| J0205.4+3211  | 2.5               | 0.0            | 2.8           | 0.3             | 0.1            | 4.7           | 0.5           | 0.2            | 3.8           | 1.3            | 0.0            | 0.9           | 0.5              | 0.0            | 0.0           |
| J0205.8+6448  | 6.6               | 0.7            | 9.2           | 2.4             | 0.2            | 16.9          | 4.6           | 0.4            | 15.9          | 5.9            | 1.1            | 7.9           | 1.4              | 0.0            | 3.0           |
| J0206.5–1149  | 1.2               | 0.0            | 1.6           | 0.2             | 0.1            | 3.4           | 0.5           | 0.1            | 5.4           | 1.4            | 0.6            | 4.7           | 1.2              | 0.0            | 2.9           |
| J0207.9–6832  | 1.4               | 0.0            | 1.3           | 0.2             | 0.1            | 3.9           | 0.4           | 0.0            | 1.6           | 1.6            | 0.0            | 2.7           | 0.7              | 0.0            | 1.3           |
| J0209.5–5229  | 1.7               | 0.0            | 1.4           | 0.3             | 0.1            | 5.1           | 1.0           | 0.2            | 8.0           | 3.6            | 0.8            | 8.1           | 1.5              | 0.5            | 6.8           |
| J0210.7–5102  | 6.7               | 0.6            | 17.0          | 1.6             | 0.1            | 23.0          | 3.8           | 0.3            | 23.1          | 5.2            | 1.0            | 10.9          | 1.4              | 0.0            | 3.2           |
| J0211.2+1050  | 2.5               | 0.5            | 5.6           | 0.9             | 0.1            | 11.9          | 1.9           | 0.2            | 12.0          | 6.1            | 1.1            | 10.8          | 1.5              | 0.0            | 3.7           |
| J0212.1+5318  | 0.9               | 0.0            | 0.9           | 0.5             | 0.1            | 7.1           | 1.9           | 0.3            | 10.6          | 5.2            | 1.0            | 8.4           | 0.5              | 0.0            | 0.0           |
| J0213.1+2245  | 1.4               | 0.0            | 1.5           | 0.2             | 0.1            | 3.4           | 1.0           | 0.2            | 6.8           | 2.5            | 0.0            | 2.7           | 1.1              | 0.5            | 5.3           |
| J0214.5+6251c | 2.5               | 0.0            | 0.0           | 1.0             | 0.0            | 2.4           | 1.2           | 0.0            | 1.8           | 2.4            | 0.9            | 3.4           | 0.8              | 0.0            | 0.1           |
| J0216.9–6630  | 1.1               | 0.0            | 0.5           | 0.2             | 0.1            | 4.4           | 0.5           | 0.0            | 2.7           | 2.4            | 0.7            | 6.2           | 1.1              | 0.0            | 2.4           |
| J0217.4+0836  | 1.7               | 0.0            | 1.8           | 0.4             | 0.1            | 5.7           | 0.8           | 0.2            | 6.7           | 4.4            | 1.0            | 8.8           | 1.3              | 0.5            | 6.0           |
| J0217.5–0813  | 1.5               | 0.0            | 2.0           | 0.2             | 0.0            | 1.3           | 0.5           | 0.1            | 4.4           | 1.7            | 0.0            | 1.8           | 0.7              | 0.0            | 0.0           |
| J0217.7+7353  | 3.3               | 0.8            | 5.5           | 0.6             | 0.1            | 4.9           | 1.1           | 0.0            | 3.0           | 2.2            | 0.0            | 1.7           | 0.5              | 0.0            | 0.4           |
| J0217.9+0143  | 5.3               | 0.5            | 13.4          | 1.7             | 0.1            | 23.3          | 4.6           | 0.3            | 25.4          | 12.1           | 1.5            | 18.2          | 2.0              | 0.6            | 6.8           |
| J0218.1+4233  | 6.5               | 0.9            | 7.3           | 1.8             | 0.1            | 14.3          | 4.1           | 0.4            | 17.0          | 6.9            | 1.2            | 10.4          | 0.8              | 0.0            | 1.3           |
| J0218.7+6208c | 5.4               | 1.8            | 3.8           | 2.6             | 0.3            | 8.0           | 3.2           | 0.5            | 6.9           | 4.7            | 0.0            | 2.5           | 1.0              | 0.0            | 1.2           |
| J0219.1–1725  | 1.1               | 0.0            | 0.6           | 0.3             | 0.0            | 2.4           | 0.3           | 0.1            | 3.2           | 1.9            | 0.0            | 1.6           | 1.4              | 0.0            | 2.9           |
| J0219.2+3641  | 3.7               | 0.0            | 1.5           | 0.5             | 0.1            | 4.8           | 0.6           | 0.2            | 4.2           | 2.3            | 0.0            | 2.7           | 0.6              | 0.0            | 0.0           |
| J0221.0+3555  | 8.7               | 1.0            | 9.0           | 1.9             | 0.1            | 18.0          | 3.7           | 0.3            | 19.9          | 10.6           | 1.4            | 16.5          | 2.4              | 0.6            | 9.4           |
| J0221.2+2516  | 0.5               | 0.0            | 0.0           | 0.1             | 0.0            | 0.0           | 0.5           | 0.2            | 4.0           | 1.4            | 0.6            | 3.6           | 0.8              | 0.0            | 1.3           |
| J0221.3+6025c | 7.1               | 0.0            | 1.1           | 0.8             | 0.2            | 3.3           | 1.7           | 0.4            | 5.0           | 2.5            | 0.0            | 1.1           | 0.9              | 0.0            | 1.6           |
| J0221.4+6257c | 3.9               | 0.0            | 1.2           | 1.2             | 0.2            | 6.0           | 2.7           | 0.4            | 7.6           | 2.6            | 0.9            | 3.6           | 0.7              | 0.0            | 0.0           |
| J0222.0–1615  | 2.0               | 0.0            | 2.5           | 0.3             | 0.1            | 4.6           | 0.5           | 0.2            | 4.0           | 1.6            | 0.0            | 2.4           | 1.0              | 0.0            | 1.8           |
| J0222.6+4302  | 9.7               | 0.9            | 11.9          | 5.1             | 0.2            | 40.2          | 16.1          | 0.6            | 53.5          | 66.3           | 3.2            | 52.0          | 21.7             | 1.7            | 36.7          |
| J0222.7+6820  | 1.6               | 0.0            | 0.4           | 0.3             | 0.0            | 0.5           | 1.0           | 0.0            | 2.4           | 2.4            | 0.8            | 4.7           | 0.8              | 0.0            | 1.7           |
| J0223.0–1118  | 0.4               | 0.0            | 0.0           | 0.1             | 0.0            | 0.7           | 0.4           | 0.0            | 2.9           | 2.0            | 0.0            | 3.2           | 1.5              | 0.0            | 3.7           |
| J0224.0+6204  | 6.0               | 0.0            | 0.9           | 2.0             | 0.6            | 3.7           | 7.8           | 0.9            | 9.9           | 11.0           | 1.9            | 7.3           | 1.1              | 0.0            | 0.7           |
| J0225.9+6154c | 4.5               | 0.0            | 0.0           | 2.3             | 0.0            | 2.3           | 2.5           | 0.0            | 1.4           | 6.9            | 0.0            | 2.9           | 1.1              | 0.5            | 3.8           |
| J0226.1+0943  | 1.6               | 0.0            | 1.7           | 0.3             | 0.0            | 2.8           | 0.7           | 0.0            | 2.9           | 2.2            | 0.7            | 5.4           | 0.8              | 0.0            | 1.5           |
| J0226.5–4444  | 0.6               | 0.0            | 0.0           | 0.2             | 0.0            | 1.4           | 0.3           | 0.0            | 1.9           | 1.3            | 0.5            | 3.8           | 1.7              | 0.0            | 5.1           |
| J0227.2+6029c | 8.4               | 0.0            | 1.2           | 0.9             | 0.3            | 3.7           | 1.7           | 0.0            | 2.8           | 2.6            | 0.9            | 3.9           | 1.3              | 0.0            | 2.1           |
| J0227.3+0203  | 1.0               | 0.0            | 0.5           | 0.1             | 0.0            | 0.4           | 0.4           | 0.0            | 2.1           | 2.0            | 0.7            | 5.1           | 1.0              | 0.0            | 2.3           |
| J0227.7+2249  | 1.9               | 0.0            | 2.5           | 0.2             | 0.0            | 0.5           | 0.8           | 0.2            | 5.5           | 2.3            | 0.7            | 5.5           | 1.0              | 0.0            | 1.1           |
| J0229.3–3644  | 2.9               | 0.5            | 7.6           | 0.7             | 0.1            | 10.5          | 1.0           | 0.2            | 8.8           | 1.5            | 0.6            | 4.0           | 0.7              | 0.0            | 1.6           |
| J0230.8+4031  | 4.9               | 0.5            | 10.2          | 0.9             | 0.1            | 11.7          | 1.2           | 0.2            | 8.4           | 1.3            | 0.5            | 3.8           | 1.4              | 0.0            | 3.0           |
| J0233.9+6238c | 4.6               | 1.8            | 4.9           | 1.0             | 0.2            | 5.8           | 1.8           | 0.4            | 6.0           | 2.1            | 0.9            | 3.5           | 1.8              | 0.0            | 3.4           |
| J0237.1–6136  | 3.8               | 0.4            | 9.4           | 1.2             | 0.1            | 18.8          | 2.1           | 0.2            | 14.7          | 5.9            | 1.1            | 11.3          | 1.5              | 0.0            | 3.6           |
| J0237.5–3603  | 1.0               | 0.0            | 0.8           | 0.1             | 0.0            | 0.0           | 0.5           | 0.0            | 3.0           | 1.3            | 0.6            | 3.3           | 1.4              | 0.0            | 4.5           |
| J0237.8+2846  | 7.3               | 0.5            | 17.7          | 2.2             | 0.1            | 24.9          | 3.0           | 0.3            | 16.0          | 4.1            | 0.9            | 7.6           | 1.2              | 0.0            | 3.4           |
| J0237.9+5238  | 2.3               | 0.0            | 1.7           | 0.5             | 0.1            | 4.9           | 0.8           | 0.2            | 4.5           | 1.8            | 0.7            | 3.7           | 0.9              | 0.0            | 0.5           |

Table 1—Continued

|               | 100 MeV – 300 MeV |                |               | 300 MeV – 1 GeV |                |               | 1 GeV – 3 GeV |                |               | 3 GeV – 10 GeV |                |               | 10 GeV – 100 GeV |                |               |
|---------------|-------------------|----------------|---------------|-----------------|----------------|---------------|---------------|----------------|---------------|----------------|----------------|---------------|------------------|----------------|---------------|
| Name 2FGL     | $F_1^a$           | $\Delta F_1^a$ | $\sqrt{TS_1}$ | $F_2^a$         | $\Delta F_2^a$ | $\sqrt{TS_2}$ | $F_3^b$       | $\Delta F_3^b$ | $\sqrt{TS_3}$ | $F_4^c$        | $\Delta F_4^c$ | $\sqrt{TS_4}$ | $F_5^c$          | $\Delta F_5^c$ | $\sqrt{TS_5}$ |
| J0238.2–3905  | 0.3               | 0.0            | 0.0           | 0.1             | 0.0            | 1.1           | 0.4           | 0.0            | 1.8           | 1.8            | 0.6            | 5.0           | 1.2              | 0.0            | 2.7           |
| J0238.6–3117  | 0.9               | 0.0            | 1.0           | 0.3             | 0.0            | 2.9           | 0.7           | 0.2            | 7.2           | 3.0            | 0.8            | 7.5           | 2.0              | 0.0            | 4.2           |
| J0238.7+1637  | 15.3              | 0.6            | 31.9          | 5.3             | 0.2            | 51.5          | 14.3          | 0.6            | 51.3          | 38.5           | 2.5            | 37.6          | 7.3              | 1.1            | 17.5          |
| J0239.5+1324  | 2.3               | 0.0            | 2.9           | 0.4             | 0.0            | 3.0           | 0.5           | 0.2            | 3.9           | 1.5            | 0.7            | 3.4           | 1.3              | 0.0            | 2.9           |
| J0240.5+6113  | 60.4              | 1.8            | 70.2          | 20.6            | 0.3            | 98.4          | 41.3          | 0.9            | 80.7          | 66.2           | 3.2            | 43.0          | 5.0              | 0.8            | 12.3          |
| J0241.3+6548  | 2.9               | 0.7            | 4.3           | 0.6             | 0.0            | 2.4           | 1.0           | 0.0            | 2.1           | 3.4            | 0.0            | 3.0           | 1.7              | 0.5            | 6.7           |
| J0242.5+0006  | 1.1               | 0.0            | 1.1           | 0.3             | 0.0            | 2.5           | 0.3           | 0.1            | 3.2           | 1.2            | 0.5            | 3.6           | 1.3              | 0.0            | 2.8           |
| J0242.9+7118  | 1.1               | 0.0            | 0.0           | 0.3             | 0.0            | 1.3           | 0.8           | 0.0            | 2.1           | 2.1            | 0.7            | 3.9           | 0.7              | 0.3            | 4.5           |
| J0245.1+2406  | 3.4               | 0.6            | 6.8           | 0.6             | 0.1            | 7.4           | 0.9           | 0.2            | 5.5           | 3.0            | 0.0            | 3.1           | 0.9              | 0.0            | 1.0           |
| J0245.9–4652  | 8.9               | 0.5            | 22.9          | 2.1             | 0.1            | 29.6          | 4.2           | 0.3            | 25.9          | 5.2            | 1.0            | 10.4          | 1.2              | 0.0            | 2.3           |
| J0248.1+6021  | 7.0               | 1.7            | 7.9           | 2.3             | 0.2            | 12.2          | 4.5           | 0.5            | 11.8          | 3.2            | 1.0            | 4.0           | 1.0              | 0.0            | 0.6           |
| J0248.5+5131  | 2.2               | 0.0            | 0.0           | 0.4             | 0.0            | 1.1           | 0.9           | 0.0            | 2.5           | 2.9            | 0.9            | 5.2           | 1.8              | 0.0            | 3.7           |
| J0248.6+8440  | 0.6               | 0.0            | 0.0           | 0.1             | 0.0            | 0.5           | 0.3           | 0.0            | 0.9           | 2.2            | 0.6            | 6.0           | 0.7              | 0.0            | 1.0           |
| J0250.6+1713  | 1.4               | 0.5            | 3.2           | 0.3             | 0.0            | 2.4           | 0.7           | 0.0            | 2.9           | 2.6            | 0.8            | 5.8           | 1.2              | 0.5            | 6.3           |
| J0250.7+5631  | 3.4               | 0.0            | 2.6           | 0.6             | 0.2            | 4.4           | 0.8           | 0.0            | 0.9           | 2.0            | 0.8            | 3.2           | 1.8              | 0.0            | 3.7           |
| J0251.0+2557  | 0.9               | 0.0            | 0.0           | 0.3             | 0.1            | 3.8           | 0.5           | 0.2            | 3.5           | 2.1            | 0.0            | 2.2           | 0.4              | 0.0            | 0.0           |
| J0252.7–2218  | 6.8               | 0.4            | 18.2          | 2.1             | 0.1            | 29.5          | 4.4           | 0.3            | 24.5          | 6.7            | 1.1            | 12.7          | 1.4              | 0.5            | 5.8           |
| J0253.4+3218  | 1.4               | 0.0            | 1.4           | 0.2             | 0.0            | 1.4           | 0.8           | 0.2            | 5.6           | 1.9            | 0.7            | 4.3           | 0.9              | 0.4            | 5.3           |
| J0253.5+5107  | 3.7               | 1.2            | 3.3           | 0.9             | 0.1            | 6.9           | 1.4           | 0.3            | 6.7           | 2.5            | 0.9            | 4.0           | 1.7              | 0.0            | 3.3           |
| J0253.9+5908  | 4.3               | 0.0            | 2.0           | 0.8             | 0.2            | 4.7           | 0.9           | 0.3            | 3.2           | 2.7            | 0.0            | 1.5           | 1.5              | 0.0            | 1.7           |
| J0257.7–1213  | 0.8               | 0.0            | 0.2           | 0.3             | 0.1            | 4.8           | 0.4           | 0.1            | 4.0           | 2.0            | 0.0            | 2.5           | 0.7              | 0.0            | 1.1           |
| J0257.9+2025c | 1.8               | 0.0            | 1.6           | 0.4             | 0.0            | 1.9           | 0.7           | 0.2            | 3.5           | 2.0            | 0.8            | 3.5           | 1.1              | 0.0            | 2.1           |
| J0259.5+0740  | 1.8               | 0.0            | 1.6           | 0.4             | 0.1            | 3.9           | 0.5           | 0.2            | 3.9           | 2.5            | 0.0            | 2.1           | 0.7              | 0.0            | 0.0           |
| J0302.7–7919  | 1.0               | 0.0            | 0.5           | 0.3             | 0.1            | 3.7           | 0.4           | 0.2            | 3.9           | 1.2            | 0.6            | 3.5           | 1.1              | 0.0            | 2.9           |
| J0303.4–2407  | 3.2               | 0.4            | 9.0           | 1.5             | 0.1            | 22.8          | 4.3           | 0.3            | 25.7          | 16.5           | 1.7            | 23.0          | 6.9              | 1.1            | 18.5          |
| J0303.5+4713  | 2.6               | 0.6            | 5.0           | 0.7             | 0.1            | 7.7           | 1.3           | 0.2            | 7.8           | 3.3            | 0.8            | 6.8           | 0.7              | 0.4            | 3.9           |
| J0303.5–6209  | 2.0               | 0.6            | 4.8           | 0.7             | 0.1            | 10.0          | 0.9           | 0.2            | 8.3           | 1.9            | 0.6            | 5.3           | 0.6              | 0.0            | 0.0           |
| J0303.5+6822  | 4.1               | 0.7            | 5.9           | 0.4             | 0.1            | 3.2           | 1.0           | 0.3            | 4.1           | 3.0            | 0.0            | 2.0           | 0.5              | 0.0            | 0.0           |
| J0304.5–2836  | 0.9               | 0.0            | 1.2           | 0.1             | 0.0            | 0.7           | 0.3           | 0.0            | 0.8           | 1.7            | 0.6            | 5.3           | 1.5              | 0.0            | 3.8           |
| J0305.0–1602  | 0.6               | 0.0            | 0.0           | 0.1             | 0.0            | 0.1           | 0.3           | 0.0            | 1.0           | 1.1            | 0.5            | 3.6           | 0.9              | 0.4            | 4.4           |
| J0307.4+4915  | 2.2               | 0.0            | 1.8           | 0.5             | 0.0            | 2.6           | 1.2           | 0.3            | 5.8           | 2.1            | 0.8            | 3.6           | 1.4              | 0.5            | 6.1           |
| J0308.3+7442  | 0.5               | 0.0            | 0.0           | 0.3             | 0.1            | 5.2           | 2.6           | 0.3            | 13.7          | 2.8            | 0.7            | 5.9           | 0.5              | 0.0            | 0.0           |
| J0308.7+5954  | 4.2               | 0.0            | 3.0           | 0.9             | 0.2            | 5.4           | 1.5           | 0.0            | 2.7           | 4.0            | 0.0            | 2.8           | 1.4              | 0.0            | 1.7           |
| J0309.1+1027  | 2.8               | 0.0            | 3.1           | 0.6             | 0.1            | 6.3           | 1.4           | 0.3            | 7.0           | 1.8            | 0.7            | 3.7           | 0.8              | 0.4            | 4.6           |
| J0309.3–0743  | 0.8               | 0.0            | 0.0           | 0.1             | 0.0            | 0.0           | 0.2           | 0.0            | 0.0           | 2.0            | 0.7            | 5.2           | 1.6              | 0.0            | 2.9           |
| J0310.0–6058  | 2.9               | 0.6            | 6.6           | 0.7             | 0.1            | 10.8          | 0.6           | 0.2            | 4.7           | 2.3            | 0.7            | 6.0           | 1.2              | 0.0            | 3.1           |
| J0310.2–5013  | 1.0               | 0.0            | 0.1           | 0.1             | 0.0            | 0.2           | 0.4           | 0.1            | 3.9           | 1.7            | 0.6            | 5.0           | 0.7              | 0.4            | 4.4           |
| J0310.7+3813  | 2.5               | 0.0            | 3.1           | 0.4             | 0.0            | 2.7           | 0.4           | 0.2            | 3.3           | 2.3            | 0.0            | 2.3           | 1.3              | 0.0            | 2.0           |
| J0312.5–0914  | 1.8               | 0.0            | 1.6           | 0.3             | 0.1            | 3.7           | 0.5           | 0.2            | 3.7           | 1.6            | 0.7            | 3.3           | 0.7              | 0.0            | 1.9           |
| J0312.6+0132  | 2.0               | 0.5            | 4.6           | 0.6             | 0.1            | 7.8           | 1.1           | 0.2            | 7.4           | 2.5            | 0.8            | 5.4           | 1.6              | 0.0            | 3.7           |
| J0312.8+2013  | 1.4               | 0.0            | 0.9           | 0.2             | 0.0            | 0.6           | 0.8           | 0.0            | 3.1           | 2.0            | 0.0            | 1.4           | 0.7              | 0.3            | 4.5           |
| J0314.2–5106  | 2.2               | 0.0            | 3.0           | 0.2             | 0.1            | 4.3           | 0.4           | 0.1            | 3.8           | 2.2            | 0.0            | 2.9           | 1.6              | 0.0            | 3.5           |
| J0315.8–1024  | 1.8               | 0.0            | 1.6           | 0.2             | 0.1            | 3.7           | 0.6           | 0.2            | 4.1           | 2.2            | 0.7            | 5.1           | 0.5              | 0.0            | 0.0           |
| J0315.8–2611  | 1.1               | 0.0            | 1.3           | 0.2             | 0.0            | 2.3           | 0.3           | 0.1            | 3.7           | 2.8            | 0.8            | 7.0           | 0.8              | 0.0            | 0.8           |

Table 1—Continued

|               | 100 MeV – 300 MeV |                |               | 300 MeV – 1 GeV |                |               | 1 GeV – 3 GeV |                |               | 3 GeV – 10 GeV |                |               | 10 GeV – 100 GeV |                |               |
|---------------|-------------------|----------------|---------------|-----------------|----------------|---------------|---------------|----------------|---------------|----------------|----------------|---------------|------------------|----------------|---------------|
| Name 2FGL     | $F_1^a$           | $\Delta F_1^a$ | $\sqrt{TS_1}$ | $F_2^a$         | $\Delta F_2^a$ | $\sqrt{TS_2}$ | $F_3^b$       | $\Delta F_3^b$ | $\sqrt{TS_3}$ | $F_4^c$        | $\Delta F_4^c$ | $\sqrt{TS_4}$ | $F_5^c$          | $\Delta F_5^c$ | $\sqrt{TS_5}$ |
| J0316.1–6434  | 1.6               | 0.0            | 2.3           | 0.2             | 0.0            | 2.3           | 0.3           | 0.1            | 3.2           | 2.8            | 0.8            | 6.9           | 1.6              | 0.0            | 3.2           |
| J0316.1+0904  | 1.2               | 0.0            | 0.4           | 0.6             | 0.1            | 6.0           | 1.3           | 0.2            | 7.6           | 5.3            | 1.1            | 8.2           | 3.5              | 0.8            | 10.5          |
| J0316.6+4119  | 2.2               | 0.0            | 0.0           | 0.4             | 0.0            | 0.6           | 1.3           | 0.0            | 2.5           | 2.3            | 0.9            | 3.3           | 1.5              | 0.0            | 2.6           |
| J0318.0+0255  | 1.6               | 0.0            | 0.9           | 0.4             | 0.0            | 3.1           | 0.9           | 0.2            | 6.0           | 1.8            | 0.7            | 4.2           | 0.8              | 0.0            | 1.1           |
| J0319.6+1849  | 1.1               | 0.0            | 0.5           | 0.2             | 0.0            | 1.5           | 0.4           | 0.2            | 3.4           | 3.6            | 0.9            | 7.5           | 2.0              | 0.6            | 7.7           |
| J0319.8+4130  | 11.8              | 0.5            | 9.9           | 4.6             | 0.2            | 26.2          | 13.7          | 0.6            | 39.7          | 40.6           | 2.6            | 34.1          | 11.0             | 1.3            | 22.2          |
| J0322.0+2336  | 2.2               | 0.7            | 4.5           | 0.4             | 0.1            | 4.7           | 0.8           | 0.2            | 5.5           | 3.2            | 0.9            | 6.4           | 1.5              | 0.5            | 6.6           |
| J0322.4–3717  | 1.4               | 0.0            | 1.9           | 0.2             | 0.1            | 3.6           | 0.4           | 0.1            | 4.0           | 1.4            | 0.6            | 3.7           | 0.6              | 0.0            | 0.0           |
| J0323.6–0108  | 0.8               | 0.0            | 0.4           | 0.1             | 0.0            | 0.0           | 0.5           | 0.0            | 1.8           | 1.8            | 0.6            | 5.6           | 1.2              | 0.5            | 4.7           |
| J0324.8+3408  | 2.8               | 0.4            | 6.5           | 0.7             | 0.1            | 7.0           | 0.6           | 0.2            | 3.3           | 0.7            | 0.0            | 0.0           | 0.6              | 0.0            | 0.0           |
| J0325.1–5635  | 1.6               | 0.0            | 2.3           | 0.3             | 0.0            | 3.1           | 0.5           | 0.1            | 4.6           | 1.1            | 0.5            | 3.5           | 1.0              | 0.0            | 2.1           |
| J0325.6–1650  | 0.9               | 0.0            | 0.4           | 0.3             | 0.0            | 2.7           | 0.5           | 0.2            | 4.8           | 1.5            | 0.6            | 4.5           | 1.4              | 0.0            | 1.7           |
| J0326.1+2226  | 4.0               | 0.7            | 8.4           | 1.2             | 0.1            | 12.2          | 1.0           | 0.2            | 5.4           | 1.7            | 0.0            | 1.5           | 0.5              | 0.0            | 0.0           |
| J0326.1+0224  | 1.4               | 0.5            | 3.2           | 0.3             | 0.1            | 4.2           | 0.7           | 0.2            | 5.2           | 4.4            | 1.0            | 7.7           | 0.9              | 0.4            | 4.3           |
| J0330.3+5816c | 1.7               | 0.5            | 3.2           | 1.2             | 0.2            | 6.3           | 1.5           | 0.0            | 1.9           | 2.9            | 0.0            | 1.2           | 0.5              | 0.0            | 0.0           |
| J0332.1+6309  | 2.5               | 0.0            | 1.9           | 0.6             | 0.0            | 2.4           | 0.9           | 0.3            | 3.7           | 2.0            | 0.8            | 3.3           | 1.4              | 0.0            | 3.4           |
| J0332.5–1118  | 1.2               | 0.0            | 0.9           | 0.3             | 0.1            | 4.3           | 0.7           | 0.0            | 3.1           | 1.5            | 0.0            | 1.9           | 0.6              | 0.0            | 0.0           |
| J0333.7+2918  | 1.6               | 0.0            | 1.1           | 0.5             | 0.0            | 3.1           | 1.0           | 0.2            | 6.2           | 4.5            | 1.0            | 7.3           | 1.1              | 0.4            | 5.2           |
| J0334.2–4008  | 4.4               | 0.4            | 12.3          | 1.5             | 0.1            | 23.6          | 2.9           | 0.3            | 20.0          | 8.8            | 1.3            | 15.5          | 2.1              | 0.6            | 8.5           |
| J0334.3+6538  | 0.8               | 0.0            | 0.0           | 0.3             | 0.0            | 0.8           | 0.8           | 0.2            | 3.8           | 2.5            | 0.8            | 4.3           | 0.8              | 0.3            | 4.7           |
| J0334.3–3728  | 1.8               | 0.4            | 5.2           | 0.8             | 0.1            | 13.1          | 2.8           | 0.3            | 18.6          | 9.0            | 1.3            | 15.1          | 1.4              | 0.5            | 6.8           |
| J0335.3–4501  | 0.5               | 0.0            | 0.0           | 0.2             | 0.1            | 4.1           | 0.4           | 0.1            | 4.3           | 1.4            | 0.5            | 4.4           | 1.0              | 0.4            | 5.7           |
| J0336.0+7504  | 1.2               | 0.0            | 0.7           | 0.3             | 0.1            | 3.7           | 1.2           | 0.2            | 7.4           | 2.1            | 0.7            | 4.8           | 0.8              | 0.0            | 2.2           |
| J0337.0+3200c | 5.3               | 1.8            | 8.5           | 0.5             | 0.2            | 4.1           | 1.2           | 0.3            | 4.8           | 3.0            | 0.0            | 2.1           | 0.6              | 0.0            | 0.0           |
| J0338.2+1306  | 0.3               | 0.0            | 0.0           | 0.2             | 0.0            | 0.9           | 0.7           | 0.0            | 1.3           | 2.4            | 0.8            | 4.3           | 1.1              | 0.5            | 5.1           |
| J0339.2–1734  | 0.8               | 0.0            | 0.1           | 0.2             | 0.0            | 1.0           | 0.5           | 0.2            | 4.1           | 2.0            | 0.7            | 4.4           | 1.5              | 0.0            | 4.0           |
| J0339.4–0144  | 2.5               | 0.5            | 5.4           | 0.8             | 0.1            | 9.7           | 1.3           | 0.2            | 8.5           | 1.5            | 0.7            | 3.6           | 0.5              | 0.0            | 0.0           |
| J0340.4+4131  | 1.2               | 0.0            | 0.9           | 0.4             | 0.1            | 5.5           | 3.2           | 0.3            | 15.8          | 7.5            | 1.2            | 11.2          | 1.2              | 0.0            | 2.1           |
| J0340.5+5307  | 8.6               | 0.8            | 11.9          | 2.0             | 0.2            | 10.1          | 1.6           | 0.0            | 2.7           | 1.4            | 0.0            | 0.0           | 0.5              | 0.0            | 0.0           |
| J0340.6–2113  | 2.0               | 0.0            | 2.6           | 0.2             | 0.1            | 3.4           | 0.7           | 0.2            | 5.8           | 1.6            | 0.0            | 1.7           | 0.6              | 0.0            | 0.0           |
| J0340.7–2421  | 2.0               | 0.0            | 2.0           | 0.2             | 0.0            | 1.6           | 0.4           | 0.1            | 3.6           | 1.7            | 0.0            | 2.0           | 1.0              | 0.0            | 2.1           |
| J0341.8+3148c | 2.1               | 0.0            | 0.0           | 1.0             | 0.2            | 7.3           | 1.0           | 0.3            | 3.4           | 2.2            | 0.9            | 3.2           | 0.9              | 0.4            | 3.6           |
| J0342.4+3859  | 2.1               | 0.6            | 3.7           | 0.4             | 0.1            | 4.2           | 0.6           | 0.2            | 3.4           | 2.1            | 0.7            | 4.4           | 1.0              | 0.4            | 5.4           |
| J0345.2–2356  | 2.0               | 0.7            | 4.9           | 0.5             | 0.1            | 7.4           | 0.7           | 0.2            | 6.0           | 1.2            | 0.5            | 3.9           | 0.6              | 0.0            | 0.0           |
| J0348.6–2750  | 1.7               | 0.0            | 2.4           | 0.3             | 0.1            | 4.6           | 0.4           | 0.1            | 4.4           | 1.5            | 0.6            | 4.8           | 1.0              | 0.0            | 2.1           |
| J0350.0–2104  | 4.1               | 0.5            | 11.0          | 1.3             | 0.1            | 17.7          | 1.9           | 0.2            | 12.0          | 2.1            | 0.7            | 5.3           | 0.7              | 0.0            | 1.5           |
| J0353.2+5653  | 1.0               | 0.0            | 0.0           | 0.5             | 0.0            | 1.6           | 0.8           | 0.3            | 3.6           | 2.1            | 0.0            | 1.0           | 0.7              | 0.4            | 3.8           |
| J0354.1+8010  | 1.5               | 0.4            | 3.9           | 0.4             | 0.1            | 6.3           | 1.1           | 0.2            | 8.2           | 1.7            | 0.6            | 5.0           | 1.0              | 0.0            | 2.8           |
| J0357.0–4950  | 0.3               | 0.0            | 0.0           | 0.1             | 0.0            | 0.2           | 0.4           | 0.1            | 5.0           | 1.4            | 0.0            | 1.8           | 1.4              | 0.0            | 3.2           |
| J0357.8+3205  | 5.5               | 0.5            | 13.2          | 3.3             | 0.1            | 33.3          | 8.1           | 0.4            | 31.3          | 4.4            | 1.0            | 7.9           | 0.7              | 0.0            | 0.0           |
| J0359.1+6003  | 3.0               | 0.0            | 2.0           | 0.7             | 0.1            | 5.4           | 1.2           | 0.3            | 5.2           | 2.4            | 0.8            | 3.9           | 0.7              | 0.0            | 0.0           |
| J0359.5+5410  | 2.9               | 0.0            | 3.0           | 1.2             | 0.2            | 8.3           | 3.1           | 0.4            | 8.6           | 5.5            | 1.2            | 6.6           | 0.5              | 0.0            | 0.0           |
| J0401.6–3153  | 2.0               | 0.0            | 3.0           | 0.2             | 0.0            | 2.1           | 0.4           | 0.0            | 1.7           | 2.2            | 0.0            | 3.4           | 0.8              | 0.0            | 1.5           |
| J0402.0–2616  | 1.6               | 0.0            | 2.4           | 0.3             | 0.0            | 2.2           | 0.5           | 0.1            | 4.5           | 1.6            | 0.0            | 1.9           | 1.5              | 0.0            | 3.2           |

Table 1—Continued

|               | 100 MeV – 300 MeV |                |               | 300 MeV – 1 GeV |                |               | 1 GeV – 3 GeV |                |               | 3 GeV – 10 GeV |                |               | 10 GeV – 100 GeV |                |               |
|---------------|-------------------|----------------|---------------|-----------------|----------------|---------------|---------------|----------------|---------------|----------------|----------------|---------------|------------------|----------------|---------------|
| Name 2FGL     | $F_1^a$           | $\Delta F_1^a$ | $\sqrt{TS_1}$ | $F_2^a$         | $\Delta F_2^a$ | $\sqrt{TS_2}$ | $F_3^b$       | $\Delta F_3^b$ | $\sqrt{TS_3}$ | $F_4^c$        | $\Delta F_4^c$ | $\sqrt{TS_4}$ | $F_5^c$          | $\Delta F_5^c$ | $\sqrt{TS_5}$ |
| J0403.9–3604  | 14.0              | 0.6            | 33.9          | 3.7             | 0.1            | 45.7          | 5.2           | 0.3            | 28.8          | 5.0            | 1.0            | 9.9           | 0.8              | 0.0            | 1.8           |
| J0404.0+3843  | 2.3               | 0.7            | 3.6           | 0.7             | 0.0            | 3.0           | 1.2           | 0.0            | 2.8           | 1.6            | 0.0            | 0.2           | 0.8              | 0.0            | 1.1           |
| J0404.6+5822  | 3.3               | 0.9            | 4.7           | 0.6             | 0.0            | 2.5           | 1.1           | 0.0            | 2.8           | 3.2            | 0.0            | 2.8           | 0.7              | 0.0            | 1.3           |
| J0405.8–1309  | 2.0               | 0.0            | 2.8           | 0.3             | 0.0            | 3.0           | 0.6           | 0.0            | 2.3           | 2.2            | 0.0            | 2.1           | 0.8              | 0.0            | 2.1           |
| J0407.3–3826  | 3.0               | 0.5            | 7.0           | 0.8             | 0.1            | 13.1          | 1.6           | 0.2            | 11.6          | 4.1            | 0.9            | 8.6           | 1.2              | 0.0            | 2.2           |
| J0407.7+0740  | 1.7               | 0.6            | 3.2           | 0.3             | 0.1            | 3.5           | 0.6           | 0.2            | 3.6           | 2.4            | 0.0            | 1.9           | 1.1              | 0.0            | 2.6           |
| J0409.5+0509  | 1.9               | 0.6            | 3.5           | 0.4             | 0.1            | 3.7           | 0.6           | 0.0            | 1.2           | 2.6            | 0.0            | 2.4           | 0.9              | 0.0            | 1.7           |
| J0409.8–0357  | 1.9               | 0.0            | 2.2           | 0.2             | 0.1            | 3.4           | 0.6           | 0.2            | 4.4           | 1.6            | 0.6            | 4.3           | 1.5              | 0.0            | 3.0           |
| J0413.5–5332  | 1.8               | 0.5            | 4.8           | 0.5             | 0.1            | 8.7           | 0.9           | 0.2            | 8.2           | 2.0            | 0.7            | 5.4           | 1.4              | 0.0            | 3.5           |
| J0414.9–0855  | 1.3               | 0.0            | 1.8           | 0.1             | 0.0            | 0.0           | 0.5           | 0.0            | 1.4           | 1.9            | 0.0            | 2.8           | 1.9              | 0.0            | 3.8           |
| J0415.2+5518  | 1.9               | 0.0            | 0.0           | 0.8             | 0.0            | 3.0           | 1.1           | 0.0            | 1.9           | 2.5            | 0.9            | 3.6           | 1.3              | 0.0            | 1.9           |
| J0416.0–4355  | 1.7               | 0.0            | 2.6           | 0.2             | 0.1            | 3.4           | 0.5           | 0.1            | 4.5           | 1.7            | 0.0            | 2.3           | 0.5              | 0.0            | 0.0           |
| J0416.7–1849  | 1.2               | 0.4            | 3.3           | 0.4             | 0.1            | 6.7           | 1.0           | 0.2            | 8.5           | 1.5            | 0.6            | 4.5           | 0.8              | 0.4            | 4.2           |
| J0416.8+0105  | 1.3               | 0.0            | 0.5           | 0.3             | 0.0            | 1.1           | 0.4           | 0.2            | 3.5           | 2.0            | 0.7            | 5.1           | 1.4              | 0.0            | 3.4           |
| J0418.9+6636  | 1.9               | 0.0            | 1.3           | 0.5             | 0.1            | 4.6           | 1.3           | 0.2            | 6.6           | 2.5            | 0.8            | 4.3           | 1.0              | 0.0            | 2.1           |
| J0420.9–3743  | 2.0               | 0.0            | 0.9           | 0.4             | 0.0            | 2.4           | 0.7           | 0.2            | 4.9           | 1.6            | 0.0            | 1.2           | 1.0              | 0.0            | 2.6           |
| J0422.1–0645  | 1.2               | 0.0            | 0.9           | 0.3             | 0.1            | 5.0           | 0.5           | 0.2            | 4.1           | 2.3            | 0.0            | 2.5           | 1.1              | 0.0            | 2.7           |
| J0423.2–0120  | 10.3              | 0.7            | 20.4          | 2.5             | 0.1            | 28.3          | 4.9           | 0.4            | 24.1          | 13.6           | 1.6            | 18.3          | 2.4              | 0.6            | 9.0           |
| J0423.4+5612  | 2.8               | 0.0            | 2.2           | 0.6             | 0.0            | 2.8           | 0.6           | 0.0            | 0.9           | 3.8            | 0.0            | 3.0           | 1.1              | 0.5            | 4.1           |
| J0423.8+4149  | 2.3               | 0.0            | 2.0           | 0.6             | 0.0            | 3.0           | 1.7           | 0.3            | 7.5           | 10.0           | 1.4            | 12.5          | 3.3              | 0.7            | 10.1          |
| J0424.3–5332  | 2.0               | 0.0            | 3.0           | 0.3             | 0.0            | 2.9           | 0.5           | 0.1            | 5.1           | 2.1            | 0.0            | 2.8           | 1.0              | 0.0            | 1.9           |
| J0424.7+0034  | 2.5               | 0.7            | 4.7           | 0.7             | 0.1            | 8.9           | 1.7           | 0.2            | 10.3          | 2.0            | 0.7            | 4.7           | 1.7              | 0.0            | 3.4           |
| J0426.6+0509c | 2.5               | 0.6            | 4.4           | 0.6             | 0.1            | 6.3           | 0.9           | 0.0            | 3.1           | 1.9            | 0.0            | 1.1           | 0.9              | 0.0            | 0.0           |
| J0426.7+5434  | 4.3               | 0.7            | 7.6           | 1.8             | 0.2            | 12.0          | 3.2           | 0.4            | 9.7           | 3.4            | 1.0            | 4.4           | 0.9              | 0.0            | 1.7           |
| J0427.2–6705  | 1.9               | 0.0            | 2.7           | 0.3             | 0.1            | 4.0           | 0.4           | 0.1            | 3.3           | 1.9            | 0.0            | 2.8           | 0.6              | 0.0            | 0.0           |
| J0428.0–3845  | 4.6               | 1.1            | 4.3           | 0.9             | 0.2            | 5.8           | 0.9           | 0.0            | 1.6           | 3.8            | 0.0            | 3.1           | 0.7              | 0.0            | 0.0           |
| J0428.6–3756  | 18.5              | 1.0            | 22.2          | 7.3             | 0.2            | 49.9          | 22.4          | 0.7            | 64.2          | 75.1           | 3.5            | 53.4          | 14.6             | 1.5            | 28.0          |
| J0430.2+3508c | 3.7               | 0.0            | 2.4           | 0.5             | 0.1            | 4.3           | 1.3           | 0.3            | 5.1           | 3.9            | 0.0            | 2.9           | 0.9              | 0.0            | 1.0           |
| J0430.4–2507  | 1.3               | 0.0            | 1.0           | 0.2             | 0.0            | 1.7           | 0.4           | 0.1            | 3.8           | 1.6            | 0.0            | 1.9           | 0.8              | 0.0            | 1.9           |
| J0431.5+3622  | 3.9               | 0.0            | 2.9           | 0.7             | 0.0            | 3.0           | 1.3           | 0.0            | 2.6           | 2.8            | 1.0            | 4.1           | 1.0              | 0.0            | 1.9           |
| J0433.4–6029  | 1.4               | 0.4            | 3.4           | 0.6             | 0.1            | 9.6           | 0.9           | 0.2            | 7.1           | 1.7            | 0.0            | 2.5           | 0.5              | 0.0            | 0.0           |
| J0433.5+2905  | 2.2               | 0.7            | 3.6           | 1.1             | 0.1            | 9.3           | 3.0           | 0.4            | 11.5          | 12.3           | 1.6            | 13.9          | 2.2              | 0.6            | 7.3           |
| J0433.7+3233  | 2.3               | 0.0            | 1.9           | 0.2             | 0.0            | 0.0           | 1.1           | 0.0            | 3.1           | 2.4            | 0.0            | 1.8           | 0.9              | 0.4            | 4.3           |
| J0433.9–5726  | 1.5               | 0.0            | 2.5           | 0.1             | 0.0            | 0.8           | 0.4           | 0.1            | 4.7           | 1.3            | 0.5            | 4.6           | 1.0              | 0.4            | 4.9           |
| J0434.1–2014  | 1.4               | 0.0            | 1.2           | 0.3             | 0.1            | 4.5           | 0.6           | 0.2            | 5.2           | 2.5            | 0.0            | 3.0           | 0.9              | 0.0            | 1.2           |
| J0435.1–2341  | 1.8               | 0.0            | 1.9           | 0.2             | 0.1            | 3.5           | 0.7           | 0.0            | 2.8           | 2.3            | 0.0            | 2.9           | 0.7              | 0.0            | 0.0           |
| J0436.2+6759  | 1.7               | 0.0            | 1.3           | 0.4             | 0.0            | 2.8           | 0.7           | 0.0            | 1.8           | 1.4            | 0.6            | 3.6           | 0.9              | 0.0            | 2.3           |
| J0437.3–4712  | 1.8               | 0.4            | 5.8           | 1.0             | 0.1            | 16.8          | 1.9           | 0.2            | 14.2          | 1.8            | 0.6            | 6.2           | 0.4              | 0.0            | 0.0           |
| J0438.0–7331  | 0.5               | 0.0            | 0.0           | 0.1             | 0.0            | 0.2           | 0.5           | 0.0            | 1.7           | 1.6            | 0.6            | 4.3           | 0.8              | 0.4            | 5.0           |
| J0438.8–4521  | 1.9               | 0.0            | 2.0           | 0.4             | 0.1            | 6.7           | 1.1           | 0.2            | 8.9           | 1.3            | 0.5            | 4.0           | 0.8              | 0.0            | 1.8           |
| J0439.0–1252  | 1.2               | 0.0            | 1.0           | 0.3             | 0.1            | 3.6           | 0.6           | 0.0            | 2.0           | 2.5            | 0.0            | 2.9           | 0.9              | 0.0            | 0.8           |
| J0439.8–1858  | 1.6               | 0.0            | 2.2           | 0.2             | 0.0            | 0.9           | 0.4           | 0.1            | 3.9           | 2.3            | 0.7            | 5.5           | 1.5              | 0.0            | 5.0           |
| J0440.1–3211  | 0.7               | 0.0            | 0.3           | 0.1             | 0.0            | 0.0           | 0.3           | 0.1            | 3.5           | 1.9            | 0.0            | 2.4           | 1.5              | 0.0            | 3.1           |
| J0440.4+1433  | 2.1               | 0.0            | 1.5           | 0.5             | 0.1            | 4.1           | 1.1           | 0.0            | 2.9           | 3.3            | 0.0            | 3.0           | 0.6              | 0.0            | 0.0           |

Table 1—Continued

|               | 100 MeV – 300 MeV |                |               | 300 MeV – 1 GeV |                |               | 1 GeV – 3 GeV |                |               | 3 GeV – 10 GeV |                |               | 10 GeV – 100 GeV |                |               |
|---------------|-------------------|----------------|---------------|-----------------|----------------|---------------|---------------|----------------|---------------|----------------|----------------|---------------|------------------|----------------|---------------|
| Name 2FGL     | $F_1^a$           | $\Delta F_1^a$ | $\sqrt{TS_1}$ | $F_2^a$         | $\Delta F_2^a$ | $\sqrt{TS_2}$ | $F_3^b$       | $\Delta F_3^b$ | $\sqrt{TS_3}$ | $F_4^c$        | $\Delta F_4^c$ | $\sqrt{TS_4}$ | $F_5^c$          | $\Delta F_5^c$ | $\sqrt{TS_5}$ |
| J0440.5+2554c | 3.6               | 0.0            | 2.6           | 0.5             | 0.2            | 3.6           | 1.1           | 0.3            | 3.8           | 2.8            | 0.0            | 1.5           | 0.8              | 0.0            | 0.0           |
| J0440.9+2749  | 1.5               | 0.0            | 0.0           | 0.6             | 0.0            | 2.8           | 0.5           | 0.0            | 0.3           | 2.5            | 0.8            | 4.9           | 1.2              | 0.5            | 4.6           |
| J0442.7–0017  | 12.4              | 0.6            | 24.2          | 2.9             | 0.1            | 32.5          | 4.9           | 0.3            | 25.3          | 8.5            | 1.3            | 13.7          | 0.9              | 0.4            | 4.5           |
| J0448.5–1633  | 1.3               | 0.0            | 1.5           | 0.2             | 0.1            | 3.7           | 0.5           | 0.1            | 4.6           | 2.2            | 0.7            | 5.3           | 1.3              | 0.5            | 6.4           |
| J0448.6–2118  | 1.6               | 0.0            | 1.5           | 0.2             | 0.1            | 3.3           | 0.6           | 0.0            | 2.7           | 2.7            | 0.0            | 2.8           | 0.5              | 0.0            | 0.0           |
| J0448.9+1121  | 6.2               | 0.5            | 12.5          | 2.0             | 0.1            | 17.4          | 3.1           | 0.3            | 13.1          | 3.7            | 1.0            | 5.8           | 1.2              | 0.0            | 2.1           |
| J0449.4–4350  | 5.2               | 0.5            | 14.1          | 2.0             | 0.1            | 28.9          | 7.4           | 0.4            | 37.9          | 32.6           | 2.3            | 35.2          | 11.3             | 1.3            | 24.3          |
| J0451.8–7011  | 1.2               | 0.0            | 0.5           | 0.3             | 0.0            | 1.1           | 0.6           | 0.2            | 4.2           | 1.9            | 0.0            | 2.1           | 0.9              | 0.0            | 0.8           |
| J0453.1–2807  | 6.6               | 0.5            | 15.0          | 1.3             | 0.1            | 18.1          | 1.7           | 0.2            | 12.8          | 2.7            | 0.0            | 3.2           | 1.3              | 0.0            | 2.2           |
| J0455.8–6920  | 1.1               | 0.0            | 0.0           | 0.6             | 0.1            | 6.5           | 0.5           | 0.2            | 3.2           | 2.0            | 0.0            | 2.0           | 0.9              | 0.0            | 1.3           |
| J0456.1–4613  | 4.1               | 0.5            | 9.3           | 1.0             | 0.1            | 14.2          | 1.2           | 0.2            | 8.8           | 1.7            | 0.0            | 1.7           | 0.8              | 0.0            | 1.1           |
| J0456.5+2658  | 2.4               | 0.7            | 3.5           | 0.8             | 0.1            | 5.8           | 1.2           | 0.3            | 4.9           | 2.4            | 0.9            | 4.1           | 0.9              | 0.0            | 1.1           |
| J0456.5–3132  | 1.8               | 0.0            | 2.6           | 0.3             | 0.1            | 4.5           | 0.4           | 0.1            | 3.7           | 2.0            | 0.0            | 2.9           | 0.5              | 0.0            | 0.0           |
| J0457.0–2325  | 22.7              | 0.6            | 51.4          | 8.1             | 0.2            | 79.9          | 18.8          | 0.6            | 66.8          | 39.3           | 2.6            | 39.6          | 4.4              | 0.9            | 12.7          |
| J0458.4+0654  | 2.4               | 0.6            | 4.6           | 0.3             | 0.1            | 3.3           | 0.5           | 0.2            | 3.6           | 2.1            | 0.0            | 2.6           | 0.9              | 0.0            | 1.6           |
| J0501.2–0155  | 2.5               | 0.5            | 5.3           | 0.5             | 0.1            | 6.3           | 0.8           | 0.2            | 6.0           | 1.7            | 0.7            | 3.9           | 0.7              | 0.0            | 0.4           |
| J0502.5+0607  | 2.1               | 0.0            | 0.0           | 0.4             | 0.1            | 4.4           | 0.5           | 0.2            | 3.9           | 1.6            | 0.0            | 1.0           | 0.5              | 0.0            | 0.0           |
| J0503.2+4643  | 3.1               | 0.0            | 2.5           | 0.9             | 0.2            | 6.5           | 1.0           | 0.0            | 1.9           | 4.2            | 0.0            | 3.1           | 1.1              | 0.0            | 1.9           |
| J0503.3+4517  | 1.3               | 0.0            | 0.0           | 0.5             | 0.0            | 2.1           | 1.2           | 0.0            | 2.5           | 3.0            | 1.0            | 4.1           | 1.3              | 0.5            | 4.4           |
| J0505.4+0419  | 3.1               | 0.0            | 0.5           | 0.5             | 0.0            | 2.7           | 0.6           | 0.2            | 3.6           | 2.4            | 0.0            | 2.7           | 1.4              | 0.0            | 3.2           |
| J0505.5+0501  | 6.2               | 0.0            | 2.1           | 0.4             | 0.1            | 3.7           | 1.3           | 0.2            | 7.1           | 1.8            | 0.7            | 4.1           | 0.9              | 0.0            | 2.0           |
| J0505.8–0411  | 1.1               | 0.0            | 0.3           | 0.3             | 0.1            | 3.6           | 0.7           | 0.2            | 4.8           | 2.6            | 0.0            | 3.0           | 0.7              | 0.0            | 0.0           |
| J0505.9+6116  | 0.6               | 0.0            | 0.0           | 0.3             | 0.0            | 1.0           | 0.8           | 0.0            | 2.1           | 1.8            | 0.7            | 3.7           | 1.4              | 0.0            | 3.4           |
| J0506.5–0901  | 1.9               | 0.0            | 2.2           | 0.2             | 0.1            | 3.3           | 0.8           | 0.0            | 3.1           | 1.9            | 0.0            | 1.5           | 1.4              | 0.0            | 3.1           |
| J0506.7–5435  | 0.6               | 0.0            | 0.0           | 0.2             | 0.0            | 1.4           | 0.5           | 0.0            | 2.3           | 2.1            | 0.7            | 6.1           | 0.7              | 0.3            | 5.2           |
| J0507.5–6102  | 2.6               | 0.6            | 6.1           | 0.6             | 0.1            | 9.3           | 1.0           | 0.2            | 8.6           | 2.0            | 0.7            | 5.2           | 1.4              | 0.0            | 3.2           |
| J0508.0+6737  | 1.5               | 0.0            | 2.3           | 0.2             | 0.1            | 3.9           | 1.0           | 0.2            | 7.4           | 6.8            | 1.0            | 13.6          | 6.3              | 0.9            | 19.8          |
| J0508.1–1936  | 1.6               | 0.0            | 1.7           | 0.3             | 0.0            | 2.6           | 0.5           | 0.1            | 4.6           | 0.9            | 0.0            | 0.0           | 0.6              | 0.0            | 0.0           |
| J0509.2+1013  | 2.4               | 0.6            | 4.2           | 0.5             | 0.1            | 4.7           | 1.2           | 0.2            | 6.2           | 2.4            | 0.8            | 4.9           | 0.8              | 0.0            | 1.8           |
| J0509.4+0542  | 4.0               | 0.9            | 8.0           | 1.4             | 0.1            | 15.7          | 3.2           | 0.3            | 16.8          | 12.6           | 1.5            | 17.1          | 2.6              | 0.6            | 10.0          |
| J0509.9+1802  | 3.4               | 0.0            | 3.1           | 0.5             | 0.1            | 4.6           | 0.8           | 0.2            | 4.3           | 3.6            | 0.9            | 6.1           | 0.9              | 0.0            | 1.4           |
| J0512.9+4040  | 0.4               | 0.0            | 0.0           | 0.4             | 0.0            | 1.2           | 0.8           | 0.3            | 4.0           | 4.1            | 1.1            | 5.8           | 1.1              | 0.0            | 2.1           |
| J0515.0–4411  | 2.4               | 0.0            | 2.7           | 0.4             | 0.1            | 5.6           | 0.4           | 0.1            | 3.5           | 0.8            | 0.0            | 0.0           | 0.5              | 0.0            | 0.0           |
| J0515.5+7355  | 0.8               | 0.0            | 0.6           | 0.1             | 0.0            | 0.3           | 0.5           | 0.0            | 2.1           | 2.1            | 0.0            | 3.0           | 1.3              | 0.0            | 3.8           |
| J0515.9+1528  | 2.3               | 0.0            | 1.8           | 0.4             | 0.0            | 1.8           | 1.1           | 0.3            | 5.7           | 2.7            | 0.8            | 5.1           | 1.4              | 0.5            | 6.9           |
| J0516.5–4601  | 1.5               | 0.6            | 3.4           | 0.2             | 0.1            | 3.6           | 0.4           | 0.1            | 3.7           | 2.2            | 0.0            | 2.5           | 0.6              | 0.0            | 0.0           |
| J0516.7+2634  | 4.4               | 0.9            | 5.5           | 0.8             | 0.2            | 5.0           | 1.2           | 0.3            | 4.3           | 3.2            | 0.0            | 2.6           | 0.6              | 0.0            | 0.1           |
| J0516.8–6207  | 3.0               | 0.6            | 7.4           | 0.9             | 0.1            | 13.3          | 2.4           | 0.2            | 16.4          | 7.3            | 1.1            | 13.6          | 1.1              | 0.4            | 5.6           |
| J0517.0+4532  | 1.5               | 0.0            | 0.2           | 0.5             | 0.1            | 4.2           | 1.1           | 0.0            | 2.8           | 2.3            | 0.9            | 3.5           | 1.3              | 0.0            | 3.0           |
| J0517.5+0900  | 1.1               | 0.0            | 0.0           | 0.8             | 0.1            | 7.4           | 0.8           | 0.2            | 3.9           | 2.6            | 0.9            | 4.9           | 1.1              | 0.0            | 1.9           |
| J0521.4–1736  | 1.6               | 0.0            | 1.8           | 0.3             | 0.1            | 4.2           | 0.6           | 0.0            | 2.3           | 1.9            | 0.0            | 2.4           | 0.9              | 0.0            | 1.2           |
| J0521.7+2113  | 5.8               | 1.0            | 7.3           | 1.8             | 0.2            | 13.1          | 5.9           | 0.4            | 20.8          | 25.9           | 2.2            | 23.1          | 8.4              | 1.2            | 18.8          |
| J0521.9+0108  | 1.0               | 0.0            | 0.4           | 0.1             | 0.0            | 0.0           | 0.5           | 0.0            | 1.8           | 1.5            | 0.6            | 4.2           | 1.7              | 0.0            | 3.4           |
| J0523.0–3628  | 9.6               | 0.6            | 22.1          | 2.3             | 0.1            | 29.5          | 4.0           | 0.3            | 22.0          | 6.6            | 1.1            | 11.9          | 1.7              | 0.0            | 3.4           |



Table 1—Continued

|               | 100 MeV – 300 MeV |                |               | 300 MeV – 1 GeV |                |               | 1 GeV – 3 GeV |                |               | 3 GeV – 10 GeV |                |               | 10 GeV – 100 GeV |                |               |
|---------------|-------------------|----------------|---------------|-----------------|----------------|---------------|---------------|----------------|---------------|----------------|----------------|---------------|------------------|----------------|---------------|
| Name 2FGL     | $F_1^a$           | $\Delta F_1^a$ | $\sqrt{TS_1}$ | $F_2^a$         | $\Delta F_2^a$ | $\sqrt{TS_2}$ | $F_3^b$       | $\Delta F_3^b$ | $\sqrt{TS_3}$ | $F_4^c$        | $\Delta F_4^c$ | $\sqrt{TS_4}$ | $F_5^c$          | $\Delta F_5^c$ | $\sqrt{TS_5}$ |
| J0523.3–2530  | 1.7               | 0.4            | 4.5           | 0.5             | 0.1            | 7.7           | 1.7           | 0.2            | 13.0          | 5.2            | 1.0            | 10.3          | 0.8              | 0.0            | 0.0           |
| J0524.1+2843  | 3.1               | 0.0            | 2.0           | 0.7             | 0.0            | 3.0           | 1.1           | 0.0            | 2.6           | 2.5            | 0.9            | 3.9           | 1.4              | 0.0            | 3.1           |
| J0525.5–6011  | 1.2               | 0.0            | 1.0           | 0.2             | 0.0            | 1.1           | 0.4           | 0.0            | 2.1           | 2.4            | 0.7            | 6.0           | 0.6              | 0.0            | 0.0           |
| J0526.1–4829  | 1.9               | 0.0            | 0.5           | 0.7             | 0.1            | 7.7           | 1.0           | 0.2            | 7.3           | 2.4            | 0.8            | 5.3           | 1.8              | 0.0            | 4.0           |
| J0526.6–6825e | 19.0              | 0.9            | 24.0          | 6.6             | 0.2            | 40.8          | 15.7          | 0.7            | 33.6          | 31.8           | 2.8            | 17.4          | 5.1              | 1.1            | 7.5           |
| J0526.6+2248  | 5.7               | 1.6            | 4.8           | 1.0             | 0.2            | 5.0           | 1.4           | 0.0            | 2.6           | 3.2            | 0.0            | 2.3           | 1.3              | 0.0            | 1.9           |
| J0526.6+4308  | 2.6               | 0.0            | 2.2           | 0.6             | 0.1            | 4.6           | 0.8           | 0.3            | 3.5           | 2.7            | 0.0            | 1.5           | 0.5              | 0.0            | 0.0           |
| J0526.8+6326  | 1.4               | 0.0            | 1.3           | 0.3             | 0.0            | 2.0           | 0.5           | 0.2            | 4.0           | 1.7            | 0.0            | 1.5           | 0.8              | 0.0            | 0.6           |
| J0529.2+0935  | 3.5               | 0.8            | 5.3           | 0.5             | 0.1            | 4.9           | 0.7           | 0.2            | 3.7           | 1.2            | 0.0            | 0.0           | 0.8              | 0.4            | 4.1           |
| J0529.3+3821  | 0.9               | 0.0            | 0.0           | 0.8             | 0.2            | 5.4           | 1.2           | 0.0            | 2.1           | 3.4            | 0.0            | 2.0           | 2.1              | 0.0            | 3.7           |
| J0530.8–0517c | 1.6               | 0.0            | 1.8           | 0.4             | 0.1            | 3.7           | 1.3           | 0.3            | 5.4           | 1.0            | 0.0            | 0.0           | 0.5              | 0.0            | 0.0           |
| J0530.8+1333  | 7.3               | 0.7            | 11.9          | 1.6             | 0.1            | 12.4          | 2.3           | 0.3            | 8.4           | 2.6            | 1.0            | 3.7           | 0.7              | 0.0            | 1.0           |
| J0531.8–3831  | 2.0               | 0.8            | 4.4           | 0.3             | 0.1            | 4.5           | 0.4           | 0.2            | 3.2           | 1.0            | 0.0            | 0.6           | 1.0              | 0.0            | 2.1           |
| J0531.8–8324  | 1.5               | 0.0            | 1.2           | 0.5             | 0.1            | 5.8           | 1.0           | 0.2            | 6.3           | 1.5            | 0.7            | 3.2           | 1.0              | 0.5            | 4.2           |
| J0532.0–4826  | 3.7               | 0.8            | 4.9           | 0.8             | 0.1            | 9.3           | 2.5           | 0.3            | 15.4          | 6.2            | 1.1            | 11.6          | 1.7              | 0.5            | 6.7           |
| J0532.5–7223  | 2.4               | 0.5            | 4.8           | 0.3             | 0.0            | 2.2           | 0.7           | 0.0            | 2.9           | 1.4            | 0.0            | 1.6           | 1.1              | 0.0            | 1.4           |
| J0532.7+0733  | 5.0               | 0.7            | 8.2           | 1.6             | 0.1            | 14.7          | 3.4           | 0.3            | 15.2          | 6.9            | 1.2            | 10.5          | 0.9              | 0.4            | 4.2           |
| J0533.0+4823  | 4.2               | 0.6            | 8.0           | 1.2             | 0.1            | 11.5          | 2.5           | 0.3            | 11.6          | 3.8            | 1.0            | 6.0           | 1.1              | 0.5            | 4.7           |
| J0533.3–6651  | 2.8               | 0.0            | 3.0           | 0.4             | 0.1            | 4.1           | 0.9           | 0.0            | 3.0           | 2.8            | 0.0            | 1.9           | 1.6              | 0.0            | 2.3           |
| J0533.9+6759  | 0.6               | 0.0            | 0.8           | 0.2             | 0.1            | 4.0           | 1.2           | 0.2            | 8.7           | 3.7            | 0.8            | 7.4           | 0.6              | 0.0            | 0.1           |
| J0534.5+2201  | 194.8             | 1.7            | 193.5         | 57.8            | 0.4            | 240.0         | 145.5         | 1.6            | 204.5         | 349.6          | 7.3            | 131.7         | 74.5             | 3.3            | 69.6          |
| J0534.8–0548c | 4.1               | 0.0            | 0.9           | 0.7             | 0.0            | 1.4           | 1.6           | 0.4            | 4.8           | 3.9            | 1.2            | 4.3           | 1.4              | 0.0            | 1.3           |
| J0534.9–0450c | 4.4               | 0.0            | 1.0           | 0.6             | 0.2            | 3.6           | 1.3           | 0.3            | 4.3           | 2.5            | 1.0            | 3.3           | 1.0              | 0.0            | 1.7           |
| J0536.2–3348  | 4.2               | 0.5            | 10.0          | 0.9             | 0.1            | 12.8          | 1.2           | 0.2            | 9.3           | 3.8            | 0.9            | 8.0           | 1.9              | 0.6            | 7.3           |
| J0537.7–5716  | 1.6               | 0.0            | 1.8           | 0.1             | 0.0            | 0.5           | 0.6           | 0.0            | 2.8           | 1.3            | 0.6            | 3.6           | 1.3              | 0.0            | 3.6           |
| J0538.1+2718  | 2.5               | 0.0            | 0.8           | 0.8             | 0.2            | 4.4           | 1.6           | 0.0            | 3.0           | 3.3            | 1.1            | 4.1           | 1.2              | 0.0            | 2.3           |
| J0538.5–3909  | 1.3               | 0.0            | 0.1           | 0.3             | 0.1            | 4.4           | 0.4           | 0.1            | 3.3           | 2.0            | 0.0            | 2.9           | 1.3              | 0.0            | 3.7           |
| J0538.5–0534c | 2.5               | 0.7            | 3.8           | 1.8             | 0.2            | 9.9           | 1.3           | 0.3            | 4.5           | 1.3            | 0.0            | 0.0           | 0.6              | 0.0            | 0.0           |
| J0538.8–4405  | 28.6              | 0.6            | 63.5          | 10.4            | 0.2            | 98.0          | 28.0          | 0.7            | 88.2          | 81.5           | 3.6            | 61.9          | 16.7             | 1.6            | 30.6          |
| J0539.3–0323  | 3.1               | 0.0            | 1.6           | 0.7             | 0.1            | 5.2           | 1.1           | 0.0            | 2.5           | 2.6            | 0.0            | 2.6           | 1.0              | 0.0            | 0.4           |
| J0539.3–2841  | 3.5               | 0.5            | 7.8           | 0.5             | 0.1            | 7.4           | 0.6           | 0.0            | 2.9           | 2.0            | 0.0            | 2.8           | 0.8              | 0.0            | 0.9           |
| J0540.1–7554  | 1.7               | 0.0            | 1.0           | 0.3             | 0.0            | 2.8           | 0.6           | 0.0            | 2.7           | 1.4            | 0.6            | 4.0           | 0.6              | 0.0            | 0.0           |
| J0540.3+3549c | 2.2               | 0.6            | 4.0           | 1.4             | 0.2            | 8.6           | 2.4           | 0.4            | 6.3           | 2.8            | 1.1            | 3.2           | 0.7              | 0.0            | 0.9           |
| J0540.4+5822  | 1.6               | 0.0            | 1.6           | 0.3             | 0.0            | 1.7           | 0.8           | 0.0            | 2.8           | 2.8            | 0.8            | 5.6           | 0.8              | 0.3            | 5.2           |
| J0540.4–5415  | 2.8               | 0.8            | 6.4           | 0.4             | 0.1            | 6.2           | 0.8           | 0.2            | 5.8           | 1.7            | 0.0            | 2.4           | 0.7              | 0.0            | 0.5           |
| J0541.8–0203c | 2.3               | 0.0            | 1.8           | 0.9             | 0.2            | 5.7           | 1.9           | 0.4            | 5.4           | 3.9            | 0.0            | 1.9           | 2.1              | 0.0            | 2.6           |
| J0543.2–0120c | 2.3               | 0.0            | 0.0           | 0.8             | 0.2            | 4.4           | 1.6           | 0.4            | 5.0           | 3.4            | 0.0            | 1.6           | 1.8              | 0.0            | 3.2           |
| J0543.9–5532  | 1.6               | 0.0            | 0.0           | 0.3             | 0.1            | 5.0           | 1.2           | 0.2            | 9.0           | 5.0            | 1.0            | 10.3          | 3.0              | 0.7            | 10.2          |
| J0545.6+6018  | 0.7               | 0.0            | 0.0           | 0.3             | 0.0            | 2.3           | 0.7           | 0.2            | 4.8           | 2.8            | 0.7            | 6.6           | 0.9              | 0.0            | 2.0           |
| J0547.1+0020c | 3.1               | 0.7            | 5.5           | 1.2             | 0.2            | 8.5           | 1.5           | 0.3            | 5.0           | 3.8            | 1.1            | 4.5           | 0.8              | 0.0            | 0.2           |
| J0547.4+3722  | 2.6               | 0.0            | 1.5           | 0.6             | 0.1            | 4.8           | 0.5           | 0.0            | 0.0           | 3.1            | 0.0            | 2.9           | 1.0              | 0.0            | 0.7           |
| J0547.5–0141c | 2.5               | 0.0            | 3.0           | 0.9             | 0.2            | 6.0           | 1.4           | 0.0            | 2.7           | 2.5            | 0.0            | 1.2           | 0.9              | 0.0            | 0.7           |
| J0553.9+3104  | 0.5               | 0.0            | 0.0           | 0.6             | 0.1            | 6.5           | 2.6           | 0.3            | 9.6           | 3.7            | 0.0            | 2.2           | 0.7              | 0.0            | 0.0           |
| J0555.9–4348  | 2.2               | 0.0            | 3.0           | 0.3             | 0.0            | 1.5           | 0.5           | 0.2            | 4.4           | 2.4            | 0.0            | 2.9           | 1.2              | 0.0            | 2.3           |

Table 1—Continued

|               | 100 MeV – 300 MeV |                |               | 300 MeV – 1 GeV |                |               | 1 GeV – 3 GeV |                |               | 3 GeV – 10 GeV |                |               | 10 GeV – 100 GeV |                |               |
|---------------|-------------------|----------------|---------------|-----------------|----------------|---------------|---------------|----------------|---------------|----------------|----------------|---------------|------------------|----------------|---------------|
| Name 2FGL     | $F_1^a$           | $\Delta F_1^a$ | $\sqrt{TS_1}$ | $F_2^a$         | $\Delta F_2^a$ | $\sqrt{TS_2}$ | $F_3^b$       | $\Delta F_3^b$ | $\sqrt{TS_3}$ | $F_4^c$        | $\Delta F_4^c$ | $\sqrt{TS_4}$ | $F_5^c$          | $\Delta F_5^c$ | $\sqrt{TS_5}$ |
| J0558.2–3837  | 1.6               | 0.5            | 4.0           | 0.2             | 0.1            | 3.3           | 0.6           | 0.0            | 2.5           | 2.0            | 0.7            | 5.5           | 1.2              | 0.0            | 2.1           |
| J0558.7–7501  | 2.1               | 0.0            | 1.5           | 0.4             | 0.0            | 2.8           | 0.8           | 0.2            | 5.8           | 1.6            | 0.6            | 4.2           | 1.2              | 0.0            | 1.8           |
| J0600.8–1949  | 2.0               | 0.0            | 2.2           | 0.3             | 0.1            | 4.5           | 0.5           | 0.2            | 3.3           | 2.0            | 0.0            | 1.8           | 0.5              | 0.0            | 0.0           |
| J0600.9+3839  | 1.9               | 0.0            | 1.5           | 0.5             | 0.0            | 2.3           | 0.9           | 0.0            | 2.4           | 2.2            | 0.0            | 1.3           | 0.8              | 0.4            | 5.0           |
| J0601.1–7037  | 3.3               | 0.5            | 7.7           | 1.4             | 0.1            | 17.0          | 3.2           | 0.3            | 17.9          | 4.7            | 1.0            | 9.0           | 0.7              | 0.3            | 4.3           |
| J0602.3+5315  | 1.4               | 0.0            | 1.5           | 0.1             | 0.0            | 0.0           | 0.4           | 0.2            | 3.2           | 2.1            | 0.8            | 3.9           | 0.9              | 0.4            | 4.7           |
| J0602.7–4011  | 1.3               | 0.0            | 0.6           | 0.3             | 0.1            | 4.7           | 0.7           | 0.2            | 4.9           | 3.6            | 0.9            | 7.3           | 1.5              | 0.0            | 3.1           |
| J0604.2–4817  | 0.6               | 0.0            | 0.0           | 0.2             | 0.1            | 3.2           | 0.5           | 0.2            | 4.6           | 2.1            | 0.0            | 2.4           | 0.9              | 0.4            | 5.7           |
| J0605.0+0001  | 0.8               | 0.0            | 0.0           | 0.3             | 0.0            | 1.1           | 0.6           | 0.2            | 3.4           | 2.0            | 0.0            | 1.5           | 0.8              | 0.4            | 3.8           |
| J0605.3+3758  | 0.5               | 0.0            | 0.0           | 0.2             | 0.1            | 3.3           | 1.0           | 0.2            | 5.5           | 3.2            | 0.0            | 3.0           | 0.6              | 0.0            | 0.0           |
| J0607.4+4739  | 1.4               | 0.4            | 3.3           | 0.5             | 0.1            | 6.1           | 1.8           | 0.3            | 10.3          | 6.2            | 1.1            | 10.9          | 0.9              | 0.4            | 4.4           |
| J0607.5–0618c | 1.4               | 0.4            | 3.5           | 0.7             | 0.1            | 5.1           | 1.2           | 0.3            | 4.3           | 1.7            | 0.0            | 0.2           | 1.4              | 0.0            | 1.7           |
| J0608.0–1521  | 4.3               | 0.5            | 9.1           | 1.3             | 0.1            | 13.2          | 2.1           | 0.3            | 10.2          | 3.0            | 0.9            | 5.4           | 0.6              | 0.0            | 0.0           |
| J0608.0–0836  | 2.6               | 0.7            | 4.0           | 0.9             | 0.1            | 6.8           | 1.3           | 0.3            | 5.8           | 4.5            | 1.1            | 7.0           | 0.8              | 0.0            | 1.3           |
| J0608.3+2037  | 2.5               | 0.0            | 2.1           | 1.7             | 0.2            | 9.4           | 3.0           | 0.5            | 6.9           | 3.1            | 1.2            | 3.2           | 1.5              | 0.0            | 2.2           |
| J0609.4–0248  | 2.3               | 0.8            | 4.0           | 0.4             | 0.0            | 1.6           | 0.6           | 0.2            | 3.8           | 2.7            | 0.9            | 5.1           | 1.3              | 0.5            | 5.3           |
| J0609.6–1847  | 1.4               | 0.0            | 0.3           | 0.4             | 0.0            | 2.8           | 0.5           | 0.2            | 3.8           | 2.0            | 0.0            | 1.5           | 0.8              | 0.0            | 0.0           |
| J0610.3–2059  | 2.0               | 0.0            | 2.2           | 0.3             | 0.1            | 4.5           | 0.9           | 0.2            | 6.1           | 1.3            | 0.6            | 3.2           | 0.9              | 0.0            | 1.4           |
| J0611.0+4321  | 2.0               | 0.0            | 2.0           | 0.2             | 0.0            | 0.0           | 0.8           | 0.0            | 2.8           | 2.6            | 0.0            | 3.0           | 0.9              | 0.4            | 3.7           |
| J0611.8–6059  | 1.4               | 0.5            | 3.4           | 0.2             | 0.1            | 3.7           | 0.5           | 0.2            | 4.0           | 1.3            | 0.5            | 4.0           | 0.6              | 0.0            | 1.7           |
| J0612.8+4122  | 2.2               | 0.6            | 4.8           | 0.9             | 0.1            | 10.2          | 3.0           | 0.3            | 15.5          | 7.3            | 1.2            | 11.2          | 3.1              | 0.7            | 10.2          |
| J0613.8–0200  | 1.4               | 0.0            | 0.0           | 1.0             | 0.1            | 9.5           | 4.3           | 0.4            | 17.1          | 8.7            | 1.3            | 12.1          | 0.8              | 0.0            | 0.4           |
| J0614.1–3329  | 3.5               | 0.4            | 10.6          | 2.9             | 0.1            | 38.5          | 13.7          | 0.5            | 53.8          | 41.0           | 2.6            | 39.5          | 2.5              | 0.6            | 8.9           |
| J0616.6+2425  | 2.2               | 0.0            | 0.0           | 0.8             | 0.0            | 2.8           | 1.0           | 0.3            | 3.9           | 3.1            | 0.0            | 2.2           | 0.9              | 0.0            | 0.4           |
| J0616.9+5701  | 1.1               | 0.0            | 1.1           | 0.3             | 0.1            | 4.8           | 0.6           | 0.2            | 5.1           | 2.3            | 0.7            | 5.7           | 1.7              | 0.5            | 7.7           |
| J0617.2+2234e | 27.4              | 0.9            | 36.8          | 15.1            | 0.3            | 75.9          | 44.8          | 1.0            | 77.2          | 141.4          | 4.8            | 60.9          | 31.2             | 2.2            | 33.3          |
| J0617.6–1716  | 1.7               | 0.0            | 1.4           | 0.4             | 0.1            | 4.2           | 0.8           | 0.2            | 4.7           | 3.0            | 0.9            | 5.6           | 1.8              | 0.6            | 6.5           |
| J0620.8–2556  | 2.1               | 0.0            | 3.0           | 0.2             | 0.1            | 3.2           | 0.8           | 0.0            | 2.9           | 1.9            | 0.7            | 4.6           | 1.0              | 0.0            | 0.9           |
| J0621.2+2508  | 2.4               | 0.0            | 1.4           | 0.6             | 0.0            | 2.6           | 0.9           | 0.3            | 4.3           | 3.0            | 0.9            | 4.8           | 0.6              | 0.0            | 0.0           |
| J0621.9+3750  | 1.0               | 0.0            | 1.6           | 0.9             | 0.1            | 11.2          | 1.7           | 0.3            | 8.8           | 2.0            | 0.0            | 1.4           | 0.5              | 0.0            | 0.0           |
| J0622.9+3326  | 3.2               | 0.6            | 5.9           | 1.2             | 0.1            | 11.0          | 3.0           | 0.3            | 12.8          | 9.9            | 1.4            | 13.2          | 1.4              | 0.5            | 6.0           |
| J0625.2+4441  | 1.5               | 0.0            | 1.5           | 0.3             | 0.0            | 2.7           | 0.4           | 0.2            | 3.2           | 2.1            | 0.7            | 5.5           | 0.9              | 0.4            | 5.0           |
| J0626.8–4258  | 0.8               | 0.0            | 0.1           | 0.2             | 0.0            | 1.4           | 0.5           | 0.0            | 2.1           | 1.1            | 0.5            | 3.2           | 1.8              | 0.0            | 3.9           |
| J0627.1–3528  | 1.8               | 0.0            | 2.6           | 0.4             | 0.1            | 5.5           | 1.0           | 0.2            | 7.3           | 3.3            | 0.9            | 6.6           | 1.3              | 0.5            | 6.3           |
| J0628.9–6246  | 1.0               | 0.0            | 0.3           | 0.2             | 0.0            | 1.1           | 0.5           | 0.2            | 4.4           | 1.8            | 0.0            | 2.0           | 1.1              | 0.5            | 4.1           |
| J0629.3–2001  | 2.6               | 0.5            | 5.2           | 0.8             | 0.1            | 9.0           | 1.6           | 0.2            | 9.1           | 7.0            | 1.2            | 10.6          | 1.4              | 0.0            | 1.5           |
| J0630.9–2406  | 1.8               | 0.0            | 2.3           | 0.6             | 0.1            | 7.9           | 2.0           | 0.3            | 12.3          | 8.4            | 1.3            | 13.6          | 4.5              | 0.9            | 12.9          |
| J0631.5+1035  | 2.4               | 0.8            | 3.5           | 1.3             | 0.2            | 9.3           | 4.5           | 0.4            | 13.5          | 11.5           | 1.7            | 11.0          | 1.1              | 0.5            | 3.7           |
| J0631.6+0640  | 7.8               | 0.0            | 1.7           | 1.4             | 0.3            | 5.4           | 2.8           | 0.5            | 5.8           | 8.3            | 1.7            | 7.4           | 1.5              | 0.0            | 1.8           |
| J0631.7+0428  | 4.2               | 0.9            | 4.9           | 1.2             | 0.2            | 5.6           | 2.6           | 0.5            | 6.3           | 4.0            | 1.4            | 3.9           | 0.9              | 0.0            | 0.0           |
| J0633.7+0633  | 8.3               | 0.0            | 0.6           | 3.0             | 0.3            | 10.4          | 12.4          | 0.7            | 24.5          | 26.3           | 2.4            | 19.3          | 1.9              | 0.0            | 2.8           |
| J0633.8+7132  | 2.2               | 0.0            | 2.9           | 0.3             | 0.1            | 4.3           | 0.7           | 0.0            | 3.2           | 0.9            | 0.0            | 0.8           | 0.7              | 0.0            | 0.0           |
| J0633.9+1746  | 195.4             | 1.2            | 236.3         | 145.5           | 0.6            | 486.3         | 597.1         | 3.2            | 497.2         | 1167.4         | 13.1           | 268.7         | 28.0             | 2.0            | 39.1          |
| J0634.3+0356c | 2.1               | 0.0            | 0.0           | 1.2             | 0.3            | 4.1           | 1.7           | 0.5            | 4.0           | 3.9            | 1.4            | 3.4           | 1.8              | 0.0            | 2.3           |

Table 1—Continued

|               | 100 MeV – 300 MeV |                |               | 300 MeV – 1 GeV |                |               | 1 GeV – 3 GeV |                |               | 3 GeV – 10 GeV |                |               | 10 GeV – 100 GeV |                |               |
|---------------|-------------------|----------------|---------------|-----------------|----------------|---------------|---------------|----------------|---------------|----------------|----------------|---------------|------------------|----------------|---------------|
| Name 2FGL     | $F_1^a$           | $\Delta F_1^a$ | $\sqrt{TS_1}$ | $F_2^a$         | $\Delta F_2^a$ | $\sqrt{TS_2}$ | $F_3^b$       | $\Delta F_3^b$ | $\sqrt{TS_3}$ | $F_4^c$        | $\Delta F_4^c$ | $\sqrt{TS_4}$ | $F_5^c$          | $\Delta F_5^c$ | $\sqrt{TS_5}$ |
| J0635.0–2334  | 1.1               | 0.0            | 0.0           | 0.4             | 0.0            | 3.0           | 0.7           | 0.2            | 4.9           | 1.2            | 0.0            | 1.1           | 0.7              | 0.0            | 0.5           |
| J0635.5–7516  | 5.6               | 0.6            | 10.7          | 1.2             | 0.1            | 13.4          | 1.6           | 0.2            | 10.4          | 2.0            | 0.0            | 2.6           | 0.8              | 0.0            | 0.4           |
| J0636.0+0554  | 5.0               | 0.0            | 2.8           | 2.1             | 0.3            | 9.2           | 1.7           | 0.4            | 4.5           | 1.9            | 0.0            | 0.3           | 0.6              | 0.0            | 0.0           |
| J0637.0+0416c | 3.1               | 0.0            | 1.6           | 1.0             | 0.2            | 4.4           | 2.0           | 0.4            | 5.0           | 3.3            | 1.2            | 3.5           | 0.6              | 0.0            | 0.0           |
| J0637.8+0737  | 3.2               | 1.0            | 5.2           | 1.1             | 0.2            | 6.2           | 1.1           | 0.3            | 3.5           | 2.9            | 0.0            | 1.6           | 0.6              | 0.0            | 0.0           |
| J0641.1+1006c | 4.2               | 1.0            | 6.9           | 1.2             | 0.2            | 7.7           | 1.7           | 0.4            | 5.2           | 3.7            | 0.0            | 1.9           | 1.6              | 0.0            | 2.7           |
| J0641.2+7315  | 2.0               | 0.0            | 2.5           | 0.5             | 0.1            | 7.3           | 0.4           | 0.0            | 1.1           | 2.1            | 0.0            | 3.0           | 1.3              | 0.0            | 3.7           |
| J0642.9+0319  | 3.0               | 0.7            | 5.3           | 1.1             | 0.2            | 5.9           | 1.0           | 0.3            | 3.2           | 4.0            | 0.0            | 2.3           | 0.9              | 0.0            | 0.1           |
| J0643.2+0858  | 4.2               | 1.1            | 6.2           | 1.5             | 0.2            | 10.1          | 3.3           | 0.4            | 9.8           | 4.1            | 1.1            | 5.8           | 1.0              | 0.0            | 0.9           |
| J0644.2–6713  | 3.0               | 0.5            | 6.8           | 0.8             | 0.1            | 11.3          | 1.7           | 0.2            | 12.0          | 5.4            | 1.0            | 10.2          | 1.7              | 0.0            | 4.1           |
| J0644.6+6034  | 1.6               | 0.0            | 2.6           | 0.2             | 0.1            | 4.2           | 0.6           | 0.2            | 5.0           | 1.8            | 0.6            | 4.9           | 0.8              | 0.3            | 5.0           |
| J0647.7+0032  | 2.3               | 0.5            | 4.8           | 1.3             | 0.2            | 8.1           | 1.1           | 0.4            | 3.3           | 2.6            | 0.0            | 0.9           | 1.7              | 0.0            | 2.5           |
| J0647.7–5132  | 1.3               | 0.0            | 1.6           | 0.2             | 0.0            | 1.4           | 0.4           | 0.0            | 1.2           | 2.0            | 0.0            | 2.8           | 1.6              | 0.0            | 4.0           |
| J0647.8–6102  | 1.8               | 0.0            | 2.0           | 0.3             | 0.1            | 4.3           | 0.8           | 0.0            | 3.1           | 1.6            | 0.6            | 3.9           | 1.4              | 0.0            | 3.1           |
| J0648.7–1739  | 2.4               | 0.9            | 3.9           | 0.4             | 0.1            | 3.6           | 1.1           | 0.3            | 4.7           | 2.2            | 0.8            | 3.9           | 1.2              | 0.0            | 2.3           |
| J0648.9+1516  | 2.4               | 0.6            | 4.0           | 0.3             | 0.0            | 1.4           | 0.7           | 0.2            | 5.0           | 5.7            | 1.1            | 9.4           | 2.2              | 0.6            | 8.1           |
| J0649.7–3138  | 1.3               | 0.0            | 1.1           | 0.2             | 0.0            | 0.7           | 0.4           | 0.2            | 3.2           | 1.6            | 0.7            | 3.5           | 0.9              | 0.4            | 4.8           |
| J0650.4–1632  | 1.8               | 0.0            | 0.0           | 0.6             | 0.1            | 4.6           | 0.9           | 0.3            | 3.9           | 2.2            | 0.0            | 1.2           | 1.0              | 0.0            | 0.2           |
| J0650.7+2505  | 1.4               | 0.0            | 1.3           | 0.3             | 0.0            | 2.4           | 0.9           | 0.2            | 6.6           | 5.6            | 1.1            | 9.5           | 3.6              | 0.8            | 12.3          |
| J0653.7+2818  | 0.6               | 0.0            | 0.0           | 0.2             | 0.0            | 1.7           | 0.3           | 0.1            | 3.3           | 2.2            | 0.7            | 5.1           | 0.8              | 0.0            | 0.9           |
| J0654.2+4514  | 4.1               | 0.4            | 9.8           | 1.3             | 0.1            | 16.4          | 2.9           | 0.3            | 16.6          | 5.9            | 1.0            | 10.8          | 0.7              | 0.3            | 4.8           |
| J0654.5+5043  | 1.5               | 0.4            | 4.0           | 0.8             | 0.1            | 11.3          | 2.3           | 0.2            | 15.7          | 6.5            | 1.0            | 12.2          | 1.3              | 0.4            | 6.3           |
| J0656.2–0320  | 5.4               | 0.8            | 7.3           | 1.9             | 0.2            | 11.1          | 2.9           | 0.4            | 8.5           | 6.0            | 1.3            | 6.6           | 0.7              | 0.0            | 0.0           |
| J0658.4+0633  | 1.9               | 0.0            | 1.0           | 0.6             | 0.0            | 3.0           | 0.8           | 0.0            | 1.9           | 2.0            | 0.8            | 3.9           | 0.7              | 0.0            | 1.4           |
| J0659.7+1417  | 5.4               | 0.6            | 10.6          | 1.0             | 0.1            | 10.8          | 0.8           | 0.2            | 4.6           | 0.9            | 0.0            | 0.0           | 0.8              | 0.0            | 1.8           |
| J0700.3+1710  | 2.2               | 0.6            | 3.8           | 0.4             | 0.1            | 4.8           | 0.6           | 0.0            | 2.2           | 2.0            | 0.0            | 1.9           | 0.9              | 0.0            | 1.2           |
| J0700.3–6611  | 1.9               | 0.5            | 4.5           | 1.0             | 0.1            | 13.7          | 3.1           | 0.3            | 17.9          | 8.5            | 1.2            | 14.6          | 2.5              | 0.6            | 9.5           |
| J0701.7–4630  | 2.4               | 0.4            | 6.6           | 0.6             | 0.1            | 8.1           | 1.5           | 0.2            | 9.4           | 3.0            | 0.0            | 3.1           | 0.5              | 0.0            | 0.0           |
| J0702.7–1951  | 0.8               | 0.0            | 0.0           | 0.2             | 0.0            | 0.0           | 1.3           | 0.3            | 5.8           | 3.0            | 1.0            | 4.3           | 1.2              | 0.0            | 2.0           |
| J0703.1–3912  | 0.7               | 0.0            | 0.0           | 0.3             | 0.0            | 1.3           | 0.8           | 0.0            | 3.1           | 1.3            | 0.6            | 3.4           | 0.9              | 0.0            | 0.8           |
| J0705.3–1043c | 2.2               | 0.0            | 0.0           | 0.8             | 0.2            | 3.9           | 1.8           | 0.0            | 2.7           | 3.8            | 0.0            | 1.8           | 1.3              | 0.0            | 0.5           |
| J0706.5+3744  | 0.9               | 0.0            | 0.5           | 0.2             | 0.0            | 1.8           | 0.7           | 0.2            | 6.0           | 2.6            | 0.8            | 5.5           | 1.6              | 0.5            | 7.3           |
| J0706.5+7741  | 0.9               | 0.0            | 0.6           | 0.2             | 0.1            | 4.6           | 1.0           | 0.2            | 8.7           | 2.7            | 0.7            | 7.8           | 0.9              | 0.0            | 2.4           |
| J0706.7–4845  | 1.4               | 0.0            | 0.7           | 0.5             | 0.1            | 6.1           | 0.7           | 0.2            | 5.1           | 1.7            | 0.7            | 3.7           | 0.8              | 0.0            | 0.4           |
| J0708.5–1020c | 3.9               | 0.0            | 2.9           | 0.8             | 0.2            | 4.3           | 1.3           | 0.4            | 3.5           | 2.2            | 0.0            | 0.5           | 1.0              | 0.0            | 0.5           |
| J0709.0+2236  | 1.5               | 0.5            | 3.4           | 0.3             | 0.0            | 1.9           | 0.6           | 0.2            | 4.7           | 1.9            | 0.0            | 2.1           | 0.7              | 0.0            | 0.0           |
| J0709.3–0256  | 3.0               | 0.6            | 5.7           | 1.0             | 0.1            | 8.2           | 0.8           | 0.3            | 3.6           | 2.0            | 0.8            | 3.5           | 0.6              | 0.0            | 0.0           |
| J0710.5+5908  | 1.3               | 0.0            | 2.3           | 0.2             | 0.0            | 1.7           | 0.5           | 0.1            | 5.1           | 1.7            | 0.6            | 5.3           | 2.1              | 0.5            | 10.1          |
| J0710.8+4733  | 2.2               | 0.5            | 5.2           | 0.5             | 0.1            | 6.6           | 0.8           | 0.2            | 6.3           | 2.2            | 0.0            | 2.2           | 0.4              | 0.0            | 0.0           |
| J0712.9+5032  | 1.0               | 0.0            | 0.5           | 0.5             | 0.1            | 8.5           | 1.2           | 0.2            | 8.7           | 3.6            | 0.8            | 7.9           | 1.1              | 0.4            | 5.0           |
| J0713.5–0952  | 3.0               | 0.9            | 4.7           | 0.9             | 0.2            | 5.4           | 1.5           | 0.4            | 4.7           | 1.9            | 0.0            | 0.5           | 0.7              | 0.0            | 0.5           |
| J0714.0+1933  | 4.4               | 0.5            | 10.8          | 1.8             | 0.1            | 22.0          | 4.2           | 0.3            | 21.3          | 7.5            | 1.2            | 11.9          | 0.9              | 0.4            | 4.8           |
| J0718.7–4320  | 1.3               | 0.0            | 0.9           | 0.5             | 0.1            | 6.5           | 1.6           | 0.2            | 9.6           | 5.9            | 1.1            | 10.1          | 2.7              | 0.7            | 10.2          |
| J0719.2–5000  | 2.0               | 0.0            | 2.0           | 0.3             | 0.1            | 3.3           | 0.9           | 0.0            | 3.1           | 1.9            | 0.7            | 4.4           | 0.6              | 0.0            | 0.0           |

Table 1—Continued

|               | 100 MeV – 300 MeV |                |               | 300 MeV – 1 GeV |                |               | 1 GeV – 3 GeV |                |               | 3 GeV – 10 GeV |                |               | 10 GeV – 100 GeV |                |               |
|---------------|-------------------|----------------|---------------|-----------------|----------------|---------------|---------------|----------------|---------------|----------------|----------------|---------------|------------------|----------------|---------------|
| Name 2FGL     | $F_1^a$           | $\Delta F_1^a$ | $\sqrt{TS_1}$ | $F_2^a$         | $\Delta F_2^a$ | $\sqrt{TS_2}$ | $F_3^b$       | $\Delta F_3^b$ | $\sqrt{TS_3}$ | $F_4^c$        | $\Delta F_4^c$ | $\sqrt{TS_4}$ | $F_5^c$          | $\Delta F_5^c$ | $\sqrt{TS_5}$ |
| J0719.3+3306  | 4.9               | 0.4            | 13.9          | 2.0             | 0.1            | 27.3          | 6.6           | 0.4            | 32.2          | 15.1           | 1.6            | 21.2          | 3.3              | 0.7            | 11.8          |
| J0721.2–0223  | 1.1               | 0.0            | 0.0           | 0.2             | 0.0            | 0.1           | 0.6           | 0.0            | 1.4           | 2.4            | 0.0            | 2.5           | 1.0              | 0.5            | 4.7           |
| J0721.5+0404c | 2.7               | 0.0            | 3.1           | 0.5             | 0.0            | 3.1           | 0.6           | 0.2            | 3.3           | 0.8            | 0.0            | 0.0           | 0.8              | 0.0            | 1.6           |
| J0721.9+7120  | 13.5              | 0.4            | 38.5          | 4.8             | 0.1            | 65.5          | 13.6          | 0.5            | 64.2          | 43.7           | 2.3            | 48.3          | 8.5              | 1.0            | 22.2          |
| J0723.9+2901  | 1.7               | 0.4            | 3.9           | 0.3             | 0.1            | 5.1           | 0.4           | 0.1            | 3.7           | 1.4            | 0.6            | 3.9           | 1.1              | 0.0            | 1.2           |
| J0725.3+1426  | 9.2               | 0.5            | 20.3          | 2.9             | 0.1            | 32.2          | 7.4           | 0.4            | 32.5          | 18.0           | 1.8            | 22.6          | 3.0              | 0.7            | 9.8           |
| J0725.6+2159  | 2.1               | 0.5            | 4.6           | 0.4             | 0.1            | 4.9           | 0.6           | 0.0            | 3.0           | 0.9            | 0.0            | 0.0           | 1.6              | 0.0            | 3.7           |
| J0725.8–0549  | 1.3               | 0.0            | 0.5           | 0.3             | 0.0            | 1.2           | 0.6           | 0.0            | 1.5           | 1.4            | 0.7            | 3.3           | 1.5              | 0.0            | 3.5           |
| J0726.0–0053  | 1.7               | 0.6            | 3.4           | 0.4             | 0.1            | 4.2           | 0.7           | 0.2            | 5.2           | 1.9            | 0.7            | 4.3           | 1.6              | 0.0            | 3.5           |
| J0727.0–4726  | 1.9               | 0.5            | 3.6           | 0.5             | 0.1            | 5.1           | 1.0           | 0.2            | 5.2           | 2.6            | 0.0            | 2.0           | 0.9              | 0.0            | 1.1           |
| J0729.9+3304  | 0.7               | 0.0            | 0.0           | 0.3             | 0.0            | 2.2           | 0.4           | 0.1            | 3.3           | 1.7            | 0.0            | 1.4           | 0.8              | 0.4            | 4.8           |
| J0730.2–1141  | 27.6              | 0.8            | 39.7          | 8.6             | 0.2            | 56.1          | 18.0          | 0.7            | 48.6          | 32.7           | 2.5            | 29.1          | 5.8              | 1.0            | 14.0          |
| J0730.6–6607  | 0.9               | 0.0            | 0.5           | 0.2             | 0.0            | 1.3           | 0.2           | 0.0            | 0.0           | 1.4            | 0.6            | 3.8           | 0.9              | 0.4            | 4.8           |
| J0733.9+5023  | 1.6               | 0.0            | 2.2           | 0.4             | 0.1            | 5.9           | 0.6           | 0.1            | 5.2           | 2.2            | 0.0            | 3.1           | 0.5              | 0.0            | 0.0           |
| J0734.2–7706  | 2.2               | 0.0            | 2.1           | 0.6             | 0.1            | 6.7           | 0.9           | 0.2            | 5.0           | 2.6            | 0.0            | 2.0           | 0.9              | 0.0            | 2.4           |
| J0734.6–1558  | 6.9               | 0.7            | 10.1          | 2.5             | 0.2            | 16.7          | 4.7           | 0.4            | 14.8          | 6.2            | 1.3            | 7.4           | 0.9              | 0.0            | 0.1           |
| J0737.1–3235  | 3.7               | 0.0            | 2.8           | 0.5             | 0.1            | 3.8           | 1.5           | 0.3            | 5.6           | 4.0            | 0.0            | 2.6           | 0.9              | 0.0            | 0.0           |
| J0737.5–8246  | 0.5               | 0.0            | 0.0           | 0.2             | 0.0            | 1.4           | 0.2           | 0.0            | 0.0           | 2.2            | 0.0            | 2.1           | 1.0              | 0.4            | 5.2           |
| J0738.0+1742  | 3.4               | 0.4            | 8.4           | 1.4             | 0.1            | 18.4          | 3.3           | 0.3            | 19.6          | 13.3           | 1.5            | 18.6          | 3.9              | 0.8            | 12.6          |
| J0739.2+0138  | 5.6               | 0.5            | 12.7          | 1.5             | 0.1            | 17.0          | 1.8           | 0.2            | 10.9          | 4.1            | 0.9            | 7.9           | 0.9              | 0.0            | 1.8           |
| J0742.4–2821  | 1.7               | 0.0            | 0.2           | 0.7             | 0.2            | 4.8           | 1.2           | 0.3            | 4.2           | 4.2            | 0.0            | 2.4           | 1.0              | 0.0            | 0.1           |
| J0742.6+5442  | 3.9               | 0.5            | 10.6          | 0.9             | 0.1            | 14.4          | 2.5           | 0.2            | 17.0          | 3.6            | 0.8            | 7.9           | 0.8              | 0.0            | 0.0           |
| J0742.7–3113  | 3.1               | 0.0            | 1.6           | 0.6             | 0.1            | 4.1           | 1.2           | 0.0            | 2.8           | 3.6            | 0.0            | 2.6           | 1.8              | 0.0            | 2.6           |
| J0744.1–2523  | 2.0               | 0.5            | 3.9           | 1.1             | 0.2            | 8.2           | 2.3           | 0.4            | 7.4           | 4.4            | 1.2            | 5.1           | 0.6              | 0.0            | 0.0           |
| J0745.0+7436  | 1.2               | 0.0            | 2.0           | 0.2             | 0.1            | 3.9           | 0.3           | 0.1            | 3.3           | 2.0            | 0.6            | 5.5           | 0.9              | 0.4            | 4.9           |
| J0745.5+7910  | 0.8               | 0.0            | 0.3           | 0.2             | 0.1            | 4.0           | 0.3           | 0.1            | 3.6           | 1.8            | 0.0            | 2.6           | 0.5              | 0.0            | 1.4           |
| J0745.9+8512  | 0.4               | 0.0            | 0.0           | 0.1             | 0.0            | 0.0           | 0.5           | 0.0            | 2.0           | 1.1            | 0.5            | 3.7           | 1.0              | 0.0            | 3.6           |
| J0746.0–0222  | 1.0               | 0.0            | 0.6           | 0.1             | 0.0            | 0.6           | 0.7           | 0.0            | 3.0           | 2.4            | 0.7            | 5.7           | 1.1              | 0.5            | 5.2           |
| J0746.5–0713  | 0.9               | 0.0            | 0.0           | 0.3             | 0.0            | 1.9           | 0.4           | 0.2            | 3.2           | 2.2            | 0.8            | 4.5           | 0.9              | 0.0            | 1.4           |
| J0746.5–4758  | 1.7               | 0.0            | 1.1           | 0.3             | 0.0            | 1.4           | 0.6           | 0.2            | 3.5           | 2.3            | 0.0            | 2.1           | 0.9              | 0.4            | 4.0           |
| J0746.6+2549  | 3.2               | 0.5            | 7.0           | 0.5             | 0.1            | 6.3           | 0.4           | 0.2            | 3.4           | 2.6            | 0.0            | 3.1           | 0.5              | 0.0            | 0.0           |
| J0747.2–1654  | 2.8               | 0.0            | 1.6           | 0.5             | 0.1            | 4.5           | 0.7           | 0.2            | 3.6           | 1.5            | 0.0            | 0.0           | 0.5              | 0.0            | 0.0           |
| J0747.5–3305  | 1.6               | 0.0            | 1.2           | 0.9             | 0.2            | 6.2           | 2.5           | 0.4            | 6.4           | 4.2            | 0.0            | 1.9           | 0.8              | 0.0            | 0.0           |
| J0747.7+4501  | 0.9               | 0.0            | 0.3           | 0.2             | 0.1            | 4.1           | 0.6           | 0.0            | 2.4           | 1.5            | 0.6            | 3.4           | 0.5              | 0.0            | 0.0           |
| J0748.5–2204  | 2.5               | 0.7            | 3.6           | 0.7             | 0.0            | 3.1           | 1.3           | 0.0            | 2.5           | 2.5            | 0.0            | 1.2           | 1.1              | 0.0            | 1.3           |
| J0750.6+1230  | 3.3               | 0.5            | 7.4           | 0.7             | 0.1            | 9.4           | 1.0           | 0.2            | 7.3           | 2.8            | 0.8            | 6.5           | 0.9              | 0.0            | 1.7           |
| J0751.1+1809  | 1.0               | 0.0            | 0.9           | 0.4             | 0.1            | 7.4           | 2.0           | 0.2            | 13.1          | 5.2            | 1.0            | 10.0          | 0.5              | 0.0            | 0.0           |
| J0753.0+5352  | 1.2               | 0.0            | 1.0           | 0.4             | 0.1            | 6.7           | 0.7           | 0.2            | 6.7           | 2.3            | 0.7            | 5.8           | 1.1              | 0.4            | 6.0           |
| J0753.2–1634  | 3.0               | 0.0            | 2.6           | 0.2             | 0.0            | 0.3           | 0.5           | 0.2            | 3.5           | 2.7            | 0.0            | 2.3           | 1.0              | 0.0            | 2.4           |
| J0753.2+1937  | 2.9               | 0.6            | 6.0           | 0.4             | 0.0            | 2.7           | 0.4           | 0.0            | 1.3           | 0.8            | 0.0            | 0.0           | 1.0              | 0.0            | 2.8           |
| J0754.4–1147  | 1.6               | 0.0            | 1.2           | 0.3             | 0.1            | 4.0           | 1.0           | 0.2            | 6.0           | 3.5            | 0.9            | 6.2           | 0.9              | 0.4            | 4.2           |
| J0754.8+4824  | 1.5               | 0.4            | 4.1           | 0.3             | 0.1            | 5.4           | 0.8           | 0.2            | 6.7           | 2.9            | 0.7            | 7.3           | 1.1              | 0.0            | 3.3           |
| J0756.3–6433  | 0.6               | 0.0            | 0.0           | 0.4             | 0.0            | 2.7           | 0.5           | 0.0            | 1.1           | 1.3            | 0.0            | 1.3           | 1.5              | 0.0            | 4.3           |
| J0757.1+0957  | 2.6               | 0.4            | 6.3           | 0.7             | 0.1            | 11.3          | 1.3           | 0.2            | 9.5           | 3.6            | 0.9            | 8.0           | 1.0              | 0.5            | 5.1           |

Table 1—Continued

|               | 100 MeV – 300 MeV |                |               | 300 MeV – 1 GeV |                |               | 1 GeV – 3 GeV |                |               | 3 GeV – 10 GeV |                |               | 10 GeV – 100 GeV |                |               |
|---------------|-------------------|----------------|---------------|-----------------|----------------|---------------|---------------|----------------|---------------|----------------|----------------|---------------|------------------|----------------|---------------|
| Name 2FGL     | $F_1^a$           | $\Delta F_1^a$ | $\sqrt{TS_1}$ | $F_2^a$         | $\Delta F_2^a$ | $\sqrt{TS_2}$ | $F_3^b$       | $\Delta F_3^b$ | $\sqrt{TS_3}$ | $F_4^c$        | $\Delta F_4^c$ | $\sqrt{TS_4}$ | $F_5^c$          | $\Delta F_5^c$ | $\sqrt{TS_5}$ |
| J0758.0–2615c | 2.8               | 0.0            | 2.2           | 0.6             | 0.1            | 4.9           | 1.0           | 0.3            | 4.3           | 2.9            | 0.0            | 1.7           | 0.7              | 0.0            | 1.1           |
| J0758.8–1448  | 1.7               | 0.0            | 1.1           | 0.4             | 0.0            | 2.8           | 0.8           | 0.2            | 5.2           | 2.4            | 0.0            | 2.3           | 0.9              | 0.0            | 1.5           |
| J0801.5+4401  | 1.1               | 0.0            | 0.9           | 0.2             | 0.1            | 3.9           | 0.6           | 0.2            | 5.4           | 1.8            | 0.0            | 2.2           | 0.6              | 0.0            | 0.0           |
| J0802.6–0940  | 1.4               | 0.0            | 0.8           | 0.4             | 0.0            | 2.5           | 0.7           | 0.0            | 2.0           | 2.5            | 0.0            | 3.2           | 1.4              | 0.0            | 3.6           |
| J0802.7–5615  | 1.7               | 0.0            | 1.1           | 0.4             | 0.0            | 2.3           | 0.7           | 0.2            | 4.0           | 1.6            | 0.7            | 3.3           | 0.5              | 0.0            | 0.0           |
| J0803.2–0339  | 1.9               | 0.0            | 2.5           | 0.2             | 0.1            | 3.7           | 0.8           | 0.2            | 6.5           | 3.3            | 0.8            | 7.2           | 0.9              | 0.4            | 4.5           |
| J0805.2–0121  | 0.5               | 0.0            | 0.0           | 0.2             | 0.1            | 3.8           | 0.5           | 0.0            | 2.6           | 1.5            | 0.7            | 3.8           | 0.6              | 0.0            | 0.0           |
| J0805.3+7535  | 0.5               | 0.0            | 0.0           | 0.2             | 0.0            | 4.0           | 0.8           | 0.1            | 8.3           | 4.5            | 0.8            | 10.6          | 2.4              | 0.6            | 10.2          |
| J0805.5+6145  | 3.7               | 0.4            | 9.5           | 0.8             | 0.1            | 13.0          | 0.8           | 0.2            | 6.8           | 1.7            | 0.0            | 2.1           | 0.4              | 0.0            | 0.0           |
| J0807.0–6511  | 0.6               | 0.0            | 0.0           | 0.2             | 0.0            | 0.7           | 0.2           | 0.0            | 0.0           | 1.4            | 0.0            | 0.5           | 0.8              | 0.4            | 4.5           |
| J0807.1–0543  | 2.3               | 0.0            | 2.3           | 0.4             | 0.1            | 4.6           | 0.7           | 0.2            | 5.3           | 4.4            | 1.0            | 8.6           | 1.6              | 0.0            | 3.6           |
| J0808.2–0750  | 9.7               | 0.6            | 21.7          | 3.6             | 0.1            | 36.2          | 11.4          | 0.5            | 42.6          | 32.9           | 2.4            | 32.2          | 7.4              | 1.1            | 17.6          |
| J0809.8+5218  | 1.8               | 0.4            | 5.3           | 0.4             | 0.1            | 7.6           | 1.8           | 0.2            | 14.2          | 5.3            | 1.0            | 11.1          | 2.6              | 0.6            | 11.1          |
| J0811.1–7527  | 1.4               | 0.0            | 1.1           | 0.4             | 0.1            | 5.6           | 1.6           | 0.2            | 10.0          | 7.9            | 1.2            | 12.9          | 3.5              | 0.7            | 11.5          |
| J0811.4+0149  | 1.6               | 0.4            | 4.0           | 0.5             | 0.1            | 7.4           | 0.9           | 0.2            | 7.8           | 1.9            | 0.7            | 4.4           | 1.5              | 0.0            | 4.2           |
| J0812.6+6511  | 1.5               | 0.0            | 0.0           | 0.3             | 0.0            | 1.7           | 0.6           | 0.0            | 3.1           | 1.6            | 0.0            | 2.5           | 0.8              | 0.0            | 1.6           |
| J0814.0–1006  | 3.3               | 0.0            | 3.5           | 0.3             | 0.1            | 3.9           | 1.0           | 0.2            | 5.8           | 2.0            | 0.8            | 3.8           | 1.7              | 0.0            | 2.8           |
| J0814.7+6429  | 3.5               | 0.0            | 2.6           | 0.4             | 0.1            | 5.7           | 1.0           | 0.2            | 8.4           | 3.0            | 0.7            | 8.4           | 0.7              | 0.0            | 1.7           |
| J0816.4–1311  | 2.0               | 0.0            | 2.8           | 0.5             | 0.1            | 6.8           | 1.4           | 0.2            | 9.0           | 9.3            | 1.4            | 14.6          | 3.3              | 0.8            | 10.7          |
| J0816.5+5739  | 1.6               | 0.0            | 2.5           | 0.3             | 0.0            | 3.0           | 0.7           | 0.2            | 6.5           | 2.9            | 0.7            | 7.2           | 1.3              | 0.0            | 3.9           |
| J0816.7–2420  | 2.6               | 0.0            | 3.0           | 0.5             | 0.1            | 5.3           | 0.7           | 0.2            | 4.2           | 1.5            | 0.6            | 4.1           | 1.1              | 0.0            | 1.5           |
| J0816.9+2049  | 2.1               | 0.4            | 4.9           | 0.3             | 0.1            | 4.0           | 0.6           | 0.0            | 2.3           | 2.0            | 0.0            | 3.1           | 0.7              | 0.0            | 0.0           |
| J0817.9+3238  | 0.7               | 0.0            | 0.0           | 0.2             | 0.1            | 3.6           | 0.6           | 0.0            | 2.3           | 1.2            | 0.5            | 3.5           | 0.9              | 0.0            | 2.8           |
| J0818.2–0935  | 2.1               | 0.0            | 0.8           | 0.4             | 0.1            | 5.8           | 1.2           | 0.2            | 7.7           | 3.1            | 0.9            | 5.4           | 1.0              | 0.4            | 4.9           |
| J0818.2+4223  | 6.0               | 0.5            | 15.8          | 2.0             | 0.1            | 27.6          | 6.2           | 0.4            | 32.4          | 15.4           | 1.6            | 21.3          | 2.3              | 0.6            | 9.5           |
| J0819.3+2750  | 1.8               | 0.0            | 2.8           | 0.2             | 0.0            | 2.2           | 0.5           | 0.0            | 2.4           | 1.0            | 0.5            | 3.7           | 0.6              | 0.0            | 0.0           |
| J0819.6–0803  | 1.4               | 0.0            | 1.0           | 0.1             | 0.0            | 0.0           | 0.6           | 0.0            | 2.6           | 2.1            | 0.0            | 1.9           | 1.6              | 0.0            | 4.2           |
| J0821.0–4254  | 2.2               | 0.0            | 0.0           | 1.9             | 0.0            | 2.5           | 1.5           | 0.5            | 3.6           | 6.1            | 0.0            | 2.9           | 1.8              | 0.0            | 1.9           |
| J0823.0–4246  | 4.2               | 1.1            | 3.3           | 1.9             | 0.0            | 1.4           | 3.7           | 0.7            | 5.9           | 10.3           | 2.1            | 6.5           | 2.4              | 0.0            | 2.4           |
| J0823.0+4041  | 1.6               | 0.7            | 4.0           | 0.3             | 0.0            | 3.0           | 0.8           | 0.2            | 6.8           | 1.2            | 0.0            | 0.5           | 0.9              | 0.0            | 2.3           |
| J0823.4–4305  | 2.4               | 0.0            | 0.0           | 2.4             | 0.0            | 2.6           | 1.1           | 0.0            | 0.3           | 6.5            | 1.7            | 5.0           | 1.5              | 0.7            | 3.8           |
| J0824.7+3914  | 1.4               | 0.6            | 3.4           | 0.3             | 0.0            | 2.6           | 0.6           | 0.2            | 4.8           | 1.4            | 0.0            | 1.7           | 0.5              | 0.0            | 0.0           |
| J0824.9+5552  | 3.0               | 0.5            | 7.8           | 0.6             | 0.1            | 10.1          | 0.5           | 0.1            | 4.7           | 1.3            | 0.5            | 3.9           | 0.7              | 0.0            | 1.4           |
| J0825.9+0308  | 1.5               | 0.0            | 1.5           | 0.3             | 0.0            | 2.4           | 0.6           | 0.0            | 2.5           | 2.1            | 0.7            | 4.6           | 1.5              | 0.0            | 4.5           |
| J0825.9–2229  | 3.6               | 0.5            | 8.0           | 1.2             | 0.1            | 14.1          | 3.3           | 0.3            | 17.5          | 9.7            | 1.4            | 14.4          | 3.1              | 0.7            | 9.7           |
| J0825.9–3216  | 2.9               | 0.0            | 2.5           | 0.6             | 0.0            | 3.1           | 0.8           | 0.3            | 3.7           | 1.6            | 0.7            | 3.4           | 0.8              | 0.0            | 0.0           |
| J0830.5+2407  | 4.1               | 0.5            | 9.5           | 0.8             | 0.1            | 10.9          | 0.9           | 0.2            | 7.5           | 1.0            | 0.5            | 3.6           | 0.8              | 0.0            | 0.0           |
| J0831.9+0429  | 4.7               | 0.5            | 12.7          | 1.6             | 0.1            | 22.1          | 3.7           | 0.3            | 21.5          | 9.5            | 1.3            | 15.5          | 1.4              | 0.5            | 6.5           |
| J0833.1–4511e | ...               | 0.0            | 0.0           | ...             | 0.0            | 0.0           | ...           | 0.0            | 0.0           | ...            | 0.0            | 0.0           | ...              | 0.0            | 0.0           |
| J0834.3+4400  | 1.4               | 0.0            | 1.5           | 0.1             | 0.0            | 0.6           | 0.5           | 0.0            | 3.1           | 1.3            | 0.6            | 4.2           | 1.1              | 0.0            | 2.8           |
| J0834.3+4221  | 1.3               | 0.5            | 3.6           | 0.3             | 0.1            | 4.9           | 0.6           | 0.1            | 5.4           | 1.2            | 0.6            | 3.3           | 0.7              | 0.0            | 0.0           |
| J0835.3–4510  | 594.3             | 2.3            | 384.0         | 337.6           | 1.0            | 654.8         | 1096.9        | 4.5            | 591.7         | 2167.9         | 18.4           | 324.0         | 97.1             | 3.8            | 65.6          |
| J0838.8–2828  | 0.6               | 0.0            | 0.0           | 0.3             | 0.1            | 3.7           | 0.7           | 0.2            | 4.8           | 3.6            | 0.9            | 6.8           | 0.7              | 0.0            | 0.0           |
| J0839.4+1802  | 2.0               | 0.4            | 4.8           | 0.3             | 0.0            | 2.4           | 0.2           | 0.0            | 0.0           | 2.1            | 0.0            | 3.2           | 1.3              | 0.0            | 3.6           |

Table 1—Continued

|               | 100 MeV – 300 MeV |                |               | 300 MeV – 1 GeV |                |               | 1 GeV – 3 GeV |                |               | 3 GeV – 10 GeV |                |               | 10 GeV – 100 GeV |                |               |
|---------------|-------------------|----------------|---------------|-----------------|----------------|---------------|---------------|----------------|---------------|----------------|----------------|---------------|------------------|----------------|---------------|
| Name 2FGL     | $F_1^a$           | $\Delta F_1^a$ | $\sqrt{TS_1}$ | $F_2^a$         | $\Delta F_2^a$ | $\sqrt{TS_2}$ | $F_3^b$       | $\Delta F_3^b$ | $\sqrt{TS_3}$ | $F_4^c$        | $\Delta F_4^c$ | $\sqrt{TS_4}$ | $F_5^c$          | $\Delta F_5^c$ | $\sqrt{TS_5}$ |
| J0839.6+0059  | 1.5               | 0.0            | 1.7           | 0.3             | 0.1            | 4.1           | 0.7           | 0.2            | 6.1           | 1.7            | 0.6            | 4.7           | 0.7              | 0.0            | 0.0           |
| J0839.7+3541  | 1.0               | 0.0            | 0.9           | 0.2             | 0.0            | 1.1           | 0.6           | 0.0            | 3.2           | 2.6            | 0.0            | 3.0           | 1.2              | 0.0            | 2.6           |
| J0840.7+1310  | 1.6               | 0.0            | 2.0           | 0.4             | 0.1            | 5.9           | 0.5           | 0.2            | 3.7           | 2.6            | 0.0            | 3.1           | 0.6              | 0.0            | 0.0           |
| J0841.3–3556  | 1.5               | 0.0            | 0.1           | 0.2             | 0.0            | 0.0           | 1.2           | 0.3            | 5.6           | 6.5            | 1.2            | 9.4           | 2.1              | 0.6            | 7.2           |
| J0841.6+7052  | 5.2               | 0.6            | 13.5          | 0.7             | 0.1            | 12.1          | 0.6           | 0.1            | 6.1           | 1.0            | 0.4            | 3.9           | 0.4              | 0.0            | 0.0           |
| J0842.9–4721  | 5.5               | 1.2            | 5.6           | 3.0             | 0.3            | 10.1          | 1.9           | 0.0            | 2.4           | 3.2            | 0.0            | 1.7           | 1.0              | 0.0            | 1.0           |
| J0843.6+6715  | 1.1               | 0.0            | 0.3           | 0.2             | 0.0            | 2.7           | 0.4           | 0.1            | 4.6           | 2.6            | 0.6            | 7.5           | 0.4              | 0.0            | 0.0           |
| J0843.9+5312  | 1.5               | 0.0            | 2.5           | 0.2             | 0.0            | 2.5           | 0.3           | 0.1            | 3.4           | 2.0            | 0.6            | 6.2           | 0.6              | 0.0            | 1.6           |
| J0844.8–5459  | 1.7               | 0.0            | 0.7           | 0.5             | 0.1            | 4.4           | 1.2           | 0.3            | 5.8           | 4.8            | 1.1            | 7.3           | 1.2              | 0.0            | 2.0           |
| J0844.9+6214  | 1.2               | 0.0            | 1.3           | 0.3             | 0.0            | 2.9           | 0.5           | 0.0            | 2.1           | 1.7            | 0.0            | 2.0           | 0.7              | 0.0            | 1.5           |
| J0846.0+2820  | 2.0               | 0.0            | 2.8           | 0.3             | 0.0            | 1.8           | 0.4           | 0.1            | 3.4           | 1.3            | 0.0            | 1.7           | 0.8              | 0.0            | 1.9           |
| J0846.7–4053  | 5.7               | 1.2            | 5.0           | 1.2             | 0.2            | 5.2           | 1.8           | 0.0            | 2.3           | 2.1            | 0.0            | 0.0           | 1.0              | 0.5            | 3.3           |
| J0847.0–2334  | 2.2               | 0.0            | 2.7           | 0.3             | 0.1            | 4.0           | 0.6           | 0.2            | 3.9           | 2.1            | 0.8            | 4.4           | 1.2              | 0.0            | 2.3           |
| J0847.2+1134  | 0.3               | 0.0            | 0.0           | 0.2             | 0.0            | 1.0           | 0.4           | 0.1            | 3.7           | 1.7            | 0.6            | 5.0           | 1.0              | 0.4            | 5.9           |
| J0848.1–0703  | 1.1               | 0.0            | 0.1           | 0.2             | 0.0            | 2.0           | 0.5           | 0.0            | 2.0           | 2.3            | 0.0            | 2.8           | 1.5              | 0.0            | 3.4           |
| J0848.5–4535  | 7.9               | 0.0            | 2.7           | 2.5             | 0.4            | 8.2           | 3.5           | 0.6            | 6.4           | 6.4            | 0.0            | 3.1           | 1.4              | 0.0            | 0.9           |
| J0848.7–4324  | 6.9               | 1.2            | 7.6           | 4.2             | 0.3            | 13.8          | 3.0           | 0.6            | 5.9           | 2.0            | 0.0            | 0.0           | 0.8              | 0.0            | 0.0           |
| J0849.0+0455  | 0.8               | 0.0            | 0.3           | 0.2             | 0.0            | 2.3           | 0.4           | 0.0            | 1.6           | 2.3            | 0.7            | 5.4           | 1.9              | 0.0            | 3.8           |
| J0849.2+6606  | 1.8               | 0.0            | 2.6           | 0.2             | 0.0            | 1.1           | 0.6           | 0.0            | 3.1           | 1.9            | 0.6            | 5.6           | 1.0              | 0.0            | 3.1           |
| J0849.8+4852  | 1.8               | 0.4            | 5.1           | 0.6             | 0.1            | 11.1          | 1.8           | 0.2            | 14.0          | 2.3            | 0.7            | 6.1           | 1.2              | 0.0            | 2.8           |
| J0849.9–3540  | 3.2               | 0.0            | 1.9           | 0.4             | 0.1            | 3.5           | 1.3           | 0.3            | 6.1           | 4.1            | 1.0            | 6.5           | 1.8              | 0.0            | 2.6           |
| J0850.1–4846  | 4.3               | 1.3            | 5.0           | 1.2             | 0.3            | 5.0           | 1.6           | 0.0            | 2.1           | 3.4            | 0.0            | 2.1           | 1.5              | 0.0            | 2.1           |
| J0850.2–1212  | 3.9               | 0.5            | 10.4          | 1.5             | 0.1            | 19.3          | 3.5           | 0.3            | 20.4          | 8.9            | 1.3            | 14.0          | 1.2              | 0.5            | 5.4           |
| J0851.7–4635  | 25.6              | 0.0            | 0.2           | 1.4             | 0.4            | 3.9           | 1.4           | 0.0            | 1.2           | 6.0            | 0.0            | 2.5           | 1.8              | 0.7            | 4.7           |
| J0852.4–5756  | 2.0               | 0.7            | 3.5           | 0.4             | 0.1            | 4.0           | 1.2           | 0.2            | 6.2           | 2.2            | 0.8            | 3.8           | 1.5              | 0.0            | 3.0           |
| J0853.1–3659  | 2.3               | 0.0            | 0.8           | 0.2             | 0.0            | 0.0           | 0.8           | 0.2            | 3.8           | 3.0            | 0.9            | 4.6           | 1.6              | 0.0            | 2.2           |
| J0853.5–4711  | 16.7              | 0.0            | 0.3           | 1.2             | 0.0            | 1.7           | 1.2           | 0.4            | 3.3           | 5.4            | 0.0            | 2.8           | 2.3              | 0.8            | 5.5           |
| J0854.7–4501  | 4.9               | 2.4            | 4.3           | 1.2             | 0.3            | 5.1           | 5.0           | 0.6            | 10.5          | 7.7            | 1.7            | 6.5           | 2.1              | 0.0            | 2.6           |
| J0854.8+2005  | 3.5               | 0.8            | 4.5           | 1.2             | 0.1            | 14.3          | 2.4           | 0.3            | 14.8          | 8.3            | 1.2            | 14.3          | 1.0              | 0.4            | 5.6           |
| J0855.1–0712  | 2.4               | 0.0            | 2.6           | 0.2             | 0.1            | 3.2           | 0.6           | 0.0            | 2.5           | 1.3            | 0.0            | 1.3           | 0.6              | 0.0            | 0.0           |
| J0855.4–4625  | 17.1              | 0.0            | 0.5           | 1.1             | 0.0            | 1.1           | 2.1           | 0.5            | 4.8           | 5.7            | 0.0            | 2.2           | 2.1              | 0.8            | 5.0           |
| J0856.0+7136  | 1.5               | 0.0            | 1.1           | 0.2             | 0.1            | 3.5           | 0.5           | 0.1            | 5.0           | 1.0            | 0.0            | 0.8           | 0.4              | 0.0            | 0.0           |
| J0856.3+2058  | 3.2               | 0.0            | 1.9           | 0.4             | 0.0            | 2.6           | 0.8           | 0.2            | 5.8           | 2.0            | 0.0            | 2.3           | 1.3              | 0.0            | 2.6           |
| J0856.6–1105  | 1.8               | 0.5            | 4.5           | 0.7             | 0.1            | 10.9          | 1.9           | 0.2            | 13.2          | 7.9            | 1.2            | 13.2          | 1.3              | 0.5            | 6.0           |
| J0858.0–4815  | 11.8              | 0.0            | 4.2           | 2.3             | 0.3            | 9.6           | 3.7           | 0.5            | 8.0           | 3.9            | 0.0            | 1.4           | 0.9              | 0.0            | 0.3           |
| J0858.1–1952  | 2.3               | 0.0            | 2.4           | 0.4             | 0.1            | 4.3           | 0.8           | 0.2            | 4.6           | 1.3            | 0.6            | 3.2           | 1.0              | 0.0            | 1.5           |
| J0858.2–3129  | 0.7               | 0.0            | 0.0           | 0.1             | 0.0            | 0.0           | 0.7           | 0.0            | 2.1           | 2.4            | 0.0            | 3.2           | 1.0              | 0.4            | 5.0           |
| J0858.3–4333  | 6.6               | 1.2            | 8.1           | 2.7             | 0.3            | 11.4          | 3.5           | 0.6            | 7.3           | 4.4            | 0.0            | 1.8           | 0.7              | 0.0            | 0.0           |
| J0859.4–2532  | 1.7               | 0.0            | 1.5           | 0.4             | 0.0            | 2.3           | 0.8           | 0.0            | 2.6           | 1.5            | 0.0            | 0.8           | 1.0              | 0.4            | 4.3           |
| J0900.5–4441c | 3.7               | 0.0            | 0.0           | 1.2             | 0.3            | 5.1           | 1.6           | 0.5            | 3.5           | 5.5            | 0.0            | 2.5           | 1.7              | 0.0            | 1.7           |
| J0900.9+6736  | 1.9               | 0.0            | 2.8           | 0.3             | 0.1            | 4.8           | 0.4           | 0.1            | 3.6           | 0.9            | 0.4            | 3.3           | 0.6              | 0.0            | 1.0           |
| J0901.7–4655  | 5.1               | 1.8            | 3.2           | 2.0             | 0.3            | 7.9           | 3.3           | 0.5            | 7.3           | 3.5            | 1.3            | 3.6           | 1.9              | 0.0            | 1.7           |
| J0902.4+2050  | 1.3               | 0.0            | 0.5           | 0.3             | 0.0            | 2.7           | 0.8           | 0.2            | 6.8           | 2.4            | 0.7            | 5.8           | 1.3              | 0.0            | 3.4           |
| J0902.8–4741c | 4.3               | 0.0            | 0.7           | 0.5             | 0.0            | 1.0           | 3.5           | 0.5            | 7.6           | 4.7            | 0.0            | 1.9           | 1.5              | 0.0            | 1.2           |

Table 1—Continued

|               | 100 MeV – 300 MeV |                |               | 300 MeV – 1 GeV |                |               | 1 GeV – 3 GeV |                |               | 3 GeV – 10 GeV |                |               | 10 GeV – 100 GeV |                |               |
|---------------|-------------------|----------------|---------------|-----------------|----------------|---------------|---------------|----------------|---------------|----------------|----------------|---------------|------------------|----------------|---------------|
| Name 2FGL     | $F_1^a$           | $\Delta F_1^a$ | $\sqrt{TS_1}$ | $F_2^a$         | $\Delta F_2^a$ | $\sqrt{TS_2}$ | $F_3^b$       | $\Delta F_3^b$ | $\sqrt{TS_3}$ | $F_4^c$        | $\Delta F_4^c$ | $\sqrt{TS_4}$ | $F_5^c$          | $\Delta F_5^c$ | $\sqrt{TS_5}$ |
| J0903.4+4651  | 1.1               | 0.0            |               | 1.1             | 0.2            | 0.1           | 3.8           | 0.3            | 0.1           | 3.6            | 2.1            | 0.0           | 2.9              | 0.8            | 0.0           |
| J0903.6+4238  | 1.2               | 0.0            |               | 0.8             | 0.3            | 0.0           | 2.9           | 0.3            | 0.1           | 3.3            | 2.1            | 0.0           | 2.6              | 0.9            | 0.0           |
| J0904.0–4823c | 20.7              | 0.0            |               | 0.2             | 1.7            | 0.3           | 6.1           | 1.9            | 0.5           | 4.0            | 5.8            | 0.0           | 2.6              | 1.1            | 0.0           |
| J0904.8–3513  | 2.1               | 0.7            |               | 3.4             | 0.6            | 0.1           | 5.2           | 1.2            | 0.3           | 5.5            | 2.0            | 0.8           | 3.5              | 0.7            | 0.0           |
| J0904.9–5735  | 1.4               | 0.0            |               | 0.0             | 0.5            | 0.0           | 2.7           | 1.4            | 0.3           | 7.4            | 2.9            | 0.9           | 5.2              | 0.9            | 0.4           |
| J0905.6+1357  | 1.4               | 0.0            |               | 1.8             | 0.2            | 0.1           | 3.6           | 0.7            | 0.2           | 6.3            | 4.3            | 0.9           | 8.7              | 2.3            | 0.6           |
| J0906.2–0906  | 1.5               | 0.0            |               | 1.8             | 0.3            | 0.0           | 2.2           | 0.5            | 0.2           | 4.5            | 2.4            | 0.7           | 5.9              | 1.4            | 0.0           |
| J0907.9–4716c | 3.6               | 0.0            |               | 0.0             | 1.4            | 0.3           | 5.6           | 2.1            | 0.5           | 4.9            | 3.4            | 1.2           | 3.7              | 1.2            | 0.0           |
| J0908.5–4913  | 6.4               | 2.0            |               | 5.8             | 2.3            | 0.3           | 9.1           | 3.3            | 0.6           | 6.2            | 4.9            | 0.0           | 1.7              | 1.1            | 0.0           |
| J0908.7–2119  | 2.0               | 0.0            |               | 0.7             | 0.3            | 0.1           | 3.9           | 0.8            | 0.0           | 2.6            | 1.5            | 0.0           | 0.6              | 1.3            | 0.0           |
| J0909.1+0121  | 6.3               | 1.2            |               | 5.5             | 1.9            | 0.2           | 13.6          | 2.6            | 0.3           | 12.5           | 5.8            | 1.1           | 10.1             | 0.6            | 0.0           |
| J0909.2+2308  | 1.5               | 0.0            |               | 0.0             | 0.3            | 0.1           | 3.6           | 0.5            | 0.0           | 1.4            | 2.8            | 0.8           | 6.1              | 1.6            | 0.6           |
| J0909.6+0158  | 5.3               | 0.0            |               | 2.1             | 0.6            | 0.0           | 2.2           | 0.7            | 0.2           | 4.0            | 1.8            | 0.7           | 3.9              | 0.5            | 0.0           |
| J0909.7–0229  | 1.7               | 0.4            |               | 4.3             | 0.8            | 0.1           | 12.3          | 1.6            | 0.2           | 11.2           | 3.8            | 0.9           | 8.5              | 0.9            | 0.0           |
| J0910.4–5050  | 6.4               | 1.4            |               | 5.8             | 2.2            | 0.3           | 9.1           | 2.9            | 0.5           | 6.2            | 3.8            | 0.0           | 1.5              | 1.7            | 0.0           |
| J0910.6+3329  | 1.3               | 0.0            |               | 1.8             | 0.3            | 0.1           | 5.5           | 0.5            | 0.1           | 4.6            | 2.9            | 0.8           | 7.1              | 1.2            | 0.4           |
| J0910.9+2246  | 2.4               | 0.0            |               | 1.6             | 0.5            | 0.0           | 2.5           | 1.1            | 0.2           | 7.5            | 2.2            | 0.7           | 5.0              | 1.0            | 0.0           |
| J0912.1+4126  | 1.2               | 0.5            |               | 3.3             | 0.2            | 0.1           | 3.7           | 0.3            | 0.1           | 3.6            | 1.5            | 0.0           | 2.3              | 1.5            | 0.0           |
| J0912.5+2758  | 1.1               | 0.0            |               | 1.8             | 0.1            | 0.0           | 0.5           | 0.4            | 0.0           | 2.2            | 0.8            | 0.0           | 0.0              | 0.9            | 0.4           |
| J0912.9–2102  | 2.4               | 0.0            |               | 1.7             | 0.2            | 0.0           | 0.5           | 0.8            | 0.2           | 5.6            | 1.9            | 0.7           | 4.1              | 1.5            | 0.0           |
| J0913.0+1553  | 1.5               | 0.5            |               | 4.0             | 0.2            | 0.0           | 1.1           | 0.4            | 0.1           | 3.5            | 0.9            | 0.0           | 0.0              | 1.6            | 0.0           |
| J0914.1–4756  | 5.6               | 1.1            |               | 6.9             | 2.5            | 0.3           | 10.4          | 2.0            | 0.5           | 4.1            | 5.8            | 0.0           | 2.9              | 0.6            | 0.0           |
| J0915.8+2932  | 0.7               | 0.0            |               | 0.0             | 0.4            | 0.1           | 7.8           | 1.6            | 0.2           | 12.4           | 5.0            | 0.9           | 11.8             | 1.8            | 0.6           |
| J0917.0+3900  | 1.6               | 0.0            |               | 2.1             | 0.2            | 0.1           | 4.4           | 0.4            | 0.1           | 3.8            | 1.2            | 0.0           | 1.7              | 0.8            | 0.0           |
| J0919.3–2203  | 1.7               | 0.0            |               | 1.5             | 0.2            | 0.0           | 1.5           | 0.6            | 0.0           | 1.9            | 1.8            | 0.7           | 4.2              | 0.8            | 0.0           |
| J0920.9+4441  | 10.8              | 0.4            |               | 30.9            | 3.6            | 0.1           | 49.8          | 7.3            | 0.4           | 38.7           | 14.9           | 1.5           | 23.1             | 1.5            | 0.5           |
| J0921.9+2335  | 0.9               | 0.0            |               | 0.7             | 0.2            | 0.0           | 0.9           | 0.5            | 0.0           | 2.8            | 1.8            | 0.6           | 4.9              | 1.2            | 0.0           |
| J0921.9+6216  | 2.1               | 0.4            |               | 6.0             | 0.4            | 0.1           | 7.1           | 0.8            | 0.2           | 7.3            | 0.9            | 0.5           | 3.2              | 1.0            | 0.0           |
| J0922.2–5214c | 2.5               | 0.6            |               | 4.3             | 1.8            | 0.2           | 8.6           | 1.9            | 0.0           | 2.8            | 2.4            | 0.0           | 0.2              | 1.1            | 0.0           |
| J0922.7+0435  | 1.5               | 0.0            |               | 1.6             | 0.2            | 0.1           | 3.4           | 0.4            | 0.1           | 4.0            | 2.0            | 0.0           | 2.5              | 1.3            | 0.0           |
| J0923.2+4125  | 1.6               | 0.5            |               | 4.3             | 0.4            | 0.1           | 6.6           | 1.0            | 0.2           | 8.3            | 1.8            | 0.6           | 5.2              | 0.8            | 0.0           |
| J0923.5+1508  | 1.3               | 0.0            |               | 1.0             | 0.3            | 0.0           | 2.7           | 0.5            | 0.0           | 1.5            | 1.3            | 0.6           | 3.8              | 0.6            | 0.0           |
| J0924.0+2819  | 2.7               | 0.4            |               | 6.9             | 0.4            | 0.1           | 5.8           | 0.5            | 0.1           | 4.5            | 2.1            | 0.0           | 2.8              | 0.9            | 0.0           |
| J0927.9–2041  | 1.7               | 0.5            |               | 3.8             | 0.4            | 0.1           | 5.2           | 0.6            | 0.2           | 4.3            | 1.5            | 0.0           | 0.8              | 0.6            | 0.0           |
| J0928.8–3530  | 0.8               | 0.0            |               | 0.0             | 0.2            | 0.0           | 0.0           | 0.9            | 0.0           | 3.0            | 1.9            | 0.7           | 4.0              | 0.6            | 0.0           |
| J0929.5+5009  | 1.2               | 0.0            |               | 1.0             | 0.3            | 0.0           | 3.0           | 0.6            | 0.1           | 6.2            | 2.0            | 0.0           | 2.6              | 1.0            | 0.4           |
| J0930.4+8611  | 1.0               | 0.0            |               | 0.8             | 0.3            | 0.1           | 5.2           | 0.9            | 0.2           | 7.5            | 1.6            | 0.6           | 4.0              | 0.6            | 0.3           |
| J0934.0–6231  | 0.9               | 0.0            |               | 0.5             | 0.3            | 0.0           | 2.6           | 1.9            | 0.3           | 9.4            | 5.4            | 1.1           | 8.1              | 1.3            | 0.0           |
| J0934.7+3932  | 1.4               | 0.0            |               | 1.7             | 0.2            | 0.1           | 3.9           | 0.5            | 0.0           | 2.7            | 1.9            | 0.0           | 1.9              | 0.7            | 0.0           |
| J0937.6+5009  | 1.7               | 0.5            |               | 4.7             | 0.2            | 0.1           | 4.7           | 0.4            | 0.1           | 4.5            | 1.6            | 0.0           | 2.2              | 0.7            | 0.0           |
| J0937.9–1434  | 0.7               | 0.0            |               | 0.0             | 0.3            | 0.0           | 2.8           | 0.4            | 0.1           | 3.9            | 2.2            | 0.0           | 2.9              | 0.9            | 0.0           |
| J0939.1–1734  | 1.9               | 0.0            |               | 2.8             | 0.4            | 0.1           | 5.1           | 0.9            | 0.2           | 6.5            | 2.1            | 0.8           | 4.6              | 0.8            | 0.0           |
| J0940.3–2827  | 2.0               | 0.0            |               | 2.5             | 0.3            | 0.1           | 3.8           | 0.7            | 0.2           | 4.5            | 3.0            | 0.0           | 3.1              | 0.5            | 0.0           |
| J0940.8–6105  | 1.7               | 0.0            |               | 0.2             | 0.5            | 0.0           | 2.3           | 0.9            | 0.3           | 3.9            | 2.6            | 0.0           | 2.4              | 1.0            | 0.0           |

Table 1—Continued

|               | 100 MeV – 300 MeV |                |               | 300 MeV – 1 GeV |                |               | 1 GeV – 3 GeV |                |               | 3 GeV – 10 GeV |                |               | 10 GeV – 100 GeV |                |               |
|---------------|-------------------|----------------|---------------|-----------------|----------------|---------------|---------------|----------------|---------------|----------------|----------------|---------------|------------------|----------------|---------------|
| Name 2FGL     | $F_1^a$           | $\Delta F_1^a$ | $\sqrt{TS_1}$ | $F_2^a$         | $\Delta F_2^a$ | $\sqrt{TS_2}$ | $F_3^b$       | $\Delta F_3^b$ | $\sqrt{TS_3}$ | $F_4^c$        | $\Delta F_4^c$ | $\sqrt{TS_4}$ | $F_5^c$          | $\Delta F_5^c$ | $\sqrt{TS_5}$ |
| J0941.4+2724  | 1.2               | 0.0            | 1.3           | 0.2             | 0.1            | 4.2           | 0.4           | 0.1            | 4.6           | 1.9            | 0.0            | 2.8           | 0.7              | 0.0            | 1.6           |
| J0941.4+6148  | 0.9               | 0.0            | 0.7           | 0.2             | 0.0            | 2.5           | 0.5           | 0.1            | 5.4           | 1.3            | 0.5            | 4.4           | 0.7              | 0.0            | 1.2           |
| J0941.9–0755  | 0.4               | 0.0            | 0.0           | 0.2             | 0.0            | 2.4           | 0.4           | 0.1            | 3.6           | 1.3            | 0.6            | 3.6           | 0.8              | 0.0            | 1.8           |
| J0942.8–7558  | 2.4               | 0.0            | 1.3           | 0.4             | 0.1            | 4.2           | 0.8           | 0.2            | 4.5           | 1.3            | 0.0            | 0.0           | 0.6              | 0.0            | 0.0           |
| J0945.9+5751  | 1.1               | 0.0            | 1.3           | 0.2             | 0.0            | 3.5           | 0.5           | 0.1            | 5.6           | 1.2            | 0.5            | 3.9           | 0.9              | 0.0            | 2.5           |
| J0946.2+0104  | 1.7               | 0.0            | 0.5           | 0.2             | 0.0            | 0.2           | 0.4           | 0.0            | 0.7           | 1.9            | 0.0            | 2.2           | 0.9              | 0.4            | 4.6           |
| J0946.5+1015  | 2.2               | 0.4            | 5.2           | 0.5             | 0.1            | 7.9           | 0.9           | 0.2            | 7.6           | 2.0            | 0.0            | 2.2           | 0.6              | 0.0            | 0.0           |
| J0946.9–2541  | 0.9               | 0.0            | 0.1           | 0.3             | 0.0            | 1.9           | 0.6           | 0.2            | 4.6           | 2.9            | 0.0            | 3.0           | 0.8              | 0.0            | 0.6           |
| J0948.8+4040  | 1.3               | 0.4            | 3.6           | 0.2             | 0.1            | 3.9           | 0.3           | 0.1            | 3.5           | 0.9            | 0.5            | 3.4           | 0.6              | 0.0            | 0.0           |
| J0948.8+0020  | 6.6               | 0.8            | 8.6           | 1.8             | 0.1            | 17.4          | 2.2           | 0.3            | 12.3          | 2.7            | 0.8            | 5.2           | 0.7              | 0.0            | 0.0           |
| J0950.1+4554  | 0.5               | 0.0            | 0.0           | 0.1             | 0.0            | 0.9           | 0.3           | 0.1            | 3.8           | 2.1            | 0.0            | 3.1           | 1.7              | 0.0            | 4.1           |
| J0952.7–3717  | 1.8               | 0.6            | 3.5           | 0.3             | 0.1            | 3.7           | 0.7           | 0.0            | 2.0           | 2.6            | 0.0            | 3.0           | 0.7              | 0.0            | 0.0           |
| J0953.1–0839  | 1.1               | 0.0            | 1.2           | 0.3             | 0.1            | 4.1           | 1.9           | 0.2            | 13.0          | 6.0            | 1.1            | 11.3          | 2.5              | 0.7            | 9.7           |
| J0953.6–1504  | 0.7               | 0.0            | 0.0           | 0.2             | 0.1            | 3.7           | 0.9           | 0.2            | 6.8           | 2.0            | 0.7            | 4.1           | 0.7              | 0.0            | 0.0           |
| J0953.9–7659  | 2.8               | 0.0            | 2.2           | 0.5             | 0.0            | 2.8           | 0.8           | 0.0            | 1.6           | 3.1            | 0.0            | 3.0           | 1.4              | 0.0            | 3.4           |
| J0955.0–3949  | 1.9               | 0.6            | 3.6           | 0.6             | 0.1            | 6.6           | 1.4           | 0.3            | 7.4           | 2.4            | 0.8            | 4.6           | 0.8              | 0.0            | 0.1           |
| J0955.9+6936  | 1.7               | 0.3            | 5.2           | 0.3             | 0.1            | 5.7           | 1.1           | 0.2            | 9.3           | 1.4            | 0.5            | 4.4           | 0.8              | 0.0            | 2.3           |
| J0956.9+2516  | 1.7               | 0.4            | 4.5           | 0.6             | 0.1            | 9.8           | 1.0           | 0.2            | 8.3           | 2.1            | 0.7            | 4.8           | 0.5              | 0.0            | 0.0           |
| J0957.6–1350  | 1.5               | 0.4            | 3.5           | 0.4             | 0.1            | 5.7           | 0.5           | 0.2            | 3.5           | 1.9            | 0.0            | 2.1           | 0.6              | 0.0            | 0.0           |
| J0957.7+5522  | 5.0               | 0.4            | 16.8          | 2.3             | 0.1            | 39.6          | 8.1           | 0.4            | 45.4          | 26.1           | 1.9            | 34.5          | 6.9              | 1.0            | 20.4          |
| J0957.7+4735  | 1.0               | 0.0            | 0.9           | 0.2             | 0.1            | 4.2           | 0.4           | 0.1            | 4.2           | 0.9            | 0.0            | 0.9           | 0.5              | 0.0            | 0.0           |
| J0958.6+6533  | 2.4               | 0.4            | 6.6           | 0.6             | 0.1            | 9.9           | 1.2           | 0.2            | 9.7           | 2.1            | 0.6            | 5.6           | 1.3              | 0.0            | 3.2           |
| J0958.6–2446  | 1.9               | 0.0            | 2.3           | 0.3             | 0.0            | 2.9           | 0.5           | 0.0            | 1.7           | 2.5            | 0.0            | 2.4           | 1.2              | 0.0            | 2.7           |
| J1001.0+2913  | 1.5               | 0.4            | 4.2           | 0.4             | 0.1            | 7.6           | 0.5           | 0.1            | 5.4           | 2.3            | 0.7            | 6.5           | 1.0              | 0.4            | 4.1           |
| J1003.0+2219  | 0.9               | 0.0            | 0.4           | 0.3             | 0.1            | 4.3           | 0.5           | 0.0            | 2.9           | 2.3            | 0.0            | 2.8           | 0.6              | 0.0            | 0.0           |
| J1007.1–2157  | 3.1               | 0.5            | 7.1           | 0.5             | 0.1            | 6.4           | 0.5           | 0.2            | 3.6           | 1.4            | 0.6            | 3.7           | 1.3              | 0.0            | 2.0           |
| J1007.7+0621  | 1.3               | 0.0            | 0.0           | 0.4             | 0.1            | 6.7           | 0.8           | 0.2            | 7.0           | 1.5            | 0.6            | 4.0           | 1.0              | 0.0            | 2.3           |
| J1008.6+0028  | 1.6               | 0.0            | 2.2           | 0.2             | 0.0            | 1.2           | 0.5           | 0.2            | 4.1           | 1.7            | 0.0            | 1.7           | 1.1              | 0.0            | 2.1           |
| J1009.7–3123  | 2.4               | 0.0            | 2.8           | 0.3             | 0.1            | 4.3           | 0.8           | 0.0            | 2.9           | 2.4            | 0.8            | 4.5           | 0.9              | 0.0            | 0.4           |
| J1010.7–5643c | 5.1               | 0.0            | 2.9           | 2.4             | 0.3            | 8.5           | 2.9           | 0.6            | 5.1           | 2.7            | 0.0            | 0.0           | 0.8              | 0.0            | 0.0           |
| J1010.8–0158  | 0.7               | 0.0            | 0.0           | 0.3             | 0.0            | 2.1           | 0.5           | 0.2            | 4.2           | 1.5            | 0.6            | 4.3           | 0.8              | 0.0            | 1.5           |
| J1012.1–4236  | 2.2               | 0.0            | 1.5           | 0.2             | 0.0            | 0.1           | 0.6           | 0.2            | 4.3           | 1.8            | 0.7            | 3.6           | 0.6              | 0.0            | 0.0           |
| J1012.1+0631  | 2.8               | 0.6            | 6.6           | 0.3             | 0.0            | 2.7           | 0.4           | 0.1            | 3.8           | 1.8            | 0.6            | 5.3           | 1.3              | 0.0            | 2.7           |
| J1012.5+4227  | 1.0               | 0.0            | 1.3           | 0.2             | 0.0            | 1.9           | 0.3           | 0.1            | 3.4           | 2.2            | 0.0            | 3.0           | 1.1              | 0.0            | 2.6           |
| J1012.6+2440  | 3.9               | 0.5            | 11.8          | 1.5             | 0.1            | 21.7          | 3.7           | 0.3            | 22.1          | 6.4            | 1.1            | 11.4          | 0.9              | 0.0            | 2.5           |
| J1013.6+3434  | 1.7               | 0.0            | 2.0           | 0.2             | 0.0            | 1.7           | 0.3           | 0.1            | 3.4           | 1.1            | 0.5            | 3.7           | 0.7              | 0.0            | 0.5           |
| J1014.1+2306  | 2.1               | 0.0            | 2.3           | 0.3             | 0.1            | 4.5           | 0.5           | 0.1            | 4.1           | 0.9            | 0.0            | 0.2           | 0.7              | 0.0            | 1.0           |
| J1015.1+4925  | 2.5               | 0.3            | 9.3           | 1.2             | 0.1            | 22.6          | 5.5           | 0.3            | 33.4          | 18.4           | 1.7            | 27.6          | 7.1              | 1.0            | 19.5          |
| J1016.0+0513  | 3.1               | 0.0            | 0.9           | 1.3             | 0.1            | 11.9          | 2.9           | 0.3            | 15.0          | 10.2           | 1.4            | 15.2          | 2.9              | 0.7            | 10.4          |
| J1016.1+5600  | 1.8               | 0.0            | 2.6           | 0.3             | 0.0            | 3.1           | 0.4           | 0.1            | 4.0           | 0.8            | 0.0            | 0.5           | 0.4              | 0.0            | 0.0           |
| J1016.2–0638  | 2.0               | 0.0            | 2.2           | 0.2             | 0.1            | 3.2           | 0.5           | 0.2            | 4.6           | 1.0            | 0.0            | 0.0           | 0.6              | 0.0            | 0.0           |
| J1016.4–4244  | 1.4               | 0.0            | 0.0           | 0.3             | 0.0            | 1.8           | 0.7           | 0.0            | 2.2           | 2.1            | 0.8            | 4.3           | 1.4              | 0.0            | 2.7           |
| J1016.5–5858  | 15.5              | 0.0            | 1.8           | 2.9             | 0.0            | 2.1           | 6.7           | 1.0            | 7.5           | 12.3           | 2.4            | 6.7           | 2.9              | 0.0            | 2.6           |
| J1017.0+3531  | 2.1               | 0.0            | 2.0           | 0.3             | 0.1            | 4.4           | 0.3           | 0.0            | 0.9           | 1.1            | 0.0            | 0.0           | 0.5              | 0.0            | 0.0           |



Table 1—Continued

|               | 100 MeV – 300 MeV |                |               | 300 MeV – 1 GeV |                |               | 1 GeV – 3 GeV |                |               | 3 GeV – 10 GeV |                |               | 10 GeV – 100 GeV |                |               |
|---------------|-------------------|----------------|---------------|-----------------|----------------|---------------|---------------|----------------|---------------|----------------|----------------|---------------|------------------|----------------|---------------|
| Name 2FGL     | $F_1^a$           | $\Delta F_1^a$ | $\sqrt{TS_1}$ | $F_2^a$         | $\Delta F_2^a$ | $\sqrt{TS_2}$ | $F_3^b$       | $\Delta F_3^b$ | $\sqrt{TS_3}$ | $F_4^c$        | $\Delta F_4^c$ | $\sqrt{TS_4}$ | $F_5^c$          | $\Delta F_5^c$ | $\sqrt{TS_5}$ |
| J1018.3–3119  | 2.5               | 0.7            | 5.3           | 0.3             | 0.1            | 3.5           | 0.5           | 0.2            | 3.8           | 1.6            | 0.0            | 1.2           | 0.5              | 0.0            | 0.0           |
| J1018.6+0531  | 3.9               | 1.1            | 3.5           | 0.6             | 0.0            | 2.8           | 0.7           | 0.2            | 4.0           | 2.7            | 0.0            | 2.6           | 1.0              | 0.0            | 1.7           |
| J1019.0+5915  | 0.6               | 0.0            | 0.0           | 0.2             | 0.0            | 2.2           | 0.4           | 0.1            | 4.5           | 1.6            | 0.0            | 3.0           | 0.6              | 0.0            | 0.7           |
| J1019.0–5856  | 27.1              | 2.2            | 8.5           | 12.2            | 0.8            | 17.4          | 21.2          | 1.2            | 20.7          | 28.7           | 3.0            | 13.7          | 2.0              | 0.7            | 4.6           |
| J1019.8+6322  | 0.5               | 0.0            | 0.0           | 0.1             | 0.0            | 3.3           | 0.4           | 0.1            | 4.5           | 1.3            | 0.0            | 1.6           | 0.5              | 0.0            | 0.2           |
| J1020.0–6029  | 2.2               | 0.0            | 0.7           | 1.2             | 0.2            | 6.1           | 1.5           | 0.0            | 1.9           | 1.4            | 0.0            | 0.0           | 0.6              | 0.0            | 0.0           |
| J1021.6+8021  | 1.0               | 0.0            | 0.0           | 0.2             | 0.1            | 4.7           | 0.3           | 0.1            | 3.4           | 1.0            | 0.4            | 4.3           | 0.4              | 0.0            | 0.0           |
| J1022.7–5741  | 37.4              | 0.0            | 1.6           | 7.7             | 1.4            | 5.8           | 10.3          | 1.8            | 5.8           | 13.7           | 3.1            | 5.0           | 3.5              | 0.0            | 3.1           |
| J1023.1–0115  | 0.8               | 0.0            | 0.0           | 0.2             | 0.0            | 1.6           | 0.6           | 0.2            | 5.0           | 2.3            | 0.7            | 5.8           | 1.1              | 0.0            | 2.5           |
| J1023.5–5749c | 33.0              | 0.0            | 0.6           | 4.7             | 0.0            | 0.9           | 11.3          | 1.8            | 6.6           | 21.4           | 3.4            | 8.2           | 3.5              | 0.0            | 2.8           |
| J1023.6+2959  | 0.6               | 0.0            | 0.1           | 0.2             | 0.0            | 1.3           | 0.2           | 0.0            | 0.1           | 1.1            | 0.0            | 0.7           | 1.6              | 0.0            | 4.7           |
| J1023.6+3947  | 1.7               | 0.0            | 2.3           | 0.3             | 0.1            | 5.8           | 0.6           | 0.1            | 6.5           | 1.6            | 0.0            | 2.3           | 0.7              | 0.0            | 1.5           |
| J1023.6+0040  | 1.2               | 0.0            | 3.1           | 0.4             | 0.1            | 5.2           | 0.5           | 0.0            | 2.3           | 1.3            | 0.0            | 1.3           | 0.5              | 0.0            | 0.0           |
| J1023.8–3248  | 2.2               | 0.0            | 2.0           | 0.3             | 0.1            | 4.2           | 0.5           | 0.0            | 1.5           | 1.0            | 0.0            | 0.0           | 1.0              | 0.0            | 2.2           |
| J1023.8–4335  | 0.9               | 0.0            | 0.1           | 0.3             | 0.1            | 3.9           | 0.8           | 0.2            | 5.6           | 3.5            | 0.9            | 6.2           | 2.2              | 0.6            | 7.8           |
| J1024.6–0719  | 1.7               | 0.0            | 1.8           | 0.1             | 0.0            | 0.2           | 0.7           | 0.2            | 5.3           | 2.4            | 0.0            | 2.9           | 0.5              | 0.0            | 0.0           |
| J1026.3–8546  | 1.5               | 0.0            | 1.3           | 0.3             | 0.1            | 3.5           | 0.7           | 0.0            | 2.9           | 2.7            | 0.9            | 5.2           | 1.0              | 0.4            | 4.7           |
| J1026.7–1749  | 0.9               | 0.0            | 0.1           | 0.4             | 0.0            | 3.0           | 0.6           | 0.0            | 2.3           | 3.1            | 0.8            | 6.7           | 1.1              | 0.0            | 2.0           |
| J1027.4–5730c | 11.0              | 0.0            | 2.1           | 3.2             | 0.5            | 7.2           | 5.9           | 0.8            | 8.0           | 7.1            | 0.0            | 2.6           | 1.9              | 0.0            | 1.6           |
| J1028.5–5819  | 17.3              | 5.5            | 5.8           | 8.6             | 0.5            | 21.6          | 26.6          | 1.0            | 36.7          | 52.3           | 3.4            | 26.0          | 4.7              | 1.0            | 9.3           |
| J1029.5–2022  | 1.4               | 0.0            | 1.4           | 0.2             | 0.0            | 1.6           | 0.5           | 0.0            | 2.0           | 1.4            | 0.6            | 3.7           | 1.1              | 0.0            | 2.0           |
| J1029.9+7437  | 1.2               | 0.4            | 3.6           | 0.3             | 0.1            | 6.0           | 0.5           | 0.1            | 4.3           | 2.3            | 0.0            | 3.1           | 1.0              | 0.0            | 2.7           |
| J1030.4–6015  | 4.3               | 1.1            | 5.4           | 1.5             | 0.3            | 6.1           | 1.9           | 0.0            | 2.4           | 1.8            | 0.0            | 0.0           | 0.9              | 0.0            | 0.6           |
| J1031.0+5053  | 0.6               | 0.0            | 0.0           | 0.2             | 0.1            | 5.2           | 0.7           | 0.1            | 8.0           | 3.2            | 0.7            | 8.6           | 1.1              | 0.4            | 6.9           |
| J1032.6+3733  | 1.7               | 0.0            | 2.6           | 0.3             | 0.1            | 6.2           | 0.7           | 0.1            | 6.9           | 1.9            | 0.6            | 5.3           | 1.3              | 0.0            | 1.7           |
| J1032.9–8401  | 1.0               | 0.0            | 0.0           | 0.4             | 0.1            | 4.5           | 0.6           | 0.0            | 1.5           | 1.9            | 0.0            | 1.5           | 1.5              | 0.0            | 2.8           |
| J1033.2+4117  | 2.2               | 0.4            | 6.2           | 0.6             | 0.1            | 10.4          | 0.8           | 0.2            | 7.5           | 1.9            | 0.6            | 5.9           | 0.9              | 0.0            | 3.2           |
| J1033.5–5032  | 0.5               | 0.0            | 0.0           | 0.2             | 0.0            | 0.4           | 0.9           | 0.0            | 3.0           | 1.9            | 0.8            | 3.7           | 1.7              | 0.0            | 3.8           |
| J1033.9+6050  | 4.7               | 0.4            | 14.2          | 1.6             | 0.1            | 27.2          | 3.6           | 0.3            | 26.0          | 8.0            | 1.1            | 16.2          | 0.8              | 0.3            | 5.0           |
| J1036.1–6722  | 0.9               | 0.0            | 0.6           | 0.6             | 0.1            | 7.0           | 3.2           | 0.3            | 14.0          | 4.7            | 1.1            | 7.0           | 0.6              | 0.0            | 0.0           |
| J1036.4–5828c | 9.5               | 0.0            | 0.0           | 2.5             | 0.0            | 2.8           | 3.0           | 0.7            | 4.8           | 4.5            | 0.0            | 1.4           | 2.6              | 0.0            | 2.9           |
| J1037.5–2820  | 3.7               | 0.6            | 7.8           | 0.6             | 0.1            | 7.7           | 1.1           | 0.2            | 7.2           | 1.0            | 0.0            | 0.1           | 1.2              | 0.0            | 2.7           |
| J1037.6+5712  | 1.3               | 0.0            | 2.2           | 0.6             | 0.1            | 13.5          | 1.7           | 0.2            | 15.1          | 8.7            | 1.2            | 16.9          | 2.8              | 0.6            | 11.2          |
| J1038.2–2423  | 1.6               | 0.0            | 1.8           | 0.3             | 0.1            | 3.9           | 0.5           | 0.2            | 3.8           | 1.4            | 0.0            | 0.8           | 1.3              | 0.0            | 2.6           |
| J1038.6–5850c | 18.0              | 0.0            | 1.1           | 1.8             | 0.0            | 1.5           | 2.7           | 0.7            | 4.3           | 4.9            | 1.5            | 4.3           | 2.9              | 0.0            | 2.9           |
| J1040.7+0614  | 3.4               | 0.5            | 7.7           | 0.5             | 0.1            | 7.1           | 0.9           | 0.2            | 7.1           | 2.7            | 0.8            | 6.2           | 0.7              | 0.0            | 0.0           |
| J1042.6+8053  | 3.2               | 0.0            | 1.9           | 0.4             | 0.0            | 2.6           | 0.6           | 0.1            | 5.2           | 1.1            | 0.0            | 1.2           | 0.4              | 0.0            | 0.0           |
| J1043.1+2404  | 1.4               | 0.0            | 2.0           | 0.3             | 0.1            | 5.7           | 0.6           | 0.1            | 5.4           | 2.4            | 0.7            | 5.8           | 1.5              | 0.0            | 3.4           |
| J1044.5–5737  | 21.2              | 2.2            | 19.7          | 6.7             | 0.3            | 28.9          | 14.4          | 0.7            | 28.3          | 20.8           | 2.2            | 15.6          | 1.4              | 0.0            | 1.8           |
| J1045.0–5941  | 17.0              | 4.9            | 5.1           | 8.1             | 0.6            | 16.2          | 16.5          | 1.0            | 21.4          | 35.8           | 3.0            | 18.8          | 6.7              | 1.2            | 9.8           |
| J1045.5–2931  | 2.3               | 0.5            | 5.0           | 0.4             | 0.1            | 5.5           | 0.5           | 0.2            | 4.1           | 2.2            | 0.7            | 5.4           | 0.7              | 0.0            | 0.3           |
| J1046.8–6005c | 6.9               | 0.0            | 0.0           | 1.4             | 0.0            | 0.8           | 2.9           | 0.7            | 4.3           | 6.0            | 1.8            | 4.2           | 2.9              | 0.0            | 2.8           |
| J1047.7–6216  | 5.2               | 1.2            | 5.9           | 1.9             | 0.2            | 10.2          | 2.4           | 0.4            | 6.6           | 4.9            | 1.2            | 5.7           | 1.3              | 0.0            | 2.4           |
| J1048.2–5831  | 13.2              | 3.6            | 7.3           | 7.5             | 0.4            | 25.9          | 23.8          | 0.9            | 40.6          | 41.4           | 2.9            | 26.1          | 2.5              | 0.7            | 6.2           |

Table 1—Continued

|               | 100 MeV – 300 MeV |                |               | 300 MeV – 1 GeV |                |               | 1 GeV – 3 GeV |                |               | 3 GeV – 10 GeV |                |               | 10 GeV – 100 GeV |                |               |
|---------------|-------------------|----------------|---------------|-----------------|----------------|---------------|---------------|----------------|---------------|----------------|----------------|---------------|------------------|----------------|---------------|
| Name 2FGL     | $F_1^a$           | $\Delta F_1^a$ | $\sqrt{TS_1}$ | $F_2^a$         | $\Delta F_2^a$ | $\sqrt{TS_2}$ | $F_3^b$       | $\Delta F_3^b$ | $\sqrt{TS_3}$ | $F_4^c$        | $\Delta F_4^c$ | $\sqrt{TS_4}$ | $F_5^c$          | $\Delta F_5^c$ | $\sqrt{TS_5}$ |
| J1048.3+7144  | 3.9               | 0.8            | 5.8           | 0.9             | 0.1            | 11.8          | 2.3           | 0.2            | 17.1          | 3.4            | 0.7            | 8.7           | 0.7              | 0.3            | 4.4           |
| J1048.6+2336  | 1.2               | 0.0            | 0.0           | 0.2             | 0.1            | 3.5           | 0.5           | 0.2            | 4.7           | 1.8            | 0.0            | 2.1           | 0.7              | 0.0            | 1.3           |
| J1049.4+1551  | 1.0               | 0.0            | 0.8           | 0.2             | 0.0            | 1.5           | 0.4           | 0.0            | 1.3           | 1.3            | 0.5            | 4.7           | 0.7              | 0.0            | 2.0           |
| J1049.7+7240  | 2.6               | 0.0            | 1.5           | 0.3             | 0.1            | 3.6           | 0.6           | 0.0            | 2.9           | 1.7            | 0.6            | 4.9           | 0.4              | 0.0            | 0.0           |
| J1050.3–5922c | 7.6               | 0.0            | 0.5           | 1.2             | 0.0            | 1.2           | 4.1           | 0.7            | 6.6           | 4.9            | 1.7            | 3.6           | 0.8              | 0.0            | 0.0           |
| J1051.3+3938  | 0.4               | 0.0            | 0.0           | 0.1             | 0.0            | 0.2           | 0.5           | 0.0            | 3.0           | 1.9            | 0.0            | 2.6           | 0.7              | 0.4            | 4.3           |
| J1051.8+0107  | 1.6               | 0.0            | 1.2           | 0.3             | 0.0            | 2.1           | 0.6           | 0.0            | 2.8           | 1.9            | 0.7            | 4.4           | 0.8              | 0.0            | 1.1           |
| J1053.6+4928  | 1.4               | 0.0            | 2.9           | 0.1             | 0.0            | 3.3           | 0.4           | 0.1            | 5.2           | 3.4            | 0.8            | 8.7           | 1.1              | 0.4            | 6.7           |
| J1054.5+2212  | 2.5               | 0.4            | 7.0           | 0.4             | 0.1            | 7.5           | 1.2           | 0.2            | 9.9           | 3.2            | 0.8            | 8.3           | 1.4              | 0.5            | 7.1           |
| J1056.0–5853  | 5.0               | 0.0            | 1.0           | 2.4             | 0.3            | 9.1           | 3.4           | 0.6            | 6.8           | 5.9            | 0.0            | 2.9           | 1.0              | 0.0            | 0.4           |
| J1056.2–6021  | 7.3               | 0.0            | 1.7           | 2.0             | 0.3            | 8.1           | 4.7           | 0.7            | 8.2           | 9.7            | 2.1            | 5.8           | 1.2              | 0.0            | 0.0           |
| J1057.0–8004  | 1.9               | 0.5            | 4.3           | 1.2             | 0.1            | 13.5          | 2.2           | 0.3            | 11.8          | 3.8            | 0.9            | 6.5           | 0.9              | 0.0            | 1.2           |
| J1057.1+7001  | 1.8               | 0.5            | 4.9           | 0.5             | 0.1            | 8.4           | 0.6           | 0.1            | 5.9           | 0.7            | 0.0            | 0.4           | 0.4              | 0.0            | 0.0           |
| J1057.9–5226  | 14.8              | 0.7            | 28.0          | 11.7            | 0.2            | 81.6          | 43.9          | 1.0            | 93.0          | 49.5           | 2.9            | 38.7          | 1.4              | 0.0            | 2.7           |
| J1058.4+0133  | 5.1               | 1.1            | 5.2           | 1.7             | 0.1            | 16.2          | 4.1           | 0.3            | 20.2          | 9.2            | 1.3            | 14.0          | 2.5              | 0.7            | 8.7           |
| J1058.6+5628  | 2.8               | 0.3            | 9.5           | 1.0             | 0.1            | 19.4          | 3.1           | 0.2            | 24.9          | 12.0           | 1.3            | 21.3          | 4.7              | 0.8            | 16.1          |
| J1058.7–6621  | 2.7               | 0.8            | 3.9           | 0.5             | 0.0            | 2.0           | 0.8           | 0.3            | 3.2           | 2.3            | 0.8            | 3.9           | 1.0              | 0.0            | 1.7           |
| J1059.0+0222  | 3.7               | 0.0            | 1.7           | 0.4             | 0.0            | 1.5           | 0.6           | 0.2            | 3.7           | 2.2            | 0.0            | 2.5           | 1.1              | 0.0            | 2.3           |
| J1059.3–6118c | 10.8              | 0.0            | 2.2           | 1.9             | 0.4            | 5.9           | 2.2           | 0.5            | 4.5           | 3.9            | 0.0            | 0.9           | 2.2              | 0.0            | 2.3           |
| J1059.3–1132  | 2.0               | 0.4            | 5.1           | 0.7             | 0.1            | 10.1          | 1.6           | 0.2            | 10.9          | 5.6            | 1.1            | 10.5          | 1.8              | 0.0            | 3.9           |
| J1059.4+8113  | 2.8               | 0.9            | 3.3           | 0.5             | 0.1            | 6.5           | 0.5           | 0.1            | 4.9           | 1.0            | 0.4            | 3.7           | 0.7              | 0.0            | 2.0           |
| J1059.9–2051  | 1.6               | 0.4            | 3.9           | 0.2             | 0.0            | 0.9           | 0.4           | 0.2            | 3.8           | 1.5            | 0.0            | 1.1           | 1.1              | 0.0            | 2.4           |
| J1100.9+4014  | 0.3               | 0.0            | 0.0           | 0.3             | 0.0            | 3.1           | 0.3           | 0.1            | 3.8           | 2.2            | 0.0            | 3.2           | 1.4              | 0.5            | 6.5           |
| J1102.1–6308c | 9.4               | 1.4            | 8.6           | 1.4             | 0.2            | 6.7           | 1.5           | 0.0            | 2.4           | 3.4            | 0.0            | 1.7           | 0.7              | 0.0            | 0.0           |
| J1103.4–2330  | 0.6               | 0.0            | 0.0           | 0.3             | 0.0            | 2.6           | 0.4           | 0.0            | 1.6           | 2.6            | 0.0            | 3.1           | 1.7              | 0.0            | 4.1           |
| J1103.9–5356  | 3.5               | 1.0            | 4.9           | 1.4             | 0.2            | 10.9          | 3.4           | 0.4            | 13.1          | 9.0            | 1.4            | 11.8          | 2.4              | 0.7            | 7.3           |
| J1104.3+0729  | 1.9               | 0.0            | 2.7           | 0.3             | 0.1            | 4.8           | 0.5           | 0.2            | 4.4           | 2.7            | 0.0            | 2.9           | 1.8              | 0.0            | 4.0           |
| J1104.4+3812  | 10.0              | 0.4            | 28.8          | 4.5             | 0.1            | 59.0          | 17.6          | 0.6            | 71.2          | 81.1           | 3.5            | 65.7          | 42.3             | 2.5            | 55.3          |
| J1104.7–6036  | 12.4              | 3.2            | 5.2           | 2.5             | 0.4            | 7.1           | 7.1           | 0.7            | 11.7          | 13.4           | 2.1            | 9.0           | 1.7              | 0.0            | 1.8           |
| J1105.4–7622  | 2.1               | 0.6            | 3.6           | 0.5             | 0.0            | 2.5           | 0.9           | 0.0            | 2.1           | 1.9            | 0.8            | 3.5           | 0.7              | 0.0            | 1.4           |
| J1105.6–6114  | 8.9               | 0.0            | 1.4           | 2.0             | 0.5            | 4.6           | 4.5           | 0.7            | 7.1           | 4.7            | 1.7            | 3.3           | 1.3              | 0.0            | 1.6           |
| J1106.1+2814  | 1.4               | 0.4            | 3.7           | 0.3             | 0.1            | 5.1           | 0.8           | 0.2            | 7.6           | 1.7            | 0.6            | 4.9           | 0.7              | 0.0            | 0.1           |
| J1106.3–3643  | 2.1               | 0.0            | 2.7           | 0.4             | 0.0            | 2.8           | 0.4           | 0.2            | 3.2           | 1.6            | 0.7            | 3.6           | 1.3              | 0.0            | 2.9           |
| J1107.2–4448  | 3.6               | 0.6            | 6.5           | 0.6             | 0.1            | 6.8           | 0.7           | 0.2            | 4.7           | 2.2            | 0.0            | 1.8           | 0.7              | 0.0            | 0.0           |
| J1107.5+0223  | 1.8               | 0.0            | 2.1           | 0.3             | 0.0            | 2.8           | 0.5           | 0.2            | 3.9           | 2.2            | 0.0            | 2.4           | 1.6              | 0.0            | 4.1           |
| J1107.8+1505  | 1.1               | 0.0            | 1.1           | 0.1             | 0.0            | 0.7           | 0.6           | 0.0            | 3.1           | 2.5            | 0.7            | 7.3           | 0.8              | 0.0            | 0.7           |
| J1109.3+2414  | 0.7               | 0.0            | 0.3           | 0.2             | 0.0            | 1.5           | 0.3           | 0.0            | 1.4           | 1.8            | 0.0            | 2.1           | 0.7              | 0.4            | 4.7           |
| J1110.1–1835  | 0.7               | 0.0            | 0.0           | 0.2             | 0.1            | 3.3           | 0.7           | 0.2            | 5.6           | 1.9            | 0.7            | 4.9           | 1.3              | 0.0            | 2.4           |
| J1110.2+7134  | 1.1               | 0.0            | 0.6           | 0.2             | 0.0            | 1.6           | 0.3           | 0.1            | 3.2           | 1.5            | 0.0            | 3.3           | 0.8              | 0.0            | 2.5           |
| J1112.1–6040  | 4.2               | 0.0            | 0.0           | 2.1             | 0.4            | 5.5           | 8.8           | 0.8            | 13.0          | 30.8           | 2.9            | 16.6          | 1.7              | 0.7            | 4.1           |
| J1112.4+3450  | 2.3               | 0.4            | 6.1           | 0.8             | 0.1            | 12.0          | 1.4           | 0.2            | 11.7          | 3.3            | 0.8            | 7.2           | 1.0              | 0.0            | 1.9           |
| J1112.5–6105  | 6.1               | 0.0            | 0.0           | 2.6             | 0.6            | 4.7           | 5.6           | 0.8            | 7.8           | 7.3            | 2.2            | 3.9           | 2.8              | 0.8            | 6.1           |
| J1115.0–0701  | 0.7               | 0.0            | 0.0           | 0.2             | 0.0            | 1.5           | 0.3           | 0.0            | 0.9           | 1.6            | 0.0            | 1.2           | 1.6              | 0.0            | 4.8           |
| J1117.2–4844  | 2.8               | 0.6            | 5.0           | 0.3             | 0.1            | 3.4           | 0.6           | 0.2            | 3.8           | 2.9            | 0.0            | 2.3           | 0.7              | 0.0            | 0.5           |

Table 1—Continued

|               | 100 MeV – 300 MeV |                |               | 300 MeV – 1 GeV |                |               | 1 GeV – 3 GeV |                |               | 3 GeV – 10 GeV |                |               | 10 GeV – 100 GeV |                |               |
|---------------|-------------------|----------------|---------------|-----------------|----------------|---------------|---------------|----------------|---------------|----------------|----------------|---------------|------------------|----------------|---------------|
| Name 2FGL     | $F_1^a$           | $\Delta F_1^a$ | $\sqrt{TS_1}$ | $F_2^a$         | $\Delta F_2^a$ | $\sqrt{TS_2}$ | $F_3^b$       | $\Delta F_3^b$ | $\sqrt{TS_3}$ | $F_4^c$        | $\Delta F_4^c$ | $\sqrt{TS_4}$ | $F_5^c$          | $\Delta F_5^c$ | $\sqrt{TS_5}$ |
| J1117.2+2013  | 1.1               | 0.0            |               | 1.5             | 0.2            | 0.1           | 4.1           | 1.2            | 0.2           | 10.3           | 6.2            | 1.1           | 12.4             | 2.5            | 0.6           |
| J1117.2–5341  | 2.6               | 0.0            |               | 1.9             | 0.3            | 0.0           | 0.6           | 0.8            | 0.0           | 2.7            | 2.0            | 0.8           | 3.8              | 1.6            | 0.0           |
| J1118.0+5354  | 1.3               | 0.0            |               | 2.5             | 0.2            | 0.0           | 3.7           | 0.5            | 0.1           | 6.2            | 2.2            | 0.6           | 6.6              | 1.0            | 0.4           |
| J1118.1–4629  | 1.7               | 0.6            |               | 3.2             | 0.4            | 0.1           | 4.9           | 0.7            | 0.0           | 1.9            | 1.4            | 0.0           | 0.5              | 0.9            | 0.0           |
| J1118.8–6128  | 11.7              | 2.3            |               | 5.5             | 3.5            | 0.4           | 11.3          | 7.2            | 0.7           | 13.0           | 13.4           | 2.1           | 8.7              | 1.5            | 0.6           |
| J1118.9–6027c | 9.3               | 0.0            |               | 3.3             | 1.6            | 0.3           | 6.2           | 2.6            | 0.5           | 5.5            | 3.7            | 0.0           | 1.1              | 0.6            | 0.0           |
| J1120.0–2204  | 1.7               | 0.3            |               | 5.6             | 0.7            | 0.1           | 11.5          | 2.4            | 0.3           | 14.6           | 3.1            | 0.8           | 7.0              | 0.5            | 0.0           |
| J1120.4+0710  | 0.6               | 0.0            |               | 0.0             | 0.3            | 0.1           | 4.3           | 0.7            | 0.2           | 5.6            | 2.5            | 0.8           | 5.9              | 1.0            | 0.0           |
| J1121.0+4211  | 0.5               | 0.0            |               | 0.0             | 0.2            | 0.0           | 2.0           | 0.7            | 0.1           | 7.2            | 3.2            | 0.8           | 8.3              | 2.5            | 0.6           |
| J1121.5–0554  | 4.8               | 0.6            |               | 10.6            | 1.6            | 0.1           | 19.7          | 3.1            | 0.3           | 17.8           | 7.4            | 1.2           | 13.3             | 0.9            | 0.0           |
| J1123.3–2527  | 0.6               | 0.0            |               | 0.0             | 0.2            | 0.0           | 1.0           | 0.7            | 0.0           | 3.0            | 2.2            | 0.7           | 5.0              | 0.5            | 0.0           |
| J1124.2–3654  | 2.2               | 0.0            |               | 0.8             | 0.5            | 0.1           | 5.3           | 1.5            | 0.2           | 9.0            | 4.5            | 1.0           | 7.5              | 1.0            | 0.0           |
| J1124.2+2338  | 1.3               | 0.4            |               | 3.3             | 0.3            | 0.1           | 6.0           | 0.3            | 0.1           | 3.3            | 1.4            | 0.5           | 4.5              | 0.7            | 0.0           |
| J1124.6–5913  | 9.5               | 0.0            |               | 2.5             | 2.8            | 0.2           | 13.0          | 6.5            | 0.5           | 17.5           | 6.4            | 1.3           | 7.2              | 1.5            | 0.0           |
| J1125.0–5821  | 8.1               | 0.0            |               | 2.4             | 0.6            | 0.2           | 3.3           | 1.2            | 0.0           | 2.3            | 3.1            | 1.0           | 4.3              | 0.9            | 0.0           |
| J1125.2+4933  | 1.0               | 0.0            |               | 1.2             | 0.2            | 0.0           | 1.5           | 0.4            | 0.0           | 2.3            | 0.6            | 0.0           | 0.0              | 1.5            | 0.0           |
| J1125.6–3559  | 1.6               | 0.0            |               | 0.1             | 0.2            | 0.0           | 0.5           | 0.8            | 0.2           | 5.3            | 1.8            | 0.7           | 3.9              | 1.8            | 0.0           |
| J1126.0–0743  | 0.6               | 0.0            |               | 0.0             | 0.1            | 0.0           | 0.2           | 0.5            | 0.0           | 2.0            | 1.2            | 0.6           | 3.6              | 1.4            | 0.0           |
| J1126.6–1856  | 5.3               | 0.5            |               | 12.1            | 1.6            | 0.1           | 20.7          | 2.7            | 0.3           | 16.0           | 4.8            | 1.0           | 8.2              | 1.1            | 0.0           |
| J1127.6+3622  | 1.8               | 0.0            |               | 2.2             | 0.3            | 0.1           | 5.0           | 0.5            | 0.1           | 5.0            | 1.6            | 0.6           | 4.9              | 1.1            | 0.0           |
| J1129.0–0532  | 3.6               | 0.6            |               | 7.3             | 0.5            | 0.1           | 6.3           | 0.5            | 0.2           | 3.8            | 2.0            | 0.0           | 2.7              | 0.8            | 0.0           |
| J1129.5+3758  | 1.5               | 0.5            |               | 4.0             | 0.3            | 0.1           | 6.0           | 0.8            | 0.2           | 7.2            | 2.6            | 0.7           | 6.3              | 0.8            | 0.0           |
| J1130.3–1448  | 8.2               | 0.6            |               | 16.3            | 1.2            | 0.1           | 14.9          | 1.6            | 0.2           | 11.0           | 2.1            | 0.0           | 2.8              | 0.9            | 0.0           |
| J1130.9+5809  | 1.3               | 0.0            |               | 2.1             | 0.2            | 0.0           | 3.0           | 0.3            | 0.0           | 1.8            | 1.1            | 0.4           | 4.3              | 1.4            | 0.0           |
| J1132.9+0033  | 2.4               | 0.5            |               | 5.8             | 0.5            | 0.1           | 7.9           | 1.4            | 0.2           | 10.0           | 3.7            | 0.9           | 7.6              | 1.2            | 0.5           |
| J1134.4–7415  | 2.2               | 0.0            |               | 1.9             | 0.5            | 0.0           | 3.0           | 0.7            | 0.2           | 3.5            | 1.5            | 0.7           | 3.3              | 0.5            | 0.0           |
| J1135.2–6829  | 2.7               | 0.7            |               | 3.9             | 0.6            | 0.0           | 2.7           | 0.6            | 0.2           | 3.2            | 2.6            | 0.0           | 2.4              | 1.0            | 0.0           |
| J1135.3–6054  | 4.7               | 1.3            |               | 4.6             | 2.6            | 0.2           | 12.7          | 4.5            | 0.5           | 10.7           | 8.2            | 1.6           | 7.5              | 0.9            | 0.0           |
| J1136.3+6736  | 0.5               | 0.0            |               | 0.0             | 0.2            | 0.0           | 1.3           | 0.4            | 0.1           | 4.8            | 2.1            | 0.6           | 6.1              | 0.6            | 0.3           |
| J1136.7+7009  | 0.5               | 0.0            |               | 0.0             | 0.2            | 0.0           | 5.0           | 0.8            | 0.1           | 8.8            | 2.2            | 0.6           | 6.3              | 1.9            | 0.5           |
| J1137.0+2553  | 0.4               | 0.0            |               | 0.0             | 0.1            | 0.0           | 0.0           | 0.5            | 0.0           | 3.1            | 1.2            | 0.0           | 1.5              | 0.7            | 0.4           |
| J1138.8–6233c | 3.7               | 0.0            |               | 0.3             | 1.3            | 0.0           | 2.6           | 2.2            | 0.6           | 3.9            | 5.4            | 1.8           | 3.7              | 1.3            | 0.0           |
| J1141.0+6803  | 0.5               | 0.0            |               | 0.0             | 0.1            | 0.0           | 0.9           | 0.4            | 0.0           | 1.8            | 1.2            | 0.5           | 4.8              | 0.6            | 0.3           |
| J1141.7–1404  | 0.6               | 0.0            |               | 0.0             | 0.2            | 0.0           | 1.6           | 0.4            | 0.2           | 3.6            | 1.7            | 0.6           | 4.4              | 1.0            | 0.0           |
| J1141.9+1550  | 1.7               | 0.0            |               | 2.4             | 0.3            | 0.0           | 3.0           | 0.7            | 0.2           | 5.8            | 1.3            | 0.6           | 3.6              | 0.7            | 0.4           |
| J1142.9+0121  | 1.6               | 0.0            |               | 1.9             | 0.3            | 0.1           | 4.5           | 0.9            | 0.2           | 7.3            | 3.0            | 0.8           | 6.6              | 1.3            | 0.0           |
| J1143.1+6119  | 1.2               | 0.4            |               | 3.8             | 0.2            | 0.1           | 3.9           | 0.5            | 0.1           | 4.8            | 2.5            | 0.7           | 6.6              | 0.7            | 0.0           |
| J1146.8–3812  | 2.1               | 0.5            |               | 4.6             | 0.6            | 0.1           | 7.3           | 1.2            | 0.2           | 7.9            | 4.3            | 1.0           | 7.3              | 0.9            | 0.0           |
| J1146.9+4000  | 3.1               | 0.4            |               | 8.4             | 0.9            | 0.1           | 14.7          | 1.7            | 0.2           | 13.2           | 3.0            | 0.8           | 7.5              | 0.7            | 0.3           |
| J1147.7–0724  | 2.6               | 0.6            |               | 5.8             | 0.7            | 0.1           | 9.8           | 1.3            | 0.2           | 8.9            | 2.3            | 0.8           | 5.0              | 1.6            | 0.0           |
| J1150.1+2419  | 1.4               | 0.4            |               | 3.8             | 0.4            | 0.1           | 6.9           | 1.0            | 0.2           | 8.0            | 2.8            | 0.8           | 6.8              | 1.6            | 0.0           |
| J1150.5+4154  | 0.9               | 0.0            |               | 0.7             | 0.3            | 0.1           | 6.1           | 1.4            | 0.2           | 12.3           | 6.2            | 1.1           | 12.0             | 3.0            | 0.7           |
| J1151.5–1347  | 0.9               | 0.0            |               | 0.5             | 0.2            | 0.0           | 2.1           | 0.3            | 0.0           | 0.4            | 1.8            | 0.7           | 4.2              | 1.6            | 0.0           |
| J1151.5+5857  | 1.5               | 0.0            |               | 2.4             | 0.2            | 0.0           | 2.9           | 0.5            | 0.1           | 5.3            | 1.9            | 0.6           | 6.4              | 1.1            | 0.4           |

Table 1—Continued

|               | 100 MeV – 300 MeV |                |               | 300 MeV – 1 GeV |                |               | 1 GeV – 3 GeV |                |               | 3 GeV – 10 GeV |                |               | 10 GeV – 100 GeV |                |               |
|---------------|-------------------|----------------|---------------|-----------------|----------------|---------------|---------------|----------------|---------------|----------------|----------------|---------------|------------------|----------------|---------------|
| Name 2FGL     | $F_1^a$           | $\Delta F_1^a$ | $\sqrt{TS_1}$ | $F_2^a$         | $\Delta F_2^a$ | $\sqrt{TS_2}$ | $F_3^b$       | $\Delta F_3^b$ | $\sqrt{TS_3}$ | $F_4^c$        | $\Delta F_4^c$ | $\sqrt{TS_4}$ | $F_5^c$          | $\Delta F_5^c$ | $\sqrt{TS_5}$ |
| J1152.4–0840  | 2.1               | 0.0            | 1.6           | 0.3             | 0.1            | 4.8           | 0.9           | 0.2            | 6.3           | 2.7            | 0.8            | 6.5           | 1.7              | 0.0            | 2.6           |
| J1153.2+4935  | 1.7               | 0.4            | 4.9           | 0.4             | 0.1            | 8.3           | 0.6           | 0.1            | 6.0           | 1.7            | 0.0            | 2.8           | 0.6              | 0.0            | 0.1           |
| J1154.0–0010  | 1.9               | 0.0            | 2.8           | 0.3             | 0.0            | 2.5           | 0.4           | 0.1            | 3.8           | 1.6            | 0.6            | 5.0           | 1.5              | 0.5            | 7.1           |
| J1154.1–3242  | 1.3               | 0.0            | 1.2           | 0.2             | 0.1            | 3.7           | 0.9           | 0.2            | 6.0           | 2.7            | 0.8            | 5.5           | 1.6              | 0.0            | 3.6           |
| J1154.4+6019  | 2.7               | 0.0            | 2.4           | 0.3             | 0.1            | 5.3           | 0.4           | 0.1            | 4.1           | 1.5            | 0.0            | 1.8           | 0.4              | 0.0            | 0.0           |
| J1156.7–0751  | 1.7               | 0.8            | 3.6           | 0.4             | 0.0            | 2.9           | 0.7           | 0.0            | 3.1           | 1.8            | 0.0            | 1.1           | 1.2              | 0.0            | 1.0           |
| J1158.8+0939  | 1.4               | 0.0            | 1.5           | 0.3             | 0.1            | 4.2           | 0.6           | 0.0            | 3.1           | 1.8            | 0.7            | 4.6           | 1.0              | 0.0            | 2.5           |
| J1159.0–2226  | 3.0               | 0.0            | 0.7           | 0.6             | 0.1            | 5.5           | 1.0           | 0.2            | 6.7           | 2.0            | 0.7            | 4.5           | 1.3              | 0.0            | 1.6           |
| J1159.3–2142  | 3.8               | 1.1            | 3.4           | 0.5             | 0.1            | 5.0           | 1.4           | 0.2            | 8.5           | 2.6            | 0.8            | 5.0           | 1.0              | 0.4            | 4.8           |
| J1159.5+2914  | 8.3               | 0.5            | 20.0          | 2.3             | 0.1            | 32.8          | 5.1           | 0.3            | 28.8          | 9.6            | 1.3            | 16.8          | 1.5              | 0.5            | 7.4           |
| J1200.0+0159  | 1.7               | 0.0            | 1.9           | 0.2             | 0.1            | 3.5           | 0.6           | 0.0            | 2.9           | 2.1            | 0.7            | 5.0           | 0.8              | 0.0            | 0.0           |
| J1203.2+6030  | 2.1               | 0.0            | 3.4           | 0.2             | 0.1            | 3.3           | 0.7           | 0.1            | 6.8           | 1.8            | 0.6            | 5.6           | 1.2              | 0.0            | 3.9           |
| J1203.6–6243c | 11.1              | 0.0            | 2.8           | 2.1             | 0.4            | 5.6           | 4.6           | 0.7            | 7.4           | 5.6            | 1.6            | 4.3           | 0.8              | 0.0            | 0.0           |
| J1204.2+1144  | 1.6               | 0.0            | 2.0           | 0.2             | 0.1            | 3.6           | 0.5           | 0.2            | 4.5           | 2.4            | 0.7            | 6.0           | 0.8              | 0.0            | 0.6           |
| J1204.3–0711  | 2.2               | 0.0            | 2.5           | 0.2             | 0.1            | 3.2           | 0.4           | 0.2            | 3.5           | 2.1            | 0.7            | 5.0           | 1.4              | 0.0            | 2.5           |
| J1206.0–2638  | 1.9               | 0.7            | 3.8           | 0.6             | 0.1            | 7.1           | 0.6           | 0.2            | 4.0           | 2.1            | 0.0            | 1.8           | 0.6              | 0.0            | 0.0           |
| J1207.3–5055  | 1.1               | 0.0            | 0.2           | 0.3             | 0.1            | 3.4           | 0.6           | 0.2            | 3.7           | 1.7            | 0.7            | 3.3           | 0.8              | 0.0            | 0.6           |
| J1208.5–6240  | 10.6              | 0.0            | 0.0           | 1.8             | 0.5            | 3.6           | 5.7           | 0.8            | 8.6           | 11.7           | 2.1            | 7.6           | 2.4              | 0.0            | 2.4           |
| J1208.6–2257  | 2.2               | 0.0            | 2.4           | 0.3             | 0.1            | 3.9           | 0.6           | 0.0            | 2.2           | 1.6            | 0.0            | 0.8           | 1.2              | 0.0            | 1.5           |
| J1208.8+5441  | 3.8               | 0.4            | 10.9          | 0.9             | 0.1            | 15.9          | 1.9           | 0.2            | 15.3          | 2.4            | 0.7            | 6.4           | 0.5              | 0.0            | 0.0           |
| J1209.6+4121  | 0.7               | 0.0            | 0.5           | 0.1             | 0.0            | 0.0           | 0.3           | 0.0            | 0.9           | 2.4            | 0.7            | 6.4           | 1.4              | 0.0            | 4.1           |
| J1209.7+1807  | 1.9               | 0.0            | 2.2           | 0.2             | 0.1            | 3.6           | 0.6           | 0.0            | 3.1           | 0.9            | 0.0            | 0.5           | 1.4              | 0.0            | 2.9           |
| J1213.2–2616  | 2.0               | 0.7            | 4.1           | 0.4             | 0.0            | 3.1           | 0.5           | 0.0            | 1.4           | 2.3            | 0.0            | 2.4           | 1.4              | 0.0            | 3.6           |
| J1214.0–6237  | 10.6              | 0.0            | 2.7           | 2.7             | 0.4            | 7.5           | 6.3           | 0.7            | 10.3          | 9.8            | 2.0            | 6.3           | 2.4              | 0.0            | 1.3           |
| J1214.1–4410  | 1.5               | 0.0            | 1.1           | 0.3             | 0.1            | 3.4           | 0.6           | 0.2            | 3.5           | 2.1            | 0.8            | 4.1           | 0.5              | 0.0            | 0.0           |
| J1214.6+1309  | 1.4               | 0.4            | 3.3           | 0.3             | 0.1            | 4.7           | 0.7           | 0.2            | 5.4           | 0.7            | 0.0            | 0.0           | 0.5              | 0.0            | 0.0           |
| J1214.8+1653  | 1.0               | 0.0            | 0.0           | 0.2             | 0.1            | 3.8           | 0.5           | 0.1            | 4.4           | 2.2            | 0.0            | 3.2           | 0.7              | 0.0            | 2.1           |
| J1214.9+5004  | 1.2               | 0.0            | 1.5           | 0.3             | 0.0            | 3.2           | 0.4           | 0.0            | 1.5           | 1.5            | 0.5            | 5.4           | 1.2              | 0.0            | 3.1           |
| J1217.8+3006  | 3.7               | 1.0            | 4.4           | 1.4             | 0.1            | 13.9          | 3.9           | 0.3            | 20.8          | 12.0           | 1.5            | 17.4          | 3.7              | 0.8            | 11.4          |
| J1218.5–0122  | 2.4               | 0.0            | 3.1           | 0.4             | 0.1            | 5.9           | 1.5           | 0.2            | 9.7           | 3.1            | 0.8            | 6.9           | 0.9              | 0.4            | 3.7           |
| J1218.8–4827  | 2.4               | 0.7            | 4.3           | 0.5             | 0.0            | 2.8           | 0.7           | 0.2            | 4.0           | 2.4            | 0.0            | 2.6           | 0.5              | 0.0            | 0.0           |
| J1219.2+7107  | 0.6               | 0.0            | 0.0           | 0.2             | 0.0            | 4.1           | 0.4           | 0.1            | 4.7           | 1.3            | 0.0            | 2.0           | 0.5              | 0.0            | 0.0           |
| J1219.7+0201  | 2.1               | 0.8            | 3.3           | 0.3             | 0.1            | 3.5           | 0.5           | 0.0            | 2.3           | 1.1            | 0.0            | 1.0           | 1.0              | 0.0            | 1.3           |
| J1219.8–0310  | 1.0               | 0.0            | 0.0           | 0.2             | 0.0            | 1.1           | 0.5           | 0.2            | 4.7           | 1.8            | 0.7            | 4.0           | 1.3              | 0.0            | 2.7           |
| J1221.3+3010  | 2.5               | 0.0            | 0.2           | 0.4             | 0.1            | 4.5           | 1.5           | 0.2            | 8.8           | 8.7            | 1.3            | 12.6          | 4.2              | 0.8            | 13.0          |
| J1221.4–0633  | 1.8               | 0.5            | 3.8           | 0.3             | 0.1            | 4.7           | 0.6           | 0.2            | 4.9           | 1.9            | 0.7            | 4.3           | 0.7              | 0.0            | 0.0           |
| J1221.4+2814  | 3.9               | 0.5            | 9.9           | 1.4             | 0.1            | 19.9          | 3.9           | 0.3            | 23.7          | 13.5           | 1.5            | 20.3          | 3.9              | 0.8            | 13.0          |
| J1222.4+0413  | 6.1               | 0.7            | 10.0          | 1.1             | 0.1            | 12.6          | 1.0           | 0.2            | 7.6           | 1.6            | 0.0            | 1.9           | 1.0              | 0.0            | 2.2           |
| J1223.3+7954  | 0.6               | 0.0            | 0.0           | 0.1             | 0.0            | 0.0           | 0.3           | 0.0            | 0.7           | 1.1            | 0.0            | 1.4           | 0.6              | 0.3            | 4.6           |
| J1223.9+8043  | 1.3               | 0.0            | 1.5           | 0.4             | 0.1            | 6.9           | 0.8           | 0.2            | 6.7           | 2.9            | 0.7            | 7.5           | 0.7              | 0.0            | 1.6           |
| J1224.4+2436  | 2.2               | 0.6            | 5.2           | 0.3             | 0.0            | 2.2           | 0.5           | 0.0            | 2.3           | 2.4            | 0.7            | 6.2           | 1.2              | 0.0            | 3.7           |
| J1224.9+2122  | 40.4              | 0.7            | 81.5          | 12.9            | 0.2            | 115.7         | 28.9          | 0.7            | 92.4          | 60.8           | 3.1            | 52.5          | 9.4              | 1.2            | 22.0          |
| J1225.0+4335  | 1.3               | 0.4            | 3.6           | 0.2             | 0.1            | 3.6           | 0.3           | 0.1            | 3.6           | 2.3            | 0.0            | 3.0           | 0.6              | 0.0            | 0.0           |
| J1226.0+2953  | 0.9               | 0.0            | 0.2           | 0.3             | 0.1            | 6.0           | 1.0           | 0.2            | 7.5           | 4.4            | 0.9            | 9.4           | 0.6              | 0.0            | 0.0           |

Table 1—Continued

|              | 100 MeV – 300 MeV |                |               | 300 MeV – 1 GeV |                |               | 1 GeV – 3 GeV |                |               | 3 GeV – 10 GeV |                |               | 10 GeV – 100 GeV |                |               |
|--------------|-------------------|----------------|---------------|-----------------|----------------|---------------|---------------|----------------|---------------|----------------|----------------|---------------|------------------|----------------|---------------|
| Name 2FGL    | $F_1^a$           | $\Delta F_1^a$ | $\sqrt{TS_1}$ | $F_2^a$         | $\Delta F_2^a$ | $\sqrt{TS_2}$ | $F_3^b$       | $\Delta F_3^b$ | $\sqrt{TS_3}$ | $F_4^c$        | $\Delta F_4^c$ | $\sqrt{TS_4}$ | $F_5^c$          | $\Delta F_5^c$ | $\sqrt{TS_5}$ |
| J1226.7–1331 | 1.8               | 0.7            | 4.0           | 0.3             | 0.0            | 1.9           | 1.1           | 0.2            | 6.8           | 3.3            | 0.9            | 7.1           | 1.9              | 0.0            | 3.9           |
| J1226.9+4940 | 2.1               | 0.0            | 0.5           | 0.4             | 0.0            | 3.1           | 0.3           | 0.1            | 3.2           | 2.0            | 0.0            | 2.8           | 0.9              | 0.0            | 1.5           |
| J1227.7–4853 | 3.0               | 0.6            | 6.9           | 1.5             | 0.1            | 16.5          | 3.0           | 0.3            | 13.9          | 3.5            | 0.9            | 6.3           | 0.8              | 0.0            | 1.8           |
| J1228.6+4857 | 3.2               | 0.0            | 2.0           | 0.3             | 0.1            | 4.7           | 0.7           | 0.2            | 5.9           | 1.1            | 0.0            | 0.7           | 1.4              | 0.0            | 4.6           |
| J1228.7–8310 | 1.8               | 0.6            | 3.3           | 0.5             | 0.0            | 2.9           | 0.8           | 0.0            | 2.6           | 1.7            | 0.0            | 0.8           | 0.7              | 0.0            | 0.5           |
| J1229.1+0202 | 52.8              | 0.8            | 84.5          | 10.9            | 0.2            | 90.3          | 14.0          | 0.5            | 53.0          | 14.8           | 1.6            | 20.5          | 0.9              | 0.4            | 4.8           |
| J1230.2+2517 | 1.9               | 0.0            | 1.7           | 0.3             | 0.1            | 4.5           | 0.8           | 0.2            | 7.5           | 1.6            | 0.7            | 3.8           | 1.1              | 0.0            | 2.4           |
| J1230.2–5258 | 2.4               | 0.0            | 1.9           | 0.4             | 0.0            | 2.1           | 1.0           | 0.0            | 3.1           | 1.9            | 0.8            | 3.4           | 1.1              | 0.0            | 1.2           |
| J1230.8+1224 | 1.6               | 0.5            | 4.2           | 0.5             | 0.1            | 8.2           | 1.4           | 0.2            | 11.0          | 3.3            | 0.8            | 8.0           | 1.4              | 0.0            | 4.4           |
| J1231.1–6512 | 2.4               | 0.7            | 3.3           | 0.9             | 0.2            | 5.4           | 1.6           | 0.4            | 4.6           | 3.5            | 0.0            | 1.8           | 1.0              | 0.0            | 0.5           |
| J1231.2–1411 | 4.2               | 0.6            | 11.2          | 3.3             | 0.1            | 41.0          | 13.7          | 0.5            | 52.3          | 33.4           | 2.4            | 33.2          | 1.3              | 0.5            | 6.5           |
| J1231.3–5112 | 1.4               | 0.5            | 3.5           | 0.8             | 0.1            | 8.1           | 1.1           | 0.2            | 5.5           | 1.4            | 0.0            | 0.2           | 0.5              | 0.0            | 0.0           |
| J1231.6+1417 | 1.7               | 0.0            | 1.9           | 0.2             | 0.1            | 3.7           | 0.5           | 0.0            | 2.2           | 1.6            | 0.6            | 4.7           | 1.1              | 0.0            | 2.5           |
| J1231.7+2848 | 1.5               | 0.0            | 1.9           | 0.7             | 0.1            | 12.1          | 2.4           | 0.2            | 17.2          | 8.6            | 1.2            | 15.6          | 3.8              | 0.8            | 12.7          |
| J1233.7–0145 | 2.0               | 0.5            | 4.1           | 0.4             | 0.1            | 5.9           | 0.7           | 0.2            | 5.7           | 1.4            | 0.6            | 3.6           | 0.9              | 0.4            | 4.7           |
| J1234.0–5733 | 2.6               | 0.8            | 3.6           | 0.7             | 0.0            | 2.8           | 1.6           | 0.3            | 6.1           | 2.8            | 1.0            | 3.9           | 2.3              | 0.0            | 2.9           |
| J1236.1–6155 | 5.9               | 0.0            | 2.9           | 1.0             | 0.3            | 3.8           | 2.0           | 0.0            | 2.2           | 6.5            | 0.0            | 2.8           | 1.8              | 0.0            | 1.3           |
| J1238.1–1953 | 1.9               | 0.0            | 2.4           | 0.3             | 0.0            | 1.8           | 0.7           | 0.0            | 3.0           | 1.2            | 0.5            | 3.6           | 0.6              | 0.0            | 0.0           |
| J1239.5+0443 | 6.1               | 0.6            | 12.2          | 1.9             | 0.1            | 23.2          | 3.7           | 0.3            | 20.6          | 7.5            | 1.2            | 13.4          | 1.8              | 0.0            | 4.4           |
| J1239.5+0728 | 1.3               | 0.0            | 1.1           | 0.1             | 0.0            | 0.0           | 0.4           | 0.1            | 3.3           | 2.5            | 0.0            | 3.2           | 0.9              | 0.0            | 2.3           |
| J1240.6–7151 | 2.5               | 0.0            | 2.6           | 0.3             | 0.1            | 3.2           | 0.8           | 0.0            | 2.1           | 2.0            | 0.8            | 4.2           | 2.0              | 0.6            | 6.3           |
| J1241.6–1457 | 1.1               | 0.0            | 0.4           | 0.2             | 0.0            | 1.2           | 0.5           | 0.0            | 1.9           | 1.7            | 0.6            | 4.7           | 0.9              | 0.0            | 1.0           |
| J1243.1+3627 | 1.2               | 0.0            | 2.0           | 0.3             | 0.1            | 5.7           | 0.9           | 0.2            | 8.8           | 5.4            | 1.0            | 11.6          | 3.2              | 0.7            | 11.6          |
| J1243.9–6232 | 2.9               | 0.0            | 0.0           | 1.4             | 0.3            | 5.0           | 2.9           | 0.0            | 3.1           | 4.5            | 1.6            | 3.4           | 1.3              | 0.0            | 0.7           |
| J1245.1+5708 | 1.7               | 0.0            | 2.4           | 0.2             | 0.0            | 2.6           | 0.4           | 0.1            | 3.8           | 1.8            | 0.0            | 3.2           | 1.2              | 0.0            | 4.2           |
| J1246.7–2546 | 10.0              | 0.5            | 22.4          | 3.3             | 0.1            | 34.0          | 7.1           | 0.4            | 31.2          | 16.0           | 1.7            | 19.6          | 1.2              | 0.5            | 4.9           |
| J1248.2+5820 | 1.8               | 0.5            | 5.8           | 0.9             | 0.1            | 17.2          | 3.1           | 0.2            | 22.6          | 10.1           | 1.2            | 18.9          | 3.0              | 0.6            | 12.5          |
| J1248.6–5510 | 2.3               | 0.7            | 3.4           | 0.4             | 0.1            | 3.5           | 0.9           | 0.3            | 3.8           | 1.8            | 0.0            | 1.0           | 1.1              | 0.0            | 1.6           |
| J1249.5–2811 | 0.8               | 0.0            | 0.0           | 0.3             | 0.0            | 2.1           | 0.6           | 0.0            | 2.4           | 2.3            | 0.0            | 2.9           | 1.6              | 0.0            | 4.0           |
| J1249.9+3705 | 0.7               | 0.0            | 0.0           | 0.1             | 0.0            | 0.8           | 0.4           | 0.1            | 4.7           | 2.5            | 0.8            | 6.1           | 1.0              | 0.4            | 5.3           |
| J1251.2+1045 | 0.9               | 0.0            | 0.2           | 0.2             | 0.0            | 1.3           | 0.6           | 0.0            | 2.8           | 2.1            | 0.0            | 2.6           | 1.3              | 0.0            | 2.8           |
| J1253.1+5302 | 1.8               | 0.3            | 5.9           | 0.9             | 0.1            | 16.5          | 2.5           | 0.2            | 18.6          | 10.0           | 1.3            | 17.7          | 2.4              | 0.6            | 10.2          |
| J1254.1+6237 | 0.9               | 0.0            | 1.1           | 0.2             | 0.0            | 1.6           | 0.3           | 0.1            | 4.4           | 1.1            | 0.0            | 1.5           | 0.9              | 0.0            | 3.0           |
| J1254.2–2203 | 2.6               | 0.0            | 2.0           | 0.3             | 0.1            | 3.6           | 0.7           | 0.2            | 4.8           | 2.2            | 0.0            | 1.8           | 1.3              | 0.0            | 2.5           |
| J1254.4+2209 | 1.6               | 0.0            | 2.1           | 0.2             | 0.1            | 3.2           | 0.5           | 0.1            | 4.4           | 2.2            | 0.7            | 5.7           | 1.0              | 0.0            | 2.9           |
| J1255.8–5828 | 4.3               | 0.0            | 2.9           | 0.7             | 0.2            | 4.9           | 1.3           | 0.0            | 3.0           | 2.1            | 0.0            | 1.0           | 0.7              | 0.0            | 0.0           |
| J1256.1–0547 | 39.8              | 0.7            | 72.1          | 11.3            | 0.2            | 95.7          | 20.3          | 0.6            | 68.1          | 42.2           | 2.7            | 40.0          | 5.9              | 1.0            | 16.0          |
| J1256.5–1145 | 2.1               | 0.0            | 2.9           | 0.3             | 0.0            | 2.7           | 0.7           | 0.2            | 5.1           | 1.6            | 0.7            | 3.4           | 1.2              | 0.5            | 5.8           |
| J1257.0+3650 | 0.6               | 0.0            | 0.0           | 0.2             | 0.1            | 4.2           | 0.7           | 0.1            | 7.1           | 1.4            | 0.6            | 3.6           | 1.4              | 0.0            | 3.3           |
| J1258.2+3231 | 2.2               | 0.0            | 2.6           | 0.3             | 0.1            | 5.1           | 0.4           | 0.1            | 4.1           | 1.2            | 0.0            | 1.5           | 0.7              | 0.0            | 0.8           |
| J1258.4–1801 | 3.1               | 0.5            | 6.5           | 0.4             | 0.1            | 5.3           | 0.5           | 0.2            | 3.6           | 2.1            | 0.7            | 5.1           | 0.7              | 0.0            | 1.1           |
| J1258.8–2223 | 2.0               | 0.9            | 4.0           | 0.8             | 0.1            | 9.4           | 1.9           | 0.3            | 10.6          | 3.3            | 0.9            | 6.5           | 0.8              | 0.0            | 0.0           |
| J1259.8–3749 | 1.5               | 0.0            | 1.4           | 0.2             | 0.0            | 0.7           | 0.8           | 0.0            | 2.7           | 1.9            | 0.7            | 3.9           | 1.6              | 0.0            | 3.9           |
| J1301.5+0835 | 0.6               | 0.0            | 0.0           | 0.2             | 0.1            | 4.0           | 0.6           | 0.2            | 5.3           | 2.0            | 0.6            | 5.4           | 0.5              | 0.0            | 0.0           |

Table 1—Continued

|               | 100 MeV – 300 MeV |                |               | 300 MeV – 1 GeV |                |               | 1 GeV – 3 GeV |                |               | 3 GeV – 10 GeV |                |               | 10 GeV – 100 GeV |                |               |
|---------------|-------------------|----------------|---------------|-----------------|----------------|---------------|---------------|----------------|---------------|----------------|----------------|---------------|------------------|----------------|---------------|
| Name 2FGL     | $F_1^a$           | $\Delta F_1^a$ | $\sqrt{TS_1}$ | $F_2^a$         | $\Delta F_2^a$ | $\sqrt{TS_2}$ | $F_3^b$       | $\Delta F_3^b$ | $\sqrt{TS_3}$ | $F_4^c$        | $\Delta F_4^c$ | $\sqrt{TS_4}$ | $F_5^c$          | $\Delta F_5^c$ | $\sqrt{TS_5}$ |
| J1301.6+3331  | 2.0               | 0.0            |               | 2.0             | 0.3            | 0.0           | 2.7           | 0.4            | 0.1           | 5.1            | 1.3            | 0.5           | 4.1              | 0.9            | 0.0           |
| J1302.4–3257  | 1.5               | 0.4            |               | 4.0             | 0.6            | 0.1           | 7.9           | 1.9            | 0.3           | 10.4           | 4.5            | 1.0           | 7.6              | 1.0            | 0.0           |
| J1303.1+2435  | 1.6               | 0.3            |               | 5.1             | 0.8            | 0.1           | 14.4          | 2.5            | 0.2           | 17.6           | 4.2            | 0.9           | 9.4              | 1.3            | 0.5           |
| J1303.5–4622  | 0.6               | 0.0            |               | 0.0             | 0.3            | 0.1           | 3.5           | 0.7            | 0.2           | 4.1            | 1.7            | 0.0           | 1.2              | 0.9            | 0.0           |
| J1303.7–6316c | 4.3               | 1.7            |               | 3.3             | 1.5            | 0.0           | 2.9           | 3.2            | 0.0           | 3.1            | 7.0            | 0.0           | 2.2              | 1.9            | 0.8           |
| J1303.8–5537  | 5.0               | 0.8            |               | 6.5             | 0.7            | 0.1           | 5.7           | 0.8            | 0.3           | 3.5            | 2.8            | 0.0           | 2.6              | 0.7            | 0.0           |
| J1304.1–2415  | 0.9               | 0.0            |               | 0.0             | 0.4            | 0.0           | 2.6           | 0.8            | 0.0           | 2.9            | 2.3            | 0.8           | 4.9              | 0.7            | 0.4           |
| J1304.3–4353  | 3.2               | 0.0            |               | 3.1             | 0.7            | 0.1           | 8.2           | 2.7            | 0.3           | 14.3           | 10.9           | 1.5           | 14.2             | 2.7            | 0.7           |
| J1305.0+1152  | 1.2               | 0.0            |               | 0.9             | 0.3            | 0.1           | 4.7           | 0.6            | 0.0           | 2.7            | 2.4            | 0.0           | 2.8              | 0.7            | 0.0           |
| J1305.1–2110  | 2.8               | 0.0            |               | 3.0             | 0.4            | 0.0           | 2.8           | 0.8            | 0.0           | 2.2            | 1.4            | 0.6           | 3.4              | 1.3            | 0.0           |
| J1305.7+7854  | 1.3               | 0.0            |               | 1.8             | 0.2            | 0.1           | 4.3           | 0.4            | 0.0           | 1.7            | 1.4            | 0.0           | 2.9              | 0.9            | 0.0           |
| J1305.8–4925  | 1.2               | 0.0            |               | 0.3             | 0.3            | 0.1           | 3.3           | 0.9            | 0.0           | 2.3            | 2.7            | 0.0           | 2.4              | 1.6            | 0.0           |
| J1306.2–6044  | 3.8               | 0.0            |               | 2.4             | 1.2            | 0.2           | 6.2           | 4.7            | 0.5           | 11.1           | 10.7           | 1.8           | 8.7              | 1.4            | 0.0           |
| J1306.9–4028  | 1.2               | 0.0            |               | 0.2             | 0.5            | 0.0           | 3.1           | 0.8            | 0.2           | 4.9            | 2.5            | 0.0           | 2.1              | 0.5            | 0.0           |
| J1307.5–4300  | 2.7               | 0.0            |               | 1.9             | 0.4            | 0.0           | 2.9           | 1.2            | 0.2           | 7.2            | 6.2            | 1.2           | 9.5              | 2.3            | 0.6           |
| J1307.6–6704  | 5.4               | 1.2            |               | 6.3             | 1.2            | 0.2           | 7.7           | 1.4            | 0.3           | 5.3            | 3.5            | 1.1           | 4.7              | 1.1            | 0.0           |
| J1308.5+3547  | 1.6               | 0.4            |               | 4.5             | 0.3            | 0.1           | 5.9           | 1.1            | 0.2           | 9.3            | 1.9            | 0.6           | 5.5              | 0.5            | 0.0           |
| J1309.3+1154  | 0.8               | 0.0            |               | 0.0             | 0.2            | 0.0           | 1.2           | 0.5            | 0.0           | 2.6            | 1.7            | 0.6           | 4.5              | 1.0            | 0.0           |
| J1309.4+4304  | 1.4               | 0.0            |               | 2.4             | 0.2            | 0.1           | 4.3           | 1.3            | 0.2           | 11.4           | 5.2            | 0.9           | 11.5             | 1.7            | 0.5           |
| J1309.6–6230c | 3.6               | 0.0            |               | 0.0             | 1.7            | 0.4           | 5.4           | 2.7            | 0.7           | 4.3            | 8.1            | 2.1           | 4.6              | 2.0            | 0.0           |
| J1310.6+3222  | 5.6               | 0.4            |               | 16.3            | 1.8            | 0.1           | 27.7          | 4.2            | 0.3           | 27.0           | 9.9            | 1.3           | 16.8             | 1.3            | 0.5           |
| J1310.9+0036  | 1.1               | 0.0            |               | 0.0             | 0.2            | 0.0           | 0.2           | 0.8            | 0.0           | 2.4            | 1.1            | 0.0           | 0.0              | 1.4            | 0.5           |
| J1311.7–3429  | 5.4               | 0.7            |               | 13.7            | 2.4            | 0.1           | 26.5          | 6.5            | 0.4           | 28.4           | 13.1           | 1.6           | 17.2             | 1.0            | 0.0           |
| J1312.0–6458  | 2.6               | 0.0            |               | 0.0             | 1.0            | 0.2           | 4.8           | 1.5            | 0.0           | 2.0            | 3.8            | 0.0           | 1.6              | 1.2            | 0.0           |
| J1312.4–2157  | 1.5               | 0.0            |               | 0.6             | 0.5            | 0.1           | 5.9           | 2.0            | 0.3           | 11.0           | 5.9            | 1.1           | 9.8              | 1.6            | 0.0           |
| J1312.7+0051  | 1.2               | 0.0            |               | 0.8             | 0.4            | 0.1           | 4.6           | 2.0            | 0.3           | 10.6           | 3.9            | 0.9           | 7.7              | 1.1            | 0.0           |
| J1312.8+4828  | 6.1               | 0.4            |               | 19.1            | 2.6            | 0.1           | 40.4          | 6.4            | 0.4           | 37.4           | 18.9           | 1.7           | 27.8             | 3.2            | 0.7           |
| J1312.9–2351  | 1.5               | 0.5            |               | 3.5             | 0.2            | 0.0           | 0.6           | 0.6            | 0.2           | 4.3            | 3.2            | 0.0           | 3.1              | 1.8            | 0.0           |
| J1313.0–0425  | 1.4               | 0.0            |               | 1.0             | 0.3            | 0.0           | 2.7           | 0.5            | 0.2           | 4.4            | 2.1            | 0.0           | 2.0              | 0.5            | 0.0           |
| J1314.5–5330  | 3.3               | 1.0            |               | 4.6             | 0.8            | 0.1           | 6.2           | 1.6            | 0.3           | 6.4            | 3.9            | 0.0           | 3.0              | 0.7            | 0.0           |
| J1314.6+2348  | 1.8               | 0.0            |               | 2.4             | 0.5            | 0.1           | 8.4           | 1.0            | 0.2           | 8.9            | 3.1            | 0.8           | 7.5              | 0.8            | 0.4           |
| J1315.6–0730  | 1.5               | 0.0            |               | 1.4             | 0.2            | 0.0           | 0.7           | 0.6            | 0.2           | 5.0            | 1.3            | 0.6           | 3.3              | 1.4            | 0.0           |
| J1315.9–3339  | 2.4               | 0.8            |               | 4.7             | 1.0            | 0.1           | 10.7          | 2.3            | 0.3           | 12.3           | 4.1            | 1.0           | 7.4              | 0.8            | 0.4           |
| J1317.2–6304  | 5.7               | 1.3            |               | 5.7             | 2.0            | 0.3           | 7.2           | 5.5            | 0.7           | 8.5            | 5.3            | 1.9           | 3.4              | 1.1            | 0.0           |
| J1317.9+3426  | 0.6               | 0.0            |               | 0.0             | 0.2            | 0.1           | 3.9           | 0.4            | 0.0           | 2.5            | 2.0            | 0.0           | 3.1              | 0.4            | 0.0           |
| J1318.9–1228  | 2.0               | 0.0            |               | 2.1             | 0.2            | 0.0           | 0.6           | 0.6            | 0.2           | 4.6            | 1.3            | 0.0           | 0.9              | 1.4            | 0.0           |
| J1320.1–5756  | 3.7               | 0.9            |               | 4.2             | 0.8            | 0.0           | 2.9           | 1.0            | 0.0           | 1.8            | 1.8            | 0.8           | 3.2              | 0.7            | 0.0           |
| J1321.1+2215  | 2.4               | 0.0            |               | 2.4             | 0.5            | 0.1           | 7.7           | 1.1            | 0.2           | 8.8            | 2.3            | 0.7           | 5.6              | 1.1            | 0.0           |
| J1322.6+8313  | 1.4               | 0.4            |               | 3.8             | 0.3            | 0.0           | 3.0           | 0.4            | 0.0           | 1.5            | 1.0            | 0.4           | 3.4              | 0.5            | 0.0           |
| J1322.7–0938  | 1.6               | 0.6            |               | 3.2             | 0.2            | 0.1           | 3.2           | 0.7            | 0.0           | 3.0            | 1.0            | 0.0           | 0.0              | 1.1            | 0.0           |
| J1323.0+2941  | 1.2               | 0.4            |               | 3.5             | 0.4            | 0.1           | 7.3           | 1.2            | 0.2           | 9.8            | 2.3            | 0.7           | 6.1              | 0.9            | 0.4           |
| J1324.0–4330e | 13.4              | 1.3            |               | 10.6            | 2.3            | 0.2           | 11.6          | 3.1            | 0.5           | 6.5            | 9.2            | 0.0           | 2.7              | 2.4            | 0.0           |
| J1324.4–5411  | 2.8               | 1.2            |               | 3.7             | 0.5            | 0.1           | 3.6           | 0.8            | 0.3           | 3.4            | 3.6            | 0.0           | 2.8              | 1.0            | 0.0           |
| J1325.6–4300  | 14.7              | 1.1            |               | 14.2            | 2.1            | 0.1           | 16.8          | 2.1            | 0.3           | 10.2           | 3.4            | 1.0           | 5.6              | 1.5            | 0.6           |

Table 1—Continued

|              | 100 MeV – 300 MeV |                |               | 300 MeV – 1 GeV |                |               | 1 GeV – 3 GeV |                |               | 3 GeV – 10 GeV |                |               | 10 GeV – 100 GeV |                |               |
|--------------|-------------------|----------------|---------------|-----------------|----------------|---------------|---------------|----------------|---------------|----------------|----------------|---------------|------------------|----------------|---------------|
| Name 2FGL    | $F_1^a$           | $\Delta F_1^a$ | $\sqrt{TS_1}$ | $F_2^a$         | $\Delta F_2^a$ | $\sqrt{TS_2}$ | $F_3^b$       | $\Delta F_3^b$ | $\sqrt{TS_3}$ | $F_4^c$        | $\Delta F_4^c$ | $\sqrt{TS_4}$ | $F_5^c$          | $\Delta F_5^c$ | $\sqrt{TS_5}$ |
| J1326.4–4729 | 0.7               | 0.0            | 0.2           | 0.5             | 0.1            | 3.5           | 1.4           | 0.3            | 5.2           | 2.5            | 0.9            | 3.7           | 0.7              | 0.0            | 0.0           |
| J1326.7–5254 | 3.4               | 1.0            | 5.0           | 1.3             | 0.1            | 10.6          | 3.5           | 0.4            | 13.7          | 5.6            | 1.2            | 7.3           | 1.2              | 0.5            | 4.3           |
| J1326.8+2210 | 4.4               | 0.7            | 10.6          | 1.0             | 0.1            | 14.2          | 1.5           | 0.2            | 11.4          | 1.8            | 0.7            | 4.3           | 0.9              | 0.0            | 2.5           |
| J1328.5–4728 | 0.9               | 0.0            | 0.0           | 0.3             | 0.0            | 0.0           | 0.9           | 0.3            | 3.8           | 2.8            | 1.0            | 4.4           | 2.1              | 0.6            | 8.6           |
| J1329.2–5608 | 4.1               | 1.0            | 6.2           | 1.4             | 0.2            | 10.1          | 3.0           | 0.4            | 10.5          | 4.3            | 1.1            | 5.5           | 0.9              | 0.4            | 3.7           |
| J1329.3–0528 | 4.9               | 0.0            | 1.9           | 0.4             | 0.0            | 0.9           | 0.7           | 0.2            | 3.6           | 1.4            | 0.6            | 3.7           | 0.7              | 0.0            | 0.0           |
| J1329.5–3448 | 1.7               | 0.5            | 3.4           | 0.3             | 0.0            | 1.3           | 0.8           | 0.0            | 2.7           | 1.9            | 0.0            | 2.1           | 0.8              | 0.0            | 1.7           |
| J1329.7–6108 | 3.4               | 0.0            | 0.7           | 0.8             | 0.2            | 3.6           | 2.0           | 0.5            | 5.0           | 4.1            | 1.3            | 4.0           | 0.6              | 0.0            | 0.0           |
| J1330.1–7002 | 6.8               | 0.6            | 11.2          | 2.4             | 0.1            | 20.2          | 5.3           | 0.4            | 20.0          | 9.2            | 1.4            | 11.9          | 1.8              | 0.6            | 6.0           |
| J1330.9+7001 | 1.0               | 0.0            | 1.7           | 0.1             | 0.0            | 1.3           | 0.3           | 0.1            | 4.2           | 1.4            | 0.5            | 5.5           | 1.1              | 0.0            | 3.0           |
| J1332.0–0508 | 11.7              | 1.2            | 10.1          | 3.6             | 0.2            | 24.3          | 4.7           | 0.4            | 20.6          | 3.0            | 0.8            | 7.0           | 1.6              | 0.0            | 3.1           |
| J1332.5–1255 | 6.1               | 0.8            | 11.6          | 1.5             | 0.1            | 16.7          | 2.9           | 0.3            | 16.0          | 5.9            | 1.1            | 10.2          | 1.1              | 0.4            | 5.0           |
| J1332.7+4725 | 1.7               | 0.0            | 2.5           | 0.2             | 0.1            | 4.0           | 0.5           | 0.0            | 2.7           | 1.3            | 0.0            | 1.2           | 0.5              | 0.0            | 0.0           |
| J1332.7+2726 | 0.8               | 0.0            | 0.2           | 0.3             | 0.0            | 2.7           | 0.5           | 0.1            | 4.9           | 1.8            | 0.0            | 2.8           | 0.5              | 0.0            | 0.0           |
| J1333.5+5058 | 2.4               | 0.4            | 6.6           | 0.5             | 0.1            | 8.9           | 0.9           | 0.2            | 8.1           | 1.4            | 0.5            | 4.7           | 0.9              | 0.0            | 3.1           |
| J1335.3–4058 | 1.3               | 0.0            | 0.3           | 0.3             | 0.0            | 1.5           | 0.5           | 0.2            | 3.5           | 3.3            | 0.0            | 3.1           | 1.4              | 0.0            | 2.5           |
| J1335.4–5658 | 3.0               | 1.3            | 3.6           | 0.5             | 0.2            | 3.5           | 1.2           | 0.3            | 4.4           | 4.2            | 0.0            | 2.8           | 0.9              | 0.0            | 0.3           |
| J1337.7–1257 | 3.9               | 0.8            | 7.3           | 0.9             | 0.1            | 10.4          | 1.3           | 0.2            | 7.8           | 2.5            | 0.8            | 5.1           | 1.3              | 0.0            | 3.0           |
| J1338.9+1152 | 0.7               | 0.0            | 0.0           | 0.2             | 0.1            | 3.6           | 0.5           | 0.2            | 4.7           | 1.9            | 0.7            | 5.0           | 0.9              | 0.4            | 5.4           |
| J1339.2–2348 | 1.5               | 0.5            | 3.3           | 0.4             | 0.0            | 3.1           | 0.7           | 0.0            | 2.4           | 2.0            | 0.0            | 1.9           | 1.2              | 0.0            | 3.0           |
| J1340.5–0412 | 0.7               | 0.0            | 0.0           | 0.2             | 0.0            | 1.7           | 0.4           | 0.2            | 3.5           | 1.6            | 0.0            | 1.4           | 1.5              | 0.0            | 3.5           |
| J1340.5+4407 | 1.5               | 0.0            | 1.6           | 0.2             | 0.0            | 1.4           | 0.5           | 0.0            | 2.8           | 1.1            | 0.5            | 3.5           | 1.2              | 0.0            | 2.9           |
| J1341.3–2048 | 1.9               | 0.0            | 1.8           | 0.5             | 0.1            | 5.6           | 0.6           | 0.0            | 1.5           | 1.3            | 0.0            | 1.0           | 0.7              | 0.0            | 0.6           |
| J1344.2–1723 | 3.7               | 0.5            | 9.0           | 1.4             | 0.1            | 16.4          | 3.8           | 0.3            | 18.4          | 9.8            | 1.4            | 13.6          | 2.0              | 0.6            | 7.5           |
| J1345.4+4453 | 3.8               | 0.6            | 10.4          | 1.1             | 0.1            | 18.1          | 1.6           | 0.2            | 12.4          | 2.4            | 0.7            | 6.8           | 1.5              | 0.0            | 4.3           |
| J1345.8–3356 | 1.5               | 0.5            | 3.3           | 0.4             | 0.0            | 2.7           | 0.6           | 0.0            | 1.9           | 2.1            | 0.7            | 4.6           | 1.2              | 0.0            | 1.8           |
| J1345.9+0706 | 0.7               | 0.0            | 0.0           | 0.3             | 0.0            | 3.0           | 0.5           | 0.2            | 3.8           | 1.5            | 0.6            | 4.0           | 0.8              | 0.0            | 1.5           |
| J1346.0–2605 | 1.2               | 0.0            | 0.6           | 0.2             | 0.0            | 1.3           | 0.7           | 0.2            | 5.1           | 2.4            | 0.0            | 1.7           | 0.7              | 0.0            | 0.9           |
| J1346.6–6027 | 5.8               | 0.0            | 2.2           | 1.0             | 0.3            | 3.8           | 1.8           | 0.0            | 1.9           | 6.6            | 0.0            | 2.9           | 2.1              | 0.0            | 2.5           |
| J1347.0–2956 | 0.8               | 0.0            | 0.0           | 0.2             | 0.0            | 0.6           | 0.6           | 0.0            | 2.2           | 1.9            | 0.0            | 2.3           | 1.0              | 0.5            | 4.2           |
| J1347.7–3752 | 2.6               | 0.0            | 3.1           | 0.4             | 0.1            | 4.6           | 0.6           | 0.2            | 4.0           | 2.0            | 0.7            | 5.1           | 0.9              | 0.0            | 0.0           |
| J1349.9–6222 | 4.9               | 1.5            | 3.6           | 2.6             | 0.4            | 7.5           | 5.8           | 0.8            | 7.8           | 10.1           | 2.3            | 5.2           | 1.1              | 0.0            | 0.0           |
| J1350.8+3035 | 1.3               | 0.0            | 1.7           | 0.4             | 0.1            | 7.7           | 0.5           | 0.1            | 5.0           | 1.0            | 0.0            | 0.1           | 0.7              | 0.0            | 1.9           |
| J1351.1+0032 | 2.2               | 0.0            | 2.8           | 0.4             | 0.1            | 5.4           | 0.8           | 0.2            | 6.7           | 1.9            | 0.0            | 1.7           | 0.8              | 0.0            | 0.2           |
| J1351.1–2749 | 1.9               | 0.7            | 4.2           | 0.3             | 0.1            | 3.9           | 0.7           | 0.0            | 2.5           | 1.8            | 0.0            | 2.1           | 0.8              | 0.0            | 1.3           |
| J1351.3–2909 | 2.0               | 0.0            | 0.5           | 0.4             | 0.1            | 4.8           | 0.7           | 0.2            | 4.7           | 2.1            | 0.0            | 2.1           | 0.8              | 0.0            | 1.8           |
| J1351.4+1115 | 0.4               | 0.0            | 0.0           | 0.2             | 0.0            | 1.1           | 0.3           | 0.0            | 1.2           | 1.4            | 0.6            | 4.2           | 1.1              | 0.4            | 6.6           |
| J1352.6–4413 | 2.4               | 0.0            | 2.7           | 0.3             | 0.0            | 1.1           | 0.8           | 0.0            | 2.9           | 1.8            | 0.7            | 4.1           | 0.9              | 0.0            | 0.7           |
| J1353.3+1435 | 2.0               | 0.0            | 2.9           | 0.3             | 0.0            | 3.0           | 0.3           | 0.1            | 3.6           | 2.2            | 0.0            | 2.6           | 1.1              | 0.0            | 2.5           |
| J1353.5–6640 | 4.0               | 0.0            | 2.9           | 0.2             | 0.0            | 0.0           | 1.1           | 0.0            | 2.9           | 2.5            | 0.9            | 4.2           | 1.2              | 0.5            | 5.5           |
| J1354.5+3703 | 1.0               | 0.0            | 1.1           | 0.2             | 0.0            | 1.9           | 0.5           | 0.1            | 4.9           | 1.0            | 0.5            | 3.6           | 0.8              | 0.0            | 0.6           |
| J1354.7–1047 | 3.8               | 0.5            | 7.9           | 0.7             | 0.1            | 8.5           | 1.1           | 0.2            | 7.9           | 2.9            | 0.0            | 2.4           | 1.3              | 0.0            | 2.5           |
| J1356.0–6436 | 6.0               | 1.3            | 5.8           | 1.8             | 0.2            | 9.0           | 1.8           | 0.4            | 4.6           | 4.7            | 0.0            | 2.6           | 0.8              | 0.0            | 0.3           |
| J1358.0+0137 | 1.7               | 0.0            | 1.6           | 0.3             | 0.0            | 2.6           | 0.6           | 0.2            | 4.5           | 1.4            | 0.0            | 1.1           | 0.9              | 0.0            | 0.6           |

Table 1—Continued

|               | 100 MeV – 300 MeV |                |               | 300 MeV – 1 GeV |                |               | 1 GeV – 3 GeV |                |               | 3 GeV – 10 GeV |                |               | 10 GeV – 100 GeV |                |               |
|---------------|-------------------|----------------|---------------|-----------------|----------------|---------------|---------------|----------------|---------------|----------------|----------------|---------------|------------------|----------------|---------------|
| Name 2FGL     | $F_1^a$           | $\Delta F_1^a$ | $\sqrt{TS_1}$ | $F_2^a$         | $\Delta F_2^a$ | $\sqrt{TS_2}$ | $F_3^b$       | $\Delta F_3^b$ | $\sqrt{TS_3}$ | $F_4^c$        | $\Delta F_4^c$ | $\sqrt{TS_4}$ | $F_5^c$          | $\Delta F_5^c$ | $\sqrt{TS_5}$ |
| J1358.1+7644  | 1.5               | 0.0            | 1.7           | 0.3             | 0.1            | 5.4           | 0.8           | 0.1            | 8.3           | 2.1            | 0.6            | 6.2           | 0.4              | 0.0            | 0.0           |
| J1358.8–6027c | 3.1               | 0.0            | 0.0           | 1.7             | 0.0            | 3.1           | 2.9           | 0.6            | 5.1           | 4.6            | 1.6            | 3.5           | 0.9              | 0.0            | 0.0           |
| J1359.4+5541  | 1.7               | 0.4            | 4.6           | 0.4             | 0.1            | 7.0           | 0.6           | 0.1            | 6.1           | 1.5            | 0.0            | 1.9           | 0.4              | 0.0            | 0.0           |
| J1359.9–3746  | 0.7               | 0.0            | 0.0           | 0.2             | 0.0            | 0.6           | 0.6           | 0.0            | 1.9           | 2.1            | 0.8            | 4.4           | 0.9              | 0.4            | 4.5           |
| J1400.2–2412  | 0.8               | 0.0            | 0.0           | 0.2             | 0.0            | 1.0           | 0.7           | 0.2            | 5.2           | 1.9            | 0.0            | 1.9           | 0.9              | 0.0            | 0.9           |
| J1400.6–5601  | 2.4               | 0.7            | 4.0           | 0.6             | 0.1            | 5.0           | 1.5           | 0.3            | 5.8           | 2.1            | 0.8            | 3.5           | 0.7              | 0.0            | 0.1           |
| J1400.7–1438  | 1.7               | 0.0            | 1.5           | 0.4             | 0.0            | 3.1           | 0.7           | 0.2            | 4.7           | 2.8            | 0.0            | 2.9           | 0.5              | 0.0            | 0.0           |
| J1404.0–5244  | 2.1               | 0.0            | 0.9           | 0.5             | 0.0            | 1.7           | 1.1           | 0.3            | 4.6           | 3.2            | 0.0            | 2.0           | 0.6              | 0.0            | 0.0           |
| J1405.1+0405  | 0.5               | 0.0            | 0.0           | 0.2             | 0.0            | 1.9           | 0.4           | 0.1            | 3.4           | 1.7            | 0.7            | 4.0           | 0.9              | 0.0            | 0.5           |
| J1405.5–6121  | 17.5              | 2.5            | 6.5           | 4.6             | 0.6            | 8.0           | 10.7          | 1.1            | 10.9          | 14.5           | 2.9            | 6.0           | 4.3              | 0.0            | 3.1           |
| J1406.2–2510  | 1.1               | 0.0            | 0.9           | 0.2             | 0.0            | 0.9           | 0.6           | 0.0            | 1.8           | 2.5            | 0.8            | 5.8           | 1.0              | 0.4            | 5.1           |
| J1407.4–2948  | 2.0               | 0.0            | 2.2           | 0.4             | 0.1            | 4.6           | 0.5           | 0.2            | 3.2           | 1.2            | 0.0            | 0.1           | 0.5              | 0.0            | 0.0           |
| J1407.5–4257  | 0.6               | 0.0            | 0.0           | 0.4             | 0.0            | 2.6           | 0.5           | 0.2            | 3.4           | 2.3            | 0.8            | 4.9           | 1.2              | 0.0            | 1.7           |
| J1407.6–5937c | 5.3               | 0.0            | 0.0           | 0.9             | 0.3            | 3.6           | 1.9           | 0.0            | 2.1           | 5.4            | 0.0            | 1.9           | 2.6              | 0.0            | 2.9           |
| J1408.8–0751  | 3.9               | 0.5            | 8.6           | 0.8             | 0.1            | 10.0          | 1.5           | 0.2            | 9.9           | 2.0            | 0.7            | 4.9           | 1.6              | 0.0            | 3.8           |
| J1409.9–6129  | 8.0               | 0.0            | 0.0           | 3.4             | 0.0            | 2.4           | 6.3           | 1.1            | 6.2           | 11.6           | 2.9            | 4.8           | 3.8              | 1.2            | 4.5           |
| J1410.3+2811  | 0.6               | 0.0            | 0.2           | 0.2             | 0.0            | 1.7           | 0.4           | 0.0            | 2.8           | 1.2            | 0.0            | 1.0           | 1.0              | 0.4            | 4.7           |
| J1410.4+7411  | 1.4               | 0.0            | 2.6           | 0.2             | 0.0            | 1.5           | 0.4           | 0.1            | 5.3           | 2.0            | 0.6            | 5.7           | 0.7              | 0.3            | 4.7           |
| J1411.9–5744  | 4.6               | 0.0            | 1.8           | 0.9             | 0.2            | 4.6           | 0.9           | 0.0            | 0.9           | 4.9            | 0.0            | 3.0           | 1.4              | 0.0            | 1.9           |
| J1413.4–6204  | 9.9               | 0.0            | 2.0           | 5.0             | 0.5            | 11.8          | 20.2          | 1.1            | 24.0          | 53.7           | 3.8            | 21.3          | 2.0              | 0.8            | 3.5           |
| J1414.1–5450  | 3.2               | 0.9            | 3.6           | 0.7             | 0.2            | 4.4           | 1.2           | 0.0            | 2.2           | 2.0            | 0.0            | 0.8           | 1.0              | 0.0            | 0.8           |
| J1415.7–6520  | 4.2               | 0.0            | 2.1           | 0.5             | 0.2            | 3.3           | 0.8           | 0.0            | 0.9           | 3.3            | 0.0            | 2.2           | 1.8              | 0.0            | 2.6           |
| J1416.0+1323  | 1.4               | 0.4            | 3.3           | 0.2             | 0.1            | 3.6           | 0.4           | 0.1            | 3.4           | 1.4            | 0.0            | 0.6           | 0.8              | 0.0            | 1.9           |
| J1416.3–2415  | 0.5               | 0.0            | 0.0           | 0.1             | 0.0            | 0.3           | 0.3           | 0.0            | 0.0           | 2.3            | 0.0            | 2.3           | 0.8              | 0.4            | 4.5           |
| J1417.5–4404  | 2.2               | 0.6            | 3.9           | 0.5             | 0.0            | 2.9           | 0.8           | 0.2            | 4.4           | 2.0            | 0.8            | 3.5           | 0.7              | 0.0            | 1.1           |
| J1417.7–5028  | 2.4               | 0.0            | 1.5           | 0.5             | 0.0            | 2.4           | 0.9           | 0.3            | 4.3           | 1.8            | 0.0            | 0.9           | 1.4              | 0.0            | 2.3           |
| J1418.1+2539  | 1.0               | 0.0            | 0.7           | 0.2             | 0.0            | 2.1           | 0.6           | 0.0            | 2.9           | 2.0            | 0.0            | 2.1           | 1.5              | 0.0            | 3.3           |
| J1418.4–0234  | 0.6               | 0.0            | 0.0           | 0.3             | 0.0            | 2.5           | 1.3           | 0.2            | 9.1           | 8.3            | 1.3            | 13.9          | 2.3              | 0.6            | 8.8           |
| J1418.7–6058  | 38.1              | 5.6            | 4.1           | 11.5            | 1.3            | 9.6           | 33.6          | 2.1            | 18.1          | 74.4           | 5.4            | 17.7          | 2.4              | 0.9            | 4.0           |
| J1419.4+3820  | 1.8               | 0.0            | 2.5           | 0.3             | 0.1            | 4.4           | 0.4           | 0.1            | 4.6           | 1.1            | 0.0            | 1.1           | 0.7              | 0.0            | 1.0           |
| J1419.4–0835  | 1.1               | 0.0            | 0.4           | 0.3             | 0.1            | 3.9           | 0.6           | 0.2            | 5.3           | 1.6            | 0.6            | 3.9           | 0.7              | 0.0            | 0.4           |
| J1419.4+7730  | 1.2               | 0.0            | 1.6           | 0.1             | 0.0            | 1.1           | 0.4           | 0.0            | 2.6           | 1.8            | 0.0            | 3.1           | 0.9              | 0.0            | 3.4           |
| J1420.1–6047  | 26.9              | 0.0            | 0.0           | 7.0             | 1.3            | 5.5           | 16.7          | 1.9            | 9.2           | 20.7           | 4.3            | 5.5           | 3.6              | 0.0            | 2.8           |
| J1420.2+5422  | 1.7               | 0.4            | 5.0           | 0.3             | 0.1            | 5.9           | 0.4           | 0.1            | 4.9           | 2.1            | 0.6            | 6.2           | 1.0              | 0.0            | 1.8           |
| J1421.1–1117  | 1.1               | 0.0            | 0.4           | 0.3             | 0.0            | 2.3           | 0.5           | 0.2            | 3.9           | 2.7            | 0.0            | 2.8           | 0.8              | 0.0            | 0.0           |
| J1422.3–6841  | 3.4               | 0.8            | 4.6           | 0.7             | 0.1            | 5.3           | 0.7           | 0.0            | 1.1           | 1.9            | 0.7            | 4.0           | 1.2              | 0.0            | 2.0           |
| J1422.5–6137c | 4.1               | 0.0            | 0.0           | 0.2             | 0.0            | 0.0           | 4.4           | 0.7            | 7.6           | 20.9           | 2.7            | 10.3          | 2.2              | 0.0            | 1.9           |
| J1423.9–7842  | 0.9               | 0.0            | 0.0           | 0.3             | 0.0            | 1.4           | 0.5           | 0.2            | 3.2           | 2.1            | 0.7            | 4.9           | 0.7              | 0.0            | 0.0           |
| J1424.2–1752  | 1.2               | 0.0            | 0.6           | 0.3             | 0.0            | 2.7           | 0.7           | 0.0            | 2.1           | 2.6            | 0.8            | 5.7           | 1.4              | 0.0            | 3.6           |
| J1425.1+3615  | 1.5               | 0.0            | 2.3           | 0.3             | 0.1            | 5.5           | 0.6           | 0.2            | 5.2           | 1.7            | 0.6            | 4.5           | 0.9              | 0.4            | 5.7           |
| J1426.1+3406  | 0.9               | 0.0            | 0.8           | 0.2             | 0.0            | 1.6           | 0.3           | 0.1            | 4.1           | 1.5            | 0.6            | 4.8           | 1.2              | 0.0            | 2.3           |
| J1427.0+2347  | 3.0               | 0.5            | 8.4           | 1.8             | 0.1            | 25.9          | 7.1           | 0.4            | 35.6          | 30.5           | 2.2            | 33.0          | 15.8             | 1.5            | 29.5          |
| J1427.4–3306  | 2.0               | 0.5            | 4.0           | 0.6             | 0.1            | 7.0           | 0.6           | 0.2            | 3.7           | 2.5            | 0.0            | 3.1           | 1.0              | 0.0            | 1.8           |
| J1427.6–6048c | 7.7               | 0.0            | 2.5           | 1.3             | 0.4            | 3.2           | 3.6           | 0.9            | 4.3           | 4.6            | 0.0            | 0.6           | 2.6              | 0.0            | 2.3           |



Table 1—Continued

|               | 100 MeV – 300 MeV |                |               | 300 MeV – 1 GeV |                |               | 1 GeV – 3 GeV |                |               | 3 GeV – 10 GeV |                |               | 10 GeV – 100 GeV |                |               |
|---------------|-------------------|----------------|---------------|-----------------|----------------|---------------|---------------|----------------|---------------|----------------|----------------|---------------|------------------|----------------|---------------|
| Name 2FGL     | $F_1^a$           | $\Delta F_1^a$ | $\sqrt{TS_1}$ | $F_2^a$         | $\Delta F_2^a$ | $\sqrt{TS_2}$ | $F_3^b$       | $\Delta F_3^b$ | $\sqrt{TS_3}$ | $F_4^c$        | $\Delta F_4^c$ | $\sqrt{TS_4}$ | $F_5^c$          | $\Delta F_5^c$ | $\sqrt{TS_5}$ |
| J1428.0–4206  | 10.9              | 0.6            | 21.6          | 4.4             | 0.2            | 39.9          | 11.7          | 0.5            | 40.8          | 26.9           | 2.2            | 26.2          | 3.5              | 0.8            | 9.9           |
| J1428.6+4240  | 0.7               | 0.0            | 0.0           | 0.1             | 0.0            | 0.0           | 0.4           | 0.1            | 5.1           | 1.4            | 0.5            | 4.5           | 2.7              | 0.6            | 11.8          |
| J1430.0–5909  | 9.4               | 1.7            | 7.3           | 4.2             | 0.3            | 15.8          | 9.0           | 0.7            | 16.3          | 16.0           | 2.2            | 10.6          | 1.1              | 0.0            | 1.0           |
| J1433.8+4205  | 1.4               | 0.0            | 1.5           | 0.2             | 0.1            | 4.0           | 0.5           | 0.1            | 4.9           | 1.4            | 0.6            | 4.6           | 0.4              | 0.0            | 0.0           |
| J1435.1+2022  | 1.4               | 0.0            | 1.2           | 0.2             | 0.1            | 3.5           | 0.7           | 0.0            | 3.1           | 1.4            | 0.6            | 3.7           | 0.7              | 0.0            | 1.2           |
| J1436.9+2319  | 2.4               | 0.0            | 3.1           | 0.3             | 0.0            | 2.5           | 0.3           | 0.1            | 3.2           | 1.8            | 0.0            | 1.9           | 1.2              | 0.0            | 2.8           |
| J1437.1+5640  | 0.5               | 0.0            | 0.0           | 0.1             | 0.0            | 1.3           | 0.4           | 0.0            | 2.9           | 1.8            | 0.6            | 6.4           | 0.7              | 0.3            | 5.0           |
| J1437.2–5211  | 3.2               | 0.8            | 4.2           | 0.6             | 0.0            | 2.6           | 1.4           | 0.0            | 2.7           | 3.4            | 0.0            | 2.4           | 0.7              | 0.0            | 0.0           |
| J1438.7+3712  | 2.2               | 0.4            | 6.2           | 0.7             | 0.1            | 12.2          | 1.6           | 0.2            | 12.6          | 4.1            | 0.9            | 9.3           | 0.8              | 0.0            | 1.6           |
| J1439.2+3932  | 0.4               | 0.0            | 0.0           | 0.1             | 0.0            | 0.6           | 0.3           | 0.1            | 3.8           | 1.5            | 0.6            | 3.7           | 1.2              | 0.0            | 3.8           |
| J1440.3–1540  | 1.7               | 0.0            | 1.4           | 0.3             | 0.1            | 4.0           | 0.4           | 0.0            | 0.6           | 2.0            | 0.0            | 1.7           | 0.9              | 0.0            | 1.4           |
| J1440.3+4948  | 1.9               | 0.0            | 3.1           | 0.2             | 0.0            | 2.0           | 0.3           | 0.1            | 3.7           | 1.2            | 0.0            | 1.0           | 0.7              | 0.0            | 0.2           |
| J1440.9+0611  | 1.4               | 0.4            | 3.4           | 0.4             | 0.1            | 5.6           | 0.6           | 0.2            | 4.4           | 2.0            | 0.7            | 5.2           | 1.3              | 0.5            | 6.1           |
| J1441.1–3304  | 2.0               | 0.6            | 3.7           | 0.4             | 0.0            | 2.7           | 0.7           | 0.0            | 2.5           | 1.9            | 0.0            | 1.2           | 0.5              | 0.0            | 0.0           |
| J1441.6–5956  | 3.3               | 0.0            | 0.0           | 1.8             | 0.4            | 5.1           | 4.1           | 0.8            | 5.3           | 10.6           | 2.5            | 5.2           | 2.0              | 0.0            | 0.9           |
| J1442.0+4352  | 0.6               | 0.0            | 0.0           | 0.1             | 0.0            | 0.0           | 0.3           | 0.1            | 4.3           | 1.9            | 0.6            | 5.7           | 0.7              | 0.4            | 4.4           |
| J1442.7+1159  | 0.7               | 0.0            | 0.1           | 0.1             | 0.0            | 0.0           | 0.2           | 0.0            | 0.6           | 2.8            | 0.7            | 7.1           | 1.8              | 0.0            | 3.8           |
| J1443.9–3908  | 1.4               | 0.0            | 0.9           | 0.5             | 0.1            | 5.6           | 1.8           | 0.3            | 9.2           | 9.9            | 1.4            | 13.7          | 4.0              | 0.8            | 11.1          |
| J1444.1+2500  | 1.7               | 0.0            | 2.7           | 0.3             | 0.1            | 4.9           | 0.5           | 0.0            | 2.5           | 3.1            | 0.8            | 7.6           | 1.2              | 0.0            | 2.6           |
| J1446.6–5753  | 2.8               | 0.9            | 3.5           | 1.9             | 0.3            | 7.6           | 1.9           | 0.5            | 4.2           | 2.8            | 0.0            | 0.6           | 0.8              | 0.0            | 0.0           |
| J1446.8–4701  | 2.4               | 0.0            | 2.0           | 0.4             | 0.0            | 2.2           | 1.1           | 0.3            | 5.1           | 2.9            | 0.9            | 4.8           | 0.8              | 0.0            | 0.0           |
| J1448.0+3608  | 1.0               | 0.0            | 0.9           | 0.2             | 0.1            | 5.0           | 0.8           | 0.2            | 7.3           | 3.1            | 0.8            | 7.3           | 1.2              | 0.5            | 6.1           |
| J1451.0+5159  | 1.8               | 0.0            | 0.6           | 0.3             | 0.1            | 3.6           | 0.4           | 0.1            | 4.1           | 1.7            | 0.7            | 3.7           | 1.2              | 0.0            | 3.2           |
| J1454.4+5123  | 2.8               | 0.0            | 2.1           | 0.5             | 0.1            | 6.2           | 1.5           | 0.2            | 11.4          | 4.4            | 0.9            | 10.0          | 1.5              | 0.5            | 7.3           |
| J1456.7–6247c | 3.4               | 1.5            | 3.2           | 0.6             | 0.2            | 3.4           | 1.3           | 0.4            | 4.0           | 3.1            | 0.0            | 1.2           | 1.9              | 0.0            | 2.5           |
| J1457.4–3540  | 14.7              | 0.7            | 29.2          | 4.7             | 0.2            | 43.3          | 9.7           | 0.5            | 37.2          | 18.8           | 1.9            | 21.8          | 1.9              | 0.6            | 6.9           |
| J1458.5–2121  | 2.0               | 0.0            | 1.8           | 0.3             | 0.0            | 1.8           | 0.7           | 0.2            | 4.8           | 1.8            | 0.0            | 1.2           | 0.9              | 0.0            | 0.4           |
| J1459.4–6054  | 13.0              | 1.6            | 11.2          | 5.7             | 0.3            | 23.5          | 11.5          | 0.7            | 22.7          | 15.0           | 1.9            | 11.7          | 1.5              | 0.0            | 1.6           |
| J1501.0+2238  | 0.7               | 0.0            | 0.0           | 0.2             | 0.1            | 3.5           | 1.5           | 0.2            | 11.3          | 4.7            | 1.0            | 9.3           | 2.2              | 0.6            | 9.2           |
| J1502.1+5548  | 1.7               | 0.0            | 1.5           | 0.3             | 0.1            | 6.2           | 0.4           | 0.0            | 2.2           | 2.0            | 0.0            | 2.6           | 0.7              | 0.0            | 0.6           |
| J1502.4+4804  | 2.0               | 0.4            | 5.4           | 0.3             | 0.1            | 4.9           | 0.6           | 0.1            | 6.0           | 1.2            | 0.0            | 0.4           | 0.7              | 0.0            | 0.9           |
| J1503.7–1541  | 1.4               | 0.0            | 1.2           | 0.3             | 0.0            | 2.1           | 0.7           | 0.0            | 1.5           | 3.5            | 0.9            | 6.5           | 1.4              | 0.5            | 4.9           |
| J1503.9–5800c | 10.6              | 0.0            | 2.0           | 1.4             | 0.4            | 3.6           | 2.6           | 0.7            | 4.1           | 6.3            | 1.8            | 4.2           | 2.2              | 0.0            | 1.3           |
| J1504.3+1029  | 39.1              | 1.4            | 31.8          | 14.2            | 0.3            | 63.3          | 32.8          | 0.8            | 70.7          | 70.8           | 3.4            | 50.6          | 6.8              | 1.0            | 18.1          |
| J1504.9–3433  | 2.2               | 0.0            | 1.5           | 0.4             | 0.0            | 2.2           | 0.8           | 0.0            | 2.6           | 1.7            | 0.7            | 3.5           | 1.3              | 0.0            | 1.9           |
| J1505.1+0324  | 3.2               | 0.6            | 6.5           | 0.9             | 0.1            | 10.6          | 1.0           | 0.2            | 6.8           | 1.6            | 0.7            | 3.7           | 1.3              | 0.0            | 2.4           |
| J1506.0+3729  | 1.4               | 0.4            | 3.8           | 0.4             | 0.1            | 6.4           | 0.7           | 0.1            | 6.7           | 1.9            | 0.0            | 2.9           | 0.5              | 0.0            | 0.0           |
| J1506.6+0806  | 0.6               | 0.0            | 0.0           | 0.4             | 0.0            | 2.8           | 0.5           | 0.2            | 3.8           | 2.3            | 0.0            | 3.0           | 1.5              | 0.0            | 3.3           |
| J1506.9+1052  | 6.4               | 0.0            | 2.2           | 1.2             | 0.0            | 3.1           | 1.4           | 0.0            | 2.1           | 1.8            | 0.0            | 0.2           | 1.1              | 0.0            | 2.8           |
| J1507.0–6223  | 4.0               | 0.0            | 0.0           | 0.5             | 0.0            | 0.4           | 1.7           | 0.0            | 3.0           | 4.1            | 0.0            | 2.3           | 1.4              | 0.6            | 3.8           |
| J1508.5+2709  | 1.5               | 0.0            | 2.2           | 0.2             | 0.0            | 1.6           | 0.4           | 0.0            | 1.3           | 1.0            | 0.5            | 3.4           | 1.4              | 0.0            | 3.8           |
| J1508.5–4957  | 6.0               | 0.0            | 2.9           | 0.9             | 0.2            | 5.3           | 1.2           | 0.0            | 2.3           | 2.1            | 0.8            | 3.5           | 1.0              | 0.0            | 1.8           |
| J1508.9–4342  | 2.9               | 0.0            | 2.2           | 0.4             | 0.1            | 4.1           | 0.7           | 0.0            | 1.8           | 1.6            | 0.0            | 0.7           | 0.5              | 0.0            | 0.0           |
| J1509.6–5850  | 14.7              | 0.0            | 1.8           | 3.7             | 0.5            | 7.5           | 11.7          | 0.9            | 14.9          | 28.0           | 3.0            | 13.1          | 2.5              | 0.0            | 2.8           |

Table 1—Continued

|               | 100 MeV – 300 MeV |                |               | 300 MeV – 1 GeV |                |               | 1 GeV – 3 GeV |                |               | 3 GeV – 10 GeV |                |               | 10 GeV – 100 GeV |                |               |
|---------------|-------------------|----------------|---------------|-----------------|----------------|---------------|---------------|----------------|---------------|----------------|----------------|---------------|------------------|----------------|---------------|
| Name 2FGL     | $F_1^a$           | $\Delta F_1^a$ | $\sqrt{TS_1}$ | $F_2^a$         | $\Delta F_2^a$ | $\sqrt{TS_2}$ | $F_3^b$       | $\Delta F_3^b$ | $\sqrt{TS_3}$ | $F_4^c$        | $\Delta F_4^c$ | $\sqrt{TS_4}$ | $F_5^c$          | $\Delta F_5^c$ | $\sqrt{TS_5}$ |
| J1509.7+5556  | 1.0               | 0.5            | 3.5           | 0.1             | 0.0            | 0.8           | 0.4           | 0.0            | 1.7           | 1.2            | 0.5            | 4.5           | 0.6              | 0.3            | 4.3           |
| J1510.9–0545  | 7.8               | 0.0            | 2.2           | 1.2             | 0.2            | 7.0           | 2.0           | 0.3            | 9.1           | 3.2            | 1.0            | 4.9           | 0.9              | 0.0            | 1.0           |
| J1510.9–5808c | 10.1              | 0.0            | 0.3           | 1.9             | 0.5            | 3.8           | 3.4           | 0.0            | 2.4           | 7.9            | 0.0            | 2.4           | 2.4              | 0.0            | 1.7           |
| J1511.8–0513  | 5.5               | 0.0            | 1.2           | 0.7             | 0.0            | 2.0           | 0.9           | 0.3            | 4.1           | 2.4            | 0.8            | 4.6           | 1.6              | 0.0            | 3.8           |
| J1512.2+0201  | 1.5               | 0.5            | 3.2           | 0.6             | 0.1            | 7.7           | 1.3           | 0.2            | 8.4           | 3.1            | 0.9            | 6.0           | 1.0              | 0.5            | 4.3           |
| J1512.5–6247c | 4.6               | 1.1            | 4.2           | 1.4             | 0.3            | 5.7           | 1.1           | 0.0            | 1.0           | 3.3            | 0.0            | 1.2           | 1.7              | 0.0            | 3.0           |
| J1512.8–0906  | 73.9              | 0.9            | 112.0         | 19.3            | 0.3            | 128.7         | 33.7          | 0.8            | 86.6          | 60.4           | 3.2            | 45.5          | 8.8              | 1.2            | 18.1          |
| J1513.5–2546  | 0.8               | 0.0            | 0.0           | 0.3             | 0.1            | 3.4           | 0.8           | 0.2            | 4.5           | 2.6            | 0.0            | 2.7           | 0.7              | 0.0            | 0.7           |
| J1513.6–3233  | 3.3               | 0.6            | 5.6           | 0.7             | 0.1            | 6.7           | 1.8           | 0.3            | 8.3           | 2.8            | 0.0            | 2.0           | 1.1              | 0.0            | 1.6           |
| J1513.9–2256  | 1.7               | 0.0            | 0.9           | 0.4             | 0.0            | 2.1           | 0.8           | 0.0            | 2.6           | 2.5            | 0.0            | 2.4           | 2.2              | 0.0            | 3.4           |
| J1514.0–5915e | ...               | 0.0            | 0.0           | ...             | 0.0            | 0.0           | ...           | 0.0            | 0.0           | ...            | 0.0            | 0.0           | ...              | 0.0            | 0.0           |
| J1514.1–4946  | 3.6               | 0.8            | 4.9           | 0.9             | 0.1            | 7.2           | 5.5           | 0.4            | 18.5          | 16.1           | 1.8            | 16.4          | 1.0              | 0.5            | 3.3           |
| J1514.6–4751  | 3.7               | 0.0            | 2.7           | 0.7             | 0.1            | 5.8           | 1.6           | 0.3            | 6.9           | 4.7            | 1.1            | 6.9           | 1.5              | 0.0            | 2.5           |
| J1514.6+4449  | 2.0               | 0.0            | 3.1           | 0.3             | 0.1            | 5.2           | 0.4           | 0.1            | 4.5           | 2.0            | 0.6            | 5.4           | 0.5              | 0.0            | 0.0           |
| J1516.9+1925  | 2.0               | 0.0            | 2.5           | 0.3             | 0.1            | 4.1           | 0.5           | 0.0            | 1.4           | 1.9            | 0.0            | 2.1           | 1.1              | 0.0            | 2.1           |
| J1517.2+3645  | 0.6               | 0.0            | 0.0           | 0.3             | 0.0            | 2.9           | 0.3           | 0.1            | 3.4           | 1.6            | 0.0            | 2.5           | 0.6              | 0.0            | 0.0           |
| J1517.7–2421  | 3.9               | 0.7            | 7.8           | 1.3             | 0.1            | 13.3          | 3.7           | 0.3            | 16.9          | 13.3           | 1.6            | 16.9          | 2.8              | 0.7            | 8.7           |
| J1518.0+6526  | 0.4               | 0.0            | 0.0           | 0.1             | 0.0            | 3.4           | 0.3           | 0.1            | 3.9           | 1.3            | 0.5            | 4.1           | 1.8              | 0.5            | 8.1           |
| J1518.2–2733  | 2.5               | 0.0            | 0.6           | 0.5             | 0.0            | 2.2           | 0.9           | 0.2            | 4.8           | 2.7            | 0.0            | 2.4           | 1.1              | 0.5            | 4.5           |
| J1518.4–5233  | 1.8               | 0.0            | 0.0           | 0.5             | 0.0            | 1.5           | 1.0           | 0.3            | 3.8           | 4.2            | 1.2            | 4.9           | 1.6              | 0.0            | 1.5           |
| J1520.8–0349  | 1.2               | 0.0            | 0.3           | 0.3             | 0.0            | 2.0           | 0.7           | 0.2            | 4.1           | 3.8            | 1.0            | 7.0           | 0.9              | 0.4            | 4.6           |
| J1520.9+4209  | 0.9               | 0.0            | 2.4           | 0.4             | 0.1            | 6.4           | 0.6           | 0.0            | 3.1           | 0.8            | 0.0            | 0.0           | 0.6              | 0.0            | 0.2           |
| J1521.8–5735  | 5.1               | 1.5            | 4.7           | 2.9             | 0.3            | 10.0          | 7.9           | 0.8            | 11.6          | 12.1           | 2.2            | 7.3           | 1.2              | 0.0            | 0.0           |
| J1522.0+4348  | 2.3               | 0.6            | 5.5           | 0.2             | 0.1            | 4.1           | 0.3           | 0.0            | 1.1           | 1.1            | 0.0            | 1.5           | 0.4              | 0.0            | 0.0           |
| J1522.1+3144  | 30.0              | 0.6            | 65.9          | 8.2             | 0.2            | 84.5          | 14.9          | 0.5            | 61.5          | 25.4           | 2.0            | 31.6          | 3.7              | 0.7            | 12.8          |
| J1522.7–2731  | 4.6               | 1.0            | 4.7           | 1.2             | 0.1            | 10.1          | 2.7           | 0.3            | 12.2          | 7.6            | 1.3            | 10.7          | 1.1              | 0.5            | 3.8           |
| J1528.0–5841  | 7.2               | 0.0            | 2.7           | 1.3             | 0.0            | 3.0           | 3.3           | 0.5            | 7.3           | 4.5            | 1.4            | 3.9           | 0.7              | 0.0            | 0.0           |
| J1531.0+5725  | 1.2               | 0.0            | 1.9           | 0.1             | 0.0            | 0.1           | 0.3           | 0.1            | 3.9           | 1.6            | 0.0            | 1.8           | 1.0              | 0.0            | 2.6           |
| J1535.4+3720  | 1.1               | 0.0            | 1.3           | 0.2             | 0.0            | 1.6           | 0.4           | 0.1            | 4.0           | 1.7            | 0.0            | 1.9           | 1.0              | 0.0            | 2.5           |
| J1536.4–4949  | 7.7               | 0.8            | 9.8           | 2.6             | 0.2            | 16.5          | 9.6           | 0.6            | 25.9          | 24.4           | 2.2            | 20.3          | 3.7              | 0.8            | 9.1           |
| J1537.4–7957  | 2.4               | 0.0            | 2.7           | 0.3             | 0.0            | 1.0           | 0.7           | 0.2            | 4.0           | 1.6            | 0.7            | 3.6           | 0.8              | 0.0            | 1.1           |
| J1538.1+8159  | 0.4               | 0.0            | 0.0           | 0.1             | 0.0            | 0.0           | 0.3           | 0.1            | 3.7           | 1.4            | 0.5            | 4.7           | 0.9              | 0.3            | 5.9           |
| J1539.2–3325  | 0.4               | 0.0            | 0.0           | 0.2             | 0.0            | 1.4           | 1.5           | 0.3            | 7.4           | 7.0            | 1.3            | 8.6           | 0.8              | 0.0            | 0.0           |
| J1539.3–4636  | 4.8               | 1.0            | 5.5           | 0.6             | 0.2            | 3.9           | 1.1           | 0.3            | 3.9           | 2.1            | 0.0            | 0.8           | 1.1              | 0.0            | 1.8           |
| J1539.5+2747  | 0.8               | 0.0            | 0.3           | 0.2             | 0.0            | 2.0           | 0.6           | 0.2            | 5.3           | 1.5            | 0.6            | 3.6           | 0.9              | 0.0            | 2.5           |
| J1540.4+1438  | 2.0               | 0.0            | 2.1           | 0.3             | 0.0            | 2.2           | 0.6           | 0.2            | 4.5           | 1.8            | 0.0            | 1.7           | 1.2              | 0.0            | 2.3           |
| J1542.9+6129  | 3.7               | 0.3            | 11.9          | 1.4             | 0.1            | 24.8          | 4.5           | 0.3            | 30.8          | 16.6           | 1.5            | 25.7          | 4.3              | 0.7            | 14.2          |
| J1543.7–0241  | 2.1               | 0.0            | 1.6           | 0.3             | 0.1            | 3.4           | 0.7           | 0.2            | 4.0           | 1.3            | 0.0            | 0.0           | 0.6              | 0.0            | 0.0           |
| J1544.1–2554  | 2.7               | 0.0            | 2.7           | 0.6             | 0.1            | 6.0           | 1.0           | 0.3            | 5.1           | 2.5            | 0.9            | 4.0           | 0.7              | 0.0            | 0.0           |
| J1544.5–1126  | 1.2               | 0.0            | 0.3           | 0.5             | 0.1            | 4.8           | 0.8           | 0.2            | 4.5           | 2.5            | 0.0            | 2.3           | 0.7              | 0.0            | 0.0           |
| J1546.1+0820  | 0.9               | 0.0            | 0.4           | 0.1             | 0.0            | 0.0           | 0.6           | 0.0            | 2.5           | 1.1            | 0.6            | 3.2           | 1.4              | 0.0            | 3.8           |
| J1548.3+1453  | 2.6               | 0.0            | 2.9           | 0.3             | 0.1            | 4.6           | 0.8           | 0.2            | 5.7           | 2.3            | 0.8            | 4.8           | 1.0              | 0.4            | 4.8           |
| J1548.8–2251  | 1.9               | 0.0            | 1.2           | 0.4             | 0.1            | 3.9           | 0.8           | 0.2            | 4.2           | 2.1            | 0.8            | 3.9           | 1.5              | 0.5            | 6.2           |
| J1549.5+0237  | 3.8               | 0.6            | 7.2           | 0.8             | 0.1            | 8.8           | 1.7           | 0.3            | 9.3           | 3.0            | 0.8            | 6.1           | 0.7              | 0.0            | 1.4           |

Table 1—Continued

|               | 100 MeV – 300 MeV |                |               | 300 MeV – 1 GeV |                |               | 1 GeV – 3 GeV |                |               | 3 GeV – 10 GeV |                |               | 10 GeV – 100 GeV |                |               |
|---------------|-------------------|----------------|---------------|-----------------|----------------|---------------|---------------|----------------|---------------|----------------|----------------|---------------|------------------|----------------|---------------|
| Name 2FGL     | $F_1^a$           | $\Delta F_1^a$ | $\sqrt{TS_1}$ | $F_2^a$         | $\Delta F_2^a$ | $\sqrt{TS_2}$ | $F_3^b$       | $\Delta F_3^b$ | $\sqrt{TS_3}$ | $F_4^c$        | $\Delta F_4^c$ | $\sqrt{TS_4}$ | $F_5^c$          | $\Delta F_5^c$ | $\sqrt{TS_5}$ |
| J1549.7–0657  | 1.5               | 0.0            | 0.8           | 0.3             | 0.0            | 1.9           | 0.7           | 0.2            | 4.4           | 1.9            | 0.8            | 3.8           | 1.1              | 0.0            | 1.8           |
| J1550.7+0526  | 2.4               | 0.0            | 2.7           | 0.5             | 0.1            | 6.2           | 0.6           | 0.2            | 4.4           | 2.9            | 0.8            | 5.9           | 0.8              | 0.0            | 0.0           |
| J1551.0–4636  | 2.1               | 0.8            | 3.4           | 0.8             | 0.2            | 4.4           | 1.3           | 0.0            | 2.0           | 1.3            | 0.0            | 0.0           | 1.3              | 0.0            | 2.0           |
| J1551.3–5333c | 12.4              | 0.0            | 1.9           | 2.2             | 0.0            | 2.2           | 3.6           | 1.0            | 3.7           | 11.7           | 3.0            | 4.6           | 2.0              | 0.0            | 0.7           |
| J1551.9+0855  | 0.9               | 0.0            | 0.0           | 0.3             | 0.0            | 2.4           | 0.4           | 0.2            | 3.2           | 1.4            | 0.6            | 3.5           | 1.2              | 0.0            | 2.2           |
| J1552.8–4824  | 4.3               | 1.0            | 5.7           | 1.1             | 0.2            | 5.0           | 1.0           | 0.0            | 0.6           | 2.8            | 0.0            | 0.6           | 0.7              | 0.0            | 0.0           |
| J1552.8–5609  | 4.9               | 0.0            | 1.9           | 1.2             | 0.2            | 5.0           | 4.0           | 0.5            | 9.1           | 13.7           | 2.0            | 10.1          | 4.0              | 0.9            | 7.5           |
| J1553.2–2424  | 3.1               | 0.0            | 2.6           | 0.6             | 0.0            | 3.0           | 0.9           | 0.0            | 2.4           | 2.0            | 0.8            | 3.5           | 0.5              | 0.0            | 0.0           |
| J1553.5–3116  | 0.4               | 0.0            | 0.0           | 0.1             | 0.0            | 0.0           | 0.7           | 0.0            | 2.8           | 3.2            | 0.9            | 5.4           | 1.0              | 0.4            | 4.5           |
| J1553.5+1255  | 3.7               | 0.6            | 9.3           | 1.8             | 0.1            | 20.7          | 4.3           | 0.3            | 21.4          | 6.2            | 1.1            | 10.9          | 1.4              | 0.0            | 3.5           |
| J1553.5–0324  | 1.9               | 0.0            | 1.2           | 0.4             | 0.1            | 3.3           | 1.0           | 0.0            | 2.1           | 3.3            | 0.0            | 2.1           | 2.1              | 0.0            | 3.4           |
| J1554.4–5317c | 11.0              | 0.0            | 1.1           | 2.5             | 0.6            | 4.3           | 6.6           | 1.2            | 6.1           | 13.6           | 3.1            | 5.0           | 3.8              | 0.0            | 1.9           |
| J1555.7+1111  | 3.3               | 0.5            | 7.8           | 1.8             | 0.1            | 22.0          | 7.8           | 0.4            | 34.6          | 43.4           | 2.7            | 40.7          | 22.4             | 1.9            | 37.2          |
| J1558.3+8513  | 2.7               | 0.4            | 7.2           | 0.3             | 0.1            | 4.4           | 0.5           | 0.1            | 4.5           | 1.8            | 0.6            | 5.6           | 0.4              | 0.0            | 0.0           |
| J1558.6–7039  | 1.0               | 0.0            | 0.2           | 0.4             | 0.0            | 2.3           | 0.8           | 0.0            | 2.6           | 2.3            | 0.0            | 2.5           | 1.3              | 0.0            | 2.5           |
| J1558.9–6428  | 2.2               | 0.6            | 3.6           | 0.5             | 0.0            | 3.0           | 1.1           | 0.2            | 6.0           | 3.2            | 1.0            | 5.1           | 1.6              | 0.5            | 5.7           |
| J1559.0+5627  | 1.8               | 0.0            | 1.8           | 0.3             | 0.1            | 5.5           | 1.2           | 0.2            | 10.3          | 2.5            | 0.7            | 6.4           | 1.3              | 0.0            | 3.9           |
| J1600.7–3053  | 0.5               | 0.0            | 0.0           | 0.1             | 0.0            | 0.0           | 0.7           | 0.2            | 4.6           | 3.7            | 1.0            | 6.2           | 0.5              | 0.0            | 0.0           |
| J1601.1–4220  | 4.4               | 0.0            | 3.0           | 0.9             | 0.2            | 5.7           | 1.1           | 0.3            | 3.5           | 4.3            | 0.0            | 2.7           | 1.5              | 0.0            | 2.4           |
| J1602.4+2308  | 0.7               | 0.0            | 0.0           | 0.3             | 0.0            | 1.6           | 0.5           | 0.2            | 4.4           | 1.3            | 0.6            | 3.4           | 0.7              | 0.0            | 0.0           |
| J1603.8–4904  | 6.0               | 2.1            | 4.4           | 3.2             | 0.3            | 12.4          | 8.2           | 0.7            | 15.8          | 32.7           | 2.8            | 19.8          | 11.4             | 1.4            | 17.0          |
| J1604.5–4442  | 8.1               | 1.0            | 8.1           | 2.2             | 0.2            | 12.1          | 4.0           | 0.5            | 11.2          | 11.3           | 1.7            | 10.4          | 2.5              | 0.0            | 3.0           |
| J1604.6+5710  | 4.0               | 0.7            | 10.8          | 0.9             | 0.1            | 14.0          | 1.4           | 0.2            | 11.5          | 3.5            | 0.8            | 8.1           | 0.8              | 0.0            | 0.9           |
| J1607.0+1552  | 2.1               | 0.5            | 4.6           | 0.8             | 0.1            | 10.7          | 1.4           | 0.2            | 10.0          | 5.6            | 1.0            | 10.7          | 1.0              | 0.0            | 1.8           |
| J1608.5+1029  | 4.8               | 0.5            | 10.3          | 1.1             | 0.1            | 13.1          | 1.5           | 0.2            | 9.3           | 2.5            | 0.0            | 3.0           | 0.6              | 0.0            | 1.3           |
| J1610.1–4808  | 5.8               | 1.8            | 4.9           | 1.6             | 0.3            | 5.6           | 1.9           | 0.5            | 3.7           | 3.0            | 0.0            | 1.0           | 0.6              | 0.0            | 0.0           |
| J1610.6–4002  | 4.5               | 1.0            | 5.0           | 1.0             | 0.2            | 6.0           | 1.4           | 0.3            | 4.8           | 2.2            | 1.0            | 3.2           | 1.0              | 0.0            | 0.0           |
| J1610.8–6650  | 1.2               | 0.0            | 0.3           | 0.3             | 0.1            | 4.2           | 1.5           | 0.2            | 8.8           | 7.3            | 1.2            | 11.3          | 3.5              | 0.8            | 11.2          |
| J1612.0+1403  | 2.5               | 0.0            | 3.0           | 0.3             | 0.0            | 2.2           | 0.4           | 0.2            | 3.4           | 2.6            | 0.0            | 2.8           | 0.6              | 0.0            | 0.0           |
| J1613.4+3409  | 1.3               | 0.4            | 3.4           | 0.2             | 0.0            | 2.3           | 0.5           | 0.1            | 5.3           | 1.1            | 0.0            | 0.7           | 1.0              | 0.0            | 2.3           |
| J1614.5–2230  | 7.3               | 0.0            | 1.5           | 0.6             | 0.1            | 5.8           | 3.9           | 0.4            | 15.4          | 7.6            | 1.3            | 9.9           | 0.8              | 0.0            | 0.0           |
| J1614.8+4703  | 1.3               | 0.0            | 1.6           | 0.2             | 0.1            | 3.5           | 0.4           | 0.0            | 2.0           | 1.2            | 0.0            | 0.8           | 0.9              | 0.0            | 2.1           |
| J1614.9–5212  | 5.4               | 0.0            | 0.0           | 2.0             | 0.0            | 1.7           | 3.4           | 0.0            | 2.7           | 6.7            | 0.0            | 1.4           | 2.7              | 1.0            | 4.0           |
| J1615.0–5051  | 14.4              | 3.6            | 4.8           | 5.8             | 0.7            | 8.8           | 8.7           | 1.2            | 7.6           | 15.5           | 3.3            | 5.4           | 4.9              | 0.0            | 2.9           |
| J1615.2–5138  | 11.8              | 0.0            | 1.2           | 2.8             | 0.7            | 4.1           | 9.7           | 1.1            | 10.2          | 24.8           | 3.4            | 9.5           | 4.1              | 1.3            | 4.2           |
| J1616.8–2302  | 3.0               | 0.0            | 0.0           | 0.4             | 0.0            | 0.5           | 0.8           | 0.0            | 1.3           | 3.2            | 1.0            | 5.3           | 1.4              | 0.0            | 1.3           |
| J1617.3–5336  | 4.7               | 1.5            | 3.3           | 0.7             | 0.0            | 0.6           | 2.3           | 0.5            | 5.5           | 3.4            | 0.0            | 0.9           | 0.6              | 0.0            | 0.0           |
| J1617.5–2657  | 3.8               | 0.0            | 2.4           | 0.7             | 0.0            | 2.8           | 1.3           | 0.0            | 2.7           | 3.7            | 0.0            | 2.9           | 0.9              | 0.0            | 0.0           |
| J1617.6–2526c | 2.6               | 1.2            | 3.4           | 0.8             | 0.2            | 5.2           | 0.9           | 0.3            | 3.3           | 3.7            | 0.0            | 2.7           | 0.7              | 0.0            | 0.0           |
| J1617.6–4219  | 5.8               | 0.0            | 3.0           | 0.8             | 0.2            | 4.1           | 1.1           | 0.0            | 1.4           | 2.1            | 0.0            | 0.9           | 1.1              | 0.0            | 1.3           |
| J1618.0–5825  | 5.2               | 0.9            | 6.1           | 0.5             | 0.0            | 1.5           | 0.9           | 0.3            | 3.6           | 3.1            | 0.0            | 2.1           | 1.2              | 0.0            | 1.5           |
| J1618.2–7718  | 4.2               | 1.1            | 3.9           | 1.1             | 0.1            | 10.5          | 2.0           | 0.3            | 10.6          | 1.5            | 0.6            | 3.5           | 0.7              | 0.0            | 1.5           |
| J1619.0–4650  | 6.0               | 1.3            | 6.5           | 2.5             | 0.3            | 8.8           | 2.1           | 0.0            | 2.5           | 1.8            | 0.0            | 0.0           | 0.8              | 0.0            | 0.0           |
| J1619.6–4509  | 5.5               | 0.0            | 1.4           | 0.9             | 0.0            | 1.8           | 1.5           | 0.4            | 3.7           | 4.7            | 0.0            | 1.9           | 1.4              | 0.6            | 4.0           |

Table 1—Continued

|               | 100 MeV – 300 MeV |                |               | 300 MeV – 1 GeV |                |               | 1 GeV – 3 GeV |                |               | 3 GeV – 10 GeV |                |               | 10 GeV – 100 GeV |                |               |
|---------------|-------------------|----------------|---------------|-----------------|----------------|---------------|---------------|----------------|---------------|----------------|----------------|---------------|------------------|----------------|---------------|
| Name 2FGL     | $F_1^a$           | $\Delta F_1^a$ | $\sqrt{TS_1}$ | $F_2^a$         | $\Delta F_2^a$ | $\sqrt{TS_2}$ | $F_3^b$       | $\Delta F_3^b$ | $\sqrt{TS_3}$ | $F_4^c$        | $\Delta F_4^c$ | $\sqrt{TS_4}$ | $F_5^c$          | $\Delta F_5^c$ | $\sqrt{TS_5}$ |
| J1619.7–5040c | 3.2               | 0.0            | 0.0           | 3.1             | 1.0            | 3.6           | 5.7           | 1.2            | 5.1           | 11.8           | 3.0            | 4.5           | 3.8              | 0.0            | 2.5           |
| J1620.5–2320c | 11.9              | 0.0            | 0.8           | 0.7             | 0.2            | 4.2           | 1.0           | 0.3            | 3.7           | 3.6            | 0.0            | 2.8           | 1.2              | 0.0            | 1.8           |
| J1620.6–5111c | 7.4               | 2.8            | 3.3           | 2.9             | 0.7            | 4.4           | 5.8           | 1.0            | 6.0           | 10.9           | 0.0            | 2.8           | 1.5              | 0.0            | 0.0           |
| J1620.8–4928  | 9.7               | 0.0            | 0.6           | 6.1             | 0.6            | 11.7          | 21.6          | 1.3            | 20.2          | 43.2           | 3.9            | 15.4          | 2.4              | 0.9            | 3.4           |
| J1622.8–5006  | 7.5               | 0.0            | 0.0           | 3.3             | 0.0            | 3.0           | 7.7           | 1.2            | 7.1           | 27.7           | 3.7            | 9.5           | 3.9              | 0.0            | 2.4           |
| J1622.8–0314  | 1.0               | 0.0            | 0.0           | 0.4             | 0.1            | 4.4           | 0.6           | 0.2            | 3.2           | 2.4            | 0.8            | 4.7           | 0.9              | 0.0            | 1.2           |
| J1623.2+4328  | 1.9               | 0.4            | 4.8           | 0.3             | 0.0            | 2.8           | 0.3           | 0.0            | 1.6           | 2.1            | 0.0            | 2.6           | 0.7              | 0.0            | 1.2           |
| J1624.0–4941c | 13.5              | 0.0            | 1.3           | 1.5             | 0.0            | 0.1           | 6.7           | 1.3            | 5.6           | 10.5           | 0.0            | 1.6           | 1.9              | 0.0            | 0.4           |
| J1624.1–4040  | 5.0               | 0.9            | 6.7           | 1.6             | 0.2            | 9.6           | 4.1           | 0.5            | 10.8          | 6.2            | 1.4            | 6.1           | 0.6              | 0.0            | 0.0           |
| J1624.2–2124  | 1.9               | 0.5            | 3.9           | 1.1             | 0.2            | 7.7           | 0.9           | 0.0            | 1.4           | 1.3            | 0.0            | 0.0           | 0.8              | 0.0            | 0.0           |
| J1624.4+1123  | 2.1               | 0.0            | 2.0           | 0.3             | 0.1            | 3.7           | 0.5           | 0.0            | 1.6           | 2.4            | 0.0            | 3.0           | 0.5              | 0.0            | 0.0           |
| J1625.2–0020  | 0.8               | 0.0            | 1.0           | 0.2             | 0.1            | 4.8           | 3.7           | 0.3            | 18.4          | 4.9            | 1.0            | 8.2           | 0.5              | 0.0            | 0.0           |
| J1625.7–2526  | 9.1               | 1.4            | 12.2          | 3.5             | 0.2            | 20.6          | 6.7           | 0.5            | 18.6          | 10.8           | 1.7            | 10.4          | 1.4              | 0.6            | 4.1           |
| J1626.0–7636  | 2.9               | 0.0            | 1.2           | 0.2             | 0.0            | 0.0           | 0.8           | 0.0            | 2.8           | 2.3            | 0.0            | 2.8           | 0.7              | 0.3            | 4.5           |
| J1626.1–2948  | 2.7               | 0.9            | 3.8           | 1.4             | 0.1            | 10.7          | 1.6           | 0.3            | 6.4           | 3.7            | 1.1            | 5.3           | 1.1              | 0.0            | 0.5           |
| J1626.4–4408  | 6.9               | 1.7            | 5.3           | 1.6             | 0.3            | 6.7           | 1.5           | 0.4            | 3.8           | 5.5            | 1.4            | 5.3           | 0.7              | 0.0            | 0.0           |
| J1627.0–2425c | 5.0               | 1.5            | 7.0           | 2.0             | 0.2            | 10.5          | 3.8           | 0.5            | 8.8           | 8.1            | 1.8            | 6.5           | 1.5              | 0.0            | 0.3           |
| J1627.8+3219  | 0.7               | 0.0            | 0.0           | 0.3             | 0.0            | 2.9           | 0.6           | 0.1            | 6.0           | 2.1            | 0.7            | 5.2           | 1.0              | 0.0            | 0.9           |
| J1628.1–4857c | 22.1              | 0.0            | 2.5           | 4.7             | 0.6            | 8.7           | 6.5           | 1.1            | 6.5           | 11.7           | 0.0            | 2.8           | 1.9              | 0.0            | 0.6           |
| J1628.3–3206  | 2.2               | 0.0            | 2.6           | 0.5             | 0.1            | 4.2           | 1.5           | 0.3            | 5.9           | 4.5            | 0.0            | 3.1           | 1.0              | 0.0            | 1.5           |
| J1629.4+8236  | 1.1               | 0.0            | 1.4           | 0.5             | 0.1            | 8.9           | 1.0           | 0.2            | 7.8           | 1.4            | 0.5            | 4.1           | 1.2              | 0.0            | 2.8           |
| J1629.6–6141  | 4.6               | 0.7            | 6.6           | 0.5             | 0.1            | 4.8           | 1.5           | 0.3            | 6.9           | 2.3            | 0.0            | 1.7           | 0.6              | 0.0            | 0.0           |
| J1630.1–4615  | 5.6               | 1.7            | 5.0           | 2.9             | 0.4            | 8.9           | 3.8           | 0.7            | 6.2           | 5.1            | 0.0            | 1.7           | 0.7              | 0.0            | 0.0           |
| J1630.2–4752  | 6.8               | 0.0            | 0.0           | 4.0             | 0.0            | 2.8           | 4.5           | 0.0            | 2.2           | 9.8            | 0.0            | 1.9           | 4.9              | 1.3            | 5.7           |
| J1630.3+3732  | 1.2               | 0.0            | 1.5           | 0.2             | 0.0            | 2.8           | 0.8           | 0.2            | 6.5           | 3.1            | 0.8            | 7.7           | 0.4              | 0.0            | 0.0           |
| J1630.4+5218  | 1.4               | 0.0            | 2.3           | 0.2             | 0.1            | 3.7           | 0.7           | 0.2            | 6.0           | 2.6            | 0.7            | 7.4           | 1.2              | 0.0            | 3.1           |
| J1631.0–1050  | 2.4               | 0.0            | 1.5           | 0.5             | 0.1            | 4.0           | 1.1           | 0.0            | 2.6           | 4.2            | 0.0            | 3.1           | 0.6              | 0.0            | 0.0           |
| J1631.6–2819  | 3.8               | 1.0            | 4.8           | 0.7             | 0.2            | 5.0           | 1.3           | 0.0            | 2.9           | 1.7            | 0.0            | 0.1           | 0.5              | 0.0            | 0.0           |
| J1631.7–4720c | 4.0               | 0.0            | 0.0           | 3.0             | 0.0            | 1.4           | 7.1           | 1.1            | 7.1           | 9.1            | 2.6            | 4.0           | 3.5              | 1.1            | 4.4           |
| J1632.4–4820c | 10.1              | 0.0            | 0.0           | 3.0             | 0.0            | 1.3           | 7.0           | 1.2            | 6.3           | 10.3           | 2.8            | 4.2           | 3.0              | 1.2            | 3.4           |
| J1632.4–4753c | 7.1               | 0.0            | 0.0           | 3.9             | 0.0            | 0.5           | 5.9           | 1.6            | 3.9           | 20.6           | 3.7            | 6.9           | 5.6              | 1.5            | 4.9           |
| J1632.6–2328c | 3.7               | 0.0            | 2.0           | 0.8             | 0.2            | 4.9           | 1.3           | 0.4            | 4.2           | 4.6            | 0.0            | 3.1           | 0.9              | 0.0            | 0.7           |
| J1634.4–4743c | 26.2              | 0.0            | 2.6           | 1.8             | 0.0            | 0.0           | 5.4           | 1.6            | 3.5           | 18.0           | 3.9            | 5.5           | 6.5              | 0.0            | 3.1           |
| J1635.2+3810  | 21.8              | 1.0            | 46.7          | 5.7             | 0.2            | 61.9          | 10.5          | 0.5            | 46.5          | 14.4           | 1.5            | 20.6          | 0.8              | 0.4            | 5.6           |
| J1635.4–4717c | 5.7               | 0.0            | 0.0           | 5.7             | 0.0            | 2.5           | 7.9           | 1.5            | 5.8           | 15.9           | 3.4            | 5.7           | 4.5              | 1.3            | 4.9           |
| J1636.3–4740c | 23.0              | 0.0            | 0.8           | 6.6             | 1.0            | 6.0           | 12.4          | 1.7            | 7.9           | 18.9           | 3.8            | 5.9           | 3.7              | 0.0            | 1.9           |
| J1636.6–0841  | 2.9               | 0.0            | 2.2           | 0.5             | 0.0            | 2.3           | 0.9           | 0.3            | 4.0           | 2.2            | 0.0            | 1.5           | 1.4              | 0.0            | 2.6           |
| J1637.7+4714  | 3.6               | 0.4            | 9.5           | 0.8             | 0.1            | 12.7          | 1.4           | 0.2            | 11.2          | 3.8            | 0.9            | 8.1           | 1.1              | 0.0            | 2.6           |
| J1637.9–3451  | 2.9               | 0.0            | 2.0           | 0.1             | 0.0            | 0.0           | 1.3           | 0.0            | 2.9           | 2.3            | 0.9            | 3.5           | 1.3              | 0.5            | 4.7           |
| J1638.0–4703c | 26.3              | 0.0            | 2.5           | 4.6             | 0.0            | 2.9           | 11.6          | 1.4            | 8.9           | 20.0           | 3.6            | 6.6           | 4.1              | 0.0            | 2.2           |
| J1639.7–5504  | 5.1               | 1.2            | 5.4           | 0.8             | 0.0            | 2.9           | 1.3           | 0.0            | 2.2           | 2.0            | 0.0            | 0.4           | 1.0              | 0.0            | 1.7           |
| J1639.8–5145  | 6.3               | 2.0            | 5.2           | 1.6             | 0.2            | 7.4           | 2.6           | 0.4            | 6.8           | 6.3            | 1.4            | 6.5           | 1.8              | 0.0            | 1.8           |
| J1639.8–4921c | 15.5              | 0.0            | 1.7           | 1.5             | 0.0            | 1.3           | 2.2           | 0.0            | 1.8           | 6.1            | 1.7            | 4.6           | 2.4              | 0.0            | 1.8           |
| J1640.5–4633  | 18.8              | 0.0            | 2.6           | 5.4             | 0.7            | 8.6           | 7.3           | 1.1            | 7.0           | 21.4           | 3.4            | 7.8           | 4.3              | 1.3            | 4.3           |

Table 1—Continued

|               | 100 MeV – 300 MeV |                |               | 300 MeV – 1 GeV |                |               | 1 GeV – 3 GeV |                |               | 3 GeV – 10 GeV |                |               | 10 GeV – 100 GeV |                |               |
|---------------|-------------------|----------------|---------------|-----------------|----------------|---------------|---------------|----------------|---------------|----------------|----------------|---------------|------------------|----------------|---------------|
| Name 2FGL     | $F_1^a$           | $\Delta F_1^a$ | $\sqrt{TS_1}$ | $F_2^a$         | $\Delta F_2^a$ | $\sqrt{TS_2}$ | $F_3^b$       | $\Delta F_3^b$ | $\sqrt{TS_3}$ | $F_4^c$        | $\Delta F_4^c$ | $\sqrt{TS_4}$ | $F_5^c$          | $\Delta F_5^c$ | $\sqrt{TS_5}$ |
| J1640.7+3945  | 9.6               | 0.0            | 2.3           | 1.9             | 0.2            | 9.1           | 3.0           | 0.4            | 11.0          | 8.2            | 1.3            | 10.9          | 1.5              | 0.0            | 2.8           |
| J1641.0+1141  | 2.1               | 0.0            | 2.6           | 0.3             | 0.0            | 1.4           | 0.5           | 0.0            | 1.8           | 1.7            | 0.7            | 4.1           | 1.0              | 0.0            | 2.3           |
| J1641.6–0614  | 6.9               | 0.0            | 2.1           | 0.8             | 0.0            | 2.9           | 1.3           | 0.0            | 3.0           | 2.4            | 0.9            | 4.2           | 1.3              | 0.0            | 2.3           |
| J1641.8–5319  | 5.9               | 0.0            | 2.2           | 0.6             | 0.2            | 3.5           | 1.7           | 0.4            | 5.4           | 4.5            | 0.0            | 3.1           | 0.5              | 0.0            | 0.0           |
| J1642.9+3949  | 8.4               | 2.2            | 4.0           | 1.6             | 0.2            | 7.8           | 2.9           | 0.4            | 10.5          | 4.8            | 1.1            | 7.3           | 1.4              | 0.0            | 2.2           |
| J1643.3–4928  | 8.0               | 0.0            | 0.0           | 2.5             | 0.0            | 3.0           | 2.4           | 0.6            | 4.6           | 6.9            | 0.0            | 3.1           | 1.4              | 0.0            | 0.9           |
| J1643.5–0641  | 4.1               | 0.0            | 0.5           | 0.6             | 0.0            | 2.0           | 0.8           | 0.3            | 3.7           | 2.8            | 1.0            | 3.8           | 0.9              | 0.5            | 3.6           |
| J1645.7–2148c | 2.4               | 0.0            | 3.0           | 0.7             | 0.1            | 5.6           | 1.3           | 0.3            | 4.6           | 2.8            | 0.0            | 1.3           | 0.6              | 0.0            | 0.0           |
| J1646.7–1333  | 1.2               | 0.0            | 0.0           | 0.3             | 0.0            | 0.4           | 1.0           | 0.0            | 2.2           | 1.7            | 0.8            | 3.5           | 1.7              | 0.0            | 3.1           |
| J1647.0+4351  | 1.6               | 0.0            | 2.0           | 0.3             | 0.1            | 4.7           | 0.3           | 0.0            | 1.3           | 1.5            | 0.0            | 2.1           | 0.7              | 0.0            | 0.8           |
| J1647.5+4950  | 2.6               | 0.4            | 6.8           | 0.6             | 0.1            | 9.6           | 1.2           | 0.2            | 9.8           | 1.9            | 0.6            | 5.2           | 0.6              | 0.0            | 0.0           |
| J1648.1–4930  | 4.4               | 0.0            | 0.0           | 1.1             | 0.3            | 3.9           | 1.4           | 0.0            | 1.3           | 3.5            | 1.3            | 3.5           | 1.2              | 0.6            | 3.6           |
| J1648.4–4612  | 11.0              | 0.0            | 0.0           | 3.1             | 0.0            | 2.4           | 7.3           | 1.1            | 7.1           | 18.2           | 3.1            | 7.3           | 2.7              | 0.0            | 1.3           |
| J1649.2–3004  | 1.4               | 0.0            | 0.0           | 0.4             | 0.0            | 1.0           | 0.8           | 0.3            | 3.4           | 4.6            | 1.2            | 5.6           | 1.2              | 0.0            | 0.9           |
| J1649.6+5238  | 1.6               | 0.0            | 2.4           | 0.3             | 0.1            | 5.0           | 0.4           | 0.1            | 3.6           | 2.1            | 0.6            | 5.7           | 0.6              | 0.0            | 1.4           |
| J1650.1–5044  | 10.7              | 1.9            | 9.5           | 2.2             | 0.2            | 11.0          | 5.6           | 0.5            | 14.5          | 16.9           | 2.0            | 13.8          | 2.2              | 0.7            | 6.3           |
| J1650.6–4603c | 15.8              | 0.0            | 2.6           | 2.4             | 0.8            | 3.3           | 7.0           | 1.2            | 6.5           | 19.9           | 3.1            | 8.0           | 4.2              | 0.0            | 2.6           |
| J1650.8+0830  | 2.2               | 0.6            | 3.9           | 0.4             | 0.1            | 4.5           | 0.5           | 0.2            | 3.2           | 2.5            | 0.0            | 2.8           | 0.5              | 0.0            | 0.0           |
| J1651.8–4439c | 7.3               | 0.0            | 3.0           | 2.5             | 0.5            | 5.0           | 4.3           | 1.1            | 4.2           | 11.9           | 0.0            | 2.8           | 1.2              | 0.0            | 0.0           |
| J1652.5–4351c | 2.5               | 0.0            | 0.0           | 1.6             | 0.0            | 2.2           | 5.4           | 1.0            | 5.7           | 12.2           | 2.9            | 4.9           | 1.2              | 0.0            | 0.0           |
| J1653.6–0159  | 2.6               | 0.7            | 5.4           | 1.5             | 0.1            | 14.0          | 3.3           | 0.3            | 14.1          | 7.5            | 1.3            | 9.6           | 0.9              | 0.0            | 0.0           |
| J1653.9+3945  | 2.7               | 0.4            | 6.9           | 1.3             | 0.1            | 19.8          | 5.0           | 0.3            | 28.4          | 26.0           | 2.0            | 30.9          | 12.5             | 1.3            | 27.1          |
| J1653.9–4627c | 4.9               | 0.0            | 0.0           | 1.7             | 0.5            | 3.3           | 2.7           | 0.7            | 4.0           | 9.9            | 2.2            | 5.9           | 3.5              | 0.0            | 2.6           |
| J1656.1–3256  | 7.1               | 1.1            | 7.0           | 0.9             | 0.2            | 5.5           | 0.9           | 0.3            | 3.3           | 2.3            | 0.0            | 0.8           | 0.5              | 0.0            | 0.0           |
| J1656.4–0738  | 2.5               | 0.8            | 3.5           | 0.4             | 0.1            | 3.2           | 0.8           | 0.0            | 1.4           | 3.4            | 0.0            | 2.7           | 0.9              | 0.0            | 0.3           |
| J1656.5+6012  | 1.4               | 0.4            | 4.0           | 0.2             | 0.0            | 1.1           | 0.3           | 0.1            | 3.8           | 1.3            | 0.0            | 1.8           | 0.8              | 0.0            | 2.3           |
| J1656.9–2008  | 0.6               | 0.0            | 0.0           | 0.4             | 0.0            | 1.9           | 0.7           | 0.3            | 3.3           | 3.5            | 1.0            | 5.5           | 1.9              | 0.0            | 2.2           |
| J1657.1–1027  | 3.5               | 0.0            | 2.8           | 0.6             | 0.1            | 4.1           | 1.1           | 0.0            | 2.2           | 3.3            | 0.0            | 2.5           | 1.4              | 0.0            | 1.1           |
| J1657.5–4652  | 5.3               | 0.0            | 0.0           | 1.8             | 0.0            | 2.2           | 2.5           | 0.6            | 4.4           | 4.2            | 1.6            | 3.5           | 1.8              | 0.7            | 4.3           |
| J1657.9+4809  | 1.8               | 0.4            | 4.7           | 0.7             | 0.1            | 11.1          | 1.0           | 0.2            | 8.1           | 1.2            | 0.5            | 3.2           | 1.1              | 0.0            | 3.0           |
| J1658.1–4743  | 8.6               | 3.0            | 3.7           | 1.4             | 0.3            | 4.4           | 2.5           | 0.0            | 3.0           | 5.7            | 0.0            | 2.6           | 1.9              | 0.0            | 2.0           |
| J1658.4–5322  | 5.0               | 0.9            | 6.8           | 1.3             | 0.2            | 9.1           | 2.7           | 0.4            | 9.4           | 2.1            | 0.8            | 3.5           | 0.8              | 0.0            | 0.4           |
| J1659.2–0142  | 2.2               | 0.0            | 1.1           | 0.5             | 0.0            | 2.9           | 0.7           | 0.2            | 3.6           | 3.1            | 1.0            | 4.5           | 1.5              | 0.0            | 3.1           |
| J1700.2+6831  | 6.3               | 0.5            | 17.4          | 1.8             | 0.1            | 26.7          | 3.3           | 0.3            | 22.1          | 6.5            | 1.0            | 13.3          | 1.1              | 0.0            | 2.7           |
| J1700.8–4912  | 3.9               | 1.8            | 3.3           | 0.9             | 0.2            | 4.7           | 1.5           | 0.0            | 2.2           | 3.7            | 0.0            | 1.8           | 1.5              | 0.0            | 1.4           |
| J1701.2–3007  | 3.5               | 1.0            | 4.0           | 1.1             | 0.2            | 7.3           | 2.6           | 0.4            | 9.0           | 5.2            | 1.2            | 6.5           | 1.5              | 0.0            | 1.8           |
| J1702.5–5654  | 4.3               | 0.7            | 7.6           | 1.5             | 0.1            | 13.0          | 3.0           | 0.3            | 11.8          | 4.9            | 1.1            | 6.9           | 0.9              | 0.0            | 0.5           |
| J1703.2–6217  | 7.1               | 0.6            | 11.8          | 1.5             | 0.1            | 14.8          | 2.7           | 0.3            | 12.6          | 3.8            | 1.0            | 6.5           | 0.9              | 0.4            | 4.2           |
| J1704.3+1235  | 1.5               | 0.0            | 1.1           | 0.4             | 0.0            | 2.8           | 0.6           | 0.0            | 1.6           | 1.5            | 0.7            | 3.3           | 1.0              | 0.0            | 2.6           |
| J1704.6–0529  | 2.3               | 0.8            | 3.2           | 0.6             | 0.1            | 4.6           | 1.1           | 0.3            | 4.6           | 2.7            | 0.9            | 4.0           | 1.2              | 0.0            | 1.6           |
| J1704.9–4618  | 9.3               | 2.3            | 10.5          | 1.8             | 0.3            | 6.3           | 1.8           | 0.5            | 3.5           | 4.7            | 0.0            | 1.5           | 1.0              | 0.0            | 0.0           |
| J1708.4+1003c | 2.7               | 0.0            | 2.5           | 0.3             | 0.1            | 3.4           | 0.8           | 0.0            | 2.7           | 1.1            | 0.0            | 1.0           | 0.9              | 0.0            | 1.1           |
| J1709.0–0821  | 3.3               | 0.8            | 4.4           | 0.7             | 0.1            | 4.9           | 1.1           | 0.3            | 4.3           | 1.8            | 0.0            | 0.3           | 1.0              | 0.0            | 0.4           |
| J1709.7–4429  | 88.0              | 1.6            | 67.0          | 47.1            | 0.5            | 147.3         | 153.1         | 1.8            | 162.7         | 335.0          | 7.6            | 101.4         | 23.3             | 1.9            | 27.2          |

Table 1—Continued

|               | 100 MeV – 300 MeV |                |               | 300 MeV – 1 GeV |                |               | 1 GeV – 3 GeV |                |               | 3 GeV – 10 GeV |                |               | 10 GeV – 100 GeV |                |               |
|---------------|-------------------|----------------|---------------|-----------------|----------------|---------------|---------------|----------------|---------------|----------------|----------------|---------------|------------------|----------------|---------------|
| Name 2FGL     | $F_1^a$           | $\Delta F_1^a$ | $\sqrt{TS_1}$ | $F_2^a$         | $\Delta F_2^a$ | $\sqrt{TS_2}$ | $F_3^b$       | $\Delta F_3^b$ | $\sqrt{TS_3}$ | $F_4^c$        | $\Delta F_4^c$ | $\sqrt{TS_4}$ | $F_5^c$          | $\Delta F_5^c$ | $\sqrt{TS_5}$ |
| J1709.7+4319  | 3.1               | 0.4            | 8.3           | 0.9             | 0.1            | 14.6          | 1.5           | 0.2            | 12.0          | 4.5            | 0.9            | 9.8           | 0.8              | 0.4            | 4.9           |
| J1710.0–0323  | 3.1               | 0.8            | 4.3           | 0.6             | 0.1            | 4.6           | 1.1           | 0.3            | 4.4           | 3.0            | 0.0            | 2.0           | 0.5              | 0.0            | 0.0           |
| J1710.5–5020  | 2.5               | 0.6            | 4.5           | 1.1             | 0.2            | 6.4           | 1.3           | 0.0            | 2.1           | 2.7            | 0.0            | 1.4           | 1.6              | 0.0            | 2.2           |
| J1712.4–3941  | 3.1               | 0.0            | 0.0           | 1.4             | 0.0            | 1.3           | 2.1           | 0.0            | 0.9           | 8.5            | 2.4            | 4.2           | 3.5              | 1.1            | 4.4           |
| J1714.0+0751  | 2.4               | 0.0            | 1.9           | 0.4             | 0.1            | 4.8           | 0.9           | 0.2            | 5.4           | 2.8            | 0.9            | 4.9           | 0.8              | 0.0            | 1.3           |
| J1714.5–3829  | 9.3               | 0.0            | 1.3           | 3.8             | 0.5            | 8.1           | 11.1          | 1.0            | 12.2          | 30.8           | 3.5            | 11.9          | 2.8              | 1.1            | 3.3           |
| J1714.8+6836  | 1.1               | 0.0            | 2.9           | 0.3             | 0.1            | 7.0           | 1.1           | 0.2            | 8.7           | 1.1            | 0.5            | 3.7           | 0.6              | 0.0            | 1.1           |
| J1715.4–4024c | 8.6               | 0.0            | 2.9           | 1.7             | 0.0            | 2.7           | 3.1           | 0.0            | 3.0           | 8.1            | 2.0            | 5.1           | 2.9              | 1.0            | 4.3           |
| J1716.6–0526c | 2.6               | 0.0            | 3.0           | 0.8             | 0.2            | 5.1           | 1.1           | 0.0            | 1.7           | 3.7            | 0.0            | 2.6           | 1.1              | 0.0            | 1.4           |
| J1717.3–2809  | 6.0               | 1.2            | 5.4           | 0.7             | 0.0            | 1.6           | 1.7           | 0.0            | 2.8           | 3.2            | 1.2            | 3.6           | 1.8              | 0.0            | 2.0           |
| J1717.5–5802  | 2.6               | 0.7            | 4.0           | 0.5             | 0.1            | 4.3           | 0.9           | 0.2            | 4.4           | 2.8            | 0.0            | 2.5           | 0.8              | 0.0            | 0.0           |
| J1717.7–3342  | 12.5              | 1.3            | 9.7           | 4.8             | 0.3            | 17.0          | 6.2           | 0.7            | 11.1          | 11.8           | 2.1            | 7.9           | 2.4              | 0.0            | 3.1           |
| J1718.1–3725  | 3.0               | 0.0            | 0.0           | 2.2             | 0.0            | 3.1           | 3.8           | 0.0            | 2.5           | 8.2            | 2.4            | 4.0           | 2.8              | 1.0            | 4.0           |
| J1718.3–3827  | 13.5              | 3.1            | 4.6           | 3.8             | 0.5            | 8.4           | 9.2           | 1.0            | 10.7          | 10.1           | 2.4            | 5.2           | 1.0              | 0.0            | 0.0           |
| J1718.4–3056  | 6.0               | 0.0            | 2.8           | 0.7             | 0.2            | 3.2           | 1.5           | 0.0            | 1.5           | 5.7            | 0.0            | 2.9           | 1.1              | 0.5            | 3.6           |
| J1719.3+1744  | 1.3               | 0.0            | 1.1           | 0.3             | 0.1            | 4.7           | 1.7           | 0.2            | 10.8          | 5.6            | 1.1            | 9.8           | 2.2              | 0.6            | 8.4           |
| J1721.0+0711  | 2.1               | 0.0            | 0.5           | 0.4             | 0.1            | 4.4           | 1.1           | 0.2            | 5.9           | 2.6            | 0.0            | 2.1           | 1.1              | 0.0            | 2.0           |
| J1721.5–0718c | 1.8               | 0.6            | 4.2           | 0.6             | 0.1            | 4.4           | 1.1           | 0.3            | 3.9           | 1.5            | 0.0            | 0.0           | 0.7              | 0.0            | 0.0           |
| J1722.5–0420  | 2.9               | 0.0            | 3.0           | 0.7             | 0.2            | 4.7           | 1.4           | 0.3            | 4.8           | 3.5            | 0.0            | 2.5           | 0.6              | 0.0            | 0.0           |
| J1722.7+1013  | 2.9               | 0.0            | 2.5           | 1.0             | 0.1            | 10.5          | 1.5           | 0.3            | 8.1           | 4.5            | 1.0            | 8.0           | 1.0              | 0.4            | 4.5           |
| J1724.0+4003  | 3.7               | 0.5            | 9.0           | 0.8             | 0.1            | 12.2          | 1.9           | 0.2            | 13.2          | 3.5            | 0.8            | 7.7           | 0.7              | 0.0            | 0.8           |
| J1724.9–0508c | 1.5               | 0.0            | 0.0           | 0.5             | 0.2            | 3.6           | 0.8           | 0.3            | 3.3           | 3.5            | 0.0            | 1.9           | 1.8              | 0.0            | 3.4           |
| J1725.0+1151  | 3.9               | 1.3            | 3.8           | 0.6             | 0.1            | 5.3           | 2.4           | 0.3            | 11.5          | 10.3           | 1.4            | 13.9          | 3.7              | 0.8            | 10.4          |
| J1725.1–7714  | 2.4               | 0.7            | 4.4           | 0.3             | 0.1            | 3.8           | 0.8           | 0.2            | 5.0           | 2.3            | 0.0            | 2.3           | 0.6              | 0.0            | 0.0           |
| J1725.2+5853  | 1.3               | 0.0            | 1.4           | 0.3             | 0.0            | 3.1           | 0.4           | 0.1            | 4.0           | 1.1            | 0.5            | 3.8           | 1.1              | 0.0            | 2.6           |
| J1726.6–3545  | 4.9               | 0.0            | 2.3           | 2.3             | 0.4            | 5.6           | 5.7           | 1.0            | 5.9           | 5.8            | 0.0            | 0.8           | 1.9              | 0.0            | 0.6           |
| J1727.1+4531  | 4.4               | 0.4            | 11.0          | 0.9             | 0.1            | 13.7          | 1.3           | 0.2            | 9.8           | 1.8            | 0.6            | 5.4           | 0.5              | 0.0            | 0.0           |
| J1727.1–0704  | 2.7               | 0.0            | 0.8           | 0.6             | 0.0            | 2.0           | 1.3           | 0.3            | 5.0           | 3.1            | 0.0            | 1.2           | 0.9              | 0.0            | 0.0           |
| J1727.3–4611  | 4.2               | 0.0            | 2.5           | 0.7             | 0.2            | 4.3           | 1.2           | 0.0            | 2.2           | 4.1            | 0.0            | 2.9           | 0.8              | 0.0            | 0.9           |
| J1727.6+0647  | 3.1               | 0.8            | 5.0           | 0.4             | 0.1            | 3.8           | 0.9           | 0.0            | 2.7           | 2.6            | 0.0            | 2.4           | 0.7              | 0.0            | 1.5           |
| J1727.8–2308  | 5.9               | 1.5            | 5.6           | 0.9             | 0.2            | 4.6           | 1.8           | 0.0            | 2.8           | 4.7            | 0.0            | 2.7           | 1.7              | 0.0            | 2.6           |
| J1727.9+1220  | 2.1               | 0.0            | 0.0           | 0.5             | 0.0            | 2.3           | 0.9           | 0.0            | 2.8           | 1.8            | 0.7            | 3.8           | 1.3              | 0.0            | 2.0           |
| J1728.0–2737c | 7.9               | 2.8            | 5.9           | 0.8             | 0.3            | 3.3           | 2.0           | 0.0            | 2.8           | 4.3            | 0.0            | 1.7           | 1.7              | 0.0            | 1.2           |
| J1728.2+5015  | 1.3               | 0.0            | 1.6           | 0.2             | 0.1            | 3.3           | 0.4           | 0.1            | 4.0           | 3.0            | 0.8            | 6.8           | 0.8              | 0.3            | 5.3           |
| J1728.2+0429  | 4.4               | 0.7            | 6.7           | 0.7             | 0.1            | 6.5           | 0.9           | 0.2            | 4.4           | 2.7            | 0.0            | 2.2           | 0.9              | 0.0            | 1.4           |
| J1729.5–0854  | 1.8               | 0.5            | 3.9           | 1.1             | 0.2            | 6.9           | 1.4           | 0.3            | 4.6           | 1.1            | 0.0            | 0.0           | 0.6              | 0.0            | 0.0           |
| J1730.5–3350  | 4.5               | 2.0            | 3.2           | 2.7             | 0.5            | 6.1           | 3.6           | 0.0            | 1.8           | 4.5            | 0.0            | 0.1           | 2.2              | 0.0            | 1.1           |
| J1730.6–2409  | 4.1               | 0.0            | 2.8           | 0.9             | 0.2            | 5.2           | 2.4           | 0.5            | 5.8           | 5.3            | 0.0            | 2.6           | 0.9              | 0.0            | 0.1           |
| J1730.6–0353  | 0.7               | 0.0            | 0.0           | 0.3             | 0.0            | 0.9           | 1.5           | 0.3            | 6.5           | 2.7            | 0.9            | 4.1           | 0.5              | 0.0            | 0.0           |
| J1730.7+0023  | 3.5               | 0.7            | 5.3           | 0.8             | 0.1            | 6.5           | 2.0           | 0.3            | 9.0           | 2.9            | 0.9            | 4.7           | 1.1              | 0.5            | 4.5           |
| J1730.8+5427  | 2.1               | 0.0            | 3.2           | 0.3             | 0.1            | 4.4           | 0.2           | 0.0            | 0.0           | 0.9            | 0.4            | 3.2           | 0.4              | 0.0            | 0.0           |
| J1731.3+3718  | 1.1               | 0.0            | 0.1           | 0.3             | 0.0            | 2.9           | 0.5           | 0.2            | 4.3           | 1.4            | 0.6            | 3.6           | 0.8              | 0.0            | 0.0           |
| J1731.6–3234c | 8.7               | 0.0            | 2.3           | 1.3             | 0.4            | 3.7           | 3.8           | 0.9            | 4.4           | 7.6            | 2.4            | 3.6           | 1.4              | 0.0            | 0.1           |
| J1731.8–3004  | 5.2               | 0.0            | 0.0           | 1.9             | 0.0            | 3.1           | 2.5           | 0.6            | 4.5           | 6.4            | 1.7            | 4.7           | 2.7              | 0.0            | 3.0           |

Table 1—Continued

|               | 100 MeV – 300 MeV |                |               | 300 MeV – 1 GeV |                |               | 1 GeV – 3 GeV |                |               | 3 GeV – 10 GeV |                |               | 10 GeV – 100 GeV |                |               |
|---------------|-------------------|----------------|---------------|-----------------|----------------|---------------|---------------|----------------|---------------|----------------|----------------|---------------|------------------|----------------|---------------|
| Name 2FGL     | $F_1^a$           | $\Delta F_1^a$ | $\sqrt{TS_1}$ | $F_2^a$         | $\Delta F_2^a$ | $\sqrt{TS_2}$ | $F_3^b$       | $\Delta F_3^b$ | $\sqrt{TS_3}$ | $F_4^c$        | $\Delta F_4^c$ | $\sqrt{TS_4}$ | $F_5^c$          | $\Delta F_5^c$ | $\sqrt{TS_5}$ |
| J1731.9–2703c | 8.9               | 0.0            | 1.3           | 1.5             | 0.3            | 5.9           | 1.6           | 0.5            | 3.6           | 5.0            | 1.6            | 4.1           | 2.2              | 0.0            | 2.4           |
| J1732.5–3131  | 10.3              | 4.5            | 6.8           | 6.5             | 0.4            | 19.0          | 31.3          | 1.2            | 34.8          | 57.8           | 4.0            | 21.6          | 2.7              | 0.0            | 2.5           |
| J1733.1–1307  | 6.7               | 0.8            | 9.0           | 1.6             | 0.2            | 10.4          | 2.6           | 0.4            | 8.5           | 5.0            | 1.2            | 5.9           | 1.0              | 0.0            | 0.1           |
| J1733.2–2913c | 12.3              | 0.0            | 0.7           | 1.8             | 0.0            | 3.0           | 2.7           | 0.0            | 3.1           | 4.6            | 1.7            | 3.5           | 1.9              | 0.8            | 3.3           |
| J1733.4–2812c | 12.1              | 0.0            | 2.4           | 1.4             | 0.4            | 4.8           | 2.1           | 0.0            | 2.2           | 4.4            | 1.5            | 3.5           | 2.4              | 0.0            | 2.8           |
| J1734.3+3858  | 4.6               | 0.6            | 11.3          | 1.3             | 0.1            | 18.7          | 2.8           | 0.3            | 17.9          | 6.7            | 1.1            | 12.0          | 0.8              | 0.4            | 4.0           |
| J1734.7–2533  | 4.5               | 1.2            | 6.0           | 2.2             | 0.3            | 8.7           | 1.6           | 0.5            | 3.3           | 3.2            | 0.0            | 0.5           | 0.8              | 0.0            | 0.0           |
| J1735.9+2033  | 0.5               | 0.0            | 0.0           | 0.1             | 0.0            | 0.4           | 0.4           | 0.2            | 3.5           | 2.9            | 0.8            | 6.5           | 1.8              | 0.5            | 7.6           |
| J1736.0–4443  | 4.6               | 0.9            | 5.4           | 0.5             | 0.2            | 3.7           | 1.9           | 0.3            | 7.1           | 5.1            | 1.2            | 6.5           | 0.7              | 0.0            | 0.0           |
| J1736.6+0626  | 3.5               | 0.7            | 5.4           | 0.4             | 0.1            | 3.6           | 0.7           | 0.2            | 3.7           | 1.5            | 0.0            | 0.4           | 1.2              | 0.0            | 1.1           |
| J1737.2–3213  | 7.8               | 0.0            | 1.0           | 3.1             | 0.5            | 7.3           | 3.9           | 1.0            | 4.2           | 9.3            | 2.6            | 4.1           | 1.9              | 0.0            | 0.2           |
| J1738.9+8716  | 1.2               | 0.0            | 1.3           | 0.4             | 0.1            | 6.0           | 1.0           | 0.2            | 7.8           | 2.8            | 0.7            | 7.4           | 0.7              | 0.3            | 4.2           |
| J1738.9–2908  | 8.6               | 2.4            | 6.4           | 4.2             | 0.5            | 10.8          | 7.1           | 0.9            | 8.6           | 7.8            | 0.0            | 2.3           | 2.0              | 0.0            | 2.0           |
| J1739.5+4955  | 2.2               | 0.0            | 3.0           | 0.5             | 0.1            | 7.6           | 0.9           | 0.2            | 7.9           | 1.4            | 0.6            | 3.9           | 1.5              | 0.0            | 3.9           |
| J1739.6–2726  | 3.5               | 1.7            | 3.2           | 3.2             | 0.3            | 10.6          | 5.2           | 0.7            | 8.4           | 4.8            | 1.7            | 3.4           | 0.9              | 0.0            | 0.0           |
| J1740.2+5212  | 5.7               | 0.5            | 14.4          | 1.4             | 0.1            | 19.8          | 2.0           | 0.2            | 14.1          | 2.7            | 0.7            | 6.5           | 1.2              | 0.0            | 3.5           |
| J1740.3+4738  | 1.5               | 0.0            | 1.9           | 0.3             | 0.0            | 3.0           | 0.6           | 0.0            | 2.9           | 1.1            | 0.5            | 3.8           | 1.5              | 0.0            | 3.8           |
| J1740.4–3054c | 7.0               | 3.1            | 3.4           | 2.1             | 0.6            | 4.2           | 7.6           | 1.1            | 7.3           | 16.2           | 3.3            | 5.9           | 1.8              | 0.0            | 0.4           |
| J1741.0+1347  | 0.9               | 0.0            | 0.0           | 0.2             | 0.0            | 0.8           | 0.7           | 0.0            | 2.3           | 2.9            | 0.0            | 2.9           | 1.3              | 0.0            | 2.3           |
| J1741.1–6750  | 2.5               | 0.0            | 2.5           | 0.3             | 0.1            | 3.4           | 0.8           | 0.0            | 3.1           | 2.3            | 0.0            | 2.6           | 0.4              | 0.0            | 0.0           |
| J1741.9–2054  | 11.4              | 1.2            | 12.8          | 6.0             | 0.2            | 30.9          | 15.2          | 0.7            | 31.2          | 8.1            | 1.5            | 7.8           | 1.1              | 0.0            | 0.9           |
| J1742.0–2540c | 8.6               | 0.0            | 2.8           | 1.8             | 0.3            | 6.4           | 2.2           | 0.5            | 4.5           | 4.6            | 0.0            | 1.4           | 2.8              | 0.0            | 2.7           |
| J1742.1+5948  | 1.7               | 0.4            | 4.7           | 0.2             | 0.0            | 2.2           | 0.4           | 0.1            | 4.4           | 1.9            | 0.0            | 2.8           | 1.1              | 0.0            | 3.8           |
| J1742.5–3323  | 4.8               | 0.0            | 0.7           | 1.4             | 0.3            | 5.1           | 5.5           | 0.7            | 9.3           | 4.4            | 1.6            | 3.2           | 1.6              | 0.0            | 0.5           |
| J1743.2–2304  | 8.0               | 1.5            | 6.0           | 1.6             | 0.2            | 7.0           | 1.5           | 0.4            | 3.7           | 5.9            | 0.0            | 2.8           | 1.2              | 0.0            | 0.6           |
| J1743.9–3039c | 7.0               | 0.0            | 0.0           | 4.6             | 0.0            | 1.9           | 5.1           | 0.0            | 2.3           | 8.9            | 2.7            | 3.9           | 4.3              | 0.0            | 3.1           |
| J1744.1+1934  | 0.7               | 0.0            | 0.0           | 0.1             | 0.0            | 0.2           | 0.4           | 0.2            | 3.5           | 2.3            | 0.8            | 5.3           | 1.8              | 0.0            | 3.5           |
| J1744.1–7620  | 1.4               | 0.0            | 2.7           | 0.6             | 0.1            | 8.7           | 3.2           | 0.3            | 15.9          | 6.5            | 1.2            | 10.3          | 0.5              | 0.0            | 0.0           |
| J1744.6–1135  | 3.8               | 0.8            | 5.2           | 1.5             | 0.2            | 10.2          | 4.3           | 0.5            | 11.9          | 4.0            | 1.2            | 4.6           | 1.4              | 0.0            | 2.1           |
| J1745.1–1729  | 4.2               | 0.0            | 2.2           | 0.6             | 0.0            | 1.7           | 1.4           | 0.4            | 4.8           | 2.8            | 1.1            | 3.3           | 1.3              | 0.6            | 3.3           |
| J1745.5–0751  | 2.4               | 0.0            | 1.0           | 0.2             | 0.0            | 0.0           | 0.9           | 0.3            | 3.3           | 2.9            | 1.1            | 3.8           | 1.3              | 0.5            | 4.7           |
| J1745.5–3028c | 10.8              | 0.0            | 0.0           | 3.5             | 0.0            | 0.6           | 4.9           | 1.3            | 4.0           | 8.3            | 2.8            | 3.4           | 2.4              | 1.0            | 3.2           |
| J1745.6+1015  | 2.7               | 0.0            | 1.9           | 0.5             | 0.1            | 5.1           | 1.0           | 0.2            | 5.4           | 2.8            | 0.9            | 5.0           | 0.5              | 0.0            | 0.0           |
| J1745.6+0203  | 2.5               | 0.0            | 0.7           | 0.6             | 0.0            | 2.5           | 1.1           | 0.0            | 2.6           | 3.1            | 0.0            | 2.7           | 1.1              | 0.0            | 1.7           |
| J1745.6–2858  | 40.2              | 5.1            | 8.2           | 22.0            | 1.9            | 13.2          | 63.1          | 2.7            | 24.8          | 114.5          | 7.3            | 19.7          | 13.2             | 2.0            | 9.5           |
| J1746.0+2316  | 2.0               | 0.5            | 3.9           | 0.3             | 0.1            | 3.6           | 0.4           | 0.0            | 0.8           | 1.3            | 0.0            | 0.0           | 0.5              | 0.0            | 0.0           |
| J1746.5–3238  | 7.4               | 2.5            | 6.2           | 3.6             | 0.4            | 12.5          | 8.9           | 0.8            | 14.5          | 11.0           | 2.1            | 7.1           | 1.7              | 0.0            | 1.3           |
| J1746.6–2851c | 6.2               | 0.0            | 0.0           | 7.9             | 0.0            | 1.3           | 10.9          | 0.0            | 2.2           | 29.1           | 5.8            | 5.7           | 3.4              | 1.3            | 3.4           |
| J1747.1–3000  | 23.5              | 6.5            | 3.6           | 10.8            | 0.9            | 12.8          | 20.5          | 1.3            | 18.1          | 27.3           | 3.4            | 10.5          | 2.2              | 0.8            | 3.6           |
| J1747.2–3507  | 7.3               | 1.5            | 5.8           | 0.8             | 0.2            | 3.5           | 1.4           | 0.4            | 3.6           | 4.2            | 0.0            | 1.9           | 1.3              | 0.0            | 1.5           |
| J1747.3–2825c | 3.4               | 0.0            | 0.0           | 2.2             | 0.6            | 3.5           | 11.1          | 1.6            | 7.2           | 25.7           | 4.4            | 6.7           | 2.2              | 0.0            | 0.1           |
| J1747.5–4036  | 3.9               | 0.0            | 1.5           | 0.7             | 0.0            | 3.0           | 1.3           | 0.3            | 4.9           | 2.7            | 1.0            | 3.7           | 1.0              | 0.0            | 0.7           |
| J1747.6+0324  | 2.4               | 1.2            | 3.6           | 0.6             | 0.0            | 2.9           | 0.8           | 0.3            | 3.8           | 2.4            | 0.9            | 3.9           | 1.2              | 0.0            | 1.9           |
| J1748.0–2447  | 8.9               | 1.4            | 8.0           | 3.3             | 0.3            | 12.4          | 9.3           | 0.8            | 15.2          | 19.1           | 2.4            | 11.4          | 1.4              | 0.6            | 3.7           |

Table 1—Continued

|               | 100 MeV – 300 MeV |                |               | 300 MeV – 1 GeV |                |               | 1 GeV – 3 GeV |                |               | 3 GeV – 10 GeV |                |               | 10 GeV – 100 GeV |                |               |
|---------------|-------------------|----------------|---------------|-----------------|----------------|---------------|---------------|----------------|---------------|----------------|----------------|---------------|------------------|----------------|---------------|
| Name 2FGL     | $F_1^a$           | $\Delta F_1^a$ | $\sqrt{TS_1}$ | $F_2^a$         | $\Delta F_2^a$ | $\sqrt{TS_2}$ | $F_3^b$       | $\Delta F_3^b$ | $\sqrt{TS_3}$ | $F_4^c$        | $\Delta F_4^c$ | $\sqrt{TS_4}$ | $F_5^c$          | $\Delta F_5^c$ | $\sqrt{TS_5}$ |
| J1748.6–2913  | 19.1              | 0.0            | 2.4           | 4.3             | 0.9            | 5.4           | 11.3          | 1.3            | 9.4           | 12.2           | 2.9            | 5.0           | 3.4              | 0.0            | 2.4           |
| J1748.7–2020  | 9.6               | 1.6            | 7.3           | 1.9             | 0.2            | 8.3           | 1.8           | 0.5            | 4.5           | 3.5            | 1.3            | 3.5           | 1.4              | 0.0            | 1.4           |
| J1748.8+3418  | 2.2               | 0.0            | 3.0           | 0.2             | 0.1            | 3.5           | 0.5           | 0.1            | 4.5           | 2.2            | 0.0            | 2.5           | 1.3              | 0.0            | 1.5           |
| J1748.8+7006  | 1.8               | 0.5            | 5.1           | 0.5             | 0.1            | 9.3           | 1.5           | 0.2            | 11.8          | 5.5            | 0.9            | 11.8          | 1.0              | 0.4            | 7.0           |
| J1748.9–3923  | 4.8               | 0.0            | 2.1           | 0.5             | 0.0            | 1.1           | 1.4           | 0.3            | 4.8           | 4.5            | 0.0            | 3.0           | 1.6              | 0.0            | 1.9           |
| J1749.1+0515  | 2.4               | 0.9            | 3.5           | 0.4             | 0.1            | 3.2           | 0.9           | 0.0            | 2.3           | 2.1            | 0.0            | 1.6           | 1.1              | 0.0            | 1.4           |
| J1749.1+4323  | 1.7               | 0.4            | 4.5           | 0.4             | 0.1            | 6.1           | 1.1           | 0.2            | 8.7           | 2.2            | 0.7            | 5.7           | 1.4              | 0.0            | 4.6           |
| J1749.7–3134c | 7.6               | 0.0            | 0.7           | 1.5             | 0.4            | 4.8           | 2.8           | 0.0            | 2.8           | 7.8            | 0.0            | 3.0           | 1.5              | 0.0            | 0.6           |
| J1751.5+0938  | 4.1               | 0.7            | 7.9           | 1.7             | 0.1            | 15.9          | 3.4           | 0.3            | 15.0          | 7.6            | 1.3            | 10.4          | 1.4              | 0.5            | 5.9           |
| J1753.8–5012  | 2.9               | 0.6            | 5.5           | 0.9             | 0.1            | 8.0           | 1.5           | 0.3            | 7.0           | 3.4            | 0.0            | 2.6           | 0.6              | 0.0            | 0.0           |
| J1753.8–4446  | 1.3               | 0.0            | 0.0           | 0.4             | 0.1            | 3.5           | 1.0           | 0.3            | 4.6           | 3.5            | 0.0            | 2.5           | 1.0              | 0.0            | 1.3           |
| J1754.1–2930  | 10.7              | 0.0            | 3.9           | 2.2             | 0.4            | 7.2           | 2.7           | 0.6            | 4.6           | 6.8            | 0.0            | 2.8           | 0.8              | 0.0            | 0.0           |
| J1754.3+3212  | 2.2               | 0.5            | 5.5           | 0.4             | 0.1            | 6.7           | 1.8           | 0.2            | 12.6          | 6.4            | 1.1            | 11.4          | 1.7              | 0.5            | 7.5           |
| J1754.4–2538c | 1.0               | 0.0            | 0.0           | 0.5             | 0.0            | 0.0           | 4.0           | 0.9            | 4.6           | 11.9           | 0.0            | 3.0           | 1.8              | 0.0            | 0.5           |
| J1755.5–6423  | 2.8               | 0.0            | 3.0           | 0.4             | 0.0            | 2.8           | 0.7           | 0.0            | 2.4           | 1.3            | 0.0            | 0.7           | 1.1              | 0.0            | 2.6           |
| J1756.5+5523  | 1.3               | 0.0            | 1.7           | 0.2             | 0.0            | 2.1           | 0.4           | 0.0            | 1.6           | 1.7            | 0.6            | 4.7           | 0.8              | 0.4            | 4.7           |
| J1757.5–6028  | 1.1               | 0.0            | 0.3           | 0.2             | 0.0            | 0.9           | 0.5           | 0.2            | 4.0           | 2.2            | 0.7            | 5.0           | 0.7              | 0.0            | 1.3           |
| J1758.8–2402c | 10.1              | 0.0            | 1.4           | 2.7             | 0.7            | 4.1           | 5.0           | 1.2            | 4.4           | 13.1           | 3.1            | 4.9           | 3.5              | 0.0            | 2.4           |
| J1759.2–3853  | 2.1               | 0.0            | 0.0           | 0.7             | 0.0            | 2.5           | 1.1           | 0.3            | 3.9           | 2.9            | 1.0            | 3.9           | 0.8              | 0.0            | 0.0           |
| J1759.2–4819  | 2.1               | 0.0            | 1.2           | 0.5             | 0.1            | 4.6           | 1.0           | 0.2            | 5.0           | 4.0            | 1.1            | 6.0           | 1.1              | 0.0            | 1.5           |
| J1759.4–2954  | 4.9               | 2.2            | 3.6           | 0.9             | 0.3            | 3.7           | 1.7           | 0.5            | 3.9           | 4.7            | 0.0            | 1.9           | 2.1              | 0.0            | 1.9           |
| J1759.5–0521  | 4.1               | 1.1            | 3.9           | 0.6             | 0.2            | 3.3           | 1.2           | 0.0            | 1.2           | 3.7            | 0.0            | 1.6           | 1.5              | 0.0            | 1.9           |
| J1800.5+7829  | 5.8               | 0.4            | 16.5          | 1.4             | 0.1            | 22.3          | 3.3           | 0.3            | 22.6          | 8.6            | 1.1            | 17.2          | 2.7              | 0.6            | 11.5          |
| J1800.8–2400  | 10.4              | 0.0            | 0.0           | 2.2             | 0.0            | 0.6           | 6.2           | 1.2            | 5.4           | 20.0           | 3.5            | 7.2           | 3.2              | 1.1            | 3.9           |
| J1801.3–2326e | 24.7              | 3.9            | 7.1           | 19.4            | 0.7            | 28.7          | 43.7          | 1.7            | 30.9          | 83.8           | 5.6            | 19.1          | 11.0             | 1.9            | 7.7           |
| J1801.7+4405  | 1.6               | 0.5            | 3.8           | 0.3             | 0.1            | 4.5           | 0.5           | 0.1            | 4.1           | 1.1            | 0.0            | 0.6           | 0.6              | 0.0            | 0.0           |
| J1802.3–2445c | 6.6               | 1.8            | 3.8           | 11.3            | 0.0            | 3.7           | 5.1           | 0.0            | 3.1           | 7.1            | 0.0            | 1.7           | 2.6              | 0.0            | 2.2           |
| J1802.6–3940  | 16.9              | 1.1            | 23.7          | 6.3             | 0.2            | 42.8          | 12.9          | 0.6            | 36.8          | 30.2           | 2.5            | 24.2          | 4.7              | 0.9            | 11.7          |
| J1802.8–6706  | 2.3               | 0.0            | 2.5           | 0.3             | 0.0            | 2.1           | 0.5           | 0.2            | 4.1           | 2.0            | 0.0            | 2.2           | 0.7              | 0.0            | 1.0           |
| J1803.3–2148  | 16.1              | 3.4            | 4.5           | 4.5             | 0.7            | 7.1           | 11.3          | 1.3            | 9.8           | 25.5           | 3.5            | 9.3           | 2.3              | 0.9            | 3.5           |
| J1803.6+2523c | 2.4               | 0.6            | 4.6           | 0.3             | 0.1            | 3.6           | 0.6           | 0.0            | 1.8           | 1.0            | 0.0            | 0.0           | 0.7              | 0.0            | 0.0           |
| J1805.0–0845  | 5.6               | 1.2            | 4.9           | 0.9             | 0.0            | 2.4           | 1.8           | 0.0            | 2.6           | 4.6            | 0.0            | 2.6           | 1.9              | 0.0            | 2.3           |
| J1805.6–2136e | 9.3               | 0.0            | 0.0           | 7.7             | 0.7            | 11.4          | 24.3          | 1.6            | 17.3          | 43.9           | 4.8            | 10.8          | 8.2              | 1.7            | 5.9           |
| J1805.8+0612  | 2.0               | 0.0            | 0.5           | 0.3             | 0.1            | 3.4           | 1.2           | 0.3            | 5.9           | 3.3            | 1.0            | 5.2           | 0.8              | 0.0            | 0.8           |
| J1806.7+6948  | 3.8               | 0.6            | 10.5          | 1.2             | 0.1            | 19.0          | 3.2           | 0.3            | 20.8          | 7.5            | 1.0            | 14.5          | 1.7              | 0.5            | 8.0           |
| J1807.7–0419  | 3.3               | 0.8            | 4.4           | 0.9             | 0.2            | 4.1           | 1.4           | 0.0            | 1.4           | 1.4            | 0.0            | 0.0           | 1.1              | 0.0            | 1.7           |
| J1808.3–3356  | 2.8               | 0.9            | 3.2           | 0.6             | 0.0            | 2.3           | 1.7           | 0.3            | 6.1           | 4.5            | 0.0            | 2.7           | 0.7              | 0.0            | 0.0           |
| J1808.5–2037c | 10.6              | 2.1            | 5.4           | 3.9             | 0.6            | 6.6           | 4.5           | 0.0            | 2.5           | 9.7            | 2.7            | 4.2           | 1.4              | 0.0            | 0.0           |
| J1808.6–1950c | 4.9               | 0.0            | 0.0           | 2.7             | 0.6            | 4.9           | 6.7           | 1.1            | 6.5           | 9.3            | 2.9            | 3.7           | 3.7              | 0.0            | 2.3           |
| J1809.4+2042  | 2.5               | 0.0            | 2.9           | 0.4             | 0.0            | 2.8           | 0.2           | 0.0            | 0.0           | 1.9            | 0.7            | 3.7           | 1.4              | 0.0            | 4.3           |
| J1809.7+2909  | 1.4               | 0.5            | 3.3           | 0.3             | 0.1            | 4.5           | 0.5           | 0.2            | 3.8           | 3.1            | 0.8            | 6.8           | 1.3              | 0.5            | 5.7           |
| J1809.8–2332  | 32.0              | 2.6            | 13.7          | 18.1            | 0.4            | 47.0          | 57.3          | 1.3            | 70.2          | 108.0          | 4.7            | 44.0          | 5.3              | 1.0            | 9.7           |
| J1810.7+1742  | 3.3               | 0.6            | 7.0           | 1.1             | 0.1            | 11.5          | 2.2           | 0.3            | 10.9          | 2.5            | 0.8            | 4.8           | 0.5              | 0.0            | 0.0           |
| J1810.8+1606  | 2.1               | 0.0            | 1.3           | 0.4             | 0.1            | 3.8           | 0.6           | 0.2            | 3.4           | 2.8            | 0.9            | 5.0           | 1.5              | 0.0            | 2.6           |



Table 1—Continued

|               | 100 MeV – 300 MeV |                |               | 300 MeV – 1 GeV |                |               | 1 GeV – 3 GeV |                |               | 3 GeV – 10 GeV |                |               | 10 GeV – 100 GeV |                |               |
|---------------|-------------------|----------------|---------------|-----------------|----------------|---------------|---------------|----------------|---------------|----------------|----------------|---------------|------------------|----------------|---------------|
| Name 2FGL     | $F_1^a$           | $\Delta F_1^a$ | $\sqrt{TS_1}$ | $F_2^a$         | $\Delta F_2^a$ | $\sqrt{TS_2}$ | $F_3^b$       | $\Delta F_3^b$ | $\sqrt{TS_3}$ | $F_4^c$        | $\Delta F_4^c$ | $\sqrt{TS_4}$ | $F_5^c$          | $\Delta F_5^c$ | $\sqrt{TS_5}$ |
| J1811.0+5340  | 0.8               | 0.0            | 0.1           | 0.2             | 0.0            | 2.0           | 0.5           | 0.2            | 4.2           | 1.4            | 0.5            | 4.4           | 1.2              | 0.0            | 3.2           |
| J1811.1–1905c | 8.2               | 1.8            | 4.8           | 3.3             | 0.6            | 6.2           | 4.6           | 0.0            | 2.8           | 8.3            | 2.5            | 3.8           | 3.0              | 0.0            | 2.3           |
| J1811.3–2421  | 5.1               | 1.5            | 3.7           | 1.8             | 0.4            | 4.9           | 2.3           | 0.6            | 3.9           | 4.7            | 0.0            | 1.4           | 1.0              | 0.0            | 0.0           |
| J1811.3+0339  | 1.3               | 0.0            | 0.0           | 0.2             | 0.0            | 0.0           | 0.9           | 0.0            | 2.2           | 3.8            | 1.0            | 5.9           | 1.1              | 0.5            | 4.8           |
| J1813.4–1246  | 36.6              | 2.1            | 24.4          | 11.3            | 0.4            | 36.7          | 21.8          | 0.9            | 32.9          | 30.9           | 2.8            | 17.5          | 1.5              | 0.6            | 3.3           |
| J1813.5+3143  | 1.6               | 0.5            | 3.8           | 0.4             | 0.1            | 6.3           | 1.5           | 0.2            | 9.7           | 2.7            | 0.8            | 5.7           | 1.6              | 0.5            | 6.5           |
| J1813.6–2821  | 3.9               | 1.1            | 3.8           | 0.5             | 0.0            | 0.7           | 1.1           | 0.3            | 3.5           | 3.9            | 0.0            | 2.5           | 0.9              | 0.0            | 0.0           |
| J1813.7–1139c | 6.3               | 1.3            | 6.8           | 2.3             | 0.4            | 7.5           | 2.1           | 0.6            | 3.8           | 5.0            | 1.6            | 3.9           | 0.9              | 0.0            | 0.0           |
| J1813.7+0617  | 1.9               | 0.0            | 0.2           | 0.3             | 0.0            | 0.9           | 1.2           | 0.3            | 6.1           | 3.4            | 0.0            | 2.8           | 1.8              | 0.0            | 3.1           |
| J1814.1–1735c | 9.6               | 0.0            | 3.1           | 3.4             | 0.5            | 7.5           | 7.1           | 1.2            | 6.6           | 9.7            | 3.0            | 3.7           | 1.4              | 0.0            | 0.0           |
| J1815.6–6407  | 1.7               | 0.7            | 3.4           | 0.4             | 0.1            | 4.7           | 0.8           | 0.0            | 3.1           | 2.5            | 0.0            | 3.1           | 0.5              | 0.0            | 0.0           |
| J1816.5+4511  | 1.5               | 0.0            | 1.7           | 0.3             | 0.1            | 5.6           | 1.3           | 0.2            | 9.6           | 2.4            | 0.8            | 5.3           | 1.3              | 0.0            | 3.3           |
| J1816.7–4942  | 1.5               | 0.0            | 0.8           | 0.5             | 0.1            | 5.8           | 1.1           | 0.2            | 6.3           | 1.4            | 0.6            | 3.3           | 1.2              | 0.0            | 1.9           |
| J1817.6–1651c | 7.9               | 0.0            | 2.5           | 1.8             | 0.5            | 3.7           | 4.4           | 0.0            | 2.4           | 12.0           | 0.0            | 2.7           | 2.6              | 0.0            | 1.3           |
| J1818.6+0903  | 4.8               | 0.0            | 1.7           | 0.8             | 0.1            | 5.8           | 1.4           | 0.3            | 6.2           | 1.8            | 0.8            | 3.4           | 1.1              | 0.5            | 4.6           |
| J1818.7+2138  | 2.1               | 0.0            | 1.8           | 0.3             | 0.0            | 1.7           | 0.7           | 0.0            | 2.1           | 2.5            | 0.0            | 3.0           | 1.0              | 0.0            | 2.1           |
| J1819.3–1523  | 10.8              | 2.1            | 7.3           | 6.4             | 0.5            | 14.3          | 7.1           | 1.1            | 7.2           | 9.6            | 2.6            | 4.3           | 1.8              | 0.0            | 0.8           |
| J1820.6+3625  | 1.6               | 0.0            | 2.3           | 0.1             | 0.0            | 0.3           | 0.4           | 0.0            | 1.9           | 1.8            | 0.0            | 2.1           | 0.8              | 0.4            | 5.1           |
| J1820.6–3219  | 1.2               | 0.0            | 0.0           | 0.6             | 0.0            | 2.3           | 1.1           | 0.3            | 4.4           | 2.4            | 1.0            | 3.3           | 1.0              | 0.0            | 0.0           |
| J1821.8+0830  | 6.5               | 0.0            | 2.6           | 0.6             | 0.0            | 2.5           | 0.7           | 0.3            | 3.5           | 3.2            | 0.0            | 2.2           | 1.0              | 0.0            | 1.3           |
| J1823.1–1338c | 20.2              | 0.0            | 2.9           | 3.1             | 0.9            | 3.7           | 7.6           | 1.4            | 5.7           | 23.2           | 3.8            | 7.4           | 4.1              | 0.0            | 2.1           |
| J1823.4–3014  | 3.3               | 0.0            | 1.7           | 0.6             | 0.1            | 4.8           | 1.0           | 0.3            | 3.8           | 4.2            | 0.0            | 2.5           | 2.1              | 0.0            | 3.1           |
| J1823.6–3453  | 0.9               | 0.0            | 0.0           | 0.3             | 0.0            | 1.4           | 1.1           | 0.3            | 5.1           | 5.3            | 1.2            | 7.5           | 2.2              | 0.6            | 8.1           |
| J1823.7+6856  | 1.5               | 0.5            | 3.9           | 0.3             | 0.1            | 5.9           | 0.6           | 0.2            | 5.0           | 1.8            | 0.5            | 5.7           | 0.5              | 0.0            | 0.0           |
| J1823.8+4312  | 1.8               | 0.0            | 2.3           | 0.2             | 0.1            | 3.4           | 0.7           | 0.0            | 2.9           | 1.4            | 0.0            | 1.6           | 0.9              | 0.0            | 2.2           |
| J1824.0+5650  | 5.6               | 0.5            | 12.5          | 1.2             | 0.1            | 16.4          | 2.3           | 0.2            | 15.2          | 3.9            | 0.8            | 8.5           | 0.9              | 0.0            | 2.3           |
| J1824.5–1351e | 16.6              | 0.0            | 0.0           | 7.4             | 0.0            | 2.9           | 9.3           | 2.5            | 3.8           | 30.6           | 7.8            | 4.1           | 23.3             | 3.3            | 8.8           |
| J1824.5+1013  | 2.8               | 0.0            | 0.4           | 0.5             | 0.0            | 2.6           | 0.9           | 0.0            | 2.5           | 2.9            | 0.9            | 5.1           | 0.9              | 0.0            | 1.4           |
| J1824.8–2449  | 3.1               | 1.1            | 4.2           | 1.1             | 0.2            | 6.9           | 2.4           | 0.4            | 7.3           | 3.2            | 1.1            | 3.9           | 0.6              | 0.0            | 0.0           |
| J1825.1–5231  | 2.0               | 0.0            | 3.0           | 0.7             | 0.1            | 9.5           | 2.0           | 0.3            | 10.7          | 2.6            | 0.9            | 4.7           | 1.6              | 0.0            | 3.2           |
| J1826.1–1256  | 29.5              | 3.8            | 9.7           | 14.8            | 0.6            | 27.3          | 45.1          | 1.6            | 37.2          | 62.1           | 4.5            | 19.6          | 3.1              | 0.0            | 1.8           |
| J1826.3–1450  | 35.7              | 5.0            | 5.4           | 10.8            | 0.9            | 10.8          | 18.1          | 1.5            | 13.8          | 24.0           | 3.3            | 9.4           | 4.3              | 0.0            | 2.9           |
| J1827.4–0846  | 5.4               | 0.0            | 0.7           | 1.7             | 0.4            | 4.9           | 2.5           | 0.6            | 4.3           | 4.8            | 1.7            | 3.6           | 2.7              | 0.0            | 3.1           |
| J1827.4–1445c | 19.3              | 0.0            | 0.0           | 1.6             | 0.0            | 0.0           | 5.1           | 0.0            | 2.5           | 12.3           | 0.0            | 3.1           | 1.7              | 0.8            | 3.2           |
| J1827.6+1149  | 4.0               | 0.0            | 2.0           | 0.6             | 0.0            | 2.8           | 0.7           | 0.2            | 3.4           | 1.9            | 0.8            | 3.6           | 1.0              | 0.0            | 0.5           |
| J1828.3–1124c | 7.0               | 0.0            | 3.0           | 3.4             | 0.5            | 7.8           | 4.7           | 0.0            | 2.6           | 5.7            | 0.0            | 0.4           | 1.0              | 0.0            | 0.0           |
| J1828.7+3231  | 1.5               | 0.0            | 0.9           | 0.4             | 0.0            | 2.8           | 0.7           | 0.2            | 4.6           | 2.7            | 0.0            | 3.1           | 0.6              | 0.0            | 0.0           |
| J1829.1+2725  | 2.5               | 0.6            | 4.7           | 0.6             | 0.1            | 6.2           | 0.5           | 0.2            | 3.3           | 2.5            | 0.0            | 2.4           | 0.8              | 0.0            | 1.0           |
| J1829.1–0340c | 3.2               | 0.0            | 0.0           | 0.9             | 0.0            | 1.0           | 1.7           | 0.6            | 3.4           | 6.0            | 1.8            | 4.3           | 0.6              | 0.0            | 0.0           |
| J1829.2+5402  | 1.1               | 0.0            | 1.0           | 0.3             | 0.0            | 2.6           | 0.5           | 0.1            | 4.8           | 1.9            | 0.6            | 5.5           | 1.3              | 0.0            | 4.1           |
| J1829.3–2419  | 3.9               | 1.5            | 4.2           | 0.6             | 0.0            | 2.0           | 0.9           | 0.3            | 3.5           | 3.6            | 0.0            | 1.8           | 1.7              | 0.6            | 5.1           |
| J1829.7+4846  | 1.8               | 0.5            | 4.5           | 0.7             | 0.1            | 10.0          | 1.1           | 0.2            | 7.9           | 1.4            | 0.6            | 3.7           | 0.8              | 0.0            | 1.6           |
| J1829.8–0204c | 2.5               | 0.0            | 0.0           | 1.7             | 0.0            | 2.2           | 3.0           | 0.6            | 5.5           | 5.4            | 1.7            | 4.1           | 2.0              | 0.0            | 2.1           |
| J1830.0+1325  | 3.3               | 0.0            | 1.8           | 0.4             | 0.0            | 1.7           | 0.7           | 0.2            | 3.2           | 1.5            | 0.7            | 3.3           | 1.8              | 0.0            | 2.9           |

Table 1—Continued

|               | 100 MeV – 300 MeV |                |               | 300 MeV – 1 GeV |                |               | 1 GeV – 3 GeV |                |               | 3 GeV – 10 GeV |                |               | 10 GeV – 100 GeV |                |               |
|---------------|-------------------|----------------|---------------|-----------------|----------------|---------------|---------------|----------------|---------------|----------------|----------------|---------------|------------------|----------------|---------------|
| Name 2FGL     | $F_1^a$           | $\Delta F_1^a$ | $\sqrt{TS_1}$ | $F_2^a$         | $\Delta F_2^a$ | $\sqrt{TS_2}$ | $F_3^b$       | $\Delta F_3^b$ | $\sqrt{TS_3}$ | $F_4^c$        | $\Delta F_4^c$ | $\sqrt{TS_4}$ | $F_5^c$          | $\Delta F_5^c$ | $\sqrt{TS_5}$ |
| J1830.1+0617  | 2.9               | 0.0            | 1.5           | 0.6             | 0.1            | 4.1           | 2.3           | 0.4            | 8.3           | 7.2            | 1.4            | 8.1           | 1.6              | 0.0            | 3.1           |
| J1830.2–4441  | 2.0               | 0.6            | 3.4           | 1.0             | 0.1            | 10.3          | 1.3           | 0.2            | 7.5           | 1.8            | 0.7            | 3.5           | 0.6              | 0.0            | 0.0           |
| J1830.4–1634  | 12.3              | 2.5            | 8.1           | 1.0             | 0.3            | 3.9           | 1.2           | 0.4            | 3.2           | 4.0            | 1.3            | 3.9           | 1.7              | 0.0            | 1.4           |
| J1830.9–3132  | 1.9               | 0.0            | 0.4           | 0.2             | 0.0            | 0.0           | 1.0           | 0.0            | 2.1           | 3.1            | 1.0            | 4.4           | 0.9              | 0.0            | 1.2           |
| J1831.2–1518  | 7.7               | 3.7            | 4.6           | 1.8             | 0.4            | 6.2           | 2.6           | 0.0            | 3.1           | 2.5            | 0.0            | 0.0           | 3.0              | 0.0            | 2.5           |
| J1832.0–0200  | 5.9               | 1.0            | 5.0           | 2.7             | 0.5            | 6.1           | 2.2           | 0.6            | 3.9           | 5.2            | 0.0            | 1.5           | 2.9              | 0.0            | 3.0           |
| J1832.2–6502  | 1.0               | 0.0            | 0.0           | 0.1             | 0.0            | 0.0           | 0.6           | 0.2            | 4.8           | 2.4            | 0.8            | 5.1           | 0.5              | 0.0            | 0.0           |
| J1832.7–5700  | 2.0               | 0.6            | 4.0           | 0.3             | 0.0            | 1.9           | 0.8           | 0.2            | 4.8           | 1.6            | 0.6            | 3.8           | 0.9              | 0.0            | 1.1           |
| J1833.1–0437c | 6.9               | 1.6            | 5.5           | 1.3             | 0.4            | 3.8           | 2.8           | 0.0            | 2.8           | 5.5            | 1.6            | 4.3           | 1.1              | 0.0            | 0.0           |
| J1833.6–1032  | 5.1               | 2.1            | 3.3           | 3.7             | 0.4            | 10.3          | 7.9           | 1.0            | 9.0           | 8.8            | 2.3            | 4.5           | 2.3              | 0.0            | 1.4           |
| J1833.6–2104  | 40.5              | 1.2            | 38.5          | 7.9             | 0.2            | 40.4          | 10.6          | 0.6            | 26.4          | 10.4           | 1.6            | 10.3          | 2.1              | 0.6            | 6.1           |
| J1834.3–0848  | 5.4               | 2.3            | 3.3           | 3.6             | 0.5            | 8.1           | 7.7           | 1.2            | 7.0           | 18.0           | 3.5            | 6.0           | 3.2              | 1.1            | 3.7           |
| J1834.7–0705c | 4.4               | 0.0            | 0.0           | 4.9             | 0.8            | 5.0           | 8.1           | 1.3            | 6.5           | 9.3            | 3.1            | 3.5           | 6.7              | 1.5            | 6.8           |
| J1835.4+1036  | 4.3               | 0.0            | 3.2           | 0.5             | 0.0            | 2.1           | 1.1           | 0.0            | 2.7           | 3.0            | 0.0            | 2.6           | 0.9              | 0.0            | 1.0           |
| J1835.4+1349  | 2.5               | 1.1            | 3.4           | 0.4             | 0.1            | 3.5           | 1.1           | 0.0            | 2.4           | 3.0            | 0.0            | 2.6           | 1.3              | 0.0            | 2.3           |
| J1835.5–0649  | 5.9               | 0.0            | 0.0           | 2.4             | 0.0            | 0.0           | 5.1           | 0.0            | 1.9           | 13.7           | 3.2            | 5.1           | 3.6              | 1.3            | 3.6           |
| J1835.6–3258  | 0.5               | 0.0            | 0.0           | 0.3             | 0.0            | 2.9           | 1.3           | 0.3            | 5.8           | 2.0            | 0.8            | 3.5           | 0.5              | 0.0            | 0.0           |
| J1836.2+5926  | 29.7              | 0.6            | 79.3          | 21.9            | 0.2            | 190.7         | 83.9          | 1.1            | 192.1         | 139.0          | 4.1            | 94.5          | 2.9              | 0.6            | 12.0          |
| J1836.2+3137  | 2.5               | 0.0            | 1.6           | 0.3             | 0.1            | 3.9           | 0.6           | 0.2            | 4.0           | 2.5            | 0.0            | 2.1           | 1.4              | 0.0            | 2.9           |
| J1836.8–0623c | 18.0              | 0.0            | 0.9           | 3.7             | 0.0            | 2.4           | 6.6           | 1.2            | 5.7           | 10.2           | 3.0            | 3.8           | 3.4              | 1.2            | 3.9           |
| J1837.3–0700c | 10.2              | 3.9            | 3.5           | 2.7             | 0.7            | 4.0           | 6.6           | 1.3            | 5.5           | 14.1           | 0.0            | 2.8           | 4.4              | 0.0            | 2.6           |
| J1837.9+3821  | 1.8               | 0.5            | 4.0           | 0.3             | 0.0            | 2.1           | 0.7           | 0.0            | 2.7           | 1.5            | 0.0            | 1.5           | 0.4              | 0.0            | 0.0           |
| J1838.7+4759  | 1.7               | 0.0            | 2.2           | 0.3             | 0.0            | 2.2           | 0.5           | 0.2            | 4.5           | 4.5            | 0.9            | 9.2           | 1.6              | 0.5            | 6.5           |
| J1839.0–0102  | 3.6               | 1.1            | 3.3           | 1.6             | 0.4            | 4.4           | 1.7           | 0.0            | 1.1           | 5.4            | 0.0            | 2.3           | 1.6              | 0.0            | 2.2           |
| J1839.0–0539  | 43.5              | 0.0            | 1.4           | 11.1            | 1.2            | 10.1          | 22.2          | 1.7            | 14.6          | 55.7           | 4.8            | 15.7          | 4.4              | 0.0            | 2.4           |
| J1839.3–0558c | 33.3              | 0.0            | 0.9           | 4.6             | 0.0            | 2.2           | 10.6          | 1.6            | 6.8           | 18.1           | 3.9            | 5.4           | 2.6              | 0.0            | 0.9           |
| J1839.7–0334c | 6.8               | 2.2            | 4.3           | 1.9             | 0.6            | 3.4           | 2.7           | 0.8            | 3.7           | 5.8            | 0.0            | 1.5           | 1.7              | 0.0            | 1.4           |
| J1840.3–0413c | 4.4               | 0.0            | 0.0           | 3.7             | 0.0            | 2.7           | 4.4           | 1.0            | 4.8           | 10.7           | 0.0            | 2.6           | 3.5              | 0.0            | 2.2           |
| J1841.2–0459c | 14.9              | 0.0            | 1.3           | 2.7             | 0.6            | 4.6           | 7.8           | 1.1            | 7.9           | 18.5           | 3.2            | 7.1           | 2.9              | 0.0            | 0.9           |
| J1841.7+3221  | 3.2               | 0.0            | 2.9           | 0.4             | 0.1            | 5.2           | 0.7           | 0.2            | 4.6           | 2.8            | 0.8            | 5.5           | 1.5              | 0.5            | 6.5           |
| J1842.3+2740  | 2.8               | 0.0            | 2.7           | 0.4             | 0.0            | 2.8           | 0.6           | 0.2            | 3.6           | 2.0            | 0.8            | 4.0           | 0.8              | 0.0            | 0.7           |
| J1842.3–5839  | 1.4               | 0.0            | 0.9           | 0.2             | 0.0            | 0.7           | 0.6           | 0.0            | 2.4           | 2.3            | 0.7            | 5.2           | 1.6              | 0.0            | 3.1           |
| J1842.8–0359c | 6.4               | 0.0            | 0.0           | 3.2             | 0.0            | 1.4           | 6.2           | 1.2            | 5.4           | 10.2           | 3.0            | 4.0           | 2.8              | 0.0            | 1.0           |
| J1843.7–0312c | 8.0               | 0.0            | 0.0           | 3.1             | 0.7            | 5.0           | 8.2           | 1.2            | 7.5           | 4.9            | 0.0            | 0.0           | 1.3              | 0.0            | 0.0           |
| J1844.3+1548  | 4.5               | 0.8            | 6.0           | 0.5             | 0.1            | 4.3           | 1.6           | 0.3            | 6.6           | 4.2            | 1.1            | 6.0           | 1.7              | 0.0            | 3.3           |
| J1844.3–0343c | 16.4              | 0.0            | 2.5           | 3.8             | 0.0            | 2.8           | 6.0           | 1.3            | 5.1           | 20.7           | 3.5            | 7.2           | 1.7              | 0.0            | 0.0           |
| J1844.7+5716  | 2.1               | 0.0            | 2.0           | 0.3             | 0.1            | 3.9           | 0.6           | 0.0            | 2.4           | 1.4            | 0.0            | 1.1           | 0.6              | 0.0            | 0.0           |
| J1844.9–1116  | 5.0               | 0.8            | 6.3           | 1.8             | 0.2            | 8.0           | 1.5           | 0.0            | 1.9           | 1.0            | 0.0            | 0.0           | 1.0              | 0.0            | 1.6           |
| J1846.4+0920  | 3.4               | 0.0            | 2.5           | 0.7             | 0.0            | 2.9           | 4.1           | 0.4            | 13.3          | 10.2           | 1.6            | 10.9          | 1.6              | 0.0            | 2.4           |
| J1846.6–2519  | 3.5               | 0.9            | 4.5           | 0.6             | 0.1            | 4.3           | 0.8           | 0.3            | 3.4           | 4.1            | 0.0            | 2.9           | 1.0              | 0.0            | 0.2           |
| J1847.2–0236  | 11.5              | 3.9            | 4.5           | 4.5             | 0.6            | 8.7           | 9.1           | 1.2            | 8.3           | 11.3           | 0.0            | 2.2           | 3.1              | 0.0            | 1.6           |
| J1848.2–0139c | 14.7              | 0.0            | 0.6           | 2.9             | 0.7            | 4.0           | 9.4           | 1.3            | 7.8           | 13.7           | 3.3            | 4.8           | 1.9              | 0.0            | 0.4           |
| J1848.5+3216  | 7.6               | 0.0            | 1.6           | 0.7             | 0.2            | 4.0           | 1.1           | 0.3            | 4.8           | 2.8            | 0.9            | 4.9           | 0.9              | 0.0            | 0.4           |
| J1848.6+3241  | 5.7               | 0.0            | 0.7           | 0.9             | 0.0            | 2.7           | 0.8           | 0.3            | 3.5           | 2.9            | 0.0            | 2.3           | 0.9              | 0.0            | 0.9           |

Table 1—Continued

|               | 100 MeV – 300 MeV |                |               | 300 MeV – 1 GeV |                |               | 1 GeV – 3 GeV |                |               | 3 GeV – 10 GeV |                |               | 10 GeV – 100 GeV |                |               |
|---------------|-------------------|----------------|---------------|-----------------|----------------|---------------|---------------|----------------|---------------|----------------|----------------|---------------|------------------|----------------|---------------|
| Name 2FGL     | $F_1^a$           | $\Delta F_1^a$ | $\sqrt{TS_1}$ | $F_2^a$         | $\Delta F_2^a$ | $\sqrt{TS_2}$ | $F_3^b$       | $\Delta F_3^b$ | $\sqrt{TS_3}$ | $F_4^c$        | $\Delta F_4^c$ | $\sqrt{TS_4}$ | $F_5^c$          | $\Delta F_5^c$ | $\sqrt{TS_5}$ |
| J1849.3–0055  | 5.9               | 0.0            | 0.0           | 2.2             | 0.0            | 2.2           | 5.3           | 1.0            | 5.6           | 15.6           | 3.0            | 6.4           | 3.7              | 0.0            | 2.8           |
| J1849.4+6706  | 7.7               | 0.4            | 22.0          | 2.5             | 0.1            | 36.3          | 5.9           | 0.3            | 33.7          | 13.3           | 1.3            | 21.4          | 1.7              | 0.5            | 8.7           |
| J1849.5+2744  | 1.3               | 0.0            | 0.0           | 0.3             | 0.0            | 1.4           | 1.0           | 0.2            | 6.0           | 2.4            | 0.0            | 2.5           | 0.7              | 0.0            | 0.5           |
| J1849.7–4310  | 0.8               | 0.0            | 0.0           | 0.3             | 0.1            | 3.3           | 1.2           | 0.2            | 6.9           | 2.9            | 0.9            | 5.6           | 1.3              | 0.0            | 1.5           |
| J1849.9–0125c | 18.0              | 0.0            | 2.0           | 3.7             | 0.8            | 4.9           | 6.2           | 1.2            | 5.3           | 9.6            | 2.8            | 3.9           | 2.2              | 0.0            | 1.3           |
| J1850.7–0014c | 4.2               | 0.0            | 0.0           | 2.3             | 0.5            | 5.1           | 5.0           | 1.0            | 5.4           | 3.2            | 0.0            | 0.0           | 1.5              | 0.0            | 0.0           |
| J1852.5+4856  | 3.5               | 0.5            | 8.6           | 1.2             | 0.1            | 16.3          | 2.2           | 0.2            | 14.7          | 4.6            | 0.9            | 9.7           | 1.4              | 0.5            | 5.8           |
| J1852.7+0047c | 38.1              | 0.0            | 5.0           | 3.8             | 0.6            | 6.9           | 3.5           | 0.0            | 1.6           | 10.9           | 0.0            | 2.8           | 1.6              | 0.0            | 0.2           |
| J1852.8+0156c | 10.5              | 0.0            | 2.1           | 3.4             | 0.5            | 7.8           | 4.7           | 1.0            | 5.2           | 10.2           | 0.0            | 2.6           | 1.4              | 0.0            | 0.0           |
| J1855.9+0121e | 48.5              | 0.0            | 3.1           | 21.4            | 1.0            | 21.9          | 60.2          | 2.0            | 36.2          | 119.1          | 6.4            | 25.7          | 9.0              | 1.7            | 7.1           |
| J1856.2+0450c | 7.5               | 2.0            | 4.7           | 4.1             | 0.4            | 10.1          | 3.1           | 0.8            | 4.2           | 7.0            | 0.0            | 2.2           | 1.2              | 0.0            | 0.3           |
| J1857.2+0055c | 6.5               | 0.0            | 0.0           | 2.4             | 0.6            | 4.4           | 7.1           | 1.2            | 6.7           | 15.7           | 3.1            | 6.1           | 2.4              | 0.8            | 4.1           |
| J1857.6+0211  | 16.5              | 4.2            | 6.2           | 5.3             | 0.6            | 10.3          | 12.1          | 1.1            | 12.2          | 14.0           | 2.8            | 6.1           | 1.0              | 0.0            | 0.0           |
| J1857.8+0355c | 8.7               | 0.0            | 0.5           | 1.6             | 0.4            | 3.6           | 8.0           | 1.0            | 8.5           | 8.7            | 2.3            | 4.4           | 1.4              | 0.0            | 0.0           |
| J1858.1–2510  | 3.5               | 0.0            | 2.8           | 0.8             | 0.1            | 6.4           | 0.9           | 0.3            | 4.0           | 3.8            | 0.0            | 2.8           | 0.7              | 0.0            | 0.3           |
| J1858.3–2218  | 1.7               | 0.0            | 0.5           | 0.3             | 0.0            | 0.6           | 1.5           | 0.3            | 7.1           | 3.4            | 0.0            | 3.0           | 0.9              | 0.0            | 0.5           |
| J1858.5+0129c | 21.9              | 0.0            | 0.1           | 2.1             | 0.0            | 1.9           | 4.6           | 1.1            | 4.5           | 12.1           | 0.0            | 3.0           | 1.3              | 0.0            | 0.0           |
| J1859.3+0312c | 5.9               | 0.0            | 0.6           | 3.8             | 0.5            | 8.3           | 4.2           | 1.0            | 4.5           | 4.7            | 0.0            | 0.2           | 3.1              | 0.0            | 1.7           |
| J1901.1+0427  | 7.5               | 1.8            | 4.3           | 5.7             | 0.5            | 12.3          | 8.2           | 1.1            | 8.4           | 8.7            | 2.6            | 3.9           | 1.6              | 0.0            | 0.0           |
| J1902.0–5109  | 1.8               | 0.4            | 4.5           | 0.9             | 0.1            | 11.1          | 2.5           | 0.3            | 13.1          | 4.4            | 1.0            | 8.2           | 0.9              | 0.0            | 1.1           |
| J1902.3–1106  | 3.4               | 0.9            | 3.7           | 0.6             | 0.2            | 4.2           | 1.1           | 0.3            | 4.0           | 3.1            | 0.0            | 1.4           | 1.1              | 0.0            | 1.1           |
| J1902.5–6746  | 2.0               | 0.0            | 2.2           | 0.6             | 0.1            | 7.5           | 0.5           | 0.2            | 3.8           | 1.7            | 0.0            | 1.7           | 0.7              | 0.0            | 1.7           |
| J1902.7–7053  | 2.1               | 0.5            | 4.6           | 0.3             | 0.1            | 4.2           | 1.2           | 0.2            | 7.9           | 1.9            | 0.7            | 4.7           | 0.9              | 0.0            | 1.1           |
| J1903.3+5539  | 2.1               | 0.4            | 5.9           | 0.7             | 0.1            | 11.1          | 2.6           | 0.2            | 16.8          | 8.7            | 1.2            | 14.6          | 2.8              | 0.6            | 11.2          |
| J1904.8–0705  | 4.7               | 1.0            | 4.8           | 0.8             | 0.2            | 5.2           | 1.9           | 0.4            | 6.4           | 3.2            | 1.1            | 4.0           | 0.9              | 0.0            | 0.9           |
| J1904.9–3720c | 0.7               | 0.0            | 0.4           | 0.8             | 0.1            | 8.3           | 1.3           | 0.0            | 2.7           | 2.8            | 0.0            | 1.9           | 0.6              | 0.0            | 0.0           |
| J1906.5+0720  | 7.1               | 1.9            | 4.6           | 6.7             | 0.5            | 15.5          | 11.8          | 1.0            | 12.8          | 12.3           | 2.7            | 5.4           | 3.0              | 0.0            | 2.7           |
| J1907.9+0602  | 19.3              | 2.1            | 11.7          | 11.0            | 0.4            | 29.7          | 30.4          | 1.1            | 35.8          | 52.4           | 3.7            | 21.9          | 3.4              | 0.9            | 5.9           |
| J1908.8–0132  | 2.5               | 0.6            | 4.3           | 0.3             | 0.0            | 0.9           | 1.5           | 0.3            | 4.9           | 4.5            | 0.0            | 3.0           | 1.1              | 0.0            | 1.9           |
| J1911.0+0905  | 3.9               | 0.0            | 0.0           | 5.4             | 0.4            | 15.0          | 15.8          | 1.0            | 19.2          | 45.7           | 3.7            | 18.8          | 6.4              | 1.3            | 8.2           |
| J1911.1–2005  | 9.4               | 1.2            | 8.5           | 2.8             | 0.2            | 19.6          | 5.1           | 0.4            | 19.4          | 6.7            | 1.2            | 9.3           | 0.9              | 0.0            | 0.2           |
| J1911.5–1908  | 3.2               | 0.0            | 0.6           | 0.5             | 0.0            | 1.8           | 0.7           | 0.0            | 1.6           | 2.1            | 0.8            | 3.7           | 1.8              | 0.0            | 3.0           |
| J1912.0+1609  | 7.5               | 1.4            | 6.3           | 1.1             | 0.2            | 4.9           | 1.2           | 0.0            | 1.2           | 4.4            | 0.0            | 3.0           | 1.2              | 0.0            | 1.3           |
| J1913.4+4440  | 0.5               | 0.0            | 0.0           | 0.2             | 0.0            | 0.8           | 0.5           | 0.0            | 2.4           | 2.2            | 0.0            | 2.7           | 1.5              | 0.0            | 3.0           |
| J1913.8–1237  | 3.9               | 0.0            | 2.9           | 0.7             | 0.0            | 3.1           | 0.9           | 0.0            | 1.6           | 3.0            | 0.0            | 1.9           | 0.9              | 0.0            | 0.0           |
| J1914.0+1436  | 4.7               | 1.3            | 5.1           | 1.8             | 0.3            | 6.6           | 2.4           | 0.0            | 3.0           | 3.3            | 1.2            | 3.5           | 0.7              | 0.0            | 0.2           |
| J1914.4+0951c | 7.8               | 2.0            | 6.8           | 1.7             | 0.0            | 2.7           | 2.9           | 0.8            | 3.8           | 6.4            | 0.0            | 1.5           | 1.2              | 0.0            | 0.2           |
| J1916.1+1106  | 6.1               | 0.0            | 2.8           | 1.8             | 0.4            | 4.6           | 3.0           | 0.0            | 2.0           | 9.6            | 0.0            | 3.1           | 2.4              | 0.0            | 1.6           |
| J1917.0–3027  | 1.6               | 0.0            | 0.8           | 0.4             | 0.0            | 2.2           | 0.6           | 0.2            | 3.4           | 2.7            | 0.8            | 5.2           | 1.2              | 0.0            | 2.0           |
| J1917.6–1921  | 2.8               | 0.0            | 1.7           | 0.6             | 0.1            | 5.9           | 2.3           | 0.3            | 11.7          | 8.1            | 1.3            | 11.1          | 2.8              | 0.7            | 9.0           |
| J1918.2–4110  | 2.0               | 0.0            | 2.4           | 0.4             | 0.1            | 5.1           | 1.8           | 0.3            | 10.0          | 7.4            | 1.3            | 10.8          | 2.2              | 0.7            | 6.8           |
| J1919.5–7324  | 2.8               | 0.0            | 2.4           | 0.3             | 0.1            | 3.7           | 0.6           | 0.0            | 2.0           | 1.7            | 0.0            | 2.0           | 0.5              | 0.0            | 0.0           |
| J1921.1+1436c | 8.9               | 2.4            | 4.2           | 2.9             | 0.5            | 6.0           | 4.9           | 0.9            | 5.8           | 6.9            | 0.0            | 1.7           | 1.0              | 0.0            | 0.0           |
| J1921.3+0131  | 2.6               | 0.6            | 4.5           | 0.5             | 0.1            | 3.5           | 1.8           | 0.4            | 6.2           | 3.3            | 0.0            | 1.6           | 1.4              | 0.0            | 2.7           |

Table 1—Continued

|               | 100 MeV – 300 MeV |                |               | 300 MeV – 1 GeV |                |               | 1 GeV – 3 GeV |                |               | 3 GeV – 10 GeV |                |               | 10 GeV – 100 GeV |                |               |
|---------------|-------------------|----------------|---------------|-----------------|----------------|---------------|---------------|----------------|---------------|----------------|----------------|---------------|------------------|----------------|---------------|
| Name 2FGL     | $F_1^a$           | $\Delta F_1^a$ | $\sqrt{TS_1}$ | $F_2^a$         | $\Delta F_2^a$ | $\sqrt{TS_2}$ | $F_3^b$       | $\Delta F_3^b$ | $\sqrt{TS_3}$ | $F_4^c$        | $\Delta F_4^c$ | $\sqrt{TS_4}$ | $F_5^c$          | $\Delta F_5^c$ | $\sqrt{TS_5}$ |
| J1921.3–1231  | 1.4               | 0.0            | 0.0           | 0.4             | 0.1            | 3.7           | 1.1           | 0.0            | 3.1           | 2.2            | 0.8            | 3.8           | 1.5              | 0.0            | 2.9           |
| J1921.9–1608  | 1.3               | 0.0            | 0.4           | 0.4             | 0.0            | 2.4           | 1.0           | 0.2            | 5.7           | 3.6            | 0.9            | 7.0           | 2.8              | 0.7            | 9.0           |
| J1922.6–7454  | 2.3               | 0.0            | 2.5           | 0.3             | 0.0            | 1.5           | 0.7           | 0.0            | 2.5           | 1.4            | 0.6            | 3.9           | 1.1              | 0.0            | 2.7           |
| J1923.2+1408e | 17.1              | 2.7            | 6.6           | 10.3            | 0.5            | 22.2          | 28.2          | 1.2            | 30.4          | 79.2           | 4.4            | 26.5          | 15.3             | 1.7            | 14.4          |
| J1923.4+2013  | 5.8               | 1.3            | 4.7           | 0.9             | 0.2            | 3.7           | 1.4           | 0.4            | 3.3           | 2.7            | 0.0            | 0.9           | 1.1              | 0.0            | 0.0           |
| J1923.5–2105  | 8.9               | 0.7            | 16.0          | 2.9             | 0.1            | 26.7          | 6.9           | 0.4            | 27.8          | 15.8           | 1.7            | 19.0          | 0.8              | 0.4            | 4.1           |
| J1924.8+1724c | 4.6               | 1.4            | 5.1           | 1.4             | 0.3            | 5.1           | 4.2           | 0.7            | 6.7           | 4.0            | 0.0            | 0.7           | 1.4              | 0.0            | 0.3           |
| J1924.8–2912  | 6.2               | 0.7            | 10.9          | 1.5             | 0.1            | 14.4          | 2.3           | 0.3            | 11.1          | 5.6            | 1.2            | 7.8           | 1.5              | 0.0            | 2.2           |
| J1924.9–1036  | 2.8               | 0.8            | 4.1           | 0.4             | 0.1            | 3.9           | 1.1           | 0.3            | 5.2           | 2.0            | 0.9            | 3.2           | 1.3              | 0.0            | 1.6           |
| J1925.7–7836c | 1.8               | 0.6            | 3.4           | 0.3             | 0.1            | 3.5           | 0.8           | 0.0            | 2.7           | 2.6            | 0.0            | 2.8           | 1.0              | 0.0            | 1.3           |
| J1927.0+6153  | 1.1               | 0.0            | 0.0           | 0.4             | 0.1            | 4.5           | 1.4           | 0.2            | 9.8           | 4.8            | 0.9            | 9.7           | 2.7              | 0.6            | 11.2          |
| J1927.5+6117  | 2.6               | 0.0            | 3.0           | 0.5             | 0.0            | 2.9           | 0.7           | 0.2            | 4.8           | 1.6            | 0.6            | 4.0           | 1.2              | 0.0            | 3.7           |
| J1928.8+1740c | 5.6               | 0.0            | 2.5           | 2.0             | 0.4            | 5.9           | 3.4           | 0.0            | 3.0           | 5.9            | 0.0            | 1.7           | 2.2              | 0.0            | 2.3           |
| J1931.1+0938  | 5.9               | 1.1            | 6.1           | 1.1             | 0.2            | 6.7           | 1.3           | 0.3            | 4.9           | 6.5            | 1.3            | 8.5           | 2.6              | 0.7            | 8.4           |
| J1931.8+1325  | 6.1               | 0.9            | 7.3           | 1.2             | 0.2            | 5.3           | 1.1           | 0.0            | 1.0           | 4.2            | 0.0            | 2.3           | 0.5              | 0.0            | 0.0           |
| J1932.1+1913  | 7.1               | 1.2            | 7.2           | 3.3             | 0.3            | 11.8          | 6.4           | 0.7            | 10.4          | 5.9            | 1.7            | 4.2           | 1.1              | 0.0            | 1.1           |
| J1933.3+0722  | 4.1               | 1.0            | 4.6           | 0.5             | 0.0            | 1.5           | 0.9           | 0.3            | 3.9           | 2.7            | 0.9            | 4.4           | 1.6              | 0.0            | 3.2           |
| J1936.5–0855  | 2.7               | 0.0            | 1.5           | 0.6             | 0.1            | 4.9           | 0.9           | 0.0            | 2.0           | 3.0            | 0.0            | 2.4           | 0.8              | 0.0            | 0.0           |
| J1936.8–4721  | 1.0               | 0.0            | 0.6           | 0.2             | 0.0            | 0.7           | 0.5           | 0.2            | 3.7           | 1.9            | 0.7            | 4.2           | 1.2              | 0.5            | 5.2           |
| J1936.9+8402  | 0.5               | 0.0            | 0.0           | 0.2             | 0.0            | 2.1           | 0.4           | 0.1            | 4.0           | 2.1            | 0.0            | 3.0           | 0.5              | 0.0            | 0.0           |
| J1937.2–3955  | 2.4               | 0.5            | 4.6           | 0.6             | 0.1            | 6.1           | 0.9           | 0.2            | 5.2           | 2.0            | 0.7            | 4.4           | 1.1              | 0.0            | 1.6           |
| J1940.8–6213  | 1.5               | 0.5            | 3.2           | 0.3             | 0.1            | 4.5           | 0.7           | 0.2            | 4.6           | 2.4            | 0.0            | 2.3           | 0.6              | 0.0            | 0.0           |
| J1941.6+7218  | 1.5               | 0.6            | 4.5           | 0.6             | 0.1            | 8.5           | 0.9           | 0.2            | 6.3           | 2.0            | 0.0            | 2.1           | 0.4              | 0.0            | 0.0           |
| J1942.5–1024  | 4.1               | 0.0            | 2.7           | 0.5             | 0.1            | 4.5           | 0.8           | 0.0            | 2.0           | 1.1            | 0.0            | 0.0           | 1.1              | 0.0            | 1.8           |
| J1942.7–8049c | 2.2               | 0.0            | 1.8           | 0.6             | 0.1            | 6.3           | 0.7           | 0.2            | 3.7           | 3.2            | 0.0            | 2.2           | 0.8              | 0.0            | 0.0           |
| J1942.8+1033  | 2.9               | 0.8            | 4.2           | 0.6             | 0.0            | 2.7           | 1.7           | 0.3            | 7.2           | 9.4            | 1.4            | 12.0          | 2.8              | 0.7            | 9.0           |
| J1942.9–3528  | 2.2               | 0.0            | 2.3           | 0.4             | 0.0            | 2.1           | 0.9           | 0.2            | 4.7           | 3.1            | 0.0            | 2.5           | 1.2              | 0.0            | 1.6           |
| J1944.3+7325  | 1.8               | 0.7            | 4.0           | 0.3             | 0.1            | 4.1           | 0.5           | 0.0            | 1.9           | 2.0            | 0.0            | 3.0           | 0.4              | 0.0            | 0.0           |
| J1946.1–3115  | 2.7               | 0.0            | 2.8           | 0.3             | 0.1            | 3.6           | 1.0           | 0.0            | 3.0           | 2.2            | 0.0            | 1.7           | 1.4              | 0.0            | 2.0           |
| J1946.4–5402  | 0.8               | 0.0            | 1.6           | 0.4             | 0.1            | 6.6           | 1.5           | 0.2            | 9.4           | 2.2            | 0.8            | 4.4           | 0.5              | 0.0            | 0.0           |
| J1946.7–1118  | 3.0               | 0.0            | 1.5           | 0.4             | 0.1            | 3.4           | 0.9           | 0.0            | 2.5           | 2.2            | 0.8            | 3.9           | 0.8              | 0.0            | 0.0           |
| J1947.8–0739  | 3.3               | 0.0            | 3.0           | 0.7             | 0.1            | 6.3           | 0.9           | 0.0            | 2.4           | 3.1            | 0.0            | 2.7           | 0.9              | 0.0            | 0.0           |
| J1949.4–1457  | 1.6               | 0.0            | 0.4           | 0.5             | 0.1            | 5.0           | 0.7           | 0.2            | 4.0           | 2.4            | 0.0            | 2.3           | 0.6              | 0.0            | 0.0           |
| J1949.7+2405  | 2.6               | 0.7            | 3.9           | 1.2             | 0.2            | 5.3           | 2.4           | 0.0            | 2.8           | 2.5            | 0.0            | 0.1           | 1.9              | 0.0            | 2.4           |
| J1949.9+0907  | 3.3               | 0.0            | 2.5           | 0.6             | 0.0            | 2.9           | 0.6           | 0.2            | 3.5           | 1.8            | 0.0            | 1.7           | 1.9              | 0.0            | 3.4           |
| J1950.3+1223  | 4.2               | 1.1            | 5.5           | 0.8             | 0.1            | 6.5           | 1.1           | 0.3            | 5.0           | 2.7            | 0.0            | 2.1           | 0.8              | 0.0            | 0.4           |
| J1952.6–3252  | 1.9               | 0.0            | 1.2           | 0.5             | 0.1            | 4.7           | 0.6           | 0.0            | 1.0           | 2.2            | 0.0            | 1.9           | 1.1              | 0.0            | 1.4           |
| J1953.0+3253  | 9.0               | 1.0            | 11.4          | 5.5             | 0.2            | 31.5          | 18.3          | 0.7            | 40.3          | 27.7           | 2.4            | 21.0          | 1.5              | 0.6            | 4.4           |
| J1954.3+2836  | 9.4               | 1.6            | 5.8           | 4.1             | 0.3            | 16.1          | 13.4          | 0.7            | 24.4          | 22.3           | 2.4            | 14.4          | 2.0              | 0.0            | 2.8           |
| J1954.4–1607  | 2.1               | 0.0            | 1.2           | 0.5             | 0.0            | 2.6           | 0.9           | 0.0            | 2.5           | 2.2            | 0.8            | 4.6           | 0.7              | 0.0            | 0.0           |
| J1954.6–1122  | 4.3               | 0.7            | 7.6           | 1.0             | 0.1            | 9.3           | 3.0           | 0.3            | 13.4          | 4.5            | 1.0            | 7.3           | 2.0              | 0.0            | 3.7           |
| J1955.0–5639  | 1.1               | 0.0            | 0.9           | 0.3             | 0.0            | 2.2           | 0.5           | 0.0            | 2.1           | 1.5            | 0.7            | 3.3           | 1.6              | 0.0            | 4.1           |
| J1955.2+1356  | 4.0               | 0.9            | 5.7           | 0.8             | 0.1            | 7.0           | 1.4           | 0.3            | 6.4           | 3.9            | 1.0            | 6.1           | 1.6              | 0.0            | 2.4           |
| J1955.9–0241  | 3.0               | 0.0            | 2.7           | 0.7             | 0.1            | 6.0           | 0.7           | 0.0            | 1.0           | 2.6            | 0.0            | 2.3           | 1.0              | 0.0            | 1.6           |

Table 1—Continued

|               | 100 MeV – 300 MeV |                |               | 300 MeV – 1 GeV |                |               | 1 GeV – 3 GeV |                |               | 3 GeV – 10 GeV |                |               | 10 GeV – 100 GeV |                |               |
|---------------|-------------------|----------------|---------------|-----------------|----------------|---------------|---------------|----------------|---------------|----------------|----------------|---------------|------------------|----------------|---------------|
| Name 2FGL     | $F_1^a$           | $\Delta F_1^a$ | $\sqrt{TS_1}$ | $F_2^a$         | $\Delta F_2^a$ | $\sqrt{TS_2}$ | $F_3^b$       | $\Delta F_3^b$ | $\sqrt{TS_3}$ | $F_4^c$        | $\Delta F_4^c$ | $\sqrt{TS_4}$ | $F_5^c$          | $\Delta F_5^c$ | $\sqrt{TS_5}$ |
| J1957.9+5033  | 3.2               | 0.4            | 7.6           | 1.4             | 0.1            | 17.5          | 3.2           | 0.3            | 16.1          | 2.1            | 0.0            | 2.5           | 0.7              | 0.0            | 0.0           |
| J1958.2–3848  | 4.8               | 0.5            | 9.8           | 1.3             | 0.1            | 14.1          | 2.9           | 0.3            | 14.8          | 4.6            | 1.0            | 8.0           | 1.0              | 0.0            | 1.0           |
| J1958.4–3012  | 11.6              | 0.0            | 0.0           | 0.3             | 0.0            | 0.5           | 0.9           | 0.0            | 2.7           | 1.4            | 0.7            | 3.2           | 1.7              | 0.0            | 3.8           |
| J1958.6+4020  | 4.3               | 0.0            | 2.2           | 0.6             | 0.0            | 2.8           | 1.2           | 0.0            | 3.0           | 2.4            | 0.9            | 4.0           | 1.2              | 0.0            | 1.0           |
| J1958.6+2845  | 6.0               | 0.0            | 1.8           | 4.1             | 0.3            | 16.7          | 12.0          | 0.7            | 23.0          | 17.5           | 2.1            | 12.8          | 1.9              | 0.6            | 5.3           |
| J1958.9+3844  | 5.8               | 1.2            | 6.7           | 0.6             | 0.2            | 4.4           | 1.2           | 0.0            | 2.3           | 3.3            | 0.0            | 2.3           | 0.9              | 0.0            | 0.0           |
| J1959.1–4245  | 4.1               | 0.6            | 8.5           | 1.2             | 0.1            | 14.4          | 1.9           | 0.3            | 11.4          | 4.3            | 1.0            | 7.3           | 0.6              | 0.0            | 0.0           |
| J1959.5+2047  | 2.0               | 0.0            | 1.5           | 0.8             | 0.1            | 6.9           | 2.3           | 0.3            | 9.2           | 3.1            | 0.9            | 4.9           | 0.5              | 0.0            | 0.0           |
| J1959.6–2931  | 15.5              | 0.0            | 1.9           | 0.4             | 0.1            | 3.5           | 0.9           | 0.0            | 2.5           | 2.6            | 0.0            | 1.9           | 0.7              | 0.0            | 0.7           |
| J1959.9+4212  | 3.9               | 0.0            | 2.1           | 0.6             | 0.0            | 2.2           | 0.7           | 0.2            | 3.3           | 3.5            | 0.0            | 2.4           | 1.2              | 0.0            | 2.6           |
| J1959.9–4727  | 0.6               | 0.0            | 0.0           | 0.2             | 0.0            | 1.5           | 1.1           | 0.2            | 7.8           | 4.5            | 1.0            | 9.2           | 1.2              | 0.5            | 4.2           |
| J1959.9+3336c | 3.3               | 0.7            | 4.9           | 1.3             | 0.3            | 5.2           | 1.4           | 0.4            | 3.5           | 1.3            | 0.0            | 0.0           | 1.2              | 0.0            | 1.2           |
| J2000.0+6509  | 4.1               | 0.4            | 10.0          | 1.3             | 0.1            | 17.4          | 3.7           | 0.3            | 21.2          | 13.8           | 1.4            | 20.7          | 6.8              | 0.9            | 19.3          |
| J2000.8–1751  | 4.6               | 0.9            | 8.2           | 1.1             | 0.1            | 10.9          | 1.8           | 0.3            | 9.0           | 3.9            | 1.0            | 6.2           | 1.8              | 0.0            | 3.2           |
| J2001.1+4352  | 5.5               | 1.0            | 8.0           | 2.3             | 0.2            | 17.2          | 7.4           | 0.5            | 24.0          | 33.1           | 2.4            | 27.9          | 10.6             | 1.3            | 20.8          |
| J2001.7+7042  | 2.1               | 0.0            | 0.0           | 0.5             | 0.0            | 2.4           | 0.9           | 0.0            | 2.8           | 2.4            | 0.7            | 4.7           | 1.1              | 0.0            | 2.9           |
| J2002.8–2150  | 1.2               | 0.0            | 0.0           | 0.4             | 0.0            | 2.5           | 0.7           | 0.0            | 3.0           | 2.9            | 0.0            | 2.8           | 0.7              | 0.0            | 1.2           |
| J2004.4+3339c | 1.7               | 0.0            | 0.0           | 1.1             | 0.3            | 4.4           | 2.7           | 0.5            | 6.2           | 7.1            | 1.6            | 5.8           | 1.5              | 0.6            | 3.8           |
| J2004.5+7754  | 1.6               | 0.5            | 4.1           | 0.4             | 0.1            | 5.6           | 0.5           | 0.2            | 4.2           | 2.7            | 0.7            | 5.9           | 1.4              | 0.0            | 2.7           |
| J2004.6+7004  | 3.9               | 0.0            | 2.7           | 0.5             | 0.0            | 2.5           | 0.8           | 0.2            | 4.6           | 2.5            | 0.7            | 5.4           | 1.3              | 0.4            | 6.3           |
| J2006.2–0929  | 2.5               | 0.0            | 2.4           | 0.4             | 0.1            | 4.6           | 0.6           | 0.2            | 3.4           | 1.4            | 0.0            | 0.3           | 0.9              | 0.0            | 0.6           |
| J2006.5–2256  | 1.8               | 0.5            | 3.5           | 0.5             | 0.1            | 5.1           | 0.6           | 0.2            | 3.9           | 2.7            | 0.0            | 2.7           | 0.7              | 0.0            | 0.0           |
| J2006.9–1734  | 2.5               | 0.8            | 4.4           | 0.4             | 0.1            | 4.3           | 0.7           | 0.0            | 1.9           | 2.7            | 0.0            | 3.0           | 0.6              | 0.0            | 0.0           |
| J2007.9–4430  | 1.6               | 0.5            | 3.5           | 0.3             | 0.1            | 4.3           | 0.5           | 0.2            | 3.7           | 1.7            | 0.0            | 1.2           | 1.0              | 0.0            | 2.4           |
| J2009.1–0339  | 2.3               | 0.0            | 1.9           | 0.4             | 0.1            | 4.1           | 0.7           | 0.2            | 3.5           | 2.0            | 0.8            | 3.8           | 0.6              | 0.0            | 0.0           |
| J2009.2–1505  | 1.3               | 0.4            | 3.6           | 0.6             | 0.1            | 5.6           | 0.8           | 0.0            | 2.1           | 0.7            | 0.0            | 0.0           | 0.9              | 0.0            | 0.2           |
| J2009.5–4850  | 1.7               | 0.0            | 2.3           | 0.6             | 0.1            | 8.8           | 2.4           | 0.3            | 14.4          | 10.4           | 1.4            | 14.8          | 4.6              | 0.9            | 12.9          |
| J2009.7+7225  | 1.9               | 0.6            | 4.3           | 0.5             | 0.1            | 5.9           | 1.3           | 0.2            | 8.2           | 2.8            | 0.7            | 5.8           | 1.0              | 0.0            | 2.2           |
| J2009.8+2747  | 2.0               | 0.0            | 1.6           | 0.6             | 0.2            | 3.2           | 1.3           | 0.0            | 1.3           | 1.5            | 0.0            | 0.0           | 0.9              | 0.0            | 0.0           |
| J2012.1+4630  | 3.3               | 0.0            | 2.4           | 0.5             | 0.1            | 3.9           | 1.6           | 0.3            | 6.3           | 6.8            | 1.3            | 8.9           | 2.3              | 0.6            | 7.7           |
| J2012.4+3955c | 2.6               | 1.0            | 3.9           | 1.6             | 0.3            | 7.1           | 2.3           | 0.5            | 5.5           | 2.6            | 0.0            | 0.6           | 0.8              | 0.0            | 0.0           |
| J2013.8+4115c | 5.3               | 0.0            | 1.6           | 1.9             | 0.3            | 8.3           | 2.0           | 0.5            | 4.7           | 4.0            | 0.0            | 2.2           | 0.6              | 0.0            | 0.0           |
| J2014.0–0046  | 2.6               | 0.0            | 0.7           | 0.5             | 0.0            | 2.8           | 0.8           | 0.0            | 2.4           | 2.9            | 0.9            | 5.1           | 1.1              | 0.5            | 3.9           |
| J2014.7+0646  | 1.2               | 0.0            | 0.0           | 0.4             | 0.0            | 1.9           | 0.7           | 0.0            | 2.2           | 1.7            | 0.7            | 3.3           | 1.6              | 0.0            | 3.6           |
| J2015.1–0137  | 4.2               | 0.0            | 1.9           | 0.5             | 0.0            | 2.7           | 1.0           | 0.2            | 6.0           | 2.6            | 0.8            | 5.0           | 1.4              | 0.0            | 2.1           |
| J2015.6+3709  | 21.0              | 2.5            | 10.8          | 5.7             | 0.4            | 16.5          | 9.6           | 0.7            | 16.0          | 13.2           | 2.0            | 10.0          | 1.9              | 0.7            | 4.6           |
| J2016.3–0904  | 2.1               | 0.6            | 4.2           | 0.5             | 0.1            | 6.3           | 1.2           | 0.2            | 8.1           | 3.7            | 0.9            | 6.8           | 1.8              | 0.6            | 6.5           |
| J2017.3+0603  | 2.3               | 0.0            | 2.2           | 0.7             | 0.1            | 8.0           | 4.5           | 0.4            | 20.3          | 17.7           | 1.8            | 21.4          | 1.2              | 0.5            | 5.2           |
| J2017.4–3215  | 1.9               | 0.5            | 3.7           | 0.4             | 0.1            | 4.6           | 0.6           | 0.0            | 1.2           | 1.4            | 0.0            | 0.5           | 1.6              | 0.0            | 2.9           |
| J2017.5–1618  | 1.9               | 0.0            | 1.7           | 0.3             | 0.1            | 3.9           | 0.7           | 0.2            | 4.3           | 4.6            | 1.0            | 8.0           | 0.7              | 0.0            | 0.0           |
| J2018.0+3626  | 7.8               | 0.0            | 2.0           | 3.5             | 0.4            | 8.9           | 10.1          | 0.9            | 13.6          | 13.0           | 2.2            | 8.1           | 1.0              | 0.0            | 0.5           |
| J2018.2+3850c | 4.2               | 0.0            | 0.0           | 1.5             | 0.3            | 4.5           | 1.9           | 0.5            | 3.9           | 5.4            | 1.5            | 4.6           | 2.0              | 0.6            | 5.7           |
| J2019.1+4040  | 11.2              | 0.0            | 0.0           | 2.5             | 0.0            | 2.3           | 5.2           | 1.0            | 5.8           | 9.1            | 2.3            | 5.0           | 5.6              | 1.2            | 7.9           |
| J2020.0+4159  | 7.0               | 1.7            | 6.6           | 2.1             | 0.3            | 7.1           | 2.1           | 0.6            | 3.7           | 5.3            | 0.0            | 1.9           | 1.5              | 0.0            | 1.0           |

Table 1—Continued

|               | 100 MeV – 300 MeV |                |               | 300 MeV – 1 GeV |                |               | 1 GeV – 3 GeV |                |               | 3 GeV – 10 GeV |                |               | 10 GeV – 100 GeV |                |               |
|---------------|-------------------|----------------|---------------|-----------------|----------------|---------------|---------------|----------------|---------------|----------------|----------------|---------------|------------------|----------------|---------------|
| Name 2FGL     | $F_1^a$           | $\Delta F_1^a$ | $\sqrt{TS_1}$ | $F_2^a$         | $\Delta F_2^a$ | $\sqrt{TS_2}$ | $F_3^b$       | $\Delta F_3^b$ | $\sqrt{TS_3}$ | $F_4^c$        | $\Delta F_4^c$ | $\sqrt{TS_4}$ | $F_5^c$          | $\Delta F_5^c$ | $\sqrt{TS_5}$ |
| J2021.0+3651  | 33.9              | 2.9            | 15.0          | 19.8            | 0.5            | 48.6          | 56.3          | 1.3            | 66.5          | 97.3           | 4.4            | 40.9          | 3.4              | 0.8            | 7.1           |
| J2021.5+0632  | 2.1               | 0.0            | 1.0           | 0.3             | 0.0            | 1.7           | 0.6           | 0.2            | 3.4           | 2.2            | 0.8            | 4.8           | 0.6              | 0.0            | 0.0           |
| J2021.5+4026  | 79.9              | 8.9            | 19.5          | 38.0            | 0.7            | 62.5          | 102.9         | 1.7            | 87.0          | 160.4          | 5.5            | 54.4          | 5.6              | 1.2            | 8.1           |
| J2022.3–4518  | 1.2               | 0.0            | 0.7           | 0.3             | 0.0            | 2.7           | 0.7           | 0.2            | 5.2           | 1.3            | 0.0            | 1.0           | 0.5              | 0.0            | 0.0           |
| J2022.5+7614  | 2.3               | 0.5            | 5.2           | 0.6             | 0.1            | 8.0           | 1.4           | 0.2            | 9.0           | 1.8            | 0.6            | 4.5           | 1.2              | 0.0            | 2.9           |
| J2022.8+3843c | 4.6               | 1.3            | 3.8           | 2.7             | 0.4            | 7.2           | 3.0           | 0.0            | 2.9           | 4.4            | 0.0            | 1.2           | 0.6              | 0.0            | 0.0           |
| J2023.4–1137  | 1.4               | 0.0            | 0.9           | 0.3             | 0.1            | 4.5           | 0.8           | 0.2            | 5.4           | 3.2            | 0.9            | 6.2           | 1.6              | 0.0            | 2.9           |
| J2025.1+3341  | 9.1               | 0.0            | 3.1           | 2.7             | 0.3            | 9.4           | 2.9           | 0.5            | 6.2           | 4.9            | 1.3            | 5.1           | 1.0              | 0.0            | 0.5           |
| J2025.6–0736  | 12.6              | 0.8            | 25.7          | 4.4             | 0.2            | 43.0          | 8.5           | 0.4            | 35.3          | 14.2           | 1.6            | 19.1          | 1.2              | 0.5            | 5.4           |
| J2028.3+3332  | 4.4               | 1.2            | 3.6           | 2.1             | 0.2            | 9.6           | 9.5           | 0.6            | 20.5          | 13.4           | 1.8            | 11.3          | 0.6              | 0.0            | 0.0           |
| J2029.4+4924  | 2.4               | 0.6            | 4.3           | 0.9             | 0.1            | 6.7           | 4.1           | 0.4            | 12.2          | 4.8            | 1.2            | 5.6           | 1.0              | 0.0            | 1.3           |
| J2030.0+3640  | 3.0               | 1.1            | 3.3           | 0.9             | 0.2            | 4.3           | 6.7           | 0.6            | 14.4          | 8.8            | 1.7            | 7.1           | 0.7              | 0.0            | 0.0           |
| J2030.3–0622  | 4.5               | 0.8            | 7.4           | 0.7             | 0.1            | 7.7           | 0.6           | 0.2            | 3.8           | 1.2            | 0.6            | 3.2           | 1.2              | 0.0            | 2.8           |
| J2030.7+4417  | 3.8               | 1.0            | 4.2           | 2.9             | 0.3            | 12.3          | 5.6           | 0.6            | 11.0          | 8.2            | 1.7            | 6.4           | 1.0              | 0.0            | 0.9           |
| J2031.0+1938  | 1.9               | 0.0            | 2.0           | 0.1             | 0.0            | 0.0           | 0.5           | 0.2            | 4.0           | 2.8            | 0.0            | 3.2           | 1.2              | 0.5            | 5.1           |
| J2031.4–1842  | 2.6               | 0.0            | 3.0           | 0.3             | 0.0            | 1.9           | 0.6           | 0.0            | 1.9           | 2.2            | 0.0            | 2.6           | 0.6              | 0.0            | 0.0           |
| J2031.7+1223  | 1.9               | 0.7            | 3.6           | 0.6             | 0.1            | 6.8           | 1.1           | 0.2            | 6.2           | 1.6            | 0.0            | 1.1           | 1.5              | 0.0            | 3.0           |
| J2032.1+4049  | 18.6              | 8.5            | 6.6           | 5.4             | 0.6            | 11.0          | 5.1           | 0.8            | 6.6           | 6.7            | 0.0            | 2.0           | 1.7              | 0.0            | 1.1           |
| J2032.2+4126  | 25.0              | 0.0            | 0.2           | 3.8             | 0.4            | 9.9           | 15.9          | 0.9            | 23.0          | 56.6           | 3.6            | 26.2          | 3.6              | 0.9            | 6.5           |
| J2033.6+3927  | 9.5               | 1.6            | 7.6           | 3.1             | 0.4            | 8.8           | 0.9           | 0.0            | 0.0           | 5.7            | 0.0            | 1.5           | 2.3              | 0.0            | 2.6           |
| J2034.7–4201  | 1.4               | 0.0            | 1.2           | 0.3             | 0.0            | 2.5           | 0.4           | 0.0            | 0.7           | 1.3            | 0.6            | 3.7           | 1.1              | 0.0            | 2.5           |
| J2034.9+3632  | 1.4               | 0.0            | 0.0           | 0.9             | 0.0            | 2.0           | 1.3           | 0.4            | 3.5           | 5.9            | 1.4            | 5.9           | 0.9              | 0.0            | 0.4           |
| J2035.4+1058  | 4.4               | 0.7            | 8.1           | 0.9             | 0.1            | 9.3           | 1.5           | 0.2            | 8.5           | 2.0            | 0.7            | 4.2           | 0.5              | 0.0            | 0.0           |
| J2036.0+4224c | 11.2              | 0.0            | 2.0           | 1.7             | 0.5            | 3.6           | 1.1           | 0.0            | 0.0           | 5.4            | 0.0            | 1.5           | 2.2              | 0.0            | 2.1           |
| J2036.6+6551  | 1.5               | 0.0            | 1.3           | 0.3             | 0.0            | 1.9           | 0.9           | 0.0            | 3.1           | 1.9            | 0.7            | 4.5           | 0.9              | 0.0            | 2.3           |
| J2038.0+4145c | 9.9               | 0.0            | 1.3           | 2.5             | 0.6            | 4.1           | 2.7           | 0.0            | 2.0           | 4.3            | 0.0            | 0.8           | 1.3              | 0.0            | 0.6           |
| J2039.1–1046  | 1.5               | 0.5            | 3.4           | 0.5             | 0.1            | 7.6           | 1.7           | 0.2            | 10.8          | 4.6            | 1.0            | 8.1           | 1.8              | 0.6            | 7.0           |
| J2039.6+5218  | 1.4               | 0.0            | 0.0           | 0.3             | 0.0            | 0.6           | 0.7           | 0.0            | 1.5           | 3.2            | 0.0            | 3.1           | 1.0              | 0.4            | 4.2           |
| J2039.8–5620  | 2.1               | 0.4            | 5.0           | 0.7             | 0.1            | 9.8           | 2.0           | 0.2            | 11.9          | 4.2            | 1.0            | 7.6           | 0.7              | 0.0            | 0.0           |
| J2040.1+4105c | 8.9               | 0.0            | 1.9           | 1.5             | 0.4            | 3.8           | 1.8           | 0.6            | 3.2           | 4.8            | 0.0            | 1.2           | 1.2              | 0.0            | 0.1           |
| J2040.2–7109  | 1.1               | 0.0            | 0.6           | 0.2             | 0.0            | 1.3           | 0.6           | 0.0            | 3.1           | 2.2            | 0.0            | 2.8           | 1.4              | 0.0            | 2.7           |
| J2041.2+4735  | 3.7               | 0.0            | 2.8           | 1.3             | 0.2            | 6.8           | 3.2           | 0.5            | 7.9           | 4.0            | 1.3            | 3.9           | 0.7              | 0.0            | 0.4           |
| J2041.5+5003  | 2.1               | 0.0            | 0.0           | 1.1             | 0.3            | 4.5           | 1.5           | 0.4            | 4.2           | 4.3            | 0.0            | 3.1           | 0.6              | 0.0            | 0.0           |
| J2042.0+4252c | 10.8              | 1.7            | 9.8           | 2.2             | 0.4            | 7.0           | 1.4           | 0.0            | 0.5           | 2.3            | 0.0            | 0.0           | 0.9              | 0.0            | 0.0           |
| J2042.1+2428  | 1.6               | 0.0            | 1.4           | 0.2             | 0.0            | 0.3           | 0.4           | 0.0            | 0.8           | 2.7            | 0.8            | 5.8           | 1.5              | 0.0            | 2.9           |
| J2042.8–7317  | 1.7               | 0.5            | 3.9           | 0.3             | 0.0            | 2.1           | 0.4           | 0.0            | 0.8           | 1.6            | 0.6            | 4.3           | 1.0              | 0.0            | 2.7           |
| J2043.2+1711  | 1.7               | 0.4            | 4.4           | 0.8             | 0.1            | 10.8          | 3.8           | 0.3            | 20.0          | 8.4            | 1.3            | 12.6          | 1.4              | 0.0            | 3.5           |
| J2043.3+5105  | 2.2               | 0.9            | 4.5           | 1.4             | 0.2            | 8.2           | 2.0           | 0.4            | 6.0           | 3.6            | 0.0            | 1.8           | 0.6              | 0.0            | 0.0           |
| J2043.7+2743  | 1.2               | 0.0            | 0.9           | 0.4             | 0.1            | 4.8           | 1.3           | 0.3            | 6.0           | 2.6            | 0.0            | 1.9           | 0.7              | 0.0            | 1.2           |
| J2044.4–4757  | 1.5               | 0.0            | 0.9           | 0.3             | 0.1            | 3.8           | 0.9           | 0.2            | 6.0           | 1.6            | 0.7            | 3.7           | 0.5              | 0.0            | 0.0           |
| J2046.0+4954  | 4.8               | 1.0            | 5.5           | 1.2             | 0.3            | 4.9           | 2.6           | 0.5            | 6.4           | 2.6            | 0.0            | 0.9           | 1.3              | 0.0            | 1.6           |
| J2046.2–4259  | 1.5               | 0.0            | 1.6           | 0.3             | 0.0            | 1.7           | 0.5           | 0.0            | 1.5           | 1.7            | 0.7            | 4.1           | 0.8              | 0.0            | 1.1           |
| J2046.7+1055  | 1.5               | 0.0            | 0.0           | 0.3             | 0.1            | 3.6           | 0.9           | 0.2            | 6.0           | 1.6            | 0.7            | 3.3           | 0.6              | 0.0            | 0.0           |
| J2047.9+4536c | 4.2               | 0.8            | 5.3           | 1.5             | 0.3            | 5.8           | 1.7           | 0.0            | 1.7           | 4.8            | 0.0            | 2.7           | 0.6              | 0.0            | 0.0           |

Table 1—Continued

|               | 100 MeV – 300 MeV |                |               | 300 MeV – 1 GeV |                |               | 1 GeV – 3 GeV |                |               | 3 GeV – 10 GeV |                |               | 10 GeV – 100 GeV |                |               |
|---------------|-------------------|----------------|---------------|-----------------|----------------|---------------|---------------|----------------|---------------|----------------|----------------|---------------|------------------|----------------|---------------|
| Name 2FGL     | $F_1^a$           | $\Delta F_1^a$ | $\sqrt{TS_1}$ | $F_2^a$         | $\Delta F_2^a$ | $\sqrt{TS_2}$ | $F_3^b$       | $\Delta F_3^b$ | $\sqrt{TS_3}$ | $F_4^c$        | $\Delta F_4^c$ | $\sqrt{TS_4}$ | $F_5^c$          | $\Delta F_5^c$ | $\sqrt{TS_5}$ |
| J2049.8+1001  | 1.8               | 0.6            | 3.5           | 0.4             | 0.1            | 5.4           | 0.9           | 0.2            | 6.0           | 3.2            | 0.0            | 3.2           | 0.8              | 0.0            | 0.7           |
| J2050.0+0408  | 1.8               | 0.0            | 2.1           | 0.3             | 0.0            | 2.4           | 0.7           | 0.2            | 5.1           | 1.8            | 0.7            | 4.3           | 1.5              | 0.0            | 3.0           |
| J2051.0+3040e | 5.6               | 0.6            | 9.2           | 3.0             | 0.2            | 18.5          | 9.1           | 0.6            | 17.2          | 15.8           | 2.4            | 8.2           | 3.6              | 0.0            | 2.8           |
| J2051.8+5054  | 4.4               | 0.0            | 1.3           | 0.9             | 0.2            | 4.5           | 1.5           | 0.4            | 4.1           | 4.2            | 1.2            | 4.4           | 1.3              | 0.0            | 1.6           |
| J2053.2+1212c | 1.9               | 0.6            | 3.7           | 0.3             | 0.1            | 3.8           | 0.7           | 0.0            | 2.8           | 2.2            | 0.0            | 2.4           | 1.0              | 0.0            | 1.9           |
| J2055.4–0023  | 0.5               | 0.0            | 0.0           | 0.1             | 0.0            | 0.4           | 0.5           | 0.0            | 1.5           | 2.4            | 0.0            | 2.2           | 1.0              | 0.5            | 4.7           |
| J2055.8+2539  | 2.9               | 0.4            | 7.7           | 2.5             | 0.1            | 28.1          | 8.1           | 0.4            | 31.7          | 7.3            | 1.2            | 10.4          | 0.5              | 0.0            | 0.0           |
| J2055.8+4754  | 3.8               | 0.0            | 1.3           | 0.8             | 0.2            | 4.2           | 1.1           | 0.0            | 1.1           | 3.6            | 0.0            | 1.9           | 1.7              | 0.0            | 2.9           |
| J2056.2–4715  | 13.7              | 0.6            | 30.1          | 3.9             | 0.1            | 42.2          | 7.3           | 0.4            | 32.6          | 12.6           | 1.5            | 17.3          | 1.8              | 0.6            | 6.9           |
| J2056.7+4939  | 7.3               | 0.0            | 0.2           | 1.0             | 0.0            | 2.8           | 1.4           | 0.0            | 1.5           | 4.1            | 1.3            | 4.0           | 1.2              | 0.5            | 4.8           |
| J2102.2+4546  | 4.7               | 1.3            | 6.0           | 1.3             | 0.2            | 7.1           | 2.5           | 0.4            | 7.0           | 4.2            | 0.0            | 2.7           | 0.7              | 0.0            | 0.0           |
| J2103.3+4357c | 5.0               | 1.2            | 5.1           | 1.2             | 0.2            | 6.2           | 1.4           | 0.4            | 4.0           | 2.7            | 0.0            | 1.2           | 1.2              | 0.0            | 1.8           |
| J2103.4+4706  | 1.8               | 0.0            | 0.0           | 1.0             | 0.0            | 3.1           | 1.4           | 0.4            | 3.9           | 3.4            | 1.1            | 4.1           | 2.4              | 0.0            | 2.0           |
| J2103.5–1112  | 1.5               | 0.0            | 1.4           | 0.3             | 0.0            | 2.4           | 0.6           | 0.2            | 4.2           | 2.7            | 0.0            | 2.7           | 0.9              | 0.0            | 1.4           |
| J2103.6–6236  | 0.6               | 0.0            | 0.0           | 0.3             | 0.1            | 5.7           | 0.9           | 0.2            | 7.7           | 4.0            | 0.9            | 8.4           | 0.8              | 0.4            | 4.9           |
| J2104.9+3555  | 2.2               | 0.9            | 3.5           | 0.5             | 0.0            | 2.9           | 0.6           | 0.2            | 3.2           | 2.8            | 0.0            | 2.8           | 0.9              | 0.0            | 1.6           |
| J2107.6+2506  | 2.2               | 0.0            | 2.2           | 0.3             | 0.1            | 3.8           | 0.5           | 0.2            | 3.5           | 1.9            | 0.0            | 1.4           | 0.7              | 0.0            | 0.0           |
| J2107.8+3652  | 1.9               | 0.0            | 0.0           | 0.2             | 0.0            | 0.0           | 0.7           | 0.2            | 4.1           | 1.9            | 0.0            | 1.9           | 0.9              | 0.4            | 4.4           |
| J2107.9+5207c | 3.7               | 0.7            | 5.7           | 2.3             | 0.2            | 10.1          | 2.8           | 0.6            | 5.5           | 4.4            | 1.5            | 3.6           | 1.1              | 0.0            | 1.0           |
| J2108.6–1603  | 2.1               | 0.0            | 2.4           | 0.4             | 0.0            | 2.4           | 0.7           | 0.0            | 3.1           | 2.1            | 0.0            | 2.1           | 0.7              | 0.0            | 0.0           |
| J2108.7–0246  | 0.4               | 0.0            | 0.0           | 0.2             | 0.0            | 1.2           | 0.7           | 0.0            | 2.6           | 2.3            | 0.0            | 2.6           | 1.4              | 0.0            | 3.4           |
| J2108.9–6636  | 1.2               | 0.0            | 1.2           | 0.2             | 0.0            | 1.9           | 0.6           | 0.2            | 5.4           | 2.1            | 0.0            | 3.1           | 0.7              | 0.4            | 4.5           |
| J2109.9+0807  | 2.5               | 0.0            | 1.7           | 0.4             | 0.1            | 3.9           | 0.6           | 0.2            | 3.8           | 2.9            | 0.8            | 5.7           | 1.0              | 0.0            | 0.3           |
| J2110.3+3822  | 3.4               | 0.0            | 3.0           | 0.4             | 0.0            | 1.2           | 0.9           | 0.0            | 2.2           | 1.9            | 0.7            | 3.7           | 1.2              | 0.0            | 2.4           |
| J2111.3+4605  | 1.9               | 0.7            | 3.3           | 1.1             | 0.1            | 8.3           | 4.8           | 0.4            | 15.1          | 14.6           | 1.7            | 14.4          | 1.0              | 0.0            | 1.1           |
| J2112.3–4832  | 2.0               | 0.5            | 4.4           | 0.3             | 0.1            | 3.5           | 0.5           | 0.0            | 1.6           | 1.4            | 0.0            | 1.3           | 0.9              | 0.0            | 1.8           |
| J2112.5+0818  | 1.7               | 0.0            | 0.0           | 0.4             | 0.0            | 1.7           | 0.6           | 0.0            | 2.2           | 2.4            | 0.8            | 5.1           | 0.8              | 0.0            | 1.8           |
| J2112.5–3042  | 0.8               | 0.0            | 1.1           | 0.4             | 0.1            | 6.6           | 2.6           | 0.3            | 14.0          | 7.6            | 1.3            | 11.4          | 0.7              | 0.0            | 0.0           |
| J2114.1+5440  | 2.7               | 0.0            | 1.1           | 0.8             | 0.0            | 2.6           | 1.5           | 0.0            | 2.4           | 3.4            | 1.1            | 3.8           | 1.1              | 0.0            | 0.7           |
| J2115.3+2932  | 2.0               | 0.5            | 3.8           | 0.6             | 0.1            | 6.3           | 1.2           | 0.2            | 6.8           | 1.9            | 0.7            | 4.0           | 1.5              | 0.0            | 3.1           |
| J2115.4+1213  | 1.9               | 0.0            | 2.0           | 0.3             | 0.1            | 4.5           | 0.5           | 0.0            | 1.8           | 2.3            | 0.0            | 2.7           | 1.1              | 0.0            | 1.8           |
| J2116.2+3339  | 1.6               | 0.0            | 1.3           | 0.4             | 0.1            | 5.3           | 1.6           | 0.2            | 9.2           | 9.6            | 1.4            | 13.9          | 2.9              | 0.7            | 9.9           |
| J2117.5+3730  | 0.7               | 0.0            | 0.0           | 0.5             | 0.1            | 5.9           | 1.6           | 0.3            | 8.2           | 1.6            | 0.7            | 3.3           | 1.0              | 0.0            | 1.1           |
| J2120.6–1301  | 2.4               | 0.0            | 3.0           | 0.3             | 0.1            | 3.9           | 0.6           | 0.2            | 4.6           | 2.3            | 0.0            | 2.3           | 0.5              | 0.0            | 0.0           |
| J2121.0+1901  | 2.6               | 0.5            | 5.7           | 0.8             | 0.1            | 10.7          | 1.4           | 0.2            | 8.7           | 5.7            | 1.0            | 10.5          | 1.0              | 0.4            | 5.9           |
| J2124.0–1513  | 2.7               | 0.6            | 5.6           | 0.3             | 0.0            | 1.6           | 0.7           | 0.0            | 2.8           | 1.6            | 0.0            | 1.6           | 0.7              | 0.0            | 0.6           |
| J2124.6–3357  | 1.4               | 0.0            | 2.6           | 1.0             | 0.1            | 15.4          | 6.1           | 0.4            | 29.0          | 12.7           | 1.5            | 17.1          | 0.7              | 0.0            | 0.6           |
| J2125.0–4632  | 1.9               | 0.0            | 2.4           | 0.4             | 0.1            | 5.8           | 0.7           | 0.2            | 4.8           | 2.1            | 0.0            | 2.6           | 0.7              | 0.0            | 0.8           |
| J2127.8+3614  | 0.7               | 0.0            | 0.0           | 0.4             | 0.0            | 2.8           | 0.8           | 0.0            | 2.7           | 3.3            | 0.9            | 5.7           | 1.4              | 0.5            | 5.7           |
| J2128.7+5824  | 2.8               | 0.6            | 5.0           | 1.0             | 0.2            | 6.2           | 1.5           | 0.0            | 3.1           | 2.6            | 0.0            | 1.1           | 0.5              | 0.0            | 0.0           |
| J2129.8–0428  | 1.4               | 0.0            | 1.2           | 0.3             | 0.1            | 4.6           | 0.8           | 0.2            | 6.2           | 1.6            | 0.6            | 4.7           | 1.0              | 0.0            | 1.4           |
| J2131.0–5417  | 2.9               | 0.5            | 6.6           | 0.4             | 0.1            | 5.8           | 0.6           | 0.2            | 4.8           | 1.4            | 0.0            | 0.9           | 0.8              | 0.0            | 0.8           |
| J2131.6–0914  | 2.0               | 0.0            | 2.7           | 0.2             | 0.1            | 3.4           | 0.5           | 0.2            | 4.2           | 1.9            | 0.0            | 2.5           | 0.9              | 0.4            | 4.9           |
| J2132.5+2605  | 1.8               | 0.0            | 1.8           | 0.3             | 0.1            | 3.8           | 0.8           | 0.0            | 2.9           | 1.2            | 0.6            | 3.2           | 1.3              | 0.0            | 2.9           |

Table 1—Continued

|              | 100 MeV – 300 MeV |                |               | 300 MeV – 1 GeV |                |               | 1 GeV – 3 GeV |                |               | 3 GeV – 10 GeV |                |               | 10 GeV – 100 GeV |                |               |
|--------------|-------------------|----------------|---------------|-----------------|----------------|---------------|---------------|----------------|---------------|----------------|----------------|---------------|------------------|----------------|---------------|
| Name 2FGL    | $F_1^a$           | $\Delta F_1^a$ | $\sqrt{TS_1}$ | $F_2^a$         | $\Delta F_2^a$ | $\sqrt{TS_2}$ | $F_3^b$       | $\Delta F_3^b$ | $\sqrt{TS_3}$ | $F_4^c$        | $\Delta F_4^c$ | $\sqrt{TS_4}$ | $F_5^c$          | $\Delta F_5^c$ | $\sqrt{TS_5}$ |
| J2133.5–6431 | 1.4               | 0.0            | 0.0           | 0.4             | 0.0            | 2.1           | 1.0           | 0.2            | 7.1           | 1.2            | 0.5            | 3.6           | 0.4              | 0.0            | 0.0           |
| J2133.8–0154 | 1.9               | 0.0            | 2.5           | 0.5             | 0.1            | 7.1           | 0.7           | 0.2            | 5.1           | 1.9            | 0.7            | 4.9           | 0.6              | 0.0            | 0.0           |
| J2133.9+6645 | 1.7               | 0.0            | 1.2           | 0.4             | 0.0            | 1.2           | 0.9           | 0.0            | 1.9           | 3.7            | 0.9            | 6.1           | 0.8              | 0.4            | 3.7           |
| J2134.5–6513 | 2.2               | 0.0            | 2.2           | 0.3             | 0.0            | 1.9           | 0.5           | 0.0            | 2.0           | 1.3            | 0.6            | 3.9           | 0.9              | 0.0            | 1.9           |
| J2134.6–2130 | 0.7               | 0.0            | 0.0           | 0.3             | 0.1            | 4.8           | 0.5           | 0.2            | 4.2           | 1.8            | 0.0            | 2.1           | 1.3              | 0.5            | 5.0           |
| J2135.6–4959 | 2.2               | 0.5            | 5.1           | 0.6             | 0.1            | 8.2           | 0.9           | 0.2            | 6.5           | 2.2            | 0.0            | 2.0           | 0.5              | 0.0            | 0.0           |
| J2139.1–2054 | 0.7               | 0.0            | 0.4           | 0.1             | 0.0            | 0.0           | 0.4           | 0.0            | 2.2           | 2.3            | 0.0            | 3.4           | 1.3              | 0.0            | 2.7           |
| J2139.3–4236 | 4.3               | 0.4            | 10.9          | 1.6             | 0.1            | 21.3          | 4.7           | 0.3            | 25.3          | 11.5           | 1.5            | 16.7          | 2.5              | 0.7            | 8.1           |
| J2139.8+4714 | 1.6               | 0.4            | 3.9           | 1.0             | 0.1            | 8.9           | 3.5           | 0.4            | 12.4          | 2.1            | 0.8            | 3.5           | 0.6              | 0.0            | 0.0           |
| J2141.7–3739 | 1.5               | 0.5            | 3.7           | 0.3             | 0.1            | 4.4           | 0.4           | 0.0            | 0.9           | 2.2            | 0.0            | 3.0           | 1.3              | 0.0            | 2.5           |
| J2143.2–3929 | 1.1               | 0.0            | 0.8           | 0.2             | 0.0            | 1.7           | 0.5           | 0.2            | 4.2           | 2.1            | 0.7            | 5.1           | 1.5              | 0.0            | 2.8           |
| J2143.5+1743 | 12.8              | 0.7            | 24.0          | 2.6             | 0.1            | 27.3          | 4.0           | 0.3            | 19.2          | 5.9            | 1.1            | 10.7          | 0.7              | 0.0            | 0.0           |
| J2144.8–3356 | 1.7               | 0.4            | 4.3           | 0.8             | 0.1            | 12.4          | 1.6           | 0.2            | 11.6          | 3.4            | 0.9            | 6.4           | 1.5              | 0.0            | 3.4           |
| J2146.5–1530 | 2.4               | 0.0            | 2.6           | 0.3             | 0.1            | 4.4           | 0.8           | 0.0            | 3.1           | 1.4            | 0.0            | 1.3           | 0.7              | 0.0            | 0.0           |
| J2146.6–1345 | 1.1               | 0.0            | 0.0           | 0.2             | 0.0            | 0.8           | 0.8           | 0.2            | 5.6           | 3.1            | 0.8            | 7.0           | 2.2              | 0.6            | 8.8           |
| J2147.3+0930 | 8.3               | 0.6            | 17.2          | 1.9             | 0.1            | 23.2          | 2.9           | 0.3            | 16.8          | 3.9            | 0.9            | 7.5           | 0.9              | 0.4            | 4.0           |
| J2147.4–7534 | 8.3               | 0.6            | 15.9          | 2.0             | 0.1            | 22.4          | 3.0           | 0.3            | 16.6          | 4.7            | 1.0            | 9.0           | 0.8              | 0.4            | 4.0           |
| J2148.2+0659 | 2.3               | 0.6            | 4.6           | 0.4             | 0.1            | 4.9           | 0.7           | 0.0            | 2.9           | 1.5            | 0.0            | 1.3           | 0.5              | 0.0            | 0.0           |
| J2149.6+0326 | 1.9               | 0.0            | 2.4           | 0.3             | 0.0            | 2.8           | 0.9           | 0.2            | 6.6           | 1.9            | 0.7            | 4.2           | 0.8              | 0.0            | 0.0           |
| J2150.2–1412 | 2.2               | 0.0            | 0.7           | 0.2             | 0.0            | 0.1           | 0.4           | 0.2            | 3.3           | 1.4            | 0.6            | 3.6           | 0.8              | 0.0            | 1.7           |
| J2150.8–2738 | 1.4               | 0.0            | 1.2           | 0.3             | 0.1            | 4.2           | 0.4           | 0.0            | 1.3           | 1.2            | 0.5            | 3.4           | 0.9              | 0.0            | 1.8           |
| J2151.5–3021 | 5.7               | 0.7            | 11.4          | 0.8             | 0.1            | 9.5           | 0.8           | 0.0            | 2.8           | 0.9            | 0.0            | 0.0           | 0.5              | 0.0            | 0.0           |
| J2152.4+1735 | 2.2               | 0.0            | 2.0           | 0.4             | 0.0            | 2.9           | 0.6           | 0.0            | 2.4           | 1.4            | 0.6            | 3.6           | 1.0              | 0.0            | 2.4           |
| J2154.0–1138 | 2.2               | 0.5            | 4.8           | 0.5             | 0.1            | 7.5           | 0.7           | 0.2            | 5.5           | 2.1            | 0.0            | 2.8           | 0.5              | 0.0            | 0.0           |
| J2157.4+3129 | 4.5               | 0.5            | 9.5           | 1.3             | 0.1            | 14.9          | 2.5           | 0.3            | 13.7          | 2.1            | 0.7            | 4.2           | 1.0              | 0.0            | 1.6           |
| J2157.9–1501 | 1.7               | 0.5            | 4.3           | 0.4             | 0.1            | 5.6           | 1.0           | 0.2            | 7.2           | 1.9            | 0.7            | 4.4           | 1.7              | 0.0            | 4.0           |
| J2158.8–3013 | 8.9               | 0.6            | 22.6          | 4.1             | 0.1            | 50.2          | 15.2          | 0.6            | 59.7          | 62.4           | 3.2            | 53.3          | 26.6             | 2.1            | 39.5          |
| J2159.9+1023 | 1.2               | 0.0            | 1.0           | 0.2             | 0.0            | 1.6           | 0.6           | 0.0            | 2.7           | 1.7            | 0.6            | 4.3           | 0.8              | 0.0            | 0.4           |
| J2200.1–6931 | 2.1               | 0.5            | 4.6           | 0.3             | 0.1            | 5.2           | 0.5           | 0.1            | 4.9           | 2.0            | 0.0            | 3.1           | 0.5              | 0.0            | 0.0           |
| J2201.2+5926 | 5.2               | 1.3            | 6.4           | 0.7             | 0.2            | 4.1           | 1.1           | 0.0            | 1.9           | 3.1            | 0.0            | 1.6           | 1.5              | 0.0            | 3.0           |
| J2201.9–8335 | 4.9               | 0.6            | 11.0          | 1.6             | 0.1            | 16.7          | 3.1           | 0.3            | 15.1          | 2.1            | 0.7            | 4.7           | 0.6              | 0.0            | 0.0           |
| J2202.8+4216 | 12.0              | 0.6            | 23.4          | 3.9             | 0.1            | 35.1          | 8.8           | 0.5            | 32.7          | 16.4           | 1.7            | 19.9          | 2.3              | 0.6            | 8.9           |
| J2203.4+1726 | 6.4               | 0.5            | 15.3          | 2.2             | 0.1            | 27.3          | 5.6           | 0.4            | 27.2          | 8.5            | 1.2            | 14.5          | 2.7              | 0.7            | 10.2          |
| J2204.6+0442 | 1.2               | 0.0            | 0.9           | 0.3             | 0.1            | 3.9           | 0.7           | 0.2            | 6.0           | 2.0            | 0.0            | 2.4           | 0.8              | 0.0            | 1.2           |
| J2206.6+6500 | 3.9               | 0.6            | 7.7           | 1.3             | 0.2            | 9.4           | 1.2           | 0.3            | 4.3           | 3.3            | 0.0            | 2.9           | 0.6              | 0.0            | 0.0           |
| J2206.6–0029 | 0.7               | 0.0            | 0.0           | 0.3             | 0.1            | 3.7           | 0.5           | 0.2            | 3.3           | 1.4            | 0.6            | 3.8           | 0.8              | 0.0            | 0.8           |
| J2208.1–5345 | 2.9               | 0.4            | 7.2           | 0.5             | 0.1            | 7.3           | 1.1           | 0.2            | 8.5           | 2.6            | 0.8            | 5.3           | 0.9              | 0.0            | 2.7           |
| J2210.1+5913 | 3.6               | 0.0            | 0.0           | 1.1             | 0.2            | 6.4           | 1.4           | 0.4            | 4.3           | 2.5            | 0.0            | 0.9           | 1.1              | 0.0            | 1.8           |
| J2211.9+2355 | 1.3               | 0.0            | 0.4           | 0.2             | 0.1            | 3.2           | 0.7           | 0.2            | 4.7           | 2.8            | 0.8            | 6.7           | 1.2              | 0.0            | 3.4           |
| J2212.6+0702 | 1.2               | 0.0            | 0.8           | 0.4             | 0.1            | 5.9           | 0.9           | 0.2            | 6.8           | 2.2            | 0.7            | 5.0           | 0.5              | 0.0            | 0.0           |
| J2213.1–2527 | 1.5               | 0.4            | 3.6           | 0.3             | 0.1            | 4.3           | 0.7           | 0.2            | 5.1           | 1.9            | 0.7            | 4.8           | 0.7              | 0.0            | 0.3           |
| J2213.7–4754 | 1.4               | 0.4            | 3.7           | 0.2             | 0.0            | 2.0           | 0.5           | 0.0            | 2.3           | 1.6            | 0.0            | 1.3           | 1.5              | 0.0            | 3.9           |
| J2214.7+3000 | 1.6               | 0.3            | 4.9           | 1.1             | 0.1            | 16.7          | 4.4           | 0.3            | 23.9          | 10.5           | 1.3            | 16.3          | 0.9              | 0.0            | 0.9           |
| J2215.7+5135 | 0.8               | 0.0            | 0.5           | 0.3             | 0.1            | 4.4           | 1.5           | 0.2            | 7.8           | 4.5            | 1.0            | 7.5           | 0.6              | 0.0            | 1.5           |



Table 1—Continued

|               | 100 MeV – 300 MeV |                |               | 300 MeV – 1 GeV |                |               | 1 GeV – 3 GeV |                |               | 3 GeV – 10 GeV |                |               | 10 GeV – 100 GeV |                |               |
|---------------|-------------------|----------------|---------------|-----------------|----------------|---------------|---------------|----------------|---------------|----------------|----------------|---------------|------------------|----------------|---------------|
| Name 2FGL     | $F_1^a$           | $\Delta F_1^a$ | $\sqrt{TS_1}$ | $F_2^a$         | $\Delta F_2^a$ | $\sqrt{TS_2}$ | $F_3^b$       | $\Delta F_3^b$ | $\sqrt{TS_3}$ | $F_4^c$        | $\Delta F_4^c$ | $\sqrt{TS_4}$ | $F_5^c$          | $\Delta F_5^c$ | $\sqrt{TS_5}$ |
| J2217.1+2422  | 2.5               | 0.0            | 3.1           | 0.4             | 0.1            | 5.3           | 0.8           | 0.2            | 6.1           | 1.5            | 0.6            | 4.2           | 1.0              | 0.0            | 2.5           |
| J2219.1+1805  | 1.2               | 0.0            | 0.8           | 0.3             | 0.0            | 2.4           | 0.6           | 0.0            | 2.6           | 1.4            | 0.6            | 4.1           | 0.9              | 0.0            | 2.2           |
| J2219.6+5850  | 4.8               | 0.0            | 2.7           | 1.1             | 0.2            | 6.3           | 1.4           | 0.4            | 4.0           | 3.0            | 1.1            | 3.6           | 1.1              | 0.0            | 1.2           |
| J2221.0+6307  | 2.6               | 0.6            | 5.2           | 1.5             | 0.2            | 9.0           | 1.3           | 0.3            | 4.0           | 3.7            | 0.0            | 2.4           | 0.8              | 0.0            | 1.2           |
| J2221.6–5223  | 0.7               | 0.0            | 0.0           | 0.3             | 0.1            | 4.7           | 0.4           | 0.1            | 4.3           | 2.3            | 0.7            | 6.0           | 0.8              | 0.0            | 1.9           |
| J2222.0–3503  | 0.7               | 0.0            | 0.0           | 0.3             | 0.0            | 3.2           | 0.4           | 0.1            | 4.2           | 2.6            | 0.0            | 2.8           | 0.6              | 0.0            | 0.0           |
| J2223.4+0104  | 0.5               | 0.0            | 0.0           | 0.2             | 0.0            | 0.9           | 0.5           | 0.0            | 2.0           | 1.7            | 0.6            | 4.8           | 0.7              | 0.4            | 4.6           |
| J2225.6–0454  | 4.0               | 0.5            | 8.8           | 1.2             | 0.1            | 14.6          | 2.0           | 0.2            | 12.1          | 2.9            | 0.8            | 5.7           | 0.8              | 0.0            | 1.3           |
| J2227.8+0051  | 0.7               | 0.0            | 0.0           | 0.2             | 0.1            | 3.4           | 0.7           | 0.0            | 2.7           | 2.3            | 0.0            | 2.2           | 0.9              | 0.0            | 0.8           |
| J2228.6–1633  | 1.6               | 0.0            | 1.9           | 0.3             | 0.0            | 2.5           | 0.4           | 0.1            | 4.3           | 2.3            | 0.0            | 3.1           | 1.2              | 0.0            | 3.2           |
| J2229.0+6114  | 21.8              | 0.9            | 27.2          | 10.1            | 0.2            | 53.9          | 25.3          | 0.8            | 54.3          | 49.0           | 2.8            | 34.0          | 2.1              | 0.6            | 6.3           |
| J2229.7–0832  | 12.6              | 0.6            | 27.2          | 2.7             | 0.1            | 31.1          | 3.8           | 0.3            | 21.2          | 5.0            | 1.0            | 9.6           | 1.0              | 0.0            | 1.6           |
| J2231.0+6512  | 2.4               | 0.8            | 3.2           | 1.0             | 0.2            | 6.5           | 1.4           | 0.3            | 4.6           | 3.5            | 0.0            | 2.8           | 1.0              | 0.0            | 1.6           |
| J2232.4+1143  | 7.7               | 0.6            | 16.3          | 1.9             | 0.1            | 22.3          | 2.4           | 0.3            | 14.2          | 3.0            | 0.8            | 7.0           | 0.9              | 0.0            | 2.6           |
| J2234.7+0945  | 1.6               | 0.0            | 1.1           | 0.3             | 0.1            | 4.1           | 1.4           | 0.2            | 9.1           | 1.7            | 0.7            | 3.6           | 0.5              | 0.0            | 0.0           |
| J2234.9–4831  | 2.0               | 0.0            | 3.1           | 0.4             | 0.1            | 7.1           | 0.6           | 0.2            | 5.2           | 2.0            | 0.0            | 2.7           | 0.7              | 0.0            | 0.0           |
| J2236.1–3628  | 1.5               | 0.0            | 2.2           | 0.2             | 0.1            | 4.0           | 0.5           | 0.1            | 4.8           | 1.8            | 0.0            | 2.0           | 1.4              | 0.0            | 2.3           |
| J2236.4+2828  | 4.5               | 0.4            | 11.8          | 1.7             | 0.1            | 22.8          | 4.4           | 0.3            | 23.3          | 7.4            | 1.2            | 13.1          | 1.7              | 0.5            | 7.4           |
| J2236.5–1431  | 3.5               | 0.5            | 8.2           | 1.4             | 0.1            | 18.6          | 3.2           | 0.3            | 18.6          | 6.7            | 1.2            | 11.7          | 1.1              | 0.5            | 5.4           |
| J2237.2+6316  | 4.9               | 0.0            | 2.8           | 0.8             | 0.2            | 5.0           | 1.3           | 0.0            | 2.3           | 3.8            | 0.0            | 2.6           | 1.3              | 0.0            | 2.4           |
| J2237.2–3920  | 1.2               | 0.0            | 1.4           | 0.3             | 0.0            | 3.1           | 0.4           | 0.1            | 3.4           | 1.1            | 0.5            | 3.8           | 0.9              | 0.0            | 2.0           |
| J2238.4+5902  | 16.4              | 0.0            | 2.5           | 2.7             | 0.2            | 11.8          | 7.3           | 0.5            | 17.3          | 9.0            | 1.5            | 9.2           | 1.5              | 0.0            | 2.6           |
| J2239.8+5825  | 6.0               | 0.0            | 0.1           | 0.9             | 0.0            | 1.9           | 1.9           | 0.0            | 3.1           | 3.2            | 1.1            | 3.9           | 0.7              | 0.0            | 0.0           |
| J2241.7–5236  | 1.5               | 0.3            | 3.6           | 1.1             | 0.1            | 15.4          | 4.2           | 0.3            | 26.2          | 12.1           | 1.5            | 18.6          | 0.6              | 0.0            | 0.0           |
| J2243.2–2540  | 2.4               | 0.4            | 6.1           | 0.7             | 0.1            | 10.9          | 1.2           | 0.2            | 8.9           | 2.9            | 0.8            | 7.1           | 1.4              | 0.0            | 2.9           |
| J2243.9+2021  | 2.4               | 0.5            | 5.6           | 0.5             | 0.1            | 8.0           | 2.8           | 0.3            | 18.0          | 10.3           | 1.3            | 16.1          | 4.9              | 0.9            | 13.9          |
| J2244.1+4059  | 2.5               | 0.7            | 5.3           | 1.1             | 0.1            | 12.8          | 2.0           | 0.3            | 11.3          | 4.7            | 1.0            | 8.7           | 1.2              | 0.0            | 2.2           |
| J2246.3+1549  | 5.1               | 1.2            | 5.4           | 1.0             | 0.2            | 6.9           | 0.9           | 0.0            | 2.7           | 2.8            | 0.0            | 3.0           | 0.8              | 0.4            | 4.3           |
| J2246.8–5203  | 0.8               | 0.0            | 0.0           | 0.2             | 0.0            | 1.4           | 0.4           | 0.0            | 1.9           | 1.4            | 0.6            | 3.3           | 1.7              | 0.0            | 3.4           |
| J2247.2–0002  | 1.0               | 0.0            | 0.5           | 0.3             | 0.1            | 4.0           | 0.7           | 0.2            | 5.4           | 1.4            | 0.6            | 4.2           | 1.2              | 0.0            | 2.2           |
| J2247.8+4412  | 0.6               | 0.0            | 0.0           | 0.3             | 0.0            | 1.1           | 0.6           | 0.2            | 3.8           | 2.2            | 0.0            | 2.0           | 0.9              | 0.4            | 5.1           |
| J2249.1+5758  | 7.9               | 0.0            | 1.3           | 0.5             | 0.0            | 1.3           | 0.9           | 0.3            | 3.5           | 3.6            | 1.0            | 5.0           | 1.1              | 0.0            | 0.6           |
| J2250.0+3825  | 1.5               | 0.0            | 1.7           | 0.3             | 0.0            | 2.4           | 0.9           | 0.2            | 6.1           | 1.4            | 0.6            | 3.7           | 1.6              | 0.5            | 7.3           |
| J2250.2–4205  | 0.4               | 0.0            | 0.0           | 0.2             | 0.0            | 1.2           | 0.5           | 0.1            | 5.5           | 2.0            | 0.7            | 5.5           | 1.2              | 0.0            | 2.3           |
| J2250.7+6305c | 2.9               | 0.0            | 0.0           | 1.0             | 0.2            | 5.7           | 1.3           | 0.0            | 2.3           | 3.0            | 0.0            | 1.7           | 1.3              | 0.0            | 1.9           |
| J2250.8–2808  | 3.2               | 0.6            | 7.8           | 1.0             | 0.1            | 14.5          | 2.9           | 0.3            | 18.4          | 6.1            | 1.1            | 11.7          | 1.5              | 0.5            | 6.2           |
| J2251.1–4927  | 0.4               | 0.0            | 0.0           | 0.2             | 0.0            | 2.3           | 0.5           | 0.1            | 4.6           | 2.0            | 0.7            | 4.9           | 1.0              | 0.0            | 2.6           |
| J2251.8+4211  | 2.1               | 0.7            | 4.2           | 0.4             | 0.1            | 4.9           | 0.6           | 0.0            | 1.8           | 1.3            | 0.0            | 0.6           | 0.8              | 0.0            | 1.7           |
| J2251.9+4032  | 2.1               | 0.0            | 1.8           | 0.3             | 0.1            | 3.5           | 0.7           | 0.2            | 4.9           | 2.4            | 0.7            | 5.4           | 1.3              | 0.0            | 3.2           |
| J2253.9+1609  | 175.0             | 1.5            | 217.2         | 49.1            | 0.4            | 255.3         | 86.1          | 1.2            | 167.1         | 122.1          | 4.3            | 77.0          | 7.2              | 1.0            | 17.8          |
| J2254.1+1401  | 3.9               | 0.0            | 2.4           | 0.7             | 0.1            | 6.3           | 0.6           | 0.0            | 1.9           | 1.6            | 0.0            | 1.9           | 0.8              | 0.4            | 3.9           |
| J2255.2+2408  | 1.5               | 0.0            | 1.7           | 0.2             | 0.1            | 3.5           | 1.0           | 0.2            | 7.6           | 2.2            | 0.7            | 5.1           | 1.3              | 0.0            | 2.2           |
| J2256.4–2009  | 0.8               | 0.0            | 0.3           | 0.2             | 0.1            | 3.6           | 0.6           | 0.2            | 4.8           | 1.6            | 0.6            | 4.7           | 1.4              | 0.0            | 3.8           |
| J2256.9–1023  | 1.0               | 0.0            | 0.7           | 0.3             | 0.1            | 4.6           | 1.1           | 0.2            | 9.0           | 1.5            | 0.0            | 1.5           | 0.8              | 0.0            | 1.9           |

Table 1—Continued

|               | 100 MeV – 300 MeV |                |               | 300 MeV – 1 GeV |                |               | 1 GeV – 3 GeV |                |               | 3 GeV – 10 GeV |                |               | 10 GeV – 100 GeV |                |               |
|---------------|-------------------|----------------|---------------|-----------------|----------------|---------------|---------------|----------------|---------------|----------------|----------------|---------------|------------------|----------------|---------------|
| Name 2FGL     | $F_1^a$           | $\Delta F_1^a$ | $\sqrt{TS_1}$ | $F_2^a$         | $\Delta F_2^a$ | $\sqrt{TS_2}$ | $F_3^b$       | $\Delta F_3^b$ | $\sqrt{TS_3}$ | $F_4^c$        | $\Delta F_4^c$ | $\sqrt{TS_4}$ | $F_5^c$          | $\Delta F_5^c$ | $\sqrt{TS_5}$ |
| J2257.5+6222c | 2.4               | 0.0            |               | 2.6             | 0.7            | 0.2           | 5.0           | 2.2            | 0.4           | 5.9            | 3.3            | 0.0           | 1.6              | 0.5            | 0.0           |
| J2257.9–3646  | 0.9               | 0.0            |               | 0.0             | 0.1            | 0.0           | 0.6           | 0.5            | 0.1           | 5.0            | 0.8            | 0.0           | 0.6              | 0.8            | 0.4           |
| J2258.0–2759  | 5.2               | 0.5            | 14.0          | 1.5             | 0.1            | 20.7          | 2.5           | 0.3            | 16.1          | 3.1            | 0.8            | 7.5           | 1.2              | 0.0            | 2.7           |
| J2258.8–5524  | 0.7               | 0.0            |               | 0.1             | 0.2            | 0.0           | 2.6           | 0.4            | 0.0           | 2.0            | 2.2            | 0.0           | 3.4              | 1.1            | 0.0           |
| J2259.0–8254  | 2.1               | 0.0            |               | 1.7             | 0.4            | 0.0           | 2.4           | 0.9            | 0.0           | 2.9            | 2.2            | 0.8           | 4.7              | 0.5            | 0.0           |
| J2300.0–3553  | 1.3               | 0.0            |               | 1.0             | 0.2            | 0.1           | 3.3           | 0.4            | 0.1           | 4.2            | 0.8            | 0.0           | 0.0              | 0.7            | 0.0           |
| J2300.6+3139  | 0.8               | 0.0            |               | 0.1             | 0.3            | 0.0           | 2.4           | 0.4            | 0.1           | 3.8            | 3.6            | 0.8           | 7.9              | 0.9            | 0.0           |
| J2302.7+4443  | 1.8               | 0.0            |               | 3.1             | 1.1            | 0.1           | 14.6          | 5.2            | 0.4           | 24.6           | 16.8           | 1.7           | 20.7             | 1.1            | 0.0           |
| J2304.7+3703  | 0.5               | 0.0            |               | 0.0             | 0.2            | 0.0           | 1.2           | 0.5            | 0.0           | 1.9            | 1.4            | 0.6           | 3.4              | 0.8            | 0.4           |
| J2308.0+1457  | 2.9               | 0.9            |               | 4.6             | 0.5            | 0.1           | 5.1           | 0.8            | 0.2           | 4.8            | 2.0            | 0.7           | 4.4              | 1.2            | 0.5           |
| J2309.8–3627  | 0.9               | 0.0            |               | 0.9             | 0.2            | 0.0           | 2.4           | 0.4            | 0.0           | 2.8            | 2.0            | 0.7           | 4.7              | 1.7            | 0.0           |
| J2310.9+0204  | 0.9               | 0.0            |               | 0.4             | 0.2            | 0.1           | 3.2           | 0.3            | 0.1           | 3.2            | 1.1            | 0.6           | 3.4              | 1.3            | 0.0           |
| J2311.0+3425  | 6.2               | 0.5            | 15.4          | 1.6             | 0.1            | 21.1          | 3.8           | 0.3            | 20.6          | 7.7            | 1.2            | 13.3          | 1.4              | 0.0            | 3.3           |
| J2314.0+1446  | 1.5               | 0.0            |               | 0.4             | 0.3            | 0.0           | 2.0           | 0.7            | 0.2           | 5.5            | 1.3            | 0.6           | 3.6              | 1.4            | 0.5           |
| J2315.7–5014  | 1.4               | 0.0            |               | 1.2             | 0.3            | 0.1           | 4.4           | 0.5            | 0.2           | 4.0            | 2.1            | 0.7           | 5.6              | 0.7            | 0.0           |
| J2317.3–4534  | 1.4               | 0.4            |               | 3.8             | 0.2            | 0.1           | 3.7           | 0.7            | 0.2           | 6.2            | 2.6            | 0.7           | 6.6              | 1.3            | 0.0           |
| J2319.1–4208  | 1.4               | 0.0            |               | 2.4             | 0.2            | 0.0           | 1.4           | 0.3            | 0.0           | 1.4            | 1.9            | 0.0           | 2.5              | 1.7            | 0.0           |
| J2319.3–3830  | 1.5               | 0.0            |               | 2.0             | 0.2            | 0.0           | 1.0           | 0.3            | 0.1           | 3.3            | 1.3            | 0.6           | 3.7              | 0.7            | 0.0           |
| J2321.0+2737  | 2.1               | 0.0            |               | 2.9             | 0.2            | 0.1           | 3.2           | 0.6            | 0.2           | 4.5            | 2.2            | 0.0           | 1.7              | 0.8            | 0.0           |
| J2322.2+3206  | 1.3               | 0.4            |               | 3.3             | 0.6            | 0.1           | 7.7           | 1.1            | 0.2           | 7.4            | 2.9            | 0.8           | 6.0              | 0.8            | 0.0           |
| J2322.6+3435  | 0.6               | 0.0            |               | 0.0             | 0.3            | 0.0           | 3.1           | 0.4            | 0.0           | 1.5            | 1.0            | 0.0           | 0.3              | 1.1            | 0.4           |
| J2323.0–4918  | 1.4               | 0.0            |               | 0.0             | 0.2            | 0.0           | 0.6           | 0.4            | 0.0           | 1.4            | 1.5            | 0.6           | 4.3              | 0.7            | 0.0           |
| J2323.4+5849  | 0.5               | 0.0            |               | 0.0             | 0.6            | 0.1           | 5.0           | 3.3            | 0.4           | 10.5           | 17.2           | 1.8           | 15.4             | 4.5            | 0.8           |
| J2323.6–0316  | 3.4               | 0.5            | 8.0           | 1.0             | 0.1            | 13.5          | 1.7           | 0.2            | 11.2          | 3.8            | 0.9            | 8.0           | 1.1              | 0.0            | 2.5           |
| J2323.8+4212  | 2.0               | 0.5            | 4.9           | 0.4             | 0.1            | 6.2           | 1.5           | 0.2            | 9.6           | 5.7            | 1.0            | 10.3          | 3.5              | 0.7            | 11.8          |
| J2324.6+0801  | 1.2               | 0.0            |               | 0.1             | 0.3            | 0.0           | 2.5           | 0.5            | 0.2           | 4.0            | 1.1            | 0.5           | 3.7              | 1.5            | 0.0           |
| J2324.7–4042  | 1.5               | 0.0            |               | 0.0             | 0.4            | 0.0           | 2.1           | 0.9            | 0.2           | 6.3            | 3.8            | 0.9           | 7.8              | 2.6            | 0.7           |
| J2325.3+3957  | 1.6               | 0.0            |               | 1.3             | 0.6            | 0.1           | 8.3           | 1.6            | 0.2           | 10.6           | 6.5            | 1.1           | 11.0             | 1.5            | 0.5           |
| J2325.3–3557  | 2.1               | 0.4            |               | 7.1             | 0.9            | 0.1           | 15.4          | 2.4            | 0.2           | 16.4           | 5.1            | 1.0           | 10.7             | 0.5            | 0.0           |
| J2325.4+1650  | 1.7               | 0.0            |               | 2.1             | 0.2            | 0.0           | 1.0           | 0.4            | 0.1           | 3.6            | 1.6            | 0.0           | 1.8              | 1.5            | 0.0           |
| J2325.4–4758  | 4.2               | 0.0            |               | 2.5             | 0.3            | 0.1           | 4.3           | 0.6            | 0.2           | 5.2            | 2.0            | 0.7           | 5.1              | 1.4            | 0.0           |
| J2327.5+0940  | 7.3               | 0.9            | 16.0          | 1.5             | 0.1            | 18.9          | 1.9           | 0.2            | 13.0          | 1.6            | 0.6            | 4.7           | 0.5              | 0.0            | 0.0           |
| J2327.9–4037  | 3.1               | 0.6            |               | 3.6             | 0.8            | 0.1           | 7.0           | 1.1            | 0.2           | 7.4            | 2.7            | 0.0           | 2.5              | 0.9            | 0.0           |
| J2329.2+3755  | 1.3               | 0.0            |               | 1.1             | 0.4            | 0.0           | 2.7           | 0.5            | 0.2           | 3.6            | 2.3            | 0.7           | 5.4              | 1.5            | 0.5           |
| J2329.2–4956  | 8.9               | 0.6            | 22.7          | 2.5             | 0.1            | 34.2          | 5.3           | 0.3            | 29.8          | 6.7            | 1.1            | 13.0          | 1.0              | 0.4            | 5.0           |
| J2329.7–4744  | 2.0               | 0.0            |               | 0.1             | 0.4            | 0.0           | 2.1           | 0.5            | 0.2           | 4.3            | 1.4            | 0.0           | 1.5              | 0.7            | 0.0           |
| J2330.2+1107  | 2.8               | 0.0            |               | 2.7             | 0.4            | 0.0           | 3.1           | 0.7            | 0.0           | 3.0            | 1.4            | 0.0           | 1.6              | 0.5            | 0.0           |
| J2330.6–3723  | 1.1               | 0.0            |               | 0.5             | 0.2            | 0.0           | 1.5           | 0.5            | 0.0           | 2.7            | 1.3            | 0.6           | 4.0              | 1.1            | 0.0           |
| J2330.9–2144  | 3.8               | 0.4            | 10.1          | 1.0             | 0.1            | 14.9          | 1.8           | 0.2            | 12.6          | 3.8            | 0.9            | 8.0           | 0.8              | 0.0            | 1.6           |
| J2331.8–1607  | 1.2               | 0.0            |               | 1.4             | 0.3            | 0.0           | 3.1           | 0.5            | 0.1           | 5.2            | 1.7            | 0.6           | 4.5              | 0.6            | 0.0           |
| J2332.5–5535  | 1.6               | 0.0            |               | 2.7             | 0.3            | 0.0           | 3.0           | 0.6            | 0.1           | 5.8            | 1.9            | 0.7           | 4.6              | 0.5            | 0.0           |
| J2333.3+6237  | 3.5               | 0.0            |               | 2.1             | 1.1            | 0.2           | 6.5           | 1.0            | 0.3           | 3.3            | 1.9            | 0.0           | 0.5              | 1.5            | 0.0           |
| J2334.3+0734  | 2.1               | 0.5            |               | 4.4             | 0.4            | 0.1           | 6.0           | 0.7            | 0.2           | 5.4            | 1.9            | 0.0           | 2.2              | 1.1            | 0.0           |
| J2334.8+1431  | 0.9               | 0.0            |               | 0.5             | 0.2            | 0.0           | 1.7           | 0.7            | 0.2           | 5.6            | 4.0            | 0.9           | 8.5              | 0.8            | 0.4           |

Table 1—Continued

|               | 100 MeV – 300 MeV |                |               | 300 MeV – 1 GeV |                |               | 1 GeV – 3 GeV |                |               | 3 GeV – 10 GeV |                |               | 10 GeV – 100 GeV |                |               |
|---------------|-------------------|----------------|---------------|-----------------|----------------|---------------|---------------|----------------|---------------|----------------|----------------|---------------|------------------|----------------|---------------|
| Name 2FGL     | $F_1^a$           | $\Delta F_1^a$ | $\sqrt{TS_1}$ | $F_2^a$         | $\Delta F_2^a$ | $\sqrt{TS_2}$ | $F_3^b$       | $\Delta F_3^b$ | $\sqrt{TS_3}$ | $F_4^c$        | $\Delta F_4^c$ | $\sqrt{TS_4}$ | $F_5^c$          | $\Delta F_5^c$ | $\sqrt{TS_5}$ |
| J2336.3–4111  | 2.0               | 0.0            |               | 2.9             | 0.5            | 0.1           | 7.6           | 1.4            | 0.2           | 11.3           | 1.3            | 0.5           | 3.8              | 0.9            | 1.1           |
| J2338.1–0229  | 3.3               | 0.5            |               | 7.6             | 0.8            | 0.1           | 11.8          | 1.5            | 0.2           | 10.4           | 2.4            | 0.8           | 5.5              | 1.4            | 3.2           |
| J2339.0+2125  | 1.2               | 0.0            |               | 1.4             | 0.2            | 0.0           | 2.0           | 0.4            | 0.0           | 1.4            | 1.1            | 0.5           | 3.6              | 1.6            | 4.4           |
| J2339.6–0532  | 1.4               | 0.3            |               | 5.5             | 0.6            | 0.1           | 11.4          | 4.3            | 0.3           | 25.1           | 8.7            | 1.3           | 14.3             | 0.9            | 5.1           |
| J2341.7+8016  | 1.8               | 0.0            |               | 2.5             | 0.4            | 0.1           | 6.0           | 1.9            | 0.2           | 11.4           | 7.6            | 1.1           | 12.7             | 2.2            | 9.5           |
| J2343.3–4752  | 1.7               | 0.0            |               | 2.3             | 0.2            | 0.1           | 4.5           | 0.4            | 0.1           | 4.5            | 1.9            | 0.0           | 2.5              | 1.1            | 2.4           |
| J2343.6+3437  | 0.8               | 0.0            |               | 0.6             | 0.1            | 0.0           | 0.3           | 0.4            | 0.0           | 1.3            | 2.0            | 0.0           | 2.2              | 1.4            | 4.4           |
| J2345.0–1553  | 3.3               | 0.8            |               | 4.2             | 1.4            | 0.1           | 14.8          | 3.2            | 0.3           | 18.2           | 9.4            | 1.3           | 14.9             | 1.1            | 5.2           |
| J2347.0+5142  | 0.5               | 0.0            |               | 0.0             | 0.2            | 0.1           | 3.6           | 1.3            | 0.2           | 8.2            | 3.0            | 0.8           | 5.8              | 2.4            | 10.1          |
| J2347.2+0707  | 0.7               | 0.0            |               | 0.0             | 0.3            | 0.1           | 3.8           | 0.5            | 0.0           | 1.8            | 2.0            | 0.7           | 5.2              | 0.8            | 4.1           |
| J2347.9–1629  | 3.4               | 0.9            |               | 4.1             | 0.7            | 0.1           | 7.4           | 1.0            | 0.2           | 7.0            | 3.3            | 0.9           | 7.2              | 1.0            | 2.6           |
| J2350.2–3002  | 2.8               | 0.0            |               | 2.1             | 0.3            | 0.0           | 2.1           | 0.5            | 0.1           | 4.1            | 1.9            | 0.0           | 3.1              | 1.4            | 3.5           |
| J2351.6–7558  | 0.8               | 0.0            |               | 0.1             | 0.2            | 0.0           | 0.7           | 0.4            | 0.1           | 4.0            | 2.3            | 0.0           | 2.7              | 1.0            | 1.4           |
| J2352.0+1753  | 1.3               | 0.0            |               | 1.6             | 0.2            | 0.0           | 2.3           | 0.6            | 0.2           | 6.1            | 1.2            | 0.5           | 3.8              | 1.7            | 4.1           |
| J2353.3+6643c | 2.7               | 0.0            |               | 0.0             | 1.1            | 0.2           | 6.8           | 1.6            | 0.0           | 3.2            | 3.9            | 0.0           | 2.8              | 1.3            | 2.6           |
| J2353.5–3034  | 2.2               | 0.0            |               | 0.5             | 0.3            | 0.0           | 2.4           | 0.4            | 0.1           | 4.2            | 1.4            | 0.6           | 4.4              | 0.8            | 1.7           |
| J2354.2–6615  | 0.6               | 0.0            |               | 0.0             | 0.2            | 0.1           | 3.8           | 0.4            | 0.1           | 4.3            | 2.2            | 0.0           | 2.7              | 0.7            | 1.2           |
| J2356.0–5256  | 2.2               | 0.4            |               | 5.4             | 0.5            | 0.1           | 8.0           | 0.9            | 0.2           | 6.6            | 2.0            | 0.0           | 1.7              | 0.8            | 2.0           |
| J2356.1+4034  | 1.0               | 0.0            |               | 0.9             | 0.2            | 0.0           | 1.2           | 0.4            | 0.0           | 1.4            | 2.4            | 0.7           | 5.5              | 0.9            | 3.8           |
| J2356.3+0432  | 1.6               | 0.5            |               | 3.5             | 0.3            | 0.0           | 2.7           | 0.3            | 0.0           | 0.9            | 1.9            | 0.0           | 2.2              | 0.6            | 0.0           |
| J2358.4–1811  | 1.2               | 0.0            |               | 1.4             | 0.1            | 0.0           | 0.0           | 0.3            | 0.1           | 3.3            | 1.4            | 0.6           | 4.4              | 0.7            | 0.1           |
| J2358.9+6325  | 2.8               | 1.1            |               | 3.5             | 0.9            | 0.2           | 5.8           | 1.1            | 0.0           | 2.1            | 3.4            | 0.0           | 2.5              | 0.5            | 0.0           |
| J2359.0–3037  | 1.2               | 0.0            |               | 0.4             | 0.2            | 0.0           | 1.7           | 0.5            | 0.1           | 4.8            | 1.3            | 0.5           | 3.8              | 0.7            | 4.4           |
| J2359.4+6751c | 3.7               | 0.9            |               | 4.9             | 0.6            | 0.2           | 3.7           | 1.1            | 0.3           | 3.8            | 2.8            | 0.0           | 1.8              | 0.5            | 0.0           |
| J2359.6+6543c | 4.8               | 0.0            |               | 2.4             | 0.9            | 0.2           | 5.6           | 1.9            | 0.4           | 5.6            | 2.8            | 1.0           | 4.0              | 1.8            | 2.8           |

Note. — This table is published in its entirety in the electronic edition of the Astrophysical Journal Supplements. A portion is shown here for guidance regarding its form and content.

<sup>a</sup>In units of  $10^{-8}$  photons  $\text{cm}^{-2} \text{s}^{-1}$

<sup>b</sup>In units of  $10^{-9}$  photons  $\text{cm}^{-2} \text{s}^{-1}$

<sup>c</sup>In units of  $10^{-10}$  photons  $\text{cm}^{-2} \text{s}^{-1}$
