# Supplementary material for: Fermi Large Area Telescope Second Source Catalog
Source: arXiv:1108.1435 ancillary file (2012-02-23)
Supplement: Supplementary file 3 [file table8_full.pdf]

Table 1. List of 1FGL sources not in the 2FGL catalog

| 1FGL          | 1FGL Assoc. <sup>(a)</sup> | $l^{(a)}$<br>(deg.) | $b^{(a)}$<br>(deg.) | $\theta_{95}^{(a)}$<br>(deg.) | $\sigma^{(a)}$ | $\Gamma_{25}^{(a)}$ | $p > 90\%$ | 2FGL <sup>(b)</sup><br>$(\Delta < d_{99.9})$ | 2FGL <sup>(c)</sup><br>$(d_{99.9} < \Delta < 1^\circ)$ | $\Delta^{(d)}$<br>(deg.) | $\Delta / d_{99.9}$ | 2FGL <sup>(e)</sup> Flags <sup>(f)</sup><br>Seed |
|---------------|----------------------------|---------------------|---------------------|-------------------------------|----------------|---------------------|------------|----------------------------------------------|--------------------------------------------------------|--------------------------|---------------------|--------------------------------------------------|
| J0000.8+6600c | ...                        | 117.812             | 3.635               | 0.112                         | 9.8            | 2.60                | ...        | ...                                          | J2359.6+6543c                                          | 0.298                    | 1.241               | ... S                                            |
| J0006.9+4652  | ...                        | 115.082             | -15.311             | 0.194                         | 10.2           | 2.55                | T          | ...                                          | J0007.8+4713                                           | 0.381                    | 1.249               | T S                                              |
| J0008.3+1452  | ...                        | 107.655             | -46.708             | 0.144                         | 4.7            | 2.00                | ...        | ...                                          | ...                                                    | ...                      | ...                 | T C                                              |
| J0013.7-5022  | BZB J0014-5022             | 317.624             | -65.666             | 0.151                         | 4.4            | 2.23                | ...        | ...                                          | ...                                                    | ...                      | ...                 | T C                                              |
| J0016.6+1706  | ...                        | 111.135             | -44.964             | 0.197                         | 4.7            | 2.57                | ...        | ...                                          | ...                                                    | ...                      | ...                 | ... NC                                           |
| J0019.3+2017  | PKS 0017+200               | 112.787             | -41.944             | 0.203                         | 5.9            | 2.38                | ...        | ...                                          | ...                                                    | ...                      | ...                 | T C                                              |
| J0028.9-7028  | ...                        | 305.664             | -46.535             | 0.172                         | 6.3            | 2.19                | ...        | J0029.2-7043                                 | ...                                                    | 0.253                    | 0.704               | T C                                              |
| J0038.6+2048  | ...                        | 118.912             | -41.969             | 0.146                         | 4.6            | 1.63                | ...        | ...                                          | ...                                                    | ...                      | ...                 | ... NC                                           |
| J0041.9+2318  | PKS 0039+230               | 120.104             | -39.515             | 0.221                         | 5.0            | 2.52                | ...        | ...                                          | ...                                                    | ...                      | ...                 | T C                                              |
| J0059.6+1904  | ...                        | 125.615             | -43.751             | 0.091                         | 5.8            | 2.39                | ...        | ...                                          | ...                                                    | ...                      | ...                 | ... BC                                           |
| J0110.0-4023  | ...                        | 287.889             | -76.190             | 0.085                         | 4.2            | 1.34                | ...        | ...                                          | ...                                                    | ...                      | ...                 | T C                                              |
| J0122.2+5200  | ...                        | 127.740             | -10.571             | 0.168                         | 4.1            | 2.18                | ...        | ...                                          | ...                                                    | ...                      | ...                 | T C                                              |
| J0136.3-2220  | ...                        | 190.201             | -78.746             | 0.113                         | 4.6            | 1.60                | ...        | ...                                          | ...                                                    | ...                      | ...                 | ... BC                                           |
| J0147.4+1547  | ...                        | 142.143             | -44.981             | 0.119                         | 4.9            | 1.81                | ...        | ...                                          | ...                                                    | ...                      | ...                 | T C                                              |
| J0202.1+0849  | RX J0202.4+0849            | 150.851             | -50.172             | 0.120                         | 4.5            | 1.97                | ...        | ...                                          | ...                                                    | ...                      | ...                 | T C                                              |
| J0208.6+3522  | BZB J0208+3523             | 140.222             | -24.884             | 0.046                         | 6.3            | 1.68                | ...        | ...                                          | ...                                                    | ...                      | ...                 | T C                                              |
| J0214.1+6020  | ...                        | 133.000             | -0.899              | 0.162                         | 4.3            | 2.10                | ...        | ...                                          | ...                                                    | ...                      | ...                 | T C                                              |
| J0218.8+6158c | ...                        | 133.007             | 0.823               | 0.144                         | 7.4            | 2.35                | ...        | J0218.7+6208c                                | ...                                                    | 0.168                    | 0.685               | T S                                              |
| J0226.0+3922  | ...                        | 142.200             | -19.934             | 0.359                         | 5.3            | 2.88                | ...        | ...                                          | ...                                                    | ...                      | ...                 | T C                                              |
| J0233.4+6654  | ...                        | 132.715             | 5.989               | 0.043                         | 4.6            | 1.61                | ...        | ...                                          | ...                                                    | ...                      | ...                 | ... NC                                           |
| J0247.4-6003  | ...                        | 279.996             | -51.598             | 0.099                         | 4.4            | 1.90                | ...        | ...                                          | ...                                                    | ...                      | ...                 | ... O                                            |
| J0256.1+0323  | ...                        | 172.399             | -47.152             | 0.166                         | 5.6            | 2.23                | ...        | ...                                          | ...                                                    | ...                      | ...                 | T C                                              |
| J0256.9+2920  | ...                        | 153.270             | -26.027             | 0.116                         | 4.2            | 1.69                | ...        | ...                                          | ...                                                    | ...                      | ...                 | ... NC                                           |

Table 1—Continued

| 1FGL         | 1FGL Assoc. <sup>(a)</sup> | $l^{(a)}$<br>(deg.) | $b^{(a)}$<br>(deg.) | $\theta_{95}^{(a)}$<br>(deg.) | $\sigma^{(a)}$ | $\Gamma_{25}^{(a)}$ | $\text{Var}^{(a)}$<br>$p > 90\%$ | 2FGL <sup>(b)</sup><br>$(\Delta < d_{99,9})$ | 2FGL <sup>(c)</sup><br>$(d_{99,9} < \Delta < 1^\circ)$ | $\Delta^{(d)}$<br>(deg.) | $\Delta / d_{99,9}$ | 2FGL <sup>(e)</sup><br>Seed | Flags <sup>(f)</sup> |
|--------------|----------------------------|---------------------|---------------------|-------------------------------|----------------|---------------------|----------------------------------|----------------------------------------------|--------------------------------------------------------|--------------------------|---------------------|-----------------------------|----------------------|
| J0259.9+5925 | ...                        | 138.629             | 0.523               | 0.199                         | 4.4            | 2.44                | ...                              | ...                                          | J0253.9+5908                                           | 0.823                    | 2.012               | ...                         | BC                   |
| J0305.0-0601 | CRATES J0305-0607          | 185.421             | -51.874             | 0.204                         | 4.7            | 2.05                | ...                              | ...                                          | ...                                                    | ...                      | ...                 | ...                         | NC, V                |
| J0308.3+0403 | NGC 1218                   | 174.884             | -44.566             | 0.074                         | 5.2            | 1.86                | ...                              | ...                                          | ...                                                    | ...                      | ...                 | T                           | C                    |
| J0311.3-0922 | ...                        | 191.349             | -52.533             | 0.138                         | 6.4            | 2.35                | ...                              | ...                                          | J0312.5-0914                                           | 0.320                    | 1.079               | ...                         | O                    |
| J0334.2+3233 | ...                        | 158.445             | -18.859             | 0.505                         | 6.3            | 2.81                | ...                              | J0337.0+3200c                                | ...                                                    | 0.808                    | 0.990               | T                           | C                    |
| J0336.0+7845 | ...                        | 130.709             | 18.450              | 0.071                         | 4.4            | 1.79                | ...                              | ...                                          | ...                                                    | ...                      | ...                 | T                           | C                    |
| J0338.8+1313 | ...                        | 173.496             | -32.742             | 0.092                         | 5.0            | 1.78                | ...                              | J0338.2+1306                                 | ...                                                    | 0.188                    | 0.894               | T                           | C                    |
| J0343.4-2536 | PKS 0341-256               | 220.700             | -51.637             | 0.286                         | 5.0            | 2.75                | T                                | ...                                          | ...                                                    | ...                      | ...                 | T                           | C                    |
| J0402.2+6810 | ...                        | 139.235             | 11.578              | 0.120                         | 4.4            | 0.99                | ...                              | ...                                          | ...                                                    | ...                      | ...                 | ...                         | NC <sub>1</sub>      |
| J0404.5-0850 | ...                        | 200.459             | -40.939             | 0.196                         | 4.6            | 2.08                | ...                              | ...                                          | ...                                                    | ...                      | ...                 | T                           | C <sub>1</sub>       |
| J0411.6+5459 | ...                        | 149.049             | 2.619               | 0.141                         | 4.4            | 1.85                | ...                              | ...                                          | ...                                                    | ...                      | ...                 | T                           | C                    |
| J0412.2+2103 | ...                        | 173.373             | -21.582             | 0.257                         | 4.8            | 2.65                | T                                | ...                                          | ...                                                    | ...                      | ...                 | ...                         | NC, Sun              |
| J0419.0+3811 | 3C 111                     | 161.653             | -8.607              | 0.287                         | 4.3            | 2.61                | ...                              | ...                                          | ...                                                    | ...                      | ...                 | T                           | C                    |
| J0422.1+0211 | PKS 0420+022               | 191.589             | -31.455             | 0.276                         | 4.4            | 2.54                | ...                              | ...                                          | ...                                                    | ...                      | ...                 | ...                         | NC, V                |
| J0427.3+2028 | ...                        | 176.342             | -19.314             | 0.114                         | 4.7            | 1.44                | ...                              | ...                                          | ...                                                    | ...                      | ...                 | T                           | C                    |
| J0427.9+5556 | ...                        | 150.023             | 4.918               | 0.145                         | 4.8            | 1.47                | ...                              | ...                                          | J0423.4+5612                                           | 0.677                    | 1.860               | ...                         | S                    |
| J0439.6-0538 | ...                        | 202.137             | -31.776             | 0.153                         | 4.1            | 1.46                | ...                              | ...                                          | ...                                                    | ...                      | ...                 | ...                         | NC                   |
| J0445.2-6008 | ...                        | 269.931             | -38.844             | 0.196                         | 4.6            | 1.98                | ...                              | ...                                          | ...                                                    | ...                      | ...                 | T                           | C                    |
| J0459.7-6921 | LMC field                  | 280.572             | -35.005             | 0.183                         | 6.4            | 2.49                | ...                              | J0455.8-6920                                 | ...                                                    | 0.342                    | 0.961               | T                           | C, LMC               |
| J0500.1+5237 | ...                        | 155.626             | 6.336               | 0.049                         | 5.6            | 1.59                | ...                              | ...                                          | ...                                                    | ...                      | ...                 | T                           | C                    |
| J0500.8+3437 | ...                        | 169.938             | -4.633              | 0.088                         | 4.5            | 2.11                | ...                              | ...                                          | ...                                                    | ...                      | ...                 | T                           | C                    |
| J0502.9+1857 | ...                        | 182.946             | -13.636             | 0.325                         | 4.2            | 2.48                | ...                              | ...                                          | ...                                                    | ...                      | ...                 | T                           | C                    |
| J0513.0+4048 | ...                        | 166.426             | 1.007               | 0.087                         | 5.2            | 1.65                | ...                              | J0512.9+4040                                 | ...                                                    | 0.139                    | 0.670               | T                           | C                    |

Table 1—Continued

| 1FGL          | 1FGL Assoc. <sup>(a)</sup> | $l^{(a)}$<br>(deg.) | $b^{(a)}$<br>(deg.) | $\theta_{95}^{(a)}$<br>(deg.) | $\sigma^{(a)}$ | $\Gamma_{25}^{(a)}$ | $\text{Var}^{(a)}$<br>$p > 90\%$ | 2FGL <sup>(b)</sup><br>$(\Delta < d_{99.9})$ | 2FGL <sup>(c)</sup><br>$(d_{99.9} < \Delta < 1^\circ)$ | $\Delta^{(d)}$<br>$(\text{deg.})$ | $\Delta/d_{99.9}$ | 2FGL <sup>(e)</sup><br>Seed | Flags <sup>(f)</sup> |
|---------------|----------------------------|---------------------|---------------------|-------------------------------|----------------|---------------------|----------------------------------|----------------------------------------------|--------------------------------------------------------|-----------------------------------|-------------------|-----------------------------|----------------------|
| J0517.6–1737  | ...                        | 219.241             | –28.404             | 0.170                         | 5.7            | 2.40                | ...                              | ...                                          | ...                                                    | ...                               | ...               | T                           | C                    |
| J0518.6–7222  | LMC field                  | 283.615             | –32.732             | 0.151                         | 4.3            | 2.23                | ...                              | ...                                          | ...                                                    | ...                               | ...               | ...                         | NC, LMC              |
| J0520.2+2632  | ...                        | 178.956             | –6.013              | 0.086                         | 6.8            | 2.77                | T                                | ...                                          | ...                                                    | ...                               | ...               | T                           | C                    |
| J0527.6+6646  | ...                        | 145.589             | 17.068              | 0.111                         | 4.1            | 2.09                | ...                              | ...                                          | ...                                                    | ...                               | ...               | T                           | C                    |
| J0528.4+3838  | ...                        | 169.898             | 2.200               | 0.258                         | 4.9            | 2.45                | T                                | J0529.3+3821                                 | ...                                                    | 0.344                             | 0.802             | T                           | C                    |
| J0531.3–6716  | LMC field                  | 277.429             | –32.567             | 0.195                         | 12.4           | 2.58                | ...                              | ...                                          | J0533.3–6651                                           | 0.471                             | 1.031             | T                           | S                    |
| J0534.7–0531c | ...                        | 209.074             | –19.560             | 0.104                         | 6.9            | 2.37                | ...                              | ...                                          | J0534.8–0548                                           | 0.291                             | 1.230             | ...                         | O, Ori               |
| J0536.2–0607c | ...                        | 209.826             | –19.500             | 0.145                         | 4.4            | 2.34                | ...                              | ...                                          | ...                                                    | ...                               | ...               | ...                         | NC, Ori              |
| J0538.9–6914  | LMC field                  | 279.625             | –31.634             | 0.075                         | 26.2           | 2.35                | T                                | ...                                          | ...                                                    | ...                               | ...               | T                           | C <sub>LMC</sub>     |
| J0539.4–0400  | CRATES J0539–0356          | 208.224             | –17.826             | 0.281                         | 4.1            | 2.46                | ...                              | ...                                          | J0539.3–0323                                           | 0.621                             | 1.287             | ...                         | O, Ori               |
| J0540.4–0737c | ...                        | 211.744             | –19.224             | 0.100                         | 4.7            | 2.16                | ...                              | ...                                          | ...                                                    | ...                               | ...               | ...                         | NC, Ori              |
| J0540.9–0547  | PKS 0539–057               | 210.058             | –18.309             | 0.387                         | 6.3            | 2.37                | ...                              | J0538.5–0534c                                | ...                                                    | 0.620                             | 0.941             | T                           | S, Ori               |
| J0549.9+2654c | ...                        | 182.232             | –0.241              | 0.188                         | 5.7            | 2.72                | ...                              | ...                                          | ...                                                    | ...                               | ...               | ...                         | BC                   |
| J0550.8–4400  | ...                        | 250.425             | –28.944             | 0.153                         | 5.2            | 1.61                | ...                              | ...                                          | J0555.9–4348                                           | 0.926                             | 2.629             | ...                         | NC                   |
| J0551.6+0449c | ...                        | 201.656             | –10.965             | 0.248                         | 5.1            | 2.71                | ...                              | ...                                          | ...                                                    | ...                               | ...               | ...                         | NC                   |
| J0622.3–2604  | CRATES J0622–2606          | 233.780             | –17.555             | 0.092                         | 7.1            | 2.00                | ...                              | ...                                          | J0620.8–2556                                           | 0.351                             | 1.103             | T                           | S                    |
| J0623.5+3330  | ...                        | 179.936             | 9.306               | 0.119                         | 5.3            | 2.07                | ...                              | J0622.9+3326                                 | ...                                                    | 0.138                             | 0.721             | T                           | C                    |
| J0625.7+0001  | ...                        | 209.966             | –5.702              | 0.133                         | 4.6            | 1.02                | ...                              | ...                                          | ...                                                    | ...                               | ...               | ...                         | BC                   |
| J0625.9–0613  | ...                        | 215.606             | –8.501              | 0.161                         | 4.8            | 2.62                | ...                              | ...                                          | ...                                                    | ...                               | ...               | ...                         | NC                   |
| J0625.9–5430  | CGRaBS J0625–5438          | 263.248             | –25.385             | 0.272                         | 5.8            | 3.00                | ...                              | ...                                          | ...                                                    | ...                               | ...               | ...                         | BC                   |
| J0630.1+0622  | ...                        | 204.836             | –1.805              | 0.105                         | 6.9            | 2.24                | ...                              | ...                                          | J0631.6+0640                                           | 0.491                             | 2.400             | ...                         | BC, Monoceros Loop   |
| J0636.0+0458c | ...                        | 206.742             | –1.147              | 0.072                         | 8.0            | 2.27                | ...                              | ...                                          | ...                                                    | ...                               | ...               | T                           | C                    |
| J0641.5+1023c | ...                        | 202.550             | 2.547               | 0.169                         | 4.5            | 2.20                | ...                              | J0641.1+1006c                                | ...                                                    | 0.306                             | 0.866             | T                           | C                    |

Table 1—Continued

| 1FGL          | 1FGL Assoc. <sup>(a)</sup> | $l^{(a)}$<br>(deg.) | $b^{(a)}$<br>(deg.) | $\theta_{95}^{(a)}$<br>(deg.) | $\sigma^{(a)}$ | $\Gamma_{25}^{(a)}$ | $\text{Var}^{(a)}$<br>$p > 90\%$ | 2FGL <sup>(b)</sup><br>$(\Delta < d_{99,9})$ | 2FGL <sup>(c)</sup><br>$(d_{99,9} < \Delta < 1^\circ)$ | $\Delta^{(d)}$<br>(deg.) | $\Delta/d_{99,9}$ | 2FGL <sup>(e)</sup> Flags <sup>(f)</sup><br>Seed |
|---------------|----------------------------|---------------------|---------------------|-------------------------------|----------------|---------------------|----------------------------------|----------------------------------------------|--------------------------------------------------------|--------------------------|-------------------|--------------------------------------------------|
| J0645.5+0446  | ...                        | 208.014             | 0.856               | 0.373                         | 5.2            | 2.76                | ...                              | ...                                          | ...                                                    | ...                      | ...               | NC                                               |
| J0651.1–3022  | ...                        | 240.448             | –13.392             | 0.185                         | 4.4            | 2.31                | ...                              | ...                                          | ...                                                    | ...                      | ...               | NC                                               |
| J0653.6+8236  | ...                        | 131.223             | 26.954              | 0.072                         | 4.7            | 1.43                | ...                              | ...                                          | ...                                                    | ...                      | ...               | NC                                               |
| J0659.9+1303  | ...                        | 202.199             | 7.766               | 0.124                         | 4.1            | 2.11                | ...                              | ...                                          | ...                                                    | ...                      | ...               | C                                                |
| J0709.0–1116  | ...                        | 224.959             | –1.274              | 0.094                         | 5.3            | 1.33                | ...                              | ...                                          | ...                                                    | ...                      | ...               | NC                                               |
| J0722.3+5837  | BZB J0723+5841             | 158.255             | 26.849              | 0.144                         | 4.6            | 2.16                | ...                              | ...                                          | ...                                                    | ...                      | ...               | NC, V                                            |
| J0724.1–3522  | ...                        | 248.070             | –9.247              | 0.096                         | 6.0            | 2.44                | ...                              | ...                                          | ...                                                    | ...                      | ...               | BC                                               |
| J0724.7–2223c | ...                        | 236.544             | –3.126              | 0.099                         | 5.9            | 2.50                | ...                              | ...                                          | ...                                                    | ...                      | ...               | BC                                               |
| J0724.7–4714  | ...                        | 259.043             | –14.315             | 0.186                         | 5.0            | 2.45                | ...                              | J0727.0–4726                                 | 0.441                                                  | 0.082                    | 1.016             | O 4                                              |
| J0725.3+1431  | 4C +14.23                  | 203.561             | 13.978              | 0.077                         | 17.0           | 2.39                | T                                | J0725.3+1426                                 | ...                                                    | 0.082                    | 0.669             | T C                                              |
| J0731.2–1910c | ...                        | 234.445             | –0.250              | 0.172                         | 5.0            | 2.52                | ...                              | ...                                          | ...                                                    | ...                      | ...               | C                                                |
| J0731.9–1517  | ...                        | 231.119             | 1.757               | 0.115                         | 4.5            | 2.05                | ...                              | ...                                          | ...                                                    | ...                      | ...               | NC                                               |
| J0736.4+4053  | ...                        | 178.123             | 25.459              | 0.074                         | 5.0            | 2.00                | ...                              | ...                                          | ...                                                    | ...                      | ...               | C                                                |
| J0742.1–4849c | ...                        | 261.819             | –12.398             | 0.474                         | 5.1            | 2.92                | ...                              | ...                                          | ...                                                    | ...                      | ...               | NC                                               |
| J0747.1–2333  | ...                        | 240.087             | 0.807               | 0.205                         | 4.9            | 2.38                | ...                              | ...                                          | ...                                                    | ...                      | ...               | O                                                |
| J0753.1+4649  | ...                        | 172.303             | 29.646              | 0.068                         | 4.3            | 2.00                | ...                              | ...                                          | ...                                                    | ...                      | ...               | NC                                               |
| J0753.6–2718  | ...                        | 244.072             | 0.168               | 0.169                         | 4.9            | 2.28                | ...                              | ...                                          | ...                                                    | ...                      | ...               | NC                                               |
| J0809.4+3455  | B2 0806+35                 | 186.459             | 30.305              | 0.123                         | 4.8            | 1.77                | ...                              | ...                                          | ...                                                    | ...                      | ...               | T C                                              |
| J0827.9–3738  | PKS B0826–373              | 256.657             | 0.541               | 0.226                         | 5.7            | 2.68                | T                                | ...                                          | ...                                                    | ...                      | ...               | BC                                               |
| J0828.9+0901  | ...                        | 215.881             | 25.732              | 0.104                         | 5.1            | 1.52                | ...                              | ...                                          | ...                                                    | ...                      | ...               | T C                                              |
| J0835.4+0936  | CRATES J0835+0937          | 216.079             | 27.444              | 0.081                         | 5.0            | 1.41                | ...                              | ...                                          | ...                                                    | ...                      | ...               | NC, V                                            |
| J0841.9–4620  | ...                        | 265.181             | –2.580              | 0.275                         | 5.1            | 1.99                | ...                              | ...                                          | ...                                                    | ...                      | ...               | T C                                              |
| J0842.2+0251  | BZB J0842+0252             | 223.643             | 25.839              | 0.074                         | 5.8            | 1.81                | ...                              | ...                                          | ...                                                    | ...                      | ...               | BC                                               |

Table 1—Continued

| 1FGL          | 1FGL Assoc. <sup>(a)</sup> | $l^{(a)}$<br>(deg.) | $b^{(a)}$<br>(deg.) | $\theta_{95}^{(a)}$<br>(deg.) | $\sigma^{(a)}$ | $\Gamma_{25}^{(a)}$ | $\text{Var}^{(a)}$<br>$p > 90\%$ | 2FGL <sup>(b)</sup><br>$(\Delta < d_{99.9})$ | 2FGL <sup>(c)</sup><br>$(d_{99.9} < \Delta < 1^\circ)$ | $\Delta^{(d)}$<br>(deg.) | $\Delta / d_{99.9}$ | 2FGL <sup>(e)</sup><br>Seed | Flags <sup>(f)</sup>      |
|---------------|----------------------------|---------------------|---------------------|-------------------------------|----------------|---------------------|----------------------------------|----------------------------------------------|--------------------------------------------------------|--------------------------|---------------------|-----------------------------|---------------------------|
| J0845.5–4327c | ...                        | 263.304             | −0.299              | 0.203                         | 4.9            | 2.13                | ...                              | ...                                          | J0848.7–4324                                           | 0.590                    | 1.552               | ...                         | BC                        |
| J0845.9–0713  | ...                        | 233.610             | 21.455              | 0.180                         | 5.4            | 2.35                | ...                              | ...                                          | J0848.1–0703                                           | 0.558                    | 1.424               | ...                         | NC                        |
| J0847.4+1517  | ...                        | 211.482             | 32.439              | 0.088                         | 4.6            | 2.47                | ...                              | ...                                          | ...                                                    | ...                      | ...                 | T                           | C                         |
| J0849.0–6754  | ...                        | 283.102             | −14.962             | 0.247                         | 4.1            | 3.21                | ...                              | ...                                          | ...                                                    | ...                      | ...                 | ...                         | NC                        |
| J0849.4–2912  | ...                        | 252.614             | 9.203               | 0.148                         | 4.4            | 2.08                | ...                              | ...                                          | ...                                                    | ...                      | ...                 | T                           | C                         |
| J0850.2+3457  | RX J0850.6+3455            | 188.407             | 38.517              | 0.143                         | 4.6            | 2.03                | ...                              | ...                                          | ...                                                    | ...                      | ...                 | T                           | C                         |
| J0854.0–4632  | ...                        | 266.642             | −1.087              | 0.157                         | 7.8            | 2.10                | ...                              | J0855.4–4625                                 | ...                                                    | 0.274                    | 0.951               | T                           | S, NC, Vela Junior        |
| J0857.7–4345  | ...                        | 264.946             | 1.213               | 0.139                         | 6.9            | 2.36                | ...                              | J0858.3–4333                                 | ...                                                    | 0.229                    | 0.753               | T                           | C                         |
| J0857.9–2553  | ...                        | 251.171             | 12.752              | 0.243                         | 5.2            | 2.57                | ...                              | ...                                          | J0859.4–2532                                           | 0.497                    | 1.209               | ...                         | O $\frac{1}{2}$ $\zeta^A$ |
| J0900.5+3410  | ...                        | 189.832             | 40.490              | 0.281                         | 4.1            | 2.24                | ...                              | ...                                          | ...                                                    | ...                      | ...                 | T                           | C $\frac{1}{2}$           |
| J0919.6+6216  | OK 630                     | 152.287             | 40.770              | 0.213                         | 7.9            | 2.70                | T                                | J0921.9+6216                                 | ...                                                    | 0.276                    | 0.762               | T                           | S                         |
| J0926.9+1452  | ...                        | 216.590             | 41.071              | 0.338                         | 4.7            | 2.73                | T                                | ...                                          | J0923.5+1508                                           | 0.856                    | 1.480               | ...                         | NC, Sun                   |
| J0942.1+4313  | ...                        | 177.279             | 48.750              | 0.088                         | 5.4            | 1.29                | ...                              | ...                                          | ...                                                    | ...                      | ...                 | ...                         | NC                        |
| J0949.8+1757  | CRATES J0949+1752          | 215.484             | 47.305              | 0.162                         | 5.0            | 2.44                | ...                              | ...                                          | ...                                                    | ...                      | ...                 | T                           | C                         |
| J0952.2+3926  | BZB J0952+3936             | 182.831             | 51.032              | 0.127                         | 4.4            | 2.50                | ...                              | ...                                          | ...                                                    | ...                      | ...                 | ...                         | NC, V                     |
| J1006.3–5648  | ...                        | 281.760             | −0.887              | 0.116                         | 7.4            | 2.44                | ...                              | ...                                          | J1010.7–5643c                                          | 0.614                    | 2.161               | ...                         | BC                        |
| J1007.0+3454  | BZB J1006+3454             | 190.064             | 54.194              | 0.061                         | 4.2            | 1.77                | ...                              | ...                                          | ...                                                    | ...                      | ...                 | ...                         | NC, V                     |
| J1014.0–3146  | ...                        | 267.881             | 20.184              | 0.315                         | 4.6            | 2.40                | ...                              | ...                                          | J1009.7–3123                                           | 0.988                    | 1.815               | ...                         | BC                        |
| J1018.6–5856  | 0FGL J1018.2–5858          | 284.323             | −1.701              | 0.030                         | 43.0           | 2.33                | ...                              | J1019.0–5856                                 | ...                                                    | 0.045                    | 0.790               | T                           | C                         |
| J1023.0–5746  | LAT PSR J1023–5746         | 284.166             | −0.409              | 0.000                         | 29.3           | 2.22                | ...                              | ...                                          | J1022.7–5741                                           | 0.083                    | 1.162               | ...                         | S                         |
| J1029.2–6422  | ...                        | 288.293             | −5.623              | 0.289                         | 5.5            | 2.93                | ...                              | ...                                          | ...                                                    | ...                      | ...                 | ...                         | NC                        |
| J1034.7+7353  | ...                        | 134.668             | 39.973              | 0.142                         | 6.7            | 2.53                | ...                              | ...                                          | J1029.9+7437                                           | 0.801                    | 2.701               | ...                         | BC                        |
| J1040.9–1205  | ...                        | 259.756             | 39.607              | 0.146                         | 4.1            | 2.17                | ...                              | ...                                          | ...                                                    | ...                      | ...                 | T                           | C                         |

Table 1—Continued

| 1FGL          | 1FGL Assoc. <sup>(a)</sup> | $l^{(a)}$<br>(deg.) | $b^{(a)}$<br>(deg.) | $\theta_{95}^{(a)}$<br>(deg.) | $\sigma^{(a)}$ | $\Gamma_{25}^{(a)}$ | $\text{Var}^{(a)}$<br>$p > 90\%$ | 2FGL <sup>(b)</sup><br>$(\Delta < d_{99.9})$ | 2FGL <sup>(c)</sup><br>$(d_{99.9} < \Delta < 1^\circ)$ | $\Delta^{(d)}$<br>(deg.) | $\Delta/d_{99.9}$ | 2FGL <sup>(e)</sup><br>Seed | Flags <sup>(f)</sup> |
|---------------|----------------------------|---------------------|---------------------|-------------------------------|----------------|---------------------|----------------------------------|----------------------------------------------|--------------------------------------------------------|--------------------------|-------------------|-----------------------------|----------------------|
| J1055.6–7611  | ...                        | 296.062             | –14.882             | 0.208                         | 5.7            | 2.77                | ...                              | J1105.4–7622                                 | J1105.4–7622                                           | 0.613                    | 1.688             | ...                         | BC                   |
| J1057.2–6026c | ...                        | 289.304             | –0.633              | 0.078                         | 11.1           | 2.25                | ...                              | J1056.2–6021                                 | ...                                                    | 0.153                    | 0.835             | T                           | C                    |
| J1101.3+1009  | ...                        | 240.848             | 59.008              | 0.067                         | 4.1            | 1.57                | ...                              | ...                                          | ...                                                    | ...                      | ...               | ...                         | NC                   |
| J1104.0–6047c | ...                        | 290.206             | –0.606              | 0.063                         | 12.4           | 2.27                | ...                              | ...                                          | J1104.7–6036                                           | 0.201                    | 1.627             | ...                         | BC                   |
| J1106.2–1752  | ...                        | 270.450             | 38.269              | 0.157                         | 4.1            | 1.84                | ...                              | ...                                          | ...                                                    | ...                      | ...               | T                           | C                    |
| J1106.7–6150c | ...                        | 290.913             | –1.441              | 0.065                         | 6.9            | 2.29                | ...                              | ...                                          | ...                                                    | ...                      | ...               | ...                         | BC, Car              |
| J1108.3+0210  | PKS 1106+023               | 253.856             | 54.902              | 0.273                         | 4.5            | 2.22                | ...                              | J1107.5+0223                                 | ...                                                    | 0.302                    | 0.682             | T                           | C                    |
| J1110.3–1622  | ...                        | 270.573             | 40.066              | 0.138                         | 5.6            | 1.98                | ...                              | ...                                          | ...                                                    | ...                      | ...               | T                           | C                    |
| J1110.4–4518  | ...                        | 284.927             | 13.997              | 0.207                         | 4.2            | 2.51                | ...                              | ...                                          | J1107.2–4448                                           | 0.757                    | 1.971             | ...                         | NC <sup>†</sup><br>C |
| J1112.3+0458  | ...                        | 251.723             | 57.628              | 0.135                         | 4.3            | 2.30                | T                                | ...                                          | ...                                                    | ...                      | ...               | T                           | C, Sun               |
| J1115.2–6124c | ...                        | 291.680             | –0.651              | 0.104                         | 7.7            | 2.25                | ...                              | ...                                          | ...                                                    | ...                      | ...               | ...                         | BC, Car              |
| J1119.5–3044  | BZB J1119–3047             | 280.587             | 28.105              | 0.118                         | 4.8            | 1.53                | ...                              | ...                                          | ...                                                    | ...                      | ...               | T                           | C                    |
| J1122.9–6415  | PMN J1123–6417             | 293.501             | –3.017              | 0.096                         | 4.7            | 2.48                | T                                | ...                                          | ...                                                    | ...                      | ...               | ...                         | NC, V                |
| J1123.6–4555  | ...                        | 287.373             | 14.282              | 0.128                         | 6.5            | 2.36                | ...                              | ...                                          | ...                                                    | ...                      | ...               | T                           | C                    |
| J1124.6–5916  | PSR J1124–5916             | 292.038             | 1.752               | 0.000                         | 14.5           | 2.36                | ...                              | J1124.6–5913                                 | ...                                                    | 0.050                    | 0.682             | T                           | C                    |
| J1127.7–6244c | ...                        | 293.515             | –1.410              | 0.124                         | 6.4            | 2.17                | ...                              | ...                                          | ...                                                    | ...                      | ...               | ...                         | BC, Car              |
| J1136.0–6226c | ...                        | 294.337             | –0.827              | 0.107                         | 6.4            | 2.18                | ...                              | ...                                          | J1138.8–6233c                                          | 0.339                    | 1.075             | ...                         | O, Car               |
| J1136.5–7004  | ...                        | 296.592             | –8.130              | 0.203                         | 5.3            | 2.93                | ...                              | ...                                          | ...                                                    | ...                      | ...               | ...                         | BC                   |
| J1138.0+4109  | ...                        | 165.286             | 69.407              | 0.140                         | 4.5            | 1.83                | ...                              | ...                                          | ...                                                    | ...                      | ...               | ...                         | NC                   |
| J1153.4–8108  | ...                        | 300.605             | –18.538             | 0.355                         | 6.3            | 2.44                | T                                | ...                                          | ...                                                    | ...                      | ...               | ...                         | NC                   |
| J1207.4–6239  | ...                        | 297.911             | –0.212              | 0.072                         | 11.8           | 2.35                | ...                              | J1208.5–6240                                 | ...                                                    | 0.123                    | 0.853             | T                           | C                    |
| J1214.4–2305  | ...                        | 291.959             | 38.985              | 0.225                         | 5.3            | 2.50                | ...                              | ...                                          | ...                                                    | ...                      | ...               | T                           | C                    |
| J1220.2+3432  | CGRaBS J1220+3431          | 163.118             | 80.023              | 0.139                         | 4.7            | 1.97                | ...                              | ...                                          | ...                                                    | ...                      | ...               | T                           | C                    |

Table 1—Continued

| 1FGL          | 1FGL Assoc. <sup>(a)</sup> | $l^{(a)}$<br>(deg.) | $b^{(a)}$<br>(deg.) | $\theta_{95}^{(a)}$<br>(deg.) | $\sigma^{(a)}$ | $\Gamma_{25}^{(a)}$ | $p > 90\%$ | $2\text{FGL}^{(b)}$<br>$(\Delta < d_{99.9})$ | $2\text{FGL}^{(c)}$<br>$(d_{99.9} < \Delta < 1^\circ)$ | $\Delta^{(d)}$<br>$\Delta$ (deg.) | $\Delta/d_{99.9}$ | $2\text{FGL}^{(e)}$ Flags | Seed |
|---------------|----------------------------|---------------------|---------------------|-------------------------------|----------------|---------------------|------------|----------------------------------------------|--------------------------------------------------------|-----------------------------------|-------------------|---------------------------|------|
| J1223.4–3034  | ...                        | 295.842             | 31.914              | 0.078                         | 5.9            | 2.22                | ...        | ...                                          | ...                                                    | ...                               | ...               | T                         | C    |
| J1224.2+5012  | ...                        | 133.804             | 66.347              | 0.166                         | 5.7            | 2.72                | ...        | ...                                          | ...                                                    | ...                               | ...               | T                         | C    |
| J1226.8+0638  | BZB J1226+0638             | 285.896             | 68.700              | 0.165                         | 4.5            | 2.26                | ...        | ...                                          | ...                                                    | ...                               | ...               | T                         | C    |
| J1241.6–6240c | ...                        | 301.811             | 0.171               | 0.189                         | 8.4            | 2.51                | ...        | J1243.9–6232                                 | ...                                                    | 0.295                             | 0.928             | T                         | C    |
| J1245.8–0632  | ...                        | 300.418             | 56.310              | 0.335                         | 5.4            | 2.76                | ...        | ...                                          | ...                                                    | ...                               | ...               | ...                       | BC   |
| J1250.9–4940  | ...                        | 302.860             | 13.198              | 0.134                         | 4.7            | 2.25                | ...        | ...                                          | ...                                                    | ...                               | ...               | T                         | C    |
| J1253.7+0326  | CRATES J1253+0326          | 304.354             | 66.301              | 0.124                         | 4.8            | 1.48                | ...        | ...                                          | ...                                                    | ...                               | ...               | T                         | C    |
| J1256.1–5922  | ...                        | 303.539             | 3.488               | 0.136                         | 4.2            | 2.22                | ...        | ...                                          | ...                                                    | ...                               | ...               | T                         | C    |
| J1256.9–6337c | ...                        | 303.549             | –0.756              | 0.195                         | 5.0            | 2.26                | ...        | ...                                          | ...                                                    | ...                               | ...               | T                         | C    |
| J1258.3+2125  | ...                        | 318.729             | 84.079              | 0.096                         | 4.4            | 1.30                | ...        | ...                                          | ...                                                    | ...                               | ...               | ...                       | NC   |
| J1300.7–5547  | ...                        | 304.253             | 7.049               | 0.296                         | 7.2            | 2.80                | ...        | J1303.8–5537                                 | ...                                                    | 0.469                             | 0.916             | T                         | C    |
| J1301.4–6245c | ...                        | 304.076             | 0.089               | 0.127                         | 8.2            | 2.29                | ...        | ...                                          | ...                                                    | ...                               | ...               | T                         | C    |
| J1301.5–2046  | ...                        | 306.103             | 42.030              | 0.071                         | 4.7            | 2.08                | ...        | ...                                          | ...                                                    | ...                               | ...               | T                         | C    |
| J1315.0–6235c | ...                        | 305.646             | 0.150               | 0.186                         | 5.1            | 2.31                | ...        | ...                                          | ...                                                    | ...                               | ...               | ...                       | BC   |
| J1317.5–6318c | ...                        | 305.856             | –0.580              | 0.069                         | 6.5            | 2.06                | ...        | ...                                          | J1317.2–6304                                           | 0.228                             | 1.052             | ...                       | O    |
| J1320.1–4007  | ...                        | 308.869             | 22.413              | 0.176                         | 6.1            | 2.58                | ...        | ...                                          | ...                                                    | ...                               | ...               | ...                       | BC   |
| J1320.6–6258c | ...                        | 306.244             | –0.286              | 0.198                         | 4.8            | 2.26                | ...        | ...                                          | ...                                                    | ...                               | ...               | ...                       | NC   |
| J1322.0–4515  | ...                        | 308.567             | 17.271              | 0.221                         | 10.6           | 2.78                | ...        | ...                                          | ...                                                    | ...                               | ...               | ...                       | BC   |
| J1322.1+0838  | ...                        | 325.835             | 70.140              | 0.136                         | 5.5            | 2.09                | ...        | ...                                          | ...                                                    | ...                               | ...               | T                         | C    |
| J1331.0+5202  | CGRaBS J1330+5202          | 108.968             | 63.991              | 0.130                         | 4.2            | 2.59                | ...        | ...                                          | ...                                                    | ...                               | ...               | T                         | C    |
| J1333.4–4036  | ...                        | 311.486             | 21.569              | 0.422                         | 7.1            | 2.75                | ...        | J1335.3–4058                                 | ...                                                    | 0.526                             | 0.789             | T                         | C    |
| J1334.2–4448  | ...                        | 310.869             | 17.397              | 0.187                         | 6.6            | 2.39                | ...        | ...                                          | ...                                                    | ...                               | ...               | T                         | C    |
| J1341.3+3951  | BZB J1341+3959             | 86.972              | 73.599              | 0.176                         | 4.5            | 2.45                | ...        | ...                                          | ...                                                    | ...                               | ...               | T                         | C    |

Table 1—Continued

| 1FGL          | 1FGL Assoc. <sup>(a)</sup> | $l^{(a)}$<br>(deg.) | $b^{(a)}$<br>(deg.) | $\theta_{95}^{(a)}$<br>(deg.) | $\sigma^{(a)}$ | $\Gamma_{25}^{(a)}$ | $\text{Var}^{(a)}$<br>$p > 90\%$ | 2FGL <sup>(b)</sup><br>$(\Delta < d_{99.9})$ | 2FGL <sup>(c)</sup><br>$(d_{99.9} < \Delta < 1^\circ)$ | $\Delta^{(d)}$<br>(deg.) | $\Delta / d_{99.9}$ | 2FGL <sup>(e)</sup><br>Seed | Flags <sup>(f)</sup> |
|---------------|----------------------------|---------------------|---------------------|-------------------------------|----------------|---------------------|----------------------------------|----------------------------------------------|--------------------------------------------------------|--------------------------|---------------------|-----------------------------|----------------------|
| J1342.7+5753  | ...                        | 110.086             | 57.943              | 0.151                         | 4.2            | 2.09                | ...                              | ...                                          | ...                                                    | ...                      | ...                 | ...                         | NC                   |
| J1343.7–6239c | ...                        | 308.894             | –0.390              | 0.119                         | 9.2            | 2.29                | ...                              | ...                                          | ...                                                    | ...                      | ...                 | T                           | C                    |
| J1350.8–6212c | ...                        | 309.795             | –0.125              | 0.078                         | 13.0           | 2.39                | ...                              | J1349.9–6222                                 | ...                                                    | 0.207                    | 1.301               | ...                         | O                    |
| J1351.8–1523  | ...                        | 323.739             | 45.025              | 0.095                         | 5.1            | 1.47                | ...                              | ...                                          | ...                                                    | ...                      | ...                 | T                           | C                    |
| J1405.5–5846  | ...                        | 312.428             | 2.717               | 0.104                         | 5.4            | 2.10                | ...                              | ...                                          | ...                                                    | ...                      | ...                 | T                           | C                    |
| J1407.5–0944  | ...                        | 332.114             | 48.769              | 0.140                         | 4.4            | 2.22                | ...                              | ...                                          | ...                                                    | ...                      | ...                 | ...                         | NC                   |
| J1412.6+7406  | ...                        | 115.610             | 41.842              | 0.106                         | 4.7            | 2.71                | ...                              | J1410.4+7411                                 | ...                                                    | 0.172                    | 0.871               | T                           | C                    |
| J1416.2–1001  | ...                        | 334.780             | 47.525              | 0.234                         | 5.4            | 2.59                | ...                              | ...                                          | ...                                                    | ...                      | ...                 | T                           | C                    |
| J1422.2+5757  | 1ES 1421+582               | 101.859             | 55.293              | 0.097                         | 4.6            | 1.42                | ...                              | ...                                          | ...                                                    | ...                      | ...                 | T                           | C                    |
| J1422.7+3743  | CLASS J1423+3737           | 67.590              | 68.094              | 0.199                         | 5.6            | 2.63                | ...                              | ...                                          | J1419.4+3820                                           | 0.901                    | 2.204               | T                           | S                    |
| J1441.8–6404  | ...                        | 314.640             | –3.743              | 0.125                         | 4.1            | 2.18                | ...                              | ...                                          | ...                                                    | ...                      | ...                 | ...                         | NC                   |
| J1501.6–4204  | ...                        | 327.297             | 14.548              | 0.482                         | 6.0            | 2.87                | ...                              | ...                                          | ...                                                    | ...                      | ...                 | ...                         | NC                   |
| J1508.2–1306  | ...                        | 346.814             | 37.838              | 0.261                         | 4.7            | 1.86                | ...                              | ...                                          | ...                                                    | ...                      | ...                 | T                           | C                    |
| J1509.7–0843  | ...                        | 350.874             | 40.923              | 0.101                         | 4.1            | 1.73                | ...                              | ...                                          | ...                                                    | ...                      | ...                 | ...                         | NC                   |
| J1511.9–0211  | ...                        | 357.647             | 45.230              | 0.353                         | 5.5            | 2.58                | ...                              | ...                                          | ...                                                    | ...                      | ...                 | ...                         | BC                   |
| J1511.9–2253  | ...                        | 340.477             | 29.553              | 0.120                         | 5.8            | 2.17                | ...                              | ...                                          | ...                                                    | ...                      | ...                 | T                           | C                    |
| J1513.2–5904  | PSR B1509–58               | 320.278             | –1.073              | 0.072                         | 5.8            | 1.60                | ...                              | ...                                          | ...                                                    | ...                      | ...                 | ...                         | BC, MSH15–52         |
| J1515.5+5448  | ...                        | 89.560              | 51.948              | 0.147                         | 4.2            | 1.37                | ...                              | ...                                          | ...                                                    | ...                      | ...                 | ...                         | NC                   |
| J1527.6+4152  | ...                        | 68.075              | 54.983              | 0.101                         | 4.7            | 1.74                | ...                              | ...                                          | ...                                                    | ...                      | ...                 | ...                         | NC                   |
| J1531.8+3018  | BZU J1532+3016             | 47.842              | 54.872              | 0.131                         | 4.3            | 1.78                | ...                              | ...                                          | ...                                                    | ...                      | ...                 | T                           | C                    |
| J1542.6–5407c | ...                        | 326.398             | 0.749               | 0.093                         | 7.7            | 2.35                | ...                              | ...                                          | ...                                                    | ...                      | ...                 | ...                         | NC                   |
| J1542.9–2559  | ...                        | 344.483             | 22.729              | 0.177                         | 5.1            | 2.45                | ...                              | J1544.1–2554                                 | ...                                                    | 0.275                    | 0.728               | T                           | C                    |
| J1548.7+6311  | ...                        | 96.962              | 43.953              | 0.114                         | 4.1            | 2.00                | ...                              | ...                                          | ...                                                    | ...                      | ...                 | T                           | C                    |

Table 1—Continued

| 1FGL          | 1FGL Assoc. $(a)$ | $l^{(a)}$<br>(deg.) | $b^{(a)}$<br>(deg.) | $\theta_{95}^{(a)}$<br>(deg.) | $\sigma^{(a)}$ | $\Gamma_{25}^{(a)}$ | $p > 90\%$ | 2FGL $(b)$<br>$(\Delta < d_{99.9})$ | 2FGL $(c)$<br>$(d_{99.9} < \Delta < 1^\circ)$ | $\Delta^{(d)}$<br>(deg.) | $\Delta / d_{99.9}$ | 2FGL $(e)$<br>Seed | Flags $(f)$        |
|---------------|-------------------|---------------------|---------------------|-------------------------------|----------------|---------------------|------------|-------------------------------------|-----------------------------------------------|--------------------------|---------------------|--------------------|--------------------|
| J1548.9–5509c | ...               | 326.481             | –0.625              | 0.094                         | 6.5            | 2.36                | ...        | ...                                 | ...                                           | ...                      | ...                 | ...                | NC                 |
| J1553.6–0300c | ...               | 5.786               | 36.745              | 0.193                         | 5.4            | 2.12                | ...        | J1553.5–0324                        | 0.387                                         | 1.002                    | ...                 | ...                | O                  |
| J1553.9+4952  | ...               | 78.807              | 48.570              | 0.195                         | 5.3            | 1.84                | ...        | ...                                 | ...                                           | ...                      | ...                 | ...                | NC                 |
| J1554.0–5345c | ...               | 327.939             | –0.007              | 0.107                         | 10.2           | 2.24                | ...        | ...                                 | J1551.3–5333                                  | 0.452                    | 1.878               | ...                | BC                 |
| J1555.9–5226c | ...               | 329.006             | 0.829               | 0.101                         | 5.0            | 2.33                | ...        | ...                                 | ...                                           | ...                      | ...                 | ...                | NC                 |
| J1607.5–2030  | ...               | 353.012             | 22.746              | 0.068                         | 5.7            | 2.30                | ...        | ...                                 | ...                                           | ...                      | ...                 | ...                | BC                 |
| J1613.6–5100c | ...               | 332.011             | 0.081               | 0.066                         | 10.8           | 2.20                | ...        | ...                                 | J1615.0–5051                                  | 0.260                    | 1.574               | ...                | BC, HESS J1616–508 |
| J1614.0–2230  | PSR J1614–2230    | 352.541             | 20.301              | 0.000                         | 15.6           | 2.14                | ...        | ...                                 | J1614.5–2230                                  | 0.135                    | 1.670               | ...                | BC                 |
| J1616.1+4637  | CRATES J1616+4632 | 73.037              | 45.617              | 0.310                         | 7.6            | 2.68                | ...        | J1614.8+4703                        | ...                                           | 0.480                    | 0.832               | T                  | C                  |
| J1616.6–5035c | ...               | 332.634             | 0.060               | 0.063                         | 8.2            | 2.07                | ...        | ...                                 | ...                                           | ...                      | ...                 | ...                | BC                 |
| J1617.5–5105c | ...               | 332.393             | –0.402              | 0.067                         | 10.6           | 1.93                | ...        | ...                                 | ...                                           | ...                      | ...                 | ...                | BC                 |
| J1617.7–5843  | PMN J1617–5848    | 327.063             | –5.896              | 0.159                         | 10.2           | 2.72                | ...        | ...                                 | J1618.0–5825                                  | 0.304                    | 1.015               | ...                | O                  |
| J1619.3–5222  | ...               | 331.689             | –1.523              | 0.201                         | 5.1            | 2.16                | ...        | ...                                 | ...                                           | ...                      | ...                 | ...                | NC                 |
| J1620.9–2731  | ...               | 349.789             | 15.731              | 0.190                         | 5.6            | 2.37                | ...        | ...                                 | J1617.5–2657                                  | 0.937                    | 2.607               | ...                | NC                 |
| J1623.5–2345c | ...               | 353.124             | 17.830              | 0.357                         | 4.9            | 2.30                | ...        | ...                                 | J1620.5–2320                                  | 0.811                    | 1.375               | ...                | NC, Oph            |
| J1624.7–0642  | 4C –06.46         | 7.756               | 28.330              | 0.116                         | 4.4            | 2.05                | ...        | ...                                 | ...                                           | ...                      | ...                 | ...                | NC                 |
| J1625.8–2429c | 0FGL J1625.9–2423 | 352.911             | 16.938              | 0.089                         | 10.2           | 2.25                | ...        | ...                                 | J1627.0–2425                                  | 0.269                    | 1.212               | ...                | O, Oph             |
| J1626.0–4917c | ...               | 334.621             | –0.088              | 0.086                         | 8.8            | 2.16                | ...        | ...                                 | J1628.1–4857c                                 | 0.482                    | 1.537               | ...                | BC, G335.2+00.1    |
| J1626.2–2038  | ...               | 356.029             | 19.397              | 0.454                         | 5.7            | 2.51                | ...        | J1624.2–2124                        | ...                                           | 0.893                    | 0.928               | T                  | C                  |
| J1627.8–1711c | ...               | 359.119             | 21.325              | 0.148                         | 4.2            | 2.19                | ...        | ...                                 | ...                                           | ...                      | ...                 | ...                | NC                 |
| J1627.9+0254  | ...               | 17.616              | 32.963              | 0.168                         | 5.7            | 2.04                | ...        | ...                                 | ...                                           | ...                      | ...                 | T                  | C                  |
| J1628.6–2419c | ...               | 353.475             | 16.577              | 0.182                         | 5.2            | 2.14                | ...        | ...                                 | ...                                           | ...                      | ...                 | ...                | NC, Oph            |
| J1632.7–2431c | ...               | 353.961             | 15.743              | 0.171                         | 7.0            | 2.27                | ...        | ...                                 | ...                                           | ...                      | ...                 | ...                | O                  |

Table 1—Continued

| 1FGL          | 1FGL Assoc. <sup>(a)</sup> | $l^{(a)}$<br>(deg.) | $b^{(a)}$<br>(deg.) | $\theta_{95}^{(a)}$<br>(deg.) | $\sigma^{(a)}$ | $\Gamma_{25}^{(a)}$ | $V_{\text{ar}}^{(a)}$<br>$p > 90\%$ | 2FGL <sup>(b)</sup><br>$(\Delta < d_{99.9})$ | 2FGL <sup>(c)</sup><br>$(d_{99.9} < \Delta < 1^\circ)$ | $\Delta^{(d)}$<br>(deg.) | $\Delta / d_{99.9}$ | 2FGL <sup>(e)</sup><br>Seed | Flags <sup>(f)</sup> |
|---------------|----------------------------|---------------------|---------------------|-------------------------------|----------------|---------------------|-------------------------------------|----------------------------------------------|--------------------------------------------------------|--------------------------|---------------------|-----------------------------|----------------------|
| J1632.7–4733c | ...                        | 336.636             | 0.295               | 0.124                         | 9.2            | 2.14                | ...                                 | ...                                          | J1631.7–4720c                                          | 0.279                    | 1.168               | ...                         | O, G336.7+00.5       |
| J1632.9–4802c | ...                        | 336.308             | –0.051              | 0.053                         | 15.6           | 2.17                | ...                                 | ...                                          | J1632.4–4753c                                          | 0.167                    | 1.335               | ...                         | O                    |
| J1635.4+8228  | NGC 6251                   | 115.640             | 31.150              | 0.091                         | 10.0           | 2.50                | ...                                 | ...                                          | J1629.4+8236                                           | 0.242                    | 1.038               | ...                         | O                    |
| J1639.5–5152  | ...                        | 334.190             | –3.427              | 0.073                         | 12.7           | 2.54                | ...                                 | J1639.8–5145                                 | ...                                                    | 0.117                    | 0.698               | T                           | C                    |
| J1642.5+3947  | ...                        | 63.427              | 41.028              | 0.056                         | 34.8           | 2.49                | T                                   | J1642.9+3949                                 | ...                                                    | 0.090                    | 0.772               | T                           | S                    |
| J1647.9–1119  | ...                        | 7.274               | 20.993              | 0.173                         | 4.5            | 2.21                | ...                                 | ...                                          | ...                                                    | ...                      | ...                 | ...                         | NC                   |
| J1649.3–4501c | ...                        | 340.437             | –0.183              | 0.153                         | 10.4           | 2.32                | ...                                 | ...                                          | J1651.8–4439c                                          | 0.575                    | 1.362               | ...                         | O                    |
| J1650.3–5410  | ...                        | 333.493             | –6.157              | 0.145                         | 4.5            | 2.24                | ...                                 | ...                                          | ...                                                    | ...                      | ...                 | ...                         | NC                   |
| J1702.4–4147c | ...                        | 344.450             | 0.003               | 0.080                         | 9.8            | 2.39                | ...                                 | ...                                          | ...                                                    | ...                      | ...                 | ...                         | BC                   |
| J1705.5–4034c | ...                        | 345.764             | 0.275               | 0.115                         | 5.7            | 2.24                | ...                                 | ...                                          | ...                                                    | ...                      | ...                 | ...                         | NC                   |
| J1707.1–4158c | ...                        | 344.842             | –0.810              | 0.081                         | 5.7            | 2.14                | ...                                 | ...                                          | ...                                                    | ...                      | ...                 | T                           | C                    |
| J1707.9–4110c | ...                        | 345.563             | –0.442              | 0.139                         | 6.4            | 2.12                | ...                                 | ...                                          | ...                                                    | ...                      | ...                 | T                           | C                    |
| J1708.4–0755  | ...                        | 13.265              | 18.674              | 0.173                         | 6.8            | 2.55                | ...                                 | ...                                          | J1709.0–0821                                           | 0.462                    | 1.071               | ...                         | O                    |
| J1709.1–0343  | ...                        | 17.160              | 20.709              | 0.161                         | 6.2            | 2.50                | ...                                 | J1710.0–0323                                 | ...                                                    | 0.408                    | 0.898               | T                           | C                    |
| J1709.8–2026  | ...                        | 2.668               | 11.445              | 0.138                         | 4.8            | 2.13                | ...                                 | ...                                          | ...                                                    | ...                      | ...                 | ...                         | NC                   |
| J1715.2–3319  | ...                        | 352.757             | 3.000               | 0.140                         | 4.9            | 2.30                | ...                                 | ...                                          | ...                                                    | ...                      | ...                 | T                           | C                    |
| J1716.9–3830c | ...                        | 348.728             | –0.274              | 0.086                         | 5.6            | 2.26                | ...                                 | ...                                          | ...                                                    | ...                      | ...                 | ...                         | NC                   |
| J1720.7–3707c | ...                        | 350.299             | –0.101              | 0.091                         | 7.9            | 2.31                | ...                                 | ...                                          | ...                                                    | ...                      | ...                 | ...                         | BC                   |
| J1724.0–3448c | ...                        | 352.589             | 0.674               | 0.087                         | 5.0            | 2.27                | ...                                 | ...                                          | ...                                                    | ...                      | ...                 | ...                         | NC                   |
| J1724.0–3611c | ...                        | 351.443             | –0.106              | 0.569                         | 6.2            | 2.38                | ...                                 | ...                                          | ...                                                    | ...                      | ...                 | ...                         | NC                   |
| J1725.5–2832  | ...                        | 357.962             | 3.909               | 0.255                         | 5.8            | 2.39                | ...                                 | ...                                          | ...                                                    | ...                      | ...                 | ...                         | NC                   |
| J1726.2–0724  | ...                        | 16.132              | 15.177              | 0.255                         | 8.4            | 2.37                | ...                                 | J1727.1–0704                                 | ...                                                    | 0.401                    | 0.838               | T                           | C                    |
| J1726.2–3521c | ...                        | 352.381             | –0.014              | 0.100                         | 8.7            | 2.36                | ...                                 | ...                                          | J1726.6–3545                                           | 0.413                    | 1.474               | ...                         | BC                   |

Table 1—Continued

| 1FGL          | 1FGL Assoc. <sup>(a)</sup> | $l^{(a)}$<br>(deg.) | $b^{(a)}$<br>(deg.) | $\theta_{95}^{(a)}$<br>(deg.) | $\sigma^{(a)}$ | $\Gamma_{25}^{(a)}$ | $\text{Var}^{(a)}$<br>$p > 90\%$ | 2FGL <sup>(b)</sup><br>$(\Delta < d_{99.9})$ | 2FGL <sup>(c)</sup><br>$(d_{99.9} < \Delta < 1^\circ)$ | $\Delta^{(d)}$<br>(deg.) | $\Delta / d_{99.9}$ | 2FGL <sup>(e)</sup><br>Seed | Flags <sup>(f)</sup> |
|---------------|----------------------------|---------------------|---------------------|-------------------------------|----------------|---------------------|----------------------------------|----------------------------------------------|--------------------------------------------------------|--------------------------|---------------------|-----------------------------|----------------------|
| J1729.1–3452c | ...                        | 353.115             | −0.244              | 0.123                         | 7.2            | 2.27                | ...                              | ...                                          | ...                                                    | ...                      | ...                 | ...                         | NC                   |
| J1729.1–3641c | ...                        | 351.610             | −1.248              | 0.073                         | 7.0            | 2.28                | ...                              | ...                                          | ...                                                    | ...                      | ...                 | ...                         | NC                   |
| J1729.8–4148  | ...                        | 347.398             | −4.164              | 0.125                         | 4.3            | 1.50                | ...                              | ...                                          | ...                                                    | ...                      | ...                 | ...                         | NC                   |
| J1730.0–3408c | ...                        | 353.826             | 0.015               | 0.105                         | 10.8           | 2.44                | ...                              | ...                                          | J1730.5–3350                                           | 0.317                    | 2.007               | ...                         | BC                   |
| J1730.4+0008  | PKS 1728+004               | 23.518              | 18.000              | 0.253                         | 5.3            | 2.22                | T                                | J1730.7+0023                                 | ...                                                    | 0.263                    | 0.676               | T                           | C                    |
| J1732.3–3243c | ...                        | 355.273             | 0.386               | 0.124                         | 12.0           | 2.33                | ...                              | J1731.6–3234c                                | ...                                                    | 0.214                    | 0.917               | T                           | C                    |
| J1733.2–2628  | ...                        | 0.626               | 3.626               | 0.268                         | 14.4           | 2.46                | ...                              | ...                                          | J1731.9–2703c                                          | 0.654                    | 1.447               | ...                         | BC                   |
| J1735.1–0729  | ...                        | 17.203              | 13.233              | 0.147                         | 6.2            | 2.38                | ...                              | ...                                          | ...                                                    | ...                      | ...                 | T                           | C                    |
| J1735.4–1118  | CRATES J1735–1117          | 13.886              | 11.216              | 0.065                         | 5.8            | 2.00                | ...                              | ...                                          | ...                                                    | ...                      | ...                 | T                           | C <sub>1</sub>       |
| J1738.5–2656  | ...                        | 0.882               | 2.372               | 0.152                         | 15.4           | 2.42                | ...                              | ...                                          | J1739.6–2726                                           | 0.551                    | 1.468               | ...                         | BC                   |
| J1741.8–2101  | LAT PSR J1741–2054         | 6.311               | 4.865               | 0.000                         | 32.5           | 2.32                | ...                              | ...                                          | J1741.9–2054                                           | 0.112                    | 2.194               | ...                         | BC                   |
| J1743.5–3314  | ...                        | 356.100             | −1.863              | 0.090                         | 11.8           | 2.31                | ...                              | ...                                          | J1742.5–3323                                           | 0.256                    | 1.002               | ...                         | O                    |
| J1744.0–2931c | ...                        | 359.309             | −0.014              | 0.104                         | 10.4           | 2.28                | ...                              | ...                                          | ...                                                    | ...                      | ...                 | ...                         | BC                   |
| J1744.6–0354  | ...                        | 21.598              | 12.952              | 0.106                         | 4.6            | 2.05                | ...                              | ...                                          | ...                                                    | ...                      | ...                 | T                           | C                    |
| J1745.6–2900c | ...                        | 359.941             | −0.051              | 0.019                         | 24.5           | 2.26                | ...                              | J1745.6–2858                                 | ...                                                    | 0.036                    | 0.947               | T                           | C, Sgr A East        |
| J1747.0+0221c | ...                        | 27.593              | 15.385              | 0.261                         | 6.7            | 2.53                | ...                              | J1745.6+0203                                 | ...                                                    | 0.454                    | 0.914               | T                           | C                    |
| J1747.2–2958  | PSR J1747–2958             | 359.306             | −0.842              | 0.000                         | 23.0           | 2.32                | ...                              | ...                                          | J1747.1–3000                                           | 0.053                    | 1.045               | ...                         | BC                   |
| J1747.6–2820c | ...                        | 0.748               | −0.073              | 0.061                         | 11.7           | 2.23                | ...                              | J1747.3–2825c                                | ...                                                    | 0.113                    | 0.893               | T                           | C                    |
| J1749.5–0301  | ...                        | 23.011              | 12.298              | 0.180                         | 4.7            | 2.42                | ...                              | ...                                          | ...                                                    | ...                      | ...                 | T                           | C                    |
| J1804.1+0336  | CRATES J1803+0341          | 30.760              | 12.153              | 0.173                         | 6.0            | 2.43                | T                                | ...                                          | ...                                                    | ...                      | ...                 | ...                         | BC                   |
| J1806.8–2109c | ...                        | 9.134               | −0.241              | 0.127                         | 8.5            | 2.27                | ...                              | ...                                          | J1808.5–2037c                                          | 0.674                    | 2.606               | ...                         | NC, W30              |
| J1807.6–4341  | NGC 6541                   | 349.267             | −11.117             | 0.200                         | 4.1            | 1.99                | ...                              | ...                                          | ...                                                    | ...                      | ...                 | T                           | C                    |
| J1811.3–1959c | PSR J1810–2005             | 10.665              | −0.586              | 0.099                         | 4.2            | 2.07                | ...                              | ...                                          | ...                                                    | ...                      | ...                 | ...                         | NC                   |

Table 1—Continued

| 1FGL          | 1FGL Assoc. <sup>(a)</sup> | $l^{(a)}$<br>(deg.) | $b^{(a)}$<br>(deg.) | $\theta_{95}^{(a)}$<br>(deg.) | $\sigma^{(a)}$ | $\Gamma_{25}^{(a)}$ | $\text{Var}^{(a)}$<br>$p > 90\%$ | 2FGL <sup>(b)</sup><br>$(\Delta < d_{9.9})$ | 2FGL <sup>(c)</sup><br>$(d_{9.9} < \Delta < 1^\circ)$ | $\Delta^{(d)}$<br>(deg.) | $\Delta / d_{9.9}$ | 2FGL <sup>(e)</sup><br>Seed | Flags <sup>(f)</sup> |
|---------------|----------------------------|---------------------|---------------------|-------------------------------|----------------|---------------------|----------------------------------|---------------------------------------------|-------------------------------------------------------|--------------------------|--------------------|-----------------------------|----------------------|
| J1816.2–0942  | ...                        | 20.273              | 3.270               | 0.313                         | 10.3           | 2.76                | ...                              | ...                                         | ...                                                   | ...                      | ...                | ...                         | BC                   |
| J1817.0+2519  | ...                        | 52.584              | 18.376              | 0.341                         | 4.3            | 2.58                | ...                              | ...                                         | ...                                                   | ...                      | ...                | ...                         | NC                   |
| J1818.7–1557c | ...                        | 15.048              | −0.206              | 0.111                         | 7.7            | 2.34                | ...                              | ...                                         | ...                                                   | ...                      | ...                | ...                         | NC                   |
| J1821.1–1425c | ...                        | 16.684              | −0.001              | 0.084                         | 10.7           | 2.26                | ...                              | ...                                         | ...                                                   | ...                      | ...                | ...                         | BC, HESSJ1825–137    |
| J1822.6–0340  | ...                        | 26.365              | 4.698               | 0.271                         | 7.3            | 2.69                | T                                | ...                                         | ...                                                   | ...                      | ...                | ...                         | NC                   |
| J1823.0+0828  | ...                        | 37.333              | 10.126              | 0.204                         | 4.3            | 2.03                | ...                              | J1821.8+0830                                | ...                                                   | 0.311                    | 0.817              | T                           | C                    |
| J1825.7–1410c | ...                        | 17.416              | −0.873              | 0.055                         | 7.9            | 1.12                | ...                              | ...                                         | ...                                                   | ...                      | ...                | ...                         | BC, HESSJ1825–137    |
| J1829.6–1006c | ...                        | 21.458              | 0.181               | 0.134                         | 8.4            | 2.34                | ...                              | ...                                         | ...                                                   | ...                      | ...                | ...                         | NC                   |
| J1830.0+0043  | ...                        | 31.134              | 5.095               | 0.196                         | 7.2            | 2.61                | ...                              | ...                                         | ...                                                   | ...                      | ...                | ...                         | NC                   |
| J1830.1–0425  | ...                        | 26.569              | 2.694               | 0.141                         | 9.0            | 2.41                | ...                              | ...                                         | J1833.1–0437c                                         | 0.777                    | 2.247              | ...                         | NC                   |
| J1834.3–0842c | 0FGL J1834.4–0841          | 23.237              | −0.195              | 0.061                         | 16.9           | 2.24                | ...                              | J1834.3–0848                                | ...                                                   | 0.105                    | 0.731              | T                           | C, W41               |
| J1836.2+5925  | LAT PSR J1836+5925         | 88.876              | 24.999              | 0.000                         | 191.2          | 1.99                | ...                              | J1836.2+5926                                | ...                                                   | 0.010                    | 0.692              | T                           | C                    |
| J1839.1–0543c | 0FGL J1839.0–0549          | 26.431              | 0.118               | 0.033                         | 45.3           | 2.28                | ...                              | ...                                         | J1839.0–0539                                          | 0.075                    | 1.164              | ...                         | BC                   |
| J1842.0–1409  | ...                        | 19.248              | −4.366              | 0.078                         | 5.4            | 2.42                | ...                              | ...                                         | ...                                                   | ...                      | ...                | T                           | C                    |
| J1844.3–0309c | ...                        | 29.316              | 0.133               | 0.065                         | 9.8            | 2.15                | ...                              | J1843.7–0312c                               | ...                                                   | 0.173                    | 0.785              | T                           | C                    |
| J1846.0–0831  | ...                        | 24.738              | −2.695              | 0.107                         | 11.3           | 2.59                | T                                | ...                                         | ...                                                   | ...                      | ...                | ...                         | BC                   |
| J1848.5+3224  | B2 1846+32A                | 62.143              | 14.701              | 0.077                         | 20.7           | 2.39                | T                                | J1848.5+3216                                | ...                                                   | 0.127                    | 0.689              | T                           | S                    |
| J1855.7–1136c | ...                        | 23.042              | −6.199              | 0.189                         | 5.2            | 2.49                | ...                              | ...                                         | ...                                                   | ...                      | ...                | ...                         | NC                   |
| J1857.1+0212c | ...                        | 35.541              | −0.257              | 0.084                         | 16.1           | 2.32                | ...                              | J1857.6+0211                                | ...                                                   | 0.141                    | 0.879              | T                           | S                    |
| J1900.3+0420c | ...                        | 37.812              | −0.012              | 0.138                         | 11.3           | 2.36                | ...                              | J1901.1+0427                                | ...                                                   | 0.232                    | 0.861              | T                           | C                    |
| J1902.3+0503c | ...                        | 38.678              | −0.113              | 0.072                         | 11.0           | 2.35                | ...                              | ...                                         | ...                                                   | ...                      | ...                | ...                         | BC                   |
| J1904.4–2725  | ...                        | 9.339               | −14.757             | 0.189                         | 5.3            | 2.17                | ...                              | ...                                         | ...                                                   | ...                      | ...                | ...                         | NC                   |
| J1907.4–0358  | ...                        | 31.207              | −5.361              | 0.259                         | 7.7            | 2.77                | ...                              | ...                                         | ...                                                   | ...                      | ...                | T                           | C                    |

Table 1—Continued

| 1FGL          | 1FGL Assoc. <sup>(a)</sup> | $l^{(a)}$<br>(deg.) | $b^{(a)}$<br>(deg.) | $\theta_{95}^{(a)}$<br>(deg.) | $\sigma^{(a)}$ | $\Gamma_{25}^{(a)}$ | $\text{Var}^{(a)}$<br>$p > 90\%$ | 2FGL <sup>(b)</sup><br>$(\Delta < d_{99.9})$ | 2FGL <sup>(c)</sup><br>$(d_{99.9} < \Delta < 1^\circ)$ | $\Delta^{(d)}$<br>(deg.) | $\Delta/d_{99.9}$ | 2FGL <sup>(e)</sup><br>Seed | Flags <sup>(f)</sup> |
|---------------|----------------------------|---------------------|---------------------|-------------------------------|----------------|---------------------|----------------------------------|----------------------------------------------|--------------------------------------------------------|--------------------------|-------------------|-----------------------------|----------------------|
| J1908.2+0803c | ...                        | 42.006              | -0.034              | 0.153                         | 8.2            | 2.18                | ...                              | ...                                          | ...                                                    | ...                      | ...               | ...                         | BC                   |
| J1911.1-5306  | ...                        | 343.922             | -24.246             | 0.252                         | 4.3            | 2.25                | ...                              | ...                                          | ...                                                    | ...                      | ...               | T                           | C                    |
| J1911.7+0307  | ...                        | 38.041              | -3.085              | 0.125                         | 5.3            | 2.18                | ...                              | ...                                          | ...                                                    | ...                      | ...               | ...                         | NC                   |
| J1913.2-0744  | ...                        | 28.470              | -8.341              | 0.077                         | 5.7            | 2.35                | ...                              | ...                                          | ...                                                    | ...                      | ...               | ...                         | NC                   |
| J1913.7+1007c | ...                        | 44.480              | -0.281              | 0.200                         | 6.6            | 2.38                | ...                              | J1914.4+0951c                                | ...                                                    | 0.335                    | 0.940             | T                           | C                    |
| J1919.9+6633  | ...                        | 97.740              | 21.987              | 0.142                         | 4.9            | 2.31                | ...                              | ...                                          | ...                                                    | ...                      | ...               | ...                         | NC                   |
| J1925.1-1018  | CRATES J1925-1018          | 27.434              | -12.114             | 0.058                         | 7.7            | 2.22                | ...                              | ...                                          | J1924.9-1036                                           | 0.297                    | 1.499             | T                           | S                    |
| J1925.4-3811  | ...                        | 0.325               | -22.665             | 0.159                         | 5.3            | 2.15                | ...                              | ...                                          | ...                                                    | ...                      | ...               | ...                         | NC                   |
| J1926.1+1601c | ...                        | 51.104              | -0.194              | 0.139                         | 9.6            | 2.30                | ...                              | ...                                          | ...                                                    | ...                      | ...               | ...                         | BC                   |
| J1926.5+1647c | ...                        | 51.825              | 0.097               | 0.118                         | 4.9            | 2.14                | ...                              | ...                                          | ...                                                    | ...                      | ...               | ...                         | NC                   |
| J1927.3-7932c | ...                        | 314.679             | -28.271             | 0.591                         | 5.6            | 2.80                | ...                              | ...                                          | ...                                                    | ...                      | ...               | T                           | C                    |
| J1928.7-0506  | CRATES J1928-0456          | 32.602              | -10.610             | 0.271                         | 13.1           | 2.76                | ...                              | ...                                          | ...                                                    | ...                      | ...               | ...                         | NC, V                |
| J1930.8+1653c | ...                        | 52.396              | -0.761              | 0.137                         | 6.2            | 2.23                | ...                              | ...                                          | ...                                                    | ...                      | ...               | ...                         | BC                   |
| J1934.9+2031c | JVAS J1935+2031            | 56.052              | 0.144               | 0.279                         | 8.2            | 2.30                | ...                              | ...                                          | ...                                                    | ...                      | ...               | ...                         | BC                   |
| J1938.2+2125c | ...                        | 57.207              | -0.092              | 0.180                         | 5.3            | 2.25                | ...                              | ...                                          | ...                                                    | ...                      | ...               | ...                         | NC                   |
| J1940.1+2209c | ...                        | 58.070              | -0.098              | 0.146                         | 7.6            | 2.21                | ...                              | ...                                          | ...                                                    | ...                      | ...               | ...                         | BC                   |
| J1943.4+2340c | ...                        | 59.769              | -0.017              | 0.112                         | 5.7            | 2.23                | ...                              | ...                                          | ...                                                    | ...                      | ...               | T                           | C                    |
| J1945.0-0724c | ...                        | 32.344              | -15.259             | 0.093                         | 8.3            | 2.65                | ...                              | ...                                          | J1947.8-0739                                           | 0.760                    | 2.237             | ...                         | BC                   |
| J1948.6+2437  | ...                        | 61.178              | -0.557              | 0.133                         | 4.9            | 2.16                | ...                              | ...                                          | ...                                                    | ...                      | ...               | T                           | C                    |
| J1958.9+3459  | ...                        | 71.220              | 2.865               | 0.124                         | 5.2            | 2.26                | ...                              | ...                                          | ...                                                    | ...                      | ...               | T                           | C                    |
| J2007.0+0145  | ...                        | 43.415              | -15.905             | 0.224                         | 4.3            | 1.78                | ...                              | ...                                          | ...                                                    | ...                      | ...               | T                           | C                    |
| J2008.6-0419  | 3C 407                     | 37.975              | -19.130             | 0.216                         | 4.3            | 2.36                | ...                              | ...                                          | J2009.1-0339                                           | 0.682                    | 1.583             | ...                         | NC, V                |
| J2011.4-2903  | ...                        | 13.117              | -29.175             | 0.105                         | 4.1            | 1.74                | ...                              | ...                                          | ...                                                    | ...                      | ...               | ...                         | NC                   |

Table 1—Continued

| 1FGL          | 1FGL Assoc. <sup>(a)</sup> | $l^{(a)}$<br>(deg.) | $b^{(a)}$<br>(deg.) | $\theta_{95}^{(a)}$<br>(deg.) | $\sigma^{(a)}$ | $\Gamma_{25}^{(a)}$ | $\text{Var}^{(a)}$<br>$p > 90\%$ | 2FGL <sup>(b)</sup><br>$(\Delta < d_{99.9})$ | 2FGL <sup>(c)</sup><br>$(d_{99.9} < \Delta < 1^\circ)$ | $\Delta^{(d)}$<br>(deg.) | $\Delta/d_{99.9}$ | 2FGL <sup>(e)</sup><br>Seed | Flags <sup>(f)</sup> |
|---------------|----------------------------|---------------------|---------------------|-------------------------------|----------------|---------------------|----------------------------------|----------------------------------------------|--------------------------------------------------------|--------------------------|-------------------|-----------------------------|----------------------|
| J2015.8–3251  | ...                        | 9.180               | −31.106             | 0.164                         | 6.0            | 2.76                | ...                              | ...                                          | J2017.4–3215                                           | 0.671                    | 1.892             | ...                         | BC                   |
| J2020.0+4049  | ...                        | 78.373              | 2.533               | 0.101                         | 7.9            | 2.12                | ...                              | ...                                          | J2019.1+4040                                           | 0.219                    | 1.014             | ...                         | BC, Gamma Cygni      |
| J2020.4+7608  | CGRaBS J2022+7611          | 109.168             | 21.219              | 0.128                         | 6.0            | 2.52                | ...                              | J2022.5+7614                                 | ...                                                    | 0.166                    | 0.686             | T                           | C                    |
| J2025.9–2852  | CGRaBS J2025–2845          | 14.339              | −32.169             | 0.140                         | 5.6            | 2.43                | ...                              | ...                                          | ...                                                    | ...                      | ...               | T                           | C                    |
| J2027.6+3335  | ...                        | 73.327              | −2.861              | 0.056                         | 27.0           | 2.34                | T                                | ...                                          | J2028.3+3332                                           | 0.161                    | 1.558             | ...                         | BC                   |
| J2029.0–1840  | ...                        | 25.907              | −29.634             | 0.190                         | 4.2            | 2.07                | T                                | ...                                          | J2031.4–1842                                           | 0.564                    | 1.090             | ...                         | NC, Sun              |
| J2037.0–3329  | ...                        | 9.622               | −35.577             | 0.100                         | 5.1            | 2.02                | ...                              | ...                                          | ...                                                    | ...                      | ...               | T                           | C                    |
| J2037.1+5718c | ...                        | 93.543              | 9.777               | 0.158                         | 4.5            | 2.48                | ...                              | ...                                          | ...                                                    | ...                      | ...               | ...                         | NC                   |
| J2037.2+4944  | ...                        | 87.408              | 5.274               | 0.217                         | 4.4            | 2.13                | ...                              | ...                                          | ...                                                    | ...                      | ...               | ...                         | NC                   |
| J2040.0+4157c | ...                        | 81.502              | 0.157               | 0.197                         | 10.7           | 2.66                | ...                              | J2038.0+4145c                                | ...                                                    | 0.417                    | 0.934             | T                           | C                    |
| J2040.4+4652  | ...                        | 85.440              | 3.103               | 0.092                         | 6.8            | 2.44                | ...                              | ...                                          | ...                                                    | ...                      | ...               | T                           | C                    |
| J2040.9–3701  | ...                        | 5.462               | −36.970             | 0.190                         | 5.0            | 2.33                | ...                              | ...                                          | ...                                                    | ...                      | ...               | ...                         | BC                   |
| J2042.3+5041  | ...                        | 88.656              | 5.194               | 0.384                         | 4.7            | 2.52                | ...                              | J2043.3+5105                                 | ...                                                    | 0.445                    | 0.716             | T                           | S, G089.0+04.7       |
| J2046.4+3041  | ...                        | 73.395              | −7.786              | 0.177                         | 5.7            | 2.51                | ...                              | ...                                          | ...                                                    | ...                      | ...               | ...                         | NC, Cygnus Loop      |
| J2049.1+3142  | ...                        | 74.561              | −7.604              | 0.126                         | 5.2            | 2.37                | ...                              | ...                                          | ...                                                    | ...                      | ...               | T                           | NC, Cygnus Loop      |
| J2054.0–3307  | ...                        | 10.899              | −38.983             | 0.242                         | 4.2            | 2.51                | ...                              | ...                                          | ...                                                    | ...                      | ...               | T                           | C                    |
| J2055.2+3144  | ...                        | 75.397              | −8.588              | 0.234                         | 8.3            | 2.36                | ...                              | ...                                          | ...                                                    | ...                      | ...               | T                           | NC, Cygnus Loop      |
| J2057.4+3057  | ...                        | 75.108              | −9.456              | 0.232                         | 5.9            | 2.40                | ...                              | ...                                          | ...                                                    | ...                      | ...               | ...                         | NC, Cygnus Loop      |
| J2058.8–3903  | ...                        | 3.381               | −40.704             | 0.120                         | 4.9            | 1.67                | ...                              | ...                                          | ...                                                    | ...                      | ...               | ...                         | NC                   |
| J2103.0–1127  | ...                        | 37.520              | −34.350             | 0.083                         | 5.1            | 1.86                | ...                              | J2103.5–1112                                 | ...                                                    | 0.284                    | 0.920             | T                           | C                    |
| J2104.6+2119  | ...                        | 68.510              | −16.818             | 0.139                         | 4.2            | 2.20                | ...                              | ...                                          | ...                                                    | ...                      | ...               | T                           | C                    |
| J2105.9+6917  | ...                        | 105.221             | 14.615              | 0.193                         | 4.7            | 2.81                | ...                              | ...                                          | ...                                                    | ...                      | ...               | ...                         | NC                   |
| J2108.2+5246c | ...                        | 92.849              | 3.457               | 0.125                         | 4.9            | 1.84                | ...                              | ...                                          | ...                                                    | ...                      | ...               | ...                         | BC                   |

Table 1—Continued

| 1FGL         | 1FGL Assoc. <sup>(a)</sup> | $l^{(a)}$<br>(deg.) | $b^{(a)}$<br>(deg.) | $\theta_{95}^{(a)}$<br>(deg.) | $\sigma^{(a)}$ | $\Gamma_{25}^{(a)}$ | $p > 90\%$ | 2FGL <sup>(b)</sup><br>$(\Delta < d_{99.9})$ | 2FGL <sup>(c)</sup><br>$(d_{99.9} < \Delta < 1^\circ)$ | $\Delta^{(d)}$<br>(deg.) | $\Delta / d_{99.9}$ | 2FGL <sup>(e)</sup><br>Seed | Flags <sup>(f)</sup> |
|--------------|----------------------------|---------------------|---------------------|-------------------------------|----------------|---------------------|------------|----------------------------------------------|--------------------------------------------------------|--------------------------|---------------------|-----------------------------|----------------------|
| J2110.6+0403 | ...                        | 54.431              | -28.322             | 0.112                         | 5.0            | 2.01                | ...        | ...                                          | ...                                                    | ...                      | ...                 | T                           | C                    |
| J2117.8+0016 | CRATES J2118+0013          | 51.922              | -31.910             | 0.151                         | 5.0            | 1.89                | ...        | ...                                          | ...                                                    | ...                      | ...                 | T                           | C                    |
| J2118.3-3237 | ...                        | 12.586              | -43.953             | 0.111                         | 4.9            | 1.64                | ...        | ...                                          | ...                                                    | ...                      | ...                 | T                           | C                    |
| J2126.1-4603 | PKS 2123-463               | 353.652             | -45.582             | 0.291                         | 7.8            | 2.66                | ...        | ...                                          | J2125.0-4632                                           | 0.522                    | 1.041               | T                           | S                    |
| J2128.0+3623 | ...                        | 83.526              | -10.468             | 0.127                         | 6.1            | 1.98                | ...        | J2127.8+3614                                 | ...                                                    | 0.161                    | 0.703               | T                           | C                    |
| J2133.4+2532 | ...                        | 76.433              | -18.962             | 0.135                         | 4.8            | 2.21                | ...        | ...                                          | J2132.5+2605                                           | 0.577                    | 1.976               | ...                         | NC                   |
| J2140.8-6743 | ...                        | 324.540             | -40.478             | 0.208                         | 6.9            | 3.06                | ...        | ...                                          | ...                                                    | ...                      | ...                 | ...                         | BC                   |
| J2147.0+3119 | ...                        | 82.899              | -16.858             | 0.151                         | 4.8            | 2.58                | ...        | ...                                          | ...                                                    | ...                      | ...                 | ...                         | NC                   |
| J2152.4-7532 | ...                        | 315.624             | -36.825             | 0.174                         | 6.2            | 2.74                | ...        | ...                                          | J2147.4-7534                                           | 0.310                    | 1.143               | ...                         | BC                   |
| J2158.7+6547 | ...                        | 106.446             | 8.614               | 0.155                         | 5.9            | 2.50                | ...        | ...                                          | ...                                                    | ...                      | ...                 | ...                         | BC                   |
| J2159.9-1234 | ...                        | 44.210              | -47.382             | 0.189                         | 4.1            | 2.38                | ...        | ...                                          | ...                                                    | ...                      | ...                 | ...                         | NC, Sun              |
| J2204.3-5017 | ...                        | 345.248             | -50.786             | 0.253                         | 4.8            | 2.94                | ...        | ...                                          | ...                                                    | ...                      | ...                 | ...                         | BC                   |
| J2207.5+6440 | ...                        | 106.507             | 7.164               | 0.197                         | 10.5           | 2.65                | ...        | J2206.6+6500                                 | ...                                                    | 0.342                    | 0.743               | T                           | C                    |
| J2208.6+3903 | ...                        | 91.521              | -13.692             | 0.082                         | 4.4            | 1.31                | ...        | ...                                          | ...                                                    | ...                      | ...                 | ...                         | NC                   |
| J2214.5+5949 | ...                        | 104.383             | 2.731               | 0.118                         | 5.8            | 2.42                | ...        | ...                                          | ...                                                    | ...                      | ...                 | T                           | C                    |
| J2227.4-7804 | ...                        | 311.625             | -36.511             | 0.113                         | 7.2            | 2.58                | ...        | ...                                          | ...                                                    | ...                      | ...                 | ...                         | BC                   |
| J2227.7-3036 | ...                        | 17.931              | -58.472             | 0.118                         | 4.5            | 2.05                | T          | ...                                          | ...                                                    | ...                      | ...                 | ...                         | NC                   |
| J2250.8+6336 | ...                        | 110.010             | 3.810               | 0.142                         | 6.7            | 2.53                | ...        | ...                                          | J2250.7+6305c                                          | 0.520                    | 1.897               | ...                         | BC                   |
| J2256.1+2414 | ...                        | 91.862              | -31.577             | 0.190                         | 6.3            | 2.22                | ...        | J2255.2+2408                                 | ...                                                    | 0.222                    | 0.668               | T                           | C                    |
| J2321.4+1738 | ...                        | 94.418              | -40.190             | 0.116                         | 4.2            | 1.86                | ...        | ...                                          | ...                                                    | ...                      | ...                 | ...                         | NC                   |
| J2322.3-0153 | PKS 2320-021               | 78.951              | -56.952             | 0.186                         | 5.9            | 2.27                | ...        | ...                                          | ...                                                    | ...                      | ...                 | T                           | C                    |
| J2325.8-4043 | ...                        | 349.829             | -67.745             | 0.183                         | 15.1           | 2.31                | T          | J2324.7-4042                                 | ...                                                    | 0.208                    | 0.711               | T                           | S                    |
| J2328.6+1209 | ...                        | 93.184              | -45.882             | 0.207                         | 4.1            | 2.16                | ...        | ...                                          | ...                                                    | ...                      | ...                 | ...                         | NC                   |

Table 1—Continued

| 1FGL         | 1FGL Assoc. <sup>(a)</sup> | $l^{(a)}$<br>(deg.) | $b^{(a)}$<br>(deg.) | $\theta_{95}^{(a)}$<br>(deg.) | $\sigma^{(a)}$ | $\Gamma_{25}^{(a)}$ | $\text{Var}^{(a)}$ | 2FGL <sup>(b)</sup>   | 2FGL <sup>(c)</sup>             | $\Delta^{(d)}$ | $\Delta / d_{99.9}$ | 2FGL <sup>(e)</sup> Flags <sup>(f)</sup> |
|--------------|----------------------------|---------------------|---------------------|-------------------------------|----------------|---------------------|--------------------|-----------------------|---------------------------------|----------------|---------------------|------------------------------------------|
|              |                            |                     |                     |                               |                |                     | $p > 90\%$         | $(\Delta < d_{99.9})$ | $(d_{99.9} < \Delta < 1^\circ)$ | (deg.)         |                     | Seed                                     |
| J2334.2+4319 | ...                        | 108.343             | -17.355             | 0.117                         | 4.1            | 1.98                | ...                | ...                   | ...                             | ...            | ...                 | NC                                       |

<sup>(a)</sup>All the values reported in these columns are from the 1FGL catalog (Abdo et al. 2010g).

<sup>(b)</sup>Name of the 2FGL source associated with the 1FGL one using  $d_{99.9}$ .

<sup>(c)</sup>In this column is reported the name of the closest 2FGL source. Only 2FGL sources within a region having a radius of  $1^\circ$  centered on the 1FGL source position are reported in the table. Also, the name of the nearest 2FGL source is reported only if there is no 2FGL seed associated with the 1FGL sources or if the 1FGL source and one or more seeds have overlapping  $\theta_{99.9}$  error regions.

<sup>(d)</sup>In this column is reported the angular separation ( $\Delta$ ) between the 1FGL source and the 2FGL sources associated using  $d_{99.9}$  or the closest 2FGL source.

<sup>(e)</sup>T = The 1FGL source and one of the 2FGL list of initial seeds have an angular separation  $< d_{99.9}$ .

<sup>(f)</sup>C= Confirmed 1FGL sources. LMC, Orion, Carina and Ophiuchus indicate that the source is in a region of the sky with high diffuse emission and high density of close sources; NC = not confirmed 1FGL sources (see text); BC = 1FGL sources confirmed by the 11-m binned likelihood analysis; S = the 1FGL source was split/resolved in one or more seeds; O = overlapping  $\theta_{99.9}$  error regions with one or more seeds; V = variable source visible only in the first 11 months; Sun = the source was detected when the Sun was at an angular distance  $< 1^\circ$  and the light curve show just a flare in the time bin relative to the passage of the Sun close to the position of the source.

## REFERENCES

Abdo, A. A. 2010, ApJS, 188, 405
